# Supplementary material for: The Ultraviolet Behavior of N=8 Supergravity at Four Loops
Source: arXiv:0905.2326 ancillary file (2012-01-08)
Supplement: Supplementary file 1 [file GuideToNeq8Files.pdf]

## Guide to $N = 8$ four-loop four-point files

Directory layout:

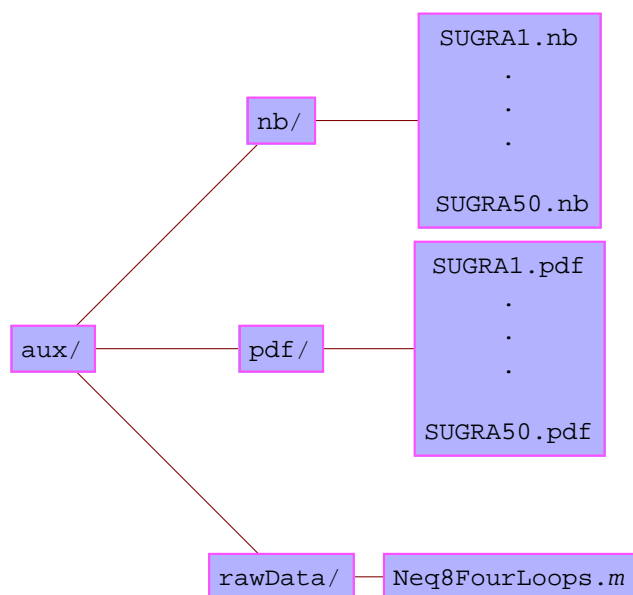

In addition to the raw data of our numerator factors, we provide a file per integral, in both mathematica notebook (nb), and portable document format (pdf), describing the graph associated with the integral, and its numerator factor. Due the size of the numerator factors, we chose to supply them as individual files, to be opened one at a time.

The `./nb/` and `./pdf/` directories contain 2D and 3D plots of the 50 graphs associated with the 50 contributing integrals ( $\mathcal{I}_1 \dots \mathcal{I}_{50}$ ), as well as typeset numerator factors broken out by scaling properties in loop momenta. To view and interact with the `./nb/` files one must use the free *Mathematica* player (Version 7 and above) available through a minimal<sup>(†)</sup> registration process from wolfram.com:

<http://www.wolfram.com/products/player/download.cgi>

(†) As of April 2009, the only required fields for the download of *Mathematica* Player are "Affiliation (faculty/student/etc).", "Operating System", and a simple math question. More personal attributes like name, email address, etc. seem to be optional.

Why bother with these notebook files? They provide an interactive manipulation of the graphs, in contrast to the static presentation of the pdfs. i.e. Using the Math Player, one is able to rotate and zoom in and out of the 3D graphs, as well as dynamically shift the nodes in the 2D plots. This can prove valuable if the initial visual presentation of a graph obscures the topology or propagator labels.

The `rawData` directory contains the single file: `Neq8FourLoops.m` which represents the raw data of our results as a Mathematica package. This is presented in a simple enough format that hopefully is not too difficult for interested parties to manipulate into the format of their choice.

The remainder of this document describes the functions defined in `Neq8FourLoops.m`, and offers some small sample calculations using them.

---

## Raw Data package: Neq8FourLoops.m

First we load the package:

```
Get[PATH <> "rawData/Neq8FourLoops.m"]
```

where PATH is a string containing the directory path where the rawData directory has been placed.

This defines objects (functions) **grav1** .... **grav50**, representing each of the 50 integrals. We provide a list of these objects in the symbol: **gravObjects**:

```
gravObjects
```

```
{grav1, grav2, grav3, grav4, grav5, grav6, grav7, grav8, grav9, grav10,
  grav11, grav12, grav13, grav14, grav15, grav16, grav17, grav18, grav19, grav20,
  grav21, grav22, grav23, grav24, grav25, grav26, grav27, grav28, grav29, grav30,
  grav31, grav32, grav33, grav34, grav35, grav36, grav37, grav38, grav39, grav40,
  grav41, grav42, grav43, grav44, grav45, grav46, grav47, grav48, grav49, grav50}
```

Each object takes the following five accessors (arguments):

```
"getNumerator", "getNumeratorList", "getEdgeGraphForm", "getVertexGraphForm", "getSymmetryFactor."
```

Let's look at each of these in turn.

### ■ "getNumerator"

```
grav12["getNumerator"]
```

$$2 \text{lsq}[\{l[8]\}] \text{lsq}[\{l[9]\}] \text{lsq}[\{l[14]\}] \text{lsq}[\{l[16]\}] \\ (13 \tau[k[1], k[2]]^2 - 7 \tau[k[1], k[3]]^2 + 2 \tau[k[1], k[4]]^2) + \\ \frac{1}{2} \tau[k[1], k[2]]^4 (\tau[l[5], l[6]]^2 + \tau[l[10], l[17]]^2)$$

This function returns the complete numerator factor of the integrand with the momenta labeling and conservation as described by the "getVertexGraphForm" (see below).

$l$  is reserved for inner (loop) momenta.  $l[8] \equiv l_8$

$k$  is reserved for external momenta.  $k[4] \equiv k_4$ .

Observe, in the numerator factor above, the use of two functions **lsq**[ $\{a\}$ ], and **tau**[ $a_-, b_-$ ]. These are defined as follows,

**lsq**[ $\{a_-\}$ ] := the D-dimensional Lorentz square of  $a$ :  $a \cdot a$

**tau**[ $a_-, b_-$ ] := twice the Lorentz product of  $a$  and  $b$ :  $2(a \cdot b)$

*Note : propagators for certain graphs were relabeled in the manuscript due to size constraints on the image. The labels in the file Neq8FourLoops.m should be used for verification purposes.*

### ■ "getNumeratorList"

```
grav12["getNumeratorList"]
```

$$\left\{ 0, 0, 0, 0, \frac{1}{2} \tau[k[1], k[2]]^4 (\tau[l[5], l[6]]^2 + \tau[l[10], l[17]]^2), \right. \\ \left. 0, 0, 0, 2 \text{lsq}[\{l[8]\}] \text{lsq}[\{l[9]\}] \text{lsq}[\{l[14]\}] \text{lsq}[\{l[16]\}] \right. \\ \left. (13 \tau[k[1], k[2]]^2 - 7 \tau[k[1], k[3]]^2 + 2 \tau[k[1], k[4]]^2) \right\}$$

This function returns the numerator expression split into a list. The first element of the list is associated with terms manifestly independent of  $l$  scaling as  $l^0$ , the second manifestly scaling as  $l^1$ , through the ninth element which is that part of the numerator which scales as  $l^8$ . This function is provided mostly as a book-keeping convenience, and, of course, is not robust under relabeling through conservation of momenta.

One reproduces "getNumerator" by simply summing over "getNumeratorList"

```
Plus @@ grav50["getNumeratorList"] === grav50["getNumerator"]
```

```
True
```

### ■ "getEdgeGraphForm"

```
grav1["getEdgeGraphForm"]
```

```
{{10 -> 1, k[1]}, {9 -> 2, k[2]}, {5 -> 3, k[4]}, {6 -> 4, k[3]}, {5 -> 6, l[17]}, {5 -> 13, l[16]},  
{6 -> 14, l[14]}, {7 -> 8, l[8]}, {12 -> 7, l[12]}, {14 -> 7, l[11]}, {8 -> 9, l[7]}, {11 -> 8, l[9]},  
{9 -> 10, l[5]}, {11 -> 10, l[6]}, {12 -> 11, l[10]}, {13 -> 12, l[13]}, {13 -> 14, l[15]}}
```

This function returns the graph associated with the integral object in an edge - focused description,  $\text{edge} \equiv \{\text{node} \rightarrow \text{node}, \text{labeled by momenta}\}$  in the following form :

```
{ {nodeA -> nodeB, momentaLabel}, {node_ -> node_, label_}, ...}.
```

To reconstruct a given (four-loop) graph by hand from the EdgeGraphForm :

- Draw 14 nodes and label them 1 through 14.
- Draw the edges by connecting the nodes with arrows as described according to the output of this function.
- Label the arrows as specified in the output.

(it is perhaps worth noting, that for all of our EdgeGraphForms, node-labels 1, 2, 3, 4 are reserved for external nodes.

To have Mathematica plot, for Version 6 and above :

```
GraphPlot[grav1["getEdgeGraphForm"], DirectedEdges -> True]
```

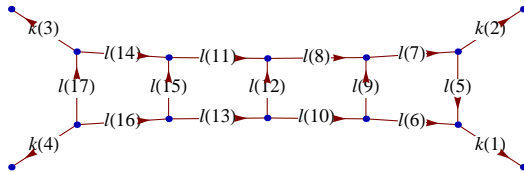

```

GraphPlot3D[grav42["getEdgeGraphForm"],
  EdgeRenderingFunction -> ({Cylinder[#1, 0.02], Specularity[White, 10],
    If[#3 != None, Style[Text[#3, (#1[[1]] + #1[[2]]) / 2,
      Background -> White], FontSize -> 9], {}]} &), ImageSize -> Large]

```

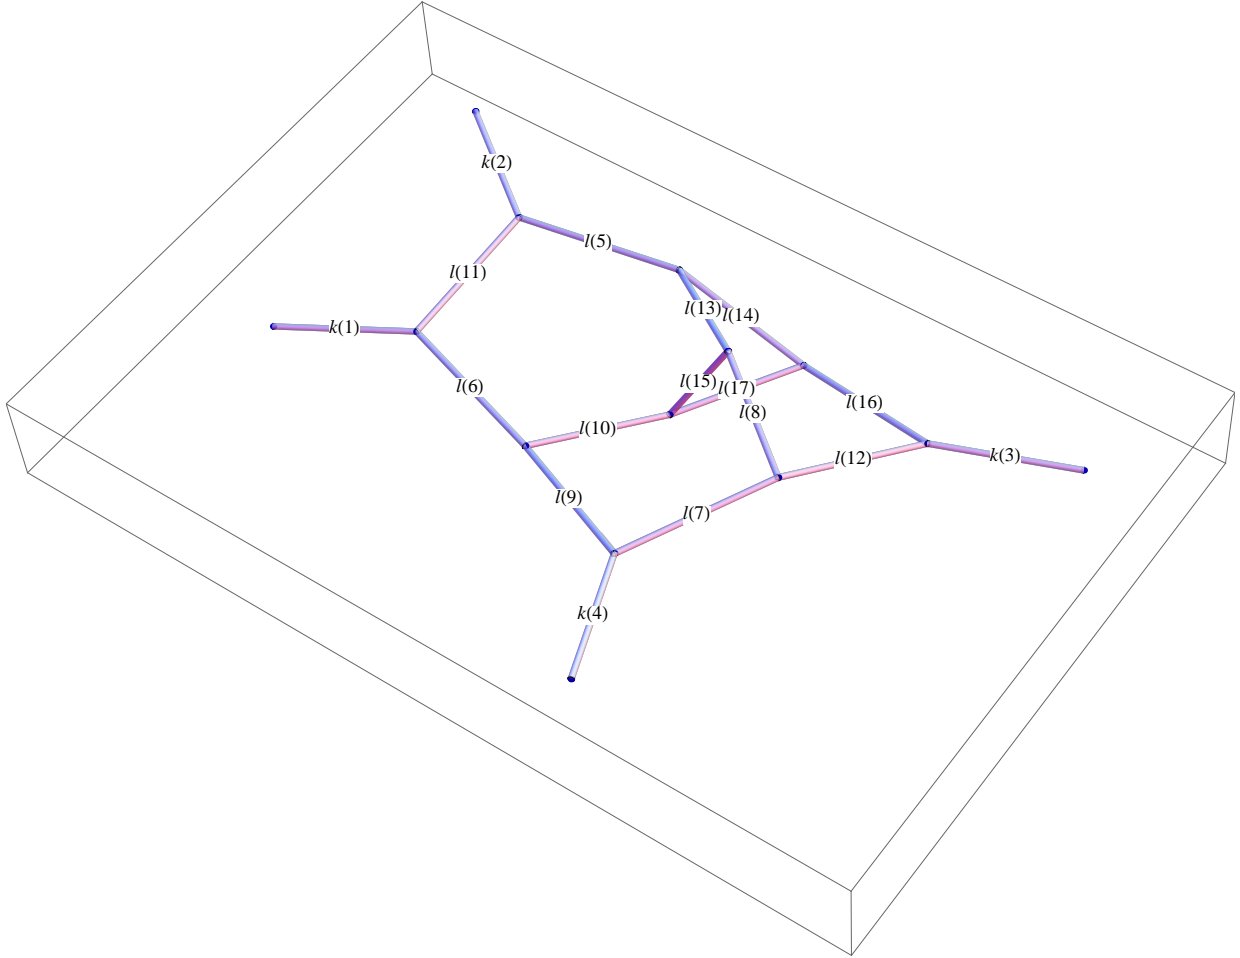

#### ■ "getVertexGraphForm"

```
grav1["getVertexGraphForm"]
```

```

{gVertex[{k[1], -l[5], -l[6]}], gVertex[{k[2], -l[7], l[5]}], gVertex[{k[3], -l[17], l[14]}],
  gVertex[{k[4], l[16], l[17]}], gVertex[{l[6], l[9], -l[10]}], gVertex[{l[7], -l[8], -l[9]}],
  gVertex[{l[8], -l[11], -l[12]}], gVertex[{l[10], l[12], -l[13]}],
  gVertex[{l[11], -l[14], -l[15]}], gVertex[{l[13], l[15], -l[16]}]}

```

This function returns the graph associated with the integral object in a vertex representation. This can be used as a way of specifying the topology of a graph using trivalent (cubic) vertices,  $\text{gVertex}[p_a, p_b, p_c]$ , where  $\{p_a, p_b, p_c\}$  are momenta labeling the propagators (edges) of the graph, and is understood that the edge labelled by  $p_a$  flows into the edge labelled by  $-p_a$ . Additionally, each vertex represents the manifest conservation of ( $D$  - dimensional) momenta :

$$\text{gVertex}[\{p_1, p_2, p_3\}] \iff (p_1 + p_2 + p_3 = 0)$$

As an example, let us use these identities to find a minimum spanning basis of momenta for graph50:

```

Reduce[grav50["getVertexGraphForm"] /. gVertex[a__] -> (Plus @@ a == 0)]

1[14] == -1[15] + 1[16] && 1[13] == -1[16] + 1[17] && 1[11] == -1[12] + 1[15] &&
1[9] == -1[10] - 1[17] && 1[7] == -1[8] - 1[15] + 1[16] && 1[5] == -1[6] - 1[16] + 1[17] &&
k[4] == 1[10] - 1[12] + 1[15] && k[3] == 1[8] - 1[10] - 1[17] &&
k[2] == 1[6] - 1[8] - 1[15] + 1[16] && k[1] == -1[6] + 1[12] - 1[16] + 1[17]

```

This is fine, but let us say we want to use  $k[1]$ ,  $k[2]$ ,  $k[3]$  as part of our independent basis.

```

Reduce[%,
  Complement[grav50["getVertexGraphForm"] /. gVertex[a__] -> {a} /. -a_ -> a // Flatten // Union,
    {k[1], k[2], k[3]}]]

k[4] == -k[1] - k[2] - k[3] && 1[7] == k[2] - 1[6] && 1[9] == k[3] - 1[8] &&
1[11] == -k[1] - k[2] - k[3] - 1[10] && 1[12] == k[1] - 1[5] && 1[13] == 1[5] + 1[6] &&
1[14] == k[2] - 1[6] + 1[8] && 1[15] == -k[2] - k[3] - 1[5] - 1[10] &&
1[16] == -k[3] - 1[5] - 1[6] + 1[8] - 1[10] && 1[17] == -k[3] + 1[8] - 1[10]

```

We may turn the above into rules for future use.

```

basis50 = Rule @@ # & /@ List @@ %

{k[4] -> -k[1] - k[2] - k[3], 1[7] -> k[2] - 1[6], 1[9] -> k[3] - 1[8],
  1[11] -> -k[1] - k[2] - k[3] - 1[10], 1[12] -> k[1] - 1[5], 1[13] -> 1[5] + 1[6],
  1[14] -> k[2] - 1[6] + 1[8], 1[15] -> -k[2] - k[3] - 1[5] - 1[10],
  1[16] -> -k[3] - 1[5] - 1[6] + 1[8] - 1[10], 1[17] -> -k[3] + 1[8] - 1[10]}

```

Note that only 4 internal loop momenta ( $l[i]$ ) appear on the RHS of the above equations, and only 3 external momenta ( $k[i]$ ), as it should be for four-point four-loop graphs:

```

Union[Flatten[{{# [2]} /. Plus -> List /. -a_ -> a} & /@ basis50]]

{k[1], k[2], k[3], 1[5], 1[6], 1[8], 1[10]}

```

#### ■ "getSymmetryFactor"

```

grav1["getSymmetryFactor"]

1
—
4

```

This function returns  $1/(\text{number of automorphisms of the graph associated with the integral})$ . This corresponds to the  $c_i$  in Equation (1) of the manuscript.

#### ■ "Stand-Alone" Accessors

For syntactic convenience we also provide standalone functions:

```

getNumerator[integralObject_],
getNumeratorList[integralObject_],
getEdgeGraphForm[integralObject_],
getVertexGraphForm[integralObject_],
getSymmetryFactor[integralObject_]

```

e.g.

```

getNumerator[grav1] == grav1["getNumerator"]

True

```

```

getNumeratorList[grav1] == grav1["getNumeratorList"]

True

getEdgeGraphForm[grav15] == grav15["getEdgeGraphForm"]

True

getVertexGraphForm[grav33] == grav33["getVertexGraphForm"]

True

getSymmetryFactor[grav34] == grav34["getSymmetryFactor"]

True

```

This allows constructs like:

```

Histogram[gsF = getSymmetryFactor /@ gravObjects,
  {Min[gsF]}, FrameLabel → {"Symmetry Factor", "Number of Integrals"},
  FrameTicks → {{Automatic, Automatic}, {Union[gsF], None}},
  ChartElementFunction → "FadingRectangle", ChartStyle → Green,
  Frame → True, PlotLabel → "Histogram of Symmetry Factors"]

```

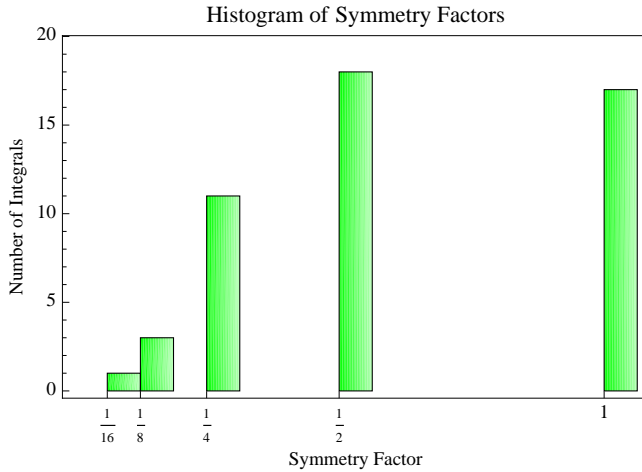


---

## Example calculations

Here we present some small sample calculations using the raw data around the  $l^8$  terms.

### ■ $l^8$ cancellations

This is a quick demonstration of how one can sketch out the  $l^8$  cancellations using the data in Neq8FourLoops.m. The actual computation proceeds similarly, here we only omit the details of the reduction down to vacuum diagram expressions.

First we collect everyone with  $l^8$  terms in their numerator:

```

nonVanishingL8 = Select[gravObjects, getNumeratorList[#][[9]] != 0 &]

{grav12, grav13, grav23, grav25, grav32, grav39, grav40, grav42, grav44, grav45, grav46, grav48}

```

As an aside, when using the Notebook interface, it's occasionally useful to define "Format"s to make certain things easier to parse visually, e.g.:

```
Map[(Format[ToExpression["grav" <> ToString[#]]] := I#) &, Range[50]];

nonVanishingL8

{I12, I13, I23, I25, I32, I39, I40, I42, I44, I45, I46, I48}
```

### ■ $V^{(d)}$ contributions

In the leading UV, the  $l^8$  terms dominate. Canceling inverse propagators in the  $l^8$  terms against propagators in the respective diagrams one finds that the first 6 members of our list **nonVanishingL8**,  $\{I_{12}, I_{13}, I_{23}, I_{25}, I_{32}, I_{39}\}$ , contribute only to the following vacuum diagram (d) (c.f. fig. 3 of the manuscript) with numerator factors that depend only on external momenta:

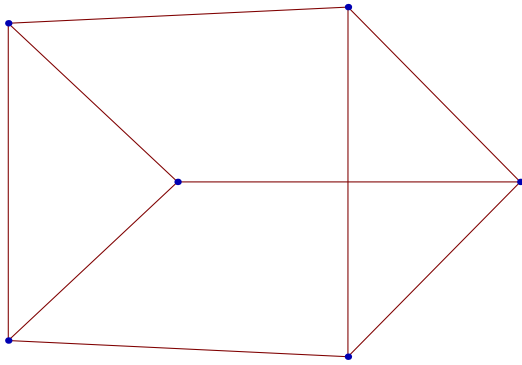

We will now proceed to establish the  $l^8$  cancellations. First we need to set up some tools. By default, in our rawData package, tau has very little defined:

```
Definition[tau]

Attributes[tau] = {Orderless}

tau[13 c - 25 d, a + b]

tau[a + b, 13 c - 25 d]
```

It will be useful to add some intelligence to our tau function, linearizing it, as we'll be applying conservation of momenta identities directly to labels a little later:

```
tau[-(a_), b_] := -tau[a, b]

tau[a_, (b_) + (c_)] := tau[a, b] + tau[a, c]

tau[c_, (b_) * (a_) ? NumberQ] := a * tau[b, c]
```

Now, e.g.

```
tau[13 c - 25 d, a + b]

13 tau[a, c] - 25 tau[a, d] + 13 tau[b, c] - 25 tau[b, d]
```

We will need to permute over the external leg labels, so we establish the following rule set:

```
(S4 = Map[Thread[Rule[k /@ Range[4], #]] &,
  Permutations[k /@ Range[4]]] // Style[#, Small] &

{{k[1] → k[1], k[2] → k[2], k[3] → k[3], k[4] → k[4]}, {k[1] → k[1], k[2] → k[2], k[3] → k[4], k[4] → k[3]},
{k[1] → k[1], k[2] → k[3], k[3] → k[2], k[4] → k[4]}, {k[1] → k[1], k[2] → k[3], k[3] → k[4], k[4] → k[2]},
{k[1] → k[1], k[2] → k[4], k[3] → k[2], k[4] → k[3]}, {k[1] → k[1], k[2] → k[4], k[3] → k[3], k[4] → k[2]},
{k[1] → k[2], k[2] → k[1], k[3] → k[3], k[4] → k[4]}, {k[1] → k[2], k[2] → k[1], k[3] → k[4], k[4] → k[3]},
{k[1] → k[2], k[2] → k[3], k[3] → k[1], k[4] → k[4]}, {k[1] → k[2], k[2] → k[3], k[3] → k[4], k[4] → k[1]},
{k[1] → k[2], k[2] → k[4], k[3] → k[1], k[4] → k[3]}, {k[1] → k[2], k[2] → k[4], k[3] → k[3], k[4] → k[1]},
{k[1] → k[3], k[2] → k[1], k[3] → k[2], k[4] → k[4]}, {k[1] → k[3], k[2] → k[1], k[3] → k[4], k[4] → k[2]},
{k[1] → k[3], k[2] → k[2], k[3] → k[1], k[4] → k[4]}, {k[1] → k[3], k[2] → k[2], k[3] → k[4], k[4] → k[1]},
{k[1] → k[3], k[2] → k[4], k[3] → k[1], k[4] → k[2]}, {k[1] → k[3], k[2] → k[4], k[3] → k[2], k[4] → k[1]},
{k[1] → k[4], k[2] → k[1], k[3] → k[2], k[4] → k[3]}, {k[1] → k[4], k[2] → k[1], k[3] → k[3], k[4] → k[2]},
{k[1] → k[4], k[2] → k[2], k[3] → k[1], k[4] → k[3]}, {k[1] → k[4], k[2] → k[2], k[3] → k[3], k[4] → k[1]},
{k[1] → k[4], k[2] → k[3], k[3] → k[1], k[4] → k[2]}, {k[1] → k[4], k[2] → k[3], k[3] → k[2], k[4] → k[1]}}
```

We will also need to invoke conservation of momentum identities for our external momenta.

```
conservationOfExternalMasslessMomentaRules = {k[4] → -k[3] - k[2] - k[1],
  tau[k[2], k[4]] → tau[k[1], k[3]],
  tau[k[2], k[3]] → tau[k[1], k[4]],
  tau[k[3], k[4]] → tau[k[1], k[2]],
  tau[k[a_], k[a_]] → 0};
```

Now we are ready to compute.

The  $l^8$  contribution in the vacuum (d) integrals will be:

$$Dvac = \sum_{S_4} \sum_{i \in \{V^{(d)}\}} c_i N_i^{(8)},$$

where  $\{V^{(d)}\}$  is the set of diagrams contributing to the (d) vacuum integral:  $\{I_{12}, I_{13}, I_{23}, I_{25}, I_{32}, I_{39}\}$ ,  $c_i$  are the symmetry factors associated with the original integral  $I_i$ , and  $S_4$  is the set of all permutations of the external momenta. All  $\text{lsq}[l_i]$  cancel against doubled propagators in the leading UV limit  $k \ll l$ , so we explicitly remove them from the numerators by setting them to unity,

```
(DVac = Sum[Sum[getSymmetryFactor[obj] * getNumeratorList[obj][[9]] /. lsq[___] → 1,
  {obj, nonVanishingL8[Range[6]]}] /. permRule, {permRule, S4}] // FullSimplify)

12 (tau[k[1], k[2]]^2 + tau[k[1], k[3]]^2 + tau[k[1], k[4]]^2 + tau[k[2], k[3]]^2 +
  tau[k[1], k[4]] tau[k[2], k[4]] + tau[k[2], k[3]] tau[k[2], k[4]] + tau[k[2], k[4]]^2 +
  tau[k[1], k[2]] (tau[k[1], k[3]] + tau[k[1], k[4]] + tau[k[2], k[3]] + tau[k[2], k[4]]) +
  (tau[k[1], k[4]] + tau[k[2], k[3]] + tau[k[2], k[4]]) tau[k[3], k[4]] +
  tau[k[3], k[4]]^2 + tau[k[1], k[3]] (tau[k[1], k[4]] + tau[k[2], k[3]] + tau[k[3], k[4]]))
```

We now apply the conservation of momenta identities,

```
Expand[DVac //. conservationOfExternalMasslessMomentaRules] // Style[#, Red, Large] &
```

0

and find that all (d)-vacuum contributions vanish.

#### ■ (e)-vacuum ( $V^{(e)}$ ) contributions:

The rest of the  $l^8$  terms,  $\{I_{40}, I_{42}, I_{44}, I_{45}, I_{46}, I_{48}\}$ , contribute to the (e) vacuum diagram:



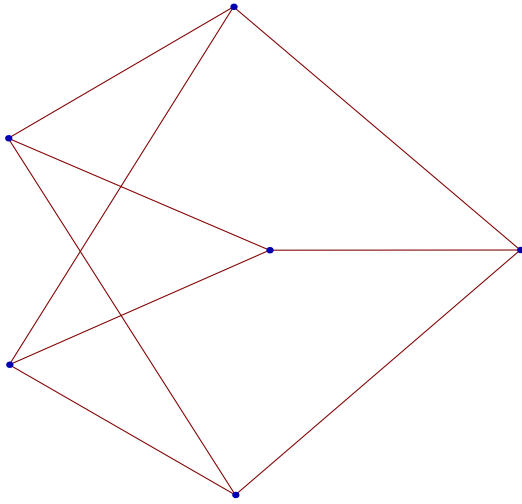

We proceed as before:

```
((Evac = Sum[Sum[getSymmetryFactor[obj] * getNumeratorList[obj][[9]] /. lsq[___] -> 1,
  {obj, nonVanishingL8[Range[7, 12]]}] /. permRule, {permRule, S4}]) /.
  conservationOfExternalMasslessMomentaRules) // Expand // Style[#, Red, Large] &
```

0

Thus we also find the  $l^8$  cancellation for  $V^{(e)}$  contributing terms. Having shown that all leading powers of  $l$  cancel, we find that there is no divergence in dimension  $D = \frac{9}{2}$ . In the manuscript we report additional cancellations of all  $l^7$ , and  $l^6$  contributions, pushing off the first dimension possibly presenting a divergence to  $D > 5$ . Additionally, as no  $l^5$  terms survive integration due to Lorentz invariance, we find that the dimension in which a potential divergence could appear is  $D \geq \frac{11}{2}$ . This is quite remarkable as  $D = \frac{11}{2}$  it is the lowest dimension where four-loop  $\mathcal{N}=4$  super-Yang-Mills amplitudes diverge. The  $\mathcal{N}=4$  super-Yang-Mills theory is intimately related to the  $\mathcal{N}=8$  supergravity theory classically, through the KLT relations, and one known to be UV finite to all loop orders.

---

## Earlier versions of *Mathematica*

To view the *Mathematica* notebooks associated with this paper, including this one, it is strongly recommended that one either use *Mathematica* Version 7 (or later), or the *Mathematica* Player Version 7 (or later) mentioned at the beginning of this document. Earlier versions may crash attempting to parse some of the newer graphical layouts.

The raw data package: `rawData/Neq8FourLoops.m`, documented above, should be compatible with all versions of *Mathematica* from version 1.0 onwards.

Certain functions used in the example calculations of this document, like `Histogram`, `GraphPlot`, etc, only became part of core *Mathematica* functionality in Version 6.0. One can consult the documentation for older versions of *Mathematica*, to see if similar functions were part of the supplemental Packages and Add-Ons. e.g. in earlier versions, there existed graph plotting functionality in `DiscreteMath`GraphPlot`` for a similar `GraphPlot` (with less features).

It should be noted that a particular construct used earlier in this document, `Sum[f[elem], {elem, arbitraryList__}]`, is a fairly recent addition to the functionality of `Sum[]`, and is not compatible with *Mathematica* v.5:

```

(* Only works in v .6 and above *)
(DVac = Sum[Sum[getSymmetryFactor[obj] * getNumeratorList[obj][[9]] /. lsq[___] :> 1,
  {obj, nonVanishingL8[Range[6]]}] /. permRule, {permRule, S4}] // FullSimplify)

12 (tau[k[1], k[2]]^2 + tau[k[1], k[3]]^2 + tau[k[1], k[4]]^2 + tau[k[2], k[3]]^2 +
  tau[k[1], k[4]] tau[k[2], k[4]] + tau[k[2], k[3]] tau[k[2], k[4]] + tau[k[2], k[4]]^2 +
  tau[k[1], k[2]] (tau[k[1], k[3]] + tau[k[1], k[4]] + tau[k[2], k[3]] + tau[k[2], k[4]]) +
  (tau[k[1], k[4]] + tau[k[2], k[3]] + tau[k[2], k[4]]) tau[k[3], k[4]] +
  tau[k[3], k[4]]^2 + tau[k[1], k[3]] (tau[k[1], k[4]] + tau[k[2], k[3]] + tau[k[3], k[4]]))

```

We chose to use it, as we find it a particularly readable construct, esp. for non-*Mathematica* programmers. The following represents the same functionality, expressed in a way that works for all versions of *Mathematica*:

```

(* Works for all versions of Mathematica *)
(DVac =
  (Plus @@ (Plus @@ (#["getNumeratorList"][[9]] * #["getSymmetryFactor"] /. lsq[___] :> 1 & /@
    nonVanishingL8[Range[6]])) /. S4 /. lsq[___] :> 1)) // FullSimplify)

12 (tau[k[1], k[2]]^2 + tau[k[1], k[3]]^2 + tau[k[1], k[4]]^2 + tau[k[2], k[3]]^2 +
  tau[k[1], k[4]] tau[k[2], k[4]] + tau[k[2], k[3]] tau[k[2], k[4]] + tau[k[2], k[4]]^2 +
  tau[k[1], k[2]] (tau[k[1], k[3]] + tau[k[1], k[4]] + tau[k[2], k[3]] + tau[k[2], k[4]]) +
  (tau[k[1], k[4]] + tau[k[2], k[3]] + tau[k[2], k[4]]) tau[k[3], k[4]] +
  tau[k[3], k[4]]^2 + tau[k[1], k[3]] (tau[k[1], k[4]] + tau[k[2], k[3]] + tau[k[3], k[4]]))

```
