# Supplementary material for: The Ultraviolet Behavior of N=8 Supergravity at Four Loops
Source: arXiv:0905.2326 ancillary file (2012-01-08)
Supplement: Supplementary file 8 [file SUGRA15.pdf]

## Integral 15: $\mathcal{I}_{15}$

$\mathcal{N} = 8$  four-point four-loop amplitude.

### ■ 2D plot of graph associated with $\mathcal{I}_{15}$

This fixes the labelling associated with the numerator expressions given below.

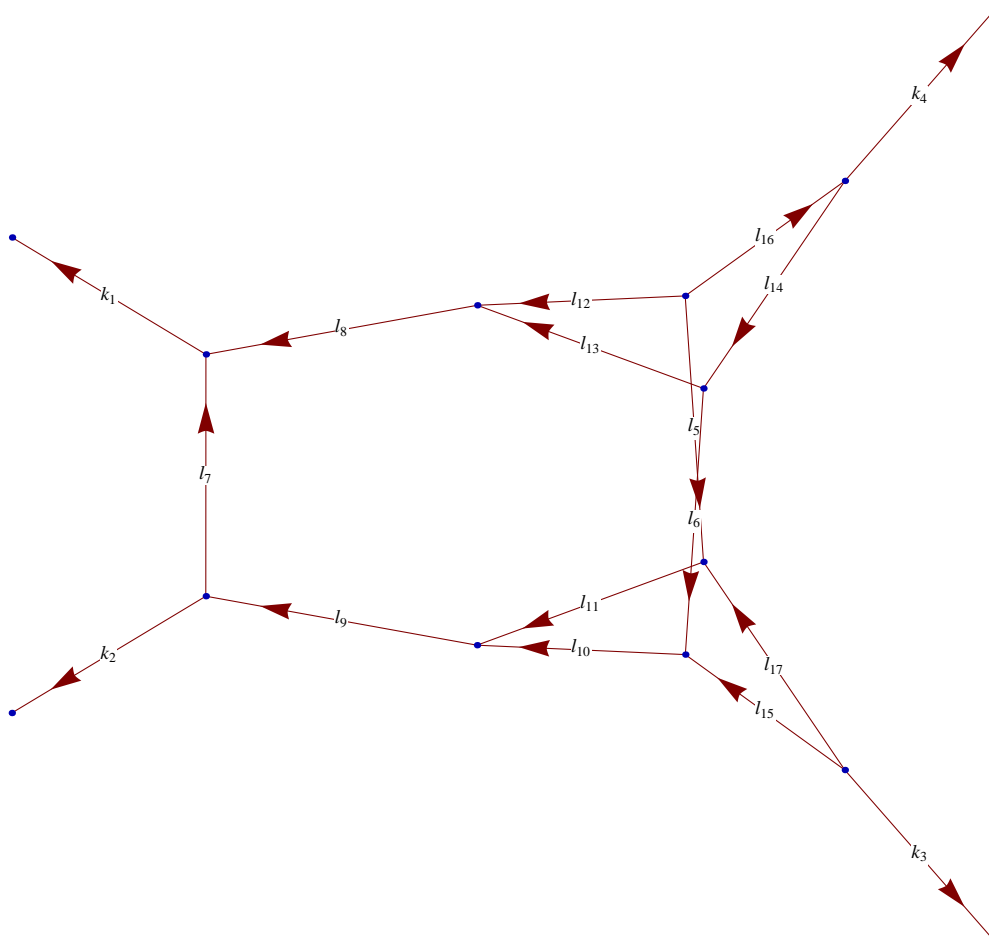

When using MathPlayer, by clicking three times (holding the click on the third click) directly on a vertex, one is able to move that vertex around, and its associated edges follow elastically. This functionality is absent when viewing as a pdf.

*Note: propagators for certain graphs were relabeled in the manuscript due to size constraints. The labels given in `aux/rawData/Neq8FourLoops.m` should be used for verification purposes.*

### ■ 3D plot of graph associated with $\mathcal{I}_{15}$

3D PLOT UNAVAILABLE FOR PDF. Please see .nb version for the 3D figure.

When using MathPlayer, by clicking anywhere in the image and dragging one should be able to rotate this 3D image. By holding (ALT) or (COMMAND) while clicking and moving the mouse up/down one should be able to zoom in/out. This functionality is absent when viewing as a pdf.

### ■ "Vertex Form" of graph associated with $\mathcal{I}_{15}$

This function returns the graph associated with the integral object in a vertex representation. This can be used as a way of specifying the topology of a graph using trivalent (cubic) vertices,  $\text{gVertex}[p_a, p_b, p_c]$ , where  $\{p_a, p_b, p_c\}$  are momenta labeling the propagators (edges) of the graph, and is understood that the edge labelled by  $p_a$  flows into the edge labelled by  $-p_a$ . Additionally, each vertex represents the manifest conservation of ( $D$  - dimensional) momenta :

$$\begin{aligned} \text{gVertex}[\{p_1, p_2, p_3\}] &\iff (p_1 + p_2 + p_3 = 0) \\ &\{\text{gVertex}(\{k_1, -l_7, -l_8\}), \text{gVertex}(\{k_2, -l_9, l_7\}), \text{gVertex}(\{k_3, l_{15}, l_{17}\}), \text{gVertex}(\{k_4, l_{14}, -l_{16}\}), \text{gVertex}(\{-l_5, l_{11}, -l_{17}\}), \\ &\quad \text{gVertex}(\{l_5, l_{16}, l_{12}\}), \text{gVertex}(\{-l_6, -l_{15}, l_{10}\}), \text{gVertex}(\{l_6, l_{13}, -l_{14}\}), \text{gVertex}(\{l_8, -l_{12}, -l_{13}\}), \text{gVertex}(\{l_9, -l_{10}, -l_{11}\})\} \end{aligned}$$

### ■ Numerator expression for integral 15:

The following notation is used:  $\tau_{i,j} \equiv \begin{cases} 2 k_i \cdot l_j & \text{if } i \leq 4, j > 4 \\ 2 l_i \cdot l_j & \text{if } i, j > 4 \end{cases}$ .

$$s \equiv 2 k_1 \cdot k_2 = 2 k_3 \cdot k_4$$

We use  $s, t, u$  to represent the traditional Mandelstam variables for massless external four-point momenta:  $t \equiv 2 k_1 \cdot k_4 = 2 k_2 \cdot k_3$ .

$$u \equiv 2 k_1 \cdot k_3 = 2 k_2 \cdot k_4$$

Furthermore we use the shorthand  $(l_i)^2$  to represent the lorentz square:  $(l_i)^2 = l_i \cdot l_i$ .

The total numerator  $\mathcal{N}_{15}$  is given by summing over the following terms, distinguished here by explicit dependence on loop momenta:  $\mathcal{N}_{15} = \sum_{i=0}^8 \mathcal{N}_{15}^{(i)}$ :

■  $\mathcal{N}_{15}^{(0)}$

$$0$$

■  $\mathcal{N}_{15}^{(1)}$

$$0$$

■  $\mathcal{N}_{15}^{(2)}$

$$-2 (l_8^2 + l_9^2) s^5$$

■  $N_{15}^{(3)}$

$$\frac{1}{2} s^2$$

$$\begin{aligned} & \left( l_9^2 (\tau_{1,15} (3 s^2 - t^2) + \tau_{1,17} (3 s^2 - t^2) - \tau_{2,5} (3 s^2 + t^2) - \tau_{2,6} (3 s^2 + t^2) - 3 s^2 \tau_{2,10} - 3 s^2 \tau_{2,11} - 4 s^2 \tau_{4,5} - 4 s^2 \tau_{4,6} - 6 s^2 \tau_{4,10} - \right. \\ & \quad \left. 6 s^2 \tau_{4,11} - 3 s^2 \tau_{4,15} - 3 s^2 \tau_{4,17} + 2 t^2 \tau_{4,5} + 2 t^2 \tau_{4,6} + t^2 \tau_{4,15} + t^2 \tau_{4,17} - 2 u^2 \tau_{4,5} - 2 u^2 \tau_{4,6}) + \right. \\ & \quad \left. \tau_{1,5} (l_9^2 (s^2 - t^2 - u^2) + l_8^2 (3 s^2 + t^2)) + \tau_{1,6} (l_9^2 (s^2 - t^2 - u^2) + l_8^2 (3 s^2 + t^2)) - 3 l_8^2 s^2 \tau_{1,12} - 3 l_8^2 s^2 \tau_{1,13} - \right. \\ & \quad \left. l_8^2 s^2 \tau_{2,5} - l_8^2 s^2 \tau_{2,6} + 3 l_8^2 s^2 \tau_{2,14} - 3 l_8^2 s^2 \tau_{2,16} + 4 l_8^2 s^2 \tau_{3,5} + 4 l_8^2 s^2 \tau_{3,6} - 6 l_8^2 s^2 \tau_{3,12} - \right. \\ & \quad \left. 6 l_8^2 s^2 \tau_{3,13} - 3 l_8^2 s^2 \tau_{3,14} + 3 l_8^2 s^2 \tau_{3,16} + l_8^2 t^2 \tau_{2,5} + l_8^2 t^2 \tau_{2,6} - l_8^2 t^2 \tau_{2,14} + l_8^2 t^2 \tau_{2,16} - \right. \\ & \quad \left. 2 l_8^2 t^2 \tau_{3,5} - 2 l_8^2 t^2 \tau_{3,6} + l_8^2 t^2 \tau_{3,14} - l_8^2 t^2 \tau_{3,16} + l_8^2 u^2 \tau_{2,5} + l_8^2 u^2 \tau_{2,6} + 2 l_8^2 u^2 \tau_{3,5} + 2 l_8^2 u^2 \tau_{3,6}) \right) \end{aligned}$$

■  $N_{15}^{(4)}$

$$\begin{aligned}
& \frac{1}{2} \left( s^2 \tau_{3,5}^4 + 4 s^2 \tau_{3,6} \tau_{3,5}^3 + 2 s^2 (3 \tau_{3,6}^2 + (t + 3u) l_8^2) \tau_{3,5}^2 - \right. \\
& 2 s \left( ((3 s^2 - t^2) \tau_{1,5} + (t^2 - 3 s^2) \tau_{1,13} + (t^2 - 3 s^2) \tau_{2,16} + 2 s (t + 3u) \tau_{3,13} + u (2 t + 3u) \tau_{3,16}) l_8^2 - 2 s \tau_{3,6}^3 \right) \tau_{3,5} + \\
& s^2 \tau_{3,6}^4 + t^2 \tau_{4,5}^4 + u^2 \tau_{4,5}^4 + (s^2 - t^2 - u^2) \tau_{4,5}^4 + t^2 \tau_{4,6}^4 + u^2 \tau_{4,6}^4 + (s^2 - t^2 - u^2) \tau_{4,6}^4 + 4 t^2 \tau_{4,5} \tau_{4,6}^3 + 4 u^2 \tau_{4,5} \tau_{4,6}^3 + \\
& 4 (s^2 - t^2 - u^2) \tau_{4,5} \tau_{4,6}^3 + 6 t^2 \tau_{4,5}^2 \tau_{4,6}^2 + 6 u^2 \tau_{4,5}^2 \tau_{4,6}^2 + 6 (s^2 - t^2 - u^2) \tau_{4,5}^2 \tau_{4,6}^2 + 4 t^2 \tau_{4,5}^3 \tau_{4,6} + 4 u^2 \tau_{4,5}^3 \tau_{4,6} + \\
& 4 (s^2 - t^2 - u^2) \tau_{4,5}^3 \tau_{4,6} + 2 t^3 \tau_{1,5}^2 l_8^2 + 2 u^3 \tau_{1,5}^2 l_8^2 - 3 t (-s^2 + t^2 + u^2) \tau_{1,5}^2 l_8^2 - 3 u (-s^2 + t^2 + u^2) \tau_{1,5}^2 l_8^2 + \\
& 2 t^3 \tau_{1,6}^2 l_8^2 + 2 u^3 \tau_{1,6}^2 l_8^2 - 3 t (-s^2 + t^2 + u^2) \tau_{1,6}^2 l_8^2 - 3 u (-s^2 + t^2 + u^2) \tau_{1,6}^2 l_8^2 + 2 t^3 \tau_{1,12}^2 l_8^2 + 2 u^3 \tau_{1,12}^2 l_8^2 - \\
& 3 t (-s^2 + t^2 + u^2) \tau_{1,12}^2 l_8^2 - 3 u (-s^2 + t^2 + u^2) \tau_{1,12}^2 l_8^2 + 2 t^3 \tau_{1,13}^2 l_8^2 + 2 u^3 \tau_{1,13}^2 l_8^2 - 3 t (-s^2 + t^2 + u^2) \tau_{1,13}^2 l_8^2 - \\
& 3 u (-s^2 + t^2 + u^2) \tau_{1,13}^2 l_8^2 + 2 t^3 \tau_{2,14}^2 l_8^2 + 2 u^3 \tau_{2,14}^2 l_8^2 - 3 t (-s^2 + t^2 + u^2) \tau_{2,14}^2 l_8^2 - 3 u (-s^2 + t^2 + u^2) \tau_{2,14}^2 l_8^2 + \\
& 2 t^3 \tau_{2,16}^2 l_8^2 + 2 u^3 \tau_{2,16}^2 l_8^2 - 3 t (-s^2 + t^2 + u^2) \tau_{2,16}^2 l_8^2 - 3 u (-s^2 + t^2 + u^2) \tau_{2,16}^2 l_8^2 + 2 s^2 (t + 3u) \tau_{3,6}^2 l_8^2 + \\
& 6 t^3 \tau_{3,12}^2 l_8^2 + 6 u^3 \tau_{3,12}^2 l_8^2 - 9 t (-s^2 + t^2 + u^2) \tau_{3,12}^2 l_8^2 - 9 u (-s^2 + t^2 + u^2) \tau_{3,12}^2 l_8^2 + 6 t^3 \tau_{3,13}^2 l_8^2 + \\
& 6 u^3 \tau_{3,13}^2 l_8^2 - 9 t (-s^2 + t^2 + u^2) \tau_{3,13}^2 l_8^2 - 9 u (-s^2 + t^2 + u^2) \tau_{3,13}^2 l_8^2 + 2 u^3 \tau_{3,14}^2 l_8^2 - 2 t (-s^2 + t^2 + u^2) \tau_{3,14}^2 l_8^2 - \\
& 3 u (-s^2 + t^2 + u^2) \tau_{3,14}^2 l_8^2 + 2 u^3 \tau_{3,16}^2 l_8^2 - 2 t (-s^2 + t^2 + u^2) \tau_{3,16}^2 l_8^2 - 3 u (-s^2 + t^2 + u^2) \tau_{3,16}^2 l_8^2 - \\
& 4 t^3 \tau_{1,6} \tau_{1,12} l_8^2 - 4 u^3 \tau_{1,6} \tau_{1,12} l_8^2 + 6 t (-s^2 + t^2 + u^2) \tau_{1,6} \tau_{1,12} l_8^2 + 6 u (-s^2 + t^2 + u^2) \tau_{1,6} \tau_{1,12} l_8^2 - 4 t^3 \tau_{1,5} \tau_{1,13} l_8^2 - \\
& 4 u^3 \tau_{1,5} \tau_{1,13} l_8^2 + 6 t (-s^2 + t^2 + u^2) \tau_{1,5} \tau_{1,13} l_8^2 + 6 u (-s^2 + t^2 + u^2) \tau_{1,5} \tau_{1,13} l_8^2 + 4 t^3 \tau_{1,6} \tau_{2,14} l_8^2 + \\
& 4 u^3 \tau_{1,6} \tau_{2,14} l_8^2 - 6 t (-s^2 + t^2 + u^2) \tau_{1,6} \tau_{2,14} l_8^2 - 6 u (-s^2 + t^2 + u^2) \tau_{1,6} \tau_{2,14} l_8^2 - 4 t^3 \tau_{1,12} \tau_{2,14} l_8^2 - \\
& 4 u^3 \tau_{1,12} \tau_{2,14} l_8^2 + 6 t (-s^2 + t^2 + u^2) \tau_{1,12} \tau_{2,14} l_8^2 + 6 u (-s^2 + t^2 + u^2) \tau_{1,12} \tau_{2,14} l_8^2 - 4 t^3 \tau_{1,5} \tau_{2,16} l_8^2 - \\
& 4 u^3 \tau_{1,5} \tau_{2,16} l_8^2 + 6 t (-s^2 + t^2 + u^2) \tau_{1,5} \tau_{2,16} l_8^2 + 6 u (-s^2 + t^2 + u^2) \tau_{1,5} \tau_{2,16} l_8^2 + 4 t^3 \tau_{1,13} \tau_{2,16} l_8^2 + \\
& 4 u^3 \tau_{1,13} \tau_{2,16} l_8^2 - 6 t (-s^2 + t^2 + u^2) \tau_{1,13} \tau_{2,16} l_8^2 - 6 u (-s^2 + t^2 + u^2) \tau_{1,13} \tau_{2,16} l_8^2 - 8 t^3 \tau_{1,6} \tau_{3,12} l_8^2 - \\
& 6 u^3 \tau_{1,6} \tau_{3,12} l_8^2 + 10 t (-s^2 + t^2 + u^2) \tau_{1,6} \tau_{3,12} l_8^2 + 9 u (-s^2 + t^2 + u^2) \tau_{1,6} \tau_{3,12} l_8^2 + 6 t^3 \tau_{1,12} \tau_{3,12} l_8^2 + \\
& 6 u^3 \tau_{1,12} \tau_{3,12} l_8^2 - 9 t (-s^2 + t^2 + u^2) \tau_{1,12} \tau_{3,12} l_8^2 - 9 u (-s^2 + t^2 + u^2) \tau_{1,12} \tau_{3,12} l_8^2 - 2 t (-s^2 + t^2 + u^2) \tau_{2,6} \tau_{3,12} l_8^2 - \\
& 2 u (-s^2 + t^2 + u^2) \tau_{2,6} \tau_{3,12} l_8^2 - 4 t^3 \tau_{2,14} \tau_{3,12} l_8^2 - 6 u^3 \tau_{2,14} \tau_{3,12} l_8^2 + 8 t (-s^2 + t^2 + u^2) \tau_{2,14} \tau_{3,12} l_8^2 + \\
& 9 u (-s^2 + t^2 + u^2) \tau_{2,14} \tau_{3,12} l_8^2 - 8 t^3 \tau_{1,5} \tau_{3,13} l_8^2 - 6 u^3 \tau_{1,5} \tau_{3,13} l_8^2 + 10 t (-s^2 + t^2 + u^2) \tau_{1,5} \tau_{3,13} l_8^2 + \\
& 9 u (-s^2 + t^2 + u^2) \tau_{1,5} \tau_{3,13} l_8^2 + 6 t^3 \tau_{1,13} \tau_{3,13} l_8^2 + 6 u^3 \tau_{1,13} \tau_{3,13} l_8^2 - 9 t (-s^2 + t^2 + u^2) \tau_{1,13} \tau_{3,13} l_8^2 - \\
& 9 u (-s^2 + t^2 + u^2) \tau_{1,13} \tau_{3,13} l_8^2 - 2 t (-s^2 + t^2 + u^2) \tau_{2,5} \tau_{3,13} l_8^2 - 2 u (-s^2 + t^2 + u^2) \tau_{2,5} \tau_{3,13} l_8^2 + 4 t^3 \tau_{2,16} \tau_{3,13} l_8^2 + \\
& 6 u^3 \tau_{2,16} \tau_{3,13} l_8^2 - 8 t (-s^2 + t^2 + u^2) \tau_{2,16} \tau_{3,13} l_8^2 - 9 u (-s^2 + t^2 + u^2) \tau_{2,16} \tau_{3,13} l_8^2 - 4 t^3 \tau_{1,6} \tau_{3,14} l_8^2 - \\
& 2 u^3 \tau_{1,6} \tau_{3,14} l_8^2 + 4 t (-s^2 + t^2 + u^2) \tau_{1,6} \tau_{3,14} l_8^2 + 3 u (-s^2 + t^2 + u^2) \tau_{1,6} \tau_{3,14} l_8^2 + 2 t^3 \tau_{1,12} \tau_{3,14} l_8^2 + \\
& 2 u^3 \tau_{1,12} \tau_{3,14} l_8^2 - 3 t (-s^2 + t^2 + u^2) \tau_{1,12} \tau_{3,14} l_8^2 - 3 u (-s^2 + t^2 + u^2) \tau_{1,12} \tau_{3,14} l_8^2 - 2 t (-s^2 + t^2 + u^2) \tau_{2,6} \tau_{3,14} l_8^2 - \\
& 2 u (-s^2 + t^2 + u^2) \tau_{2,6} \tau_{3,14} l_8^2 - 2 u^3 \tau_{2,14} \tau_{3,14} l_8^2 + 2 t (-s^2 + t^2 + u^2) \tau_{2,14} \tau_{3,14} l_8^2 + 3 u (-s^2 + t^2 + u^2) \tau_{2,14} \tau_{3,14} l_8^2 + \\
& 4 t^3 \tau_{3,12} \tau_{3,14} l_8^2 + 6 u^3 \tau_{3,12} \tau_{3,14} l_8^2 - 8 t (-s^2 + t^2 + u^2) \tau_{3,12} \tau_{3,14} l_8^2 - 9 u (-s^2 + t^2 + u^2) \tau_{3,12} \tau_{3,14} l_8^2 + \\
& 2 s \tau_{3,6} ((t^2 - 3 s^2) \tau_{1,6} + (3 s^2 - t^2) \tau_{1,12} + (t^2 - 3 s^2) \tau_{2,14} - 2 s (t + 3u) \tau_{3,12} + u (2 t + 3u) \tau_{3,14}) l_8^2 +
\end{aligned}$$

$$\begin{aligned}
& 4t^3 \tau_{1,5} \tau_{3,16} l_8^2 + 2u^3 \tau_{1,5} \tau_{3,16} l_8^2 - 4t(-s^2 + t^2 + u^2) \tau_{1,5} \tau_{3,16} l_8^2 - 3u(-s^2 + t^2 + u^2) \tau_{1,5} \tau_{3,16} l_8^2 - 2t^3 \tau_{1,13} \tau_{3,16} l_8^2 - \\
& 2u^3 \tau_{1,13} \tau_{3,16} l_8^2 + 3t(-s^2 + t^2 + u^2) \tau_{1,13} \tau_{3,16} l_8^2 + 3u(-s^2 + t^2 + u^2) \tau_{1,13} \tau_{3,16} l_8^2 + 2t(-s^2 + t^2 + u^2) \tau_{2,5} \tau_{3,16} l_8^2 + \\
& 2u(-s^2 + t^2 + u^2) \tau_{2,5} \tau_{3,16} l_8^2 - 2u^3 \tau_{2,16} \tau_{3,16} l_8^2 + 2t(-s^2 + t^2 + u^2) \tau_{2,16} \tau_{3,16} l_8^2 + 3u(-s^2 + t^2 + u^2) \tau_{2,16} \tau_{3,16} l_8^2 - \\
& 4t^3 \tau_{3,13} \tau_{3,16} l_8^2 - 6u^3 \tau_{3,13} \tau_{3,16} l_8^2 + 8t(-s^2 + t^2 + u^2) \tau_{3,13} \tau_{3,16} l_8^2 + 9u(-s^2 + t^2 + u^2) \tau_{3,13} \tau_{3,16} l_8^2 + \\
& (12l_8^2 t^4 + 2\tau_{2,10}^2 t^3 + 2\tau_{2,11}^2 t^3 + 2\tau_{4,5}^2 t^3 + 2\tau_{4,6}^2 t^3 + 6\tau_{4,10}^2 t^3 + 6\tau_{4,11}^2 t^3 + 4\tau_{2,10} \tau_{4,5} t^3 + 4\tau_{2,11} \tau_{4,6} t^3 + \\
& 6\tau_{2,10} \tau_{4,10} t^3 + 4\tau_{4,5} \tau_{4,10} t^3 + 6\tau_{2,11} \tau_{4,11} t^3 + 4\tau_{4,6} \tau_{4,11} t^3 + 2\tau_{2,11} \tau_{4,15} t^3 + 4\tau_{4,11} \tau_{4,15} t^3 + \\
& 2\tau_{2,10} \tau_{4,17} t^3 + 4\tau_{4,10} \tau_{4,17} t^3 - 20(-s^2 + t^2 + u^2) l_8^2 t^2 - 3(-s^2 + t^2 + u^2) \tau_{2,10}^2 t - 3(-s^2 + t^2 + u^2) \tau_{2,11}^2 t - \\
& 5(-s^2 + t^2 + u^2) \tau_{4,5}^2 t - 5(-s^2 + t^2 + u^2) \tau_{4,6}^2 t - 9(-s^2 + t^2 + u^2) \tau_{4,10}^2 t - 9(-s^2 + t^2 + u^2) \tau_{4,11}^2 t - \\
& 2(-s^2 + t^2 + u^2) \tau_{4,15}^2 t - 2(-s^2 + t^2 + u^2) \tau_{4,17}^2 t - 8(-s^2 + t^2 + u^2) \tau_{2,10} \tau_{4,5} t - 8(-s^2 + t^2 + u^2) \tau_{2,11} \tau_{4,6} t + \\
& 2(-s^2 + t^2 + u^2) \tau_{1,5} \tau_{4,10} t - 9(-s^2 + t^2 + u^2) \tau_{2,10} \tau_{4,10} t - 10(-s^2 + t^2 + u^2) \tau_{4,5} \tau_{4,10} t + 2(-s^2 + t^2 + u^2) \tau_{1,6} \tau_{4,11} \\
& t - 9(-s^2 + t^2 + u^2) \tau_{2,11} \tau_{4,11} t - 10(-s^2 + t^2 + u^2) \tau_{4,6} \tau_{4,11} t + 2(-s^2 + t^2 + u^2) \tau_{1,6} \tau_{4,15} t - 3(-s^2 + t^2 + u^2) \\
& \tau_{2,11} \tau_{4,15} t - 2(-s^2 + t^2 + u^2) \tau_{4,6} \tau_{4,15} t - 8(-s^2 + t^2 + u^2) \tau_{4,11} \tau_{4,15} t + 2(-s^2 + t^2 + u^2) \tau_{1,5} \tau_{4,17} t - \\
& 3(-s^2 + t^2 + u^2) \tau_{2,10} \tau_{4,17} t - 2(-s^2 + t^2 + u^2) \tau_{4,5} \tau_{4,17} t - 8(-s^2 + t^2 + u^2) \tau_{4,10} \tau_{4,17} t - 20u(-s^2 + t^2 + u^2) l_8^2 t - \\
& 2s^3 \tau_{1,15}^2 - 2s^3 \tau_{1,17}^2 - 2s^3 \tau_{2,5}^2 - 2s^3 \tau_{2,6}^2 + 2u^3 \tau_{2,10}^2 - 3u(-s^2 + t^2 + u^2) \tau_{2,10}^2 + 2u^3 \tau_{2,11}^2 - \\
& 3u(-s^2 + t^2 + u^2) \tau_{2,11}^2 + 6u^3 \tau_{4,5}^2 - 7u(-s^2 + t^2 + u^2) \tau_{4,5}^2 + 6u^3 \tau_{4,6}^2 - 7u(-s^2 + t^2 + u^2) \tau_{4,6}^2 + 6u^3 \tau_{4,10}^2 - \\
& 9u(-s^2 + t^2 + u^2) \tau_{4,10}^2 + 6u^3 \tau_{4,11}^2 - 9u(-s^2 + t^2 + u^2) \tau_{4,11}^2 + 2u^3 \tau_{4,15}^2 - 3u(-s^2 + t^2 + u^2) \tau_{4,15}^2 + \\
& 2u^3 \tau_{4,17}^2 - 3u(-s^2 + t^2 + u^2) \tau_{4,17}^2 + 6u^3 \tau_{2,10} \tau_{4,5} - 9u(-s^2 + t^2 + u^2) \tau_{2,10} \tau_{4,5} + 6u^3 \tau_{2,11} \tau_{4,6} - \\
& 9u(-s^2 + t^2 + u^2) \tau_{2,11} \tau_{4,6} + 2u(-s^2 + t^2 + u^2) \tau_{1,5} \tau_{4,10} + 6u^3 \tau_{2,10} \tau_{4,10} - 9u(-s^2 + t^2 + u^2) \tau_{2,10} \tau_{4,10} + \\
& 12u^3 \tau_{4,5} \tau_{4,10} - 14u(-s^2 + t^2 + u^2) \tau_{4,5} \tau_{4,10} + 2u(-s^2 + t^2 + u^2) \tau_{1,6} \tau_{4,11} + 6u^3 \tau_{2,11} \tau_{4,11} - \\
& 9u(-s^2 + t^2 + u^2) \tau_{2,11} \tau_{4,11} + 12u^3 \tau_{4,6} \tau_{4,11} - 14u(-s^2 + t^2 + u^2) \tau_{4,6} \tau_{4,11} + 2u(-s^2 + t^2 + u^2) \tau_{1,6} \tau_{4,15} + \\
& 2u^3 \tau_{2,11} \tau_{4,15} - 3u(-s^2 + t^2 + u^2) \tau_{2,11} \tau_{4,15} + 6u^3 \tau_{4,6} \tau_{4,15} - 5u(-s^2 + t^2 + u^2) \tau_{4,6} \tau_{4,15} + 6u^3 \tau_{4,11} \tau_{4,15} - \\
& 9u(-s^2 + t^2 + u^2) \tau_{4,11} \tau_{4,15} - 2s \tau_{2,6} (2\tau_{2,11} s^2 + (3s^2 - t^2) \tau_{4,6} + (3s^2 + t^2) \tau_{4,11} + (s^2 + t^2) \tau_{4,15}) + \\
& 2s \tau_{1,15} (2\tau_{2,6} s^2 + 2\tau_{2,11} s^2 + (3s^2 - t^2) (\tau_{4,6} + \tau_{4,11}) + u(2t + u) \tau_{4,15}) + 2u(-s^2 + t^2 + u^2) \tau_{1,5} \tau_{4,17} + \\
& 2u^3 \tau_{2,10} \tau_{4,17} - 3u(-s^2 + t^2 + u^2) \tau_{2,10} \tau_{4,17} + 6u^3 \tau_{4,5} \tau_{4,17} - 5u(-s^2 + t^2 + u^2) \tau_{4,5} \tau_{4,17} + 6u^3 \tau_{4,10} \tau_{4,17} - \\
& 9u(-s^2 + t^2 + u^2) \tau_{4,10} \tau_{4,17} - 2s \tau_{2,5} (2\tau_{2,10} s^2 + (3s^2 - t^2) \tau_{4,5} + (3s^2 + t^2) \tau_{4,10} + (s^2 + t^2) \tau_{4,17}) + \\
& 2s \tau_{1,17} (2\tau_{2,5} s^2 + 2\tau_{2,10} s^2 + (3s^2 - t^2) (\tau_{4,5} + \tau_{4,10}) + u(2t + u) \tau_{4,17}) - 8u^2(-s^2 + t^2 + u^2) l_8^2 l_9^2)
\end{aligned}$$

■  $N_{15}^{(5)}$

$$\begin{aligned}
& \frac{1}{4} (s^2 l_8^2 \tau_{1,5}^3 + s^2 (-3\tau_{1,13} - 3\tau_{2,16} + 4\tau_{3,5} - 4\tau_{3,13} + \tau_{3,16}) l_8^2 \tau_{1,5}^2 + \\
& (3\tau_{1,13}^2 l_8^2 s^2 + 2\tau_{1,13} (3\tau_{2,16} - 4\tau_{3,5} + 4\tau_{3,13} - \tau_{3,16}) l_8^2 s^2 + (3\tau_{2,16}^2 s^2 + 6\tau_{3,5}^2 s^2 - 2\tau_{2,16} (4\tau_{3,5} - 4\tau_{3,13} + \tau_{3,16}) s^2 + \\
& 2(3s^2 + t^2) \tau_{3,13}^2 + (s^2 + 2t^2) \tau_{3,16}^2 - 4(s^2 + t^2) \tau_{3,13} \tau_{3,16} + 4\tau_{3,5} ((t^2 - 3s^2) \tau_{3,13} + (s^2 - t^2) \tau_{3,16})) l_8^2 - \\
& 2(s^2 - t^2 - u^2) (\tau_{4,5}^2 - (\tau_{4,10} + \tau_{4,17})^2) l_9^2) \tau_{1,5} + s^2 \tau_{1,6}^3 l_8^2 - s^2 \tau_{1,12}^3 l_8^2 - s^2 \tau_{1,13}^3 l_8^2 + s^2 \tau_{2,14}^3 l_8^2 -
\end{aligned}$$

$$\begin{aligned}
& s^2 \tau_{2,16}^3 l_8^2 + 4 s^2 \tau_{3,5}^3 l_8^2 + 4 s^2 \tau_{3,6}^3 l_8^2 - 4 s^2 \tau_{3,12}^3 l_8^2 - 4 s^2 \tau_{3,13}^3 l_8^2 - s^2 \tau_{3,14}^3 l_8^2 + 2 t^2 \tau_{3,14}^3 l_8^2 + \\
& s^2 \tau_{3,16}^3 l_8^2 - 2 t^2 \tau_{3,16}^3 l_8^2 - 3 s^2 \tau_{1,12} \tau_{2,14}^2 l_8^2 - 3 s^2 \tau_{1,13} \tau_{2,16}^2 l_8^2 - 6 s^2 \tau_{1,13} \tau_{3,5}^2 l_8^2 - \\
& 2 t^2 \tau_{1,13} \tau_{3,5}^2 l_8^2 + 2 s^2 \tau_{2,5} \tau_{3,5}^2 l_8^2 - 2 t^2 \tau_{2,5} \tau_{3,5}^2 l_8^2 - 2 u^2 \tau_{2,5} \tau_{3,5}^2 l_8^2 - 6 s^2 \tau_{2,16} \tau_{3,5}^2 l_8^2 - \\
& 4 t^2 \tau_{2,16} \tau_{3,5}^2 l_8^2 - 6 s^2 \tau_{1,12} \tau_{3,6}^2 l_8^2 - 2 t^2 \tau_{1,12} \tau_{3,6}^2 l_8^2 + 2 s^2 \tau_{2,6} \tau_{3,6}^2 l_8^2 - 2 t^2 \tau_{2,6} \tau_{3,6}^2 l_8^2 - \\
& 2 u^2 \tau_{2,6} \tau_{3,6}^2 l_8^2 + 6 s^2 \tau_{2,14} \tau_{3,6}^2 l_8^2 + 4 t^2 \tau_{2,14} \tau_{3,6}^2 l_8^2 - 6 s^2 \tau_{1,12} \tau_{3,12}^2 l_8^2 - 2 s^2 \tau_{2,6} \tau_{3,12}^2 l_8^2 + \\
& 2 t^2 \tau_{2,6} \tau_{3,12}^2 l_8^2 + 2 u^2 \tau_{2,6} \tau_{3,12}^2 l_8^2 + 6 s^2 \tau_{2,14} \tau_{3,12}^2 l_8^2 - 2 t^2 \tau_{2,14} \tau_{3,12}^2 l_8^2 + 8 s^2 \tau_{3,6} \tau_{3,12}^2 l_8^2 - \\
& 4 t^2 \tau_{3,6} \tau_{3,12}^2 l_8^2 + 4 u^2 \tau_{3,6} \tau_{3,12}^2 l_8^2 - 6 s^2 \tau_{1,13} \tau_{3,13}^2 l_8^2 - 2 s^2 \tau_{2,5} \tau_{3,13}^2 l_8^2 + 2 t^2 \tau_{2,5} \tau_{3,13}^2 l_8^2 + \\
& 2 u^2 \tau_{2,5} \tau_{3,13}^2 l_8^2 - 6 s^2 \tau_{2,16} \tau_{3,13}^2 l_8^2 + 2 t^2 \tau_{2,16} \tau_{3,13}^2 l_8^2 + 8 s^2 \tau_{3,5} \tau_{3,13}^2 l_8^2 - 4 t^2 \tau_{3,5} \tau_{3,13}^2 l_8^2 + \\
& 4 u^2 \tau_{3,5} \tau_{3,13}^2 l_8^2 - s^2 \tau_{1,12} \tau_{3,14}^2 l_8^2 - 2 s^2 \tau_{2,6} \tau_{3,14}^2 l_8^2 + 2 t^2 \tau_{2,6} \tau_{3,14}^2 l_8^2 + 2 u^2 \tau_{2,6} \tau_{3,14}^2 l_8^2 + s^2 \tau_{2,14} \tau_{3,14}^2 l_8^2 - \\
& 2 t^2 \tau_{2,14} \tau_{3,14}^2 l_8^2 + 4 u^2 \tau_{3,6} \tau_{3,14}^2 l_8^2 - 4 s^2 \tau_{3,12} \tau_{3,14}^2 l_8^2 + 4 t^2 \tau_{3,12} \tau_{3,14}^2 l_8^2 - s^2 \tau_{1,13} \tau_{3,16}^2 l_8^2 - \\
& 2 s^2 \tau_{2,5} \tau_{3,16}^2 l_8^2 + 2 t^2 \tau_{2,5} \tau_{3,16}^2 l_8^2 + 2 u^2 \tau_{2,5} \tau_{3,16}^2 l_8^2 - s^2 \tau_{2,16} \tau_{3,16}^2 l_8^2 + 2 t^2 \tau_{2,16} \tau_{3,16}^2 l_8^2 + 4 u^2 \tau_{3,5} \tau_{3,16}^2 l_8^2 - \\
& 4 s^2 \tau_{3,13} \tau_{3,16}^2 l_8^2 + 4 t^2 \tau_{3,13} \tau_{3,16}^2 l_8^2 + 3 s^2 \tau_{1,12}^2 \tau_{2,14} l_8^2 - 3 s^2 \tau_{1,13}^2 \tau_{2,16} l_8^2 + 4 s^2 \tau_{1,13}^2 \tau_{3,5} l_8^2 + \\
& 4 s^2 \tau_{2,16}^2 \tau_{3,5} l_8^2 + 8 s^2 \tau_{1,13} \tau_{2,16} \tau_{3,5} l_8^2 + 4 s^2 \tau_{1,12}^2 \tau_{3,6} l_8^2 + 4 s^2 \tau_{2,14}^2 \tau_{3,6} l_8^2 - 8 s^2 \tau_{1,12} \tau_{2,14} \tau_{3,6} l_8^2 - \\
& 4 s^2 \tau_{1,12}^2 \tau_{3,12} l_8^2 - 4 s^2 \tau_{2,14}^2 \tau_{3,12} l_8^2 - 8 s^2 \tau_{3,6}^2 \tau_{3,12} l_8^2 + 4 t^2 \tau_{3,6}^2 \tau_{3,12} l_8^2 - 4 u^2 \tau_{3,6}^2 \tau_{3,12} l_8^2 + \\
& 8 s^2 \tau_{1,12} \tau_{2,14} \tau_{3,12} l_8^2 + 12 s^2 \tau_{1,12} \tau_{3,6} \tau_{3,12} l_8^2 - 4 t^2 \tau_{1,12} \tau_{3,6} \tau_{3,12} l_8^2 - 12 s^2 \tau_{2,14} \tau_{3,6} \tau_{3,12} l_8^2 + \\
& 4 t^2 \tau_{2,14} \tau_{3,6} \tau_{3,12} l_8^2 - 4 s^2 \tau_{1,13}^2 \tau_{3,13} l_8^2 - 4 s^2 \tau_{2,16}^2 \tau_{3,13} l_8^2 - 8 s^2 \tau_{3,5}^2 \tau_{3,13} l_8^2 + 4 t^2 \tau_{3,5}^2 \tau_{3,13} l_8^2 - \\
& 4 u^2 \tau_{3,5}^2 \tau_{3,13} l_8^2 - 8 s^2 \tau_{1,13} \tau_{2,16} \tau_{3,13} l_8^2 + 12 s^2 \tau_{1,13} \tau_{3,5} \tau_{3,13} l_8^2 - 4 t^2 \tau_{1,13} \tau_{3,5} \tau_{3,13} l_8^2 + 12 s^2 \tau_{2,16} \tau_{3,5} \tau_{3,13} l_8^2 - \\
& 4 t^2 \tau_{2,16} \tau_{3,5} \tau_{3,13} l_8^2 - s^2 \tau_{1,12}^2 \tau_{3,14} l_8^2 - s^2 \tau_{2,14}^2 \tau_{3,14} l_8^2 - 2 s^2 \tau_{3,6}^2 \tau_{3,14} l_8^2 + 4 t^2 \tau_{3,6}^2 \tau_{3,14} l_8^2 - \\
& 4 u^2 \tau_{3,6}^2 \tau_{3,14} l_8^2 - 6 s^2 \tau_{3,12}^2 \tau_{3,14} l_8^2 + 2 t^2 \tau_{3,12}^2 \tau_{3,14} l_8^2 + 2 s^2 \tau_{1,12} \tau_{2,14} \tau_{3,14} l_8^2 + 4 s^2 \tau_{1,12} \tau_{3,6} \tau_{3,14} l_8^2 - \\
& 4 t^2 \tau_{1,12} \tau_{3,6} \tau_{3,14} l_8^2 - 4 s^2 \tau_{2,14} \tau_{3,6} \tau_{3,14} l_8^2 + 4 t^2 \tau_{2,14} \tau_{3,6} \tau_{3,14} l_8^2 - 4 s^2 \tau_{1,12} \tau_{3,12} \tau_{3,14} l_8^2 - 4 s^2 \tau_{2,6} \tau_{3,12} \tau_{3,14} l_8^2 + \\
& 4 t^2 \tau_{2,6} \tau_{3,12} \tau_{3,14} l_8^2 + 4 u^2 \tau_{2,6} \tau_{3,12} \tau_{3,14} l_8^2 + 4 s^2 \tau_{2,14} \tau_{3,12} \tau_{3,14} l_8^2 - 4 t^2 \tau_{2,14} \tau_{3,12} \tau_{3,14} l_8^2 + 4 s^2 \tau_{3,6} \tau_{3,12} \tau_{3,14} l_8^2 - \\
& 4 t^2 \tau_{3,6} \tau_{3,12} \tau_{3,14} l_8^2 + 8 u^2 \tau_{3,6} \tau_{3,12} \tau_{3,14} l_8^2 - s^2 \tau_{1,6}^2 (3 \tau_{1,12} - 3 \tau_{2,14} - 4 \tau_{3,6} + 4 \tau_{3,12} + \tau_{3,14}) l_8^2 + \\
& s^2 \tau_{1,13}^2 \tau_{3,16} l_8^2 + s^2 \tau_{2,16}^2 \tau_{3,16} l_8^2 + 2 s^2 \tau_{3,5}^2 \tau_{3,16} l_8^2 - 4 t^2 \tau_{3,5}^2 \tau_{3,16} l_8^2 + 4 u^2 \tau_{3,5}^2 \tau_{3,16} l_8^2 + \\
& 6 s^2 \tau_{3,13}^2 \tau_{3,16} l_8^2 - 2 t^2 \tau_{3,13}^2 \tau_{3,16} l_8^2 + 2 s^2 \tau_{1,13} \tau_{2,16} \tau_{3,16} l_8^2 - 4 s^2 \tau_{1,13} \tau_{3,5} \tau_{3,16} l_8^2 + 4 t^2 \tau_{1,13} \tau_{3,5} \tau_{3,16} l_8^2 - \\
& 4 s^2 \tau_{2,16} \tau_{3,5} \tau_{3,16} l_8^2 + 4 t^2 \tau_{2,16} \tau_{3,5} \tau_{3,16} l_8^2 + 4 s^2 \tau_{1,13} \tau_{3,13} \tau_{3,16} l_8^2 + 4 s^2 \tau_{2,5} \tau_{3,13} \tau_{3,16} l_8^2 - 4 t^2 \tau_{2,5} \tau_{3,13} \tau_{3,16} l_8^2 - \\
& 4 u^2 \tau_{2,5} \tau_{3,13} \tau_{3,16} l_8^2 + 4 s^2 \tau_{2,16} \tau_{3,13} \tau_{3,16} l_8^2 - 4 t^2 \tau_{2,16} \tau_{3,13} \tau_{3,16} l_8^2 - 4 s^2 \tau_{3,5} \tau_{3,13} \tau_{3,16} l_8^2 + \\
& 4 t^2 \tau_{3,5} \tau_{3,13} \tau_{3,16} l_8^2 - 8 u^2 \tau_{3,5} \tau_{3,13} \tau_{3,16} l_8^2 + (s^2 \tau_{1,15}^3 - s^2 (3 \tau_{2,6} + 3 \tau_{2,11} + 4 (\tau_{4,6} + \tau_{4,11}) + \tau_{4,15}) \tau_{1,15}^2 + \\
& (-7 l_8^2 t^3 - 2 \tau_{4,15}^2 t^2 - 8 u l_8^2 t^2 + 7 s^2 l_8^2 t - 7 u^2 l_8^2 t + 3 s^2 \tau_{2,6}^2 + 3 s^2 \tau_{2,11}^2 + (6 s^2 + 4 t^2) \tau_{4,6}^2 + \\
& (6 s^2 - 2 t^2) \tau_{4,11}^2 + s^2 \tau_{4,15}^2 + 4 u (2 t + u) \tau_{4,11} \tau_{4,15} + 2 s^2 \tau_{2,11} (4 (\tau_{4,6} + \tau_{4,11}) + \tau_{4,15}) + \\
& 2 s^2 \tau_{2,6} (3 \tau_{2,11} + 4 (\tau_{4,6} + \tau_{4,11}) + \tau_{4,15}) + 4 \tau_{4,6} ((3 s^2 - t^2) \tau_{4,11} + u (2 t + u) \tau_{4,15}) - 8 u^3 l_8^2 + 8 s^2 u l_8^2) \tau_{1,15} + \\
& s^2 \tau_{1,17}^3 - s^2 \tau_{2,5}^3 - s^2 \tau_{2,6}^3 - s^2 \tau_{2,10}^3 - s^2 \tau_{2,11}^3 - 4 s^2 \tau_{4,5}^3 - 4 s^2 \tau_{4,6}^3 - 4 s^2 \tau_{4,10}^3 - 4 s^2 \tau_{4,11}^3 - \\
& s^2 \tau_{4,15}^3 + 2 t^2 \tau_{4,15}^3 - s^2 \tau_{4,17}^3 + 2 t^2 \tau_{4,17}^3 - 3 s^2 \tau_{2,5} \tau_{2,10}^2 - 3 s^2 \tau_{2,6} \tau_{2,11}^2 - 6 s^2 \tau_{2,5} \tau_{4,5}^2 - 6 s^2 \tau_{2,10} \tau_{4,5}^2 - \\
& 2 t^2 \tau_{2,10} \tau_{4,5}^2 - 6 s^2 \tau_{2,6} \tau_{4,6}^2 - 6 s^2 \tau_{2,11} \tau_{4,6}^2 - 2 t^2 \tau_{2,11} \tau_{4,6}^2 - 6 s^2 \tau_{2,5} \tau_{4,10}^2 - 2 t^2 \tau_{2,5} \tau_{4,10}^2 - 6 s^2 \tau_{2,10} \tau_{4,10}^2 - \\
& 8 s^2 \tau_{4,5} \tau_{4,10}^2 + 4 t^2 \tau_{4,5} \tau_{4,10}^2 - 4 u^2 \tau_{4,5} \tau_{4,10}^2 - 6 s^2 \tau_{2,6} \tau_{4,11}^2 - 2 t^2 \tau_{2,6} \tau_{4,11}^2 - 6 s^2 \tau_{2,11} \tau_{4,11}^2 -
\end{aligned}$$

$$\begin{aligned}
& 8s^2\tau_{4,6}\tau_{4,11}^2 + 4t^2\tau_{4,6}\tau_{4,11}^2 - 4u^2\tau_{4,6}\tau_{4,11}^2 - s^2\tau_{2,6}\tau_{4,15}^2 - 2t^2\tau_{2,6}\tau_{4,15}^2 - s^2\tau_{2,11}\tau_{4,15}^2 - 4u^2\tau_{4,6}\tau_{4,15}^2 - \\
& 4s^2\tau_{4,11}\tau_{4,15}^2 + 4t^2\tau_{4,11}\tau_{4,15}^2 - s^2\tau_{2,5}\tau_{4,17}^2 - 2t^2\tau_{2,5}\tau_{4,17}^2 - s^2\tau_{2,10}\tau_{4,17}^2 - 4u^2\tau_{4,5}\tau_{4,17}^2 - \\
& 4s^2\tau_{4,10}\tau_{4,17}^2 + 4t^2\tau_{4,10}\tau_{4,17}^2 - 3s^2\tau_{2,5}^2\tau_{2,10} - 3s^2\tau_{2,6}^2\tau_{2,11} - 4s^2\tau_{2,5}^2\tau_{4,5} - 4s^2\tau_{2,10}^2\tau_{4,5} - \\
& 8s^2\tau_{2,5}\tau_{2,10}\tau_{4,5} - 4s^2\tau_{2,6}^2\tau_{4,6} - 4s^2\tau_{2,11}^2\tau_{4,6} - 8s^2\tau_{2,6}\tau_{2,11}\tau_{4,6} - 4s^2\tau_{2,5}^2\tau_{4,10} - 4s^2\tau_{2,10}^2\tau_{4,10} - \\
& 8s^2\tau_{4,5}^2\tau_{4,10} + 4t^2\tau_{4,5}^2\tau_{4,10} - 4u^2\tau_{4,5}^2\tau_{4,10} - 8s^2\tau_{2,5}\tau_{2,10}\tau_{4,10} - 12s^2\tau_{2,5}\tau_{4,5}\tau_{4,10} + 4t^2\tau_{2,5}\tau_{4,5}\tau_{4,10} - \\
& 12s^2\tau_{2,10}\tau_{4,5}\tau_{4,10} + 4t^2\tau_{2,10}\tau_{4,5}\tau_{4,10} - 4s^2\tau_{2,6}^2\tau_{4,11} - 4s^2\tau_{2,11}^2\tau_{4,11} - 8s^2\tau_{4,6}^2\tau_{4,11} + 4t^2\tau_{4,6}^2\tau_{4,11} - \\
& 4u^2\tau_{4,6}^2\tau_{4,11} - 8s^2\tau_{2,6}\tau_{2,11}\tau_{4,11} - 12s^2\tau_{2,6}\tau_{4,6}\tau_{4,11} + 4t^2\tau_{2,6}\tau_{4,6}\tau_{4,11} - 12s^2\tau_{2,11}\tau_{4,6}\tau_{4,11} + \\
& 4t^2\tau_{2,11}\tau_{4,6}\tau_{4,11} - s^2\tau_{2,6}^2\tau_{4,15} - s^2\tau_{2,11}^2\tau_{4,15} - 2s^2\tau_{4,6}^2\tau_{4,15} + 4t^2\tau_{4,6}^2\tau_{4,15} - 4u^2\tau_{4,6}^2\tau_{4,15} - \\
& 6s^2\tau_{4,11}^2\tau_{4,15} + 2t^2\tau_{4,11}^2\tau_{4,15} - 2s^2\tau_{2,6}\tau_{2,11}\tau_{4,15} - 4u^2\tau_{2,6}\tau_{4,6}\tau_{4,15} - 8tu\tau_{2,6}\tau_{4,6}\tau_{4,15} - 4s^2\tau_{2,11}\tau_{4,6}\tau_{4,15} + \\
& 4t^2\tau_{2,11}\tau_{4,6}\tau_{4,15} - 4s^2\tau_{2,6}\tau_{4,11}\tau_{4,15} - 4t^2\tau_{2,6}\tau_{4,11}\tau_{4,15} - 4s^2\tau_{2,11}\tau_{4,11}\tau_{4,15} - 4s^2\tau_{4,6}\tau_{4,11}\tau_{4,15} + \\
& 4t^2\tau_{4,6}\tau_{4,11}\tau_{4,15} - 8u^2\tau_{4,6}\tau_{4,11}\tau_{4,15} - s^2\tau_{2,5}^2\tau_{4,17} - s^2\tau_{2,10}^2\tau_{4,17} - 2s^2\tau_{4,5}^2\tau_{4,17} + 4t^2\tau_{4,5}^2\tau_{4,17} - \\
& 4u^2\tau_{4,5}^2\tau_{4,17} - 6s^2\tau_{4,10}^2\tau_{4,17} + 2t^2\tau_{4,10}^2\tau_{4,17} - 2s^2\tau_{2,5}\tau_{2,10}\tau_{4,17} - 4u^2\tau_{2,5}\tau_{4,5}\tau_{4,17} - 8tu\tau_{2,5}\tau_{4,5}\tau_{4,17} - \\
& 4s^2\tau_{2,10}\tau_{4,5}\tau_{4,17} + 4t^2\tau_{2,10}\tau_{4,5}\tau_{4,17} - 4s^2\tau_{2,5}\tau_{4,10}\tau_{4,17} - 4t^2\tau_{2,5}\tau_{4,10}\tau_{4,17} - 4s^2\tau_{2,10}\tau_{4,10}\tau_{4,17} - \\
& 4s^2\tau_{4,5}\tau_{4,10}\tau_{4,17} + 4t^2\tau_{4,5}\tau_{4,10}\tau_{4,17} - 8u^2\tau_{4,5}\tau_{4,10}\tau_{4,17} - s^2\tau_{1,17}^2(3\tau_{2,5} + 3\tau_{2,10} + 4(\tau_{4,5} + \tau_{4,10}) + \tau_{4,17}) - \\
& (7\tau_{1,13}t^3 + 3\tau_{1,14}t^3 - 3\tau_{1,16}t^3 - 2\tau_{2,7}t^3 + 7\tau_{2,10}t^3 + 7\tau_{2,11}t^3 + 9\tau_{2,12}t^3 + 9\tau_{2,13}t^3 + 7\tau_{2,14}t^3 + 3\tau_{2,15}t^3 - \\
& 7\tau_{2,16}t^3 + 3\tau_{2,17}t^3 + 10\tau_{3,10}t^3 + 10\tau_{3,11}t^3 + 10\tau_{4,12}t^3 + 2u\tau_{1,13}t^2 + 2u\tau_{1,14}t^2 - 2u\tau_{1,16}t^2 + \\
& 6u\tau_{2,7}t^2 + 2u\tau_{2,10}t^2 + 2u\tau_{2,11}t^2 + 8u\tau_{2,12}t^2 + 8u\tau_{2,13}t^2 + 8u\tau_{2,14}t^2 + 2u\tau_{2,15}t^2 - 8u\tau_{2,16}t^2 + \\
& 2u\tau_{2,17}t^2 + 14u\tau_{3,7}t^2 + 10u\tau_{3,10}t^2 + 10u\tau_{3,11}t^2 - 14u\tau_{4,7}t^2 + 10u\tau_{4,12}t^2 - 3s^2\tau_{1,13}t + 3u^2\tau_{1,13}t - \\
& 3s^2\tau_{1,14}t + 3u^2\tau_{1,14}t + 3s^2\tau_{1,16}t - 3u^2\tau_{1,16}t - 2s^2\tau_{2,7}t + 2u^2\tau_{2,7}t - 3s^2\tau_{2,10}t + 3u^2\tau_{2,10}t - \\
& 3s^2\tau_{2,11}t + 3u^2\tau_{2,11}t - 9s^2\tau_{2,12}t + 9u^2\tau_{2,12}t - 9s^2\tau_{2,13}t + 9u^2\tau_{2,13}t - 7s^2\tau_{2,14}t + 7u^2\tau_{2,14}t - \\
& 3s^2\tau_{2,15}t + 3u^2\tau_{2,15}t + 7s^2\tau_{2,16}t - 7u^2\tau_{2,16}t - 3s^2\tau_{2,17}t + 3u^2\tau_{2,17}t - 28s^2\tau_{3,7}t + 28u^2\tau_{3,7}t - \\
& 10s^2\tau_{3,10}t + 10u^2\tau_{3,10}t - 10s^2\tau_{3,11}t + 10u^2\tau_{3,11}t + 28s^2\tau_{4,7}t - 28u^2\tau_{4,7}t - 10s^2\tau_{4,12}t + 10u^2\tau_{4,12}t + \\
& 2(t^3 - 3ut^2 - u^2t - 3u^3 + s^2(t + 3u))\tau_{1,7} + (9t + 8u)(-s^2 + t^2 + u^2)\tau_{1,10} + (9t + 8u)(-s^2 + t^2 + u^2)\tau_{1,11} + \\
& (7t^3 + 2ut^2 + 3u^2t + 2u^3 - s^2(3t + 2u))\tau_{1,12} + 2u^3\tau_{1,13} - 2s^2u\tau_{1,13} + 2u^3\tau_{1,14} - 2s^2u\tau_{1,14} - \\
& 2u^3\tau_{1,16} + 2s^2u\tau_{1,16} + 6u^3\tau_{2,7} - 6s^2u\tau_{2,7} + 2u^3\tau_{2,10} - 2s^2u\tau_{2,10} + 2u^3\tau_{2,11} - 2s^2u\tau_{2,11} + 8u^3\tau_{2,12} - \\
& 8s^2u\tau_{2,12} + 8u^3\tau_{2,13} - 8s^2u\tau_{2,13} + 8u^3\tau_{2,14} - 8s^2u\tau_{2,14} + 2u^3\tau_{2,15} - 2s^2u\tau_{2,15} - 8u^3\tau_{2,16} + \\
& 8s^2u\tau_{2,16} + 2u^3\tau_{2,17} - 2s^2u\tau_{2,17} + 14u^3\tau_{3,7} - 14s^2u\tau_{3,7} + 10u^3\tau_{3,10} - 10s^2u\tau_{3,10} + 10u^3\tau_{3,11} - \\
& 10s^2u\tau_{3,11} - 14u^3\tau_{4,7} + 14s^2u\tau_{4,7} + 10u^3\tau_{4,12} - 10s^2u\tau_{4,12} + 10(t + u)(-s^2 + t^2 + u^2)\tau_{4,13})l_8^2 + \\
& \tau_{1,17}(-7l_8^2t^3 - 2\tau_{4,17}^2t^2 - 8ul_8^2t^2 + 7s^2l_8^2t - 7u^2l_8^2t + 3s^2\tau_{2,5}^2 + 3s^2\tau_{2,10}^2 + (6s^2 + 4t^2)\tau_{4,5}^2 + \\
& (6s^2 - 2t^2)\tau_{4,10}^2 + s^2\tau_{4,17}^2 + 4u(2t + u)\tau_{4,10}\tau_{4,17} + 2s^2\tau_{2,10}(4(\tau_{4,5} + \tau_{4,10}) + \tau_{4,17}) + \\
& 2s^2\tau_{2,5}(3\tau_{2,10} + 4(\tau_{4,5} + \tau_{4,10}) + \tau_{4,17}) + 4\tau_{4,5}((3s^2 - t^2)\tau_{4,10} + u(2t + u)\tau_{4,17}) - 8u^3l_8^2 + 8s^2ul_8^2))l_9^2 + \\
& \tau_{1,6}(3\tau_{1,12}^2l_8^2s^2 + 2\tau_{1,12}(-3\tau_{2,14} - 4\tau_{3,6} + 4\tau_{3,12} + \tau_{3,14})l_8^2s^2 + \\
& (3\tau_{2,14}^2s^2 + 6\tau_{3,6}^2s^2 + 2\tau_{2,14}(4\tau_{3,6} - 4\tau_{3,12} - \tau_{3,14})s^2 + 2(3s^2 + t^2)\tau_{3,12}^2 + (s^2 + 2t^2)\tau_{3,14}^2 + \\
& 4(s^2 + t^2)\tau_{3,12}\tau_{3,14} + 4\tau_{3,6}((t^2 - 3s^2)\tau_{3,12} + (t^2 - s^2)\tau_{3,14}))l_8^2 - 2(s^2 - t^2 - u^2)(\tau_{4,6}^2 - (\tau_{4,11} + \tau_{4,15})^2)l_9^2))
\end{aligned}$$

■  $N_{15}^{(6)}$

$$\begin{aligned}
& \frac{1}{2} \left( 4(\tau_{10,12} + \tau_{11,13}) t^3 + \right. \\
& (\tau_{1,10}^2 + (4\tau_{1,12} + 2\tau_{1,14} + 4\tau_{1,17} + 4\tau_{2,7} + 8\tau_{2,12} + 4\tau_{2,14} + 2\tau_{2,17} - 2\tau_{3,7} + 4\tau_{3,10} + 3\tau_{4,7} + 6\tau_{4,12}) \tau_{1,10} + \tau_{1,11}^2 + \\
& 3\tau_{1,17}^2 + 3\tau_{2,7}^2 + \tau_{2,12}^2 + \tau_{2,13}^2 + 3\tau_{2,14}^2 + 3\tau_{2,16}^2 + 11\tau_{3,7}^2 + 7\tau_{3,10}^2 + 7\tau_{3,11}^2 + 11\tau_{4,7}^2 + 7\tau_{4,12}^2 + \\
& 7\tau_{4,13}^2 + \tau_{1,15} (2\tau_{1,13} + 3\tau_{1,15}) + \tau_{1,11} (4(\tau_{1,13} + \tau_{1,15}) - 2\tau_{1,16}) + 2\tau_{1,15} \tau_{2,7} - \tau_{1,16} \tau_{2,7} + 4\tau_{2,10} \tau_{2,12} + \\
& 4\tau_{1,15} \tau_{2,13} - 2\tau_{1,16} \tau_{2,13} + 4\tau_{2,11} \tau_{2,13} + 2\tau_{2,10} \tau_{2,14} + 4\tau_{2,12} \tau_{2,14} + 2\tau_{1,15} \tau_{2,15} + 2\tau_{2,13} \tau_{2,15} + 2\tau_{1,16} \tau_{2,16} - \\
& 2\tau_{2,11} \tau_{2,16} - 4\tau_{2,13} \tau_{2,16} + 2\tau_{2,12} \tau_{2,17} + 2\tau_{1,16} \tau_{3,7} - \tau_{2,10} \tau_{3,7} - \tau_{2,11} \tau_{3,7} - 3\tau_{2,12} \tau_{3,7} - 3\tau_{2,13} \tau_{3,7} - 5\tau_{2,14} \tau_{3,7} + \\
& 5\tau_{2,16} \tau_{3,7} + 2\tau_{2,10} \tau_{3,10} + 6\tau_{2,12} \tau_{3,10} + 10\tau_{2,14} \tau_{3,10} - 7\tau_{3,7} \tau_{3,10} + \tau_{1,14} (\tau_{2,7} + 2(\tau_{2,12} + \tau_{2,14} - \tau_{3,7} + 2\tau_{3,10})) - \\
& 4\tau_{1,16} \tau_{3,11} + 2\tau_{2,11} \tau_{3,11} + 6\tau_{2,13} \tau_{3,11} - 10\tau_{2,16} \tau_{3,11} - 7\tau_{3,7} \tau_{3,11} + 5\tau_{1,15} \tau_{4,7} + \tau_{2,10} \tau_{4,7} + \tau_{2,11} \tau_{4,7} + \\
& 2\tau_{2,12} \tau_{4,7} + 2\tau_{2,13} \tau_{4,7} + 2\tau_{2,15} \tau_{4,7} + 2\tau_{2,17} \tau_{4,7} + 2\tau_{2,10} \tau_{4,12} + 4\tau_{2,12} \tau_{4,12} + 4\tau_{2,17} \tau_{4,12} + 7\tau_{4,7} \tau_{4,12} + \\
& \tau_{1,12} (2\tau_{1,17} - \tau_{2,7} + 2\tau_{2,10} - \tau_{3,7} + 2\tau_{3,10} + \tau_{4,7} + 2\tau_{4,12}) + \tau_{1,17} (2\tau_{2,7} + 4\tau_{2,12} + 2\tau_{2,17} + 5(\tau_{4,7} + 2\tau_{4,12})) + \\
& 10\tau_{1,15} \tau_{4,13} + 2\tau_{2,11} \tau_{4,13} + 4\tau_{2,13} \tau_{4,13} + 4\tau_{2,15} \tau_{4,13} + 7\tau_{4,7} \tau_{4,13} + \\
& \tau_{2,7} (2\tau_{2,10} + 2\tau_{2,11} - \tau_{2,12} - \tau_{2,13} + \tau_{2,14} + \tau_{2,15} - \tau_{2,16} + \tau_{2,17} + 4\tau_{3,7} + 2\tau_{3,10} + 2\tau_{3,11} + 10\tau_{4,7} + \tau_{4,12} + \tau_{4,13}) + \\
& \tau_{1,13} (-\tau_{2,7} + 2\tau_{2,11} - \tau_{3,7} + 2\tau_{3,11} + \tau_{4,7} + 2\tau_{4,13}) + \\
& \left. \tau_{1,11} (4\tau_{2,7} + 8\tau_{2,13} + 2\tau_{2,15} - 4\tau_{2,16} - 2\tau_{3,7} + 4\tau_{3,11} + 3\tau_{4,7} + 6\tau_{4,13})) t^2 + \right. \\
& (3t + 2u)(t + 4u) \tau_{1,7}^2 + 4u^2 (2\tau_{2,7}^2 + 3(\tau_{3,7} + \tau_{4,7}) \tau_{2,7} + 3(\tau_{3,7}^2 + \tau_{4,7}^2)) + \\
& \tau_{1,7} \left( -(2\tau_{1,12} + 2\tau_{1,13} + \tau_{1,14} + \tau_{1,15} - \tau_{1,16} + \tau_{1,17} - 2\tau_{2,7} - \tau_{2,10} - \tau_{2,11} + 4\tau_{2,12} + 4\tau_{2,13} + 2\tau_{2,14} + \right. \\
& \tau_{2,15} - 2\tau_{2,16} + \tau_{2,17} - 10\tau_{3,7} + \tau_{3,10} + \tau_{3,11} + 2(-2\tau_{4,7} + \tau_{4,12} + \tau_{4,13})) t^2 + (t - 4u) \tau_{1,10} t + \\
& (t - 4u) \tau_{1,11} t + 12u^2 (\tau_{2,7} + \tau_{3,7} + \tau_{4,7}) + \frac{1}{2} (s^2 - t^2 - u^2) (-4\tau_{1,15} - 4\tau_{1,17} + 20\tau_{2,7} - \tau_{2,10} - \tau_{2,11} + \\
& \tau_{2,12} + \tau_{2,13} + \tau_{2,14} - \tau_{2,15} - \tau_{2,16} - \tau_{2,17} + 20\tau_{3,7} + \tau_{3,10} + \tau_{3,11} + 12\tau_{4,7} - 5(\tau_{4,12} + \tau_{4,13})) \Big) + \\
& \frac{1}{2} (s^2 - t^2 - u^2) (4\tau_{1,10}^2 + (8\tau_{1,17} - \tau_{2,7} + 2\tau_{2,10} + 2\tau_{2,17} + 5(\tau_{4,7} + 2\tau_{4,12})) \tau_{1,10} + 4(\tau_{1,11} + \tau_{1,15})^2 + 4\tau_{1,17}^2 + \\
& 14\tau_{2,7}^2 + 4\tau_{2,12}^2 + 4\tau_{2,13}^2 + 4\tau_{2,14}^2 + 4\tau_{2,16}^2 + 22\tau_{3,7}^2 + 6\tau_{3,10}^2 + 6\tau_{3,11}^2 + 22\tau_{4,7}^2 + 6\tau_{4,12}^2 + 6\tau_{4,13}^2 + \\
& \tau_{1,14} \tau_{2,7} - \tau_{1,15} \tau_{2,7} - \tau_{1,16} \tau_{2,7} + 2\tau_{1,15} \tau_{2,11} + 2\tau_{1,14} \tau_{2,12} - 2\tau_{1,16} \tau_{2,13} + 2\tau_{1,14} \tau_{2,14} + 2\tau_{1,15} \tau_{2,15} + 2\tau_{1,16} \tau_{2,16} - \\
& 8\tau_{2,13} \tau_{2,16} - \tau_{1,14} \tau_{3,7} + \tau_{1,16} \tau_{3,7} - 5\tau_{2,13} \tau_{3,7} - 5\tau_{2,14} \tau_{3,7} + 5\tau_{2,16} \tau_{3,7} + 2\tau_{1,14} \tau_{3,10} + 10\tau_{2,14} \tau_{3,10} - 6\tau_{3,7} \tau_{3,10} + \\
& \tau_{1,12} (\tau_{2,7} + 2\tau_{2,12} + 2\tau_{2,14} - \tau_{3,7} + 2\tau_{3,10}) + \tau_{2,12} (8\tau_{2,14} - 5\tau_{3,7} + 10\tau_{3,10}) - 2\tau_{1,16} \tau_{3,11} + 10\tau_{2,13} \tau_{3,11} - \\
& 10\tau_{2,16} \tau_{3,11} - 6\tau_{3,7} \tau_{3,11} + \tau_{1,13} (\tau_{2,7} + 2\tau_{2,13} - 2\tau_{2,16} - \tau_{3,7} + 2\tau_{3,11}) + 5\tau_{1,15} \tau_{4,7} + \tau_{2,10} \tau_{4,7} + \tau_{2,11} \tau_{4,7} + \\
& \tau_{2,15} \tau_{4,7} + \tau_{2,17} \tau_{4,7} + 2\tau_{2,10} \tau_{4,12} + 2\tau_{2,17} \tau_{4,12} + 6\tau_{4,7} \tau_{4,12} + \tau_{1,17} (-\tau_{2,7} + 2\tau_{2,10} + 2\tau_{2,17} + 5(\tau_{4,7} + 2\tau_{4,12})) + \\
& \tau_{2,7} (4\tau_{2,12} + 4\tau_{2,13} + 4\tau_{2,14} - 4\tau_{2,16} + 12\tau_{3,7} + 5\tau_{3,10} + 5\tau_{3,11} + 20\tau_{4,7} - \tau_{4,12} - \tau_{4,13}) + 10\tau_{1,15} \tau_{4,13} + \\
& \left. 2\tau_{2,11} \tau_{4,13} + 2\tau_{2,15} \tau_{4,13} + 6\tau_{4,7} \tau_{4,13} + \tau_{1,11} (-\tau_{2,7} + 2\tau_{2,11} + 2\tau_{2,15} + 5(\tau_{4,7} + 2\tau_{4,13}))) \right) l_8^2 l_9^2
\end{aligned}$$

■  $N_{15}^{(7)}$

0

■  $N_{15}^{(8)}$

0
