# Supplementary material for: The Ultraviolet Behavior of N=8 Supergravity at Four Loops
Source: arXiv:0905.2326 ancillary file (2012-01-08)
Supplement: Supplementary file 17 [file SUGRA23.pdf]

## Integral 23: $\mathcal{I}_{23}$

$\mathcal{N} = 8$  four-point four-loop amplitude.

### ■ 2D plot of graph associated with $\mathcal{I}_{23}$

This fixes the labelling associated with the numerator expressions given below.

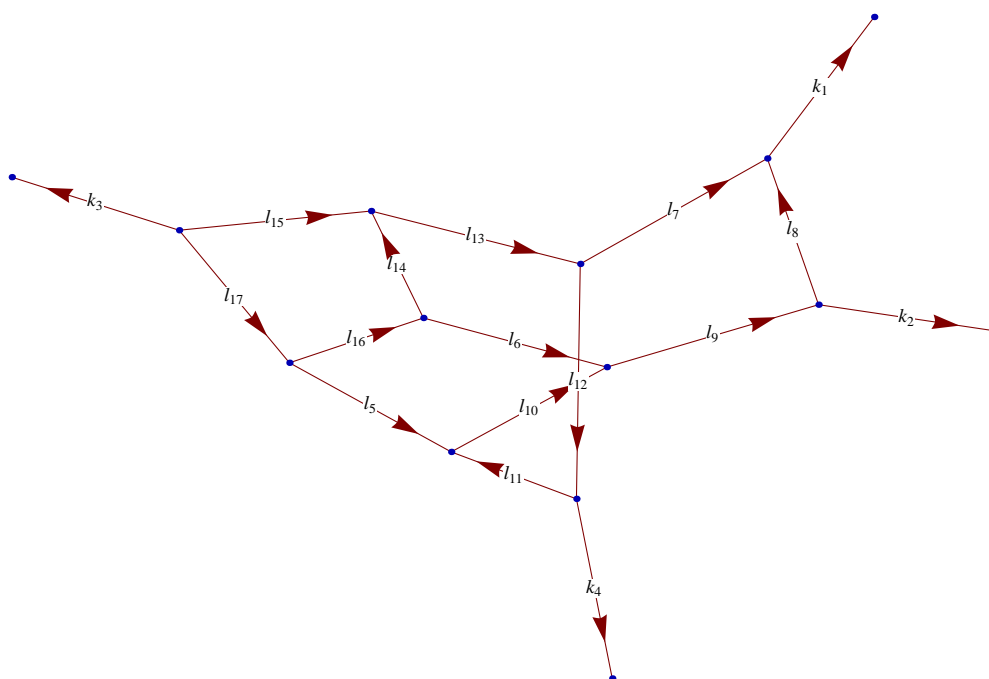

When using MathPlayer, by clicking three times (holding the click on the third click) directly on a vertex, one is able to move that vertex around, and its associated edges follow elastically. This functionality is absent when viewing as a pdf.

*Note: propagators for certain graphs were relabeled in the manuscript due to size constraints. The labels given in `aux/rawData/Neq8FourLoops.m` should be used for verification purposes.*

### ■ 3D plot of graph associated with $\mathcal{I}_{23}$

3D PLOT UNAVAILABLE FOR PDF. Please see .nb version for the 3D figure.

When using MathPlayer, by clicking anywhere in the image and dragging one should be able to rotate this 3D image. By holding (ALT) or (COMMAND) while clicking and moving the mouse up/down one should be able to zoom in/out. This functionality is absent when viewing as a pdf.

### "Vertex Form" of graph associated with $I_{23}$

This function returns the graph associated with the integral object in a vertex representation. This can be used as a way of specifying the topology of a graph using trivalent (cubic) vertices,  $\text{gVertex}[p_a, p_b, p_c]$ , where  $\{p_a, p_b, p_c\}$  are momenta labeling the propagators (edges) of the graph, and is understood that the edge labelled by  $p_a$  flows into the edge labelled by  $-p_a$ . Additionally, each vertex represents the manifest conservation of ( $D$  - dimensional) momenta :

$$\text{gVertex}[\{p_1, p_2, p_3\}] \iff (p_1 + p_2 + p_3 = 0)$$

$$\{\text{gVertex}(\{k_1, -l_8, -l_7\}), \text{gVertex}(\{k_2, -l_9, l_8\}), \text{gVertex}(\{k_3, l_{15}, l_{17}\}), \text{gVertex}(\{k_4, -l_{12}, l_{11}\}), \text{gVertex}(\{-l_5, l_{10}, -l_{11}\}), \\ \text{gVertex}(\{l_5, -l_{17}, l_{16}\}), \text{gVertex}(\{-l_6, l_9, -l_{10}\}), \text{gVertex}(\{l_6, -l_{16}, l_{14}\}), \text{gVertex}(\{l_7, -l_{13}, l_{12}\}), \text{gVertex}(\{l_{13}, -l_{14}, -l_{15}\})\}$$

### ■ Numerator expression for integral 23:

The following notation is used:  $\tau_{i,j} \equiv \begin{cases} 2 k_i \cdot l_j & \text{if } i \leq 4, j > 4 \\ 2 l_i \cdot l_j & \text{if } i, j > 4 \end{cases}$ .

$$s \equiv 2 k_1 \cdot k_2 = 2 k_3 \cdot k_4$$

We use  $s, t, u$  to represent the traditional Mandelstam variables for massless external four-point momenta:  $t \equiv 2 k_1 \cdot k_4 = 2 k_2 \cdot k_3$ .

$$u \equiv 2 k_1 \cdot k_3 = 2 k_2 \cdot k_4$$

Furthermore we use the shorthand  $(l_i)^2$  to represent the lorentz square:  $(l_i)^2 = l_i \cdot l_i$ .

The total numerator  $\mathcal{N}_{23}$  is given by summing over the following terms, distinguished here by explicit dependence on loop momenta:  $\mathcal{N}_{23} = \sum_{i=0}^8 \mathcal{N}_{23}^{(i)}$ :

#### ■ $\mathcal{N}_{23}^{(0)}$

$$0$$

#### ■ $\mathcal{N}_{23}^{(1)}$

$$0$$

#### ■ $\mathcal{N}_{23}^{(2)}$

$$s \left( s \left( s \left( \tau_{3,5} + \tau_{3,6} \right)^2 - 2 l_{11}^2 t u \right) - 3 l_{12}^2 t^3 \right) + 2 l_9^2 t^4$$

#### ■ $\mathcal{N}_{23}^{(3)}$

$$l_9^2 t^2 (2 (\tau_{1,11} - \tau_{2,8} + \tau_{2,11}) - 3 \tau_{4,8}) (-s^2 + t^2 + u^2) - l_{11}^2 t^2 (\tau_{1,12} + \tau_{2,12} - 2 \tau_{3,8} - 3 \tau_{3,10} + \tau_{3,12}) (-s^2 + t^2 + u^2) + \\ 3 l_{11}^2 t u (2 \tau_{3,10} - \tau_{3,12}) (-s^2 + t^2 + u^2) + l_{11}^2 u^2 (\tau_{1,12} + \tau_{2,12} - 2 \tau_{3,8} + 3 \tau_{3,10} - \tau_{3,12}) (-s^2 + t^2 + u^2) + \\ 3 l_{12}^2 s^2 t^2 (2 \tau_{3,11} - 3 \tau_{3,8}) + l_9^2 t^4 (-4 \tau_{1,11} + 5 \tau_{2,8} - 4 \tau_{2,11} + 6 \tau_{4,8}) + l_{11}^2 t^4 (\tau_{1,12} + \tau_{2,12} - 2 \tau_{3,8} - \tau_{3,12}) - \\ l_{11}^2 u^4 (\tau_{1,12} + \tau_{2,12} - 2 \tau_{3,8} + \tau_{3,12}) - 3 t (\tau_{3,5} + \tau_{3,6})^2 (\tau_{1,5} + \tau_{1,6} + \tau_{2,5} + \tau_{2,6} + \tau_{3,5} + \tau_{3,6}) (-s^2 + t^2 + u^2) - \\ 3 u (\tau_{3,5} + \tau_{3,6})^2 (\tau_{1,5} + \tau_{1,6} + \tau_{2,5} + \tau_{2,6} + \tau_{3,5} + \tau_{3,6}) (-s^2 + t^2 + u^2) + \\ 2 t^3 (\tau_{3,5} + \tau_{3,6})^2 (\tau_{1,5} + \tau_{1,6} + \tau_{2,5} + \tau_{2,6} + \tau_{3,5} + \tau_{3,6}) + 2 u^3 (\tau_{3,5} + \tau_{3,6})^2 (\tau_{1,5} + \tau_{1,6} + \tau_{2,5} + \tau_{2,6} + \tau_{3,5} + \tau_{3,6})$$

■  $N_{23}^{(4)}$

$\frac{1}{2}$

$$\begin{aligned}
& \left( (2(7l_9^2 - l_{10}^2)l_{11}^2 + l_7^2(l_8^2 - l_{12}^2) + 8l_{12}^2(l_{17}^2 - l_9^2))t^4 - 2(2l_9^2\tau_{1,11}^2 + 2(-3\tau_{2,8} + \tau_{2,10} + \tau_{2,11} - 4\tau_{4,8} + \tau_{4,10})l_9^2 + \tau_{3,11}l_{12}^2)\tau_{1,11} + \right. \\
& \quad 4\tau_{2,8}^2l_9^2 - 2\tau_{2,10}^2l_9^2 + 6\tau_{4,8}^2l_9^2 - 2\tau_{4,10}^2l_9^2 - 8\tau_{2,11}\tau_{4,8}l_9^2 + 2\tau_{2,8}(5\tau_{4,8} - 3\tau_{2,11})l_9^2 + 4\tau_{2,11}\tau_{4,10}l_9^2 + 2\tau_{3,10}^2l_{11}^2 - \\
& \quad 2\tau_{3,12}^2l_{11}^2 + 2\tau_{3,8}(-\tau_{1,12} - \tau_{2,12} + \tau_{3,8})l_{11}^2 - 6\tau_{3,8}\tau_{3,10}l_{11}^2 + 6\tau_{3,8}\tau_{3,12}l_{11}^2 + 2\tau_{2,10}(2(\tau_{2,11} - \tau_{4,10})l_9^2 + \tau_{3,10}l_{11}^2) + \\
& \quad 2\tau_{1,10}(\tau_{3,10}l_{11}^2 - (\tau_{2,10} - \tau_{2,11} + \tau_{4,10})l_9^2) + 9\tau_{3,8}^2l_{12}^2 + 4\tau_{3,11}^2l_{12}^2 + 2\tau_{2,11}\tau_{3,11}l_{12}^2 - 12\tau_{3,8}\tau_{3,11}l_{12}^2)t^3 + \\
& \quad 2(\tau_{3,5} + \tau_{3,6})^2(\tau_{1,5} + \tau_{1,6} + \tau_{2,5} + \tau_{2,6} + \tau_{3,5} + \tau_{3,6})^2t^2 + \\
& \quad (s^2 - t^2 - u^2)(-4l_{10}^2l_{11}^2 + l_9^2(11l_{11}^2 - 6l_{12}^2) + l_7^2(2l_8^2 + 4l_9^2 - 6l_{11}^2 - l_{12}^2) + 6l_{12}^2l_{17}^2)t^2 + \\
& \quad u(s^2 - t^2 - u^2)(l_7^2(3l_8^2 + 2l_9^2 - 4l_{11}^2) + 2(l_9^2 - 3l_{10}^2)l_{11}^2 - 3l_9^2l_{12}^2)t + \\
& \quad (s^2 - t^2 - u^2)(2l_9^2\tau_{1,10}^2 + 3\tau_{2,11}^2l_7^2 + 3\tau_{3,9}^2l_7^2 + \tau_{1,11}^2(3l_7^2 - 2l_9^2) + \\
& \quad 2((\tau_{2,10} + \tau_{4,10})(2\tau_{1,10} + \tau_{2,10} + \tau_{4,10}) - (\tau_{2,8} + \tau_{4,8})(\tau_{2,8} + 3\tau_{4,8}))l_9^2 + 6(\tau_{1,12} + \tau_{2,12} - \tau_{3,8})\tau_{3,8}l_{11}^2 - \\
& \quad 2(-\tau_{3,12}^2 + (\tau_{1,12} + \tau_{2,12} + 3\tau_{3,8})\tau_{3,12} + \tau_{3,10}(2\tau_{1,10} + 2\tau_{2,10} - 3\tau_{3,8} + \tau_{3,10}))l_{11}^2 - \\
& \quad 2(3\tau_{3,8} - 2\tau_{3,11})^2l_{12}^2 + \tau_{2,11}(6\tau_{3,9}l_7^2 - 4(\tau_{1,10} - \tau_{2,8} + \tau_{2,10} - 2\tau_{4,8} + \tau_{4,10})l_9^2 - 4\tau_{3,11}l_{12}^2) + \\
& \quad 2\tau_{1,11}(3\tau_{3,9}l_7^2 + \tau_{2,11}(3l_7^2 - l_9^2) - (\tau_{1,10} - 2\tau_{2,8} + \tau_{2,10} - 4\tau_{4,8} + \tau_{4,10})l_9^2 - 2\tau_{3,11}l_{12}^2))t + \\
& \quad 2u^2(\tau_{3,5} + \tau_{3,6})^2(\tau_{1,5} + \tau_{1,6} + \tau_{2,5} + \tau_{2,6} + \tau_{3,5} + \tau_{3,6})^2 + 2(s^2 - t^2 - u^2)(\tau_{3,5} + \tau_{3,6})^2 \\
& \quad (\tau_{1,5} + \tau_{1,6} + \tau_{2,5} + \tau_{2,6} + \tau_{3,5} + \tau_{3,6})^2 + 2u^3 \\
& \quad (l_7^2(\tau_{1,11} + \tau_{2,11} + \tau_{3,9})^2 + 2(-\tau_{3,8}^2 + 3(\tau_{3,12} - \tau_{3,10})\tau_{3,8} + \tau_{3,10}^2 - \tau_{3,12}^2 + \tau_{1,12}(\tau_{3,8} - \tau_{3,12}) + \tau_{2,12}(\tau_{3,8} - \tau_{3,12}))l_{11}^2) + \\
& \quad u(s^2 - t^2 - u^2)(-9l_{12}^2\tau_{3,8}^2 + 3(\tau_{1,11} + \tau_{2,11} + \tau_{3,9})^2l_7^2 + 2(-3\tau_{3,8}^2 + 3(\tau_{3,12} - \tau_{3,10})\tau_{3,8} + \tau_{3,10}^2 - \tau_{3,12}^2 - (\tau_{1,10} + \tau_{2,10}) \\
& \quad \tau_{3,10} + \tau_{1,12}(3\tau_{3,8} - 2\tau_{3,12}) + \tau_{2,12}(3\tau_{3,8} - 2\tau_{3,12}))l_{11}^2 - 2\tau_{3,11}(\tau_{1,11} + \tau_{2,11} - 6\tau_{3,8} + 2\tau_{3,11})l_{12}^2) + \\
& \quad u^4(l_7^2(l_8^2 + 8l_9^2 + 20l_{11}^2 + 2l_{12}^2) - 2l_{10}^2l_{11}^2) + 2u^2(s^2 - t^2 - u^2)(-l_9^2 + 2l_{10}^2)l_{11}^2 + l_7^2(l_8^2 + 2l_9^2 + 6l_{11}^2 + l_{12}^2) - l_{12}^2l_{17}^2)
\end{aligned}$$

■  $N_{23}^{(5)}$ 

$$\begin{aligned}
& -\frac{3}{4}\tau_{1,13}l_7^2l_8^2t^3 - \frac{3}{4}\tau_{2,13}l_7^2l_8^2t^3 - 2\tau_{4,13}l_7^2l_8^2t^3 - 2\tau_{1,8}l_7^2l_9^2t^3 - 4\tau_{3,8}l_7^2l_9^2t^3 + 4\tau_{3,12}l_7^2l_9^2t^3 + 2\tau_{2,12}l_7^2l_{11}^2t^3 - 2\tau_{3,5}l_7^2l_{11}^2t^3 + \\
& 6\tau_{3,8}l_7^2l_{11}^2t^3 - 4\tau_{3,12}l_7^2l_{11}^2t^3 + 2\tau_{4,12}l_7^2l_{11}^2t^3 - 3\tau_{1,5}l_9^2l_{11}^2t^3 + 2\tau_{1,10}l_9^2l_{11}^2t^3 + 2\tau_{2,5}l_9^2l_{11}^2t^3 + \tau_{2,8}l_9^2l_{11}^2t^3 + \\
& 11\tau_{3,8}l_9^2l_{11}^2t^3 - 7\tau_{3,10}l_9^2l_{11}^2t^3 - 8\tau_{3,16}l_9^2l_{11}^2t^3 + \frac{1}{4}\tau_{1,13}l_7^2l_{12}^2t^3 - \tau_{2,13}l_7^2l_{12}^2t^3 + 2\tau_{4,9}l_7^2l_{12}^2t^3 - \frac{1}{4}\tau_{4,13}l_7^2l_{12}^2t^3 - \\
& \tau_{2,8}l_9^2l_{12}^2t^3 + \tau_{2,10}l_9^2l_{12}^2t^3 - 2\tau_{2,13}l_9^2l_{12}^2t^3 - 6\tau_{3,8}l_9^2l_{12}^2t^3 + 6\tau_{3,10}l_9^2l_{12}^2t^3 + 2\tau_{3,14}l_9^2l_{12}^2t^3 + \tau_{1,11}^3l_7^2t^2 + 2\tau_{2,11}^3l_7^2t^2 + \\
& \tau_{2,8}^3l_9^2t^2 + \tau_{2,10}^3l_9^2t^2 + 2\tau_{4,8}^3l_9^2t^2 + 2\tau_{1,10}\tau_{2,10}^2l_9^2t^2 - 2\tau_{2,8}\tau_{2,10}^2l_9^2t^2 + 5\tau_{2,8}\tau_{4,8}^2l_9^2t^2 - 2\tau_{2,8}\tau_{4,10}^2l_9^2t^2 + \\
& \tau_{2,10}\tau_{4,10}^2l_9^2t^2 - 2\tau_{4,8}\tau_{4,10}^2l_9^2t^2 + \tau_{1,10}^2\tau_{2,10}l_9^2t^2 - 2\tau_{1,10}\tau_{2,8}\tau_{2,10}l_9^2t^2 + 4\tau_{2,8}^2\tau_{4,8}l_9^2t^2 - 2\tau_{2,10}^2\tau_{4,8}l_9^2t^2 - \\
& 2\tau_{1,10}\tau_{2,10}\tau_{4,8}l_9^2t^2 + 2\tau_{2,10}^2\tau_{4,10}l_9^2t^2 - 2\tau_{1,10}\tau_{2,8}\tau_{4,10}l_9^2t^2 + 2\tau_{1,10}\tau_{2,10}\tau_{4,10}l_9^2t^2 - 4\tau_{2,8}\tau_{2,10}\tau_{4,10}l_9^2t^2 - \\
& 2\tau_{1,10}\tau_{4,8}\tau_{4,10}l_9^2t^2 - 4\tau_{2,10}\tau_{4,8}\tau_{4,10}l_9^2t^2 + \tau_{3,10}^3l_{11}^2t^2 - \tau_{3,12}^3l_{11}^2t^2 + \tau_{1,10}\tau_{3,10}^2l_{11}^2t^2 + \tau_{2,10}\tau_{3,10}^2l_{11}^2t^2 - \\
& 4\tau_{3,8}\tau_{3,10}^2l_{11}^2t^2 - \tau_{1,12}\tau_{3,12}^2l_{11}^2t^2 - \tau_{2,12}\tau_{3,12}^2l_{11}^2t^2 + 4\tau_{3,8}\tau_{3,12}^2l_{11}^2t^2 + 6\tau_{3,8}^2\tau_{3,10}l_{11}^2t^2 - 2\tau_{1,10}\tau_{3,8}\tau_{3,10}l_{11}^2t^2 - \\
& 2\tau_{2,10}\tau_{3,8}\tau_{3,10}l_{11}^2t^2 - 6\tau_{3,8}^2\tau_{3,12}l_{11}^2t^2 + 2\tau_{1,12}\tau_{3,8}\tau_{3,12}l_{11}^2t^2 + 2\tau_{2,12}\tau_{3,8}\tau_{3,12}l_{11}^2t^2 - 3\tau_{3,8}^3l_{12}^2t^2 + \\
& \tau_{3,11}^3l_{12}^2t^2 - 4\tau_{3,8}\tau_{3,11}^2l_{12}^2t^2 + 6\tau_{3,8}^2\tau_{3,11}l_{12}^2t^2 + \frac{9}{8}(-s^2+t^2+u^2)\tau_{1,13}l_7^2l_8^2t + \frac{9}{8}(-s^2+t^2+u^2)\tau_{2,13}l_7^2l_8^2t + \\
& 3(-s^2+t^2+u^2)\tau_{4,13}l_7^2l_8^2t - (-s^2+t^2+u^2)\tau_{3,5}l_7^2l_9^2t - (-s^2+t^2+u^2)\tau_{3,8}l_7^2l_9^2t + (-s^2+t^2+u^2)\tau_{4,8}l_7^2l_9^2t + \\
& 3(-s^2+t^2+u^2)\tau_{2,5}l_7^2l_{11}^2t - 2(-s^2+t^2+u^2)\tau_{2,12}l_7^2l_{11}^2t - (-s^2+t^2+u^2)\tau_{3,5}l_7^2l_{11}^2t - 3(-s^2+t^2+u^2)\tau_{3,8}l_7^2l_{11}^2t + \\
& 2(-s^2+t^2+u^2)\tau_{3,12}l_7^2l_{11}^2t + 2(-s^2+t^2+u^2)\tau_{4,5}l_7^2l_{11}^2t - 2(-s^2+t^2+u^2)\tau_{4,8}l_7^2l_{11}^2t - 2(-s^2+t^2+u^2)\tau_{4,12}l_7^2l_{11}^2t + \\
& \frac{7}{2}(-s^2+t^2+u^2)\tau_{1,5}l_9^2l_{11}^2t - \frac{5}{2}(-s^2+t^2+u^2)\tau_{1,10}l_9^2l_{11}^2t - (-s^2+t^2+u^2)\tau_{2,5}l_9^2l_{11}^2t - 2(-s^2+t^2+u^2)\tau_{2,8}l_9^2l_{11}^2t + \\
& \frac{1}{2}(-s^2+t^2+u^2)\tau_{2,10}l_9^2l_{11}^2t - \frac{15}{2}(-s^2+t^2+u^2)\tau_{3,8}l_9^2l_{11}^2t + 5(-s^2+t^2+u^2)\tau_{3,10}l_9^2l_{11}^2t + 6(-s^2+t^2+u^2)\tau_{3,16}l_9^2l_{11}^2t - \\
& \frac{3}{2}(-s^2+t^2+u^2)\tau_{1,13}l_7^2l_{12}^2t - \frac{3}{2}(-s^2+t^2+u^2)\tau_{2,13}l_7^2l_{12}^2t - \frac{9}{4}(-s^2+t^2+u^2)\tau_{4,9}l_7^2l_{12}^2t - \frac{3}{4}(-s^2+t^2+u^2)\tau_{4,13}l_7^2l_{12}^2t + \\
& 2(-s^2+t^2+u^2)\tau_{2,8}l_9^2l_{12}^2t - 2(-s^2+t^2+u^2)\tau_{2,10}l_9^2l_{12}^2t + 3(-s^2+t^2+u^2)\tau_{2,13}l_9^2l_{12}^2t + 3(-s^2+t^2+u^2)\tau_{3,8}l_9^2l_{12}^2t - \\
& 3(-s^2+t^2+u^2)\tau_{3,10}l_9^2l_{12}^2t - (-s^2+t^2+u^2)\tau_{3,14}l_9^2l_{12}^2t + 2s^2\tau_{3,9}^3l_7^2 - \frac{3}{4}u^3\tau_{1,13}l_7^2l_8^2 + \frac{9}{8}u(-s^2+t^2+u^2)\tau_{1,13}l_7^2l_8^2 - \\
& \frac{3}{4}u^3\tau_{2,13}l_7^2l_8^2 + \frac{9}{8}u(-s^2+t^2+u^2)\tau_{2,13}l_7^2l_8^2 - 2u^3\tau_{4,13}l_7^2l_8^2 + 3u(-s^2+t^2+u^2)\tau_{4,13}l_7^2l_8^2 + (s^2-t^2-u^2)\tau_{4,8}^3l_9^2 + \\
& 2(s^2-t^2-u^2)\tau_{2,8}^2\tau_{4,8}^2l_9^2 + (-s^2+t^2+u^2)\tau_{4,8}\tau_{4,10}^2l_9^2 + (-s^2+t^2+u^2)\tau_{1,10}^2\tau_{4,8}l_9^2 + (s^2-t^2-u^2)\tau_{2,8}^2\tau_{4,8}l_9^2 + \\
& (-s^2+t^2+u^2)\tau_{2,10}^2\tau_{4,8}l_9^2 + 2(-s^2+t^2+u^2)\tau_{1,10}\tau_{2,10}\tau_{4,8}l_9^2 + 2(-s^2+t^2+u^2)\tau_{1,10}\tau_{4,8}\tau_{4,10}l_9^2 + \\
& 2(-s^2+t^2+u^2)\tau_{2,10}\tau_{4,8}\tau_{4,10}l_9^2 + u^3\tau_{1,8}l_7^2l_9^2 - 3u^3\tau_{1,12}l_7^2l_9^2 + 2u(-s^2+t^2+u^2)\tau_{1,12}l_7^2l_9^2 + 6u^3\tau_{3,5}l_7^2l_9^2 -
\end{aligned}$$

$$\begin{aligned}
& 4u(-s^2+t^2+u^2)\tau_{3,5}l_7^2l_9^2-8u^3\tau_{3,8}l_7^2l_9^2+5u(-s^2+t^2+u^2)\tau_{3,8}l_7^2l_9^2+8u^3\tau_{3,12}l_7^2l_9^2-3u(-s^2+t^2+u^2)\tau_{3,12}l_7^2l_9^2+ \\
& u(-s^2+t^2+u^2)\tau_{4,5}l_7^2l_9^2+2u(-s^2+t^2+u^2)\tau_{4,8}l_7^2l_9^2+\tau_{2,11}^2((2\tau_{1,10}-\tau_{2,8}+\tau_{2,10})l_9^2t^2+2(s^2+2t^2)\tau_{3,9}l_7^2)+ \\
& \tau_{1,11}^2(4\tau_{2,11}l_7^2t^2+(-2u\tau_{1,10}+(t+2u)(\tau_{2,8}-\tau_{2,10})+2s(\tau_{4,10}-\tau_{4,8}))l_9^2t+2(s^2+t^2)\tau_{3,9}l_7^2)+u^2\tau_{3,10}^3l_{11}^2+ \\
& (s^2-t^2-u^2)\tau_{3,10}^3l_{11}^2-u^2\tau_{3,12}^3l_{11}^2+(-s^2+t^2+u^2)\tau_{3,12}^3l_{11}^2+u^2\tau_{1,10}\tau_{3,10}^2l_{11}^2+(s^2-t^2-u^2)\tau_{1,10}\tau_{3,10}^2l_{11}^2+ \\
& u^2\tau_{2,10}\tau_{3,10}^2l_{11}^2+(s^2-t^2-u^2)\tau_{2,10}\tau_{3,10}^2l_{11}^2-4u^2\tau_{3,8}\tau_{3,10}^2l_{11}^2+4(-s^2+t^2+u^2)\tau_{3,8}\tau_{3,10}^2l_{11}^2-u^2\tau_{1,12}\tau_{3,12}^2l_{11}^2+ \\
& (-s^2+t^2+u^2)\tau_{1,12}\tau_{3,12}^2l_{11}^2-u^2\tau_{2,12}\tau_{3,12}^2l_{11}^2+(-s^2+t^2+u^2)\tau_{2,12}\tau_{3,12}^2l_{11}^2+4u^2\tau_{3,8}\tau_{3,12}^2l_{11}^2+ \\
& 4(s^2-t^2-u^2)\tau_{3,8}\tau_{3,12}^2l_{11}^2+6u^2\tau_{3,8}^2\tau_{3,10}l_{11}^2+6(s^2-t^2-u^2)\tau_{3,8}^2\tau_{3,10}l_{11}^2-2u^2\tau_{1,10}\tau_{3,8}\tau_{3,10}l_{11}^2+ \\
& 2(-s^2+t^2+u^2)\tau_{1,10}\tau_{3,8}\tau_{3,10}l_{11}^2-2u^2\tau_{2,10}\tau_{3,8}\tau_{3,10}l_{11}^2+2(-s^2+t^2+u^2)\tau_{2,10}\tau_{3,8}\tau_{3,10}l_{11}^2-6u^2\tau_{3,8}^2\tau_{3,12}l_{11}^2+ \\
& 6(-s^2+t^2+u^2)\tau_{3,8}^2\tau_{3,12}l_{11}^2+2u^2\tau_{1,12}\tau_{3,8}\tau_{3,12}l_{11}^2+2(s^2-t^2-u^2)\tau_{1,12}\tau_{3,8}\tau_{3,12}l_{11}^2+2u^2\tau_{2,12}\tau_{3,8}\tau_{3,12}l_{11}^2+ \\
& 2(s^2-t^2-u^2)\tau_{2,12}\tau_{3,8}\tau_{3,12}l_{11}^2-10u^3\tau_{2,5}l_7^2l_{11}^2+8u(-s^2+t^2+u^2)\tau_{2,5}l_7^2l_{11}^2-6u^3\tau_{2,12}l_7^2l_{11}^2+ \\
& 3u(-s^2+t^2+u^2)\tau_{2,12}l_7^2l_{11}^2+2u^3\tau_{3,5}l_7^2l_{11}^2-3u(-s^2+t^2+u^2)\tau_{3,5}l_7^2l_{11}^2-10u^3\tau_{3,8}l_7^2l_{11}^2+5u(-s^2+t^2+u^2)\tau_{3,8}l_7^2l_{11}^2+ \\
& 6u^3\tau_{3,12}l_7^2l_{11}^2-3u(-s^2+t^2+u^2)\tau_{3,12}l_7^2l_{11}^2-4u^3\tau_{4,5}l_7^2l_{11}^2+4u(-s^2+t^2+u^2)\tau_{4,5}l_7^2l_{11}^2+2u^3\tau_{4,8}l_7^2l_{11}^2- \\
& 3u(-s^2+t^2+u^2)\tau_{4,8}l_7^2l_{11}^2-2u^3\tau_{4,12}l_7^2l_{11}^2-2u^3\tau_{1,5}l_9^2l_{11}^2+3u(-s^2+t^2+u^2)\tau_{1,5}l_9^2l_{11}^2+\frac{1}{2}u(-s^2+t^2+u^2)\tau_{1,10}l_9^2l_{11}^2- \\
& 2u^3\tau_{2,5}l_9^2l_{11}^2+u(-s^2+t^2+u^2)\tau_{2,5}l_9^2l_{11}^2-\frac{1}{2}u(-s^2+t^2+u^2)\tau_{2,8}l_9^2l_{11}^2+u(-s^2+t^2+u^2)\tau_{2,10}l_9^2l_{11}^2- \\
& 2u^3\tau_{3,8}l_9^2l_{11}^2-u(-s^2+t^2+u^2)\tau_{3,8}l_9^2l_{11}^2+2u^3\tau_{3,10}l_9^2l_{11}^2+\frac{1}{2}u(-s^2+t^2+u^2)\tau_{3,10}l_9^2l_{11}^2+2u^3\tau_{3,16}l_9^2l_{11}^2+ \\
& u(-s^2+t^2+u^2)\tau_{3,16}l_9^2l_{11}^2-3u^2\tau_{3,8}^3l_{12}^2+3(-s^2+t^2+u^2)\tau_{3,8}^3l_{12}^2+u^2\tau_{3,11}^3l_{12}^2+(s^2-t^2-u^2)\tau_{3,11}^3l_{12}^2- \\
& 4u^2\tau_{3,8}\tau_{3,11}^2l_{12}^2+4(-s^2+t^2+u^2)\tau_{3,8}\tau_{3,11}^2l_{12}^2+6u^2\tau_{3,8}^2\tau_{3,11}l_{12}^2+6(s^2-t^2-u^2)\tau_{3,8}^2\tau_{3,11}l_{12}^2+\frac{1}{2}u^3\tau_{1,13}l_7^2l_{12}^2- \\
& \frac{3}{2}u(-s^2+t^2+u^2)\tau_{1,13}l_7^2l_{12}^2-\frac{3}{2}u(-s^2+t^2+u^2)\tau_{2,13}l_7^2l_{12}^2-u^3\tau_{4,9}l_7^2l_{12}^2-\frac{3}{4}u(-s^2+t^2+u^2)\tau_{4,9}l_7^2l_{12}^2- \\
& \frac{1}{2}u^3\tau_{4,13}l_7^2l_{12}^2-\frac{3}{4}u(-s^2+t^2+u^2)\tau_{4,13}l_7^2l_{12}^2-u(-s^2+t^2+u^2)\tau_{2,10}l_9^2l_{12}^2+2u(-s^2+t^2+u^2)\tau_{2,13}l_9^2l_{12}^2+ \\
& u(-s^2+t^2+u^2)\tau_{3,8}l_9^2l_{12}^2-2u(-s^2+t^2+u^2)\tau_{3,10}l_9^2l_{12}^2+\frac{1}{2}\tau_{1,9}l_7^2\left(2s^2(\tau_{1,11}+\tau_{2,11}+\tau_{3,9})^2-\frac{1}{2}u(-9s^2+3t^2+5u^2)l_{12}^2\right)+ \\
& \tau_{2,11}(\tau_{3,11}(\tau_{3,11}-2\tau_{3,8})l_{12}^2s^2+2(2s^2+t^2)\tau_{3,9}^2l_7^2-2t(t\tau_{1,10}^2-(t\tau_{2,8}-2t\tau_{2,10}+(t+2u)\tau_{4,8}-t\tau_{4,10})\tau_{1,10}+t\tau_{2,8}^2+ \\
& t\tau_{2,10}^2+2s\tau_{4,8}(\tau_{4,10}-\tau_{4,8})+\tau_{2,8}(-2t\tau_{2,10}+(3t+2u)\tau_{4,8}-2t\tau_{4,10})+\tau_{2,10}(2s\tau_{4,8}+t\tau_{4,10}))l_9^2)+ \\
& \tau_{1,11}(\tau_{3,11}(\tau_{3,11}-2\tau_{3,8})l_{12}^2s^2+5t^2\tau_{2,11}^2l_7^2+(4s^2+t^2)\tau_{3,9}^2l_7^2+(s^2-t^2-u^2)\tau_{1,10}^2l_9^2-2t^2\tau_{2,8}^2l_9^2+ \\
& (s^2-t^2-u^2)\tau_{2,10}^2l_9^2-4t^2\tau_{4,8}^2l_9^2+2(-s^2+t^2+u^2)\tau_{4,8}^2l_9^2+2t^2\tau_{4,10}^2l_9^2+(s^2-t^2-u^2)\tau_{4,10}^2l_9^2+2t^2\tau_{2,10}\tau_{4,8}l_9^2+ \\
& (s^2-t^2-u^2)\tau_{2,10}\tau_{4,8}l_9^2+2t^2\tau_{2,10}\tau_{4,10}l_9^2+2(s^2-t^2-u^2)\tau_{2,10}\tau_{4,10}l_9^2+2t^2\tau_{4,8}\tau_{4,10}l_9^2+(s^2-t^2-u^2)\tau_{4,8}\tau_{4,10}l_9^2+
\end{aligned}$$

$$\begin{aligned}
& 2t\tau_{2,8}((t-u)\tau_{2,10} - (3t+2u)\tau_{4,8} + (t-u)\tau_{4,10})l_9^2 + 2t\tau_{1,10}(u(-\tau_{2,8} + 2\tau_{2,10} + \tau_{4,8}) + (t+2u)\tau_{4,10})l_9^2 + \\
& 2\tau_{2,11}((2s^2 + 3t^2)\tau_{3,9}l_7^2 + t((t-u)\tau_{1,10} + u\tau_{2,8} - u\tau_{2,10} + s(\tau_{4,10} - \tau_{4,8}))l_9^2) - \\
& s^2(2u(\tau_{3,8} - \tau_{3,10} - \tau_{3,15}) + 2t(\tau_{1,10} + \tau_{1,15} + \tau_{1,16} + \tau_{2,10} + \tau_{2,15} + \tau_{2,16} - 5\tau_{3,8} + 3(\tau_{3,10} + \tau_{3,15})) + (3t-u)\tau_{3,16})l_{12}^2l_{17}^2
\end{aligned}$$

■  $N_{23}^{(6)}$

$$\begin{aligned}
& -\frac{1}{2}l_6^2l_7^2l_9^2s^3 - \frac{1}{2}l_6^2l_7^2l_{11}^2s^3 - \frac{119}{32}l_7^2l_8^2l_{11}^2s^3 + \frac{17}{8}l_7^2l_8^2l_{12}^2s^3 - \frac{13}{2}l_7^2l_9^2l_{12}^2s^3 + 2l_9^2l_{12}^2l_{15}^2s^3 + \frac{25}{16}l_9^2l_{13}^2l_{15}^2s^3 - \frac{1}{4}l_9^2l_{12}^2l_{17}^2s^3 + \\
& 2\tau_{4,13}^2l_7^2l_8^2s^2 + \tau_{3,5}^2l_7^2l_9^2s^2 + 3\tau_{3,8}^2l_7^2l_9^2s^2 + \tau_{3,12}^2l_7^2l_9^2s^2 - \tau_{1,12}\tau_{3,5}l_7^2l_9^2s^2 + 2\tau_{1,12}\tau_{3,8}l_7^2l_9^2s^2 - 4\tau_{3,5}\tau_{3,8}l_7^2l_9^2s^2 - \\
& 2\tau_{1,12}\tau_{3,12}l_7^2l_9^2s^2 + 4\tau_{3,5}\tau_{3,12}l_7^2l_9^2s^2 - 4\tau_{3,8}\tau_{3,12}l_7^2l_9^2s^2 + \tau_{3,8}\tau_{4,5}l_7^2l_9^2s^2 - \tau_{3,12}\tau_{4,5}l_7^2l_9^2s^2 + \tau_{1,8}\tau_{4,8}l_7^2l_9^2s^2 + \\
& 2\tau_{3,8}\tau_{4,8}l_7^2l_9^2s^2 - 2\tau_{3,12}\tau_{4,8}l_7^2l_9^2s^2 - \tau_{2,12}^2l_7^2l_{11}^2s^2 + \tau_{3,5}^2l_7^2l_{11}^2s^2 - 3\tau_{3,12}^2l_7^2l_{11}^2s^2 - \tau_{4,12}^2l_7^2l_{11}^2s^2 + \tau_{2,5}\tau_{2,12}l_7^2l_{11}^2s^2 - \\
& \tau_{2,5}\tau_{3,5}l_7^2l_{11}^2s^2 - 2\tau_{2,12}\tau_{3,5}l_7^2l_{11}^2s^2 + 7\tau_{2,5}\tau_{3,8}l_7^2l_{11}^2s^2 + 5\tau_{2,12}\tau_{3,8}l_7^2l_{11}^2s^2 - 5\tau_{3,5}\tau_{3,8}l_7^2l_{11}^2s^2 - 7\tau_{2,5}\tau_{3,12}l_7^2l_{11}^2s^2 - \\
& 4\tau_{2,12}\tau_{3,12}l_7^2l_{11}^2s^2 + 2\tau_{3,5}\tau_{3,12}l_7^2l_{11}^2s^2 + 3\tau_{3,8}\tau_{3,12}l_7^2l_{11}^2s^2 + 2\tau_{2,5}\tau_{4,5}l_7^2l_{11}^2s^2 + \tau_{2,12}\tau_{4,5}l_7^2l_{11}^2s^2 - 2\tau_{3,5}\tau_{4,5}l_7^2l_{11}^2s^2 + \\
& 2\tau_{3,8}\tau_{4,5}l_7^2l_{11}^2s^2 - 2\tau_{3,12}\tau_{4,5}l_7^2l_{11}^2s^2 - \tau_{2,5}\tau_{4,8}l_7^2l_{11}^2s^2 + 2\tau_{3,5}\tau_{4,8}l_7^2l_{11}^2s^2 - 4\tau_{3,8}\tau_{4,8}l_7^2l_{11}^2s^2 + 2\tau_{3,12}\tau_{4,8}l_7^2l_{11}^2s^2 + \\
& \tau_{2,5}\tau_{4,12}l_7^2l_{11}^2s^2 - 2\tau_{2,12}\tau_{4,12}l_7^2l_{11}^2s^2 - 3\tau_{3,5}\tau_{4,12}l_7^2l_{11}^2s^2 + \tau_{3,8}\tau_{4,12}l_7^2l_{11}^2s^2 - 2\tau_{3,12}\tau_{4,12}l_7^2l_{11}^2s^2 - \tau_{4,8}\tau_{4,12}l_7^2l_{11}^2s^2 + \\
& 2\tau_{2,5}^2l_9^2l_{11}^2s^2 + 2\tau_{3,8}^2l_9^2l_{11}^2s^2 + 2\tau_{3,16}^2l_9^2l_{11}^2s^2 + \tau_{1,5}\tau_{1,10}l_9^2l_{11}^2s^2 + 2\tau_{1,5}\tau_{2,5}l_9^2l_{11}^2s^2 + \tau_{1,10}\tau_{2,5}l_9^2l_{11}^2s^2 - \\
& \frac{1}{2}\tau_{1,10}\tau_{2,8}l_9^2l_{11}^2s^2 - \frac{1}{2}\tau_{2,8}\tau_{2,10}l_9^2l_{11}^2s^2 - \frac{5}{2}\tau_{1,5}\tau_{3,8}l_9^2l_{11}^2s^2 + \tau_{1,10}\tau_{3,8}l_9^2l_{11}^2s^2 + 2\tau_{2,5}\tau_{3,8}l_9^2l_{11}^2s^2 + 2\tau_{2,8}\tau_{3,8}l_9^2l_{11}^2s^2 - \\
& 2\tau_{2,10}\tau_{3,8}l_9^2l_{11}^2s^2 + \frac{5}{2}\tau_{1,5}\tau_{3,10}l_9^2l_{11}^2s^2 - 2\tau_{1,10}\tau_{3,10}l_9^2l_{11}^2s^2 - 2\tau_{2,5}\tau_{3,10}l_9^2l_{11}^2s^2 - \frac{5}{2}\tau_{2,8}\tau_{3,10}l_9^2l_{11}^2s^2 + \\
& \tau_{2,10}\tau_{3,10}l_9^2l_{11}^2s^2 - 3\tau_{3,8}\tau_{3,10}l_9^2l_{11}^2s^2 - 2\tau_{2,5}\tau_{3,16}l_9^2l_{11}^2s^2 - \tau_{2,8}\tau_{3,16}l_9^2l_{11}^2s^2 + \tau_{2,10}\tau_{3,16}l_9^2l_{11}^2s^2 - 7\tau_{3,8}\tau_{3,16}l_9^2l_{11}^2s^2 + \\
& 5\tau_{3,10}\tau_{3,16}l_9^2l_{11}^2s^2 - 2\tau_{4,9}^2l_7^2l_{12}^2s^2 + \tau_{4,13}^2l_7^2l_{12}^2s^2 - \frac{5}{2}\tau_{1,9}\tau_{4,9}l_7^2l_{12}^2s^2 - \frac{1}{2}\tau_{1,9}\tau_{4,13}l_7^2l_{12}^2s^2 - \tau_{4,9}\tau_{4,13}l_7^2l_{12}^2s^2 + \\
& \tau_{3,10}^2l_9^2l_{12}^2s^2 - 3\tau_{3,14}^2l_9^2l_{12}^2s^2 - 2\tau_{2,8}\tau_{3,8}l_9^2l_{12}^2s^2 + 2\tau_{2,8}\tau_{3,10}l_9^2l_{12}^2s^2 + \tau_{1,10}\tau_{3,14}l_9^2l_{12}^2s^2 + \tau_{2,10}\tau_{3,14}l_9^2l_{12}^2s^2 + \\
& 3\tau_{3,8}\tau_{3,14}l_9^2l_{12}^2s^2 + 6\tau_{3,8}^2l_{12}^2l_{17}^2s^2 + 3\tau_{3,10}^2l_{12}^2l_{17}^2s^2 + 3\tau_{3,15}^2l_{12}^2l_{17}^2s^2 + \tau_{3,16}^2l_{12}^2l_{17}^2s^2 - 2\tau_{1,10}\tau_{3,8}l_{12}^2l_{17}^2s^2 - \\
& 2\tau_{1,15}\tau_{3,8}l_{12}^2l_{17}^2s^2 - 2\tau_{1,16}\tau_{3,8}l_{12}^2l_{17}^2s^2 - 2\tau_{2,10}\tau_{3,8}l_{12}^2l_{17}^2s^2 - 2\tau_{2,15}\tau_{3,8}l_{12}^2l_{17}^2s^2 - 2\tau_{2,16}\tau_{3,8}l_{12}^2l_{17}^2s^2 + \\
& 2\tau_{1,10}\tau_{3,10}l_{12}^2l_{17}^2s^2 + 2\tau_{1,15}\tau_{3,10}l_{12}^2l_{17}^2s^2 + 2\tau_{1,16}\tau_{3,10}l_{12}^2l_{17}^2s^2 + 2\tau_{2,10}\tau_{3,10}l_{12}^2l_{17}^2s^2 + 2\tau_{2,15}\tau_{3,10}l_{12}^2l_{17}^2s^2 + \\
& 2\tau_{2,16}\tau_{3,10}l_{12}^2l_{17}^2s^2 - 8\tau_{3,8}\tau_{3,10}l_{12}^2l_{17}^2s^2 + 2\tau_{1,10}\tau_{3,15}l_{12}^2l_{17}^2s^2 + 2\tau_{1,15}\tau_{3,15}l_{12}^2l_{17}^2s^2 + 2\tau_{1,16}\tau_{3,15}l_{12}^2l_{17}^2s^2 + \\
& 2\tau_{2,10}\tau_{3,15}l_{12}^2l_{17}^2s^2 + 2\tau_{2,15}\tau_{3,15}l_{12}^2l_{17}^2s^2 + 2\tau_{2,16}\tau_{3,15}l_{12}^2l_{17}^2s^2 - 8\tau_{3,8}\tau_{3,15}l_{12}^2l_{17}^2s^2 + 6\tau_{3,10}\tau_{3,15}l_{12}^2l_{17}^2s^2 + \\
& \tau_{1,10}\tau_{3,16}l_{12}^2l_{17}^2s^2 + \tau_{1,15}\tau_{3,16}l_{12}^2l_{17}^2s^2 + \tau_{1,16}\tau_{3,16}l_{12}^2l_{17}^2s^2 + \tau_{2,10}\tau_{3,16}l_{12}^2l_{17}^2s^2 + \tau_{2,15}\tau_{3,16}l_{12}^2l_{17}^2s^2 + \tau_{2,16}\tau_{3,16}l_{12}^2l_{17}^2s^2 - \\
& 4\tau_{3,8}\tau_{3,16}l_{12}^2l_{17}^2s^2 + 3\tau_{3,10}\tau_{3,16}l_{12}^2l_{17}^2s^2 + 3\tau_{3,15}\tau_{3,16}l_{12}^2l_{17}^2s^2 - \frac{3}{8}(s^2+t^2-u^2)l_5^2l_7^2l_9^2s - \frac{1}{8}(s^2-t^2+u^2)l_6^2l_7^2l_{11}^2s + \\
& \frac{19}{64}(s^2-t^2+u^2)l_7^2l_8^2l_{11}^2s + \frac{17}{16}(s^2+t^2-u^2)l_7^2l_8^2l_{12}^2s - \frac{5}{16}(s^2+t^2-u^2)l_5^2l_9^2l_{12}^2s + \frac{1}{16}(s^2-t^2+u^2)l_5^2l_9^2l_{12}^2s +
\end{aligned}$$

$$\begin{aligned}
& \frac{13}{8} (s^2 + t^2 - u^2) l_7^2 l_9^2 l_{12}^2 s + \frac{13}{8} (s^2 - t^2 + u^2) l_7^2 l_9^2 l_{12}^2 s - \frac{1}{4} (s^2 - t^2 + u^2) l_5^2 l_9^2 l_{15}^2 s + \frac{3}{4} (s^2 + t^2 - u^2) l_9^2 l_{12}^2 l_{15}^2 s - \\
& \frac{3}{4} (s^2 - t^2 + u^2) l_9^2 l_{12}^2 l_{15}^2 s - \frac{5}{64} (s^2 + t^2 - u^2) l_9^2 l_{13}^2 l_{15}^2 s + \frac{11}{64} (s^2 - t^2 + u^2) l_9^2 l_{13}^2 l_{15}^2 s + \frac{3}{16} (s^2 + t^2 - u^2) l_9^2 l_{12}^2 l_{17}^2 s + \\
& \frac{5}{16} (s^2 - t^2 + u^2) l_9^2 l_{12}^2 l_{17}^2 s - \frac{1}{2} (t^2 + u^2) \tau_{1,11}^2 l_7^2 l_8^2 - \frac{1}{2} (t^2 + u^2) \tau_{2,11}^2 l_7^2 l_8^2 + t^2 \tau_{4,13}^2 l_7^2 l_8^2 + u^2 \tau_{4,13}^2 l_7^2 l_8^2 - \\
& (t^2 + u^2) \tau_{1,11} \tau_{2,11} l_7^2 l_8^2 - t^2 \tau_{1,8}^2 l_7^2 l_9^2 + u^2 \tau_{1,12}^2 l_7^2 l_9^2 + 3 t^2 \tau_{3,5}^2 l_7^2 l_9^2 + u^2 \tau_{3,5}^2 l_7^2 l_9^2 - 7 t^2 \tau_{3,8}^2 l_7^2 l_9^2 + u^2 \tau_{3,8}^2 l_7^2 l_9^2 - \\
& 3 t^2 \tau_{3,12}^2 l_7^2 l_9^2 + 3 u^2 \tau_{3,12}^2 l_7^2 l_9^2 - u^2 \tau_{1,5} \tau_{1,8} l_7^2 l_9^2 + u^2 \tau_{1,5} \tau_{1,12} l_7^2 l_9^2 - u^2 \tau_{1,8} \tau_{1,12} l_7^2 l_9^2 + 2 t^2 \tau_{1,5} \tau_{3,5} l_7^2 l_9^2 + u^2 \tau_{1,8} \tau_{3,5} l_7^2 l_9^2 + \\
& t^2 \tau_{1,12} \tau_{3,5} l_7^2 l_9^2 - 3 t^2 \tau_{1,8} \tau_{3,8} l_7^2 l_9^2 - 2 u^2 \tau_{1,8} \tau_{3,8} l_7^2 l_9^2 - 2 t^2 \tau_{1,12} \tau_{3,8} l_7^2 l_9^2 + 2 u^2 \tau_{1,12} \tau_{3,8} l_7^2 l_9^2 + 4 t^2 \tau_{3,5} \tau_{3,8} l_7^2 l_9^2 - \\
& 2 u^2 \tau_{3,5} \tau_{3,8} l_7^2 l_9^2 + 2 t^2 \tau_{1,8} \tau_{3,12} l_7^2 l_9^2 + u^2 \tau_{1,8} \tau_{3,12} l_7^2 l_9^2 + 2 t^2 \tau_{1,12} \tau_{3,12} l_7^2 l_9^2 - u^2 \tau_{1,12} \tau_{3,12} l_7^2 l_9^2 - 4 t^2 \tau_{3,5} \tau_{3,12} l_7^2 l_9^2 + \\
& 2 u^2 \tau_{3,5} \tau_{3,12} l_7^2 l_9^2 + 10 t^2 \tau_{3,8} \tau_{3,12} l_7^2 l_9^2 - 4 u^2 \tau_{3,8} \tau_{3,12} l_7^2 l_9^2 - u^2 \tau_{1,8} \tau_{4,5} l_7^2 l_9^2 + u^2 \tau_{1,12} \tau_{4,5} l_7^2 l_9^2 - t^2 \tau_{3,8} \tau_{4,5} l_7^2 l_9^2 - \\
& u^2 \tau_{3,8} \tau_{4,5} l_7^2 l_9^2 + t^2 \tau_{3,12} \tau_{4,5} l_7^2 l_9^2 + u^2 \tau_{3,12} \tau_{4,5} l_7^2 l_9^2 - 2 u^2 \tau_{1,5} \tau_{4,8} l_7^2 l_9^2 - u^2 \tau_{1,8} \tau_{4,8} l_7^2 l_9^2 - 2 u^2 \tau_{1,12} \tau_{4,8} l_7^2 l_9^2 + \\
& 2 u^2 \tau_{3,5} \tau_{4,8} l_7^2 l_9^2 - 4 u^2 \tau_{3,8} \tau_{4,8} l_7^2 l_9^2 + 2 u^2 \tau_{3,12} \tau_{4,8} l_7^2 l_9^2 - 2 u^2 \tau_{4,5} \tau_{4,8} l_7^2 l_9^2 + \frac{1}{2} t^3 l_5^2 l_7^2 l_9^2 + \frac{3}{8} u (-s^2 + t^2 + u^2) l_5^2 l_7^2 l_9^2 - \\
& \frac{1}{2} t^3 l_6^2 l_7^2 l_9^2 + \frac{1}{4} t (s^2 + t^2 - u^2) l_6^2 l_7^2 l_9^2 - \frac{1}{4} u (s^2 - t^2 + u^2) l_6^2 l_7^2 l_9^2 + t^2 \tau_{2,12}^2 l_7^2 l_{11}^2 + 3 u^2 \tau_{2,12}^2 l_7^2 l_{11}^2 + t^2 \tau_{3,5}^2 l_7^2 l_{11}^2 + \\
& u^2 \tau_{3,5}^2 l_7^2 l_{11}^2 - 2 t^2 \tau_{3,8}^2 l_7^2 l_{11}^2 + 4 u^2 \tau_{3,8}^2 l_7^2 l_{11}^2 - t^2 \tau_{3,12}^2 l_7^2 l_{11}^2 + u^2 \tau_{3,12}^2 l_7^2 l_{11}^2 + 2 t^2 \tau_{4,8}^2 l_7^2 l_{11}^2 - u^2 \tau_{4,12}^2 l_7^2 l_{11}^2 - \\
& t^2 \tau_{2,5} \tau_{2,12} l_7^2 l_{11}^2 + u^2 \tau_{2,5} \tau_{2,12} l_7^2 l_{11}^2 - t^2 \tau_{2,5} \tau_{3,5} l_7^2 l_{11}^2 + u^2 \tau_{2,5} \tau_{3,5} l_7^2 l_{11}^2 + 6 u^2 \tau_{2,12} \tau_{3,5} l_7^2 l_{11}^2 - t^2 \tau_{2,5} \tau_{3,8} l_7^2 l_{11}^2 + \\
& u^2 \tau_{2,5} \tau_{3,8} l_7^2 l_{11}^2 - 5 t^2 \tau_{2,12} \tau_{3,8} l_7^2 l_{11}^2 - 3 u^2 \tau_{2,12} \tau_{3,8} l_7^2 l_{11}^2 - t^2 \tau_{3,5} \tau_{3,8} l_7^2 l_{11}^2 + 3 u^2 \tau_{3,5} \tau_{3,8} l_7^2 l_{11}^2 + t^2 \tau_{2,5} \tau_{3,12} l_7^2 l_{11}^2 - \\
& u^2 \tau_{2,5} \tau_{3,12} l_7^2 l_{11}^2 + 2 t^2 \tau_{2,12} \tau_{3,12} l_7^2 l_{11}^2 + 2 u^2 \tau_{2,12} \tau_{3,12} l_7^2 l_{11}^2 + 2 t^2 \tau_{3,5} \tau_{3,12} l_7^2 l_{11}^2 - 4 u^2 \tau_{3,5} \tau_{3,12} l_7^2 l_{11}^2 + 3 t^2 \tau_{3,8} \tau_{3,12} l_7^2 l_{11}^2 - \\
& 3 u^2 \tau_{3,8} \tau_{3,12} l_7^2 l_{11}^2 - 2 u^2 \tau_{3,5} \tau_{4,5} l_7^2 l_{11}^2 - t^2 \tau_{3,8} \tau_{4,5} l_7^2 l_{11}^2 + 3 u^2 \tau_{3,8} \tau_{4,5} l_7^2 l_{11}^2 + t^2 \tau_{3,12} \tau_{4,5} l_7^2 l_{11}^2 - 3 u^2 \tau_{3,12} \tau_{4,5} l_7^2 l_{11}^2 + \\
& t^2 \tau_{2,5} \tau_{4,8} l_7^2 l_{11}^2 - u^2 \tau_{2,5} \tau_{4,8} l_7^2 l_{11}^2 - 4 t^2 \tau_{2,12} \tau_{4,8} l_7^2 l_{11}^2 - 2 u^2 \tau_{2,12} \tau_{4,8} l_7^2 l_{11}^2 + 2 u^2 \tau_{3,5} \tau_{4,8} l_7^2 l_{11}^2 + 4 u^2 \tau_{3,8} \tau_{4,8} l_7^2 l_{11}^2 + \\
& 2 t^2 \tau_{3,12} \tau_{4,8} l_7^2 l_{11}^2 - 2 u^2 \tau_{3,12} \tau_{4,8} l_7^2 l_{11}^2 - t^2 \tau_{4,5} \tau_{4,8} l_7^2 l_{11}^2 + 3 u^2 \tau_{4,5} \tau_{4,8} l_7^2 l_{11}^2 - t^2 \tau_{2,5} \tau_{4,12} l_7^2 l_{11}^2 + u^2 \tau_{2,5} \tau_{4,12} l_7^2 l_{11}^2 - \\
& t^2 \tau_{2,12} \tau_{4,12} l_7^2 l_{11}^2 + 4 u^2 \tau_{2,12} \tau_{4,12} l_7^2 l_{11}^2 + t^2 \tau_{3,5} \tau_{4,12} l_7^2 l_{11}^2 - 3 u^2 \tau_{3,5} \tau_{4,12} l_7^2 l_{11}^2 + t^2 \tau_{3,8} \tau_{4,12} l_7^2 l_{11}^2 + u^2 \tau_{3,8} \tau_{4,12} l_7^2 l_{11}^2 - \\
& t^2 \tau_{3,12} \tau_{4,12} l_7^2 l_{11}^2 + t^2 \tau_{4,5} \tau_{4,12} l_7^2 l_{11}^2 - 3 u^2 \tau_{4,5} \tau_{4,12} l_7^2 l_{11}^2 + t^2 \tau_{4,8} \tau_{4,12} l_7^2 l_{11}^2 + u^2 \tau_{4,8} \tau_{4,12} l_7^2 l_{11}^2 + \frac{1}{4} u^3 l_6^2 l_7^2 l_{11}^2 + \\
& \frac{1}{8} t (-s^2 + t^2 + u^2) l_6^2 l_7^2 l_{11}^2 + \frac{19}{16} t^3 l_7^2 l_8^2 l_{11}^2 + \frac{19}{32} u^3 l_7^2 l_8^2 l_{11}^2 - \frac{19}{64} t (s^2 + t^2 - u^2) l_7^2 l_8^2 l_{11}^2 + \frac{19}{64} u (s^2 - t^2 + u^2) l_7^2 l_8^2 l_{11}^2 - \\
& \frac{19}{64} t (-s^2 + t^2 + u^2) l_7^2 l_8^2 l_{11}^2 - \frac{5}{2} t^2 \tau_{1,10}^2 l_9^2 l_{11}^2 - u^2 \tau_{1,10}^2 l_9^2 l_{11}^2 - t^2 \tau_{2,10}^2 l_9^2 l_{11}^2 - \frac{1}{2} u^2 \tau_{2,10}^2 l_9^2 l_{11}^2 + 2 t^2 \tau_{3,8}^2 l_9^2 l_{11}^2 - \\
& 2 u^2 \tau_{3,8}^2 l_9^2 l_{11}^2 + \frac{1}{2} t^2 \tau_{3,16}^2 l_9^2 l_{11}^2 + 2 t^2 \tau_{1,5} \tau_{1,10} l_9^2 l_{11}^2 - u^2 \tau_{1,5} \tau_{1,10} l_9^2 l_{11}^2 + 2 t^2 \tau_{1,10} \tau_{2,5} l_9^2 l_{11}^2 - u^2 \tau_{1,10} \tau_{2,5} l_9^2 l_{11}^2 -
\end{aligned}$$

$$\begin{aligned}
& \frac{3}{2} t^2 \tau_{1,5} \tau_{2,8} l_9^2 l_{11}^2 + u^2 \tau_{1,5} \tau_{2,8} l_9^2 l_{11}^2 + t^2 \tau_{1,10} \tau_{2,8} l_9^2 l_{11}^2 - \frac{3}{2} t^2 \tau_{2,5} \tau_{2,8} l_9^2 l_{11}^2 + u^2 \tau_{2,5} \tau_{2,8} l_9^2 l_{11}^2 + \frac{3}{2} t^2 \tau_{1,5} \tau_{2,10} l_9^2 l_{11}^2 - \\
& u^2 \tau_{1,5} \tau_{2,10} l_9^2 l_{11}^2 - 3 t^2 \tau_{1,10} \tau_{2,10} l_9^2 l_{11}^2 - \frac{3}{2} u^2 \tau_{1,10} \tau_{2,10} l_9^2 l_{11}^2 + \frac{3}{2} t^2 \tau_{2,5} \tau_{2,10} l_9^2 l_{11}^2 - u^2 \tau_{2,5} \tau_{2,10} l_9^2 l_{11}^2 + t^2 \tau_{2,8} \tau_{2,10} l_9^2 l_{11}^2 - \\
& \frac{1}{2} t^2 \tau_{1,5} \tau_{3,8} l_9^2 l_{11}^2 + \frac{1}{2} u^2 \tau_{1,5} \tau_{3,8} l_9^2 l_{11}^2 - 4 u^2 \tau_{1,10} \tau_{3,8} l_9^2 l_{11}^2 - t^2 \tau_{2,8} \tau_{3,8} l_9^2 l_{11}^2 - u^2 \tau_{2,8} \tau_{3,8} l_9^2 l_{11}^2 + t^2 \tau_{2,10} \tau_{3,8} l_9^2 l_{11}^2 - \\
& 2 u^2 \tau_{2,10} \tau_{3,8} l_9^2 l_{11}^2 + \frac{1}{2} t^2 \tau_{1,5} \tau_{3,10} l_9^2 l_{11}^2 - \frac{1}{2} u^2 \tau_{1,5} \tau_{3,10} l_9^2 l_{11}^2 - 2 t^2 \tau_{1,10} \tau_{3,10} l_9^2 l_{11}^2 + 3 u^2 \tau_{1,10} \tau_{3,10} l_9^2 l_{11}^2 + \\
& 2 t^2 \tau_{2,8} \tau_{3,10} l_9^2 l_{11}^2 + u^2 \tau_{2,8} \tau_{3,10} l_9^2 l_{11}^2 - 2 t^2 \tau_{2,10} \tau_{3,10} l_9^2 l_{11}^2 + \frac{3}{2} u^2 \tau_{2,10} \tau_{3,10} l_9^2 l_{11}^2 - 2 t^2 \tau_{3,8} \tau_{3,10} l_9^2 l_{11}^2 + \\
& 2 u^2 \tau_{3,8} \tau_{3,10} l_9^2 l_{11}^2 + t^2 \tau_{1,10} \tau_{3,16} l_9^2 l_{11}^2 - \frac{1}{2} t^2 \tau_{2,8} \tau_{3,16} l_9^2 l_{11}^2 + \frac{1}{2} t^2 \tau_{2,10} \tau_{3,16} l_9^2 l_{11}^2 - t^2 \tau_{3,8} \tau_{3,16} l_9^2 l_{11}^2 + u^2 \tau_{3,8} \tau_{3,16} l_9^2 l_{11}^2 + \\
& t^2 \tau_{3,10} \tau_{3,16} l_9^2 l_{11}^2 - u^2 \tau_{3,10} \tau_{3,16} l_9^2 l_{11}^2 - \frac{1}{2} t^2 \tau_{1,9}^2 l_7^2 l_{12}^2 - 2 u^2 \tau_{1,9}^2 l_7^2 l_{12}^2 - \frac{1}{2} t^2 \tau_{4,9}^2 l_7^2 l_{12}^2 - t^2 \tau_{4,13}^2 l_7^2 l_{12}^2 + \\
& u^2 \tau_{4,13}^2 l_7^2 l_{12}^2 + 2 t^2 \tau_{1,9} \tau_{4,9} l_7^2 l_{12}^2 - \frac{5}{2} u^2 \tau_{1,9} \tau_{4,9} l_7^2 l_{12}^2 - 2 u^2 \tau_{1,9} \tau_{4,13} l_7^2 l_{12}^2 - u^2 \tau_{4,9} \tau_{4,13} l_7^2 l_{12}^2 + \frac{17}{8} t^3 l_7^2 l_8^2 l_{12}^2 + \\
& \frac{17}{4} u^3 l_7^2 l_8^2 l_{12}^2 + \frac{17}{16} t (s^2 + t^2 - u^2) l_7^2 l_8^2 l_{12}^2 - \frac{17}{16} u (s^2 - t^2 + u^2) l_7^2 l_8^2 l_{12}^2 - \frac{17}{16} u (-s^2 + t^2 + u^2) l_7^2 l_8^2 l_{12}^2 - t^2 \tau_{2,8}^2 l_9^2 l_{12}^2 - \\
& 2 t^2 \tau_{3,8}^2 l_9^2 l_{12}^2 + u^2 \tau_{3,8}^2 l_9^2 l_{12}^2 - t^2 \tau_{3,10}^2 l_9^2 l_{12}^2 - u^2 \tau_{3,10}^2 l_9^2 l_{12}^2 + t^2 \tau_{3,14}^2 l_9^2 l_{12}^2 - u^2 \tau_{3,14}^2 l_9^2 l_{12}^2 + 2 t^2 \tau_{1,10} \tau_{2,8} l_9^2 l_{12}^2 + \\
& t^2 \tau_{2,8} \tau_{2,10} l_9^2 l_{12}^2 + t^2 \tau_{2,8} \tau_{3,8} l_9^2 l_{12}^2 + 2 u^2 \tau_{2,8} \tau_{3,8} l_9^2 l_{12}^2 - t^2 \tau_{2,10} \tau_{3,8} l_9^2 l_{12}^2 + 2 t^2 \tau_{1,10} \tau_{3,10} l_9^2 l_{12}^2 - 2 t^2 \tau_{2,8} \tau_{3,10} l_9^2 l_{12}^2 - \\
& 2 u^2 \tau_{2,8} \tau_{3,10} l_9^2 l_{12}^2 + 2 t^2 \tau_{2,10} \tau_{3,10} l_9^2 l_{12}^2 + 4 t^2 \tau_{3,8} \tau_{3,10} l_9^2 l_{12}^2 - t^2 \tau_{1,10} \tau_{3,14} l_9^2 l_{12}^2 - u^2 \tau_{1,10} \tau_{3,14} l_9^2 l_{12}^2 - t^2 \tau_{2,8} \tau_{3,14} l_9^2 l_{12}^2 + \\
& 3 u^2 \tau_{2,8} \tau_{3,14} l_9^2 l_{12}^2 - t^2 \tau_{2,10} \tau_{3,14} l_9^2 l_{12}^2 + t^2 \tau_{3,8} \tau_{3,14} l_9^2 l_{12}^2 - u^2 \tau_{3,8} \tau_{3,14} l_9^2 l_{12}^2 - 2 t^2 \tau_{3,10} \tau_{3,14} l_9^2 l_{12}^2 + 2 u^2 \tau_{3,10} \tau_{3,14} l_9^2 l_{12}^2 + \\
& \frac{7}{8} t^3 l_5^2 l_9^2 l_{12}^2 + \frac{1}{8} u^3 l_5^2 l_9^2 l_{12}^2 - \frac{1}{16} t (-s^2 + t^2 + u^2) l_5^2 l_9^2 l_{12}^2 + \frac{5}{16} u (-s^2 + t^2 + u^2) l_5^2 l_9^2 l_{12}^2 - \frac{1}{4} t^3 l_7^2 l_9^2 l_{12}^2 - \\
& \frac{13}{4} u^3 l_7^2 l_9^2 l_{12}^2 - \frac{13}{8} t (-s^2 + t^2 + u^2) l_7^2 l_9^2 l_{12}^2 - \frac{13}{8} u (-s^2 + t^2 + u^2) l_7^2 l_9^2 l_{12}^2 + \tau_{1,13}^2 l_7^2 ((t^2 + u^2) l_8^2 - 2 s u l_{12}^2) + \\
& \tau_{2,13}^2 l_7^2 ((t^2 + u^2) l_8^2 + (s^2 - 4 t^2 + u^2) l_{12}^2) + \tau_{2,13} (\tau_{4,13} l_7^2 ((s^2 + 2 (t^2 + u^2)) l_8^2 + (2 s^2 - 3 t^2 + 2 u^2) l_{12}^2) - ((s^2 + 2 u^2) \tau_{1,9} l_7^2 + \\
& (2 s^2 + u^2) \tau_{4,9} l_7^2 - (2 \tau_{1,10} t^2 - (t^2 + u^2) \tau_{2,8} + (s^2 + t^2) \tau_{2,10} + 2 s ((t + 2 u) \tau_{3,8} + s (\tau_{3,10} - \tau_{3,14}))) l_9^2) l_{12}^2) - \\
& \frac{1}{2} \tau_{1,13} ((2 (s^2 + u^2) \tau_{1,9} l_7^2 + (4 s^2 + u^2) \tau_{4,9} l_7^2 + 2 (-2 \tau_{1,10} t^2 + (t^2 + u^2) \tau_{2,8} + u ((2 t + u) \tau_{2,10} - 2 s \tau_{3,10})) l_9^2) l_{12}^2 + \\
& \tau_{2,13} l_7^2 ((s^2 - 4 (t^2 + u^2)) l_8^2 - 2 (2 s^2 - 3 t^2 + 2 u^2) l_{12}^2) - \tau_{4,13} l_7^2 (2 (s^2 + 2 (t^2 + u^2)) l_8^2 + (4 s^2 - 3 t^2 + 4 u^2) l_{12}^2)) +
\end{aligned}$$



$$\begin{aligned}
& t^3 l_5^2 l_9^2 l_{15}^2 + \frac{1}{2} u^3 l_5^2 l_9^2 l_{15}^2 - \frac{1}{2} u (s^2 - t^2 + u^2) l_5^2 l_9^2 l_{15}^2 - \frac{1}{4} t (-s^2 + t^2 + u^2) l_5^2 l_9^2 l_{15}^2 - \frac{3}{2} t^3 l_9^2 l_{12}^2 l_{15}^2 + \frac{3}{2} u^3 l_9^2 l_{12}^2 l_{15}^2 + \\
& \frac{3}{4} t (-s^2 + t^2 + u^2) l_9^2 l_{12}^2 l_{15}^2 - \frac{3}{4} u (-s^2 + t^2 + u^2) l_9^2 l_{12}^2 l_{15}^2 + \frac{5}{32} t^3 l_9^2 l_{13}^2 l_{15}^2 - \frac{11}{32} u^3 l_9^2 l_{13}^2 l_{15}^2 - \frac{11}{64} t (-s^2 + t^2 + u^2) l_9^2 l_{13}^2 l_{15}^2 + \\
& \frac{5}{64} u (-s^2 + t^2 + u^2) l_9^2 l_{13}^2 l_{15}^2 - \frac{3}{8} t^3 l_9^2 l_{12}^2 l_{17}^2 + \frac{3}{8} u^3 l_9^2 l_{12}^2 l_{17}^2 - \frac{5}{16} t (-s^2 + t^2 + u^2) l_9^2 l_{12}^2 l_{17}^2 - \frac{3}{16} u (-s^2 + t^2 + u^2) l_9^2 l_{12}^2 l_{17}^2
\end{aligned}$$

■  $N_{23}^{(7)}$

$$\frac{1}{48}$$

$$\begin{aligned}
& ((174 \tau_{1,15} l_7^2 l_8^2 l_{11}^2 + 312 \tau_{1,16} l_7^2 l_8^2 l_{11}^2 + 189 \tau_{2,10} l_7^2 l_8^2 l_{11}^2 - 6 \tau_{2,13} l_7^2 l_8^2 l_{11}^2 + 201 \tau_{2,15} l_7^2 l_8^2 l_{11}^2 + 339 \tau_{2,16} l_7^2 l_8^2 l_{11}^2 + 132 \tau_{4,13} l_7^2 l_8^2 l_{11}^2 + \\
& 138 \tau_{4,16} l_7^2 l_8^2 l_{11}^2 + 208 \tau_{2,9} l_7^2 l_8^2 l_{12}^2 + 24 \tau_{2,13} l_7^2 l_8^2 l_{12}^2 - 64 \tau_{3,9} l_7^2 l_8^2 l_{12}^2 - 176 \tau_{3,13} l_7^2 l_8^2 l_{12}^2 + \\
& 208 \tau_{4,9} l_7^2 l_8^2 l_{12}^2 + 24 \tau_{4,13} l_7^2 l_8^2 l_{12}^2 - 48 \tau_{1,5} l_7^2 l_9^2 l_{12}^2 - 216 \tau_{1,8} l_7^2 l_9^2 l_{12}^2 + 240 \tau_{1,11} l_7^2 l_9^2 l_{12}^2 - 192 \tau_{3,5} l_7^2 l_9^2 l_{12}^2 - \\
& 360 \tau_{3,8} l_7^2 l_9^2 l_{12}^2 + 480 \tau_{3,11} l_7^2 l_9^2 l_{12}^2 - 192 \tau_{4,5} l_7^2 l_9^2 l_{12}^2 - 408 \tau_{4,8} l_7^2 l_9^2 l_{12}^2 + 120 \tau_{4,11} l_7^2 l_9^2 l_{12}^2 + 336 \tau_{3,7} l_9^2 l_{12}^2 l_{15}^2 + \\
& 192 \tau_{3,10} l_9^2 l_{12}^2 l_{15}^2 + 48 \tau_{3,13} l_9^2 l_{12}^2 l_{15}^2 + 48 \tau_{3,14} l_9^2 l_{12}^2 l_{15}^2 + 48 \tau_{4,7} l_9^2 l_{12}^2 l_{15}^2 - 96 \tau_{4,13} l_9^2 l_{12}^2 l_{15}^2 - \\
& 24 ((\tau_{1,16} + 2 \tau_{2,13} + \tau_{2,16} + 2 \tau_{4,13} + \tau_{4,16}) l_7^2 l_8^2 + (2 \tau_{2,10} + 2 \tau_{2,13} - \tau_{3,8} + 2 \tau_{3,10}) l_9^2 l_{12}^2) l_{17}^2 t^2 + \\
& (s^2 - t^2 - u^2) (75 \tau_{1,15} l_7^2 l_8^2 l_{11}^2 + 159 \tau_{1,16} l_7^2 l_8^2 l_{11}^2 - 15 \tau_{2,10} l_7^2 l_8^2 l_{11}^2 + 210 \tau_{2,13} l_7^2 l_8^2 l_{11}^2 + 75 \tau_{2,15} l_7^2 l_8^2 l_{11}^2 + \\
& 159 \tau_{2,16} l_7^2 l_8^2 l_{11}^2 + 180 \tau_{4,13} l_7^2 l_8^2 l_{11}^2 + 84 \tau_{4,16} l_7^2 l_8^2 l_{11}^2 - 32 \tau_{3,9} l_7^2 l_8^2 l_{12}^2 - 88 \tau_{3,13} l_7^2 l_8^2 l_{12}^2 + 208 \tau_{4,9} l_7^2 l_8^2 l_{12}^2 + \\
& 24 \tau_{4,13} l_7^2 l_8^2 l_{12}^2 + 72 \tau_{1,5} l_7^2 l_9^2 l_{12}^2 - 48 \tau_{1,8} l_7^2 l_9^2 l_{12}^2 - 48 \tau_{3,5} l_7^2 l_9^2 l_{12}^2 + 120 \tau_{3,8} l_7^2 l_9^2 l_{12}^2 - 72 \tau_{4,5} l_7^2 l_9^2 l_{12}^2 - \\
& 240 \tau_{4,8} l_7^2 l_9^2 l_{12}^2 - 120 \tau_{4,11} l_7^2 l_9^2 l_{12}^2 + 144 \tau_{3,7} l_9^2 l_{12}^2 l_{15}^2 + 48 \tau_{3,10} l_9^2 l_{12}^2 l_{15}^2 + 48 \tau_{3,13} l_9^2 l_{12}^2 l_{15}^2 + 144 \tau_{3,14} l_9^2 l_{12}^2 l_{15}^2 + \\
& 48 \tau_{4,10} l_9^2 l_{12}^2 l_{15}^2 - 96 \tau_{4,13} l_9^2 l_{12}^2 l_{15}^2 - 24 (2 \tau_{2,8} - \tau_{2,10} + 3 \tau_{2,13} - 3 \tau_{3,8} + \tau_{3,10} + 2 \tau_{3,13} + 4 \tau_{3,14}) l_9^2 l_{12}^2 l_{17}^2) + \\
& 3 \tau_{1,10} ((-5 s^2 + 35 t^2 + 68 u^2) l_7^2 l_8^2 l_{11}^2 + 16 l_9^2 l_{12}^2 (l_{15}^2 u^2 + t (u - t) l_{17}^2)) + \\
& 6 \tau_{1,13} (4 l_9^2 l_{12}^2 (u^2 l_{17}^2 - 4 s^2 l_{15}^2) + l_7^2 l_8^2 ((35 s^2 - 21 t^2 - 36 u^2) l_{11}^2 - 8 (t^2 + u^2) l_{17}^2)) + \\
& u^2 (201 \tau_{1,15} l_7^2 l_8^2 l_{11}^2 + 3 \tau_{1,16} l_7^2 l_8^2 (113 l_{11}^2 - 8 l_{17}^2) + \\
& 2 (45 \tau_{2,10} l_7^2 l_8^2 l_{11}^2 + 42 \tau_{2,13} l_7^2 l_8^2 l_{11}^2 + 87 \tau_{2,15} l_7^2 l_8^2 l_{11}^2 + 156 \tau_{2,16} l_7^2 l_8^2 l_{11}^2 + 66 \tau_{4,13} l_7^2 l_8^2 l_{11}^2 + 69 \tau_{4,16} l_7^2 l_8^2 l_{11}^2 - \\
& 104 \tau_{2,9} l_7^2 l_8^2 l_{12}^2 - 12 \tau_{2,13} l_7^2 l_8^2 l_{12}^2 - 136 \tau_{3,9} l_7^2 l_8^2 l_{12}^2 - 100 \tau_{3,13} l_7^2 l_8^2 l_{12}^2 - 144 \tau_{1,8} l_7^2 l_9^2 l_{12}^2 - 60 \tau_{1,11} l_7^2 l_9^2 l_{12}^2 - \\
& 48 \tau_{3,5} l_7^2 l_9^2 l_{12}^2 + 120 \tau_{3,8} l_7^2 l_9^2 l_{12}^2 - 144 \tau_{4,8} l_7^2 l_9^2 l_{12}^2 - 60 \tau_{4,11} l_7^2 l_9^2 l_{12}^2 - 24 \tau_{3,7} l_9^2 l_{12}^2 l_{15}^2 - 24 \tau_{3,10} l_9^2 l_{12}^2 l_{15}^2 + \\
& 48 \tau_{3,13} l_9^2 l_{12}^2 l_{15}^2 + 96 \tau_{3,14} l_9^2 l_{12}^2 l_{15}^2 - 72 \tau_{4,7} l_9^2 l_{12}^2 l_{15}^2 + 24 \tau_{4,10} l_9^2 l_{12}^2 l_{15}^2 - 48 \tau_{4,13} l_9^2 l_{12}^2 l_{15}^2 - 12 \\
& ((2 \tau_{2,13} + \tau_{2,16} + 2 \tau_{4,13} + \tau_{4,16}) l_7^2 l_8^2 - (4 \tau_{2,8} + \tau_{2,10} - 3 \tau_{2,13} + 3 \tau_{3,8} + 2 \tau_{3,10} - 5 \tau_{3,13} - 4 \tau_{3,14}) l_9^2 l_{12}^2) l_{17}^2)))
\end{aligned}$$

■  $N_{23}^{(8)}$

$$\frac{1}{4} l_7^2 l_9^2 l_{11}^2 l_{17}^2 (-4 s^2 + t^2 + u^2)$$
