# Supplementary material for: The Ultraviolet Behavior of N=8 Supergravity at Four Loops
Source: arXiv:0905.2326 ancillary file (2012-01-08)
Supplement: Supplementary file 19 [file SUGRA25.pdf]

## Integral 25: $\mathcal{I}_{25}$

$\mathcal{N} = 8$  four-point four-loop amplitude.

### ■ 2D plot of graph associated with $\mathcal{I}_{25}$

This fixes the labelling associated with the numerator expressions given below.

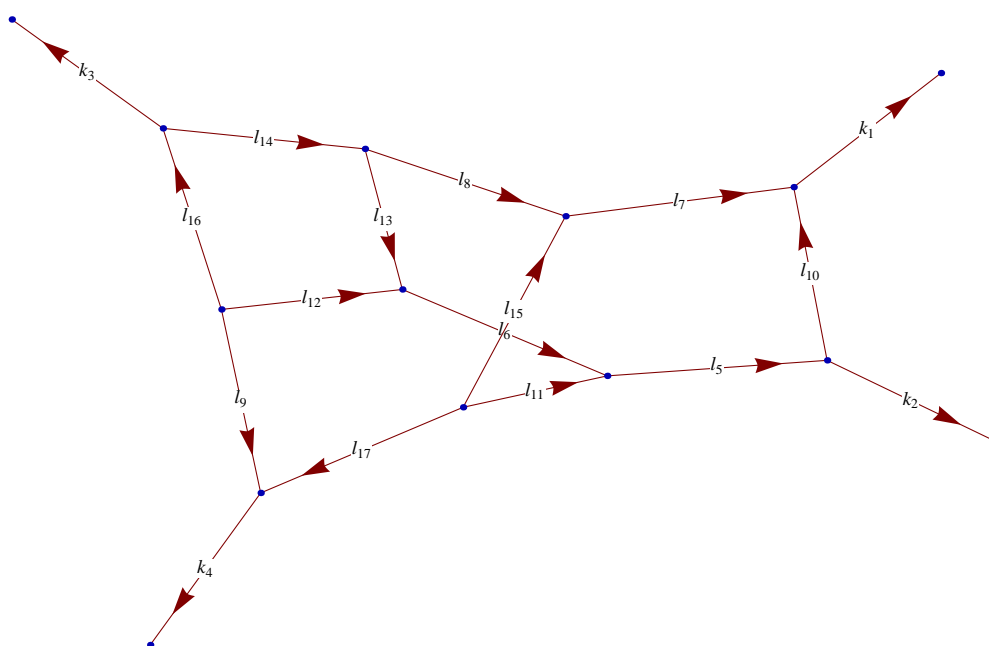

When using MathPlayer, by clicking three times (holding the click on the third click) directly on a vertex, one is able to move that vertex around, and its associated edges follow elastically. This functionality is absent when viewing as a pdf.

*Note: propagators for certain graphs were relabeled in the manuscript due to size constraints. The labels given in `aux/rawData/Neq8FourLoops.m` should be used for verification purposes.*

### ■ 3D plot of graph associated with $\mathcal{I}_{25}$

3D PLOT UNAVAILABLE FOR PDF. Please see .nb version for the 3D figure.

When using MathPlayer, by clicking anywhere in the image and dragging one should be able to rotate this 3D image. By holding (ALT) or (COMMAND) while clicking and moving the mouse up/down one should be able to zoom in/out. This functionality is absent when viewing as a pdf.

### "Vertex Form" of graph associated with $I_{25}$

This function returns the graph associated with the integral object in a vertex representation. This can be used as a way of specifying the topology of a graph using trivalent (cubic) vertices,  $\text{gVertex}[p_a, p_b, p_c]$ , where  $\{p_a, p_b, p_c\}$  are momenta labeling the propagators (edges) of the graph, and is understood that the edge labelled by  $p_a$  flows into the edge labelled by  $-p_a$ . Additionally, each vertex represents the manifest conservation of ( $D$  - dimensional) momenta :

$$\text{gVertex}[\{p_1, p_2, p_3\}] \iff (p_1 + p_2 + p_3 = 0)$$

$$\{\text{gVertex}(\{k_1, -l_{10}, -l_7\}), \text{gVertex}(\{k_2, -l_5, l_{10}\}), \text{gVertex}(\{k_3, l_{14}, -l_{16}\}), \text{gVertex}(\{k_4, -l_{17}, -l_9\}), \text{gVertex}(\{l_5, -l_{11}, -l_6\}), \\ \text{gVertex}(\{l_6, -l_{12}, -l_{13}\}), \text{gVertex}(\{l_7, -l_8, -l_{15}\}), \text{gVertex}(\{l_8, l_{13}, -l_{14}\}), \text{gVertex}(\{l_9, l_{16}, l_{12}\}), \text{gVertex}(\{l_{11}, l_{15}, l_{17}\})\}$$

### ■ Numerator expression for integral 25:

The following notation is used:  $\tau_{i,j} \equiv \begin{cases} 2 k_i \cdot l_j & \text{if } i \leq 4, j > 4 \\ 2 l_i \cdot l_j & \text{if } i, j > 4 \end{cases}$ .

$$s \equiv 2 k_1 \cdot k_2 = 2 k_3 \cdot k_4$$

We use  $s, t, u$  to represent the traditional Mandelstam variables for massless external four-point momenta:  $t \equiv 2 k_1 \cdot k_4 = 2 k_2 \cdot k_3$ .

$$u \equiv 2 k_1 \cdot k_3 = 2 k_2 \cdot k_4$$

Furthermore we use the shorthand  $(l_i)^2$  to represent the lorentz square:  $(l_i)^2 = l_i \cdot l_i$ .

The total numerator  $N_{25}$  is given by summing over the following terms, distinguished here by explicit dependence on loop momenta:  $N_{25} = \sum_{i=0}^8 N_{25}^{(i)}$ :

■  $N_{25}^{(0)}$

$$0$$

■  $N_{25}^{(1)}$

$$0$$

■  $N_{25}^{(2)}$

$$s^4 (\tau_{3,5} + \tau_{3,6})^2 + \frac{1}{2} l_{11}^2 s^5$$

■  $N_{25}^{(3)}$

$$-\frac{1}{2} s^3 \left( s (\tau_{1,13} - \tau_{1,15} (3t + u) - \tau_{4,15} (t + u) + t \tau_{2,13} - 3t \tau_{2,15} + t \tau_{4,11} + 2u \tau_{1,11} + 2u \tau_{2,11} + u \tau_{2,13} - u \tau_{2,15} + u \tau_{4,11}) + \right. \\ \left. l_{11}^2 s (\tau_{1,6} + \tau_{1,12} + \tau_{1,14} + \tau_{2,6} + \tau_{2,12} + \tau_{2,14} + 2 \tau_{3,6}) + 4 (\tau_{1,6} + \tau_{1,8} + \tau_{2,6} + \tau_{2,8}) \tau_{3,5} (\tau_{3,5} + \tau_{3,6}) \right)$$

■  $N_{25}^{(4)}$

$$\frac{1}{2} s^2 \left( l_9^2 s (2 (\tau_{1,11} + \tau_{1,15} + \tau_{2,11} + \tau_{2,15}) \tau_{4,10} - s (2 \tau_{10,13} + l_{12}^2)) + 2 (\tau_{1,6} + \tau_{1,8} + \tau_{2,6} + \tau_{2,8})^2 \tau_{3,5}^2 \right)$$

$$N_{25}^{(5)}$$

$$0$$

$$\blacksquare N_{25}^{(6)}$$

$$0$$

$$\blacksquare N_{25}^{(7)}$$

$$0$$

$$\blacksquare N_{25}^{(8)}$$

$$\frac{1}{8} l_7^2 l_{10}^2 l_{14}^2 \left( l_{17}^2 \left( 30 s^2 + 13 \left( t^2 + u^2 \right) \right) - l_9^2 \left( 32 s^2 + 19 \left( t^2 + u^2 \right) \right) \right)$$
