# Supplementary material for: The Ultraviolet Behavior of N=8 Supergravity at Four Loops
Source: arXiv:0905.2326 ancillary file (2012-01-08)
Supplement: Supplementary file 20 [file SUGRA26.pdf]

## Integral 26: $\mathcal{I}_{26}$

$\mathcal{N} = 8$  four-point four-loop amplitude.

### ■ 2D plot of graph associated with $\mathcal{I}_{26}$

This fixes the labelling associated with the numerator expressions given below.

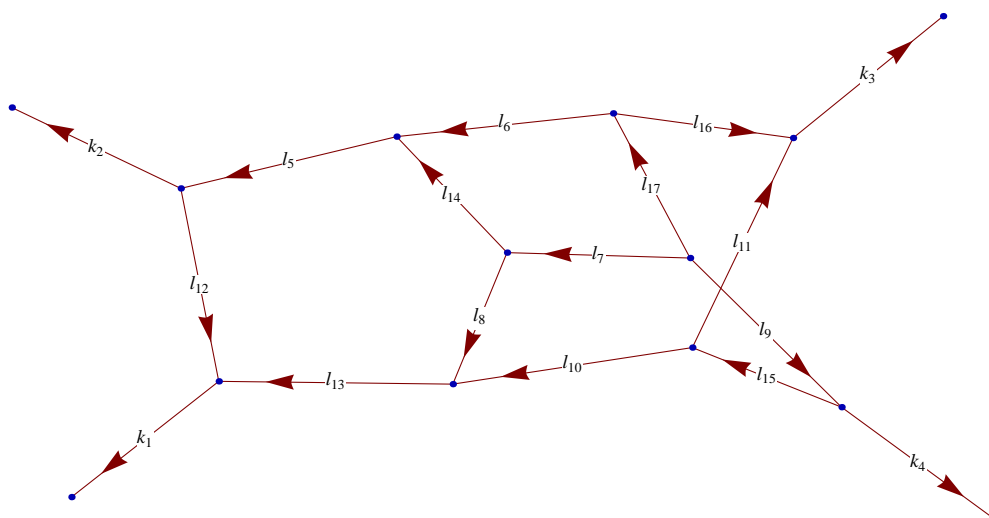

When using MathPlayer, by clicking three times (holding the click on the third click) directly on a vertex, one is able to move that vertex around, and its associated edges follow elastically. This functionality is absent when viewing as a pdf.

*Note: propagators for certain graphs were relabeled in the manuscript due to size constraints. The labels given in `aux/rawData/Neq8FourLoops.m` should be used for verification purposes.*

### ■ 3D plot of graph associated with $\mathcal{I}_{26}$

3D PLOT UNAVAILABLE FOR PDF. Please see .nb version for the 3D figure.

When using MathPlayer, by clicking anywhere in the image and dragging one should be able to rotate this 3D image. By holding (ALT) or (COMMAND) while clicking and moving the mouse up/down one should be able to zoom in/out. This functionality is absent when viewing as a pdf.

### ■ "Vertex Form" of graph associated with $I_{26}$

This function returns the graph associated with the integral object in a vertex representation. This can be used as a way of specifying the topology of a graph using trivalent (cubic) vertices,  $\text{gVertex}[p_a, p_b, p_c]$ , where  $\{p_a, p_b, p_c\}$  are momenta labeling the propagators (edges) of the graph, and is understood that the edge labelled by  $p_a$  flows into the edge labelled by  $-p_a$ . Additionally, each vertex represents the manifest conservation of ( $D$  - dimensional) momenta :

$$\text{gVertex}[\{p_1, p_2, p_3\}] \iff (p_1 + p_2 + p_3 = 0)$$

$$\{\text{gVertex}(\{k_1, -l_{12}, -l_{13}\}), \text{gVertex}(\{k_2, -l_5, l_{12}\}), \text{gVertex}(\{k_3, -l_{16}, -l_{11}\}), \text{gVertex}(\{k_4, l_{15}, -l_9\}), \text{gVertex}(\{l_5, -l_{14}, -l_6\}), \\ \text{gVertex}(\{l_6, -l_{17}, l_{16}\}), \text{gVertex}(\{-l_7, l_{14}, l_8\}), \text{gVertex}(\{l_7, l_9, l_{17}\}), \text{gVertex}(\{-l_8, l_{13}, -l_{10}\}), \text{gVertex}(\{l_{10}, l_{11}, -l_{15}\})\}$$

### ■ Numerator expression for integral 26:

The following notation is used:  $\tau_{i,j} \equiv \begin{cases} 2 k_i \cdot l_j & \text{if } i \leq 4, j > 4 \\ 2 l_i \cdot l_j & \text{if } i, j > 4 \end{cases}$ .

$$s \equiv 2 k_1 \cdot k_2 = 2 k_3 \cdot k_4$$

We use  $s, t, u$  to represent the traditional Mandelstam variables for massless external four-point momenta:  $t \equiv 2 k_1 \cdot k_4 = 2 k_2 \cdot k_3$ .

$$u \equiv 2 k_1 \cdot k_3 = 2 k_2 \cdot k_4$$

Furthermore we use the shorthand  $(l_i)^2$  to represent the lorentz square:  $(l_i)^2 = l_i \cdot l_i$ .

**The total numerator  $\mathcal{N}_{26}$  is given by summing over the following terms, distinguished here by explicit dependence on loop momenta:  $\mathcal{N}_{26} = \sum_{i=0}^8 \mathcal{N}_{26}^{(i)}$ :**

#### ■ $\mathcal{N}_{26}^{(0)}$

$$s^6$$

#### ■ $\mathcal{N}_{26}^{(1)}$

$$-2 s^5 (\tau_{1,6} + \tau_{1,7} + \tau_{2,6} + \tau_{2,7} - \tau_{3,5})$$

#### ■ $\mathcal{N}_{26}^{(2)}$

$$\frac{1}{2} s^3 \left( -4 s^2 \tau_{5,9} + 2 s \tau_{1,6}^2 + 2 s \tau_{1,7}^2 + 2 s \tau_{2,6}^2 + 2 s \tau_{2,7}^2 + 2 s \tau_{3,5}^2 + 4 s \tau_{2,6} (\tau_{2,7} - 2 \tau_{3,5}) + 4 s \tau_{1,7} (\tau_{2,6} + \tau_{2,7} - 2 \tau_{3,5}) + \right. \\ \left. 4 s \tau_{1,6} (\tau_{1,7} + \tau_{2,6} + \tau_{2,7} - 2 \tau_{3,5}) - 8 s \tau_{2,7} \tau_{3,5} + l_8^2 s^2 + 2 l_{13}^2 s^2 + 2 l_5^2 t^2 + l_8^2 t^2 - 6 l_{13}^2 t^2 - l_{16}^2 t^2 - l_8^2 u^2 - 2 l_{13}^2 u^2 + l_{16}^2 u^2 \right)$$

■  $N_{26}^{(3)}$

$$\begin{aligned}
& \frac{1}{2} s^2 \left( (4 \tau_{1,6} \tau_{5,9} + (-4 \tau_{1,11} + 2 \tau_{1,14} - 2 \tau_{2,12} + \tau_{2,14} - 2 \tau_{3,12}) l_5^2 - 2 (\tau_{1,8} - \tau_{1,16} + \tau_{2,8} + \tau_{2,16}) l_{11}^2 + \right. \\
& \quad (6 \tau_{1,5} + 7 \tau_{1,8} + 14 \tau_{2,8} - 6 \tau_{2,11}) l_{13}^2 + 2 (2 (\tau_{2,6} + \tau_{2,7} - \tau_{3,5}) \tau_{5,9} + (\tau_{1,9} - \tau_{1,10} - \tau_{2,10} + \tau_{4,7} + \tau_{4,12}) l_8^2 - 2 \tau_{3,5} l_{13}^2) + \\
& \quad \tau_{1,7} (4 \tau_{5,9} + l_8^2 - l_{16}^2) + (2 \tau_{1,8} + \tau_{1,15} - \tau_{2,7} + 2 \tau_{2,8} - \tau_{2,15} + \tau_{4,7} - 2 \tau_{4,12}) l_{16}^2) t^2 - \\
& \quad 4 (\tau_{1,6} + \tau_{1,7} + \tau_{2,6} + \tau_{2,7}) (\tau_{1,6} + \tau_{1,7} + \tau_{2,6} + \tau_{2,7} - \tau_{3,5}) \tau_{3,5} t - \\
& \quad 4 u (\tau_{1,6} + \tau_{1,7} + \tau_{2,6} + \tau_{2,7}) (\tau_{1,6} + \tau_{1,7} + \tau_{2,6} + \tau_{2,7} - \tau_{3,5}) \tau_{3,5} + \\
& \quad (s^2 - t^2 - u^2) (4 \tau_{1,6} \tau_{5,9} + 4 (\tau_{2,6} + \tau_{2,7} - \tau_{3,5}) \tau_{5,9} - 2 \tau_{1,11} l_5^2 + \tau_{2,12} l_5^2 - \tau_{3,12} l_5^2 + \\
& \quad (2 \tau_{1,9} - \tau_{1,10} - \tau_{2,10} + 2 (\tau_{4,7} + \tau_{4,12})) l_8^2 + \tau_{1,7} (4 \tau_{5,9} + l_8^2) + 2 \tau_{1,16} l_{11}^2 - 2 \tau_{2,16} l_{11}^2 + \tau_{2,8} (2 l_5^2 - 2 l_{11}^2 - 5 l_{13}^2) - \\
& \quad 5 \tau_{1,5} l_{13}^2 - 2 \tau_{2,11} l_{13}^2 - 4 \tau_{3,5} l_{13}^2 + \tau_{1,8} (3 l_5^2 - 2 (l_{11}^2 + 2 l_{13}^2)) + (\tau_{1,15} - \tau_{2,15}) l_{16}^2 + (\tau_{4,7} - 2 \tau_{4,12}) l_{16}^2) + \\
& \quad u^2 (4 \tau_{1,6} \tau_{5,9} - 2 (\tau_{1,8} - \tau_{1,16} + \tau_{2,8} + \tau_{2,16}) l_{11}^2 + (\tau_{1,8} + 2 \tau_{2,11}) l_{13}^2 + \\
& \quad 2 (2 (\tau_{2,6} + \tau_{2,7} - \tau_{3,5}) \tau_{5,9} + (\tau_{1,9} + \tau_{4,7} + \tau_{4,12}) l_8^2 - 2 \tau_{3,5} l_{13}^2) + \\
& \quad \left. (-2 \tau_{1,8} + \tau_{1,15} + \tau_{2,7} - 2 \tau_{2,8} - \tau_{2,15} + \tau_{4,7} - 2 \tau_{4,12}) l_{16}^2 + \tau_{1,7} (4 \tau_{5,9} + l_8^2 + l_{16}^2) \right)
\end{aligned}$$

■  $N_{26}^{(4)}$

$$\begin{aligned}
& -\frac{1}{4} s \left( (4 \tau_{5,9}^2 + 4 \tau_{11,12} l_5^2 - 2 l_5^2 (l_8^2 + 3 l_{11}^2 + 7 l_{12}^2 - 8 l_{13}^2 - 5 l_{16}^2) - 3 l_{13}^2 (l_{12}^2 + 8 l_{16}^2) - \right. \\
& \quad 2 ((\tau_{7,12} + 2 \tau_{9,12}) l_8^2 + 4 \tau_{12,16} l_{11}^2 - 2 \tau_{5,11} l_{13}^2 + 2 \tau_{12,15} l_{16}^2) + 2 l_8^2 (4 l_{11}^2 - 3 l_{13}^2 + l_{14}^2 - 2 (l_{15}^2 + l_{16}^2))) t^3 - \\
& \quad 4 (-l_{13}^2 \tau_{1,5}^2 + (-(\tau_{2,8} - \tau_{2,11} + \tau_{2,12}) (2 \tau_{1,14} + \tau_{2,8} - \tau_{2,11} + \tau_{2,12} + \tau_{2,14}) + \tau_{2,11} \tau_{3,12} + \\
& \quad \tau_{1,11} (2 \tau_{2,8} - 2 \tau_{2,11} + 3 \tau_{2,12} + 2 \tau_{3,12}) + \tau_{1,8} (2 \tau_{1,11} - 3 \tau_{1,14} - 2 \tau_{2,8} + 2 \tau_{2,11} - 2 \tau_{2,12} - \tau_{2,14} - \tau_{3,14})) l_5^2 - \\
& \quad (\tau_{1,10} + \tau_{2,10}) \tau_{4,12} l_8^2 - (2 \tau_{1,8}^2 + 7 \tau_{2,8} \tau_{1,8} + 8 \tau_{2,8}^2 + \tau_{2,11}^2 + \tau_{1,5} (3 \tau_{1,8} + 6 \tau_{2,8} - 4 \tau_{2,11}) - 4 (\tau_{1,8} + 2 \tau_{2,8}) \tau_{2,11}) \\
& \quad l_{13}^2 + \tau_{3,5} (2 (\tau_{1,6} + \tau_{1,7} + \tau_{2,6} + \tau_{2,7}) \tau_{5,9} + 3 (\tau_{1,5} + \tau_{1,8} + \tau_{2,8}) l_{13}^2) - (\tau_{1,7} - 2 \tau_{1,8} + \tau_{2,7} - 2 \tau_{2,8}) \tau_{4,12} l_{16}^2) t^2 + \\
& \quad 4 (\tau_{1,6} + \tau_{1,7} + \tau_{2,6} + \tau_{2,7})^2 \tau_{3,5}^2 t - \frac{1}{2} (-s^2 + t^2 + u^2) (12 \tau_{5,9}^2 + 8 \tau_{11,12} l_5^2 + 2 l_5^2 (l_8^2 - 5 l_{11}^2 - 19 l_{12}^2 - 8 l_{13}^2 - 18 l_{16}^2) - \\
& \quad l_{13}^2 (5 l_{12}^2 + 72 l_{16}^2) - 6 ((\tau_{7,12} + 2 \tau_{9,12}) l_8^2 + 4 \tau_{12,16} l_{11}^2 - 2 \tau_{5,11} l_{13}^2 + 2 \tau_{12,15} l_{16}^2) + \\
& \quad 6 l_8^2 (4 l_{11}^2 - 4 l_{13}^2 + l_{14}^2 - 2 (l_{15}^2 + l_{16}^2))) t + 4 u (\tau_{1,6} + \tau_{1,7} + \tau_{2,6} + \tau_{2,7})^2 \tau_{3,5}^2 - \\
& \quad 2 (s^2 - t^2 - u^2) (4 l_{13}^2 \tau_{1,5}^2 - (2 \tau_{1,8}^2 + (-2 \tau_{1,11} + \tau_{1,14} + 5 \tau_{2,8} - 5 \tau_{2,11} + 8 \tau_{2,12} + 3 \tau_{3,12} + \tau_{3,14}) \tau_{1,8} + \\
& \quad 2 \tau_{2,8}^2 + 2 \tau_{2,11}^2 - 2 \tau_{1,14} \tau_{2,11} + 2 \tau_{2,12} (2 \tau_{2,12} + \tau_{3,12}) + 2 \tau_{2,8} (-2 \tau_{2,11} + 3 \tau_{2,12} + \tau_{3,12}) - \\
& \quad \tau_{2,11} (5 \tau_{2,12} + \tau_{2,14} + 2 \tau_{3,12}) - \tau_{1,11} (2 \tau_{2,8} - 4 \tau_{2,11} + 5 \tau_{2,12} + 4 \tau_{3,12})) l_5^2 - 2 (\tau_{1,10} + \tau_{2,10}) \tau_{4,12} l_8^2 + \\
& \quad 2 (\tau_{1,8}^2 + 3 \tau_{2,8} \tau_{1,8} + 2 \tau_{2,8}^2 - \tau_{2,11}^2 + (\tau_{1,8} + 3 \tau_{2,8}) \tau_{2,11} + \tau_{1,5} (3 \tau_{1,8} + 4 \tau_{2,8} + \tau_{2,11})) l_{13}^2 + \\
& \quad 2 \tau_{3,5} (2 (\tau_{1,6} + \tau_{1,7} + \tau_{2,6} + \tau_{2,7}) \tau_{5,9} + 3 (\tau_{1,5} + \tau_{1,8} + \tau_{2,8}) l_{13}^2) - 2 (\tau_{1,7} - 2 \tau_{1,8} + \tau_{2,7} - 2 \tau_{2,8}) \tau_{4,12} l_{16}^2) - \\
& \quad 4 u^2 ((3 \tau_{1,8} - 2 \tau_{1,11} + 2 \tau_{2,8} - \tau_{2,11} + 2 \tau_{2,12}) (\tau_{2,11} - \tau_{2,12} - \tau_{3,12}) l_5^2 - (\tau_{1,10} + \tau_{2,10}) \tau_{4,12} l_8^2 - \\
& \quad (\tau_{2,11}^2 + 2 (\tau_{1,5} + \tau_{1,8} + \tau_{2,8}) \tau_{2,11} + \tau_{1,8} (\tau_{1,5} + \tau_{1,8} + \tau_{2,8})) l_{13}^2 + \\
& \quad \tau_{3,5} (2 (\tau_{1,6} + \tau_{1,7} + \tau_{2,6} + \tau_{2,7}) \tau_{5,9} + 3 (\tau_{1,5} + \tau_{1,8} + \tau_{2,8}) l_{13}^2) - (\tau_{1,7} - 2 \tau_{1,8} + \tau_{2,7} - 2 \tau_{2,8}) \tau_{4,12} l_{16}^2) + \\
& \quad u^3 (4 \tau_{5,9}^2 - 2 l_5^2 (l_7^2 - 3 l_8^2 + 5 l_{11}^2 + 7 l_{12}^2 + 4 l_{16}^2) - l_{13}^2 (3 l_{12}^2 + 32 l_{16}^2) - \\
& \quad 2 ((\tau_{7,12} + 2 \tau_{9,12}) l_8^2 + 4 \tau_{12,16} l_{11}^2 - 2 \tau_{5,11} l_{13}^2 + 2 \tau_{12,15} l_{16}^2) + 2 l_8^2 (4 l_{11}^2 - 6 l_{13}^2 + l_{14}^2 - 2 (l_{15}^2 + l_{16}^2))) - \\
& \quad \frac{1}{2} u (-s^2 + t^2 + u^2) (12 \tau_{5,9}^2 + 4 \tau_{11,12} l_5^2 - 5 l_{13}^2 (l_{12}^2 + 16 l_{16}^2) - 2 l_5^2 (l_7^2 - 5 l_8^2 + 7 l_{11}^2 + 19 l_{12}^2 + 16 l_{13}^2 + 27 l_{16}^2) - \\
& \quad \left. 6 ((\tau_{7,12} + 2 \tau_{9,12}) l_8^2 + 4 \tau_{12,16} l_{11}^2 - 2 \tau_{5,11} l_{13}^2 + 2 \tau_{12,15} l_{16}^2) + 6 l_8^2 (4 l_{11}^2 - 5 l_{13}^2 + l_{14}^2 - 2 (l_{15}^2 + l_{16}^2))) \right)
\end{aligned}$$

$N_{26}^{(5)}$ 

$$\begin{aligned}
& \frac{1}{8} \left( 2 \left( 4 \tau_{2,11} \tau_{11,12} l_5^2 - 4 \tau_{2,12} \tau_{11,12} l_5^2 + 4 \tau_{1,11} (2 \tau_{11,12} + l_7^2) l_5^2 + 8 \tau_{1,9} l_8^2 l_5^2 + 4 \tau_{2,9} l_8^2 l_5^2 + 4 \tau_{4,12} l_8^2 l_5^2 - 8 \tau_{1,15} l_{11}^2 l_5^2 - \right. \right. \\
& 8 \tau_{1,16} l_{11}^2 l_5^2 + 4 \tau_{2,12} l_{11}^2 l_5^2 - 8 \tau_{2,14} l_{11}^2 l_5^2 + 4 \tau_{4,14} l_{11}^2 l_5^2 + 4 \tau_{4,16} l_{11}^2 l_5^2 + 10 \tau_{1,16} l_{12}^2 l_5^2 - 2 \tau_{1,17} l_{12}^2 l_5^2 + \\
& \tau_{2,9} l_{12}^2 l_5^2 + 8 \tau_{2,16} l_{12}^2 l_5^2 - 3 \tau_{2,17} l_{12}^2 l_5^2 + 10 \tau_{3,8} l_{12}^2 l_5^2 - 2 \tau_{3,17} l_{12}^2 l_5^2 + 50 \tau_{1,6} l_{13}^2 l_5^2 - 16 \tau_{1,9} l_{13}^2 l_5^2 + 4 \tau_{1,12} l_{13}^2 l_5^2 - \\
& 50 \tau_{1,17} l_{13}^2 l_5^2 + 5 \tau_{2,6} l_{13}^2 l_5^2 - 32 \tau_{2,9} l_{13}^2 l_5^2 + 3 \tau_{2,12} l_{13}^2 l_5^2 - 18 \tau_{2,17} l_{13}^2 l_5^2 + 10 \tau_{4,12} l_{13}^2 l_5^2 - 18 \tau_{4,17} l_{13}^2 l_5^2 + \\
& 4 \tau_{1,5} \tau_{5,11} l_{13}^2 - 4 \tau_{1,10} l_8^2 l_{13}^2 - 4 \tau_{1,12} l_8^2 l_{13}^2 - 6 \tau_{2,10} l_8^2 l_{13}^2 + 2 \tau_{2,14} l_8^2 l_{13}^2 - 4 \tau_{4,12} l_8^2 l_{13}^2 - 5 \tau_{1,15} l_{12}^2 l_{13}^2 - \\
& 6 \tau_{2,11} l_{12}^2 l_{13}^2 - 9 \tau_{2,15} l_{12}^2 l_{13}^2 - 2 \tau_{4,8} l_{12}^2 l_{13}^2 - 10 \tau_{4,11} l_{12}^2 l_{13}^2 + \tau_{2,8} (-4 \tau_{11,12} l_5^2 + 7 l_{12}^2 l_5^2 + 4 (\tau_{5,11} - l_{12}^2) l_{13}^2) + \\
& 2 (2 (\tau_{2,6} + \tau_{2,10} + 2 \tau_{2,11} + \tau_{3,5} + 3 \tau_{3,10} + \tau_{3,11} + 6 \tau_{4,5} + \tau_{4,6} + \tau_{4,11}) l_{13}^2 - \\
& (12 \tau_{2,6} + 6 \tau_{2,13} - 4 \tau_{2,17} - 6 \tau_{3,6} + 4 \tau_{3,8} + 4 \tau_{3,13} + 4 \tau_{3,17} + 15 \tau_{4,6} + \tau_{4,17}) l_5^2) l_{16}^2) l^3 + \\
& 4 (2 \tau_{2,12} l_5^2 \tau_{1,11}^2 - 2 (\tau_{2,12} (\tau_{2,8} - \tau_{2,11} + \tau_{2,12}) + 2 (\tau_{2,8} + \tau_{2,12}) \tau_{3,12}) l_5^2 \tau_{1,11} + 2 \tau_{1,14} (\tau_{2,8} - \tau_{2,11} + \tau_{2,12})^2 l_5^2 + \\
& (\tau_{2,8} - \tau_{2,11} + \tau_{2,12}) ((\tau_{2,8} - \tau_{2,11} + \tau_{2,12}) \tau_{2,14} + 2 (\tau_{2,8} + \tau_{2,12}) \tau_{3,12}) l_5^2 + \\
& 2 ((\tau_{2,8} - \tau_{2,11}) (\tau_{1,5}^2 + 3 \tau_{2,8} \tau_{1,5} + 3 \tau_{2,8}^2 - (\tau_{1,5} + 2 \tau_{2,8}) \tau_{2,11}) - (\tau_{1,5} + \tau_{2,8})^2 \tau_{3,5}) l_{13}^2) l^2 + \\
& (s^2 - t^2 - u^2) (12 \tau_{2,11} \tau_{11,12} l_5^2 - 16 \tau_{2,12} \tau_{11,12} l_5^2 - 4 \tau_{2,10} l_7^2 l_5^2 - 8 \tau_{2,11} l_7^2 l_5^2 + 4 \tau_{1,11} (6 \tau_{11,12} + l_7^2) l_5^2 + \\
& 24 \tau_{1,9} l_8^2 l_5^2 + 4 \tau_{1,10} l_8^2 l_5^2 + 12 \tau_{2,9} l_8^2 l_5^2 + 4 \tau_{2,10} l_8^2 l_5^2 + 12 \tau_{4,12} l_8^2 l_5^2 + 12 \tau_{1,14} l_{11}^2 l_5^2 - 36 \tau_{1,15} l_{11}^2 l_5^2 - 48 \tau_{1,16} l_{11}^2 l_5^2 - \\
& 4 \tau_{2,12} l_{11}^2 l_5^2 + 4 \tau_{2,14} l_{11}^2 l_5^2 - 16 \tau_{2,15} l_{11}^2 l_5^2 - 24 \tau_{2,16} l_{11}^2 l_5^2 - 20 \tau_{4,12} l_{11}^2 l_5^2 + 36 \tau_{4,14} l_{11}^2 l_5^2 - 12 \tau_{4,16} l_{11}^2 l_5^2 - \\
& 4 \tau_{1,9} l_{12}^2 l_5^2 + 20 \tau_{1,16} l_{12}^2 l_5^2 - 4 \tau_{1,17} l_{12}^2 l_5^2 - 3 \tau_{2,9} l_{12}^2 l_5^2 + 18 \tau_{2,16} l_{12}^2 l_5^2 - 5 \tau_{2,17} l_{12}^2 l_5^2 + 30 \tau_{3,8} l_{12}^2 l_5^2 - \\
& 6 \tau_{3,17} l_{12}^2 l_5^2 + 12 \tau_{1,6} l_{13}^2 l_5^2 + 36 \tau_{1,9} l_{13}^2 l_5^2 + 30 \tau_{1,12} l_{13}^2 l_5^2 - 30 \tau_{1,17} l_{13}^2 l_5^2 - 95 \tau_{2,6} l_{13}^2 l_5^2 + 42 \tau_{2,9} l_{13}^2 l_5^2 + \\
& 55 \tau_{2,12} l_{13}^2 l_5^2 + 48 \tau_{2,17} l_{13}^2 l_5^2 + 42 \tau_{4,12} l_{13}^2 l_5^2 - 42 \tau_{4,17} l_{13}^2 l_5^2 + 12 \tau_{1,5} \tau_{5,11} l_{13}^2 - 12 \tau_{1,10} l_8^2 l_{13}^2 - 12 \tau_{1,12} l_8^2 l_{13}^2 - \\
& 20 \tau_{2,10} l_8^2 l_{13}^2 + 6 \tau_{2,14} l_8^2 l_{13}^2 - 12 \tau_{4,12} l_8^2 l_{13}^2 + \tau_{1,15} l_{12}^2 l_{13}^2 - 6 \tau_{2,11} l_{12}^2 l_{13}^2 - 3 \tau_{2,15} l_{12}^2 l_{13}^2 - 6 \tau_{4,8} l_{12}^2 l_{13}^2 - \\
& 4 \tau_{4,11} l_{12}^2 l_{13}^2 + 2 ((2 \tau_{2,6} - 24 \tau_{2,13} + 12 \tau_{2,17} + 34 \tau_{3,6} - 2 \tau_{3,8} - 22 \tau_{3,13} - 12 \tau_{3,17} + 25 \tau_{4,6} - 13 \tau_{4,17}) l_5^2 + \\
& 2 (10 \tau_{2,10} + 14 \tau_{2,11} + 3 \tau_{3,5} + 2 \tau_{3,6} + 11 \tau_{3,10} + 3 (\tau_{3,11} + 6 \tau_{4,5} + \tau_{4,6} - \tau_{4,11})) l_{13}^2) l_{16}^2 + \\
& \tau_{2,8} (3 (2 (2 \tau_{5,11} - l_{12}^2) l_{13}^2 + l_5^2 (7 l_{12}^2 + 4 l_{16}^2)) - 16 \tau_{11,12} l_5^2) t + 4 (t^2 + u^2) \tau_{1,8}^3 l_{13}^2 + \\
& 4 u^2 ((2 \tau_{2,12}^3 - 4 \tau_{1,11} \tau_{2,12}^2 + 4 \tau_{2,8} \tau_{2,12}^2 - 2 \tau_{2,11} \tau_{2,12}^2 + 2 (\tau_{1,11} - \tau_{2,8})^2 \tau_{2,12} + 2 \tau_{1,11} \tau_{2,11} \tau_{2,12} - \\
& 2 \tau_{2,8} \tau_{2,11} \tau_{2,12} + 2 \tau_{1,14} \tau_{2,11}^2 + \tau_{2,11}^2 \tau_{2,14} - 2 (2 \tau_{1,11} - 2 \tau_{2,8} + \tau_{2,11} - 2 \tau_{2,12}) (\tau_{2,8} + \tau_{2,12}) \tau_{3,12}) l_5^2 + \\
& 2 (\tau_{2,11} ((\tau_{1,5} + \tau_{2,8})^2 + (\tau_{1,5} + 2 \tau_{2,8}) \tau_{2,11}) - (\tau_{1,5} + \tau_{2,8})^2 \tau_{3,5}) l_{13}^2) + \\
& 4 \tau_{1,8}^2 ((2 t (2 t + u) \tau_{1,14} - 4 s u \tau_{2,12} + (s^2 + t^2) \tau_{2,14} - 2 s (2 u \tau_{3,12} + (2 t + u) \tau_{3,14})) l_5^2 + \\
& ((3 (t^2 + u^2) - s^2) \tau_{1,5} + (-s^2 + 5 t^2 + 3 u^2) \tau_{2,8} - 2 s ((u - t) \tau_{2,11} + s \tau_{3,5})) l_{13}^2) + 4 (s^2 - t^2 - u^2) \\
& (-(-2 \tau_{2,12} \tau_{1,11}^2 + (\tau_{2,12} (3 \tau_{2,8} - 2 \tau_{2,11} + 3 \tau_{2,12}) + 4 (\tau_{2,8} + \tau_{2,12}) \tau_{3,12}) \tau_{1,11} + 2 \tau_{1,14} \tau_{2,11} (\tau_{2,8} - \tau_{2,11} + \tau_{2,12}) - \\
& (\tau_{2,8} - \tau_{2,11} + \tau_{2,12}) (\tau_{2,12} (\tau_{2,8} + \tau_{2,12}) - \tau_{2,11} \tau_{2,14}) - (\tau_{2,8} + \tau_{2,12}) (3 \tau_{2,8} - 2 \tau_{2,11} + 3 \tau_{2,12}) \tau_{3,12}) l_5^2 - \\
& (\tau_{1,5}^3 + (3 \tau_{2,8} + 2 \tau_{3,5}) \tau_{1,5}^2 + (3 \tau_{2,8}^2 + 2 (\tau_{2,11} + 2 \tau_{3,5}) \tau_{2,8} - 2 \tau_{2,11}^2) \tau_{1,5} + \\
& \tau_{2,8} (\tau_{2,8}^2 + 2 (2 \tau_{2,11} + \tau_{3,5}) \tau_{2,8} - 4 \tau_{2,11}^2)) l_{13}^2) +
\end{aligned}$$

$$\begin{aligned}
& \tau_{1,8} (12 \tau_{11,12} l_5^2 t^3 - 10 l_5^2 l_{12}^2 t^3 - 12 \tau_{2,12}^2 l_5^2 t^2 + 8 \tau_{2,8} \tau_{2,14} l_5^2 t^2 + 8 \tau_{2,12} \tau_{2,14} l_5^2 t^2 - 12 \tau_{2,12} \tau_{3,12} l_5^2 t^2 + \\
& 4 \tau_{2,12} \tau_{3,14} l_5^2 t^2 + 32 u \tau_{11,12} l_5^2 t^2 - 21 u l_5^2 l_{12}^2 t^2 + 8 s \tau_{2,11} \tau_{2,14} l_5^2 t - 16 s \tau_{2,8} \tau_{3,12} l_5^2 t - 8 s \tau_{2,8} \tau_{3,14} l_5^2 t - \\
& 28 s^2 \tau_{11,12} l_5^2 t + 28 u^2 \tau_{11,12} l_5^2 t + 18 s^2 l_5^2 l_{12}^2 t - 18 u^2 l_5^2 l_{12}^2 t + 12 s^2 \tau_{2,12}^2 l_5^2 + 12 u^2 \tau_{2,12}^2 l_5^2 - \\
& 24 s u \tau_{2,8} \tau_{2,12} l_5^2 + 8 s u \tau_{2,11} \tau_{2,12} l_5^2 + 8 (3 t + u) \tau_{1,14} (s \tau_{2,11} + t (\tau_{2,8} + \tau_{2,12})) l_5^2 - 40 s u \tau_{2,8} \tau_{3,12} l_5^2 + \\
& 28 s^2 \tau_{2,12} \tau_{3,12} l_5^2 + 12 u^2 \tau_{2,12} \tau_{3,12} l_5^2 + 8 s \tau_{1,11} ((2 t + 3 u) \tau_{2,12} - 2 s \tau_{3,12}) l_5^2 - 8 s^2 \tau_{2,11} \tau_{3,14} l_5^2 + \\
& 4 s^2 \tau_{2,12} \tau_{3,14} l_5^2 - 4 u^2 \tau_{2,12} \tau_{3,14} l_5^2 + 8 u^3 \tau_{11,12} l_5^2 - 32 s^2 u \tau_{11,12} l_5^2 - 7 u^3 l_5^2 l_{12}^2 + 21 s^2 u l_5^2 l_{12}^2 - \\
& 2 (2 (2 s^2 - 3 (t^2 + u^2)) \tau_{1,5}^2 + 4 ((2 s^2 - 5 t^2 - 3 u^2) \tau_{2,8} + 2 (\tau_{3,5} s^2 + (t^2 - u^2) \tau_{2,11})) \tau_{1,5} + \\
& 2 (2 s^2 - 3 (3 t^2 + u^2)) \tau_{2,8}^2 - 4 s^2 \tau_{2,11}^2 + 8 s \tau_{2,8} ((u - 2 t) \tau_{2,11} + s \tau_{3,5})) \tau_{1,5} + \\
& 2 (t + u) ((t + u)^2 - 3 s^2) \tau_{5,11} + ((4 t + 3 u) s^2 + (t + u) (2 t^2 - 5 u t + u^2)) l_{12}^2 l_{13}^2) + \\
& 2 u^3 (4 \tau_{2,11} \tau_{11,12} l_5^2 - 8 \tau_{2,12} \tau_{11,12} l_5^2 + 4 \tau_{1,10} l_7^2 l_5^2 + 4 \tau_{1,11} (2 \tau_{11,12} + l_7^2) l_5^2 + 8 \tau_{1,9} l_8^2 l_5^2 + 4 \tau_{1,10} l_8^2 l_5^2 + \\
& 4 \tau_{2,9} l_8^2 l_5^2 + 4 \tau_{2,10} l_8^2 l_5^2 + 4 \tau_{4,12} l_8^2 l_5^2 + 16 \tau_{1,14} l_{11}^2 l_5^2 - 8 \tau_{1,15} l_{11}^2 l_5^2 - 16 \tau_{1,16} l_{11}^2 l_5^2 - 16 \tau_{2,12} l_{11}^2 l_5^2 + 16 \tau_{2,14} l_{11}^2 l_5^2 - \\
& 4 \tau_{2,15} l_{11}^2 l_5^2 - 8 \tau_{2,16} l_{11}^2 l_5^2 - 20 \tau_{4,12} l_{11}^2 l_5^2 + 28 \tau_{4,14} l_{11}^2 l_5^2 - 16 \tau_{4,16} l_{11}^2 l_5^2 + \tau_{1,9} l_{12}^2 l_5^2 + 8 \tau_{1,16} l_{12}^2 l_5^2 - 3 \tau_{1,17} l_{12}^2 l_5^2 + \\
& 10 \tau_{2,16} l_{12}^2 l_5^2 - 2 \tau_{2,17} l_{12}^2 l_5^2 + 10 \tau_{3,8} l_{12}^2 l_5^2 - 2 \tau_{3,17} l_{12}^2 l_5^2 - 4 \tau_{1,6} l_{13}^2 l_5^2 - 4 \tau_{1,9} l_{13}^2 l_5^2 + 18 \tau_{1,12} l_{13}^2 l_5^2 - 2 \tau_{1,17} l_{13}^2 l_5^2 + \\
& \tau_{2,6} l_{13}^2 l_5^2 + 6 \tau_{2,9} l_{13}^2 l_5^2 + 19 \tau_{2,12} l_{13}^2 l_5^2 - 16 \tau_{2,17} l_{13}^2 l_5^2 + 22 \tau_{4,12} l_{13}^2 l_5^2 - 6 \tau_{4,17} l_{13}^2 l_5^2 + 4 \tau_{1,5} \tau_{5,11} l_{13}^2 - 4 \tau_{1,10} l_8^2 l_{13}^2 - \\
& 4 \tau_{1,12} l_8^2 l_{13}^2 - 8 \tau_{2,10} l_8^2 l_{13}^2 + 2 \tau_{2,14} l_8^2 l_{13}^2 - 4 \tau_{4,12} l_8^2 l_{13}^2 - 9 \tau_{1,15} l_{12}^2 l_{13}^2 + 6 \tau_{2,11} l_{12}^2 l_{13}^2 - 5 \tau_{2,15} l_{12}^2 l_{13}^2 - \\
& 2 \tau_{4,8} l_{12}^2 l_{13}^2 - 4 \tau_{4,11} l_{12}^2 l_{13}^2 + 2 ((2 \tau_{2,6} - 12 \tau_{2,13} + 4 \tau_{2,17} - 2 \tau_{3,6} + 6 \tau_{3,8} - 14 \tau_{3,13} - 4 \tau_{3,17} + 7 \tau_{4,6} - 11 \tau_{4,17}) l_5^2 + \\
& 2 (-2 \tau_{2,6} + 2 \tau_{2,10} + 10 \tau_{2,11} + \tau_{3,5} + 2 \tau_{3,6} + 11 \tau_{3,10} + 7 \tau_{3,11} + 6 \tau_{4,5} + \tau_{4,6} - 11 \tau_{4,11}) l_{13}^2) l_{16}^2 + \\
& 2 \tau_{2,8} (-4 \tau_{11,12} l_5^2 + 2 (l_{12}^2 + 3 l_{16}^2) l_5^2 + (2 \tau_{5,11} - 3 l_{12}^2) l_{13}^2)) + u (s^2 - t^2 - u^2) \\
& (12 \tau_{2,11} \tau_{11,12} l_5^2 - 20 \tau_{2,12} \tau_{11,12} l_5^2 + 4 \tau_{1,10} l_7^2 l_5^2 - 4 \tau_{2,10} l_7^2 l_5^2 - 8 \tau_{2,11} l_7^2 l_5^2 + 4 \tau_{1,11} (6 \tau_{11,12} + l_7^2) l_5^2 + \\
& 24 \tau_{1,9} l_8^2 l_5^2 + 8 \tau_{1,10} l_8^2 l_5^2 + 12 \tau_{2,9} l_8^2 l_5^2 + 8 \tau_{2,10} l_8^2 l_5^2 + 12 \tau_{4,12} l_8^2 l_5^2 + 28 \tau_{1,14} l_{11}^2 l_5^2 - 36 \tau_{1,15} l_{11}^2 l_5^2 - 56 \tau_{1,16} l_{11}^2 l_5^2 - \\
& 24 \tau_{2,12} l_{11}^2 l_5^2 + 28 \tau_{2,14} l_{11}^2 l_5^2 - 20 \tau_{2,15} l_{11}^2 l_5^2 - 32 \tau_{2,16} l_{11}^2 l_5^2 - 40 \tau_{4,12} l_{11}^2 l_5^2 + 60 \tau_{4,14} l_{11}^2 l_5^2 - 32 \tau_{4,16} l_{11}^2 l_5^2 - \\
& 3 \tau_{1,9} l_{12}^2 l_5^2 + 18 \tau_{1,16} l_{12}^2 l_5^2 - 5 \tau_{1,17} l_{12}^2 l_5^2 - 4 \tau_{2,9} l_{12}^2 l_5^2 + 20 \tau_{2,16} l_{12}^2 l_5^2 - 4 \tau_{2,17} l_{12}^2 l_5^2 + 30 \tau_{3,8} l_{12}^2 l_5^2 - \\
& 6 \tau_{3,17} l_{12}^2 l_5^2 - 42 \tau_{1,6} l_{13}^2 l_5^2 + 48 \tau_{1,9} l_{13}^2 l_5^2 + 44 \tau_{1,12} l_{13}^2 l_5^2 + 18 \tau_{1,17} l_{13}^2 l_5^2 - 99 \tau_{2,6} l_{13}^2 l_5^2 + 80 \tau_{2,9} l_{13}^2 l_5^2 + \\
& 71 \tau_{2,12} l_{13}^2 l_5^2 + 50 \tau_{2,17} l_{13}^2 l_5^2 + 54 \tau_{4,12} l_{13}^2 l_5^2 - 30 \tau_{4,17} l_{13}^2 l_5^2 + 12 \tau_{1,5} \tau_{5,11} l_{13}^2 - 12 \tau_{1,10} l_8^2 l_{13}^2 - 12 \tau_{1,12} l_8^2 l_{13}^2 - \\
& 22 \tau_{2,10} l_8^2 l_{13}^2 + 6 \tau_{2,14} l_8^2 l_{13}^2 - 12 \tau_{4,12} l_8^2 l_{13}^2 - 3 \tau_{1,15} l_{12}^2 l_{13}^2 + 6 \tau_{2,11} l_{12}^2 l_{13}^2 + \tau_{2,15} l_{12}^2 l_{13}^2 - 6 \tau_{4,8} l_{12}^2 l_{13}^2 + \\
& 2 \tau_{4,11} l_{12}^2 l_{13}^2 + 2 ((16 \tau_{2,6} - 30 \tau_{2,13} + 12 \tau_{2,17} + 26 \tau_{3,6} + 8 \tau_{3,8} - 32 \tau_{3,13} - 12 \tau_{3,17} + 47 \tau_{4,6} - 23 \tau_{4,17}) l_5^2 + \\
& 2 (-3 \tau_{2,6} + 11 \tau_{2,10} + 22 \tau_{2,11} + 3 \tau_{3,5} + 4 \tau_{3,6} + 19 \tau_{3,10} + 3 (3 \tau_{3,11} + 6 \tau_{4,5} + \tau_{4,6} - 5 \tau_{4,11})) l_{13}^2) l_{16}^2 + \\
& 2 \tau_{2,8} (-10 \tau_{11,12} l_5^2 + 3 (3 l_{12}^2 + 4 l_{16}^2) l_5^2 + 2 (3 \tau_{5,11} - 2 l_{12}^2) l_{13}^2)))
\end{aligned}$$

■  $N_{26}^{(6)}$

$$\begin{aligned}
& \frac{1}{16} (-4 (8 \tau_{12,16} l_5^2 l_{11}^2 + 4 l_{13}^2 ((2 \tau_{5,11} + l_8^2) l_{16}^2 - \tau_{8,15} l_{12}^2) + l_5^2 ((2 l_{10}^2 + 7 l_{11}^2) l_{12}^2 - 2 l_8^2 (2 l_{11}^2 + 5 l_{12}^2 - 8 l_{13}^2) - \\
& 2 (3 \tau_{8,9} l_{12}^2 + (l_6^2 - 2 \tau_{12,17}) l_{13}^2 + l_7^2 (-5 l_{12}^2 + 2 l_{13}^2 - 6 l_{16}^2)) - 2 (7 l_{12}^2 + 6 l_{13}^2) l_{16}^2)) t^3 +
\end{aligned}$$

$$\begin{aligned}
& 4(34 l_5^2 l_{13}^2 \tau_{1,6}^2 - 42 \tau_{1,9} l_5^2 l_{13}^2 \tau_{1,6} - 4 \tau_{1,12} l_5^2 l_{13}^2 \tau_{1,6} - 68 \tau_{1,17} l_5^2 l_{13}^2 \tau_{1,6} + 21 \tau_{2,6} l_5^2 l_{13}^2 \tau_{1,6} - 60 \tau_{2,9} l_5^2 l_{13}^2 \tau_{1,6} - \\
& 9 \tau_{2,12} l_5^2 l_{13}^2 \tau_{1,6} - 30 \tau_{2,17} l_5^2 l_{13}^2 \tau_{1,6} + 6 \tau_{4,12} l_5^2 l_{13}^2 \tau_{1,6} - 18 \tau_{4,17} l_5^2 l_{13}^2 \tau_{1,6} + 32 \tau_{1,16}^2 l_5^2 l_{11}^2 + 4 \tau_{4,14}^2 l_5^2 l_{11}^2 - \\
& 12 \tau_{2,12} \tau_{2,15} l_5^2 l_{11}^2 + 12 \tau_{2,14} \tau_{2,15} l_5^2 l_{11}^2 - 12 \tau_{2,12} \tau_{2,16} l_5^2 l_{11}^2 + 8 \tau_{2,14} \tau_{2,16} l_5^2 l_{11}^2 - 12 \tau_{2,12} \tau_{4,12} l_5^2 l_{11}^2 + \\
& 16 \tau_{2,14} \tau_{4,12} l_5^2 l_{11}^2 - 4 \tau_{2,15} \tau_{4,12} l_5^2 l_{11}^2 - 8 \tau_{2,16} \tau_{4,12} l_5^2 l_{11}^2 + 12 \tau_{2,12} \tau_{4,14} l_5^2 l_{11}^2 - 16 \tau_{2,14} \tau_{4,14} l_5^2 l_{11}^2 - \\
& 4 \tau_{2,15} \tau_{4,14} l_5^2 l_{11}^2 - 4 \tau_{4,12} \tau_{4,14} l_5^2 l_{11}^2 - 4 \tau_{2,12} \tau_{4,16} l_5^2 l_{11}^2 + 8 \tau_{2,14} \tau_{4,16} l_5^2 l_{11}^2 - 4 \tau_{4,12} \tau_{4,16} l_5^2 l_{11}^2 + 4 \tau_{4,14} \tau_{4,16} l_5^2 l_{11}^2 - \\
& 6 \tau_{1,8}^2 l_5^2 l_{12}^2 - 4 \tau_{1,9}^2 l_5^2 l_{12}^2 - 2 \tau_{1,17}^2 l_5^2 l_{12}^2 - 2 \tau_{2,8}^2 l_5^2 l_{12}^2 - 4 \tau_{2,9}^2 l_5^2 l_{12}^2 + 2 \tau_{2,16}^2 l_5^2 l_{12}^2 - 2 \tau_{2,17}^2 l_5^2 l_{12}^2 - \\
& 4 \tau_{3,8}^2 l_5^2 l_{12}^2 - 4 \tau_{3,17}^2 l_5^2 l_{12}^2 + 6 \tau_{1,8} \tau_{1,9} l_5^2 l_{12}^2 - 8 \tau_{1,8} \tau_{1,17} l_5^2 l_{12}^2 + 4 \tau_{1,9} \tau_{1,17} l_5^2 l_{12}^2 - 9 \tau_{1,8} \tau_{2,8} l_5^2 l_{12}^2 + \\
& \tau_{1,9} \tau_{2,8} l_5^2 l_{12}^2 - 5 \tau_{1,17} \tau_{2,8} l_5^2 l_{12}^2 + 7 \tau_{1,8} \tau_{2,9} l_5^2 l_{12}^2 - 13 \tau_{1,9} \tau_{2,9} l_5^2 l_{12}^2 + 3 \tau_{1,17} \tau_{2,9} l_5^2 l_{12}^2 + 8 \tau_{2,8} \tau_{2,9} l_5^2 l_{12}^2 - \\
& \tau_{1,8} \tau_{2,16} l_5^2 l_{12}^2 - 5 \tau_{1,9} \tau_{2,16} l_5^2 l_{12}^2 + \tau_{1,17} \tau_{2,16} l_5^2 l_{12}^2 + 2 \tau_{2,8} \tau_{2,16} l_5^2 l_{12}^2 - 2 \tau_{2,9} \tau_{2,16} l_5^2 l_{12}^2 - 6 \tau_{1,8} \tau_{2,17} l_5^2 l_{12}^2 + \\
& 2 \tau_{1,9} \tau_{2,17} l_5^2 l_{12}^2 - 6 \tau_{1,17} \tau_{2,17} l_5^2 l_{12}^2 - 4 \tau_{2,8} \tau_{2,17} l_5^2 l_{12}^2 + 6 \tau_{2,9} \tau_{2,17} l_5^2 l_{12}^2 + 2 \tau_{2,16} \tau_{2,17} l_5^2 l_{12}^2 - 6 \tau_{1,8} \tau_{3,8} l_5^2 l_{12}^2 + \\
& 12 \tau_{1,9} \tau_{3,8} l_5^2 l_{12}^2 - 2 \tau_{1,17} \tau_{3,8} l_5^2 l_{12}^2 - 8 \tau_{2,8} \tau_{3,8} l_5^2 l_{12}^2 + 10 \tau_{2,9} \tau_{3,8} l_5^2 l_{12}^2 - 2 \tau_{2,16} \tau_{3,8} l_5^2 l_{12}^2 - 2 \tau_{2,17} \tau_{3,8} l_5^2 l_{12}^2 - \\
& 6 \tau_{1,8} \tau_{3,17} l_5^2 l_{12}^2 + 6 \tau_{1,9} \tau_{3,17} l_5^2 l_{12}^2 - 6 \tau_{1,17} \tau_{3,17} l_5^2 l_{12}^2 - 4 \tau_{2,8} \tau_{3,17} l_5^2 l_{12}^2 + 6 \tau_{2,9} \tau_{3,17} l_5^2 l_{12}^2 + 6 \tau_{2,16} \tau_{3,17} l_5^2 l_{12}^2 - \\
& 6 \tau_{2,17} \tau_{3,17} l_5^2 l_{12}^2 - 8 \tau_{3,8} \tau_{3,17} l_5^2 l_{12}^2 + 2 \tau_{1,16} l_5^2 (2(\tau_{2,14} + 2(\tau_{2,15} + \tau_{2,16} + \tau_{4,12} - 2\tau_{4,14} + \tau_{4,16})) - 5\tau_{2,12}) l_{11}^2 + \\
& (3\tau_{1,8} - \tau_{1,9} + \tau_{1,17} - 2\tau_{2,8} - 3\tau_{2,9} + 2\tau_{2,17} + 3\tau_{3,17}) l_{12}^2) + 8 \tau_{1,9}^2 l_5^2 l_{13}^2 + 34 \tau_{1,17}^2 l_5^2 l_{13}^2 + \\
& 4 \tau_{2,6}^2 l_5^2 l_{13}^2 + 42 \tau_{2,9}^2 l_5^2 l_{13}^2 + 8 \tau_{2,12}^2 l_5^2 l_{13}^2 + 4 \tau_{2,17}^2 l_5^2 l_{13}^2 - 4 \tau_{1,9} \tau_{1,12} l_5^2 l_{13}^2 + 42 \tau_{1,9} \tau_{1,17} l_5^2 l_{13}^2 + \\
& 4 \tau_{1,12} \tau_{1,17} l_5^2 l_{13}^2 - 13 \tau_{1,9} \tau_{2,6} l_5^2 l_{13}^2 + 14 \tau_{1,12} \tau_{2,6} l_5^2 l_{13}^2 - 21 \tau_{1,17} \tau_{2,6} l_5^2 l_{13}^2 + 24 \tau_{1,9} \tau_{2,9} l_5^2 l_{13}^2 - 14 \tau_{1,12} \tau_{2,9} l_5^2 l_{13}^2 + \\
& 48 \tau_{1,17} \tau_{2,9} l_5^2 l_{13}^2 - 46 \tau_{2,6} \tau_{2,9} l_5^2 l_{13}^2 - 3 \tau_{1,9} \tau_{2,12} l_5^2 l_{13}^2 - 10 \tau_{1,12} \tau_{2,12} l_5^2 l_{13}^2 + 9 \tau_{1,17} \tau_{2,12} l_5^2 l_{13}^2 - 8 \tau_{2,6} \tau_{2,12} l_5^2 l_{13}^2 + \\
& 24 \tau_{2,9} \tau_{2,12} l_5^2 l_{13}^2 + 22 \tau_{1,9} \tau_{2,17} l_5^2 l_{13}^2 - 14 \tau_{1,12} \tau_{2,17} l_5^2 l_{13}^2 + 30 \tau_{1,17} \tau_{2,17} l_5^2 l_{13}^2 - 8 \tau_{2,6} \tau_{2,17} l_5^2 l_{13}^2 + \\
& 46 \tau_{2,9} \tau_{2,17} l_5^2 l_{13}^2 + 8 \tau_{2,12} \tau_{2,17} l_5^2 l_{13}^2 - 22 \tau_{1,9} \tau_{4,12} l_5^2 l_{13}^2 - 12 \tau_{1,12} \tau_{4,12} l_5^2 l_{13}^2 - 6 \tau_{1,17} \tau_{4,12} l_5^2 l_{13}^2 + \\
& 4 \tau_{2,6} \tau_{4,12} l_5^2 l_{13}^2 - 12 \tau_{2,9} \tau_{4,12} l_5^2 l_{13}^2 - 4 \tau_{2,12} \tau_{4,12} l_5^2 l_{13}^2 - 4 \tau_{2,17} \tau_{4,12} l_5^2 l_{13}^2 + 18 \tau_{1,9} \tau_{4,17} l_5^2 l_{13}^2 + \\
& 18 \tau_{1,17} \tau_{4,17} l_5^2 l_{13}^2 + 8 \tau_{2,9} \tau_{4,17} l_5^2 l_{13}^2 - 2 \tau_{1,8}^2 l_{12}^2 l_{13}^2 - 2 \tau_{2,8}^2 l_{12}^2 l_{13}^2 - 7 \tau_{2,11}^2 l_{12}^2 l_{13}^2 - 10 \tau_{2,15}^2 l_{12}^2 l_{13}^2 - \\
& 12 \tau_{4,11}^2 l_{12}^2 l_{13}^2 - 4 \tau_{1,8} \tau_{2,11} l_{12}^2 l_{13}^2 + 4 \tau_{2,8} \tau_{2,11} l_{12}^2 l_{13}^2 - 6 \tau_{1,8} \tau_{2,15} l_{12}^2 l_{13}^2 - 8 \tau_{2,11} \tau_{2,15} l_{12}^2 l_{13}^2 - 7 \tau_{2,15} \tau_{4,8} l_{12}^2 l_{13}^2 - \\
& 11 \tau_{1,8} \tau_{4,11} l_{12}^2 l_{13}^2 - \tau_{2,8} \tau_{4,11} l_{12}^2 l_{13}^2 - 19 \tau_{2,11} \tau_{4,11} l_{12}^2 l_{13}^2 - 14 \tau_{2,15} \tau_{4,11} l_{12}^2 l_{13}^2 - 7 \tau_{4,8} \tau_{4,11} l_{12}^2 l_{13}^2 + \\
& 4 \tau_{1,15}^2 (6 l_5^2 l_{11}^2 - l_{12}^2 l_{13}^2) + \tau_{1,15} (4(14 \tau_{1,16} - 3 \tau_{2,12} + \tau_{2,14} + 4(\tau_{2,15} + \tau_{2,16} + \tau_{4,12} - 2 \tau_{4,14} + \tau_{4,16})) l_5^2 l_{11}^2 - \\
& (6 \tau_{1,8} + 10 \tau_{2,11} + 11 \tau_{2,15} + 7 \tau_{4,8} + 12 \tau_{4,11}) l_{12}^2 l_{13}^2) + \\
& 2(6(l_5^2 - l_{13}^2) \tau_{2,6}^2 + 2((- \tau_{2,10} + \tau_{2,11} + 3 \tau_{3,6} - \tau_{3,11} + \tau_{4,5} - 3 \tau_{4,6} + \tau_{4,11}) l_{13}^2 - \\
& (2 \tau_{2,8} - 2 \tau_{2,13} + \tau_{2,17} - 4 \tau_{3,6} + \tau_{3,8} - 2 \tau_{3,13} + \tau_{3,17} - 6 \tau_{4,6} - \tau_{4,17}) l_5^2) \tau_{2,6} + \\
& 2 \tau_{2,8}^2 l_5^2 + 2 \tau_{2,8} (-2 \tau_{2,13} + \tau_{2,17} - 5 \tau_{3,6} + \tau_{3,8} - 2 \tau_{3,13} + 2 \tau_{3,17} - \tau_{4,17}) l_5^2 + \\
& (2 \tau_{2,13}^2 - 2(\tau_{2,17} - 6 \tau_{3,6} + \tau_{3,8} - 2(\tau_{3,13} - \tau_{3,17} + \tau_{4,6}) - \tau_{4,17}) \tau_{2,13} + 4 \tau_{3,6}^2 + 2 \tau_{3,13}^2 + 10 \tau_{4,6}^2 - \\
& 4 \tau_{3,13} \tau_{3,17} + 2 \tau_{3,13} \tau_{4,6} - 2 \tau_{3,8} (\tau_{3,13} - 2(\tau_{3,17} + \tau_{4,6})) + 2 \tau_{3,13} \tau_{4,17} - 4 \tau_{3,17} \tau_{4,17} - 3 \tau_{4,6} \tau_{4,17} - \\
& 2 \tau_{2,17} (3 \tau_{3,6} - \tau_{3,8} + \tau_{3,13} + 2 \tau_{4,6} + \tau_{4,17}) + 2 \tau_{3,6} (-2 \tau_{3,8} + 5 \tau_{3,13} - 2 \tau_{3,17} + 2 \tau_{4,17})) l_5^2 - \\
& 2(2 \tau_{2,10}^2 + 3 \tau_{2,11} \tau_{2,10} + 2 \tau_{2,11}^2) l_{13}^2 + 2(-2 \tau_{2,11} \tau_{3,10} + 2 \tau_{3,6} \tau_{3,10} - \tau_{3,11} \tau_{3,10} - \\
& 2 \tau_{4,5} \tau_{3,10} - \tau_{3,6} \tau_{4,5} - \tau_{3,11} \tau_{4,5} - 2 \tau_{4,5} \tau_{4,6} + \tau_{3,5} (\tau_{3,6} - \tau_{3,11} + 2 \tau_{4,6} - 2 \tau_{4,11}) +
\end{aligned}$$

$$\begin{aligned}
& (4\tau_{2,11} - 2\tau_{3,6} + \tau_{3,11} + 2\tau_{4,5} - 2\tau_{4,6})\tau_{4,11} + \tau_{2,10}(\tau_{3,6} - 2\tau_{3,10} + \tau_{4,5} - \tau_{4,6} + 5\tau_{4,11}))l_{13}^2)l_{16}^2)t^2 + \\
& (s^2 - t^2 - u^2)(-48\tau_{12,16}l_5^2l_{11}^2 + l_{13}^2(24\tau_{8,15}l_{12}^2 + (-48\tau_{5,11} + 13l_6^2 - 24l_8^2)l_{16}^2) + \\
& 2l_5^2(9(2\tau_{8,9} - 3l_7^2)l_{12}^2 + (2l_{10}^2 - 19l_{11}^2)l_{12}^2 + 2l_8^2(6l_{11}^2 + 15l_{12}^2 - 22l_{13}^2) - \\
& 20\tau_{12,17}l_{13}^2 + 2l_6^2(2l_{11}^2 + 7l_{13}^2) + 8l_7^2(l_{13}^2 - 3l_{16}^2) + 2(21l_{12}^2 + 13l_{13}^2)l_{16}^2))t - \\
& 16s\tau_{1,14}(-6u\tau_{1,15} - 6u\tau_{1,16} + 2(t-u)\tau_{2,15} + u(-4\tau_{2,16} - \tau_{4,12} + \tau_{4,14})) \\
& l_5^2 \\
& l_{11}^2 + \\
& 4u^2(-2l_5^2l_{12}^2\tau_{1,8}^2 - 2l_{12}^2l_{13}^2\tau_{1,8}^2 + 8\tau_{1,9}l_5^2l_{12}^2\tau_{1,8} - 4\tau_{1,17}l_5^2l_{12}^2\tau_{1,8} - 9\tau_{2,8}l_5^2l_{12}^2\tau_{1,8} + \tau_{2,9}l_5^2l_{12}^2\tau_{1,8} - \\
& 4\tau_{2,16}l_5^2l_{12}^2\tau_{1,8} - 5\tau_{2,17}l_5^2l_{12}^2\tau_{1,8} - 8\tau_{3,8}l_5^2l_{12}^2\tau_{1,8} - 4\tau_{3,17}l_5^2l_{12}^2\tau_{1,8} - 4\tau_{2,11}l_{12}^2l_{13}^2\tau_{1,8} - \\
& 5\tau_{4,11}l_{12}^2l_{13}^2\tau_{1,8} + 4\tau_{4,14}^2l_5^2l_{11}^2 + 4\tau_{2,12}\tau_{2,15}l_5^2l_{11}^2 - 4\tau_{2,14}\tau_{2,15}l_5^2l_{11}^2 + 4\tau_{2,12}\tau_{2,16}l_5^2l_{11}^2 - \\
& 8\tau_{2,14}\tau_{2,16}l_5^2l_{11}^2 - 8\tau_{2,12}\tau_{4,12}l_5^2l_{11}^2 + 12\tau_{2,14}\tau_{4,12}l_5^2l_{11}^2 - 8\tau_{2,15}\tau_{4,12}l_5^2l_{11}^2 - 8\tau_{2,16}\tau_{4,12}l_5^2l_{11}^2 + \\
& 8\tau_{2,12}\tau_{4,14}l_5^2l_{11}^2 - 12\tau_{2,14}\tau_{4,14}l_5^2l_{11}^2 - 4\tau_{4,12}\tau_{4,14}l_5^2l_{11}^2 - 4\tau_{2,12}\tau_{4,16}l_5^2l_{11}^2 + 8\tau_{2,14}\tau_{4,16}l_5^2l_{11}^2 - \\
& 4\tau_{1,9}^2l_5^2l_{12}^2 - 2\tau_{1,17}^2l_5^2l_{12}^2 - 6\tau_{2,8}^2l_5^2l_{12}^2 - 4\tau_{2,9}^2l_5^2l_{12}^2 - 2\tau_{2,17}^2l_5^2l_{12}^2 - 4\tau_{3,8}^2l_5^2l_{12}^2 - 4\tau_{3,17}^2l_5^2l_{12}^2 + \\
& 6\tau_{1,9}\tau_{1,17}l_5^2l_{12}^2 + 7\tau_{1,9}\tau_{2,8}l_5^2l_{12}^2 - 6\tau_{1,17}\tau_{2,8}l_5^2l_{12}^2 - 13\tau_{1,9}\tau_{2,9}l_5^2l_{12}^2 + 2\tau_{1,17}\tau_{2,9}l_5^2l_{12}^2 + 6\tau_{2,8}\tau_{2,9}l_5^2l_{12}^2 - \\
& 6\tau_{1,9}\tau_{2,16}l_5^2l_{12}^2 + 4\tau_{1,17}\tau_{2,16}l_5^2l_{12}^2 + 6\tau_{2,8}\tau_{2,16}l_5^2l_{12}^2 - 2\tau_{2,9}\tau_{2,16}l_5^2l_{12}^2 + 3\tau_{1,9}\tau_{2,17}l_5^2l_{12}^2 - \\
& 6\tau_{1,17}\tau_{2,17}l_5^2l_{12}^2 - 8\tau_{2,8}\tau_{2,17}l_5^2l_{12}^2 + 4\tau_{2,9}\tau_{2,17}l_5^2l_{12}^2 + 2\tau_{2,16}\tau_{2,17}l_5^2l_{12}^2 + 10\tau_{1,9}\tau_{3,8}l_5^2l_{12}^2 - \\
& 2\tau_{1,17}\tau_{3,8}l_5^2l_{12}^2 - 6\tau_{2,8}\tau_{3,8}l_5^2l_{12}^2 + 12\tau_{2,9}\tau_{3,8}l_5^2l_{12}^2 - 2\tau_{2,17}\tau_{3,8}l_5^2l_{12}^2 + 6\tau_{1,9}\tau_{3,17}l_5^2l_{12}^2 - \\
& 6\tau_{1,17}\tau_{3,17}l_5^2l_{12}^2 - 6\tau_{2,8}\tau_{3,17}l_5^2l_{12}^2 + 6\tau_{2,9}\tau_{3,17}l_5^2l_{12}^2 + 6\tau_{2,16}\tau_{3,17}l_5^2l_{12}^2 - 6\tau_{2,17}\tau_{3,17}l_5^2l_{12}^2 - \\
& 8\tau_{3,8}\tau_{3,17}l_5^2l_{12}^2 + 2\tau_{1,16}^2l_5^2(8l_{11}^2 + l_{12}^2) + \tau_{1,16}l_5^2(4(\tau_{2,12} - 2\tau_{2,14} + 4(\tau_{4,12} - 2\tau_{4,14} + \tau_{4,16}))l_{11}^2 + \\
& (2\tau_{1,8} - 2\tau_{1,9} + 2\tau_{1,17} - \tau_{2,8} - 5\tau_{2,9} + \tau_{2,17} - 2\tau_{3,8} + 6\tau_{3,17})l_{12}^2) - 12\tau_{1,12}^2l_5^2l_{13}^2 + \\
& 6\tau_{1,17}^2l_5^2l_{13}^2 + 14\tau_{2,6}^2l_5^2l_{13}^2 - 4\tau_{2,9}^2l_5^2l_{13}^2 - 4\tau_{2,12}^2l_5^2l_{13}^2 + 6\tau_{2,17}^2l_5^2l_{13}^2 + 14\tau_{1,6}\tau_{1,12}l_5^2l_{13}^2 - \\
& 30\tau_{1,9}\tau_{1,12}l_5^2l_{13}^2 - 6\tau_{1,6}\tau_{1,17}l_5^2l_{13}^2 + 6\tau_{1,9}\tau_{1,17}l_5^2l_{13}^2 - 14\tau_{1,12}\tau_{1,17}l_5^2l_{13}^2 - 3\tau_{1,6}\tau_{2,6}l_5^2l_{13}^2 - \\
& 9\tau_{1,9}\tau_{2,6}l_5^2l_{13}^2 + 20\tau_{1,12}\tau_{2,6}l_5^2l_{13}^2 + 7\tau_{1,17}\tau_{2,6}l_5^2l_{13}^2 + 6\tau_{1,6}\tau_{2,9}l_5^2l_{13}^2 - 6\tau_{1,9}\tau_{2,9}l_5^2l_{13}^2 - \\
& 28\tau_{1,12}\tau_{2,9}l_5^2l_{13}^2 - 6\tau_{1,17}\tau_{2,9}l_5^2l_{13}^2 - 2\tau_{2,6}\tau_{2,9}l_5^2l_{13}^2 + 11\tau_{1,6}\tau_{2,12}l_5^2l_{13}^2 - 15\tau_{1,9}\tau_{2,12}l_5^2l_{13}^2 - \\
& 6\tau_{1,12}\tau_{2,12}l_5^2l_{13}^2 - 11\tau_{1,17}\tau_{2,12}l_5^2l_{13}^2 + 12\tau_{2,6}\tau_{2,12}l_5^2l_{13}^2 - 20\tau_{2,9}\tau_{2,12}l_5^2l_{13}^2 + 12\tau_{1,9}\tau_{2,17}l_5^2l_{13}^2 - \\
& 20\tau_{1,12}\tau_{2,17}l_5^2l_{13}^2 - 4\tau_{1,17}\tau_{2,17}l_5^2l_{13}^2 - 20\tau_{2,6}\tau_{2,17}l_5^2l_{13}^2 + 2\tau_{2,9}\tau_{2,17}l_5^2l_{13}^2 - 12\tau_{2,12}\tau_{2,17}l_5^2l_{13}^2 + \\
& 18\tau_{1,6}\tau_{4,12}l_5^2l_{13}^2 - 34\tau_{1,9}\tau_{4,12}l_5^2l_{13}^2 - 12\tau_{1,12}\tau_{4,12}l_5^2l_{13}^2 - 18\tau_{1,17}\tau_{4,12}l_5^2l_{13}^2 + 20\tau_{2,6}\tau_{4,12}l_5^2l_{13}^2 - \\
& 28\tau_{2,9}\tau_{4,12}l_5^2l_{13}^2 - 4\tau_{2,12}\tau_{4,12}l_5^2l_{13}^2 - 20\tau_{2,17}\tau_{4,12}l_5^2l_{13}^2 - 6\tau_{1,6}\tau_{4,17}l_5^2l_{13}^2 + 6\tau_{1,9}\tau_{4,17}l_5^2l_{13}^2 + \\
& 6\tau_{1,17}\tau_{4,17}l_5^2l_{13}^2 + 8\tau_{2,6}\tau_{4,17}l_5^2l_{13}^2 - 8\tau_{2,17}\tau_{4,17}l_5^2l_{13}^2 - 2\tau_{2,8}^2l_{12}^2l_{13}^2 - 7\tau_{2,11}^2l_{12}^2l_{13}^2 - 4\tau_{2,15}^2l_{12}^2l_{13}^2 + \\
& 4\tau_{2,8}\tau_{2,11}l_{12}^2l_{13}^2 - 6\tau_{2,8}\tau_{2,15}l_{12}^2l_{13}^2 + 10\tau_{2,11}\tau_{2,15}l_{12}^2l_{13}^2 - 7\tau_{2,15}\tau_{4,8}l_{12}^2l_{13}^2 - 7\tau_{2,8}\tau_{4,11}l_{12}^2l_{13}^2 + \\
& 5\tau_{2,11}\tau_{4,11}l_{12}^2l_{13}^2 - 2\tau_{2,15}\tau_{4,11}l_{12}^2l_{13}^2 - 7\tau_{4,8}\tau_{4,11}l_{12}^2l_{13}^2 + 2\tau_{1,15}^2(4l_5^2l_{11}^2 - 5l_{12}^2l_{13}^2) + \tau_{1,15} \\
& (4(6\tau_{1,16} + 3\tau_{2,12} - 3\tau_{2,14} + 3\tau_{4,12} - 7\tau_{4,14} + 4\tau_{4,16})l_5^2l_{11}^2 - (6\tau_{2,8} - 8\tau_{2,11} + 11\tau_{2,15} + 7\tau_{4,8} + 6\tau_{4,11})l_{12}^2l_{13}^2) + \\
& 2((4l_5^2 - 6l_{13}^2)\tau_{2,6}^2 + 2((-2\tau_{2,10} + \tau_{2,11} - \tau_{3,5} + 4\tau_{3,6} + \tau_{3,10} - \tau_{3,11})l_{13}^2 -
\end{aligned}$$

$$\begin{aligned}
& (5 \tau_{2,8} - 6 \tau_{2,13} + \tau_{2,17} - 7 \tau_{3,6} + 5 \tau_{3,8} - 6 \tau_{3,13} + \tau_{3,17} + \tau_{4,6} - 5 \tau_{4,17}) l_5^2 \tau_{2,6} + \\
& 2 \tau_{2,8}^2 l_5^2 + 2 \tau_{2,8} (-3 \tau_{2,13} + \tau_{2,17} - 9 \tau_{3,6} + 2 \tau_{3,8} - 3 \tau_{3,13} + 2 \tau_{3,17} - 3 \tau_{4,6} - 2 \tau_{4,17}) l_5^2 + \\
& (4 \tau_{2,13}^2 - 2 (\tau_{2,17} - 11 \tau_{3,6} + 3 \tau_{3,8} - 4 \tau_{3,13} + 2 \tau_{3,17} - 5 \tau_{4,6} - 3 \tau_{4,17}) \tau_{2,13} + 16 \tau_{3,6}^2 + 2 \tau_{3,8}^2 + \\
& 4 \tau_{3,13}^2 - 3 \tau_{4,6}^2 + 2 \tau_{4,17}^2 - 4 \tau_{3,13} \tau_{3,17} + 12 \tau_{3,13} \tau_{4,6} + 6 \tau_{3,13} \tau_{4,17} - 4 \tau_{3,17} \tau_{4,17} + 7 \tau_{4,6} \tau_{4,17} - \\
& 2 \tau_{2,17} (3 \tau_{3,6} - \tau_{3,8} + \tau_{3,13} + 2 \tau_{4,6} + \tau_{4,17}) - 2 \tau_{3,8} (3 \tau_{3,13} - 2 \tau_{3,17} + 3 \tau_{4,6} + 2 \tau_{4,17}) + \\
& 2 \tau_{3,6} (-9 \tau_{3,8} + 12 \tau_{3,13} - 2 \tau_{3,17} + 2 \tau_{4,6} + 9 \tau_{4,17})) l_5^2 - 2 (\tau_{2,10}^2 + (\tau_{3,5} - 3 \tau_{2,11}) \tau_{2,10} + 2 \tau_{2,11}^2) l_{13}^2 + \\
& 2 (-4 \tau_{3,11}^2 - (\tau_{4,5} - 9 \tau_{4,11}) \tau_{3,11} - \tau_{3,6} \tau_{4,5} - 2 (3 \tau_{3,10}^2 + \tau_{2,11} (4 \tau_{3,10} + 3 \tau_{3,11} - 5 \tau_{4,11})) + \\
& \tau_{3,5} (\tau_{3,6} - \tau_{3,11} + 2 \tau_{4,6} - 2 \tau_{4,11}) + \tau_{2,10} (2 \tau_{3,6} - 3 \tau_{3,10} + 6 \tau_{4,11}) + \\
& \tau_{3,10} (-7 \tau_{3,11} - 2 \tau_{4,5} + 16 \tau_{4,11}) - 2 (5 \tau_{4,11}^2 + \tau_{4,5} (\tau_{4,6} - \tau_{4,11}))) l_{13}^2 l_{16}^2 + \\
& 4 (s^2 - t^2 - u^2) (-l_5^2 l_{13}^2 \tau_{1,6}^2 + 9 \tau_{1,9} l_5^2 l_{13}^2 \tau_{1,6} + 7 \tau_{1,12} l_5^2 l_{13}^2 \tau_{1,6} - 7 \tau_{1,17} l_5^2 l_{13}^2 \tau_{1,6} - 36 \tau_{2,6} l_5^2 l_{13}^2 \tau_{1,6} + \\
& 15 \tau_{2,9} l_5^2 l_{13}^2 \tau_{1,6} + 16 \tau_{2,12} l_5^2 l_{13}^2 \tau_{1,6} + 27 \tau_{2,17} l_5^2 l_{13}^2 \tau_{1,6} + 12 \tau_{4,12} l_5^2 l_{13}^2 \tau_{1,6} - \\
& 12 \tau_{4,17} l_5^2 l_{13}^2 \tau_{1,6} + 4 \tau_{4,14}^2 l_5^2 l_{11}^2 - 4 \tau_{2,12} \tau_{2,15} l_5^2 l_{11}^2 + 4 \tau_{2,14} \tau_{2,15} l_5^2 l_{11}^2 - 4 \tau_{2,12} \tau_{2,16} l_5^2 l_{11}^2 - \\
& 10 \tau_{2,12} \tau_{4,12} l_5^2 l_{11}^2 + 14 \tau_{2,14} \tau_{4,12} l_5^2 l_{11}^2 - 6 \tau_{2,15} \tau_{4,12} l_5^2 l_{11}^2 - 8 \tau_{2,16} \tau_{4,12} l_5^2 l_{11}^2 + \\
& 10 \tau_{2,12} \tau_{4,14} l_5^2 l_{11}^2 - 14 \tau_{2,14} \tau_{4,14} l_5^2 l_{11}^2 - 2 \tau_{2,15} \tau_{4,14} l_5^2 l_{11}^2 - 4 \tau_{4,12} \tau_{4,14} l_5^2 l_{11}^2 - \\
& 4 \tau_{2,12} \tau_{4,16} l_5^2 l_{11}^2 + 8 \tau_{2,14} \tau_{4,16} l_5^2 l_{11}^2 - 2 \tau_{4,12} \tau_{4,16} l_5^2 l_{11}^2 + 2 \tau_{4,14} \tau_{4,16} l_5^2 l_{11}^2 - 3 \tau_{1,8}^2 l_5^2 l_{12}^2 - \\
& 4 \tau_{1,9}^2 l_5^2 l_{12}^2 - 2 \tau_{1,17}^2 l_5^2 l_{12}^2 - 3 \tau_{2,8}^2 l_5^2 l_{12}^2 - 4 \tau_{2,9}^2 l_5^2 l_{12}^2 + 3 \tau_{2,16}^2 l_5^2 l_{12}^2 - 2 \tau_{2,17}^2 l_5^2 l_{12}^2 - \\
& 4 \tau_{3,8}^2 l_5^2 l_{12}^2 - 4 \tau_{3,17}^2 l_5^2 l_{12}^2 + 6 \tau_{1,8} \tau_{1,9} l_5^2 l_{12}^2 - 5 \tau_{1,8} \tau_{1,17} l_5^2 l_{12}^2 + 3 \tau_{1,9} \tau_{1,17} l_5^2 l_{12}^2 - \\
& 8 \tau_{1,8} \tau_{2,8} l_5^2 l_{12}^2 + 2 \tau_{1,9} \tau_{2,8} l_5^2 l_{12}^2 - 5 \tau_{1,17} \tau_{2,8} l_5^2 l_{12}^2 + 2 \tau_{1,8} \tau_{2,9} l_5^2 l_{12}^2 - 14 \tau_{1,9} \tau_{2,9} l_5^2 l_{12}^2 + \\
& 6 \tau_{2,8} \tau_{2,9} l_5^2 l_{12}^2 - 5 \tau_{1,8} \tau_{2,16} l_5^2 l_{12}^2 - 4 \tau_{1,9} \tau_{2,16} l_5^2 l_{12}^2 + 2 \tau_{2,8} \tau_{2,16} l_5^2 l_{12}^2 - 5 \tau_{1,8} \tau_{2,17} l_5^2 l_{12}^2 - \\
& 6 \tau_{1,17} \tau_{2,17} l_5^2 l_{12}^2 - 5 \tau_{2,8} \tau_{2,17} l_5^2 l_{12}^2 + 3 \tau_{2,9} \tau_{2,17} l_5^2 l_{12}^2 - 7 \tau_{1,8} \tau_{3,8} l_5^2 l_{12}^2 + 11 \tau_{1,9} \tau_{3,8} l_5^2 l_{12}^2 - \\
& 2 \tau_{1,17} \tau_{3,8} l_5^2 l_{12}^2 - 7 \tau_{2,8} \tau_{3,8} l_5^2 l_{12}^2 + 11 \tau_{2,9} \tau_{3,8} l_5^2 l_{12}^2 - \tau_{2,16} \tau_{3,8} l_5^2 l_{12}^2 - 2 \tau_{2,17} \tau_{3,8} l_5^2 l_{12}^2 - \\
& 5 \tau_{1,8} \tau_{3,17} l_5^2 l_{12}^2 + 6 \tau_{1,9} \tau_{3,17} l_5^2 l_{12}^2 - 6 \tau_{1,17} \tau_{3,17} l_5^2 l_{12}^2 - 5 \tau_{2,8} \tau_{3,17} l_5^2 l_{12}^2 + 6 \tau_{2,9} \tau_{3,17} l_5^2 l_{12}^2 + \\
& 6 \tau_{2,16} \tau_{3,17} l_5^2 l_{12}^2 - 6 \tau_{2,17} \tau_{3,17} l_5^2 l_{12}^2 - 8 \tau_{3,8} \tau_{3,17} l_5^2 l_{12}^2 + 3 \tau_{1,16}^2 l_5^2 (8 l_{11}^2 + l_{12}^2) + \\
& \tau_{1,16} l_5^2 (8 (-\tau_{2,12} + \tau_{2,15} + \tau_{2,16} + 2 (\tau_{4,12} - 2 \tau_{4,14} + \tau_{4,16})) l_{11}^2 + (2 \tau_{1,8} - 5 \tau_{2,8} - 4 \tau_{2,9} + 4 \tau_{2,16} - \tau_{3,8} + 6 \tau_{3,17}) l_{12}^2) - \\
& 8 \tau_{1,9}^2 l_5^2 l_{13}^2 - 10 \tau_{1,12}^2 l_5^2 l_{13}^2 + 8 \tau_{1,17}^2 l_5^2 l_{13}^2 - 27 \tau_{2,6}^2 l_5^2 l_{13}^2 - 13 \tau_{2,9}^2 l_5^2 l_{13}^2 - 6 \tau_{2,12}^2 l_5^2 l_{13}^2 - \\
& 27 \tau_{2,17}^2 l_5^2 l_{13}^2 - 19 \tau_{1,9} \tau_{1,12} l_5^2 l_{13}^2 - 7 \tau_{1,12} \tau_{1,17} l_5^2 l_{13}^2 + 26 \tau_{1,9} \tau_{2,6} l_5^2 l_{13}^2 + 15 \tau_{1,12} \tau_{2,6} l_5^2 l_{13}^2 + \\
& 30 \tau_{1,17} \tau_{2,6} l_5^2 l_{13}^2 - 25 \tau_{1,9} \tau_{2,9} l_5^2 l_{13}^2 - 19 \tau_{1,12} \tau_{2,9} l_5^2 l_{13}^2 - 13 \tau_{1,17} \tau_{2,9} l_5^2 l_{13}^2 + 44 \tau_{2,6} \tau_{2,9} l_5^2 l_{13}^2 - \\
& 24 \tau_{1,9} \tau_{2,12} l_5^2 l_{13}^2 - 8 \tau_{1,12} \tau_{2,12} l_5^2 l_{13}^2 - 16 \tau_{1,17} \tau_{2,12} l_5^2 l_{13}^2 + 30 \tau_{2,6} \tau_{2,12} l_5^2 l_{13}^2 - 26 \tau_{2,9} \tau_{2,12} l_5^2 l_{13}^2 - \\
& 17 \tau_{1,9} \tau_{2,17} l_5^2 l_{13}^2 - 15 \tau_{1,12} \tau_{2,17} l_5^2 l_{13}^2 - 21 \tau_{1,17} \tau_{2,17} l_5^2 l_{13}^2 + 54 \tau_{2,6} \tau_{2,17} l_5^2 l_{13}^2 - 40 \tau_{2,9} \tau_{2,17} l_5^2 l_{13}^2 - \\
& 30 \tau_{2,12} \tau_{2,17} l_5^2 l_{13}^2 - 28 \tau_{1,9} \tau_{4,12} l_5^2 l_{13}^2 - 12 \tau_{1,12} \tau_{4,12} l_5^2 l_{13}^2 - 12 \tau_{1,17} \tau_{4,12} l_5^2 l_{13}^2 + \\
& 12 \tau_{2,6} \tau_{4,12} l_5^2 l_{13}^2 - 20 \tau_{2,9} \tau_{4,12} l_5^2 l_{13}^2 - 4 \tau_{2,12} \tau_{4,12} l_5^2 l_{13}^2 - 12 \tau_{2,17} \tau_{4,12} l_5^2 l_{13}^2 + 12 \tau_{1,9} \tau_{4,17} l_5^2 l_{13}^2 + \\
& 12 \tau_{1,17} \tau_{4,17} l_5^2 l_{13}^2 + 4 \tau_{2,6} \tau_{4,17} l_5^2 l_{13}^2 + 4 \tau_{2,9} \tau_{4,17} l_5^2 l_{13}^2 - 4 \tau_{2,17} \tau_{4,17} l_5^2 l_{13}^2 + 2 \tau_{1,8}^2 l_{12}^2 l_{13}^2 + \\
& 2 \tau_{2,8}^2 l_{12}^2 l_{13}^2 - \tau_{2,11}^2 l_{12}^2 l_{13}^2 + 5 \tau_{2,15}^2 l_{12}^2 l_{13}^2 + 6 \tau_{4,11}^2 l_{12}^2 l_{13}^2 - 3 \tau_{1,8} \tau_{2,15} l_{12}^2 l_{13}^2 + \\
& \tau_{2,8} \tau_{2,15} l_{12}^2 l_{13}^2 - 5 \tau_{2,11} \tau_{2,15} l_{12}^2 l_{13}^2 - 7 \tau_{2,15} \tau_{4,8} l_{12}^2 l_{13}^2 - 4 \tau_{1,8} \tau_{4,11} l_{12}^2 l_{13}^2 - 4 \tau_{2,8} \tau_{4,11} l_{12}^2 l_{13}^2 -
\end{aligned}$$

$$\begin{aligned}
& \tau_{2,11} \tau_{4,11} l_{12}^2 l_{13}^2 + 10 \tau_{2,15} \tau_{4,11} l_{12}^2 l_{13}^2 - 7 \tau_{4,8} \tau_{4,11} l_{12}^2 l_{13}^2 + \tau_{1,15}^2 (16 l_5^2 l_{11}^2 + 5 l_{12}^2 l_{13}^2) + \\
& \tau_{1,15} (2 (20 \tau_{1,16} - 2 \tau_{2,14} + 4 \tau_{2,15} + 4 \tau_{2,16} + 7 \tau_{4,12} - 15 \tau_{4,14} + 8 \tau_{4,16}) l_5^2 l_{11}^2 + \\
& (\tau_{1,8} - 3 \tau_{2,8} + 5 \tau_{2,11} + 7 \tau_{2,15} - 7 \tau_{4,8} + 15 \tau_{4,11}) l_{12}^2 l_{13}^2) + \\
& (2 (l_5^2 - 6 l_{13}^2) \tau_{2,6}^2 + 2 ((-7 \tau_{2,8} + 8 \tau_{2,13} - 2 \tau_{2,17} + 5 \tau_{3,6} - 6 \tau_{3,8} + 8 \tau_{3,13} - 2 \tau_{3,17} - 7 \tau_{4,6} + 6 \tau_{4,17}) l_5^2 + \\
& (-3 \tau_{2,10} + 2 \tau_{2,11} - \tau_{3,5} + 7 \tau_{3,6} + \tau_{3,10} - 2 \tau_{3,11} + \tau_{4,5} - 3 \tau_{4,6} + \tau_{4,11}) l_{13}^2) \tau_{2,6} + 4 \tau_{2,8}^2 l_5^2 + 6 \tau_{2,13}^2 l_5^2 + \\
& 12 \tau_{3,6}^2 l_5^2 + 2 \tau_{3,8}^2 l_5^2 + 6 \tau_{3,13}^2 l_5^2 - 17 \tau_{4,6}^2 l_5^2 + 2 \tau_{4,17}^2 l_5^2 - 12 \tau_{2,17} \tau_{3,6} l_5^2 + 4 \tau_{2,17} \tau_{3,8} l_5^2 - 22 \tau_{3,6} \tau_{3,8} l_5^2 - \\
& 4 \tau_{2,17} \tau_{3,13} l_5^2 + 34 \tau_{3,6} \tau_{3,13} l_5^2 - 8 \tau_{3,8} \tau_{3,13} l_5^2 - 8 \tau_{3,6} \tau_{3,17} l_5^2 + 8 \tau_{3,8} \tau_{3,17} l_5^2 - 8 \tau_{3,13} \tau_{3,17} l_5^2 - 8 \tau_{2,17} \tau_{4,6} l_5^2 - \\
& 20 \tau_{3,6} \tau_{4,6} l_5^2 - 2 \tau_{3,8} \tau_{4,6} l_5^2 + 14 \tau_{3,13} \tau_{4,6} l_5^2 - 4 \tau_{2,17} \tau_{4,17} l_5^2 + 22 \tau_{3,6} \tau_{4,17} l_5^2 - 4 \tau_{3,8} \tau_{4,17} l_5^2 + 8 \tau_{3,13} \tau_{4,17} l_5^2 - \\
& 8 \tau_{3,17} \tau_{4,17} l_5^2 + 4 \tau_{4,6} \tau_{4,17} l_5^2 + 2 \tau_{2,13} (-2 \tau_{2,17} + 17 \tau_{3,6} - 4 \tau_{3,8} + 6 \tau_{3,13} - 4 \tau_{3,17} + 7 \tau_{4,6} + 4 \tau_{4,17}) l_5^2 - \\
& 2 \tau_{2,8} (5 \tau_{2,13} - 2 \tau_{2,17} + 14 \tau_{3,6} - 3 \tau_{3,8} + 5 \tau_{3,13} - 4 \tau_{3,17} + 3 (\tau_{4,6} + \tau_{4,17})) l_5^2 + 2 (\tau_{2,10}^2 - \tau_{3,5} \tau_{2,10} - 4 \tau_{2,11}^2) \\
& l_{13}^2 + 2 (\tau_{2,10} (3 \tau_{3,6} - 9 \tau_{3,10} - 6 \tau_{3,11} + \tau_{4,5} - \tau_{4,6} + 15 \tau_{4,11}) + 2 (-\tau_{3,10}^2 - \tau_{3,11} \tau_{3,10} - 2 \tau_{4,5} \tau_{3,10} - 3 \\
& \tau_{4,11}^2 - \tau_{3,11} \tau_{4,5} - 2 \tau_{4,5} \tau_{4,6} + \tau_{3,5} (\tau_{3,6} - \tau_{3,11} + 2 \tau_{4,6} - 2 \tau_{4,11}) + \tau_{3,6} (\tau_{3,10} - \tau_{4,5} - \tau_{4,11}) + \\
& (4 \tau_{3,10} + 2 (\tau_{3,11} + \tau_{4,5}) - \tau_{4,6}) \tau_{4,11} + \tau_{2,11} (-5 \tau_{3,10} - 3 \tau_{3,11} + 7 \tau_{4,11})) l_{13}^2) l_{16}^2) - \\
& 4 u^3 (8 \tau_{12,16} l_5^2 l_{11}^2 + 4 l_{13}^2 ((2 \tau_{5,11} - 2 l_6^2 + l_8^2) l_{16}^2 - \tau_{8,15} l_{12}^2) + l_5^2 (-6 \tau_{8,9} l_{12}^2 + 2 l_{10}^2 l_{12}^2 + 7 l_{11}^2 l_{12}^2 - 14 l_{16}^2 l_{12}^2 - \\
& 2 l_8^2 (2 l_{11}^2 + 5 l_{12}^2 - 6 l_{13}^2) + 12 \tau_{12,17} l_{13}^2 - l_6^2 (3 l_{11}^2 + 10 l_{13}^2) + 2 l_{13}^2 l_{16}^2 + l_7^2 (l_{11}^2 + 10 l_{12}^2 + 8 l_{16}^2))) + \\
& u (s^2 - t^2 - u^2) (-48 \tau_{12,16} l_5^2 l_{11}^2 + l_{13}^2 (24 \tau_{8,15} l_{12}^2 + (-48 \tau_{5,11} + 29 l_6^2 - 24 l_8^2) l_{16}^2) + \\
& 2 l_5^2 (18 \tau_{8,9} l_{12}^2 + 2 l_{10}^2 l_{12}^2 - 19 l_{11}^2 l_{12}^2 + 42 l_{16}^2 l_{12}^2 + 2 l_8^2 (6 l_{11}^2 + 15 l_{12}^2 - 20 l_{13}^2) - \\
& 28 \tau_{12,17} l_{13}^2 + l_6^2 (7 l_{11}^2 + 22 l_{13}^2) + 12 l_{13}^2 l_{16}^2 - l_7^2 (l_{11}^2 + 27 l_{12}^2 - 4 l_{13}^2 + 20 l_{16}^2))))))
\end{aligned}$$

■  $N_{26}^{(7)}$

$$\begin{aligned}
& -\frac{1}{8} l_5^2 (l_{11}^2 l_{12}^2 (\tau_{1,15} (5 s^2 + t^2 - u^2) + \tau_{1,16} (-7 s^2 + t^2 - u^2) + \\
& s^2 (4 \tau_{2,14} + 5 \tau_{2,15} - 7 \tau_{2,16} + 34 (\tau_{4,13} + \tau_{4,14}) - 20 \tau_{4,16}) - (4 \tau_{2,13} + \tau_{2,15} + \tau_{2,16}) (t - u) (t + u)) + \\
& 2 l_{16}^2 (l_{13}^2 (\tau_{2,6} (23 s^2 - 17 t^2 + 11 u^2) + \tau_{2,10} (12 s^2 - 11 t^2 + 9 u^2) + \tau_{4,14} (-9 s^2 - 7 t^2 + 7 u^2) - \\
& 20 s^2 \tau_{2,11} + s^2 \tau_{3,10} - 8 s^2 \tau_{3,11} + 11 s^2 \tau_{3,14} - 11 s^2 \tau_{4,11} + 12 s t \tau_{2,14} + \\
& 11 t^2 \tau_{3,10} - 7 t^2 \tau_{3,14} - 11 t^2 \tau_{4,11} - 9 u^2 \tau_{3,10} + 7 u^2 \tau_{3,14} + 9 u^2 \tau_{4,11}) + \\
& \tau_{4,6} (6 l_{12}^2 s^2 + 4 l_{13}^2 t (u - t)) + 2 s \tau_{3,6} (l_{12}^2 s - l_{13}^2 (9 t + 8 u))) + 4 l_{11}^2 l_{12}^2 s^2 \tau_{1,14} + 4 l_{11}^2 l_{12}^2 \tau_{1,13} (t^2 - u^2))
\end{aligned}$$

■  $N_{26}^{(8)}$

0
