# Supplementary material for: The Ultraviolet Behavior of N=8 Supergravity at Four Loops
Source: arXiv:0905.2326 ancillary file (2012-01-08)
Supplement: Supplementary file 27 [file SUGRA32.pdf]

## Integral 32: $\mathcal{I}_{32}$

$\mathcal{N} = 8$  four-point four-loop amplitude.

### ■ 2D plot of graph associated with $\mathcal{I}_{32}$

This fixes the labelling associated with the numerator expressions given below.

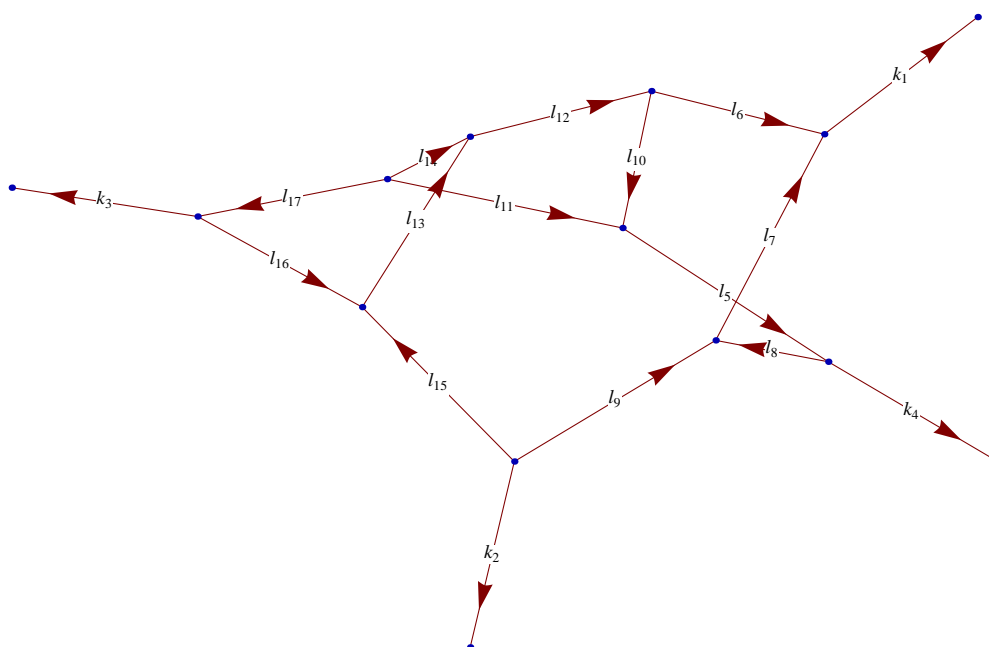

When using MathPlayer, by clicking three times (holding the click on the third click) directly on a vertex, one is able to move that vertex around, and its associated edges follow elastically. This functionality is absent when viewing as a pdf.

*Note: propagators for certain graphs were relabeled in the manuscript due to size constraints. The labels given in `aux/rawData/Neq8FourLoops.m` should be used for verification purposes.*

### ■ 3D plot of graph associated with $\mathcal{I}_{32}$

3D PLOT UNAVAILABLE FOR PDF. Please see .nb version for the 3D figure.

When using MathPlayer, by clicking anywhere in the image and dragging one should be able to rotate this 3D image. By holding (ALT) or (COMMAND) while clicking and moving the mouse up/down one should be able to zoom in/out. This functionality is absent when viewing as a pdf.

### "Vertex Form" of graph associated with $I_{32}$

This function returns the graph associated with the integral object in a vertex representation. This can be used as a way of specifying the topology of a graph using trivalent (cubic) vertices,  $\text{gVertex}[p_a, p_b, p_c]$ , where  $\{p_a, p_b, p_c\}$  are momenta labeling the propagators (edges) of the graph, and is understood that the edge labelled by  $p_a$  flows into the edge labelled by  $-p_a$ . Additionally, each vertex represents the manifest conservation of ( $D$  - dimensional) momenta :

$$\text{gVertex}[\{p_1, p_2, p_3\}] \iff (p_1 + p_2 + p_3 = 0)$$

$$\{\text{gVertex}(\{k_1, -l_7, -l_6\}), \text{gVertex}(\{k_2, l_9, l_{15}\}), \text{gVertex}(\{k_3, -l_{17}, l_{16}\}), \text{gVertex}(\{k_4, -l_5, l_8\}), \text{gVertex}(\{l_5, -l_{10}, -l_{11}\}), \\ \text{gVertex}(\{l_6, -l_{12}, l_{10}\}), \text{gVertex}(\{l_7, -l_8, -l_9\}), \text{gVertex}(\{l_{11}, l_{14}, l_{17}\}), \text{gVertex}(\{l_{12}, -l_{13}, -l_{14}\}), \text{gVertex}(\{l_{13}, -l_{15}, -l_{16}\})\}$$

### ■ Numerator expression for integral 32:

The following notation is used:  $\tau_{i,j} \equiv \begin{cases} 2 k_i \cdot l_j & \text{if } i \leq 4, j > 4 \\ 2 l_i \cdot l_j & \text{if } i, j > 4 \end{cases}$ .

$$s \equiv 2 k_1 \cdot k_2 = 2 k_3 \cdot k_4$$

We use  $s, t, u$  to represent the traditional Mandelstam variables for massless external four-point momenta:  $t \equiv 2 k_1 \cdot k_4 = 2 k_2 \cdot k_3$ .

$$u \equiv 2 k_1 \cdot k_3 = 2 k_2 \cdot k_4$$

Furthermore we use the shorthand  $(l_i)^2$  to represent the lorentz square:  $(l_i)^2 = l_i \cdot l_i$ .

The total numerator  $\mathcal{N}_{32}$  is given by summing over the following terms, distinguished here by explicit dependence on loop momenta:  $\mathcal{N}_{32} = \sum_{i=0}^8 \mathcal{N}_{32}^{(i)}$ :

■  $\mathcal{N}_{32}^{(0)}$

$$0$$

■  $\mathcal{N}_{32}^{(1)}$

$$0$$

■  $\mathcal{N}_{32}^{(2)}$

$$-\frac{1}{2} l_7^2 s^2 t^3$$

■  $\mathcal{N}_{32}^{(3)}$

$$\frac{1}{2} t^2$$

$$\begin{aligned} & (-2 l_6^2 s^2 \tau_{3,7} + 4 l_6^2 s^2 \tau_{3,10} - 4 l_6^2 s^2 \tau_{4,7} + 2 l_6^2 s^2 \tau_{4,10} + 3 l_7^2 s^2 \tau_{1,5} + 3 l_7^2 s^2 \tau_{1,6} + 4 l_7^2 s^2 \tau_{4,6} + 2 l_6^2 s \tau_{2,7} (t + 3 u) - 2 l_6^2 t^2 \tau_{3,10} + \\ & 2 l_6^2 t^2 \tau_{4,7} + 2 l_6^2 \tau_{2,10} (t + 2 u)^2 - 4 l_6^2 u^2 \tau_{3,8} + 4 l_6^2 u^2 \tau_{3,10} - 2 l_6^2 u^2 \tau_{4,7} - 2 l_6^2 u^2 \tau_{4,10} - 2 l_8^2 u^2 (2 \tau_{1,5} + \tau_{4,5} - 2 \tau_{4,7})) \end{aligned}$$

■  $N_{32}^{(4)}$ 

$$\begin{aligned}
& -4 l_5^2 l_6^2 t^4 + \frac{11}{4} l_5^2 l_7^2 t^4 + 2 l_6^2 l_8^2 t^4 - 3 l_7^2 l_8^2 t^4 + 3 l_5^2 l_{12}^2 t^4 - 2 \tau_{3,7}^2 l_6^2 t^3 + 2 \tau_{3,10}^2 l_6^2 t^3 - 2 \tau_{2,10} \tau_{3,8} l_6^2 t^3 + \\
& 2 \tau_{3,7} \tau_{3,8} l_6^2 t^3 + 2 \tau_{2,10} \tau_{3,10} l_6^2 t^3 - 2 \tau_{3,8} \tau_{3,10} l_6^2 t^3 + 2 \tau_{3,7} \tau_{4,7} l_6^2 t^3 + 2 \tau_{3,8} \tau_{4,7} l_6^2 t^3 - 4 \tau_{3,10} \tau_{4,7} l_6^2 t^3 - \\
& 2 \tau_{3,8} \tau_{4,10} l_6^2 t^3 + 2 \tau_{3,10} \tau_{4,10} l_6^2 t^3 - \frac{3}{2} \tau_{1,6}^2 l_7^2 t^3 - 3 \tau_{4,6}^2 l_7^2 t^3 - 4 \tau_{1,6} \tau_{4,6} l_7^2 t^3 + 4 (-s^2 + t^2 + u^2) l_5^2 l_6^2 t^2 - \\
& \frac{15}{4} (-s^2 + t^2 + u^2) l_5^2 l_7^2 t^2 + 4 (-s^2 + t^2 + u^2) l_6^2 l_8^2 t^2 + 2 (-s^2 + t^2 + u^2) l_7^2 l_8^2 t^2 - 3 (-s^2 + t^2 + u^2) l_5^2 l_{12}^2 t^2 + \\
& 2 (-s^2 + t^2 + u^2) \tau_{3,7}^2 l_6^2 t - 2 (-s^2 + t^2 + u^2) \tau_{3,10}^2 l_6^2 t - (-s^2 + t^2 + u^2) \tau_{2,10} \tau_{3,7} l_6^2 t + 3 (-s^2 + t^2 + u^2) \tau_{2,10} \tau_{3,8} l_6^2 t - \\
& 3 (-s^2 + t^2 + u^2) \tau_{3,7} \tau_{3,8} l_6^2 t - 2 (-s^2 + t^2 + u^2) \tau_{2,10} \tau_{3,10} l_6^2 t - (-s^2 + t^2 + u^2) \tau_{3,7} \tau_{3,10} l_6^2 t + 4 (-s^2 + t^2 + u^2) \tau_{3,8} \tau_{3,10} l_6^2 t + \\
& 2 s \tau_{2,7} (2 u \tau_{3,7} - (t + 2 u) \tau_{3,8} + t \tau_{3,10}) l_6^2 t - (-s^2 + t^2 + u^2) \tau_{3,7} \tau_{4,7} l_6^2 t - 2 (-s^2 + t^2 + u^2) \tau_{3,8} \tau_{4,7} l_6^2 t + \\
& 3 (-s^2 + t^2 + u^2) \tau_{3,10} \tau_{4,7} l_6^2 t + (-s^2 + t^2 + u^2) \tau_{3,8} \tau_{4,10} l_6^2 t - (-s^2 + t^2 + u^2) \tau_{3,10} \tau_{4,10} l_6^2 t + \frac{5}{2} u (-s^2 + t^2 + u^2) l_5^2 l_6^2 t + \\
& \frac{3}{2} (-s^2 + t^2 + u^2) \tau_{1,6}^2 l_7^2 t + 3 (-s^2 + t^2 + u^2) \tau_{4,6}^2 l_7^2 t + 4 (-s^2 + t^2 + u^2) \tau_{1,6} \tau_{4,6} l_7^2 t + \frac{21}{8} u (-s^2 + t^2 + u^2) l_5^2 l_7^2 t - \\
& (-s^2 + t^2 + u^2) \tau_{3,7} \tau_{4,5} l_8^2 t + 2 (-s^2 + t^2 + u^2) \tau_{3,7} \tau_{4,7} l_8^2 t + 5 u (-s^2 + t^2 + u^2) l_6^2 l_8^2 t + 2 u (-s^2 + t^2 + u^2) l_7^2 l_8^2 t - \\
& \frac{3}{2} u (-s^2 + t^2 + u^2) l_5^2 l_{12}^2 t + u^2 \tau_{1,5}^4 + u^2 \tau_{2,5}^4 + s^2 \tau_{3,6}^4 + 2 s (t + 2 u) \tau_{2,5} \tau_{3,6}^3 + (3 s^2 - 2 t^2 + 3 u^2) \tau_{2,5}^2 \tau_{3,6}^2 - \\
& 2 u (t + 2 u) \tau_{2,5}^3 \tau_{3,6} + 2 u \tau_{1,5}^3 (2 u \tau_{2,5} - (t + 2 u) \tau_{3,6}) + u (-s^2 + t^2 + u^2) \tau_{3,7}^2 l_6^2 - u (-s^2 + t^2 + u^2) \tau_{3,8}^2 l_6^2 - \\
& 2 u (-s^2 + t^2 + u^2) \tau_{2,10} \tau_{3,7} l_6^2 + 2 u (-s^2 + t^2 + u^2) \tau_{2,10} \tau_{3,8} l_6^2 - 2 u (-s^2 + t^2 + u^2) \tau_{3,7} \tau_{3,10} l_6^2 + 2 u (-s^2 + t^2 + u^2) \tau_{3,8} \tau_{3,10} l_6^2 + \\
& u (-s^2 + t^2 + u^2) \tau_{3,7} \tau_{4,10} l_6^2 - u (-s^2 + t^2 + u^2) \tau_{3,8} \tau_{4,10} l_6^2 + \frac{3}{4} u (-s^2 + t^2 + u^2) \tau_{1,6}^2 l_7^2 + \frac{3}{2} u (-s^2 + t^2 + u^2) \tau_{4,6}^2 l_7^2 + \\
& 2 u (-s^2 + t^2 + u^2) \tau_{1,6} \tau_{4,6} l_7^2 - 7 u^4 l_5^2 l_7^2 + 9 u^2 (-s^2 + t^2 + u^2) l_5^2 l_7^2 - u (-s^2 + t^2 + u^2) \tau_{4,5}^2 l_8^2 - 3 u (-s^2 + t^2 + u^2) \tau_{4,7}^2 l_8^2 + \\
& 3 u (-s^2 + t^2 + u^2) \tau_{4,5} \tau_{4,7} l_8^2 + \tau_{1,5} (4 u^2 \tau_{2,5}^3 - 6 u (t + 2 u) \tau_{3,6} \tau_{2,5}^2 + 2 (3 s^2 - 2 t^2 + 3 u^2) \tau_{3,6}^2 \tau_{2,5} + \\
& 2 s (t + 2 u) \tau_{3,6}^3 - s^2 t (3 \tau_{1,6} + 4 \tau_{4,6}) l_7^2 + (s^2 - t^2 - u^2) (2 t \tau_{3,7} + 3 u (\tau_{4,5} - 2 \tau_{4,7})) l_8^2) + \\
& \frac{1}{2} \tau_{1,5}^2 (12 u^2 \tau_{2,5}^2 - 12 u (t + 2 u) \tau_{3,6} \tau_{2,5} + (6 s^2 - 4 t^2 + 6 u^2) \tau_{3,6}^2 - 3 t (s^2 l_7^2 - 4 u^2 l_8^2)) + \\
& (t^4 + u^3 t + (t^2 - s^2) u t + 2 (t^2 - s^2) u^2) l_6^2 l_{15}^2
\end{aligned}$$

■  $N_{32}^{(5)}$ 

$$\begin{aligned}
& 2\tau_{2,8}l_5^2l_6^2t^3 - 4\tau_{2,11}l_5^2l_6^2t^3 + 2\tau_{3,8}l_5^2l_6^2t^3 - 4\tau_{3,11}l_5^2l_6^2t^3 + 2\tau_{4,8}l_5^2l_6^2t^3 + 2\tau_{4,9}l_5^2l_6^2t^3 - 4\tau_{4,11}l_5^2l_6^2t^3 + \tau_{1,9}l_5^2l_7^2t^3 + \\
& \frac{17}{4}\tau_{1,14}l_5^2l_7^2t^3 + 3\tau_{2,14}l_5^2l_7^2t^3 - \frac{5}{4}\tau_{2,16}l_5^2l_7^2t^3 - \frac{11}{2}\tau_{4,9}l_5^2l_7^2t^3 - 3\tau_{4,10}l_5^2l_7^2t^3 + \frac{17}{4}\tau_{4,14}l_5^2l_7^2t^3 - 6\tau_{2,5}l_6^2l_8^2t^3 - \\
& 2\tau_{3,5}l_6^2l_8^2t^3 + 4\tau_{3,9}l_6^2l_8^2t^3 + \tau_{4,5}l_6^2l_8^2t^3 + 5\tau_{4,9}l_6^2l_8^2t^3 - \tau_{1,5}l_7^2l_8^2t^3 + \frac{7}{2}\tau_{1,9}l_7^2l_8^2t^3 - \tau_{2,5}l_7^2l_8^2t^3 + 6\tau_{4,9}l_7^2l_8^2t^3 + \\
& \tau_{1,17}l_5^2l_{12}^2t^3 + \tau_{3,8}l_5^2l_{12}^2t^3 + \tau_{3,9}l_5^2l_{12}^2t^3 + \tau_{4,8}l_5^2l_{12}^2t^3 - 2\tau_{4,9}l_5^2l_{12}^2t^3 - \tau_{4,11}l_5^2l_{12}^2t^3 + \tau_{4,8}^3l_5^2t^2 - \tau_{4,10}^3l_5^2t^2 + \\
& 3\tau_{4,8}\tau_{4,10}^2l_5^2t^2 - \tau_{4,6}^2\tau_{4,8}l_5^2t^2 + \tau_{2,10}^2(\tau_{4,8} - \tau_{4,10})l_5^2t^2 + \tau_{4,6}^2\tau_{4,10}l_5^2t^2 - 3\tau_{4,8}^2\tau_{4,10}l_5^2t^2 - \tau_{3,7}^3l_6^2t^2 + \tau_{3,10}^3l_6^2t^2 + \\
& \tau_{2,7}\tau_{3,7}^2l_6^2t^2 - \tau_{2,7}\tau_{3,8}^2l_6^2t^2 - \tau_{3,7}\tau_{3,8}^2l_6^2t^2 - 2\tau_{3,8}\tau_{3,10}^2l_6^2t^2 + 2\tau_{3,7}^2\tau_{3,8}l_6^2t^2 + \tau_{3,8}^2\tau_{3,10}l_6^2t^2 - 2\tau_{2,7}\tau_{3,7}\tau_{3,10}l_6^2t^2 + \\
& 2\tau_{2,7}\tau_{3,8}\tau_{3,10}l_6^2t^2 + \tau_{3,7}^2\tau_{4,7}l_6^2t^2 - \tau_{3,8}^2\tau_{4,7}l_6^2t^2 - 2\tau_{3,10}^2\tau_{4,7}l_6^2t^2 - 2\tau_{3,7}\tau_{3,8}\tau_{4,7}l_6^2t^2 + 4\tau_{3,8}\tau_{3,10}\tau_{4,7}l_6^2t^2 + \\
& \tau_{3,8}^2\tau_{4,10}l_6^2t^2 + \tau_{3,10}^2\tau_{4,10}l_6^2t^2 - 2\tau_{3,8}\tau_{3,10}\tau_{4,10}l_6^2t^2 + \frac{1}{2}\tau_{1,5}^3l_7^2t^2 + \frac{1}{2}\tau_{1,6}^3l_7^2t^2 + 2\tau_{4,6}^3l_7^2t^2 + \frac{3}{2}\tau_{1,5}\tau_{1,6}^2l_7^2t^2 + \\
& 3\tau_{1,5}\tau_{4,6}^2l_7^2t^2 + 3\tau_{1,6}\tau_{4,6}^2l_7^2t^2 + \frac{3}{2}\tau_{1,5}^2\tau_{1,6}l_7^2t^2 + 2\tau_{1,5}^2\tau_{4,6}l_7^2t^2 + 2\tau_{1,6}^2\tau_{4,6}l_7^2t^2 + 4\tau_{1,5}\tau_{1,6}\tau_{4,6}l_7^2t^2 - \\
& 2\tau_{1,5}\tau_{3,7}^2l_8^2t^2 - \tau_{3,7}^2\tau_{4,5}l_8^2t^2 + 2\tau_{3,7}^2\tau_{4,7}l_8^2t^2 + 2\tau_{2,6}(\tau_{4,8} - \tau_{4,10})(s\tau_{4,6} + t(\tau_{2,10} - \tau_{4,8} + \tau_{4,10}))l_5^2t - \\
& 4(-s^2 + t^2 + u^2)\tau_{2,8}l_5^2l_6^2t + 6(-s^2 + t^2 + u^2)\tau_{2,11}l_5^2l_6^2t - 2(-s^2 + t^2 + u^2)\tau_{3,8}l_5^2l_6^2t + 6(-s^2 + t^2 + u^2)\tau_{3,11}l_5^2l_6^2t - \\
& 5(-s^2 + t^2 + u^2)\tau_{4,8}l_5^2l_6^2t - 3(-s^2 + t^2 + u^2)\tau_{4,9}l_5^2l_6^2t + 7(-s^2 + t^2 + u^2)\tau_{4,11}l_5^2l_6^2t + \frac{13}{4}(-s^2 + t^2 + u^2)\tau_{1,9}l_5^2l_7^2t - \\
& \frac{41}{8}(-s^2 + t^2 + u^2)\tau_{1,14}l_5^2l_7^2t + 5(-s^2 + t^2 + u^2)\tau_{1,16}l_5^2l_7^2t - \frac{17}{2}(-s^2 + t^2 + u^2)\tau_{2,14}l_5^2l_7^2t + \frac{13}{8}(-s^2 + t^2 + u^2)\tau_{2,16}l_5^2l_7^2t + \\
& \frac{25}{2}(-s^2 + t^2 + u^2)\tau_{4,9}l_5^2l_7^2t + \frac{17}{2}(-s^2 + t^2 + u^2)\tau_{4,10}l_5^2l_7^2t - \frac{81}{8}(-s^2 + t^2 + u^2)\tau_{4,14}l_5^2l_7^2t + 6(-s^2 + t^2 + u^2)\tau_{2,5}l_6^2l_8^2t - \\
& (-s^2 + t^2 + u^2)\tau_{2,11}l_6^2l_8^2t + 3(-s^2 + t^2 + u^2)\tau_{3,5}l_6^2l_8^2t + 8(-s^2 + t^2 + u^2)\tau_{3,9}l_6^2l_8^2t - (-s^2 + t^2 + u^2)\tau_{3,11}l_6^2l_8^2t - \\
& 2(-s^2 + t^2 + u^2)\tau_{4,9}l_6^2l_8^2t - 2(-s^2 + t^2 + u^2)\tau_{4,11}l_6^2l_8^2t - (-s^2 + t^2 + u^2)\tau_{4,5}l_7^2l_8^2t - \frac{5}{2}(-s^2 + t^2 + u^2)\tau_{4,9}l_7^2l_8^2t - \\
& \frac{1}{2}(-s^2 + t^2 + u^2)\tau_{4,9}l_6^2l_{11}^2t - (-s^2 + t^2 + u^2)\tau_{1,17}l_5^2l_{12}^2t - \frac{1}{2}(-s^2 + t^2 + u^2)\tau_{3,8}l_5^2l_{12}^2t - 2(-s^2 + t^2 + u^2)\tau_{3,9}l_5^2l_{12}^2t - \\
& \frac{1}{2}(-s^2 + t^2 + u^2)\tau_{4,8}l_5^2l_{12}^2t + (-s^2 + t^2 + u^2)\tau_{4,9}l_5^2l_{12}^2t + \frac{1}{2}(-s^2 + t^2 + u^2)\tau_{4,11}l_5^2l_{12}^2t - \frac{1}{2}(-s^2 + t^2 + u^2)\tau_{4,17}l_5^2l_{12}^2t + \\
& 2u(u-t)\tau_{1,8}^3l_5^2 - u^2\tau_{4,6}^2\tau_{4,8}l_5^2 + (-s^2 + t^2 + u^2)\tau_{4,6}^2\tau_{4,8}l_5^2 + u^2\tau_{4,6}^2\tau_{4,10}l_5^2 + (s^2 - t^2 - u^2)\tau_{4,6}^2\tau_{4,10}l_5^2 + \\
& \tau_{1,8}^2(-2\tau_{4,8}s^2 + \tau_{4,10}s^2 + 2(t-3u)\tau_{4,6}s + 3(s^2 - t^2 - u^2)\tau_{1,10} - 2t(t-3u)\tau_{2,6} + 2t(u-2t)\tau_{2,10} + \\
& 3t^2\tau_{4,8} + 3u^2\tau_{4,8} - 5t^2\tau_{4,10} - u^2\tau_{4,10})l_5^2 + \tau_{1,10}^2(2s(2t+u)\tau_{4,6} + (u^2 - 3s^2)\tau_{4,8} + u(2t+u)\tau_{4,10})l_5^2 +
\end{aligned}$$

$$\begin{aligned}
& 2 \tau_{1,8} (-u(2t+u) \tau_{1,10}^2 + (2 \tau_{2,10} t^2 + (t-2u) \tau_{2,6} t + ((t+4u) \tau_{4,8} + (2t-u) \tau_{4,10}) t + s(2u-3t) \tau_{4,6}) \tau_{1,10} + \\
& \quad 2 t^2 \tau_{2,6}^2 + t^2 \tau_{2,10}^2 + 2 s^2 \tau_{4,6}^2 + t(\tau_{4,8} - \tau_{4,10})((t-u) \tau_{4,8} - 2t \tau_{4,10}) - s \tau_{4,6}(u \tau_{4,8} + t \tau_{4,10}) + \\
& \quad t \tau_{2,6}(3t \tau_{2,10} - 4s \tau_{4,6} - (t-2u) \tau_{4,8} + 3t \tau_{4,10}) + t \tau_{2,10}(-2s \tau_{4,6} + (u-2t) \tau_{4,8} + 3t \tau_{4,10})) l_5^2 - \\
& u^2 \tau_{3,7}^3 l_6^2 + (-s^2 + t^2 + u^2) \tau_{3,7}^3 l_6^2 - u^2 \tau_{2,7} \tau_{3,7}^2 l_6^2 - u^2 \tau_{2,7} \tau_{3,8}^2 l_6^2 + (-s^2 + t^2 + u^2) \tau_{2,7} \tau_{3,8}^2 l_6^2 - u^2 \tau_{3,7} \tau_{3,8}^2 l_6^2 + \\
& 2(-s^2 + t^2 + u^2) \tau_{3,7} \tau_{3,8}^2 l_6^2 + (s^2 - t^2 - u^2) \tau_{3,7} \tau_{3,10}^2 l_6^2 + (-s^2 + t^2 + u^2) \tau_{3,8} \tau_{3,10}^2 l_6^2 + 2u^2 \tau_{3,7}^2 \tau_{3,8} l_6^2 + \\
& 3(s^2 - t^2 - u^2) \tau_{3,7}^2 \tau_{3,8} l_6^2 + 2u^2 \tau_{2,7} \tau_{3,7} \tau_{3,8} l_6^2 + (s^2 - t^2 - u^2) \tau_{2,7} \tau_{3,7} \tau_{3,8} l_6^2 + u^2 \tau_{3,7}^2 \tau_{3,10} l_6^2 + \\
& u^2 \tau_{3,8}^2 \tau_{3,10} l_6^2 + 2(s^2 - t^2 - u^2) \tau_{3,8}^2 \tau_{3,10} l_6^2 + (-s^2 + t^2 + u^2) \tau_{2,7} \tau_{3,7} \tau_{3,10} l_6^2 + (s^2 - t^2 - u^2) \tau_{2,7} \tau_{3,8} \tau_{3,10} l_6^2 - \\
& 2u^2 \tau_{3,7} \tau_{3,8} \tau_{3,10} l_6^2 + 2(-s^2 + t^2 + u^2) \tau_{3,7} \tau_{3,8} \tau_{3,10} l_6^2 + u^2 \tau_{3,7}^2 \tau_{4,7} l_6^2 + (s^2 - t^2 - u^2) \tau_{3,7}^2 \tau_{4,7} l_6^2 + \\
& u^2 \tau_{3,8}^2 \tau_{4,7} l_6^2 - 2u^2 \tau_{3,7} \tau_{3,8} \tau_{4,7} l_6^2 + (-s^2 + t^2 + u^2) \tau_{3,7} \tau_{3,8} \tau_{4,7} l_6^2 + (-s^2 + t^2 + u^2) \tau_{3,7} \tau_{3,10} \tau_{4,7} l_6^2 + \\
& (s^2 - t^2 - u^2) \tau_{3,8} \tau_{3,10} \tau_{4,7} l_6^2 - u^2 \tau_{3,7}^2 \tau_{4,10} l_6^2 - u^2 \tau_{3,8}^2 \tau_{4,10} l_6^2 + 2u^2 \tau_{3,7} \tau_{3,8} \tau_{4,10} l_6^2 - 2u(-s^2 + t^2 + u^2) \tau_{2,8} l_5^2 l_6^2 + \\
& 4u(-s^2 + t^2 + u^2) \tau_{2,11} l_5^2 l_6^2 - 2u(-s^2 + t^2 + u^2) \tau_{3,8} l_5^2 l_6^2 + u(-s^2 + t^2 + u^2) \tau_{3,9} l_5^2 l_6^2 + 4u(-s^2 + t^2 + u^2) \tau_{3,11} l_5^2 l_6^2 - \\
& \frac{19}{4} u(-s^2 + t^2 + u^2) \tau_{4,8} l_5^2 l_6^2 - \frac{3}{2} u(-s^2 + t^2 + u^2) \tau_{4,9} l_5^2 l_6^2 + \frac{21}{4} u(-s^2 + t^2 + u^2) \tau_{4,11} l_5^2 l_6^2 + \frac{1}{2} u^2 \tau_{1,5}^3 l_7^2 + \\
& \frac{1}{2} (s^2 - t^2 - u^2) \tau_{1,5}^3 l_7^2 + \frac{1}{2} u^2 \tau_{1,6}^3 l_7^2 + \frac{1}{2} (s^2 - t^2 - u^2) \tau_{1,6}^3 l_7^2 + 2u^2 \tau_{4,6}^3 l_7^2 + 2(s^2 - t^2 - u^2) \tau_{4,6}^3 l_7^2 + \\
& \frac{3}{2} u^2 \tau_{1,5} \tau_{1,6}^2 l_7^2 + \frac{3}{2} (s^2 - t^2 - u^2) \tau_{1,5} \tau_{1,6}^2 l_7^2 + 3u^2 \tau_{1,5} \tau_{4,6}^2 l_7^2 + 3(s^2 - t^2 - u^2) \tau_{1,5} \tau_{4,6}^2 l_7^2 + \\
& 3u^2 \tau_{1,6} \tau_{4,6}^2 l_7^2 + 3(s^2 - t^2 - u^2) \tau_{1,6} \tau_{4,6}^2 l_7^2 + \frac{3}{2} u^2 \tau_{1,5}^2 \tau_{1,6} l_7^2 + \frac{3}{2} (s^2 - t^2 - u^2) \tau_{1,5}^2 \tau_{1,6} l_7^2 + 2u^2 \tau_{1,5}^2 \tau_{4,6} l_7^2 + \\
& 2(s^2 - t^2 - u^2) \tau_{1,5}^2 \tau_{4,6} l_7^2 + 2u^2 \tau_{1,6}^2 \tau_{4,6} l_7^2 + 2(s^2 - t^2 - u^2) \tau_{1,6}^2 \tau_{4,6} l_7^2 + 4u^2 \tau_{1,5} \tau_{1,6} \tau_{4,6} l_7^2 + \\
& 4(s^2 - t^2 - u^2) \tau_{1,5} \tau_{1,6} \tau_{4,6} l_7^2 - 2u^3 \tau_{1,9} l_5^2 l_7^2 + \frac{27}{4} u(-s^2 + t^2 + u^2) \tau_{1,9} l_5^2 l_7^2 - 9u^3 \tau_{1,14} l_5^2 l_7^2 + \\
& \frac{5}{2} u(-s^2 + t^2 + u^2) \tau_{1,14} l_5^2 l_7^2 - 14u^3 \tau_{1,16} l_5^2 l_7^2 + 13u(-s^2 + t^2 + u^2) \tau_{1,16} l_5^2 l_7^2 - 5u(-s^2 + t^2 + u^2) \tau_{2,14} l_5^2 l_7^2 - \\
& 5u^3 \tau_{2,16} l_5^2 l_7^2 + \frac{11}{2} u(-s^2 + t^2 + u^2) \tau_{2,16} l_5^2 l_7^2 - 4u^3 \tau_{4,9} l_5^2 l_7^2 + \frac{51}{4} u(-s^2 + t^2 + u^2) \tau_{4,9} l_5^2 l_7^2 - \\
& 4u^3 \tau_{4,10} l_5^2 l_7^2 + 9u(-s^2 + t^2 + u^2) \tau_{4,10} l_5^2 l_7^2 + 5u^3 \tau_{4,14} l_5^2 l_7^2 - \frac{21}{2} u(-s^2 + t^2 + u^2) \tau_{4,14} l_5^2 l_7^2 + \\
& \tau_{2,10}(-2 \tau_{4,8}^2 l_5^2 t^2 - 2 \tau_{4,10}^2 l_5^2 t^2 + 4 \tau_{4,8} \tau_{4,10} l_5^2 t^2 + 2(2t^2 - 3s^2) l_5^2 l_7^2 t + (u \tau_{3,7} + s \tau_{3,8} + t \tau_{3,10})^2 l_6^2) + \\
& \frac{1}{4} \tau_{1,10} l_5^2 \left( -16s^2 \tau_{4,6}^2 + 8s((t+2u) \tau_{4,8} - u \tau_{4,10}) \tau_{4,6} + 4(s^2 - t^2 - u^2) \tau_{4,8}^2 + \right. \\
& \quad \left. 8t(t-u) \tau_{4,8} \tau_{4,10} - 8t \tau_{2,10}(-s \tau_{4,6} + u \tau_{4,8} + t \tau_{4,10}) + 8t \tau_{2,6}(3s \tau_{4,6} - (2t+3u) \tau_{4,8} + u \tau_{4,10}) + \right.
\end{aligned}$$

$$\begin{aligned}
& \frac{1}{2} \left( (-3t^3 - 36ut^2 - 13u^2t + 4u^3 + s^2(13t + 36u))l_7^2 - 16t^2\tau_{4,10}^2 \right) - 2u^2\tau_{1,5}^3l_8^2 - \frac{1}{2}u^2\tau_{4,5}^3l_8^2 + \\
& \frac{7}{2}u^2\tau_{4,7}^3l_8^2 - 2u^2\tau_{1,5}\tau_{4,5}^2l_8^2 + (-s^2 + t^2 + u^2)\tau_{3,7}\tau_{4,5}^2l_8^2 - 10u^2\tau_{1,5}\tau_{4,7}^2l_8^2 + 3(-s^2 + t^2 + u^2)\tau_{3,7}\tau_{4,7}^2l_8^2 - \\
& \frac{9}{2}u^2\tau_{4,5}\tau_{4,7}^2l_8^2 + 3(-s^2 + t^2 + u^2)\tau_{1,5}^2\tau_{3,7}l_8^2 - 3u^2\tau_{1,5}^2\tau_{4,5}l_8^2 + 3(-s^2 + t^2 + u^2)\tau_{1,5}\tau_{3,7}\tau_{4,5}l_8^2 + 9u^2\tau_{1,5}^2\tau_{4,7}l_8^2 + \\
& \frac{5}{2}u^2\tau_{4,5}^2\tau_{4,7}l_8^2 + 6(s^2 - t^2 - u^2)\tau_{1,5}\tau_{3,7}\tau_{4,7}l_8^2 + 8u^2\tau_{1,5}\tau_{4,5}\tau_{4,7}l_8^2 + 3(s^2 - t^2 - u^2)\tau_{3,7}\tau_{4,5}\tau_{4,7}l_8^2 + \\
& 5u(-s^2 + t^2 + u^2)\tau_{2,5}l_6^2l_8^2 - u(-s^2 + t^2 + u^2)\tau_{2,11}l_6^2l_8^2 + 5u(-s^2 + t^2 + u^2)\tau_{3,5}l_6^2l_8^2 + 10u(-s^2 + t^2 + u^2)\tau_{3,9}l_6^2l_8^2 - \\
& u(-s^2 + t^2 + u^2)\tau_{3,11}l_6^2l_8^2 + 5u(-s^2 + t^2 + u^2)\tau_{4,5}l_6^2l_8^2 + \frac{5}{2}u(-s^2 + t^2 + u^2)\tau_{4,9}l_6^2l_8^2 - 4u(-s^2 + t^2 + u^2)\tau_{4,11}l_6^2l_8^2 - \\
& \frac{1}{2}u(-s^2 + t^2 + u^2)\tau_{1,5}l_7^2l_8^2 - \frac{5}{4}u(-s^2 + t^2 + u^2)\tau_{1,9}l_7^2l_8^2 - \frac{1}{2}u(-s^2 + t^2 + u^2)\tau_{4,5}l_7^2l_8^2 - \frac{5}{4}u(-s^2 + t^2 + u^2)\tau_{4,9}l_7^2l_8^2 - \\
& \frac{1}{2}u(-s^2 + t^2 + u^2)\tau_{1,17}l_5^2l_{12}^2 - \frac{3}{2}u(-s^2 + t^2 + u^2)\tau_{3,9}l_5^2l_{12}^2 - \frac{1}{2}u(-s^2 + t^2 + u^2)\tau_{4,17}l_5^2l_{12}^2 - \\
& \left( (2\tau_{2,8} - \tau_{2,16} + \tau_{3,13})t^3 - \frac{1}{2}(-s^2 + t^2 + u^2)(2\tau_{2,11} + \tau_{2,13} - \tau_{2,16} + 2(\tau_{3,11} + \tau_{3,13} - \tau_{4,11} + 2\tau_{4,13} - 2\tau_{4,16}))t + \right. \\
& \quad u(-s^2 + t^2 + u^2)(\tau_{2,13} - \tau_{2,16} - \tau_{3,11} + 2(\tau_{3,13} + \tau_{4,11} - 2\tau_{4,13} + 2\tau_{4,16})) - \\
& \quad \left. u^3(\tau_{2,13} - \tau_{2,16} + 2(\tau_{3,13} + 2(\tau_{4,11} - \tau_{4,13} + \tau_{4,16}))) \right) l_6^2l_{15}^2
\end{aligned}$$

■  $N_{32}^{(6)}$

$$\begin{aligned}
& \frac{1}{4} (8\tau_{8,16}l_6^2l_{15}^2t^3 - 3l_5^2l_6^2l_{15}^2t^3 - 4l_6^2l_{13}^2l_{15}^2t^3 + 8\tau_{3,11}^2l_5^2l_6^2t^2 - 2\tau_{4,9}^2l_5^2l_6^2t^2 + 4\tau_{4,11}^2l_5^2l_6^2t^2 - 12\tau_{3,11}\tau_{4,8}l_5^2l_6^2t^2 - \\
& 6\tau_{3,11}\tau_{4,9}l_5^2l_6^2t^2 + 2\tau_{4,8}\tau_{4,9}l_5^2l_6^2t^2 + 4\tau_{3,11}\tau_{4,11}l_5^2l_6^2t^2 - 16\tau_{4,8}\tau_{4,11}l_5^2l_6^2t^2 - 4\tau_{4,9}\tau_{4,11}l_5^2l_6^2t^2 + \tau_{1,10}^2l_5^2l_7^2t^2 - \\
& 5\tau_{1,14}^2l_5^2l_7^2t^2 + 12\tau_{1,16}^2l_5^2l_7^2t^2 - 16\tau_{2,14}^2l_5^2l_7^2t^2 + 4\tau_{2,16}^2l_5^2l_7^2t^2 - 8\tau_{4,9}^2l_5^2l_7^2t^2 - 4\tau_{4,10}^2l_5^2l_7^2t^2 - 12\tau_{4,14}^2l_5^2l_7^2t^2 - \\
& 7\tau_{1,9}\tau_{1,10}l_5^2l_7^2t^2 + 11\tau_{1,9}\tau_{1,14}l_5^2l_7^2t^2 - 4\tau_{1,10}\tau_{1,14}l_5^2l_7^2t^2 + 8\tau_{1,9}\tau_{1,16}l_5^2l_7^2t^2 - 13\tau_{1,10}\tau_{1,16}l_5^2l_7^2t^2 + \\
& 19\tau_{1,14}\tau_{1,16}l_5^2l_7^2t^2 - 16\tau_{1,9}\tau_{2,10}l_5^2l_7^2t^2 - 12\tau_{1,16}\tau_{2,10}l_5^2l_7^2t^2 + 13\tau_{1,9}\tau_{2,14}l_5^2l_7^2t^2 + 6\tau_{1,10}\tau_{2,14}l_5^2l_7^2t^2 - \\
& 22\tau_{1,14}\tau_{2,14}l_5^2l_7^2t^2 + 10\tau_{1,16}\tau_{2,14}l_5^2l_7^2t^2 + 8\tau_{2,10}\tau_{2,14}l_5^2l_7^2t^2 + 10\tau_{1,9}\tau_{2,16}l_5^2l_7^2t^2 - 3\tau_{1,10}\tau_{2,16}l_5^2l_7^2t^2 + \\
& 7\tau_{1,14}\tau_{2,16}l_5^2l_7^2t^2 + 15\tau_{1,16}\tau_{2,16}l_5^2l_7^2t^2 - 4\tau_{2,10}\tau_{2,16}l_5^2l_7^2t^2 - 9\tau_{1,9}\tau_{4,9}l_5^2l_7^2t^2 - 9\tau_{1,10}\tau_{4,9}l_5^2l_7^2t^2 + 17\tau_{1,14}\tau_{4,9}l_5^2l_7^2t^2 + \\
& 8\tau_{1,16}\tau_{4,9}l_5^2l_7^2t^2 - 16\tau_{2,10}\tau_{4,9}l_5^2l_7^2t^2 + 17\tau_{2,14}\tau_{4,9}l_5^2l_7^2t^2 + 8\tau_{2,16}\tau_{4,9}l_5^2l_7^2t^2 - 8\tau_{1,9}\tau_{4,10}l_5^2l_7^2t^2 - 4\tau_{1,10}\tau_{4,10}l_5^2l_7^2t^2 + \\
& 12\tau_{1,14}\tau_{4,10}l_5^2l_7^2t^2 + 4\tau_{1,16}\tau_{4,10}l_5^2l_7^2t^2 - 8\tau_{2,10}\tau_{4,10}l_5^2l_7^2t^2 + 12\tau_{2,14}\tau_{4,10}l_5^2l_7^2t^2 + 4\tau_{2,16}\tau_{4,10}l_5^2l_7^2t^2 - \\
& 12\tau_{4,9}\tau_{4,10}l_5^2l_7^2t^2 + 3\tau_{1,9}\tau_{4,14}l_5^2l_7^2t^2 + 9\tau_{1,10}\tau_{4,14}l_5^2l_7^2t^2 - 29\tau_{1,14}\tau_{4,14}l_5^2l_7^2t^2 - 5\tau_{1,16}\tau_{4,14}l_5^2l_7^2t^2 +
\end{aligned}$$

$$\begin{aligned}
& 12 \tau_{2,10} \tau_{4,14} l_5^2 l_7^2 t^2 - 32 \tau_{2,14} \tau_{4,14} l_5^2 l_7^2 t^2 - 8 \tau_{2,16} \tau_{4,14} l_5^2 l_7^2 t^2 + 9 \tau_{4,9} \tau_{4,14} l_5^2 l_7^2 t^2 + 8 \tau_{4,10} \tau_{4,14} l_5^2 l_7^2 t^2 - \\
& 16 \tau_{3,5}^2 l_6^2 l_8^2 t^2 + 12 \tau_{4,5}^2 l_6^2 l_8^2 t^2 + 4 \tau_{4,9}^2 l_6^2 l_8^2 t^2 + 4 \tau_{4,11}^2 l_6^2 l_8^2 t^2 - 4 \tau_{2,5} \tau_{3,11} l_6^2 l_8^2 t^2 + 12 \tau_{2,5} \tau_{4,5} l_6^2 l_8^2 t^2 - \\
& 4 \tau_{3,5} \tau_{4,5} l_6^2 l_8^2 t^2 - 8 \tau_{3,11} \tau_{4,5} l_6^2 l_8^2 t^2 + 12 \tau_{2,5} \tau_{4,9} l_6^2 l_8^2 t^2 - 4 \tau_{3,5} \tau_{4,9} l_6^2 l_8^2 t^2 + 8 \tau_{3,11} \tau_{4,9} l_6^2 l_8^2 t^2 + 20 \tau_{4,5} \tau_{4,9} l_6^2 l_8^2 t^2 - \\
& 12 \tau_{2,5} \tau_{4,11} l_6^2 l_8^2 t^2 - 8 \tau_{3,5} \tau_{4,11} l_6^2 l_8^2 t^2 + 4 \tau_{3,11} \tau_{4,11} l_6^2 l_8^2 t^2 - 12 \tau_{4,5} \tau_{4,11} l_6^2 l_8^2 t^2 - 4 \tau_{4,9} \tau_{4,11} l_6^2 l_8^2 t^2 + 8 \tau_{1,5}^2 l_7^2 l_8^2 t^2 - \\
& 10 \tau_{1,9}^2 l_7^2 l_8^2 t^2 + 8 \tau_{2,5}^2 l_7^2 l_8^2 t^2 + 8 \tau_{4,5}^2 l_7^2 l_8^2 t^2 - 10 \tau_{4,9}^2 l_7^2 l_8^2 t^2 - 2 \tau_{1,5} \tau_{1,9} l_7^2 l_8^2 t^2 + 16 \tau_{1,5} \tau_{2,5} l_7^2 l_8^2 t^2 - \\
& 2 \tau_{1,9} \tau_{2,5} l_7^2 l_8^2 t^2 + 16 \tau_{1,5} \tau_{4,5} l_7^2 l_8^2 t^2 - 2 \tau_{1,9} \tau_{4,5} l_7^2 l_8^2 t^2 + 16 \tau_{2,5} \tau_{4,5} l_7^2 l_8^2 t^2 - 2 \tau_{1,5} \tau_{4,9} l_7^2 l_8^2 t^2 - 20 \tau_{1,9} \tau_{4,9} l_7^2 l_8^2 t^2 - \\
& 2 \tau_{2,5} \tau_{4,9} l_7^2 l_8^2 t^2 - 2 \tau_{4,5} \tau_{4,9} l_7^2 l_8^2 t^2 + 4 \tau_{2,13}^2 l_6^2 l_{15}^2 t^2 + 4 \tau_{2,16}^2 l_6^2 l_{15}^2 t^2 - 8 \tau_{2,13} \tau_{2,16} l_6^2 l_{15}^2 t^2 + 4 \tau_{2,16} \tau_{3,11} l_6^2 l_{15}^2 t^2 + \\
& 8 \tau_{2,13} \tau_{3,13} l_6^2 l_{15}^2 t^2 - 8 \tau_{2,16} \tau_{3,13} l_6^2 l_{15}^2 t^2 + 4 \tau_{3,11} \tau_{3,13} l_6^2 l_{15}^2 t^2 - 4 \tau_{2,16} \tau_{4,11} l_6^2 l_{15}^2 t^2 + 4 \tau_{3,11} \tau_{4,13} l_6^2 l_{15}^2 t^2 - \\
& 8 \tau_{4,11} \tau_{4,13} l_6^2 l_{15}^2 t^2 + 4 \tau_{3,11} \tau_{4,16} l_6^2 l_{15}^2 t^2 + 16 u^2 l_5^2 l_6^2 l_{15}^2 t^2 + 13 s^2 l_5^2 l_6^2 l_{15}^2 t - 13 u^2 l_5^2 l_6^2 l_{15}^2 t - 8 s^2 \tau_{2,11}^2 l_5^2 l_6^2 - \\
& 8 s^2 \tau_{3,11}^2 l_5^2 l_6^2 + 4 s^2 \tau_{4,8}^2 l_5^2 l_6^2 - 4 u^2 \tau_{4,8}^2 l_5^2 l_6^2 + 2 s^2 \tau_{4,9}^2 l_5^2 l_6^2 + 2 u^2 \tau_{4,9}^2 l_5^2 l_6^2 - 12 s^2 \tau_{4,11}^2 l_5^2 l_6^2 - 2 u^2 \tau_{4,11}^2 l_5^2 l_6^2 + \\
& 20 s^2 \tau_{3,11} \tau_{4,8} l_5^2 l_6^2 + 22 u^2 \tau_{3,11} \tau_{4,8} l_5^2 l_6^2 + 14 s^2 \tau_{3,11} \tau_{4,9} l_5^2 l_6^2 + 6 u^2 \tau_{3,11} \tau_{4,9} l_5^2 l_6^2 + 2 s^2 \tau_{4,8} \tau_{4,9} l_5^2 l_6^2 - \\
& 20 s^2 \tau_{3,11} \tau_{4,11} l_5^2 l_6^2 - 2 u^2 \tau_{3,11} \tau_{4,11} l_5^2 l_6^2 + 32 s^2 \tau_{4,8} \tau_{4,11} l_5^2 l_6^2 + 22 u^2 \tau_{4,8} \tau_{4,11} l_5^2 l_6^2 + 20 s^2 \tau_{4,9} \tau_{4,11} l_5^2 l_6^2 + \\
& 6 u^2 \tau_{4,9} \tau_{4,11} l_5^2 l_6^2 - 2 s^2 \tau_{1,9}^2 l_5^2 l_7^2 + 13 u^2 \tau_{1,9}^2 l_5^2 l_7^2 + 4 s^2 \tau_{1,14}^2 l_5^2 l_7^2 - 12 u^2 \tau_{1,14}^2 l_5^2 l_7^2 - 16 s^2 \tau_{1,16}^2 l_5^2 l_7^2 - \\
& 12 u^2 \tau_{1,16}^2 l_5^2 l_7^2 + 4 s^2 \tau_{2,16}^2 l_5^2 l_7^2 - 4 u^2 \tau_{2,16}^2 l_5^2 l_7^2 + 15 s^2 \tau_{4,9}^2 l_5^2 l_7^2 + 12 u^2 \tau_{4,9}^2 l_5^2 l_7^2 + 4 s^2 \tau_{4,10}^2 l_5^2 l_7^2 + 4 u^2 \tau_{4,10}^2 l_5^2 l_7^2 - \\
& 4 s^2 \tau_{4,14}^2 l_5^2 l_7^2 + 4 u^2 \tau_{4,14}^2 l_5^2 l_7^2 - s^2 \tau_{1,9} \tau_{1,10} l_5^2 l_7^2 + u^2 \tau_{1,9} \tau_{1,10} l_5^2 l_7^2 - 7 s^2 \tau_{1,9} \tau_{1,14} l_5^2 l_7^2 - 9 u^2 \tau_{1,9} \tau_{1,14} l_5^2 l_7^2 + \\
& 4 s^2 \tau_{1,10} \tau_{1,14} l_5^2 l_7^2 + 12 u^2 \tau_{1,10} \tau_{1,14} l_5^2 l_7^2 - 8 s^2 \tau_{1,9} \tau_{1,16} l_5^2 l_7^2 + 8 s^2 \tau_{1,10} \tau_{1,16} l_5^2 l_7^2 + 12 u^2 \tau_{1,10} \tau_{1,16} l_5^2 l_7^2 - \\
& 8 s^2 \tau_{1,14} \tau_{1,16} l_5^2 l_7^2 - 28 u^2 \tau_{1,14} \tau_{1,16} l_5^2 l_7^2 - 8 s^2 \tau_{1,14} \tau_{2,10} l_5^2 l_7^2 + 8 u^2 \tau_{1,14} \tau_{2,10} l_5^2 l_7^2 - 12 s^2 \tau_{1,16} \tau_{2,10} l_5^2 l_7^2 + \\
& 12 u^2 \tau_{1,16} \tau_{2,10} l_5^2 l_7^2 + s^2 \tau_{1,9} \tau_{2,14} l_5^2 l_7^2 - u^2 \tau_{1,9} \tau_{2,14} l_5^2 l_7^2 - 4 s^2 \tau_{1,10} \tau_{2,14} l_5^2 l_7^2 + 4 u^2 \tau_{1,10} \tau_{2,14} l_5^2 l_7^2 + 12 s^2 \tau_{1,14} \tau_{2,14} l_5^2 l_7^2 - \\
& 12 u^2 \tau_{1,14} \tau_{2,14} l_5^2 l_7^2 + 20 s^2 \tau_{1,16} \tau_{2,14} l_5^2 l_7^2 - 20 u^2 \tau_{1,16} \tau_{2,14} l_5^2 l_7^2 + 8 u^2 \tau_{1,9} \tau_{2,16} l_5^2 l_7^2 + 4 u^2 \tau_{1,10} \tau_{2,16} l_5^2 l_7^2 - \\
& 4 s^2 \tau_{1,14} \tau_{2,16} l_5^2 l_7^2 - 16 u^2 \tau_{1,14} \tau_{2,16} l_5^2 l_7^2 - 4 s^2 \tau_{1,16} \tau_{2,16} l_5^2 l_7^2 - 16 u^2 \tau_{1,16} \tau_{2,16} l_5^2 l_7^2 - 4 s^2 \tau_{2,10} \tau_{2,16} l_5^2 l_7^2 + \\
& 4 u^2 \tau_{2,10} \tau_{2,16} l_5^2 l_7^2 + 8 s^2 \tau_{2,14} \tau_{2,16} l_5^2 l_7^2 - 8 u^2 \tau_{2,14} \tau_{2,16} l_5^2 l_7^2 + 5 s^2 \tau_{1,9} \tau_{4,9} l_5^2 l_7^2 + 25 u^2 \tau_{1,9} \tau_{4,9} l_5^2 l_7^2 - s^2 \tau_{1,10} \tau_{4,9} l_5^2 l_7^2 + \\
& u^2 \tau_{1,10} \tau_{4,9} l_5^2 l_7^2 - 23 s^2 \tau_{1,14} \tau_{4,9} l_5^2 l_7^2 - 9 u^2 \tau_{1,14} \tau_{4,9} l_5^2 l_7^2 - 16 s^2 \tau_{1,16} \tau_{4,9} l_5^2 l_7^2 + s^2 \tau_{2,14} \tau_{4,9} l_5^2 l_7^2 - u^2 \tau_{2,14} \tau_{4,9} l_5^2 l_7^2 + \\
& 8 s^2 \tau_{2,16} \tau_{4,9} l_5^2 l_7^2 + 8 u^2 \tau_{2,16} \tau_{4,9} l_5^2 l_7^2 + 12 u^2 \tau_{1,9} \tau_{4,10} l_5^2 l_7^2 - 16 s^2 \tau_{1,14} \tau_{4,10} l_5^2 l_7^2 - 8 u^2 \tau_{1,14} \tau_{4,10} l_5^2 l_7^2 - \\
& 16 s^2 \tau_{1,16} \tau_{4,10} l_5^2 l_7^2 + 4 s^2 \tau_{2,14} \tau_{4,10} l_5^2 l_7^2 - 4 u^2 \tau_{2,14} \tau_{4,10} l_5^2 l_7^2 + 4 s^2 \tau_{2,16} \tau_{4,10} l_5^2 l_7^2 + 4 u^2 \tau_{2,16} \tau_{4,10} l_5^2 l_7^2 + \\
& 12 s^2 \tau_{4,9} \tau_{4,10} l_5^2 l_7^2 + 12 u^2 \tau_{4,9} \tau_{4,10} l_5^2 l_7^2 + s^2 \tau_{1,9} \tau_{4,14} l_5^2 l_7^2 - 9 u^2 \tau_{1,9} \tau_{4,14} l_5^2 l_7^2 - 4 s^2 \tau_{1,10} \tau_{4,14} l_5^2 l_7^2 + 16 s^2 \tau_{1,14} \tau_{4,14} l_5^2 l_7^2 + \\
& 4 u^2 \tau_{1,14} \tau_{4,14} l_5^2 l_7^2 + 24 s^2 \tau_{1,16} \tau_{4,14} l_5^2 l_7^2 - 4 u^2 \tau_{1,16} \tau_{4,14} l_5^2 l_7^2 + 4 s^2 \tau_{2,10} \tau_{4,14} l_5^2 l_7^2 - 4 u^2 \tau_{2,10} \tau_{4,14} l_5^2 l_7^2 - \\
& 8 s^2 \tau_{2,14} \tau_{4,14} l_5^2 l_7^2 + 8 u^2 \tau_{2,14} \tau_{4,14} l_5^2 l_7^2 - 7 s^2 \tau_{4,9} \tau_{4,14} l_5^2 l_7^2 - 9 u^2 \tau_{4,9} \tau_{4,14} l_5^2 l_7^2 - 8 u^2 \tau_{4,10} \tau_{4,14} l_5^2 l_7^2 - 16 s^2 \tau_{2,5}^2 l_6^2 l_8^2 - \\
& 8 u^2 \tau_{2,5}^2 l_6^2 l_8^2 + 8 s^2 \tau_{3,5}^2 l_6^2 l_8^2 - 32 u^2 \tau_{3,5}^2 l_6^2 l_8^2 - 20 s^2 \tau_{4,5}^2 l_6^2 l_8^2 - 68 u^2 \tau_{4,5}^2 l_6^2 l_8^2 - 20 u^2 \tau_{4,9}^2 l_6^2 l_8^2 - 4 s^2 \tau_{4,11}^2 l_6^2 l_8^2 + \\
& 4 u^2 \tau_{4,11}^2 l_6^2 l_8^2 - 8 s^2 \tau_{2,5} \tau_{3,5} l_6^2 l_8^2 - 40 u^2 \tau_{2,5} \tau_{3,5} l_6^2 l_8^2 + 4 s^2 \tau_{2,5} \tau_{3,11} l_6^2 l_8^2 + 4 u^2 \tau_{2,5} \tau_{3,11} l_6^2 l_8^2 + 8 u^2 \tau_{3,5} \tau_{3,11} l_6^2 l_8^2 - \\
& 44 s^2 \tau_{2,5} \tau_{4,5} l_6^2 l_8^2 - 52 u^2 \tau_{2,5} \tau_{4,5} l_6^2 l_8^2 + 4 s^2 \tau_{3,5} \tau_{4,5} l_6^2 l_8^2 - 100 u^2 \tau_{3,5} \tau_{4,5} l_6^2 l_8^2 + 4 s^2 \tau_{3,11} \tau_{4,5} l_6^2 l_8^2 + 4 u^2 \tau_{3,11} \tau_{4,5} l_6^2 l_8^2 - \\
& 12 s^2 \tau_{2,5} \tau_{4,9} l_6^2 l_8^2 - 40 u^2 \tau_{2,5} \tau_{4,9} l_6^2 l_8^2 + 12 s^2 \tau_{3,5} \tau_{4,9} l_6^2 l_8^2 - 64 u^2 \tau_{3,5} \tau_{4,9} l_6^2 l_8^2 - 4 s^2 \tau_{3,11} \tau_{4,9} l_6^2 l_8^2 + 12 u^2 \tau_{3,11} \tau_{4,9} l_6^2 l_8^2 - \\
& 8 s^2 \tau_{4,5} \tau_{4,9} l_6^2 l_8^2 - 92 u^2 \tau_{4,5} \tau_{4,9} l_6^2 l_8^2 + 20 s^2 \tau_{2,5} \tau_{4,11} l_6^2 l_8^2 + 12 u^2 \tau_{2,5} \tau_{4,11} l_6^2 l_8^2 + 8 s^2 \tau_{3,5} \tau_{4,11} l_6^2 l_8^2 + \\
& 24 u^2 \tau_{3,5} \tau_{4,11} l_6^2 l_8^2 - 4 s^2 \tau_{3,11} \tau_{4,11} l_6^2 l_8^2 + 4 u^2 \tau_{3,11} \tau_{4,11} l_6^2 l_8^2 + 16 s^2 \tau_{4,5} \tau_{4,11} l_6^2 l_8^2 + 16 u^2 \tau_{4,5} \tau_{4,11} l_6^2 l_8^2 +
\end{aligned}$$

$$\begin{aligned}
& 32 u^2 \tau_{4,9} \tau_{4,11} l_6^2 l_8^2 - 4 s^2 \tau_{1,5}^2 l_7^2 l_8^2 + 12 u^2 \tau_{1,5}^2 l_7^2 l_8^2 + 10 s^2 \tau_{1,9}^2 l_7^2 l_8^2 - 2 u^2 \tau_{1,9}^2 l_7^2 l_8^2 + 12 s^2 \tau_{4,5}^2 l_7^2 l_8^2 - 4 u^2 \tau_{4,5}^2 l_7^2 l_8^2 - \\
& 2 s^2 \tau_{4,9}^2 l_7^2 l_8^2 + 10 u^2 \tau_{4,9}^2 l_7^2 l_8^2 + 6 s^2 \tau_{1,5} \tau_{1,9} l_7^2 l_8^2 + 2 u^2 \tau_{1,5} \tau_{1,9} l_7^2 l_8^2 - 12 s^2 \tau_{1,5} \tau_{2,5} l_7^2 l_8^2 + 12 u^2 \tau_{1,5} \tau_{2,5} l_7^2 l_8^2 - \\
& 6 s^2 \tau_{1,9} \tau_{2,5} l_7^2 l_8^2 + 6 u^2 \tau_{1,9} \tau_{2,5} l_7^2 l_8^2 - 12 s^2 \tau_{1,5} \tau_{4,5} l_7^2 l_8^2 - 12 u^2 \tau_{1,5} \tau_{4,5} l_7^2 l_8^2 - 18 s^2 \tau_{1,9} \tau_{4,5} l_7^2 l_8^2 + 6 u^2 \tau_{1,9} \tau_{4,5} l_7^2 l_8^2 + \\
& 12 s^2 \tau_{2,5} \tau_{4,5} l_7^2 l_8^2 - 12 u^2 \tau_{2,5} \tau_{4,5} l_7^2 l_8^2 + 6 s^2 \tau_{1,5} \tau_{4,9} l_7^2 l_8^2 - 18 u^2 \tau_{1,5} \tau_{4,9} l_7^2 l_8^2 + 6 s^2 \tau_{1,9} \tau_{4,9} l_7^2 l_8^2 + 6 u^2 \tau_{1,9} \tau_{4,9} l_7^2 l_8^2 + \\
& 6 s^2 \tau_{2,5} \tau_{4,9} l_7^2 l_8^2 - 6 u^2 \tau_{2,5} \tau_{4,9} l_7^2 l_8^2 + 2 s^2 \tau_{4,5} \tau_{4,9} l_7^2 l_8^2 + 6 u^2 \tau_{4,5} \tau_{4,9} l_7^2 l_8^2 + 4 \tau_{3,9}^2 l_6^2 ((2 s^2 - u^2) l_5^2 - 2 s(t - 5 u) l_8^2) + \\
& 2 \tau_{3,9} l_6^2 ((5 u^2 - 6 s^2) \tau_{4,8} l_5^2 - 2((6 s^2 + 4 u^2) \tau_{2,5} + (3 s^2 - t^2 + 7 u^2) \tau_{3,5} - (t^2 - 10 u^2) \tau_{4,5}) l_8^2 - \\
& 4 u \tau_{3,11} ((t + 2 u) l_5^2 + s l_8^2) + u \tau_{4,11} (8(t + 2 u) l_8^2 - (8 t + 11 u) l_5^2) - 2 \tau_{4,9} ((s^2 + t^2) l_5^2 + (-2 s^2 - 3 t^2 + 7 u^2) l_8^2)) - \\
& 4 s^2 \tau_{2,13}^2 l_6^2 l_{15}^2 - 4 s^2 \tau_{2,16}^2 l_6^2 l_{15}^2 - 12 s^2 \tau_{3,13}^2 l_6^2 l_{15}^2 + 4 u^2 \tau_{3,13}^2 l_6^2 l_{15}^2 - 8 u^2 \tau_{4,11}^2 l_6^2 l_{15}^2 - 8 s^2 \tau_{4,13}^2 l_6^2 l_{15}^2 - \\
& 8 s^2 \tau_{4,16}^2 l_6^2 l_{15}^2 + 8 s^2 \tau_{2,13} \tau_{2,16} l_6^2 l_{15}^2 + 4 u^2 \tau_{2,13} \tau_{3,11} l_6^2 l_{15}^2 - 4 u^2 \tau_{2,16} \tau_{3,11} l_6^2 l_{15}^2 - 12 s^2 \tau_{2,13} \tau_{3,13} l_6^2 l_{15}^2 + \\
& 12 s^2 \tau_{2,16} \tau_{3,13} l_6^2 l_{15}^2 + 4 s^2 \tau_{3,11} \tau_{3,13} l_6^2 l_{15}^2 + 4 u^2 \tau_{3,11} \tau_{3,13} l_6^2 l_{15}^2 - 4 u^2 \tau_{2,13} \tau_{4,11} l_6^2 l_{15}^2 + \\
& 4 u^2 \tau_{2,16} \tau_{4,11} l_6^2 l_{15}^2 - 8 u^2 \tau_{3,13} \tau_{4,11} l_6^2 l_{15}^2 + 4 s^2 \tau_{2,13} \tau_{4,13} l_6^2 l_{15}^2 - 4 s^2 \tau_{2,16} \tau_{4,13} l_6^2 l_{15}^2 - \\
& 4 s^2 \tau_{3,11} \tau_{4,13} l_6^2 l_{15}^2 + 4 u^2 \tau_{3,11} \tau_{4,13} l_6^2 l_{15}^2 + 8 s^2 \tau_{3,13} \tau_{4,13} l_6^2 l_{15}^2 + 8 s^2 \tau_{4,11} \tau_{4,13} l_6^2 l_{15}^2 + 8 u^2 \tau_{4,11} \tau_{4,13} l_6^2 l_{15}^2 - \\
& 4 s^2 \tau_{2,13} \tau_{4,16} l_6^2 l_{15}^2 + 4 s^2 \tau_{2,16} \tau_{4,16} l_6^2 l_{15}^2 + 4 s^2 \tau_{3,11} \tau_{4,16} l_6^2 l_{15}^2 - 4 u^2 \tau_{3,11} \tau_{4,16} l_6^2 l_{15}^2 - 8 s^2 \tau_{3,13} \tau_{4,16} l_6^2 l_{15}^2 - \\
& 8 s^2 \tau_{4,11} \tau_{4,16} l_6^2 l_{15}^2 - 8 u^2 \tau_{4,11} \tau_{4,16} l_6^2 l_{15}^2 + 16 s^2 \tau_{4,13} \tau_{4,16} l_6^2 l_{15}^2 + 16 u^3 l_5^2 l_6^2 l_{15}^2 - 16 s^2 u l_5^2 l_6^2 l_{15}^2 + \\
& 4 \tau_{2,8} l_6^2 ((4 \tau_{2,11} s^2 - 2(t + 2 u) \tau_{3,11} s - 2 t^2 \tau_{3,9} + t^2 \tau_{4,8} + (5 s^2 - t^2) \tau_{4,11}) l_5^2 - t^2 (\tau_{2,13} + 2 \tau_{3,13}) l_{15}^2) + \\
& 4 \tau_{3,8} l_6^2 ((\tau_{2,13} - 2 \tau_{2,16} + 2 \tau_{3,13}) l_{15}^2 t^2 + (2 \tau_{3,9} t^2 - \tau_{4,8} t^2 + 2 u(t + 2 u) \tau_{3,11} + u(4 t + 5 u) \tau_{4,11}) l_5^2) + \\
& 2 \tau_{2,11} l_6^2 (-8 \tau_{3,11} l_5^2 s^2 + 14 \tau_{4,8} l_5^2 s^2 + 8 \tau_{4,9} l_5^2 s^2 - 10 \tau_{4,11} l_5^2 s^2 + 4 \tau_{2,5} l_8^2 s^2 + 2 \tau_{3,5} l_8^2 s^2 + 4 \tau_{4,5} l_8^2 s^2 - \\
& 2 \tau_{4,11} l_8^2 s^2 - 8 u \tau_{3,8} l_5^2 s + 4 u \tau_{3,9} (2 l_5^2 - l_8^2) s - 6 t^2 \tau_{4,8} l_5^2 + 7 u^2 \tau_{4,8} l_5^2 + 2 u^2 \tau_{4,9} l_5^2 + 2 t^2 \tau_{4,11} l_5^2 - \\
& u^2 \tau_{4,11} l_5^2 - 2 t^2 \tau_{3,5} l_8^2 + 2 u^2 \tau_{3,5} l_8^2 - 2 t^2 \tau_{4,5} l_8^2 - 2 t^2 \tau_{4,9} l_8^2 + 4 u^2 \tau_{4,9} l_8^2 + 2 t^2 \tau_{4,11} l_8^2 + 2 u^2 \tau_{4,11} l_8^2 + \\
& 2((\tau_{2,16} + 2 \tau_{4,16}) t^2 + u^2 (\tau_{2,13} - \tau_{2,16} + 2 \tau_{3,13})) l_{15}^2) + ((-3 t^3 + 16 u t^2 + 39 u^2 t + 16 u^3 - s^2 (39 t + 16 u)) l_5^2 l_7^2 + \\
& 2 l_6^2 (2(t^3 - u t^2 + 2 u^2 t - u^3 + s^2 (u - 2 t)) l_8^2 + (t^3 - 2 u t^2 + u^2 t + 2 u^3 - s^2 (t - 2 u)) l_9^2)) l_{17}^2)
\end{aligned}$$

■  $N_{32}^{(7)}$

$$\begin{aligned}
& \frac{1}{4} (4 \tau_{2,11} l_5^2 l_6^2 l_{15}^2 s^2 - 17 \tau_{3,8} l_5^2 l_6^2 l_{15}^2 s^2 + 6 \tau_{3,9} l_5^2 l_6^2 l_{15}^2 s^2 + 13 \tau_{3,11} l_5^2 l_6^2 l_{15}^2 s^2 - 18 \tau_{4,8} l_5^2 l_6^2 l_{15}^2 s^2 - \\
& 8 \tau_{4,9} l_5^2 l_6^2 l_{15}^2 s^2 + 4 \tau_{4,11} l_5^2 l_6^2 l_{15}^2 s^2 + (-5 s^2 + 19 t^2 + 21 u^2) \tau_{2,8} l_5^2 l_6^2 l_{15}^2 + 2(4 t - 3 u)(t + 2 u) \tau_{2,9} l_5^2 l_6^2 l_{15}^2 + \\
& 14 t^2 \tau_{2,11} l_5^2 l_6^2 l_{15}^2 - 20 u^2 \tau_{2,11} l_5^2 l_6^2 l_{15}^2 - 6 t^2 \tau_{2,16} l_5^2 l_6^2 l_{15}^2 + 47 t^2 \tau_{3,8} l_5^2 l_6^2 l_{15}^2 + 33 u^2 \tau_{3,8} l_5^2 l_6^2 l_{15}^2 + \\
& 14 t^2 \tau_{3,9} l_5^2 l_6^2 l_{15}^2 - 30 u^2 \tau_{3,9} l_5^2 l_6^2 l_{15}^2 - t^2 \tau_{3,11} l_5^2 l_6^2 l_{15}^2 - 29 u^2 \tau_{3,11} l_5^2 l_6^2 l_{15}^2 + 34 t^2 \tau_{4,8} l_5^2 l_6^2 l_{15}^2 + \\
& 56 u^2 \tau_{4,8} l_5^2 l_6^2 l_{15}^2 + 12 t^2 \tau_{4,9} l_5^2 l_6^2 l_{15}^2 + 20 u^2 \tau_{4,9} l_5^2 l_6^2 l_{15}^2 + 20 t^2 \tau_{4,11} l_5^2 l_6^2 l_{15}^2 - 26 u^2 \tau_{4,11} l_5^2 l_6^2 l_{15}^2 + \\
& (4 \tau_{2,6} l_5^2 l_7^2 s^2 + 4 \tau_{2,11} l_5^2 l_7^2 s^2 - 23 \tau_{3,9} l_5^2 l_7^2 s^2 + 8 \tau_{3,11} l_5^2 l_7^2 s^2 + 4 \tau_{3,16} l_5^2 l_7^2 s^2 - 8 \tau_{3,9} l_6^2 l_8^2 s^2 - \\
& 16 t \tau_{1,11} l_5^2 l_7^2 s - 24 u \tau_{1,11} l_5^2 l_7^2 s + (-4 s^2 + 3 t^2 + 8 u^2) \tau_{1,6} l_5^2 l_7^2 - (18 s^2 + t^2 - 8 u^2) \tau_{1,9} l_5^2 l_7^2 + \\
& 4 t^2 \tau_{2,6} l_5^2 l_7^2 + 4 u^2 \tau_{2,6} l_5^2 l_7^2 - 4 t^2 \tau_{2,11} l_5^2 l_7^2 + 4 u^2 \tau_{2,11} l_5^2 l_7^2 - 8 t^2 \tau_{3,6} l_5^2 l_7^2 + 8 u^2 \tau_{3,6} l_5^2 l_7^2 - \\
& 3 t^2 \tau_{3,9} l_5^2 l_7^2 + 7 u^2 \tau_{3,9} l_5^2 l_7^2 + 20 t^2 \tau_{3,11} l_5^2 l_7^2 + 8 t^2 \tau_{3,16} l_5^2 l_7^2 - 4 u^2 \tau_{3,16} l_5^2 l_7^2 + 4 t^2 \tau_{3,9} l_6^2 l_8^2 + \\
& 16 u^2 \tau_{3,9} l_6^2 l_8^2 - 4 t^2 \tau_{3,12} l_6^2 l_8^2 - 4 t^2 \tau_{3,13} l_6^2 l_8^2 - 2 t^2 \tau_{4,5} l_6^2 l_8^2 + 8 t^2 \tau_{4,9} l_6^2 l_8^2 + 6 u^2 \tau_{4,9} l_6^2 l_8^2 - \\
& 2(-2 \tau_{3,15} s^2 + 2 u^2 (2 \tau_{2,11} - \tau_{2,15} + 2 \tau_{3,8} + 2 \tau_{3,11} + \tau_{3,15} - 2 \tau_{3,16}) + t^2 (\tau_{2,15} + \tau_{3,11} - \tau_{3,16} + 2 \tau_{4,15})) l_6^2 l_9^2 l_{17}^2)
\end{aligned}$$

■  $N_{32}^{(8)}$

$$\frac{1}{8} (2 l_6^2 l_8^2 l_9^2 l_{17}^2 (7(s^2 + t^2) + 6 u^2) + l_5^2 (12 l_6^2 l_{15}^2 l_{16}^2 (t + 2 u)^2 - l_7^2 l_9^2 l_{17}^2 (24 s^2 + 19(t^2 + u^2))))$$
