# Supplementary material for: The Ultraviolet Behavior of N=8 Supergravity at Four Loops
Source: arXiv:0905.2326 ancillary file (2012-01-08)
Supplement: Supplementary file 28 [file SUGRA33.pdf]

## Integral 33: $\mathcal{I}_{33}$

$\mathcal{N} = 8$  four-point four-loop amplitude.

### ■ 2D plot of graph associated with $\mathcal{I}_{33}$

This fixes the labelling associated with the numerator expressions given below.

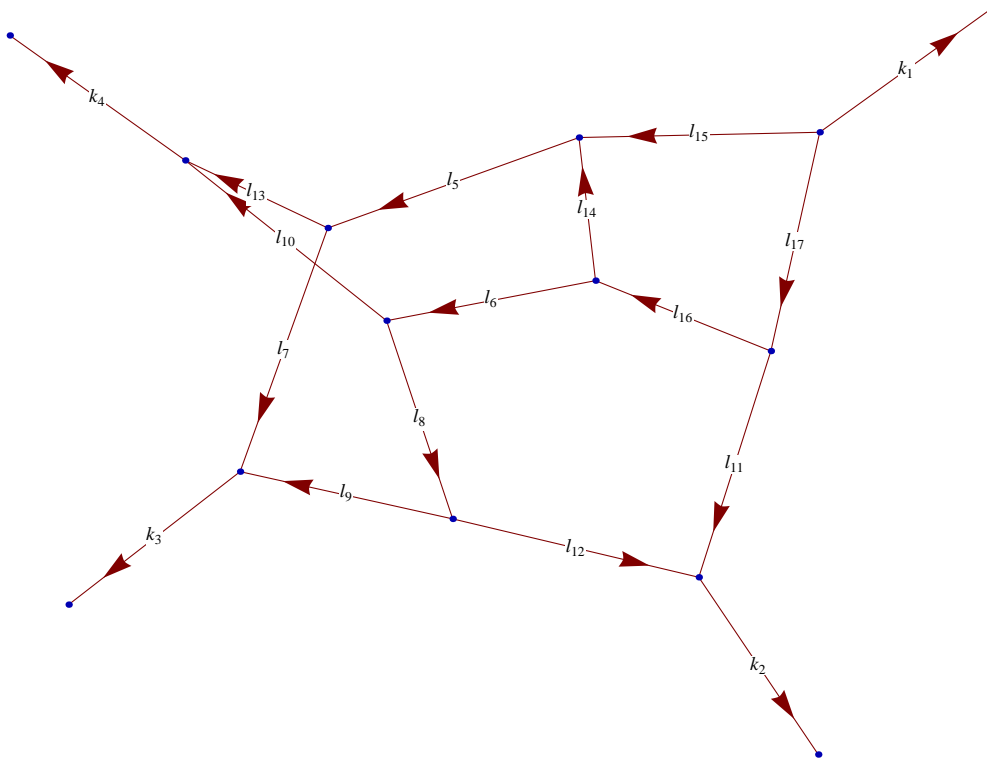

When using MathPlayer, by clicking three times (holding the click on the third click) directly on a vertex, one is able to move that vertex around, and its associated edges follow elastically. This functionality is absent when viewing as a pdf.

*Note: propagators for certain graphs were relabeled in the manuscript due to size constraints. The labels given in `aux/rawData/Neq8FourLoops.m` should be used for verification purposes.*

### ■ 3D plot of graph associated with $\mathcal{I}_{33}$

3D PLOT UNAVAILABLE FOR PDF. Please see .nb version for the 3D figure.

When using MathPlayer, by clicking anywhere in the image and dragging one should be able to rotate this 3D image. By holding (ALT) or (COMMAND) while clicking and moving the mouse up/down one should be able to zoom in/out. This functionality is absent when viewing as a pdf.

### ■ "Vertex Form" of graph associated with $\mathcal{I}_{33}$

This function returns the graph associated with the integral object in a vertex representation. This can be used as a way of specifying the topology of a graph using trivalent (cubic) vertices,  $\text{gVertex}[p_a, p_b, p_c]$ , where  $\{p_a, p_b, p_c\}$  are momenta labeling the propagators (edges) of the graph, and is understood that the edge labelled by  $p_a$  flows into the edge labelled by  $-p_a$ . Additionally, each vertex represents the manifest conservation of ( $D$  - dimensional) momenta :

$$\text{gVertex}[\{p_1, p_2, p_3\}] \iff (p_1 + p_2 + p_3 = 0)$$

$$\{\text{gVertex}(\{k_1, l_{15}, l_{17}\}), \text{gVertex}(\{k_2, -l_{12}, -l_{11}\}), \text{gVertex}(\{k_3, -l_7, -l_9\}), \text{gVertex}(\{k_4, -l_{10}, -l_{13}\}), \text{gVertex}(\{-l_5, l_7, l_{13}\}), \\ \text{gVertex}(\{l_5, -l_{14}, -l_{15}\}), \text{gVertex}(\{-l_6, l_{10}, l_8\}), \text{gVertex}(\{l_6, -l_{16}, l_{14}\}), \text{gVertex}(\{-l_8, l_9, l_{12}\}), \text{gVertex}(\{l_{11}, -l_{17}, l_{16}\})\}$$

### ■ Numerator expression for integral 33:

The following notation is used:  $\tau_{i,j} \equiv \begin{cases} 2 k_i \cdot l_j & \text{if } i \leq 4, j > 4 \\ 2 l_i \cdot l_j & \text{if } i, j > 4 \end{cases}$ .

$$s \equiv 2 k_1 \cdot k_2 = 2 k_3 \cdot k_4$$

We use  $s, t, u$  to represent the traditional Mandelstam variables for massless external four-point momenta:  $t \equiv 2 k_1 \cdot k_4 = 2 k_2 \cdot k_3$ .

$$u \equiv 2 k_1 \cdot k_3 = 2 k_2 \cdot k_4$$

Furthermore we use the shorthand  $(l_i)^2$  to represent the lorentz square:  $(l_i)^2 = l_i \cdot l_i$ .

The total numerator  $\mathcal{N}_{33}$  is given by summing over the following terms, distinguished here by explicit dependence on loop momenta:  $\mathcal{N}_{33} = \sum_{i=0}^8 \mathcal{N}_{33}^{(i)}$ :

$$\blacksquare \mathcal{N}_{33}^{(0)}$$

$$0$$

$$\blacksquare \mathcal{N}_{33}^{(1)}$$

$$0$$

$$\blacksquare \mathcal{N}_{33}^{(2)}$$

$$\frac{1}{4} s^2 (s (4 s \tau_{1,5}^2 - 2 t (4 l_7^2 s + l_6^2 t) + l_{13}^2 (t^2 - 4 u^2)) + 4 l_5^2 t^3)$$

■  $N_{33}^{(3)}$

$$\begin{aligned}
& \frac{1}{4} s \left( \left( 2 \left( (-2 \tau_{1,7} + 2 \tau_{1,10} + 2 \tau_{1,11} + \tau_{2,7} + 2 \tau_{3,11} - 2 \tau_{3,17}) l_5^2 + (\tau_{1,9} + 2 \tau_{1,14} - 2 \tau_{1,16} + \tau_{2,9} + \tau_{2,15}) l_6^2 + \right. \right. \right. \\
& \quad \left. \left. 8 \tau_{1,8} l_7^2 + 2 (4 \tau_{1,10} - \tau_{3,8} - \tau_{3,10} + 5 \tau_{3,15} + 5 \tau_{3,16} + 6 (\tau_{4,15} + \tau_{4,16})) l_7^2 \right) - \right. \\
& \quad \left. (6 \tau_{1,8} + 3 \tau_{1,9} + 9 \tau_{1,10} + \tau_{2,8} + \tau_{2,10} - 2 \tau_{3,8} - \tau_{3,10}) l_{13}^2 \right) t^3 + \frac{1}{2} (s^2 - t^2 - u^2) \\
& \quad \left( 2 \left( (-2 \tau_{1,7} + 2 \tau_{1,10} + 4 \tau_{1,11} + \tau_{2,7} - 2 (\tau_{2,17} - \tau_{3,11} + \tau_{3,17})) l_5^2 + (\tau_{1,9} + 4 \tau_{1,14} - 2 \tau_{1,16} + \tau_{2,9} + \tau_{2,15}) l_6^2 + \right. \right. \\
& \quad \left. \left. 20 \tau_{1,8} l_7^2 + 2 (10 \tau_{1,10} - \tau_{3,8} - \tau_{3,10} + 9 \tau_{3,15} + 9 \tau_{3,16} + 2 (\tau_{4,8} + 6 (\tau_{4,15} + \tau_{4,16}))) l_7^2 \right) - \right. \\
& \quad \left. (14 \tau_{1,8} + 3 \tau_{1,9} + 17 \tau_{1,10} + \tau_{2,8} + \tau_{2,10} - 12 \tau_{3,8} - 9 \tau_{3,10}) l_{13}^2 \right) t - 8 s u \tau_{1,5}^3 + \\
& \quad 8 s \tau_{1,5} \tau_{1,6} (t \tau_{2,5} + s \tau_{2,7}) - 8 s \tau_{1,5}^2 (-t \tau_{1,6} + u \tau_{2,5} + s (\tau_{1,7} + \tau_{3,6})) + \\
& \quad 4 u^3 \left( (2 \tau_{1,8} + 2 \tau_{1,10} + \tau_{3,8} + \tau_{3,10} - \tau_{3,15} - \tau_{3,16} + 2 \tau_{4,8}) l_7^2 + (-2 \tau_{1,8} + 3 \tau_{1,9} + \tau_{1,10} + \tau_{2,8} + \tau_{2,10} + 2 \tau_{3,8} + \tau_{3,10}) l_{13}^2 \right) + \\
& \quad u (s^2 - t^2 - u^2) \left( 2 \tau_{1,14} l_6^2 + 2 (8 \tau_{1,8} + 8 \tau_{1,10} + \tau_{3,8} + \tau_{3,10} + 3 \tau_{3,15} + 3 \tau_{3,16} + 4 \tau_{4,8} + 6 (\tau_{4,15} + \tau_{4,16})) l_7^2 + \right. \\
& \quad \left. (-8 \tau_{1,8} + 6 \tau_{1,9} - 2 \tau_{1,10} + 2 \tau_{2,8} + 2 \tau_{2,10} + 9 \tau_{3,8} + 6 \tau_{3,10}) l_{13}^2 \right) \Big)
\end{aligned}$$

■  $N_{33}^{(4)}$ 

$$\begin{aligned}
& -\frac{1}{2}\tau_{7,10}l_5^2t^4 + \frac{1}{2}\tau_{7,17}l_5^2t^4 + \frac{1}{2}\tau_{9,15}l_6^2t^4 - \frac{1}{2}\tau_{14,16}l_6^2t^4 - l_5^2l_6^2t^4 + \frac{1}{8}l_7^2l_{13}^2t^4 + \tau_{1,10}\tau_{3,11}l_5^2t^3 - \tau_{2,7}\tau_{3,17}l_5^2t^3 - \tau_{3,11}\tau_{3,17}l_5^2t^3 - \\
& \tau_{1,14}\tau_{1,16}l_6^2t^3 - \tau_{1,16}\tau_{2,9}l_6^2t^3 - \tau_{1,16}\tau_{2,14}l_6^2t^3 + \tau_{1,9}\tau_{2,15}l_6^2t^3 - \tau_{1,16}\tau_{2,15}l_6^2t^3 - \tau_{1,14}\tau_{3,15}l_6^2t^3 - \tau_{2,9}\tau_{3,15}l_6^2t^3 - \\
& \tau_{1,14}\tau_{3,16}l_6^2t^3 - \tau_{1,8}^2l_7^2t^3 + \tau_{1,10}^2l_7^2t^3 - 4\tau_{3,15}^2l_7^2t^3 - 4\tau_{3,16}^2l_7^2t^3 - 6\tau_{4,15}^2l_7^2t^3 - 6\tau_{4,16}^2l_7^2t^3 + 2\tau_{1,8}\tau_{3,8}l_7^2t^3 + \\
& 2\tau_{1,10}\tau_{3,8}l_7^2t^3 + 2\tau_{1,8}\tau_{3,10}l_7^2t^3 + 2\tau_{1,10}\tau_{3,10}l_7^2t^3 - 6\tau_{1,8}\tau_{3,15}l_7^2t^3 - 6\tau_{1,10}\tau_{3,15}l_7^2t^3 + 2\tau_{3,8}\tau_{3,15}l_7^2t^3 + 2\tau_{3,10}\tau_{3,15}l_7^2t^3 - \\
& 6\tau_{1,8}\tau_{3,16}l_7^2t^3 - 6\tau_{1,10}\tau_{3,16}l_7^2t^3 + 2\tau_{3,8}\tau_{3,16}l_7^2t^3 + 2\tau_{3,10}\tau_{3,16}l_7^2t^3 - 8\tau_{3,15}\tau_{3,16}l_7^2t^3 - 8\tau_{1,8}\tau_{4,15}l_7^2t^3 - \\
& 8\tau_{1,10}\tau_{4,15}l_7^2t^3 + 2\tau_{3,8}\tau_{4,15}l_7^2t^3 + 2\tau_{3,10}\tau_{4,15}l_7^2t^3 - 10\tau_{3,15}\tau_{4,15}l_7^2t^3 - 10\tau_{3,16}\tau_{4,15}l_7^2t^3 - 8\tau_{1,8}\tau_{4,16}l_7^2t^3 - \\
& 8\tau_{1,10}\tau_{4,16}l_7^2t^3 + 2\tau_{3,8}\tau_{4,16}l_7^2t^3 + 2\tau_{3,10}\tau_{4,16}l_7^2t^3 - 10\tau_{3,15}\tau_{4,16}l_7^2t^3 - 10\tau_{3,16}\tau_{4,16}l_7^2t^3 - 12\tau_{4,15}\tau_{4,16}l_7^2t^3 + \\
& \frac{7}{4}\tau_{1,8}^2l_{13}^2t^3 - \frac{3}{4}\tau_{1,9}^2l_{13}^2t^3 + \frac{1}{4}\tau_{3,8}^2l_{13}^2t^3 - 3\tau_{1,8}\tau_{1,9}l_{13}^2t^3 + \frac{5}{2}\tau_{1,8}\tau_{1,10}l_{13}^2t^3 - \frac{9}{2}\tau_{1,9}\tau_{1,10}l_{13}^2t^3 + \frac{1}{2}\tau_{1,8}\tau_{2,8}l_{13}^2t^3 - \\
& \frac{1}{2}\tau_{1,9}\tau_{2,8}l_{13}^2t^3 + \frac{1}{2}\tau_{1,8}\tau_{2,10}l_{13}^2t^3 - \frac{1}{2}\tau_{1,9}\tau_{2,10}l_{13}^2t^3 + \frac{3}{2}\tau_{1,8}\tau_{3,8}l_{13}^2t^3 + \tau_{1,9}\tau_{3,8}l_{13}^2t^3 + \frac{5}{2}\tau_{1,10}\tau_{3,8}l_{13}^2t^3 + \\
& \frac{3}{2}\tau_{1,8}\tau_{3,10}l_{13}^2t^3 + \frac{1}{2}\tau_{1,9}\tau_{3,10}l_{13}^2t^3 + 2\tau_{1,10}\tau_{3,10}l_{13}^2t^3 + \frac{1}{2}\tau_{3,8}\tau_{3,10}l_{13}^2t^3 + \frac{1}{2}(-s^2+t^2+u^2)\tau_{7,10}l_5^2t^2 - \\
& \frac{1}{2}(-s^2+t^2+u^2)\tau_{7,17}l_5^2t^2 - \frac{1}{2}(-s^2+t^2+u^2)\tau_{9,15}l_6^2t^2 + \frac{1}{2}(-s^2+t^2+u^2)\tau_{14,16}l_6^2t^2 + (-s^2+t^2+u^2)l_5^2l_6^2t^2 - \\
& \frac{3}{8}(-s^2+t^2+u^2)l_7^2l_{13}^2t^2 + \frac{1}{2}(t^2-3s^2)l_5^2l_{16}^2t^2 + \frac{1}{2}(-s^2+t^2+u^2)\tau_{2,7}\tau_{2,17}l_5^2t - (-s^2+t^2+u^2)\tau_{1,10}\tau_{3,11}l_5^2t + \\
& \frac{1}{2}(-s^2+t^2+u^2)\tau_{2,17}\tau_{3,11}l_5^2t - s\tau_{1,7}(-2t\tau_{1,11}+t\tau_{2,17}+2s\tau_{3,11})l_5^2t + (-s^2+t^2+u^2)\tau_{2,7}\tau_{3,17}l_5^2t + \\
& (-s^2+t^2+u^2)\tau_{3,11}\tau_{3,17}l_5^2t + s\tau_{1,11}(t(\tau_{3,10}+\tau_{3,17})-2u\tau_{2,7})l_5^2t + \frac{1}{4}u(-s^2+t^2+u^2)\tau_{7,10}l_5^2t - \\
& \frac{1}{4}u(-s^2+t^2+u^2)\tau_{7,17}l_5^2t + \frac{1}{2}(-s^2+t^2+u^2)\tau_{1,14}\tau_{1,16}l_6^2t + (-s^2+t^2+u^2)\tau_{1,16}\tau_{2,9}l_6^2t + \frac{1}{2}(-s^2+t^2+u^2)\tau_{1,16}\tau_{2,14}l_6^2t - \\
& \frac{1}{2}(-s^2+t^2+u^2)\tau_{1,9}\tau_{2,15}l_6^2t + \frac{1}{2}(-s^2+t^2+u^2)\tau_{1,16}\tau_{2,15}l_6^2t + \frac{1}{2}(-s^2+t^2+u^2)\tau_{2,9}\tau_{2,15}l_6^2t + \\
& (-s^2+t^2+u^2)\tau_{1,14}\tau_{3,15}l_6^2t + (-s^2+t^2+u^2)\tau_{2,9}\tau_{3,15}l_6^2t + (-s^2+t^2+u^2)\tau_{1,14}\tau_{3,16}l_6^2t - \frac{1}{4}u(-s^2+t^2+u^2)\tau_{9,15}l_6^2t + \\
& \frac{1}{4}u(-s^2+t^2+u^2)\tau_{14,16}l_6^2t + \frac{1}{2}u(-s^2+t^2+u^2)l_5^2l_6^2t + \frac{3}{2}(-s^2+t^2+u^2)\tau_{1,8}^2l_7^2t - \frac{3}{2}(-s^2+t^2+u^2)\tau_{1,10}^2l_7^2t + \\
& 3(-s^2+t^2+u^2)\tau_{3,15}^2l_7^2t + 3(-s^2+t^2+u^2)\tau_{3,16}^2l_7^2t + 6(-s^2+t^2+u^2)\tau_{4,15}^2l_7^2t + 6(-s^2+t^2+u^2)\tau_{4,16}^2l_7^2t - \\
& 2(-s^2+t^2+u^2)\tau_{1,8}\tau_{3,8}l_7^2t - 2(-s^2+t^2+u^2)\tau_{1,10}\tau_{3,8}l_7^2t - 2(-s^2+t^2+u^2)\tau_{1,8}\tau_{3,10}l_7^2t - 2(-s^2+t^2+u^2)\tau_{1,10}\tau_{3,10}l_7^2t +
\end{aligned}$$

$$\begin{aligned}
& 7(-s^2 + t^2 + u^2) \tau_{1,8} \tau_{3,15} l_7^2 t + 7(-s^2 + t^2 + u^2) \tau_{1,10} \tau_{3,15} l_7^2 t - (-s^2 + t^2 + u^2) \tau_{3,8} \tau_{3,15} l_7^2 t - (-s^2 + t^2 + u^2) \tau_{3,10} \tau_{3,15} l_7^2 t + \\
& 7(-s^2 + t^2 + u^2) \tau_{1,8} \tau_{3,16} l_7^2 t + 7(-s^2 + t^2 + u^2) \tau_{1,10} \tau_{3,16} l_7^2 t - (-s^2 + t^2 + u^2) \tau_{3,8} \tau_{3,16} l_7^2 t - (-s^2 + t^2 + u^2) \tau_{3,10} \tau_{3,16} l_7^2 t + \\
& 6(-s^2 + t^2 + u^2) \tau_{3,15} \tau_{3,16} l_7^2 t + (-s^2 + t^2 + u^2) \tau_{1,8} \tau_{4,8} l_7^2 t + (-s^2 + t^2 + u^2) \tau_{1,10} \tau_{4,8} l_7^2 t + 2(-s^2 + t^2 + u^2) \tau_{3,15} \tau_{4,8} l_7^2 t + \\
& 2(-s^2 + t^2 + u^2) \tau_{3,16} \tau_{4,8} l_7^2 t + 10(-s^2 + t^2 + u^2) \tau_{1,8} \tau_{4,15} l_7^2 t + 10(-s^2 + t^2 + u^2) \tau_{1,10} \tau_{4,15} l_7^2 t - \\
& (-s^2 + t^2 + u^2) \tau_{3,8} \tau_{4,15} l_7^2 t - (-s^2 + t^2 + u^2) \tau_{3,10} \tau_{4,15} l_7^2 t + 9(-s^2 + t^2 + u^2) \tau_{3,15} \tau_{4,15} l_7^2 t + 9(-s^2 + t^2 + u^2) \tau_{3,16} \tau_{4,15} l_7^2 t + \\
& 2(-s^2 + t^2 + u^2) \tau_{4,8} \tau_{4,15} l_7^2 t + 10(-s^2 + t^2 + u^2) \tau_{1,8} \tau_{4,16} l_7^2 t + 10(-s^2 + t^2 + u^2) \tau_{1,10} \tau_{4,16} l_7^2 t - \\
& (-s^2 + t^2 + u^2) \tau_{3,8} \tau_{4,16} l_7^2 t - (-s^2 + t^2 + u^2) \tau_{3,10} \tau_{4,16} l_7^2 t + 9(-s^2 + t^2 + u^2) \tau_{3,15} \tau_{4,16} l_7^2 t + 9(-s^2 + t^2 + u^2) \tau_{3,16} \tau_{4,16} l_7^2 t + \\
& 2(-s^2 + t^2 + u^2) \tau_{4,8} \tau_{4,16} l_7^2 t + 12(-s^2 + t^2 + u^2) \tau_{4,15} \tau_{4,16} l_7^2 t - \frac{15}{8} (-s^2 + t^2 + u^2) \tau_{1,8}^2 l_{13}^2 t + \frac{3}{8} (-s^2 + t^2 + u^2) \tau_{1,9}^2 l_{13}^2 t - \\
& (-s^2 + t^2 + u^2) \tau_{1,10}^2 l_{13}^2 t - \frac{3}{8} (-s^2 + t^2 + u^2) \tau_{3,8}^2 l_{13}^2 t + \frac{7}{2} (-s^2 + t^2 + u^2) \tau_{1,8} \tau_{1,9} l_{13}^2 t - \frac{13}{4} (-s^2 + t^2 + u^2) \tau_{1,8} \tau_{1,10} l_{13}^2 t + \\
& \frac{17}{4} (-s^2 + t^2 + u^2) \tau_{1,9} \tau_{1,10} l_{13}^2 t - \frac{5}{4} (-s^2 + t^2 + u^2) \tau_{1,8} \tau_{2,8} l_{13}^2 t + \frac{1}{4} (-s^2 + t^2 + u^2) \tau_{1,9} \tau_{2,8} l_{13}^2 t - \\
& (-s^2 + t^2 + u^2) \tau_{1,10} \tau_{2,8} l_{13}^2 t - \frac{5}{4} (-s^2 + t^2 + u^2) \tau_{1,8} \tau_{2,10} l_{13}^2 t + \frac{1}{4} (-s^2 + t^2 + u^2) \tau_{1,9} \tau_{2,10} l_{13}^2 t - \\
& (-s^2 + t^2 + u^2) \tau_{1,10} \tau_{2,10} l_{13}^2 t - \frac{3}{2} (-s^2 + t^2 + u^2) \tau_{1,8} \tau_{3,8} l_{13}^2 t - 3(-s^2 + t^2 + u^2) \tau_{1,9} \tau_{3,8} l_{13}^2 t - \\
& \frac{9}{2} (-s^2 + t^2 + u^2) \tau_{1,10} \tau_{3,8} l_{13}^2 t - \frac{3}{4} (-s^2 + t^2 + u^2) \tau_{1,8} \tau_{3,10} l_{13}^2 t - \frac{9}{4} (-s^2 + t^2 + u^2) \tau_{1,9} \tau_{3,10} l_{13}^2 t - \\
& 3(-s^2 + t^2 + u^2) \tau_{1,10} \tau_{3,10} l_{13}^2 t - \frac{1}{2} (-s^2 + t^2 + u^2) \tau_{3,8} \tau_{3,10} l_{13}^2 t - \frac{5}{8} u(-s^2 + t^2 + u^2) l_7^2 l_{13}^2 t + u^2 \tau_{1,5}^4 + \\
& \tau_{1,6}^2 (t \tau_{2,5} + s \tau_{2,7})^2 + 2 \tau_{1,5} \tau_{1,6} (t \tau_{2,5} + s \tau_{2,7}) (t \tau_{1,6} - u \tau_{2,5} - s(\tau_{1,7} + \tau_{3,6})) + 2 u \tau_{1,5}^3 (-t \tau_{1,6} + u \tau_{2,5} + s(\tau_{1,7} + \tau_{3,6})) + \\
& \tau_{1,5}^2 (t^2 \tau_{1,6}^2 - 2(s t \tau_{1,7} + (s^2 - t^2 - u^2) \tau_{2,5} + s(u \tau_{2,7} + t \tau_{3,6})) \tau_{1,6} + (u \tau_{2,5} + s(\tau_{1,7} + \tau_{3,6}))^2) + \\
& \frac{1}{2} u(-s^2 + t^2 + u^2) \tau_{2,7} \tau_{2,17} l_5^2 - \frac{1}{2} u(-s^2 + t^2 + u^2) \tau_{1,10} \tau_{3,11} l_5^2 + \frac{1}{2} u(-s^2 + t^2 + u^2) \tau_{2,17} \tau_{3,11} l_5^2 + \\
& \frac{1}{2} u(-s^2 + t^2 + u^2) \tau_{2,7} \tau_{3,17} l_5^2 + \frac{1}{2} u(-s^2 + t^2 + u^2) \tau_{3,11} \tau_{3,17} l_5^2 + \frac{1}{2} u(-s^2 + t^2 + u^2) \tau_{1,16} \tau_{2,9} l_6^2 + \\
& \frac{1}{2} u(-s^2 + t^2 + u^2) \tau_{2,9} \tau_{2,15} l_6^2 + \frac{1}{2} u(-s^2 + t^2 + u^2) \tau_{1,14} \tau_{3,15} l_6^2 + \frac{1}{2} u(-s^2 + t^2 + u^2) \tau_{2,9} \tau_{3,15} l_6^2 + \\
& \frac{1}{2} u(-s^2 + t^2 + u^2) \tau_{1,14} \tau_{3,16} l_6^2 - u^3 \tau_{1,8}^2 l_7^2 + \frac{3}{2} u(-s^2 + t^2 + u^2) \tau_{1,8}^2 l_7^2 + u^3 \tau_{1,10}^2 l_7^2 - \frac{3}{2} u(-s^2 + t^2 + u^2) \tau_{1,10}^2 l_7^2 + \\
& 2 u^3 \tau_{3,15}^2 l_7^2 + 2 u^3 \tau_{3,16}^2 l_7^2 + 3 u(-s^2 + t^2 + u^2) \tau_{4,15}^2 l_7^2 + 3 u(-s^2 + t^2 + u^2) \tau_{4,16}^2 l_7^2 - u(-s^2 + t^2 + u^2) \tau_{1,8} \tau_{3,8} l_7^2 - \\
& u(-s^2 + t^2 + u^2) \tau_{1,10} \tau_{3,8} l_7^2 - u(-s^2 + t^2 + u^2) \tau_{1,8} \tau_{3,10} l_7^2 - u(-s^2 + t^2 + u^2) \tau_{1,10} \tau_{3,10} l_7^2 - 2 u^3 \tau_{1,8} \tau_{3,15} l_7^2 +
\end{aligned}$$

$$\begin{aligned}
& 5u(-s^2 + t^2 + u^2)\tau_{1,8}\tau_{3,15}l_7^2 - 2u^3\tau_{1,10}\tau_{3,15}l_7^2 + 5u(-s^2 + t^2 + u^2)\tau_{1,10}\tau_{3,15}l_7^2 - 2u^3\tau_{3,8}\tau_{3,15}l_7^2 + \\
& u(-s^2 + t^2 + u^2)\tau_{3,8}\tau_{3,15}l_7^2 - 2u^3\tau_{3,10}\tau_{3,15}l_7^2 + u(-s^2 + t^2 + u^2)\tau_{3,10}\tau_{3,15}l_7^2 - 2u^3\tau_{1,8}\tau_{3,16}l_7^2 + \\
& 5u(-s^2 + t^2 + u^2)\tau_{1,8}\tau_{3,16}l_7^2 - 2u^3\tau_{1,10}\tau_{3,16}l_7^2 + 5u(-s^2 + t^2 + u^2)\tau_{1,10}\tau_{3,16}l_7^2 - 2u^3\tau_{3,8}\tau_{3,16}l_7^2 + \\
& u(-s^2 + t^2 + u^2)\tau_{3,8}\tau_{3,16}l_7^2 - 2u^3\tau_{3,10}\tau_{3,16}l_7^2 + u(-s^2 + t^2 + u^2)\tau_{3,10}\tau_{3,16}l_7^2 + 4u^3\tau_{3,15}\tau_{3,16}l_7^2 - \\
& 2u^3\tau_{1,8}\tau_{4,8}l_7^2 + 2u(-s^2 + t^2 + u^2)\tau_{1,8}\tau_{4,8}l_7^2 - 2u^3\tau_{1,10}\tau_{4,8}l_7^2 + 2u(-s^2 + t^2 + u^2)\tau_{1,10}\tau_{4,8}l_7^2 - 4u^3\tau_{3,15}\tau_{4,8}l_7^2 + \\
& 4u(-s^2 + t^2 + u^2)\tau_{3,15}\tau_{4,8}l_7^2 - 4u^3\tau_{3,16}\tau_{4,8}l_7^2 + 4u(-s^2 + t^2 + u^2)\tau_{3,16}\tau_{4,8}l_7^2 - 4u^3\tau_{1,8}\tau_{4,15}l_7^2 + \\
& 8u(-s^2 + t^2 + u^2)\tau_{1,8}\tau_{4,15}l_7^2 - 4u^3\tau_{1,10}\tau_{4,15}l_7^2 + 8u(-s^2 + t^2 + u^2)\tau_{1,10}\tau_{4,15}l_7^2 - 2u^3\tau_{3,8}\tau_{4,15}l_7^2 + \\
& u(-s^2 + t^2 + u^2)\tau_{3,8}\tau_{4,15}l_7^2 - 2u^3\tau_{3,10}\tau_{4,15}l_7^2 + u(-s^2 + t^2 + u^2)\tau_{3,10}\tau_{4,15}l_7^2 + 2u^3\tau_{3,15}\tau_{4,15}l_7^2 + \\
& 3u(-s^2 + t^2 + u^2)\tau_{3,15}\tau_{4,15}l_7^2 + 2u^3\tau_{3,16}\tau_{4,15}l_7^2 + 3u(-s^2 + t^2 + u^2)\tau_{3,16}\tau_{4,15}l_7^2 - 4u^3\tau_{4,8}\tau_{4,15}l_7^2 + \\
& 4u(-s^2 + t^2 + u^2)\tau_{4,8}\tau_{4,15}l_7^2 - 4u^3\tau_{1,8}\tau_{4,16}l_7^2 + 8u(-s^2 + t^2 + u^2)\tau_{1,8}\tau_{4,16}l_7^2 - 4u^3\tau_{1,10}\tau_{4,16}l_7^2 + \\
& 8u(-s^2 + t^2 + u^2)\tau_{1,10}\tau_{4,16}l_7^2 - 2u^3\tau_{3,8}\tau_{4,16}l_7^2 + u(-s^2 + t^2 + u^2)\tau_{3,8}\tau_{4,16}l_7^2 - 2u^3\tau_{3,10}\tau_{4,16}l_7^2 + \\
& u(-s^2 + t^2 + u^2)\tau_{3,10}\tau_{4,16}l_7^2 + 2u^3\tau_{3,15}\tau_{4,16}l_7^2 + 3u(-s^2 + t^2 + u^2)\tau_{3,15}\tau_{4,16}l_7^2 + 2u^3\tau_{3,16}\tau_{4,16}l_7^2 + \\
& 3u(-s^2 + t^2 + u^2)\tau_{3,16}\tau_{4,16}l_7^2 - 4u^3\tau_{4,8}\tau_{4,16}l_7^2 + 4u(-s^2 + t^2 + u^2)\tau_{4,8}\tau_{4,16}l_7^2 + 6u(-s^2 + t^2 + u^2)\tau_{4,15}\tau_{4,16}l_7^2 + \\
& u^3\tau_{1,8}^2l_{13}^2 - \frac{3}{2}u(-s^2 + t^2 + u^2)\tau_{1,8}^2l_{13}^2 + 3u^3\tau_{1,9}^2l_{13}^2 - \frac{3}{2}u(-s^2 + t^2 + u^2)\tau_{1,9}^2l_{13}^2 + 2u^3\tau_{1,10}^2l_{13}^2 - \\
& 2u(-s^2 + t^2 + u^2)\tau_{1,10}^2l_{13}^2 + \frac{1}{4}u^3\tau_{3,8}^2l_{13}^2 - \frac{3}{8}u(-s^2 + t^2 + u^2)\tau_{3,8}^2l_{13}^2 - 4u^3\tau_{1,8}\tau_{1,9}l_{13}^2 + 4u(-s^2 + t^2 + u^2)\tau_{1,8}\tau_{1,9}l_{13}^2 - \\
& 2u(-s^2 + t^2 + u^2)\tau_{1,8}\tau_{1,10}l_{13}^2 + 2u^3\tau_{1,9}\tau_{1,10}l_{13}^2 + u(-s^2 + t^2 + u^2)\tau_{1,9}\tau_{1,10}l_{13}^2 - u(-s^2 + t^2 + u^2)\tau_{1,8}\tau_{2,8}l_{13}^2 + \\
& 2u^3\tau_{1,9}\tau_{2,8}l_{13}^2 - u(-s^2 + t^2 + u^2)\tau_{1,9}\tau_{2,8}l_{13}^2 + 2u^3\tau_{1,10}\tau_{2,8}l_{13}^2 - 2u(-s^2 + t^2 + u^2)\tau_{1,10}\tau_{2,8}l_{13}^2 - \\
& u(-s^2 + t^2 + u^2)\tau_{1,8}\tau_{2,10}l_{13}^2 + 2u^3\tau_{1,9}\tau_{2,10}l_{13}^2 - u(-s^2 + t^2 + u^2)\tau_{1,9}\tau_{2,10}l_{13}^2 + 2u^3\tau_{1,10}\tau_{2,10}l_{13}^2 - \\
& 2u(-s^2 + t^2 + u^2)\tau_{1,10}\tau_{2,10}l_{13}^2 - \frac{3}{4}u(-s^2 + t^2 + u^2)\tau_{1,8}\tau_{3,8}l_{13}^2 + 4u^3\tau_{1,9}\tau_{3,8}l_{13}^2 - \frac{9}{2}u(-s^2 + t^2 + u^2)\tau_{1,9}\tau_{3,8}l_{13}^2 + \\
& 4u^3\tau_{1,10}\tau_{3,8}l_{13}^2 - \frac{21}{4}u(-s^2 + t^2 + u^2)\tau_{1,10}\tau_{3,8}l_{13}^2 + 2u^3\tau_{1,9}\tau_{3,10}l_{13}^2 - 3u(-s^2 + t^2 + u^2)\tau_{1,9}\tau_{3,10}l_{13}^2 + 2u^3\tau_{1,10}\tau_{3,10}l_{13}^2 - \\
& 3u(-s^2 + t^2 + u^2)\tau_{1,10}\tau_{3,10}l_{13}^2 - \frac{1}{4}u(-s^2 + t^2 + u^2)\tau_{3,8}\tau_{3,10}l_{13}^2 + \frac{1}{8}u^4l_7^2l_{13}^2 - \frac{3}{8}u^2(-s^2 + t^2 + u^2)l_7^2l_{13}^2
\end{aligned}$$

■  $N_{33}^{(5)}$

$$\begin{aligned}
& -\frac{1}{2}\tau_{1,9}l_7^2l_{13}^2t^3 - \frac{1}{8}\tau_{3,9}l_7^2l_{13}^2t^3 - \frac{1}{2}\tau_{3,11}l_7^2l_{13}^2t^3 - \frac{1}{8}\tau_{4,9}l_7^2l_{13}^2t^3 - \frac{1}{4}\tau_{4,10}l_7^2l_{13}^2t^3 - \frac{3}{4}\tau_{4,11}l_7^2l_{13}^2t^3 - \tau_{3,15}^3l_7^2t^2 - \\
& \tau_{3,16}^3l_7^2t^2 - 2\tau_{4,15}^3l_7^2t^2 - 2\tau_{4,16}^3l_7^2t^2 - 3\tau_{3,15}\tau_{3,16}^2l_7^2t^2 - 5\tau_{3,15}\tau_{4,15}^2l_7^2t^2 - 5\tau_{3,16}\tau_{4,15}^2l_7^2t^2 - 5\tau_{3,15}\tau_{4,16}^2l_7^2t^2 - \\
& 5\tau_{3,16}\tau_{4,16}^2l_7^2t^2 - 6\tau_{4,15}\tau_{4,16}^2l_7^2t^2 - 3\tau_{3,15}^2\tau_{3,16}l_7^2t^2 - 4\tau_{3,15}^2\tau_{4,15}l_7^2t^2 - 4\tau_{3,16}^2\tau_{4,15}l_7^2t^2 - 8\tau_{3,15}\tau_{3,16}\tau_{4,15}l_7^2t^2 - \\
& 4\tau_{3,15}^2\tau_{4,16}l_7^2t^2 - 4\tau_{3,16}^2\tau_{4,16}l_7^2t^2 - 6\tau_{4,15}^2\tau_{4,16}l_7^2t^2 - 8\tau_{3,15}\tau_{3,16}\tau_{4,16}l_7^2t^2 - 10\tau_{3,15}\tau_{4,15}\tau_{4,16}l_7^2t^2 -
\end{aligned}$$

$$\begin{aligned}
& 10 \tau_{3,16} \tau_{4,15} \tau_{4,16} l_7^2 t^2 + \frac{1}{4} \tau_{1,9}^3 l_{13}^2 t^2 + \frac{1}{4} \tau_{1,9}^2 \tau_{2,8} l_{13}^2 t^2 + \frac{1}{4} \tau_{1,9}^2 \tau_{2,10} l_{13}^2 t^2 + \frac{3}{4} (-s^2 + t^2 + u^2) \tau_{1,9} l_7^2 l_{13}^2 t + \\
& \frac{3}{16} (-s^2 + t^2 + u^2) \tau_{3,9} l_7^2 l_{13}^2 t + \frac{5}{8} (-s^2 + t^2 + u^2) \tau_{3,11} l_7^2 l_{13}^2 t + \frac{3}{16} (-s^2 + t^2 + u^2) \tau_{4,9} l_7^2 l_{13}^2 t + \frac{1}{4} (-s^2 + t^2 + u^2) \tau_{4,10} l_7^2 l_{13}^2 t + \\
& \frac{3}{4} (-s^2 + t^2 + u^2) \tau_{4,11} l_7^2 l_{13}^2 t + u^2 \tau_{3,15}^3 l_7^2 + u^2 \tau_{3,16}^3 l_7^2 + (-s^2 + t^2 + u^2) \tau_{4,15}^3 l_7^2 + (-s^2 + t^2 + u^2) \tau_{4,16}^3 l_7^2 + \\
& 3 u^2 \tau_{3,15} \tau_{3,16}^2 l_7^2 + u^2 \tau_{3,15} \tau_{4,15}^2 l_7^2 + 2 (-s^2 + t^2 + u^2) \tau_{3,15} \tau_{4,15}^2 l_7^2 + u^2 \tau_{3,16} \tau_{4,15}^2 l_7^2 + 2 (-s^2 + t^2 + u^2) \tau_{3,16} \tau_{4,15}^2 l_7^2 - \\
& 2 u^2 \tau_{4,8} \tau_{4,15}^2 l_7^2 + (-s^2 + t^2 + u^2) \tau_{4,8} \tau_{4,15}^2 l_7^2 + u^2 \tau_{3,15} \tau_{4,16}^2 l_7^2 + 2 (-s^2 + t^2 + u^2) \tau_{3,15} \tau_{4,16}^2 l_7^2 + u^2 \tau_{3,16} \tau_{4,16}^2 l_7^2 + \\
& 2 (-s^2 + t^2 + u^2) \tau_{3,16} \tau_{4,16}^2 l_7^2 - 2 u^2 \tau_{4,8} \tau_{4,16}^2 l_7^2 + (-s^2 + t^2 + u^2) \tau_{4,8} \tau_{4,16}^2 l_7^2 + 3 (-s^2 + t^2 + u^2) \tau_{4,15} \tau_{4,16}^2 l_7^2 + \\
& 3 u^2 \tau_{3,15}^2 \tau_{3,16} l_7^2 - 2 u^2 \tau_{3,15}^2 \tau_{4,8} l_7^2 + (-s^2 + t^2 + u^2) \tau_{3,15}^2 \tau_{4,8} l_7^2 - 2 u^2 \tau_{3,16}^2 \tau_{4,8} l_7^2 + (-s^2 + t^2 + u^2) \tau_{3,16}^2 \tau_{4,8} l_7^2 - \\
& 4 u^2 \tau_{3,15} \tau_{3,16} \tau_{4,8} l_7^2 + 2 (-s^2 + t^2 + u^2) \tau_{3,15} \tau_{3,16} \tau_{4,8} l_7^2 + 2 u^2 \tau_{3,15}^2 \tau_{4,15} l_7^2 + (-s^2 + t^2 + u^2) \tau_{3,15}^2 \tau_{4,15} l_7^2 + \\
& 2 u^2 \tau_{3,16}^2 \tau_{4,15} l_7^2 + (-s^2 + t^2 + u^2) \tau_{3,16}^2 \tau_{4,15} l_7^2 + 4 u^2 \tau_{3,15} \tau_{3,16} \tau_{4,15} l_7^2 + 2 (-s^2 + t^2 + u^2) \tau_{3,15} \tau_{3,16} \tau_{4,15} l_7^2 - \\
& 4 u^2 \tau_{3,15} \tau_{4,8} \tau_{4,15} l_7^2 + 2 (-s^2 + t^2 + u^2) \tau_{3,15} \tau_{4,8} \tau_{4,15} l_7^2 - 4 u^2 \tau_{3,16} \tau_{4,8} \tau_{4,15} l_7^2 + 2 (-s^2 + t^2 + u^2) \tau_{3,16} \tau_{4,8} \tau_{4,15} l_7^2 + \\
& 2 u^2 \tau_{3,15}^2 \tau_{4,16} l_7^2 + (-s^2 + t^2 + u^2) \tau_{3,15}^2 \tau_{4,16} l_7^2 + 2 u^2 \tau_{3,16}^2 \tau_{4,16} l_7^2 + (-s^2 + t^2 + u^2) \tau_{3,16}^2 \tau_{4,16} l_7^2 + \\
& 3 (-s^2 + t^2 + u^2) \tau_{4,15}^2 \tau_{4,16} l_7^2 + 4 u^2 \tau_{3,15} \tau_{3,16} \tau_{4,16} l_7^2 + 2 (-s^2 + t^2 + u^2) \tau_{3,15} \tau_{3,16} \tau_{4,16} l_7^2 - 4 u^2 \tau_{3,15} \tau_{4,8} \tau_{4,16} l_7^2 + \\
& 2 (-s^2 + t^2 + u^2) \tau_{3,15} \tau_{4,8} \tau_{4,16} l_7^2 - 4 u^2 \tau_{3,16} \tau_{4,8} \tau_{4,16} l_7^2 + 2 (-s^2 + t^2 + u^2) \tau_{3,16} \tau_{4,8} \tau_{4,16} l_7^2 + 2 u^2 \tau_{3,15} \tau_{4,15} \tau_{4,16} l_7^2 + \\
& 4 (-s^2 + t^2 + u^2) \tau_{3,15} \tau_{4,15} \tau_{4,16} l_7^2 + 2 u^2 \tau_{3,16} \tau_{4,15} \tau_{4,16} l_7^2 + 4 (-s^2 + t^2 + u^2) \tau_{3,16} \tau_{4,15} \tau_{4,16} l_7^2 - \\
& 4 u^2 \tau_{4,8} \tau_{4,15} \tau_{4,16} l_7^2 + 2 (-s^2 + t^2 + u^2) \tau_{4,8} \tau_{4,15} \tau_{4,16} l_7^2 - u^2 \tau_{1,9}^3 l_{13}^2 - s^2 \tau_{1,10}^3 l_{13}^2 - u^2 \tau_{1,9}^2 \tau_{2,8} l_{13}^2 - \\
& u^2 \tau_{1,9}^2 \tau_{2,10} l_{13}^2 + \frac{1}{4} s^2 \tau_{3,8}^2 (-\tau_{1,9} + \tau_{2,8} + \tau_{2,10} + \tau_{3,10}) l_{13}^2 - \frac{1}{2} u^3 \tau_{1,9} l_7^2 l_{13}^2 + \frac{3}{4} u (-s^2 + t^2 + u^2) \tau_{1,9} l_7^2 l_{13}^2 - \\
& \frac{1}{8} u^3 \tau_{3,9} l_7^2 l_{13}^2 + \frac{3}{16} u (-s^2 + t^2 + u^2) \tau_{3,9} l_7^2 l_{13}^2 - \frac{3}{4} u^3 \tau_{3,11} l_7^2 l_{13}^2 + \frac{3}{4} u (-s^2 + t^2 + u^2) \tau_{3,11} l_7^2 l_{13}^2 - \frac{1}{8} u^3 \tau_{4,9} l_7^2 l_{13}^2 + \\
& \frac{3}{16} u (-s^2 + t^2 + u^2) \tau_{4,9} l_7^2 l_{13}^2 + \frac{1}{8} u (-s^2 + t^2 + u^2) \tau_{4,10} l_7^2 l_{13}^2 - \frac{1}{2} u^3 \tau_{4,11} l_7^2 l_{13}^2 + \frac{5}{8} u (-s^2 + t^2 + u^2) \tau_{4,11} l_7^2 l_{13}^2 + \\
& \frac{1}{4} \tau_{1,8}^2 (4 s^2 (\tau_{3,8} - \tau_{3,15} - \tau_{3,16} - 2 \tau_{4,15} - 2 \tau_{4,16}) l_7^2 - (-4 \tau_{2,8} s^2 + (4 s^2 + 3 t^2) \tau_{1,9} + 3 t^2 (\tau_{1,10} + \tau_{2,8} + \tau_{2,10} - \tau_{3,10})) l_{13}^2) + \\
& \frac{1}{2} \tau_{3,8} (2 (t^2 - u^2) l_7^2 (\tau_{3,15} + \tau_{3,16} + \tau_{4,15} + \tau_{4,16})^2 + s \tau_{1,9} ((t + 4 u) \tau_{1,9} + t \tau_{3,10}) l_{13}^2) - \\
& s \tau_{1,10}^2 ((s (\tau_{2,10} + 2 \tau_{3,8} + \tau_{3,10}) - 2 u \tau_{1,9}) l_{13}^2 - s (\tau_{3,8} + \tau_{3,15} + \tau_{3,16}) l_7^2) + \\
& \frac{1}{4} \tau_{3,10} (4 (t^2 - u^2) (\tau_{3,15} + \tau_{3,16} + \tau_{4,15} + \tau_{4,16})^2 l_7^2 - (u l_7^2 s^2 + (4 s^2 - 3 t^2) \tau_{1,9}^2) l_{13}^2) - \\
& \frac{1}{4} \tau_{1,10} (16 \tau_{4,15}^2 l_7^2 t^2 + 16 \tau_{4,16}^2 l_7^2 t^2 + 32 \tau_{4,15} \tau_{4,16} l_7^2 t^2 - 8 s \tau_{3,15}^2 l_7^2 t - 8 s \tau_{3,16}^2 l_7^2 t + 8 u^2 \tau_{4,15}^2 l_7^2 +
\end{aligned}$$

$$\begin{aligned}
& 12(s^2 - t^2 - u^2)\tau_{4,15}^2 l_7^2 + 8u^2 \tau_{4,16}^2 l_7^2 + 12(s^2 - t^2 - u^2)\tau_{4,16}^2 l_7^2 + 8u^2 \tau_{4,8} \tau_{4,15} l_7^2 + 4(s^2 - t^2 - u^2)\tau_{4,8} \tau_{4,15} l_7^2 + \\
& 8u^2 \tau_{4,8} \tau_{4,16} l_7^2 + 4(s^2 - t^2 - u^2)\tau_{4,8} \tau_{4,16} l_7^2 + 16u^2 \tau_{4,15} \tau_{4,16} l_7^2 + 24(s^2 - t^2 - u^2)\tau_{4,15} \tau_{4,16} l_7^2 - \\
& 8s \tau_{3,16} (u \tau_{4,8} + (3t + u)(\tau_{4,15} + \tau_{4,16})) l_7^2 - 8s \tau_{3,15} (2t \tau_{3,16} + u \tau_{4,8} + (3t + u)(\tau_{4,15} + \tau_{4,16})) l_7^2 + \\
& s^2 \tau_{3,8}^2 l_{13}^2 - (2l_7^2 s^3 + 8u \tau_{1,9} (\tau_{2,8} + \tau_{2,10}) s + (4s^2 + 5t^2 - 8u^2) \tau_{1,9}^2) l_{13}^2 - \\
& 8s \tau_{3,10} (-t(\tau_{3,15} + \tau_{3,16} + \tau_{4,15} + \tau_{4,16}) l_7^2 - s \tau_{1,9} l_{13}^2) - 2s \tau_{3,8} ((5t + 8u) \tau_{1,9} l_{13}^2 - 4t(\tau_{3,15} + \tau_{3,16} + \tau_{4,15} + \tau_{4,16}) l_7^2) - \\
& \frac{1}{2} \tau_{1,8} (4\tau_{3,16}^2 l_7^2 t^2 + 8\tau_{4,15}^2 l_7^2 t^2 + 8\tau_{4,16}^2 l_7^2 t^2 + 12\tau_{3,16} \tau_{4,15} l_7^2 t^2 + 12\tau_{3,16} \tau_{4,16} l_7^2 t^2 + 16\tau_{4,15} \tau_{4,16} l_7^2 t^2 - 4s \tau_{3,15}^2 l_7^2 t + \\
& 4s \tau_{3,10} (\tau_{3,15} + \tau_{3,16} + \tau_{4,15} + \tau_{4,16}) l_7^2 t - 4s \tau_{1,10}^2 l_{13}^2 t - s \tau_{3,8} ((3\tau_{1,9} - \tau_{3,10}) l_{13}^2 - 4(\tau_{3,15} + \tau_{3,16} + \tau_{4,15} + \tau_{4,16}) l_7^2) t + \\
& 2(s^2 - t^2 - u^2) \tau_{3,16}^2 l_7^2 + 4u^2 \tau_{4,15}^2 l_7^2 + 6(s^2 - t^2 - u^2) \tau_{4,15}^2 l_7^2 + 4u^2 \tau_{4,16}^2 l_7^2 + 6(s^2 - t^2 - u^2) \tau_{4,16}^2 l_7^2 + \\
& 4u^2 \tau_{3,16} \tau_{4,8} l_7^2 + 2(s^2 - t^2 - u^2) \tau_{3,16} \tau_{4,8} l_7^2 + 4u^2 \tau_{3,16} \tau_{4,15} l_7^2 + 8(s^2 - t^2 - u^2) \tau_{3,16} \tau_{4,15} l_7^2 + \\
& 4u^2 \tau_{4,8} \tau_{4,15} l_7^2 + 2(s^2 - t^2 - u^2) \tau_{4,8} \tau_{4,15} l_7^2 + 4u^2 \tau_{3,16} \tau_{4,16} l_7^2 + 8(s^2 - t^2 - u^2) \tau_{3,16} \tau_{4,16} l_7^2 + \\
& 4u^2 \tau_{4,8} \tau_{4,16} l_7^2 + 2(s^2 - t^2 - u^2) \tau_{4,8} \tau_{4,16} l_7^2 + 8u^2 \tau_{4,15} \tau_{4,16} l_7^2 + 12(s^2 - t^2 - u^2) \tau_{4,15} \tau_{4,16} l_7^2 - \\
& 4s \tau_{3,15} (2t \tau_{3,16} + u \tau_{4,8} + (3t + u)(\tau_{4,15} + \tau_{4,16})) l_7^2 + \tau_{1,9} (t((t + 4u)(\tau_{2,8} + \tau_{2,10}) + 3t \tau_{3,10}) - (2s^2 + t^2 + 2u^2) \tau_{1,9}) \\
& l_{13}^2 + \tau_{1,10} (4(-\tau_{3,8} + \tau_{4,15} + \tau_{4,16}) l_7^2 s^2 + (t(5t + 8u) \tau_{1,9} + s(4u \tau_{2,8} - 4t \tau_{2,10} - 3t \tau_{3,8})) l_{13}^2))
\end{aligned}$$

■  $N_{33}^{(6)}$

$$\begin{aligned}
& -\frac{1}{8} l_7^2 l_{13}^2 \\
& (2\tau_{4,11}^2 (-4s^2 + 2t^2 + u^2) + \tau_{4,11} (6\tau_{3,11} (-3s^2 + t^2 + u^2) - \tau_{4,10} (s^2 - t^2 + u^2) - 2s^2 \tau_{3,9} - 2s^2 \tau_{4,9} + 2s \tau_{3,10} (2t + u)) + \\
& s^2 \tau_{3,9}^2 - 8s^2 \tau_{3,11}^2 + s^2 \tau_{4,9}^2 - 2s^2 \tau_{3,9} \tau_{3,11} + 2s^2 \tau_{3,9} \tau_{4,9} + s^2 \tau_{3,10} \tau_{4,9} - \\
& 2s^2 \tau_{3,11} \tau_{4,9} + s^2 \tau_{3,9} \tau_{4,10} - 3s^2 \tau_{3,11} \tau_{4,10} + 2s^2 \tau_{1,9} (\tau_{3,9} - 3\tau_{3,11} + \tau_{4,9} - 3\tau_{4,11}) + \\
& 2s^2 \tau_{1,10} (\tau_{3,9} - 3\tau_{3,11} + \tau_{4,9} - 3\tau_{4,11}) + 2st \tau_{3,10} \tau_{3,11} + 2t^2 \tau_{3,11}^2 + t^2 \tau_{3,11} \tau_{4,10} + 4u^2 \tau_{3,11}^2 - u^2 \tau_{3,11} \tau_{4,10})
\end{aligned}$$

■  $N_{33}^{(7)}$

$$0$$

■  $N_{33}^{(8)}$

$$0$$
