# Supplementary material for: The Ultraviolet Behavior of N=8 Supergravity at Four Loops
Source: arXiv:0905.2326 ancillary file (2012-01-08)
Supplement: Supplementary file 29 [file SUGRA34.pdf]

## Integral 34: $\mathcal{I}_{34}$

$\mathcal{N} = 8$  four-point four-loop amplitude.

### ■ 2D plot of graph associated with $\mathcal{I}_{34}$

This fixes the labelling associated with the numerator expressions given below.

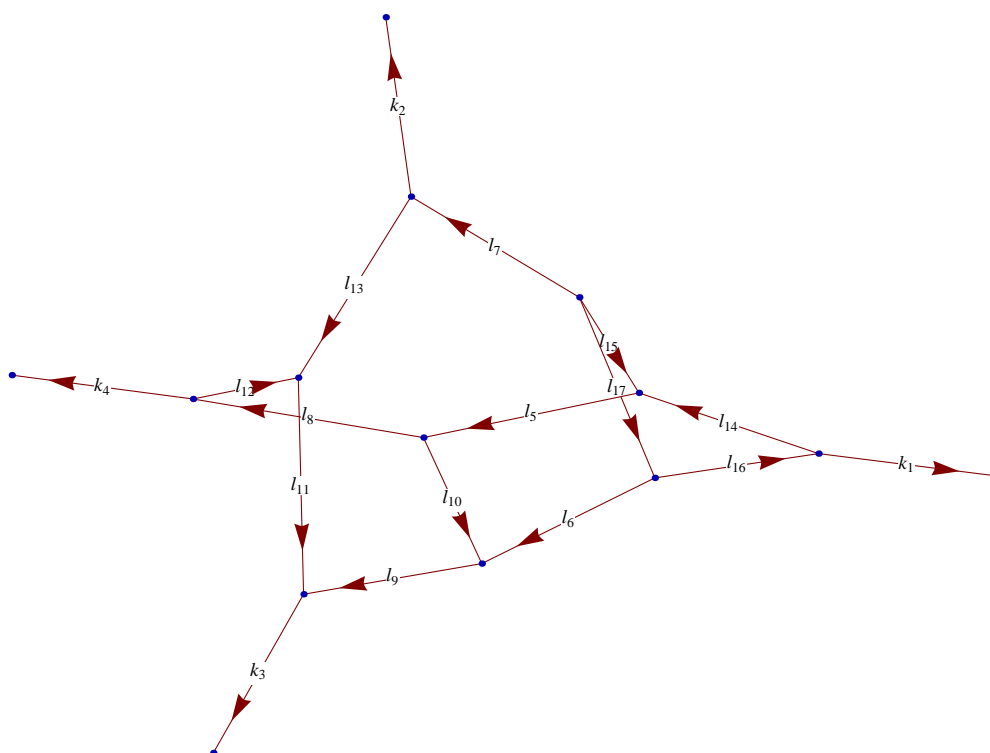

When using MathPlayer, by clicking three times (holding the click on the third click) directly on a vertex, one is able to move that vertex around, and its associated edges follow elastically. This functionality is absent when viewing as a pdf.

*Note: propagators for certain graphs were relabeled in the manuscript due to size constraints. The labels given in `aux/rawData/Neq8FourLoops.m` should be used for verification purposes.*

### ■ 3D plot of graph associated with $\mathcal{I}_{34}$

3D PLOT UNAVAILABLE FOR PDF. Please see .nb version for the 3D figure.

When using MathPlayer, by clicking anywhere in the image and dragging one should be able to rotate this 3D image. By holding (ALT) or (COMMAND) while clicking and moving the mouse up/down one should be able to zoom in/out. This functionality is absent when viewing as a pdf.

### ■ "Vertex Form" of graph associated with $\mathcal{I}_{34}$

This function returns the graph associated with the integral object in a vertex representation. This can be used as a way of specifying the topology of a graph using trivalent (cubic) vertices,  $\text{gVertex}[p_a, p_b, p_c]$ , where  $\{p_a, p_b, p_c\}$  are momenta labeling the propagators (edges) of the graph, and is understood that the edge labelled by  $p_a$  flows into the edge labelled by  $-p_a$ . Additionally, each vertex represents the manifest conservation of ( $D$  - dimensional) momenta :

$$\text{gVertex}[\{p_1, p_2, p_3\}] \iff (p_1 + p_2 + p_3 = 0)$$

$$\{\text{gVertex}(\{k_1, -l_{16}, l_{14}\}), \text{gVertex}(\{k_2, l_{13}, -l_7\}), \text{gVertex}(\{k_3, -l_{11}, -l_9\}), \text{gVertex}(\{k_4, -l_8, l_{12}\}), \text{gVertex}(\{-l_5, l_8, l_{10}\}), \\ \text{gVertex}(\{l_5, -l_{14}, -l_{15}\}), \text{gVertex}(\{-l_6, -l_{10}, l_9\}), \text{gVertex}(\{l_6, -l_{17}, l_{16}\}), \text{gVertex}(\{l_7, l_{15}, l_{17}\}), \text{gVertex}(\{l_{11}, -l_{12}, -l_{13}\})\}$$

### ■ Numerator expression for integral 34:

The following notation is used:  $\tau_{i,j} \equiv \begin{cases} 2 k_i \cdot l_j & \text{if } i \leq 4, j > 4 \\ 2 l_i \cdot l_j & \text{if } i, j > 4 \end{cases}$ .

$$s \equiv 2 k_1 \cdot k_2 = 2 k_3 \cdot k_4$$

We use  $s, t, u$  to represent the traditional Mandelstam variables for massless external four-point momenta:  $t \equiv 2 k_1 \cdot k_4 = 2 k_2 \cdot k_3$ .

$$u \equiv 2 k_1 \cdot k_3 = 2 k_2 \cdot k_4$$

Furthermore we use the shorthand  $(l_i)^2$  to represent the lorentz square:  $(l_i)^2 = l_i \cdot l_i$ .

The total numerator  $\mathcal{N}_{34}$  is given by summing over the following terms, distinguished here by explicit dependence on loop momenta:  $\mathcal{N}_{34} = \sum_{i=0}^8 \mathcal{N}_{34}^{(i)}$ :

$$\blacksquare \mathcal{N}_{34}^{(0)}$$

$$0$$

$$\blacksquare \mathcal{N}_{34}^{(1)}$$

$$0$$

$$\blacksquare \mathcal{N}_{34}^{(2)}$$

$$0$$

$$\blacksquare \mathcal{N}_{34}^{(3)}$$

$$\frac{1}{4} l_7^2 s^2 (\tau_{1,17} (s^2 - 5 t^2 + u^2) + 3 \tau_{2,14} (s^2 + t^2 - u^2) + \tau_{2,15} (4 s^2 - 2 u^2) - 3 s^2 \tau_{2,16} + \\ 4 s^2 \tau_{2,17} + 6 s^2 \tau_{3,15} + 6 s^2 \tau_{4,17} + 3 t^2 \tau_{2,16} - 2 t^2 \tau_{2,17} + 2 \tau_{1,15} (t - u) (t + 2 u) - 3 u^2 \tau_{2,16})$$

■  $N_{34}^{(4)}$ 

$$\begin{aligned}
& \frac{1}{4} \left( (4 l_8^2 l_9^2 + 2 l_7^2 (3 \tau_{11,17} - 3 \tau_{12,15} - 2 l_{10}^2)) t^4 + 2 (\tau_{1,12} (3 \tau_{2,14} - 2 (\tau_{1,15} + \tau_{1,17}))) l_7^2 + \tau_{1,11} (\tau_{1,15} + \tau_{1,17} + 3 \tau_{2,16}) l_7^2 + \right. \\
& \quad (-\tau_{1,15}^2 + (4 \tau_{1,17} - 2 \tau_{2,12} - 5 \tau_{2,14} - \tau_{2,17} + \tau_{3,14} - 5 (\tau_{3,15} + \tau_{4,17})) \tau_{1,15} + 4 \tau_{1,17}^2 + \tau_{2,17}^2 + (\tau_{2,11} + \tau_{2,12}) \tau_{2,17} + \\
& \quad 2 \tau_{2,14} \tau_{3,14} + 2 \tau_{2,17} \tau_{3,14} + 2 \tau_{3,14} \tau_{3,15} + \tau_{2,15} (-2 \tau_{2,16} + \tau_{2,17} + 4 \tau_{3,14} - 2 \tau_{4,16}) - 4 \tau_{2,17} \tau_{4,16} - 2 \tau_{4,16} \tau_{4,17} - \\
& \quad 2 \tau_{2,16} (2 \tau_{2,17} + \tau_{4,17}) + \tau_{1,17} (3 \tau_{2,11} + \tau_{2,12} - 4 \tau_{2,14} + 2 \tau_{2,15} + 3 \tau_{2,17} - \tau_{3,14} - 4 (\tau_{3,15} + \tau_{4,17}))) l_7^2 - \\
& \quad \left. ((-\tau_{1,9} + \tau_{2,8} + \tau_{3,8})^2 + (-\tau_{1,8} + \tau_{2,9} + \tau_{4,9})^2) l_{13}^2 \right) t^3 + 2 (\tau_{1,5} + \tau_{1,6})^2 ((\tau_{1,5} + \tau_{1,6} - \tau_{1,8})^2 + \tau_{1,9}^2) t^2 + \\
& \quad \frac{1}{2} (-s^2 + t^2 + u^2) (2 l_8^2 l_9^2 + l_7^2 (-24 \tau_{11,17} + 24 \tau_{12,15} + 16 l_{10}^2 + l_{13}^2)) t^2 + \\
& \quad (s^2 - t^2 - u^2) \\
& \quad (-4 \tau_{1,15}^2 - (4 \tau_{1,17} + \tau_{2,11} + 7 \tau_{2,12} + 8 \tau_{2,14} + 3 \tau_{2,15} - 6 \tau_{2,16} + 6 \tau_{2,17} - 2 \tau_{3,14} + 14 \tau_{3,15} - \tau_{4,16} + 14 \tau_{4,17}) \tau_{1,15} + \\
& \quad \tau_{1,17}^2 + 2 \tau_{2,14}^2 - \tau_{2,15}^2 + 2 \tau_{2,16}^2 + \tau_{1,12} (9 \tau_{2,14} - 5 (\tau_{1,15} + \tau_{1,17})) - \tau_{2,11} \tau_{2,15} - \tau_{2,12} \tau_{2,15} + \\
& \quad 4 \tau_{2,14} \tau_{2,15} - 4 \tau_{2,15} \tau_{2,16} + \tau_{1,11} (4 (\tau_{1,15} + \tau_{1,17}) + 9 \tau_{2,16}) + 2 \tau_{2,11} \tau_{2,17} + 2 \tau_{2,12} \tau_{2,17} + \\
& \quad 2 \tau_{2,14} \tau_{2,17} - \tau_{2,15} \tau_{2,17} - 8 \tau_{2,16} \tau_{2,17} + 4 \tau_{2,14} \tau_{3,14} + 12 \tau_{2,15} \tau_{3,14} + 6 \tau_{2,17} \tau_{3,14} + 2 \tau_{2,14} \tau_{3,15} + \\
& \quad 6 \tau_{3,14} \tau_{3,15} - 6 \tau_{2,15} \tau_{4,16} + 2 \tau_{2,16} \tau_{4,16} - 12 \tau_{2,17} \tau_{4,16} - 4 \tau_{2,16} \tau_{4,17} - 6 \tau_{4,16} \tau_{4,17} - \\
& \quad \tau_{1,17} (-8 \tau_{2,11} - 2 \tau_{2,12} + 10 \tau_{2,14} + 3 \tau_{2,15} - 3 \tau_{2,16} + 2 \tau_{3,14} + 13 \tau_{3,15} + \tau_{4,16} + 13 \tau_{4,17})) l_7^2 t + \\
& \quad 2 u (s^2 - t^2 - u^2) (l_7^2 (9 \tau_{11,17} - 9 \tau_{12,15} - 6 l_{10}^2 - l_{13}^2) - l_8^2 l_9^2) t + 2 u^2 (\tau_{1,5} + \tau_{1,6})^2 (\tau_{1,8}^2 + (\tau_{1,5} + \tau_{1,6} - \tau_{1,9})^2) - \\
& \quad 2 (s^2 - t^2 - u^2) (\tau_{1,5} + \tau_{1,6})^2 (-\tau_{1,9}^2 + (\tau_{1,5} + \tau_{1,6}) \tau_{1,9} + (\tau_{1,5} + \tau_{1,6} - \tau_{1,8}) \tau_{1,8}) + \\
& \quad u (s^2 - t^2 - u^2) \\
& \quad (\tau_{1,15}^2 - (4 \tau_{1,17} + 2 \tau_{2,11} + 8 \tau_{2,12} + 3 \tau_{2,14} - 10 \tau_{2,16} + 3 \tau_{2,17} - \tau_{3,14} + 13 \tau_{3,15} - 2 \tau_{4,16} + 13 \tau_{4,17}) \tau_{1,15} - 4 \tau_{1,17}^2 + \\
& \quad 2 \tau_{2,14}^2 + 2 \tau_{2,16}^2 - \tau_{2,17}^2 + \tau_{1,12} (9 \tau_{2,14} - 4 (\tau_{1,15} + \tau_{1,17})) - 2 \tau_{2,11} \tau_{2,15} - 2 \tau_{2,12} \tau_{2,15} + 8 \tau_{2,14} \tau_{2,15} - 2 \tau_{2,15} \tau_{2,16} + \\
& \quad \tau_{1,11} (5 (\tau_{1,15} + \tau_{1,17}) + 9 \tau_{2,16}) + \tau_{2,11} \tau_{2,17} + \tau_{2,12} \tau_{2,17} + 4 \tau_{2,14} \tau_{2,17} - \tau_{2,15} \tau_{2,17} - 4 \tau_{2,16} \tau_{2,17} + 2 \tau_{2,14} \tau_{3,14} + \\
& \quad 12 \tau_{2,15} \tau_{3,14} + 6 \tau_{2,17} \tau_{3,14} + 4 \tau_{2,14} \tau_{3,15} + 6 \tau_{3,14} \tau_{3,15} - 6 \tau_{2,15} \tau_{4,16} + 4 \tau_{2,16} \tau_{4,16} - 12 \tau_{2,17} \tau_{4,16} - 2 \tau_{2,16} \tau_{4,17} - \\
& \quad 6 \tau_{4,16} \tau_{4,17} - \tau_{1,17} (-7 \tau_{2,11} - \tau_{2,12} + 6 \tau_{2,14} + 6 \tau_{2,15} - 8 \tau_{2,16} + 3 \tau_{2,17} + \tau_{3,14} + 2 (7 \tau_{3,15} + \tau_{4,16} + 7 \tau_{4,17}))) \\
& \quad l_7^2 + u^4 (4 l_8^2 l_9^2 + 2 l_7^2 (3 \tau_{11,17} - 3 \tau_{12,15} - 2 l_{10}^2)) + \\
& \quad 2 u^3 ((4 \tau_{1,15}^2 + (4 \tau_{1,17} - \tau_{2,11} - 3 \tau_{2,12} + 3 \tau_{2,15} + 4 \tau_{2,16} + 2 \tau_{2,17} - 4 \tau_{3,15} + \tau_{4,16} - 4 \tau_{4,17}) \tau_{1,15} - \tau_{1,17}^2 + \tau_{2,15}^2 - \\
& \quad \tau_{1,12} (\tau_{1,15} + \tau_{1,17} - 3 \tau_{2,14}) - \tau_{2,11} \tau_{2,15} - \tau_{2,12} \tau_{2,15} + 4 \tau_{2,14} \tau_{2,15} + \tau_{1,11} (2 (\tau_{1,15} + \tau_{1,17}) + 3 \tau_{2,16}) + \\
& \quad 2 \tau_{2,14} \tau_{2,17} + \tau_{2,15} \tau_{2,17} + 4 \tau_{2,15} \tau_{3,14} + 2 \tau_{2,17} \tau_{3,14} + 2 \tau_{2,14} \tau_{3,15} + 2 \tau_{3,14} \tau_{3,15} - 2 \tau_{2,15} \tau_{4,16} + \\
& \quad 2 \tau_{2,16} \tau_{4,16} - 4 \tau_{2,17} \tau_{4,16} + \tau_{1,17} (2 \tau_{2,11} - \tau_{2,15} + 5 \tau_{2,16} - 5 \tau_{3,15} - \tau_{4,16} - 5 \tau_{4,17}) - 2 \tau_{4,16} \tau_{4,17})) l_7^2 - \\
& \quad ((-\tau_{1,9} + \tau_{2,8} + \tau_{3,8})^2 + (-\tau_{1,8} + \tau_{2,9} + \tau_{4,9})^2) l_{13}^2) + \frac{1}{2} u^2 (-s^2 + t^2 + u^2) \\
& \quad \left. (2 l_8^2 l_9^2 + l_7^2 (-24 \tau_{11,17} + 24 \tau_{12,15} + 16 l_{10}^2 + l_{13}^2)) \right)
\end{aligned}$$

■  $N_{34}^{(5)}$ 

$$\begin{aligned}
& \frac{1}{4} \left( (2(\tau_{1,5} + 5\tau_{1,10} + \tau_{1,11} + 4\tau_{1,12} + \tau_{3,6} + \tau_{3,12} + \tau_{4,5}) l_8^2 l_9^2 + \right. \\
& \quad l_7^2 (-2(2\tau_{1,15} + \tau_{1,17} + 2(\tau_{2,16} + \tau_{4,16})) \tau_{11,17} + 2(2\tau_{1,15} + \tau_{1,17} - 2\tau_{3,14}) \tau_{12,15} - \\
& \quad (4\tau_{2,11} - 2\tau_{2,15} + 2\tau_{2,17} - 4\tau_{3,10} + 2\tau_{3,15} - 2\tau_{3,17} + 6\tau_{4,10} + 3\tau_{4,11} - 7\tau_{4,15} + 7\tau_{4,17}) l_{13}^2) t^3 + \\
& \quad ((-4\tau_{1,17}^3 + 2(-\tau_{2,11} - \tau_{2,12} + \tau_{2,14} - 2\tau_{2,15} - 2\tau_{2,17} + \tau_{3,14} + \tau_{3,15} + \tau_{4,17}) \tau_{1,17}^2 - \\
& \quad 2(\tau_{2,15}^2 + (\tau_{2,16} + 2\tau_{2,17} + \tau_{3,14} + \tau_{4,16}) \tau_{2,15} + \tau_{2,17}^2 + \tau_{2,12}(\tau_{2,15} + \tau_{2,17}) + 2\tau_{2,14} \tau_{3,14} + \\
& \quad 2\tau_{3,14} \tau_{3,15} + \tau_{2,11}(\tau_{2,15} + 2\tau_{2,16} + \tau_{2,17} + 2\tau_{4,16}) - 2\tau_{2,16} \tau_{4,17} - 2\tau_{4,16} \tau_{4,17}) \tau_{1,17} + \\
& \quad 2\tau_{1,12}(2\tau_{1,15}^2 + (4\tau_{1,17} + \tau_{2,12} - 2\tau_{2,14} - \tau_{3,14}) \tau_{1,15} + 2\tau_{1,17}^2 + \tau_{1,17}(\tau_{2,12} - \tau_{2,14} - \tau_{3,14}) + 2\tau_{2,14} \tau_{3,14}) + \\
& \quad 2\tau_{1,11}(\tau_{1,17}^2 + (\tau_{2,11} + \tau_{2,15} - 2\tau_{2,16} + \tau_{2,17} - \tau_{4,16}) \tau_{1,17} + \tau_{1,15}(\tau_{1,17} + \tau_{2,11} + \tau_{2,15} - 3\tau_{2,16} + \tau_{2,17} - \tau_{4,16}) - \\
& \quad 2\tau_{2,16}(\tau_{2,16} + \tau_{4,16})) - (\tau_{2,15} + \tau_{2,17})(\tau_{2,12}^2 + (\tau_{2,11} + \tau_{2,15} + \tau_{2,17})^2 - 3(\tau_{3,14}^2 + (\tau_{2,16} + \tau_{4,16})^2)) - \\
& \quad 2\tau_{1,15}(5\tau_{1,17}^2 + (2\tau_{2,11} + \tau_{2,12} - 3\tau_{2,14} + 4\tau_{2,15} + 3\tau_{2,17} - 3\tau_{3,15} - 3\tau_{4,17}) \tau_{1,17} + \tau_{2,15}^2 + \\
& \quad \tau_{2,17}^2 - 3\tau_{2,16} \tau_{2,17} + \tau_{2,11}(\tau_{2,15} + \tau_{2,17}) + 2\tau_{2,14} \tau_{3,14} + \tau_{2,17} \tau_{3,14} + \tau_{2,12}(\tau_{2,15} + \tau_{2,17} + 2\tau_{3,14}) + \\
& \quad 2\tau_{3,14} \tau_{3,15} - 3\tau_{2,17} \tau_{4,16} - \tau_{2,15}(\tau_{2,16} - 2\tau_{2,17} - \tau_{3,14} + \tau_{4,16}) - 2\tau_{2,16} \tau_{4,17} - 2\tau_{4,16} \tau_{4,17}) + \\
& \quad 2\tau_{1,15}^2(-3\tau_{1,17} + \tau_{2,12} + 2\tau_{2,14} - 2\tau_{2,15} - \tau_{3,14} + 2(\tau_{3,15} + \tau_{4,17}))) l_7^2 + \\
& \quad 2(2\tau_{1,9}^3 + (-4\tau_{2,8} + \tau_{2,9} - 4\tau_{3,8}) \tau_{1,9}^2 + 2(\tau_{2,8} + \tau_{3,8})(\tau_{2,8} - \tau_{2,9} + \tau_{3,8}) \tau_{1,9} - 2\tau_{4,9}^3 - 5\tau_{2,9} \tau_{4,9}^2 + \\
& \quad \tau_{2,9}((\tau_{2,8} + \tau_{3,8})^2 - \tau_{2,9}^2) - 4\tau_{2,9}^2 \tau_{4,9} - \tau_{1,8}^2(\tau_{2,9} + 2\tau_{4,9}) + 2\tau_{1,8}(\tau_{2,9} + \tau_{4,9})(\tau_{2,9} + 2\tau_{4,9})) l_{13}^2) t^2 + \\
& \quad (s^2 - t^2 - u^2) \left( (4\tau_{1,5} - \tau_{1,6} + \tau_{1,10} + \tau_{1,12} + 4\tau_{3,6} + \tau_{3,10} - \tau_{3,11} + 4\tau_{3,12} + 4\tau_{4,5} - \tau_{4,10} - 3\tau_{4,11} + \tau_{4,12}) l_8^2 l_9^2 + \right. \\
& \quad l_7^2 (-5\tau_{1,15} + 4(\tau_{1,17} + \tau_{2,16}) + 6\tau_{4,16}) \tau_{11,17} + (5\tau_{1,15} + 4\tau_{1,17} - 2(\tau_{2,14} + 3\tau_{3,14})) \tau_{12,15} + \\
& \quad (-3\tau_{2,11} + \tau_{2,12} + \tau_{2,15} - \tau_{2,17} + 8\tau_{3,10} + \tau_{3,12} - 7\tau_{3,15} + 7\tau_{3,17} - 6\tau_{4,10} - 2\tau_{4,11} + 8\tau_{4,15} - 8\tau_{4,17}) l_{13}^2) t - \\
& \quad (s^2 - t^2 - u^2) \left( -2\tau_{1,15}^3 - (8\tau_{1,17} + \tau_{2,11} + 2\tau_{2,12} + 2\tau_{2,15} - 3\tau_{2,16} + 3\tau_{2,17} - \tau_{3,14} + 3\tau_{3,15} - \tau_{4,16} + 3\tau_{4,17}) \tau_{1,15}^2 + \right. \\
& \quad (-8\tau_{1,17}^2 + (\tau_{2,11} - \tau_{2,12} - 3\tau_{2,14} - 7\tau_{2,15} + 3\tau_{2,16} - 7\tau_{2,17} - 6\tau_{3,15} - 6\tau_{4,17}) \tau_{1,17} + 2\tau_{2,14}^2 - 2\tau_{2,15}^2 + 2\tau_{2,16}^2 - \\
& \quad 2\tau_{2,17}^2 - \tau_{2,16} \tau_{2,17} + 2\tau_{2,12}(\tau_{2,14} + 2\tau_{3,14}) + 4\tau_{3,14} \tau_{3,15} + \tau_{2,14}(\tau_{2,15} + \tau_{2,17} + 2(\tau_{3,14} + \tau_{3,15})) + \\
& \quad \tau_{2,15}(-4\tau_{2,17} + \tau_{3,14} - \tau_{4,16}) + 2\tau_{2,16} \tau_{4,16} - 4\tau_{2,17} \tau_{4,16} - 2\tau_{2,16} \tau_{4,17} - 4\tau_{4,16} \tau_{4,17}) \tau_{1,15} - \\
& \quad 2\tau_{1,17}^3 + \tau_{1,12}(-\tau_{1,15}^2 + (-3\tau_{1,17} - 2\tau_{2,12} + 4\tau_{2,14} + \tau_{2,15} + \tau_{2,17} + 2\tau_{3,14}) \tau_{1,15} - 2\tau_{1,17}^2 - \\
& \quad 2\tau_{2,14}(\tau_{2,14} + 2\tau_{3,14}) + \tau_{1,17}(-2\tau_{2,12} + 4\tau_{2,14} + \tau_{2,15} + \tau_{2,17} + 2\tau_{3,14})) + \\
& \quad \tau_{1,11}(2\tau_{1,15}^2 + (3\tau_{1,17} - 2\tau_{2,11} - \tau_{2,15} + 4\tau_{2,16} - \tau_{2,17} + 2\tau_{4,16}) \tau_{1,15} + \tau_{1,17}^2 - \\
& \quad \tau_{1,17}(2\tau_{2,11} + \tau_{2,15} - 4\tau_{2,16} + \tau_{2,17} - 2\tau_{4,16}) + 2\tau_{2,16}(\tau_{2,16} + 2\tau_{4,16})) + (\tau_{2,15} + \tau_{2,17}) \\
& \quad (\tau_{2,11}^2 + (\tau_{2,15} + \tau_{2,17}) \tau_{2,11} + \tau_{2,12}^2 - \tau_{2,12}(\tau_{2,15} + \tau_{2,17}) - 3(\tau_{3,14}(\tau_{2,14} + \tau_{3,14}) + \tau_{4,16}(\tau_{2,16} + \tau_{4,16}))) - \\
& \quad \tau_{1,17}^2(-2\tau_{2,11} - \tau_{2,12} + 3\tau_{2,14} + 3\tau_{2,15} + 2\tau_{2,17} + \tau_{3,14} + 3\tau_{3,15} + \tau_{4,16} + 3\tau_{4,17}) + \\
& \quad \tau_{1,17}(2\tau_{2,14}^2 + (\tau_{2,15} + 2(\tau_{3,14} + \tau_{3,15})) \tau_{2,14} - 2\tau_{2,15}^2 + 2\tau_{2,16}^2 - 2\tau_{2,17}^2 - \tau_{2,15}(\tau_{2,16} + 4\tau_{2,17} - 4\tau_{3,14}) + \\
& \quad 4\tau_{3,14} \tau_{3,15} + \tau_{2,17}(\tau_{3,14} - \tau_{4,16}) + 2\tau_{2,11}(\tau_{2,16} + 2\tau_{4,16}) - 4\tau_{4,16} \tau_{4,17} - \tau_{2,16}(\tau_{2,17} - 2\tau_{4,16} + 2\tau_{4,17}))) l_7^2 -
\end{aligned}$$

$$\begin{aligned}
& u^2 \left( (4 \tau_{1,15}^3 + 2 (5 \tau_{1,17} - \tau_{2,11} - \tau_{2,12} + 2 \tau_{2,15} + \tau_{2,16} + 2 \tau_{2,17} - \tau_{3,15} + \tau_{4,16} - \tau_{4,17}) \tau_{1,15}^2 + \right. \\
& \quad 2 (3 \tau_{1,17}^2 - (\tau_{2,11} + 2 \tau_{2,12} - 3 \tau_{2,15} - 3 \tau_{2,16} - 4 \tau_{2,17} + 3 (\tau_{3,15} + \tau_{4,17})) \tau_{1,17} + \tau_{2,15}^2 + \\
& \quad \tau_{2,17}^2 + 2 \tau_{2,15} \tau_{2,17} - \tau_{2,11} (\tau_{2,15} + \tau_{2,17}) + \tau_{2,12} (2 \tau_{2,14} - \tau_{2,15} - \tau_{2,17} + 2 \tau_{3,14}) - \\
& \quad \tau_{2,14} (\tau_{2,17} - 2 \tau_{3,15}) + 2 \tau_{3,14} \tau_{3,15} + 2 \tau_{2,16} \tau_{4,16} - \tau_{2,17} (\tau_{3,14} + \tau_{4,16}) - 2 \tau_{4,16} \tau_{4,17}) \tau_{1,15} + \\
& \quad 2 \tau_{1,12} (\tau_{1,15}^2 + (\tau_{1,17} - \tau_{2,12} + 2 \tau_{2,14} + \tau_{2,15} + \tau_{2,17} + \tau_{3,14}) \tau_{1,15} - 2 \tau_{2,14} (\tau_{2,14} + \tau_{3,14}) + \\
& \quad \tau_{1,17} (-\tau_{2,12} + 3 \tau_{2,14} + \tau_{2,15} + \tau_{2,17} + \tau_{3,14})) + \\
& \quad (\tau_{2,15} + \tau_{2,17}) (\tau_{2,11}^2 + (-\tau_{2,12} + \tau_{2,15} + \tau_{2,17})^2 - 3 (\tau_{2,14} + \tau_{3,14})^2 - 3 \tau_{4,16}^2) + \\
& \quad 2 \tau_{1,11} (2 \tau_{1,15}^2 + (4 \tau_{1,17} - \tau_{2,11} + \tau_{2,16} + \tau_{4,16}) \tau_{1,15} + 2 \tau_{1,17}^2 + 2 \tau_{2,16} \tau_{4,16} + \tau_{1,17} (-\tau_{2,11} + 2 \tau_{2,16} + \tau_{4,16})) + \\
& \quad 2 \tau_{1,17}^2 (\tau_{2,11} + 2 \tau_{2,16} + 2 \tau_{2,17} - 2 \tau_{3,15} - \tau_{4,16} - 2 \tau_{4,17}) + \\
& \quad 2 \tau_{1,17} (\tau_{2,15}^2 + (2 \tau_{2,17} + 3 \tau_{3,14} - \tau_{4,16}) \tau_{2,15} + \tau_{2,17}^2 - \tau_{2,12} (\tau_{2,15} + \tau_{2,17}) + \tau_{2,17} \tau_{3,14} + 2 \tau_{3,14} \tau_{3,15} + \\
& \quad \tau_{2,14} (3 \tau_{2,15} + \tau_{2,17} + 2 \tau_{3,15}) - \tau_{2,11} (\tau_{2,15} + \tau_{2,17} - 2 \tau_{4,16}) + 2 \tau_{2,16} \tau_{4,16} - \tau_{2,17} \tau_{4,16} - 2 \tau_{4,16} \tau_{4,17})) l_7^2 - \\
& \quad 2 (2 \tau_{1,8}^3 + (\tau_{2,8} - 4 (\tau_{2,9} + \tau_{4,9})) \tau_{1,8}^2 - 2 (\tau_{2,8} - \tau_{2,9} - \tau_{4,9}) (\tau_{2,9} + \tau_{4,9}) \tau_{1,8} - \tau_{2,8}^3 - 2 \tau_{3,8}^3 - \\
& \quad 4 \tau_{2,8}^2 \tau_{3,8} - \tau_{1,9}^2 (\tau_{2,8} + 2 \tau_{3,8}) + 2 \tau_{1,9} (\tau_{2,8} + \tau_{3,8}) (\tau_{2,8} + 2 \tau_{3,8}) + \tau_{2,8} ((\tau_{2,9} + \tau_{4,9})^2 - 5 \tau_{3,8}^2)) l_{13}^2) + \\
& \quad u^3 (2 (\tau_{1,6} - 5 \tau_{1,10} - 4 \tau_{1,11} - \tau_{1,12} + \tau_{3,6} + \tau_{4,5} - \tau_{4,11}) l_8^2 l_9^2 + \\
& \quad l_7^2 (-2 (\tau_{1,15} + 2 (\tau_{1,17} + \tau_{4,16})) \tau_{11,17} + 2 (\tau_{1,15} + 2 \tau_{1,17} - 2 \tau_{2,14} - 2 \tau_{3,14}) \tau_{12,15} + \\
& \quad (4 \tau_{2,12} - 2 \tau_{2,15} + 2 \tau_{2,17} + 6 \tau_{3,10} + 3 \tau_{3,12} - 7 \tau_{3,15} + 7 \tau_{3,17} - 4 \tau_{4,10} + 2 \tau_{4,15} - 2 \tau_{4,17}) l_{13}^2)) + \\
& \quad u (s^2 - t^2 - u^2) (l_7^2 (-4 \tau_{1,15} + 5 \tau_{1,17} + 2 \tau_{2,16} + 6 \tau_{4,16}) \tau_{11,17} + (4 \tau_{1,15} + 5 \tau_{1,17} - 4 \tau_{2,14} - 6 \tau_{3,14}) \tau_{12,15} - \\
& \quad (\tau_{2,11} - 3 \tau_{2,12} + \tau_{2,15} - \tau_{2,17} - 6 \tau_{3,10} - 2 \tau_{3,12} + 8 \tau_{3,15} - 8 \tau_{3,17} + 8 \tau_{4,10} + \tau_{4,11} - 7 \tau_{4,15} + 7 \tau_{4,17}) l_{13}^2) - \\
& \quad (\tau_{1,5} - 4 \tau_{1,6} + \tau_{1,10} + \tau_{1,11} - 4 \tau_{3,6} - \tau_{3,10} + \tau_{3,11} - 3 \tau_{3,12} - 4 \tau_{4,5} + \tau_{4,10} + 4 \tau_{4,11} - \tau_{4,12}) l_8^2 l_9^2) \Big)
\end{aligned}$$

■  $N_{34}^{(6)}$

$$\begin{aligned}
& \frac{1}{4} \left( 16 l_7^2 l_{14}^2 l_{16}^2 s^3 - (3 s^2 - 5 t^2 + u^2) \tau_{1,5}^2 l_8^2 l_9^2 - (3 s^2 + t^2 - 5 u^2) \tau_{1,6}^2 l_8^2 l_9^2 + \right. \\
& \quad 2 \tau_{1,5} (2 u (3 t + u) \tau_{1,10} + 2 u (3 t + u) \tau_{1,11} + s (t \tau_{3,10} - u \tau_{3,11} + (2 t + 3 u) \tau_{4,5} - (t + 3 u) (\tau_{4,10} + \tau_{4,11}))) l_8^2 l_9^2 + \\
& \quad u^2 (6 \tau_{1,10}^2 + 2 (4 \tau_{1,11} + 2 \tau_{1,12} + \tau_{3,6} + 2 \tau_{3,10} + 3 \tau_{3,12} + \tau_{4,10} + \tau_{4,11} + \tau_{4,12}) \tau_{1,10} + 4 \tau_{1,11}^2 + 2 \tau_{1,12}^2 - \\
& \quad 2 \tau_{3,6}^2 - 2 \tau_{4,5}^2 - 2 \tau_{3,6} \tau_{3,10} - 2 \tau_{3,6} \tau_{3,12} - \tau_{3,10} \tau_{4,5} + (\tau_{3,6} + 2 \tau_{3,10} + \tau_{3,11} + 2 (\tau_{3,12} + \tau_{4,5})) \tau_{4,10} + \\
& \quad 2 (\tau_{1,11} + \tau_{3,10} + \tau_{3,11} + \tau_{4,5}) \tau_{4,11} + (\tau_{3,10} + 2 \tau_{3,12}) \tau_{4,12} + 2 \tau_{1,12} (\tau_{3,6} + 2 \tau_{3,10} + 3 \tau_{3,12} + \tau_{4,10} + \tau_{4,12})) l_8^2 l_9^2 + \\
& \quad (s^2 - t^2 - u^2) (2 \tau_{1,10}^2 + (2 \tau_{1,11} + 2 \tau_{1,12} + \tau_{3,6} + 3 \tau_{3,10} + \tau_{3,11} + 4 \tau_{3,12} - \tau_{4,5} + 3 \tau_{4,10} + 4 \tau_{4,11} + \tau_{4,12}) \tau_{1,10} + \\
& \quad \tau_{1,11}^2 + \tau_{1,12}^2 - 2 \tau_{3,6}^2 - 2 \tau_{4,5}^2 - \tau_{3,10} \tau_{4,5} + 2 \tau_{3,10} \tau_{4,10} + \tau_{3,11} \tau_{4,10} + 2 \tau_{3,12} \tau_{4,10} + 2 \tau_{4,5} \tau_{4,10} + \\
& \quad \tau_{3,6} (\tau_{4,10} - 2 (\tau_{3,10} + \tau_{3,12})) + 2 \tau_{3,10} \tau_{4,11} + 2 \tau_{3,11} \tau_{4,11} + 2 \tau_{4,5} \tau_{4,11} + \tau_{1,11} (\tau_{3,10} + \tau_{3,11} - \tau_{4,5} + 2 \tau_{4,10} + 4 \tau_{4,11}) + \\
& \quad \tau_{3,10} \tau_{4,12} + 2 \tau_{3,12} \tau_{4,12} + \tau_{1,12} (\tau_{3,6} + 2 \tau_{3,10} + 4 \tau_{3,12} + \tau_{4,10} + \tau_{4,12})) l_8^2 l_9^2 + \\
& \quad t^2 (6 \tau_{1,10}^2 + 2 (2 \tau_{1,11} + 4 \tau_{1,12} + \tau_{3,10} + \tau_{3,11} + \tau_{3,12} - \tau_{4,5} + 2 \tau_{4,10} + 3 \tau_{4,11}) \tau_{1,10} + 2 \tau_{1,11}^2 - 2 \tau_{3,6}^2 - 2 \tau_{4,5}^2 + \\
& \quad 2 \tau_{1,12} (2 \tau_{1,12} + \tau_{3,12}) + \tau_{3,11} \tau_{4,10} + 2 \tau_{3,12} \tau_{4,10} + 2 \tau_{4,5} \tau_{4,10} + \tau_{3,6} (\tau_{4,10} - 2 (\tau_{3,10} + \tau_{3,12})) + 2 \tau_{3,11} \tau_{4,11} + 2 \tau_{4,5} \\
& \quad \tau_{4,11} + 2 \tau_{1,11} (\tau_{3,10} + \tau_{3,11} - \tau_{4,5} + 2 \tau_{4,10} + 3 \tau_{4,11}) + 2 \tau_{3,12} \tau_{4,12} + \tau_{3,10} (-\tau_{4,5} + 2 (\tau_{4,10} + \tau_{4,11}) + \tau_{4,12})) l_8^2 l_9^2 - \\
& \quad 2 \tau_{1,6} (2 t (t + 3 u) \tau_{1,10} + 2 t (t + 3 u) \tau_{1,12} - s ((3 t + 2 u) \tau_{3,6} + (3 t + u) \tau_{3,10} + (3 t + u) \tau_{3,12} - u \tau_{4,10} + t \tau_{4,12})) l_8^2 l_9^2 + \\
& \quad \left. 5 t^3 l_8^2 l_9^2 l_{13}^2 + 5 u^3 l_8^2 l_9^2 l_{13}^2 - \frac{67}{2} t (-s^2 + t^2 + u^2) l_8^2 l_9^2 l_{13}^2 - \frac{67}{2} u (-s^2 + t^2 + u^2) l_8^2 l_9^2 l_{13}^2 \right)
\end{aligned}$$

■  $N_{34}^{(7)}$ 

$$\frac{1}{4} l_8^2 l_9^2 l_{13}^2$$

$$\begin{aligned} & (\tau_{1,5} (27 s^2 - 12 t^2 + 8 u^2) + \tau_{1,6} (27 s^2 + 8 t^2 - 12 u^2) + (-27 \tau_{1,11} + 27 \tau_{1,12} + 9 \tau_{3,5} + 20 \tau_{3,6} + 19 \tau_{3,10} - 20 \tau_{3,11} + 9 \tau_{3,12} + \\ & \quad 20 \tau_{4,5} + 9 \tau_{4,6} - 19 \tau_{4,10} - 9 \tau_{4,11} + 20 \tau_{4,12}) (s^2 - t^2 - u^2) + \\ & \quad t^2 (-4 \tau_{1,10} - 35 \tau_{1,11} + 15 \tau_{1,12} + 2 (4 \tau_{3,5} + 7 \tau_{3,6} + 18 \tau_{3,10} - 7 \tau_{3,11} + 4 \tau_{3,12} + 11 \tau_{4,5} - \tau_{4,6} - 3 \tau_{4,10} + \tau_{4,11} + 11 \tau_{4,12})) + \\ & \quad u^2 (4 \tau_{1,10} - 15 \tau_{1,11} + 35 \tau_{1,12} - 2 (\tau_{3,5} - 11 \tau_{3,6} - 3 \tau_{3,10} + 11 \tau_{3,11} + \tau_{3,12} - 7 \tau_{4,5} - 4 \tau_{4,6} + 18 \tau_{4,10} + 4 \tau_{4,11} - 7 \tau_{4,12}))) \end{aligned}$$

■  $N_{34}^{(8)}$ 

$$0$$
