# Supplementary material for: The Ultraviolet Behavior of N=8 Supergravity at Four Loops
Source: arXiv:0905.2326 ancillary file (2012-01-08)
Supplement: Supplementary file 30 [file SUGRA35.pdf]

## Integral 35: $\mathcal{I}_{35}$

$\mathcal{N} = 8$  four-point four-loop amplitude.

### ■ 2D plot of graph associated with $\mathcal{I}_{35}$

This fixes the labelling associated with the numerator expressions given below.

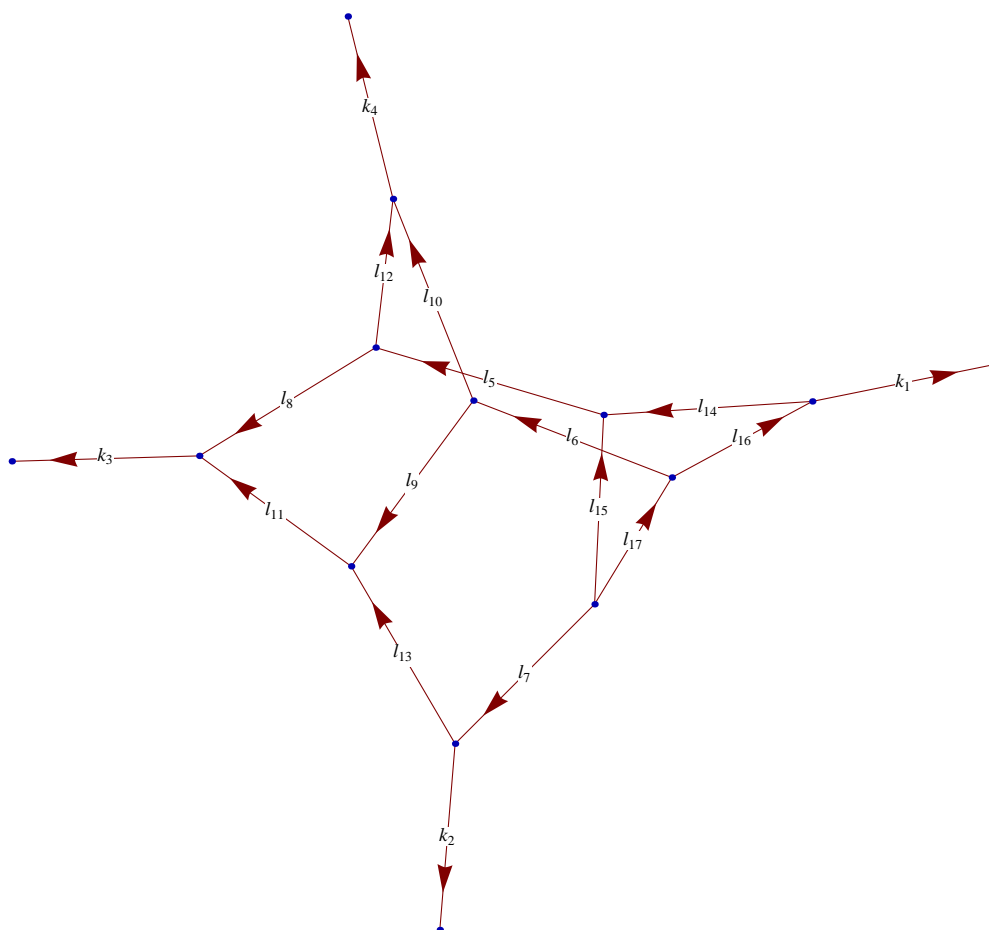

When using MathPlayer, by clicking three times (holding the click on the third click) directly on a vertex, one is able to move that vertex around, and its associated edges follow elastically. This functionality is absent when viewing as a pdf.

*Note: propagators for certain graphs were relabeled in the manuscript due to size constraints. The labels given in aux/rawData/Neq8FourLoops.m should be used for verification purposes.*

### ■ 3D plot of graph associated with $\mathcal{I}_{35}$

3D PLOT UNAVAILABLE FOR PDF. Please see .nb version for the 3D figure.

When using MathPlayer, by clicking anywhere in the image and dragging one should be able to rotate this 3D image. By holding (ALT) or (COMMAND) while clicking and moving the mouse up/down one should be able to zoom in/out. This functionality is absent when viewing as a pdf.

### ■ "Vertex Form" of graph associated with $\mathcal{I}_{35}$

This function returns the graph associated with the integral object in a vertex representation. This can be used as a way of specifying the topology of a graph using trivalent (cubic) vertices,  $\text{gVertex}[p_a, p_b, p_c]$ , where  $\{p_a, p_b, p_c\}$  are momenta labeling the propagators (edges) of the graph, and is understood that the edge labelled by  $p_a$  flows into the edge labelled by  $-p_a$ . Additionally, each vertex represents the manifest conservation of ( $D$  - dimensional) momenta :

$$\text{gVertex}[\{p_1, p_2, p_3\}] \iff (p_1 + p_2 + p_3 = 0)$$

$$\{\text{gVertex}(\{k_1, -l_{16}, l_{14}\}), \text{gVertex}(\{k_2, l_{13}, -l_7\}), \text{gVertex}(\{k_3, -l_8, -l_{11}\}), \text{gVertex}(\{k_4, -l_{10}, -l_{12}\}), \text{gVertex}(\{-l_5, l_8, l_{12}\}),$$

$$\text{gVertex}(\{l_5, -l_{14}, -l_{15}\}), \text{gVertex}(\{-l_6, l_{10}, l_9\}), \text{gVertex}(\{l_6, -l_{17}, l_{16}\}), \text{gVertex}(\{l_7, l_{15}, l_{17}\}), \text{gVertex}(\{-l_9, l_{11}, -l_{13}\})\}$$

### ■ Numerator expression for integral 35:

The following notation is used:  $\tau_{i,j} \equiv \begin{cases} 2 k_i \cdot l_j & \text{if } i \leq 4, j > 4 \\ 2 l_i \cdot l_j & \text{if } i, j > 4 \end{cases}$ .

$$s \equiv 2 k_1 \cdot k_2 = 2 k_3 \cdot k_4$$

We use  $s, t, u$  to represent the traditional Mandelstam variables for massless external four-point momenta:  $t \equiv 2 k_1 \cdot k_4 = 2 k_2 \cdot k_3$ .

$$u \equiv 2 k_1 \cdot k_3 = 2 k_2 \cdot k_4$$

Furthermore we use the shorthand  $(l_i)^2$  to represent the lorentz square:  $(l_i)^2 = l_i \cdot l_i$ .

The total numerator  $\mathcal{N}_{35}$  is given by summing over the following terms, distinguished here by explicit dependence on loop momenta:  $\mathcal{N}_{35} = \sum_{i=0}^8 \mathcal{N}_{35}^{(i)}$ :

#### ■ $\mathcal{N}_{35}^{(0)}$

$$0$$

#### ■ $\mathcal{N}_{35}^{(1)}$

$$0$$

#### ■ $\mathcal{N}_{35}^{(2)}$

$$s^4 \tau_{1,5}^2 + \frac{1}{2} t^2 (-2 l_8^2 s^3 + 2 l_5^2 s (t^2 - 2 s^2) - l_{10}^2 t (s^2 - 2 u^2))$$

■  $N_{35}^{(3)}$

$$\begin{aligned}
& \frac{1}{2} \left( (-4\tau_{1,11} + 2\tau_{1,13} + \tau_{2,14} - 2\tau_{3,6} + \tau_{3,14})l_5^2 - (2\tau_{1,15} + \tau_{2,15} - 2\tau_{3,16})l_7^2 - \right. \\
& \quad 2(-2\tau_{1,9} + 3\tau_{1,10} + 4\tau_{1,11} + \tau_{2,10} - 2\tau_{3,9} + \tau_{3,11})l_8^2 + (-3\tau_{1,9} + 5\tau_{1,12} + \tau_{2,5} - 2\tau_{2,12} - \tau_{3,9} + 5\tau_{3,12})l_{10}^2 \Big) t^4 - \\
& \quad (t^2 - 2s^2)\tau_{1,6}l_5^2t^2 + (s^2 - t^2 - u^2)((-3\tau_{1,13} + \tau_{2,11} - 2\tau_{2,14} + 4\tau_{3,6} - \tau_{3,13})l_5^2 - \\
& \quad (\tau_{1,15} + \tau_{2,15} - \tau_{2,16} - 3\tau_{3,16})l_7^2 + 2(2\tau_{1,9} - 4\tau_{1,10} + \tau_{2,9} - \tau_{2,10} + 3\tau_{3,9} - \tau_{3,11})l_8^2 - \\
& \quad \tau_{1,11}(5l_5^2 + 8l_8^2) + (-3\tau_{1,9} + 5\tau_{1,12} + 3\tau_{2,5} - 2\tau_{2,12} + 2\tau_{3,12})l_{10}^2 \Big) t^2 - \\
& \quad \frac{1}{2}u(s^2 - t^2 - u^2)(2(2\tau_{1,13} - 4\tau_{2,11} + \tau_{2,14} - 2\tau_{3,6} + 4\tau_{3,13})l_5^2 + (-2\tau_{1,15} + 2\tau_{1,17} + 2\tau_{2,15} - 4\tau_{2,16} + \tau_{2,17} - 6\tau_{3,16})l_7^2 + \\
& \quad 2(-2\tau_{1,9} + 7\tau_{1,10} - 4\tau_{2,9} + \tau_{2,10} - 6\tau_{3,9} + \tau_{3,11})l_8^2 + \\
& \quad 4\tau_{1,11}(l_5^2 + 2l_8^2) + (-3\tau_{1,9} + \tau_{1,12} - 3\tau_{2,5} + 2\tau_{2,12} + \tau_{3,9} - \tau_{3,12})l_{10}^2 \Big) t - \\
& \quad 4s^2u\tau_{1,5}^3 - 4s^2\tau_{1,5}^2(-t\tau_{1,6} + u\tau_{2,5} + s(\tau_{1,8} + \tau_{3,6})) - u^4(2\tau_{1,17} + \tau_{2,15} + \tau_{2,17})l_7^2 + \\
& \quad u^2(s^2 - t^2 - u^2)(2(\tau_{2,11} - \tau_{3,13})l_5^2 + (\tau_{1,15} - 2\tau_{1,17} - \tau_{2,15} + \tau_{2,16} - \tau_{2,17} + \tau_{3,16})l_7^2 + 2(-\tau_{1,10} + \tau_{2,9} + \tau_{3,9})l_8^2) + \\
& \quad 2\tau_{1,5}(2s^2\tau_{1,6}(t\tau_{2,5} + s\tau_{2,8}) - t^2(s^2 + t^2 - 3u^2)l_{10}^2) \Big)
\end{aligned}$$

■  $N_{35}^{(4)}$ 

$$\begin{aligned}
& \frac{1}{4} \left( 2 \tau_{11,14} l_5^2 t^4 - 2 \tau_{13,14} l_5^2 t^4 + 4 \tau_{12,16} l_7^2 t^4 + 4 l_5^2 l_{10}^2 t^4 - 4 \tau_{2,11} \tau_{3,14} l_5^2 t^3 + 4 \tau_{3,13} \tau_{3,14} l_5^2 t^3 - 16 \tau_{1,15}^2 l_7^2 t^3 - 4 \tau_{2,15}^2 l_7^2 t^3 + \right. \\
& 12 \tau_{1,12} \tau_{1,15} l_7^2 t^3 + 4 \tau_{1,12} \tau_{2,15} l_7^2 t^3 - 12 \tau_{1,15} \tau_{2,15} l_7^2 t^3 + 4 \tau_{1,12} \tau_{2,16} l_7^2 t^3 - 8 \tau_{1,15} \tau_{2,16} l_7^2 t^3 - 4 \tau_{2,15} \tau_{2,16} l_7^2 t^3 - \\
& 8 \tau_{1,12} \tau_{3,16} l_7^2 t^3 + 12 \tau_{1,15} \tau_{3,16} l_7^2 t^3 - 4 \tau_{2,12} \tau_{3,16} l_7^2 t^3 + 8 \tau_{2,15} \tau_{3,16} l_7^2 t^3 + 8 \tau_{2,16} \tau_{3,16} l_7^2 t^3 + 4 \tau_{1,9}^2 l_8^2 t^3 + 8 \tau_{1,10}^2 l_8^2 t^3 - \\
& 16 \tau_{1,9} \tau_{1,10} l_8^2 t^3 + 8 \tau_{1,10} \tau_{2,10} l_8^2 t^3 - 16 \tau_{1,10} \tau_{3,9} l_8^2 t^3 + 8 \tau_{1,10} \tau_{3,11} l_8^2 t^3 - 6 \tau_{1,9}^2 l_{10}^2 t^3 - 14 \tau_{1,12}^2 l_{10}^2 t^3 - 2 \tau_{3,9}^2 l_{10}^2 t^3 + \\
& 20 \tau_{1,9} \tau_{1,12} l_{10}^2 t^3 + 4 \tau_{1,9} \tau_{2,5} l_{10}^2 t^3 - 4 \tau_{1,12} \tau_{2,5} l_{10}^2 t^3 - 8 \tau_{1,9} \tau_{2,12} l_{10}^2 t^3 + 8 \tau_{1,12} \tau_{2,12} l_{10}^2 t^3 - 4 \tau_{1,9} \tau_{3,9} l_{10}^2 t^3 + \\
& 4 \tau_{1,12} \tau_{3,9} l_{10}^2 t^3 + 20 \tau_{1,9} \tau_{3,12} l_{10}^2 t^3 - 20 \tau_{1,12} \tau_{3,12} l_{10}^2 t^3 + 4 \tau_{3,9} \tau_{3,12} l_{10}^2 t^3 + 4 (-s^2 + t^2 + u^2) \tau_{13,14} l_5^2 t^2 - \\
& 6 (-s^2 + t^2 + u^2) \tau_{12,16} l_7^2 t^2 + 4 \tau_{1,11}^2 (t l_5^2 - 5 s l_8^2) t^2 - 4 (-s^2 + t^2 + u^2) l_5^2 l_{10}^2 t^2 + 2 (-s^2 + t^2 + u^2) \tau_{2,11} \tau_{2,14} l_5^2 t - \\
& 2 (-s^2 + t^2 + u^2) \tau_{2,14} \tau_{3,13} l_5^2 t - 2 \tau_{1,6} (2 \tau_{1,11} t^2 + (-s^2 + t^2 + u^2) \tau_{2,11} + 2 s (t + 2u) \tau_{3,13}) l_5^2 t + \\
& 2 (-s^2 + t^2 + u^2) \tau_{2,11} \tau_{3,14} l_5^2 t - 2 (-s^2 + t^2 + u^2) \tau_{3,13} \tau_{3,14} l_5^2 t + 4 \tau_{1,13} (t^2 \tau_{3,14} - (t + 2u) (u \tau_{2,11} + t \tau_{3,6} - u \tau_{3,13})) l_5^2 t + \\
& 2u (-s^2 + t^2 + u^2) \tau_{13,14} l_5^2 t + 8 (-s^2 + t^2 + u^2) \tau_{1,15}^2 l_7^2 t + 2 (-s^2 + t^2 + u^2) \tau_{2,15}^2 l_7^2 t - 4 (-s^2 + t^2 + u^2) \tau_{2,16}^2 l_7^2 t - \\
& 10 (-s^2 + t^2 + u^2) \tau_{1,12} \tau_{1,15} l_7^2 t - 4 (-s^2 + t^2 + u^2) \tau_{1,15} \tau_{1,17} l_7^2 t - 4 (-s^2 + t^2 + u^2) \tau_{1,17} \tau_{2,12} l_7^2 t - \\
& 2 (-s^2 + t^2 + u^2) \tau_{1,12} \tau_{2,15} l_7^2 t + 2 (-s^2 + t^2 + u^2) \tau_{1,15} \tau_{2,15} l_7^2 t - 4 (-s^2 + t^2 + u^2) \tau_{1,15} \tau_{2,16} l_7^2 t + \\
& 2 (-s^2 + t^2 + u^2) \tau_{2,12} \tau_{2,16} l_7^2 t - 2 (-s^2 + t^2 + u^2) \tau_{2,15} \tau_{2,16} l_7^2 t - 2 (-s^2 + t^2 + u^2) \tau_{1,15} \tau_{2,17} l_7^2 t - \\
& 2 (-s^2 + t^2 + u^2) \tau_{2,12} \tau_{2,17} l_7^2 t + 12 (-s^2 + t^2 + u^2) \tau_{1,12} \tau_{3,16} l_7^2 t - 12 (-s^2 + t^2 + u^2) \tau_{1,15} \tau_{3,16} l_7^2 t + \\
& 6 (-s^2 + t^2 + u^2) \tau_{2,12} \tau_{3,16} l_7^2 t - 8 (-s^2 + t^2 + u^2) \tau_{2,15} \tau_{3,16} l_7^2 t - 8 (-s^2 + t^2 + u^2) \tau_{2,16} \tau_{3,16} l_7^2 t - \\
& 2 (-s^2 + t^2 + u^2) \tau_{1,15} \tau_{3,17} l_7^2 t - 6u (-s^2 + t^2 + u^2) \tau_{12,16} l_7^2 t - 2 (-s^2 + t^2 + u^2) \tau_{1,9}^2 l_8^2 t - \\
& 8 (-s^2 + t^2 + u^2) \tau_{1,10}^2 l_8^2 t + 12 (-s^2 + t^2 + u^2) \tau_{1,9} \tau_{1,10} l_8^2 t - 4 (-s^2 + t^2 + u^2) \tau_{1,9} \tau_{2,9} l_8^2 t + \\
& 4 (-s^2 + t^2 + u^2) \tau_{1,10} \tau_{2,9} l_8^2 t - 4 (-s^2 + t^2 + u^2) \tau_{1,9} \tau_{2,10} l_8^2 t - 8 (-s^2 + t^2 + u^2) \tau_{1,10} \tau_{2,10} l_8^2 t + \\
& 4 (-s^2 + t^2 + u^2) \tau_{1,9} \tau_{3,9} l_8^2 t + 20 (-s^2 + t^2 + u^2) \tau_{1,10} \tau_{3,9} l_8^2 t - 4 (-s^2 + t^2 + u^2) \tau_{1,9} \tau_{3,11} l_8^2 t - \\
& 8 (-s^2 + t^2 + u^2) \tau_{1,10} \tau_{3,11} l_8^2 t + 4 \tau_{1,11} (t ((t + 2u) \tau_{1,13} - u \tau_{2,11} + t \tau_{2,14} - t \tau_{3,6} + u \tau_{3,13})) l_5^2 + \\
& 2 s ((2t - u) \tau_{1,9} - (4t + 3u) \tau_{1,10} + 2u (\tau_{2,9} + \tau_{3,9}) - t (\tau_{2,10} - 2 \tau_{3,9} + \tau_{3,11})) l_8^2) t + 6 (-s^2 + t^2 + u^2) \tau_{1,9}^2 l_{10}^2 t + \\
& 14 (-s^2 + t^2 + u^2) \tau_{1,12}^2 l_{10}^2 t - 20 (-s^2 + t^2 + u^2) \tau_{1,9} \tau_{1,12} l_{10}^2 t - 12 (-s^2 + t^2 + u^2) \tau_{1,9} \tau_{2,5} l_{10}^2 t + \\
& 12 (-s^2 + t^2 + u^2) \tau_{1,12} \tau_{2,5} l_{10}^2 t + 8 (-s^2 + t^2 + u^2) \tau_{1,9} \tau_{2,12} l_{10}^2 t - 8 (-s^2 + t^2 + u^2) \tau_{1,12} \tau_{2,12} l_{10}^2 t - \\
& 8 (-s^2 + t^2 + u^2) \tau_{1,9} \tau_{3,12} l_{10}^2 t + 8 (-s^2 + t^2 + u^2) \tau_{1,12} \tau_{3,12} l_{10}^2 t - 2 (-s^2 + t^2 + u^2) \tau_{3,9} \tau_{3,12} l_{10}^2 t + 4u^2 \tau_{1,5}^4 + \\
& 4 \tau_{1,6}^2 (t \tau_{2,5} + s \tau_{2,8})^2 + 8u \tau_{1,5}^3 (-t \tau_{1,6} + u \tau_{2,5} + s (\tau_{1,8} + \tau_{3,6})) - 4u^3 \tau_{2,15}^2 l_7^2 + 2u (-s^2 + t^2 + u^2) \tau_{2,15}^2 l_7^2 - \\
& 4u (-s^2 + t^2 + u^2) \tau_{2,16}^2 l_7^2 - 4u^3 \tau_{1,12} \tau_{1,15} l_7^2 - 2u (-s^2 + t^2 + u^2) \tau_{1,12} \tau_{1,15} l_7^2 - 4u (-s^2 + t^2 + u^2) \tau_{1,15} \tau_{1,17} l_7^2 + \\
& 8u^3 \tau_{1,17} \tau_{2,12} l_7^2 - 8u (-s^2 + t^2 + u^2) \tau_{1,17} \tau_{2,12} l_7^2 - 4u^3 \tau_{1,12} \tau_{2,15} l_7^2 + 2u (-s^2 + t^2 + u^2) \tau_{1,12} \tau_{2,15} l_7^2 - \\
& 4u^3 \tau_{1,15} \tau_{2,15} l_7^2 - 2u (-s^2 + t^2 + u^2) \tau_{1,15} \tau_{2,15} l_7^2 - 8u^3 \tau_{1,17} \tau_{2,15} l_7^2 + 4u (-s^2 + t^2 + u^2) \tau_{1,17} \tau_{2,15} l_7^2 - \\
& 8u^3 \tau_{1,12} \tau_{2,16} l_7^2 + 6u (-s^2 + t^2 + u^2) \tau_{1,12} \tau_{2,16} l_7^2 - 8u (-s^2 + t^2 + u^2) \tau_{1,15} \tau_{2,16} l_7^2 - 8u^3 \tau_{1,17} \tau_{2,16} l_7^2 + \\
& 4u (-s^2 + t^2 + u^2) \tau_{1,17} \tau_{2,16} l_7^2 - 4u^3 \tau_{2,12} \tau_{2,16} l_7^2 + 4u (-s^2 + t^2 + u^2) \tau_{2,12} \tau_{2,16} l_7^2 - 4u^3 \tau_{2,15} \tau_{2,16} l_7^2 -
\end{aligned}$$

$$\begin{aligned}
& 2u(-s^2+t^2+u^2)\tau_{2,15}\tau_{2,16}l_7^2 - 2u(-s^2+t^2+u^2)\tau_{1,15}\tau_{2,17}l_7^2 + 4u^3\tau_{2,12}\tau_{2,17}l_7^2 - 4u(-s^2+t^2+u^2)\tau_{2,12}\tau_{2,17}l_7^2 - \\
& 4u^3\tau_{2,15}\tau_{2,17}l_7^2 + 2u(-s^2+t^2+u^2)\tau_{2,15}\tau_{2,17}l_7^2 - 4u^3\tau_{2,16}\tau_{2,17}l_7^2 + 2u(-s^2+t^2+u^2)\tau_{2,16}\tau_{2,17}l_7^2 - \\
& 8u^3\tau_{1,12}\tau_{3,16}l_7^2 + 12u(-s^2+t^2+u^2)\tau_{1,12}\tau_{3,16}l_7^2 - 6u(-s^2+t^2+u^2)\tau_{1,15}\tau_{3,16}l_7^2 - 4u^3\tau_{2,12}\tau_{3,16}l_7^2 + \\
& 6u(-s^2+t^2+u^2)\tau_{2,12}\tau_{3,16}l_7^2 - 4u(-s^2+t^2+u^2)\tau_{2,15}\tau_{3,16}l_7^2 - 4u(-s^2+t^2+u^2)\tau_{2,16}\tau_{3,16}l_7^2 + \\
& 4u^3\tau_{1,15}\tau_{3,17}l_7^2 - 4u(-s^2+t^2+u^2)\tau_{1,15}\tau_{3,17}l_7^2 - 2u^2(-s^2+t^2+u^2)\tau_{12,16}l_7^2 - 4u(-s^2+t^2+u^2)\tau_{1,10}^2l_8^2 + \\
& 4u(-s^2+t^2+u^2)\tau_{1,9}\tau_{1,10}l_8^2 - 8u^3\tau_{1,9}\tau_{2,9}l_8^2 - 8u^3\tau_{1,10}\tau_{2,9}l_8^2 + 8u(-s^2+t^2+u^2)\tau_{1,10}\tau_{2,9}l_8^2 - \\
& 4u(-s^2+t^2+u^2)\tau_{1,9}\tau_{2,10}l_8^2 - 4u(-s^2+t^2+u^2)\tau_{1,10}\tau_{2,10}l_8^2 - 8u^3\tau_{1,9}\tau_{3,9}l_8^2 + 8u(-s^2+t^2+u^2)\tau_{1,9}\tau_{3,9}l_8^2 - \\
& 8u^3\tau_{1,10}\tau_{3,9}l_8^2 + 16u(-s^2+t^2+u^2)\tau_{1,10}\tau_{3,9}l_8^2 - 4u(-s^2+t^2+u^2)\tau_{1,9}\tau_{3,11}l_8^2 - 4u(-s^2+t^2+u^2)\tau_{1,10}\tau_{3,11}l_8^2 - \\
& 3u(-s^2+t^2+u^2)\tau_{1,9}^2l_{10}^2 + u(-s^2+t^2+u^2)\tau_{1,12}^2l_{10}^2 - u(-s^2+t^2+u^2)\tau_{3,9}^2l_{10}^2 + \\
& 2u(-s^2+t^2+u^2)\tau_{1,9}\tau_{1,12}l_{10}^2 - 6u(-s^2+t^2+u^2)\tau_{1,9}\tau_{2,5}l_{10}^2 + 6u(-s^2+t^2+u^2)\tau_{1,12}\tau_{2,5}l_{10}^2 + \\
& 4u(-s^2+t^2+u^2)\tau_{1,9}\tau_{2,12}l_{10}^2 - 4u(-s^2+t^2+u^2)\tau_{1,12}\tau_{2,12}l_{10}^2 + 2u(-s^2+t^2+u^2)\tau_{1,9}\tau_{3,9}l_{10}^2 - \\
& 2u(-s^2+t^2+u^2)\tau_{1,12}\tau_{3,9}l_{10}^2 - 2u(-s^2+t^2+u^2)\tau_{1,9}\tau_{3,12}l_{10}^2 + 2u(-s^2+t^2+u^2)\tau_{1,12}\tau_{3,12}l_{10}^2 - \\
& 4s((\tau_{3,9}^2 - s l_8^2)s^2 + (t^2 + u^2)l_8^2 s + u(2t + u)(\tau_{1,9} + \tau_{1,10})^2)l_{12}^2 + 4\tau_{1,5}^2 \left( -2l_{10}^2 t^3 + \tau_{1,6}^2 t^2 + (\tau_{1,8} + \tau_{3,6})^2 t^2 + \right. \\
& \quad \left( -s^2 + t^2 + u^2 \right) l_{10}^2 t + u^2 (\tau_{1,8} - \tau_{2,5} + \tau_{3,6})^2 + (s^2 - t^2 - u^2) (\tau_{1,8} + \tau_{3,6}) (\tau_{1,8} - \tau_{2,5} + \tau_{3,6}) - \\
& \quad \left. 2\tau_{1,6} (s t \tau_{1,8} + (s^2 - t^2 - u^2) \tau_{2,5} + s(u \tau_{2,8} + t \tau_{3,6})) - \frac{1}{2} u (-s^2 + t^2 + u^2) (l_{10}^2 - l_{12}^2) - u^3 l_{12}^2 \right) + 4\tau_{1,5} \\
& \quad \left( 2t(t \tau_{2,5} + s \tau_{2,8}) \tau_{1,6}^2 - 2(t \tau_{2,5} + s \tau_{2,8})(u \tau_{2,5} + s(\tau_{1,8} + \tau_{3,6})) \tau_{1,6} - \frac{1}{2} t (4(s^2 + t^2 - 3u^2) \tau_{1,9} - 4(2s^2 + t^2 - 3u^2) \right. \\
& \quad \left. \tau_{1,12} + 2(-s^2 + t^2 + u^2) \tau_{2,5} + (u^2 + 3(s^2 + t^2)) \tau_{3,9} - 2t(3t + u) \tau_{3,12}) l_{10}^2 - s(s^2 - t^2 - u^2) (\tau_{1,9} + \tau_{1,10}) l_{12}^2 \right) \Big)
\end{aligned}$$

■  $N_{35}^{(5)}$

$$\begin{aligned}
& \frac{1}{2} (\tau_{2,12}\tau_{12,16}l_7^2t^3 - \tau_{1,9}l_5^2l_{10}^2t^3 + \tau_{4,9}l_5^2l_{10}^2t^3 + 2\tau_{4,13}l_5^2l_{10}^2t^3 - \tau_{2,16}^3l_7^2t^2 + \tau_{2,12}\tau_{2,16}^2l_7^2t^2 - \tau_{2,12}\tau_{2,16}\tau_{2,17}l_7^2t^2 + \\
& \tau_{2,16}^2\tau_{3,16}l_7^2t^2 + 3u\tau_{2,12}\tau_{12,16}l_7^2t^2 - u\tau_{2,16}\tau_{12,16}l_7^2t^2 - 4\tau_{1,11}^3l_8^2t^2 + 2\tau_{1,9}\tau_{1,10}^2l_8^2t^2 + 6\tau_{1,9}\tau_{1,11}^2l_8^2t^2 - \\
& 6\tau_{1,10}\tau_{1,11}^2l_8^2t^2 - 2\tau_{1,9}^2\tau_{1,10}l_8^2t^2 - 2\tau_{1,9}^2\tau_{1,11}l_8^2t^2 - 2\tau_{1,10}^2\tau_{1,11}l_8^2t^2 + 8\tau_{1,9}\tau_{1,10}\tau_{1,11}l_8^2t^2 - 2\tau_{1,11}^2\tau_{2,9}l_8^2t^2 + \\
& 2\tau_{1,9}\tau_{1,10}\tau_{2,9}l_8^2t^2 + 2\tau_{1,9}\tau_{1,11}\tau_{2,9}l_8^2t^2 - 2\tau_{1,10}\tau_{1,11}\tau_{2,9}l_8^2t^2 - 2\tau_{1,11}^2\tau_{2,10}l_8^2t^2 + 2\tau_{1,9}\tau_{1,10}\tau_{2,10}l_8^2t^2 + \\
& 2\tau_{1,9}\tau_{1,11}\tau_{2,10}l_8^2t^2 - 2\tau_{1,10}\tau_{1,11}\tau_{2,10}l_8^2t^2 + 2\tau_{1,11}^2\tau_{3,9}l_8^2t^2 - 2\tau_{1,9}\tau_{1,10}\tau_{3,9}l_8^2t^2 - 2\tau_{1,9}\tau_{1,11}\tau_{3,9}l_8^2t^2 + \\
& 2\tau_{1,10}\tau_{1,11}\tau_{3,9}l_8^2t^2 - 2\tau_{1,11}^2\tau_{3,11}l_8^2t^2 + 2\tau_{1,9}\tau_{1,10}\tau_{3,11}l_8^2t^2 + 2\tau_{1,9}\tau_{1,11}\tau_{3,11}l_8^2t^2 - 2\tau_{1,10}\tau_{1,11}\tau_{3,11}l_8^2t^2 - \\
& 2\tau_{1,5}\tau_{1,9}^2l_{10}^2t^2 - \tau_{1,5}\tau_{3,9}^2l_{10}^2t^2 - \tau_{1,9}\tau_{3,9}^2l_{10}^2t^2 - 2\tau_{1,5}^2\tau_{1,9}l_{10}^2t^2 - 2\tau_{1,9}^2\tau_{2,5}l_{10}^2t^2 - 2\tau_{1,5}\tau_{1,9}\tau_{2,5}l_{10}^2t^2 - \\
& 2\tau_{1,5}^2\tau_{3,9}l_{10}^2t^2 - \tau_{1,9}^2\tau_{3,9}l_{10}^2t^2 - 3\tau_{1,5}\tau_{1,9}\tau_{3,9}l_{10}^2t^2 + 2\tau_{1,5}^2\tau_{3,12}l_{10}^2t^2 + 3\tau_{1,9}^2\tau_{3,12}l_{10}^2t^2 + 5\tau_{1,5}\tau_{1,9}\tau_{3,12}l_{10}^2t^2 + \\
& \tau_{1,5}\tau_{3,9}\tau_{3,12}l_{10}^2t^2 + \tau_{1,9}\tau_{3,9}\tau_{3,12}l_{10}^2t^2 + u\tau_{1,13}l_5^2l_{10}^2t^2 + u\tau_{4,13}l_5^2l_{10}^2t^2 - 2(3t + u)\tau_{1,15}^3l_7^2t - 3s^2\tau_{2,12}\tau_{12,16}l_7^2t +
\end{aligned}$$

$$\begin{aligned}
& 3u^2 \tau_{2,12} \tau_{12,16} l_7^2 t + 2s^2 \tau_{2,16} \tau_{12,16} l_7^2 t - 2u^2 \tau_{2,16} \tau_{12,16} l_7^2 t - s^2 \tau_{1,9} l_5^2 l_{10}^2 t + u^2 \tau_{1,9} l_5^2 l_{10}^2 t - 2s^2 \tau_{1,13} l_5^2 l_{10}^2 t + \\
& 2u^2 \tau_{1,13} l_5^2 l_{10}^2 t - s^2 \tau_{4,9} l_5^2 l_{10}^2 t + u^2 \tau_{4,9} l_5^2 l_{10}^2 t - 2s^2 \tau_{4,13} l_5^2 l_{10}^2 t + 2u^2 \tau_{4,13} l_5^2 l_{10}^2 t - (t^2 + u^2) \tau_{2,15}^3 l_7^2 + \\
& s^2 \tau_{2,16}^3 l_7^2 - u^2 \tau_{2,16}^3 l_7^2 - s^2 \tau_{2,12} \tau_{2,16}^2 l_7^2 - u^2 \tau_{2,12} \tau_{2,16}^2 l_7^2 - 2\tau_{1,17} (s\tau_{2,12} + u(\tau_{2,15} + \tau_{2,16}))^2 l_7^2 - \\
& s^2 \tau_{2,12}^2 \tau_{2,17} l_7^2 - u^2 \tau_{2,16}^2 \tau_{2,17} l_7^2 + s^2 \tau_{2,12} \tau_{2,16} \tau_{2,17} l_7^2 + u^2 \tau_{2,12} \tau_{2,16} \tau_{2,17} l_7^2 + s^2 \tau_{2,16}^2 \tau_{3,16} l_7^2 - \\
& u^2 \tau_{2,16}^2 \tau_{3,16} l_7^2 - 2s^2 \tau_{2,12} \tau_{2,16} \tau_{3,16} l_7^2 + \tau_{2,15}^2 (-\tau_{2,17} u^2 + (s^2 - 3(t^2 + u^2)) \tau_{2,16} + (s^2 + t^2 - u^2) \tau_{3,16}) l_7^2 - \\
& \tau_{1,15}^2 (2\tau_{1,17} t^2 + \tau_{2,17} t^2 + (-2s^2 + 9t^2 + u^2) \tau_{2,15} + (-3s^2 + 9t^2 + u^2) \tau_{2,16} + 2s((3t + u) \tau_{3,16} - t \tau_{3,17})) l_7^2 + \\
& u^3 \tau_{2,12} \tau_{12,16} l_7^2 - 3s^2 u \tau_{2,12} \tau_{12,16} l_7^2 - u^3 \tau_{2,16} \tau_{12,16} l_7^2 + s^2 u \tau_{2,16} \tau_{12,16} l_7^2 + \\
& \tau_{1,15} (2(2t + u) \tau_{12,16} s^2 - 2\tau_{2,12} (t \tau_{2,16} - t \tau_{2,17} + s \tau_{3,17}) s + (s^2 - 5t^2 - 3u^2) \tau_{2,15}^2 - 2t(t - 3u) \tau_{2,16}^2 + \\
& 4t \tau_{1,17} (s \tau_{2,12} + u(\tau_{2,15} + \tau_{2,16})) + \tau_{2,16} ((s^2 - t^2 - u^2) \tau_{2,17} - 2s(3t \tau_{3,16} + u \tau_{3,17})) + \\
& \tau_{2,15} (2(2s^2 - 5t^2 - 3u^2) \tau_{2,16} + (s^2 - t^2 - u^2) \tau_{2,17} - 2s(3t \tau_{3,16} + u \tau_{3,17}))) l_7^2 - \\
& \tau_{2,15} ((3(t^2 + u^2) - 2s^2) \tau_{2,16}^2 + 2(u^2 \tau_{2,17} - (s^2 + t^2 - u^2) \tau_{3,16}) \tau_{2,16} + \tau_{2,12} (2\tau_{3,16} s^2 + (s^2 - t^2 + u^2) (\tau_{2,16} - \tau_{2,17}))) + \\
& (u(t + u)^2 - s^2(2t + u) \tau_{12,16}) l_7^2 + 2s^2 \tau_{1,9} \tau_{1,10}^2 l_8^2 - 2u^2 \tau_{1,9} \tau_{1,10}^2 l_8^2 - 2s^2 \tau_{1,9} \tau_{1,11}^2 l_8^2 + \\
& 2u^2 \tau_{1,9} \tau_{1,11}^2 l_8^2 - 4s^2 \tau_{1,10} \tau_{1,11}^2 l_8^2 + 4u^2 \tau_{1,10} \tau_{1,11}^2 l_8^2 + 2s^2 \tau_{1,9}^2 \tau_{1,11} l_8^2 - 2u^2 \tau_{1,9}^2 \tau_{1,11} l_8^2 - \\
& 2s^2 \tau_{1,10}^2 \tau_{1,11} l_8^2 + 2u^2 \tau_{1,10}^2 \tau_{1,11} l_8^2 + 4s^2 \tau_{1,9} \tau_{1,10} \tau_{1,11} l_8^2 - 4u^2 \tau_{1,9} \tau_{1,10} \tau_{1,11} l_8^2 - 4u^2 \tau_{1,9}^2 \tau_{2,9} l_8^2 + \\
& 2s^2 \tau_{1,11}^2 \tau_{2,9} l_8^2 - 2u^2 \tau_{1,11}^2 \tau_{2,9} l_8^2 - 2s^2 \tau_{1,9} \tau_{1,10} \tau_{2,9} l_8^2 - 2u^2 \tau_{1,9} \tau_{1,10} \tau_{2,9} l_8^2 - 2s^2 \tau_{1,9} \tau_{1,11} \tau_{2,9} l_8^2 + \\
& 6u^2 \tau_{1,9} \tau_{1,11} \tau_{2,9} l_8^2 + 2s^2 \tau_{1,10} \tau_{1,11} \tau_{2,9} l_8^2 + 2u^2 \tau_{1,10} \tau_{1,11} \tau_{2,9} l_8^2 + 2s^2 \tau_{1,9}^2 \tau_{2,10} l_8^2 - 2u^2 \tau_{1,9}^2 \tau_{2,10} l_8^2 + \\
& 2s^2 \tau_{1,9} \tau_{1,10} \tau_{2,10} l_8^2 - 2u^2 \tau_{1,9} \tau_{1,10} \tau_{2,10} l_8^2 - 2s^2 \tau_{1,9} \tau_{1,11} \tau_{2,10} l_8^2 + 2u^2 \tau_{1,9} \tau_{1,11} \tau_{2,10} l_8^2 - \\
& 2s^2 \tau_{1,10} \tau_{1,11} \tau_{2,10} l_8^2 + 2u^2 \tau_{1,10} \tau_{1,11} \tau_{2,10} l_8^2 + 4s^2 \tau_{1,10}^2 \tau_{3,9} l_8^2 + 2s^2 \tau_{1,11}^2 \tau_{3,9} l_8^2 - 2u^2 \tau_{1,11}^2 \tau_{3,9} l_8^2 + \\
& 2s^2 \tau_{1,9} \tau_{1,10} \tau_{3,9} l_8^2 + 2u^2 \tau_{1,9} \tau_{1,10} \tau_{3,9} l_8^2 + 2s^2 \tau_{1,9} \tau_{1,11} \tau_{3,9} l_8^2 + 2u^2 \tau_{1,9} \tau_{1,11} \tau_{3,9} l_8^2 + 6s^2 \tau_{1,10} \tau_{1,11} \tau_{3,9} l_8^2 - \\
& 2u^2 \tau_{1,10} \tau_{1,11} \tau_{3,9} l_8^2 - 2u^2 \tau_{1,9}^2 \tau_{3,11} l_8^2 - 2s^2 \tau_{1,10}^2 \tau_{3,11} l_8^2 - 2s^2 \tau_{1,9} \tau_{1,10} \tau_{3,11} l_8^2 - 2u^2 \tau_{1,9} \tau_{1,10} \tau_{3,11} l_8^2 - \\
& 2s^2 \tau_{1,9} \tau_{1,11} \tau_{3,11} l_8^2 + 2u^2 \tau_{1,9} \tau_{1,11} \tau_{3,11} l_8^2 - 2s^2 \tau_{1,10} \tau_{1,11} \tau_{3,11} l_8^2 + 2u^2 \tau_{1,10} \tau_{1,11} \tau_{3,11} l_8^2 - s^2 \tau_{1,9}^3 l_{10}^2 + \\
& 2u^2 \tau_{1,9}^3 l_{10}^2 + (3s^2 - 2u^2) \tau_{1,12}^3 l_{10}^2 - s^2 \tau_{3,9}^3 l_{10}^2 - 2s^2 \tau_{1,5} \tau_{1,9}^2 l_{10}^2 + 6u^2 \tau_{1,5} \tau_{1,9}^2 l_{10}^2 - s^2 \tau_{1,5} \tau_{3,9}^2 l_{10}^2 + \\
& u^2 \tau_{1,5} \tau_{3,9}^2 l_{10}^2 + u^2 \tau_{1,9} \tau_{3,9}^2 l_{10}^2 + s^2 \tau_{2,5} \tau_{3,9}^2 l_{10}^2 - 2s^2 \tau_{1,5}^2 \tau_{1,9} l_{10}^2 + 4u^2 \tau_{1,5}^2 \tau_{1,9} l_{10}^2 - 2u^2 \tau_{1,5}^2 \tau_{2,5} l_{10}^2 + \\
& 3s^2 \tau_{1,9}^2 \tau_{2,5} l_{10}^2 + 2s^2 \tau_{1,5} \tau_{1,9} \tau_{2,5} l_{10}^2 - 2u^2 \tau_{1,5} \tau_{1,9} \tau_{2,5} l_{10}^2 - 2s^2 \tau_{1,9}^2 \tau_{2,12} l_{10}^2 + 2s^2 \tau_{1,5}^2 \tau_{3,9} l_{10}^2 - \\
& u^2 \tau_{1,9}^2 \tau_{3,9} l_{10}^2 - 3s^2 \tau_{1,5} \tau_{1,9} \tau_{3,9} l_{10}^2 - u^2 \tau_{1,5} \tau_{1,9} \tau_{3,9} l_{10}^2 - 2s^2 \tau_{1,5}^2 \tau_{3,12} l_{10}^2 + 2s^2 \tau_{1,9}^2 \tau_{3,12} l_{10}^2 - \\
& u^2 \tau_{1,9}^2 \tau_{3,12} l_{10}^2 + s^2 \tau_{3,9}^2 \tau_{3,12} l_{10}^2 + s^2 \tau_{1,5} \tau_{1,9} \tau_{3,12} l_{10}^2 - u^2 \tau_{1,5} \tau_{1,9} \tau_{3,12} l_{10}^2 + s^2 \tau_{1,5} \tau_{3,9} \tau_{3,12} l_{10}^2 - \\
& u^2 \tau_{1,5} \tau_{3,9} \tau_{3,12} l_{10}^2 + s^2 \tau_{1,9} \tau_{3,9} \tau_{3,12} l_{10}^2 - u^2 \tau_{1,9} \tau_{3,9} \tau_{3,12} l_{10}^2 + u^3 \tau_{1,13} l_5^2 l_{10}^2 - s^2 u \tau_{1,13} l_5^2 l_{10}^2 + \\
& u^3 \tau_{4,13} l_5^2 l_{10}^2 - s^2 u \tau_{4,13} l_5^2 l_{10}^2 + \tau_{1,12}^2 (-2(2\tau_{1,15} + \tau_{2,15} + 2\tau_{2,16}) l_7^2 s^2 - 4t(2t + 3u) \tau_{1,5} l_{10}^2 - \\
& (2\tau_{2,12} s^2 + (7s^2 - 6u^2) \tau_{1,9} + (2t^2 - 3s^2) \tau_{2,5} + (t^2 + u^2) \tau_{3,9} + (-2s^2 - 3t^2 + u^2) \tau_{3,12}) l_{10}^2) + \\
& \tau_{1,12} (2s(2\tau_{12,16} s^2 - \tau_{2,12} \tau_{2,16} s - (5t + u) \tau_{1,15}^2 + \tau_{1,15} (2(u - 2t) \tau_{2,15} + (2u - 5t) \tau_{2,16} - 2s \tau_{3,16}) - \\
& (\tau_{2,15} + \tau_{2,16}) ((t - u) \tau_{2,15} + (t - 2u) \tau_{2,16} + 2s \tau_{3,16})) l_7^2 + (2(s^2 + t^2 - 2u^2) \tau_{1,5}^2 + (4(2s^2 + t^2 - 3u^2) \tau_{1,9} + \\
& 2(-s^2 + t^2 + u^2) \tau_{2,5} + (u^2 + 3(s^2 + t^2)) \tau_{3,9} - 2t(3t + u) \tau_{3,12}) \tau_{1,5} + (5s^2 - 6u^2) \tau_{1,9}^2 + s \tau_{3,9} \\
& ((u - t) \tau_{3,9} + 2t \tau_{3,12}) + 2\tau_{1,9} (2\tau_{2,12} s^2 + (2t^2 - 3s^2) \tau_{2,5} + (t^2 + u^2) \tau_{3,9} + (-2s^2 - 3t^2 + u^2) \tau_{3,12})) l_{10}^2) +
\end{aligned}$$

$$\begin{aligned}
& (2u^2 \tau_{1,5}^3 + 2((s^2 + t^2 + u^2) \tau_{1,9} + (s^2 + t^2 + u^2) \tau_{1,10} + u(u \tau_{2,5} + 2s \tau_{3,9} - (2t + u) \tau_{3,10})) \tau_{1,5}^2 + \\
& 2((s^2 + t^2) \tau_{1,9}^2 + 2((2s^2 + t^2) \tau_{1,10} + t(-u \tau_{2,5} - s \tau_{3,9} + t \tau_{3,10})) \tau_{1,9} + (3s^2 + t^2) \tau_{1,10}^2 + \\
& s \tau_{3,9} (s \tau_{3,9} - 2t \tau_{3,10}) + 2t \tau_{1,10} (-u \tau_{2,5} - s \tau_{3,9} + t \tau_{3,10})) \tau_{1,5} + 2s^2 \tau_{1,10}^3 - \\
& 2\tau_{1,10}^2 (\tau_{2,10} s^2 + u(2t + u) \tau_{2,5} - t^2 \tau_{3,10}) + 2\tau_{1,9}^2 ((\tau_{1,10} - \tau_{2,10}) s^2 - u(2t + u) \tau_{2,5} + t^2 \tau_{3,10}) + \\
& 4\tau_{1,9} (s^2 \tau_{1,10}^2 + (-\tau_{2,10} s^2 - u(2t + u) \tau_{2,5} + t^2 \tau_{3,10}) \tau_{1,10} - s t \tau_{3,9} \tau_{3,10}) - \\
& 2s \tau_{1,10} (2t \tau_{3,9} \tau_{3,10} + u(u - 3t) l_8^2) - s(2s \tau_{2,5} \tau_{3,9}^2 - 2s \tau_{3,10} \tau_{3,9}^2 + ((s^2 - 3t^2 - 5u^2) \tau_{1,6} + \\
& 2u(u - 3t) \tau_{1,11} + s(-2t \tau_{3,10} + s \tau_{3,11} + 2(u - t) \tau_{4,6} + 2(t - 2u) \tau_{4,10} + (t - 3u) \tau_{4,11})) l_8^2) l_{12}^2)
\end{aligned}$$

■  $N_{35}^{(6)}$

$$\begin{aligned}
& \frac{1}{4} (4 l_8^2 l_{12}^2 \tau_{1,6} (\tau_{1,10} (s^2 + t^2 + 3u^2) + \tau_{1,11} (s^2 + t^2 + 3u^2) - s(-s \tau_{3,11} + \tau_{4,10} (t + 4u) + \tau_{4,11} (t + 3u) + t \tau_{3,10} - 2u \tau_{4,6})) - \\
& 2 l_8^2 l_{12}^2 \tau_{1,10}^2 (2s^2 + t^2 + 3u^2) - 2 l_8^2 l_{12}^2 \tau_{1,11}^2 (2s^2 + t^2 + 3u^2) - \\
& 4 l_8^2 l_{12}^2 \tau_{1,10} (\tau_{1,11} (2s^2 + t^2 + 3u^2) - s(-2s \tau_{3,11} + \tau_{4,10} (t + 4u) + 2\tau_{4,11} (t + 2u) + t \tau_{3,10} - 2u \tau_{4,6})) + \\
& 4 l_8^2 l_{12}^2 s \tau_{1,11} (-2s \tau_{3,11} + \tau_{4,10} (t + 4u) + 2\tau_{4,11} (t + 2u) + t \tau_{3,10} - 2u \tau_{4,6}) - \\
& s(2 l_8^2 s (l_{12}^2 (\tau_{3,11}^2 + (\tau_{4,10} + 2\tau_{4,11}) \tau_{3,11} + 3\tau_{4,11}^2 + 2(\tau_{3,10} + \tau_{4,6} - 2\tau_{4,10}) (\tau_{4,6} - \tau_{4,10}) - (\tau_{3,10} + 4\tau_{4,6} - 6\tau_{4,10}) \tau_{4,11}) + \\
& 2 l_7^2 l_{15}^2 s) - l_6^2 l_{12}^2 l_{16}^2 t(2t + u) - 2 l_8^2 l_{12}^2 \tau_{1,6}^2 (t^2 + 3u^2))
\end{aligned}$$

■  $N_{35}^{(7)}$

0

■  $N_{35}^{(8)}$

0
