# Supplementary material for: The Ultraviolet Behavior of N=8 Supergravity at Four Loops
Source: arXiv:0905.2326 ancillary file (2012-01-08)
Supplement: Supplementary file 31 [file SUGRA36.pdf]

## Integral 36: $\mathcal{I}_{36}$

$\mathcal{N} = 8$  four-point four-loop amplitude.

### ■ 2D plot of graph associated with $\mathcal{I}_{36}$

This fixes the labelling associated with the numerator expressions given below.

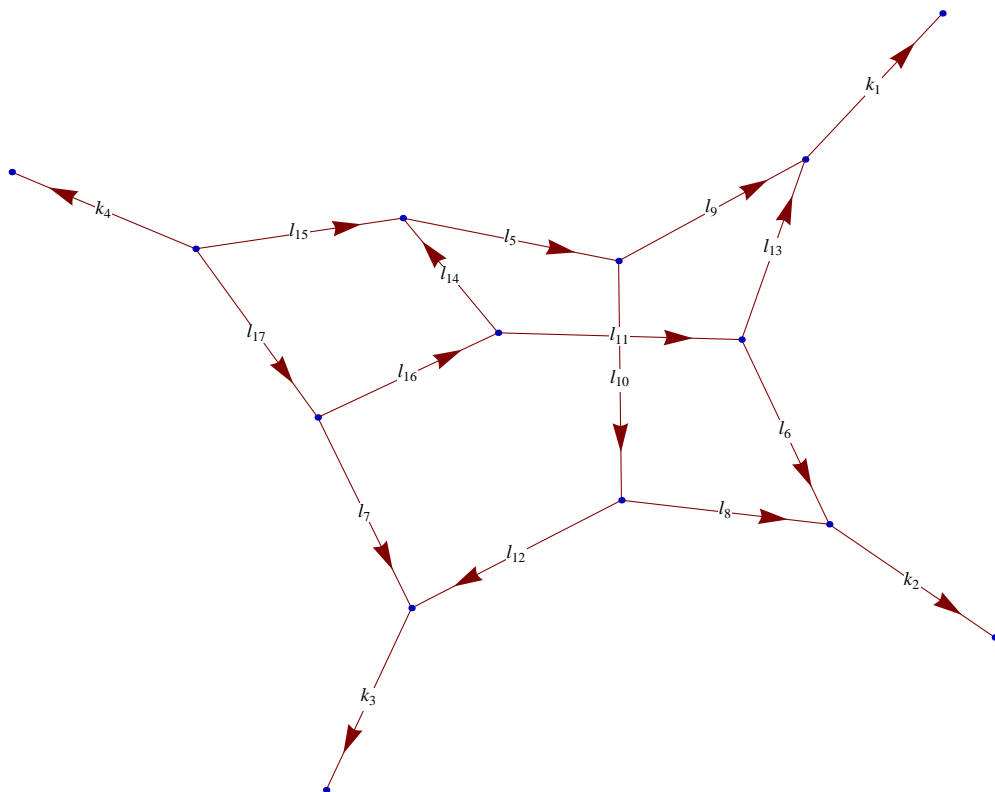

When using MathPlayer, by clicking three times (holding the click on the third click) directly on a vertex, one is able to move that vertex around, and its associated edges follow elastically. This functionality is absent when viewing as a pdf.

*Note: propagators for certain graphs were relabeled in the manuscript due to size constraints. The labels given in `aux/rawData/Neq8FourLoops.m` should be used for verification purposes.*

### ■ 3D plot of graph associated with $\mathcal{I}_{36}$

3D PLOT UNAVAILABLE FOR PDF. Please see .nb version for the 3D figure.

When using MathPlayer, by clicking anywhere in the image and dragging one should be able to rotate this 3D image. By holding (ALT) or (COMMAND) while clicking and moving the mouse up/down one should be able to zoom in/out. This functionality is absent when viewing as a pdf.

### ■ "Vertex Form" of graph associated with $\mathcal{I}_{36}$

This function returns the graph associated with the integral object in a vertex representation. This can be used as a way of specifying the topology of a graph using trivalent (cubic) vertices,  $\text{gVertex}[p_a, p_b, p_c]$ , where  $\{p_a, p_b, p_c\}$  are momenta labeling the propagators (edges) of the graph, and is understood that the edge labelled by  $p_a$  flows into the edge labelled by  $-p_a$ . Additionally, each vertex represents the manifest conservation of ( $D$  - dimensional) momenta :

$$\text{gVertex}[\{p_1, p_2, p_3\}] \iff (p_1 + p_2 + p_3 = 0)$$

$$\{\text{gVertex}(\{k_1, -l_{13}, -l_9\}), \text{gVertex}(\{k_2, -l_8, -l_6\}), \text{gVertex}(\{k_3, -l_{12}, -l_7\}), \text{gVertex}(\{k_4, l_{15}, l_{17}\}), \text{gVertex}(\{-l_5, l_{10}, l_9\}), \\ \text{gVertex}(\{l_5, -l_{14}, -l_{15}\}), \text{gVertex}(\{l_6, -l_{11}, l_{13}\}), \text{gVertex}(\{l_7, -l_{17}, l_{16}\}), \text{gVertex}(\{l_8, -l_{10}, l_{12}\}), \text{gVertex}(\{l_{11}, -l_{16}, l_{14}\})\}$$

### ■ Numerator expression for integral 36:

The following notation is used:  $\tau_{i,j} \equiv \begin{cases} 2 k_i \cdot l_j & \text{if } i \leq 4, j > 4 \\ 2 l_i \cdot l_j & \text{if } i, j > 4 \end{cases}$ .

$$s \equiv 2 k_1 \cdot k_2 = 2 k_3 \cdot k_4$$

We use  $s, t, u$  to represent the traditional Mandelstam variables for massless external four-point momenta:  $t \equiv 2 k_1 \cdot k_4 = 2 k_2 \cdot k_3$ .

$$u \equiv 2 k_1 \cdot k_3 = 2 k_2 \cdot k_4$$

Furthermore we use the shorthand  $(l_i)^2$  to represent the lorentz square:  $(l_i)^2 = l_i \cdot l_i$ .

The total numerator  $\mathcal{N}_{36}$  is given by summing over the following terms, distinguished here by explicit dependence on loop momenta:  $\mathcal{N}_{36} = \sum_{i=0}^8 \mathcal{N}_{36}^{(i)}$ :

#### ■ $\mathcal{N}_{36}^{(0)}$

$$t^4 (t + 2u)^2$$

#### ■ $\mathcal{N}_{36}^{(1)}$

$$-2 t^3 (t + 2u) (-s (\tau_{3,5} + \tau_{3,6}) + \tau_{2,7} (t + 3u) - u \tau_{1,5} - 2u \tau_{1,6} + u \tau_{2,5})$$

■  $N_{36}^{(2)}$

$$\begin{aligned}
& \frac{1}{4} \left( -8 t^2 \tau_{1,6}^2 (s^2 - 3 u^2) + 4 t^2 \tau_{2,7}^2 (4 s^2 - 3 t^2 + 9 u^2) - \right. \\
& \quad 4 t^2 \tau_{3,5}^2 (-s^2 + t^2 + u^2) - 4 t^2 \tau_{3,6}^2 (-s^2 + t^2 + u^2) - 8 t^2 \tau_{3,5} \tau_{3,6} (-s^2 + t^2 + u^2) - \\
& \quad \left. 8 t^2 \tau_{1,5} \left( -\frac{1}{2} \tau_{2,7} (s^2 + t^2 - 7 u^2) + \tau_{1,6} (s^2 - 3 u^2) - \tau_{2,5} (s^2 - 2 u^2) - s (\tau_{3,6} (t + 3 u) + u \tau_{3,5}) \right) + \right. \\
& \quad 4 t^2 \tau_{1,6} (-\tau_{2,7} (s^2 - 3 t^2 + 15 u^2) + 2 \tau_{2,5} (s^2 - 3 u^2) + 2 s (\tau_{3,6} (t + 4 u) + 2 u \tau_{3,5})) - \\
& \quad 2 t u \tau_{1,5}^2 (-s^2 + t^2 + u^2) - 2 t u \tau_{2,5}^2 (-s^2 + t^2 + u^2) - 2 t u \tau_{3,5}^2 (-s^2 + t^2 + u^2) - 2 t u \tau_{3,6}^2 (-s^2 + t^2 + u^2) - \\
& \quad 4 t u \tau_{3,5} \tau_{3,6} (-s^2 + t^2 + u^2) + 4 t \tau_{2,5} (s^2 - t^2 - u^2) (\tau_{2,7} (2 t + 5 u) - s (\tau_{3,5} + \tau_{3,6})) - \\
& \quad 8 s t^2 \tau_{2,7} (\tau_{3,5} + \tau_{3,6}) (2 t + 5 u) + 4 t^4 \tau_{3,5}^2 + 4 t^4 \tau_{3,6}^2 + 8 t^4 \tau_{3,5} \tau_{3,6} + 10 l_7^2 t^2 u (-s^2 + t^2 + u^2) + \\
& \quad \left. 6 l_7^2 t u^2 (-s^2 + t^2 + u^2) + 3 l_7^2 u^3 (-s^2 + t^2 + u^2) + 9 l_7^2 t^3 (-s^2 + t^2 + u^2) - 6 l_7^2 t^5 - 16 l_8^2 t^5 - 2 l_7^2 u^5 \right)
\end{aligned}$$

■  $N_{36}^{(3)}$ 

$$\begin{aligned}
& \frac{1}{4} (-8 \tau_{1,8} l_6^2 t^4 - 8 \tau_{2,8} l_6^2 t^4 + 4 \tau_{2,13} l_6^2 t^4 - 8 \tau_{3,8} l_6^2 t^4 - 8 \tau_{1,14} l_7^2 t^4 + 8 \tau_{1,15} l_7^2 t^4 + 4 \tau_{3,9} l_7^2 t^4 + 10 \tau_{3,11} l_7^2 t^4 - 2 \tau_{3,14} l_7^2 t^4 + \\
& 10 \tau_{3,15} l_7^2 t^4 + 12 \tau_{4,9} l_7^2 t^4 + 16 \tau_{4,11} l_7^2 t^4 - 28 \tau_{2,6} l_8^2 t^4 - 24 \tau_{2,10} l_8^2 t^4 + 8 \tau_{3,13} l_8^2 t^4 - 32 \tau_{4,6} l_8^2 t^4 - 48 \tau_{4,10} l_8^2 t^4 + \\
& 16 \tau_{4,13} l_8^2 t^4 + 8 \tau_{1,8} l_{11}^2 t^4 - 4 \tau_{2,13} l_{11}^2 t^4 + 8 \tau_{3,8} l_{11}^2 t^4 + 12 (-s^2 + t^2 + u^2) \tau_{1,8} l_6^2 t^2 + 4 (-s^2 + t^2 + u^2) \tau_{1,10} l_6^2 t^2 + \\
& 12 (-s^2 + t^2 + u^2) \tau_{2,8} l_6^2 t^2 + 4 (-s^2 + t^2 + u^2) \tau_{2,10} l_6^2 t^2 - 8 (-s^2 + t^2 + u^2) \tau_{2,13} l_6^2 t^2 + 16 (-s^2 + t^2 + u^2) \tau_{3,8} l_6^2 t^2 + \\
& 8 (-s^2 + t^2 + u^2) \tau_{1,14} l_7^2 t^2 - 18 (-s^2 + t^2 + u^2) \tau_{1,15} l_7^2 t^2 - 6 (-s^2 + t^2 + u^2) \tau_{3,9} l_7^2 t^2 - 14 (-s^2 + t^2 + u^2) \tau_{3,11} l_7^2 t^2 - \\
& 2 (-s^2 + t^2 + u^2) \tau_{3,14} l_7^2 t^2 - 14 (-s^2 + t^2 + u^2) \tau_{3,15} l_7^2 t^2 - 16 (-s^2 + t^2 + u^2) \tau_{4,9} l_7^2 t^2 - 16 (-s^2 + t^2 + u^2) \tau_{4,11} l_7^2 t^2 + \\
& 4 (-s^2 + t^2 + u^2) \tau_{2,6} l_8^2 t^2 + 4 (-s^2 + t^2 + u^2) \tau_{3,6} l_8^2 t^2 - 4 (-s^2 + t^2 + u^2) \tau_{3,13} l_8^2 t^2 - 8 (-s^2 + t^2 + u^2) \tau_{4,6} l_8^2 t^2 - \\
& 8 (-s^2 + t^2 + u^2) \tau_{4,13} l_8^2 t^2 - 8 (-s^2 + t^2 + u^2) \tau_{1,8} l_{11}^2 t^2 - 4 (-s^2 + t^2 + u^2) \tau_{2,10} l_{11}^2 t^2 + 4 (-s^2 + t^2 + u^2) \tau_{2,13} l_{11}^2 t^2 - \\
& 12 (-s^2 + t^2 + u^2) \tau_{3,8} l_{11}^2 t^2 + 4 s^2 (\tau_{1,9} + 2 \tau_{1,10}) l_{13}^2 t^2 + 8 (-s^2 + t^2 + u^2) \tau_{1,6}^3 t - 8 s^2 \tau_{2,7} (\tau_{3,5} + \tau_{3,6})^2 t + \\
& 8 s (t + 4 u) \tau_{2,7}^2 (\tau_{3,5} + \tau_{3,6}) t - 4 \tau_{1,6}^2 (3 (-s^2 + t^2 + u^2) \tau_{2,5} + (-5 s^2 + 3 t^2 + 9 u^2) \tau_{2,7} + 2 s (t \tau_{3,5} + (t - 2 u) \tau_{3,6})) t + \\
& 4 \tau_{1,5} (2 \tau_{3,6} (\tau_{3,5} + \tau_{3,6}) s^2 + 2 \tau_{2,7} ((t - u) \tau_{3,5} - 4 u \tau_{3,6}) s + 3 (-s^2 + t^2 + u^2) \tau_{1,6}^2 + (-s^2 + t^2 + u^2) \tau_{2,5}^2 + \\
& (-3 s^2 + t^2 + 5 u^2) \tau_{2,7}^2 + 2 \tau_{1,6} (2 (s^2 - t^2 - u^2) \tau_{2,5} + (3 s^2 - 2 (t^2 + 2 u^2)) \tau_{2,7} - s (t \tau_{3,5} + (t - 3 u) \tau_{3,6})) + \\
& 2 \tau_{2,5} ((-2 s^2 + t^2 + 3 u^2) \tau_{2,7} + s (t \tau_{3,5} + (t - u) \tau_{3,6}))) t + 12 u (-s^2 + t^2 + u^2) \tau_{1,8} l_6^2 t + \\
& 10 u (-s^2 + t^2 + u^2) \tau_{1,10} l_6^2 t + 11 u (-s^2 + t^2 + u^2) \tau_{2,8} l_6^2 t + 12 u (-s^2 + t^2 + u^2) \tau_{2,10} l_6^2 t - \\
& 11 u (-s^2 + t^2 + u^2) \tau_{2,13} l_6^2 t + 24 u (-s^2 + t^2 + u^2) \tau_{3,8} l_6^2 t - 30 u (-s^2 + t^2 + u^2) \tau_{1,15} l_7^2 t - \\
& 6 u (-s^2 + t^2 + u^2) \tau_{3,9} l_7^2 t - 18 u (-s^2 + t^2 + u^2) \tau_{3,11} l_7^2 t - 12 u (-s^2 + t^2 + u^2) \tau_{3,14} l_7^2 t - \\
& 18 u (-s^2 + t^2 + u^2) \tau_{3,15} l_7^2 t - 12 u (-s^2 + t^2 + u^2) \tau_{4,9} l_7^2 t - 12 u (-s^2 + t^2 + u^2) \tau_{4,11} l_7^2 t - \\
& 6 u (-s^2 + t^2 + u^2) \tau_{4,14} l_7^2 t + 2 u (-s^2 + t^2 + u^2) \tau_{2,6} l_8^2 t + 4 u (-s^2 + t^2 + u^2) \tau_{3,6} l_8^2 t - 4 u (-s^2 + t^2 + u^2) \tau_{1,8} l_{11}^2 t - \\
& 8 u (-s^2 + t^2 + u^2) \tau_{2,10} l_{11}^2 t + 2 u (-s^2 + t^2 + u^2) \tau_{2,13} l_{11}^2 t - 12 u (-s^2 + t^2 + u^2) \tau_{3,8} l_{11}^2 t + \\
& 4 \tau_{1,6} ((-s^2 + t^2 + u^2) \tau_{2,5}^2 + 2 ((-2 s^2 + t^2 + 5 u^2) \tau_{2,7} + s (t \tau_{3,5} + (t - u) \tau_{3,6})) \tau_{2,5} + \\
& 2 ((\tau_{3,6} (\tau_{3,5} + \tau_{3,6}) + t l_{13}^2) s^2 + \tau_{2,7} ((t - 3 u) \tau_{3,5} - 6 u \tau_{3,6}) s - (s^2 - 6 u^2) \tau_{2,7}^2)) t + \\
& 4 (t + 3 u) (-s^2 + t^2 + u^2) \tau_{2,7}^3 + 4 u (-s^2 + t^2 + u^2) \tau_{2,5}^2 \tau_{2,7} + 4 (s^2 - t^2 - u^2) \tau_{1,5}^2 (t (-\tau_{1,6} + \tau_{2,5} + \tau_{2,7}) + s \tau_{3,6}) + \\
& 4 (s^2 - t^2 - u^2) \tau_{2,5} \tau_{2,7} (2 s (\tau_{3,5} + \tau_{3,6}) - (t + 4 u) \tau_{2,7}) + 4 u^2 (-s^2 + t^2 + u^2) \tau_{1,8} l_6^2 - 4 u^4 \tau_{1,10} l_6^2 + \\
& 8 u^2 (-s^2 + t^2 + u^2) \tau_{1,10} l_6^2 + 2 u^4 \tau_{2,8} l_6^2 + 2 u^2 (-s^2 + t^2 + u^2) \tau_{2,8} l_6^2 - 8 u^4 \tau_{2,10} l_6^2 + 12 u^2 (-s^2 + t^2 + u^2) \tau_{2,10} l_6^2 + \\
& 2 u^4 \tau_{2,13} l_6^2 - 6 u^2 (-s^2 + t^2 + u^2) \tau_{2,13} l_6^2 - 8 u^4 \tau_{3,8} l_6^2 + 16 u^2 (-s^2 + t^2 + u^2) \tau_{3,8} l_6^2 + 8 u^4 \tau_{1,14} l_7^2 - \\
& 8 u^2 (-s^2 + t^2 + u^2) \tau_{1,14} l_7^2 + 12 u^4 \tau_{1,15} l_7^2 - 22 u^2 (-s^2 + t^2 + u^2) \tau_{1,15} l_7^2 - 2 u^2 (-s^2 + t^2 + u^2) \tau_{3,9} l_7^2 + \\
& 10 u^4 \tau_{3,11} l_7^2 - 14 u^2 (-s^2 + t^2 + u^2) \tau_{3,11} l_7^2 + 10 u^4 \tau_{3,14} l_7^2 - 14 u^2 (-s^2 + t^2 + u^2) \tau_{3,14} l_7^2 + \\
& 10 u^4 \tau_{3,15} l_7^2 - 14 u^2 (-s^2 + t^2 + u^2) \tau_{3,15} l_7^2 - 4 u^4 \tau_{4,9} l_7^2 + 8 u^4 \tau_{4,11} l_7^2 - 8 u^2 (-s^2 + t^2 + u^2) \tau_{4,11} l_7^2 + \\
& 12 u^4 \tau_{4,14} l_7^2 - 12 u^2 (-s^2 + t^2 + u^2) \tau_{4,14} l_7^2 - 4 u^2 (-s^2 + t^2 + u^2) \tau_{2,10} l_{11}^2 - 4 u^2 (-s^2 + t^2 + u^2) \tau_{3,8} l_{11}^2)
\end{aligned}$$

■  $N_{36}^{(4)}$ 

$$\begin{aligned}
& \frac{1}{4} (-8 \tau_{9,15} l_7^2 t^4 - 4 \tau_{8,13} l_{11}^2 t^4 - 4 l_7^2 l_{11}^2 t^4 + 2 l_6^2 l_{13}^2 t^4 + 4 l_{11}^2 l_{14}^2 t^4 - 3 l_{11}^2 l_{15}^2 t^4 - 8 \tau_{1,8}^2 l_6^2 t^3 - 8 \tau_{2,8}^2 l_6^2 t^3 + 8 \tau_{1,8} \tau_{1,10} l_6^2 t^3 - \\
& 16 \tau_{1,8} \tau_{2,8} l_6^2 t^3 + 8 \tau_{1,10} \tau_{2,8} l_6^2 t^3 + 8 \tau_{1,8} \tau_{2,10} l_6^2 t^3 + 8 \tau_{2,8} \tau_{2,10} l_6^2 t^3 - 8 \tau_{1,8} \tau_{3,8} l_6^2 t^3 + 8 \tau_{1,10} \tau_{3,8} l_6^2 t^3 - \\
& 8 \tau_{2,8} \tau_{3,8} l_6^2 t^3 + 8 \tau_{2,10} \tau_{3,8} l_6^2 t^3 - 8 \tau_{1,8} \tau_{3,13} l_6^2 t^3 + 8 \tau_{1,10} \tau_{3,13} l_6^2 t^3 - 8 \tau_{2,8} \tau_{3,13} l_6^2 t^3 + 8 \tau_{2,10} \tau_{3,13} l_6^2 t^3 - \\
& 4 \tau_{1,14}^2 l_7^2 t^3 - 2 \tau_{3,11}^2 l_7^2 t^3 - 4 \tau_{3,14}^2 l_7^2 t^3 - 6 \tau_{3,15}^2 l_7^2 t^3 - 8 \tau_{4,9}^2 l_7^2 t^3 - 6 \tau_{4,11}^2 l_7^2 t^3 - 4 \tau_{4,14}^2 l_7^2 t^3 - \\
& 4 \tau_{1,14} \tau_{1,15} l_7^2 t^3 + 4 \tau_{1,14} \tau_{3,9} l_7^2 t^3 + 4 \tau_{1,14} \tau_{3,11} l_7^2 t^3 - 4 \tau_{1,15} \tau_{3,11} l_7^2 t^3 - 4 \tau_{3,9} \tau_{3,11} l_7^2 t^3 - 8 \tau_{1,14} \tau_{3,14} l_7^2 t^3 - \\
& 4 \tau_{1,15} \tau_{3,14} l_7^2 t^3 - 8 \tau_{1,14} \tau_{3,15} l_7^2 t^3 - 12 \tau_{1,15} \tau_{3,15} l_7^2 t^3 - 4 \tau_{3,9} \tau_{3,15} l_7^2 t^3 - 8 \tau_{3,11} \tau_{3,15} l_7^2 t^3 - 4 \tau_{3,14} \tau_{3,15} l_7^2 t^3 + \\
& 16 \tau_{1,14} \tau_{4,9} l_7^2 t^3 + 4 \tau_{1,15} \tau_{4,9} l_7^2 t^3 - 4 \tau_{3,9} \tau_{4,9} l_7^2 t^3 - 8 \tau_{3,11} \tau_{4,9} l_7^2 t^3 + 8 \tau_{3,14} \tau_{4,9} l_7^2 t^3 - 8 \tau_{3,15} \tau_{4,9} l_7^2 t^3 + \\
& 16 \tau_{1,14} \tau_{4,11} l_7^2 t^3 - 8 \tau_{3,9} \tau_{4,11} l_7^2 t^3 - 8 \tau_{3,11} \tau_{4,11} l_7^2 t^3 + 8 \tau_{3,14} \tau_{4,11} l_7^2 t^3 - 8 \tau_{3,15} \tau_{4,11} l_7^2 t^3 - 20 \tau_{4,9} \tau_{4,11} l_7^2 t^3 - \\
& 8 \tau_{1,14} \tau_{4,14} l_7^2 t^3 - 8 \tau_{1,15} \tau_{4,14} l_7^2 t^3 + 4 \tau_{3,9} \tau_{4,14} l_7^2 t^3 - 8 \tau_{3,14} \tau_{4,14} l_7^2 t^3 - 8 \tau_{3,15} \tau_{4,14} l_7^2 t^3 + 8 \tau_{4,9} \tau_{4,14} l_7^2 t^3 + \\
& 8 \tau_{4,11} \tau_{4,14} l_7^2 t^3 - 16 \tau_{2,6}^2 l_8^2 t^3 - 16 \tau_{2,10}^2 l_8^2 t^3 - 24 \tau_{4,6}^2 l_8^2 t^3 - 48 \tau_{4,10}^2 l_8^2 t^3 - 8 \tau_{4,13}^2 l_8^2 t^3 - 32 \tau_{2,6} \tau_{2,10} l_8^2 t^3 - \\
& 40 \tau_{2,6} \tau_{4,6} l_8^2 t^3 - 40 \tau_{2,10} \tau_{4,6} l_8^2 t^3 + 8 \tau_{3,13} \tau_{4,6} l_8^2 t^3 - 56 \tau_{2,6} \tau_{4,10} l_8^2 t^3 - 48 \tau_{2,10} \tau_{4,10} l_8^2 t^3 + 16 \tau_{3,13} \tau_{4,10} l_8^2 t^3 - \\
& 64 \tau_{4,6} \tau_{4,10} l_8^2 t^3 + 16 \tau_{2,6} \tau_{4,13} l_8^2 t^3 + 8 \tau_{2,10} \tau_{4,13} l_8^2 t^3 - 8 \tau_{3,13} \tau_{4,13} l_8^2 t^3 + 16 \tau_{4,6} \tau_{4,13} l_8^2 t^3 + 32 \tau_{4,10} \tau_{4,13} l_8^2 t^3 + \\
& 8 \tau_{1,8}^2 l_{11}^2 t^3 - 8 \tau_{1,8} \tau_{1,10} l_{11}^2 t^3 - 8 \tau_{1,8} \tau_{2,13} l_{11}^2 t^3 + 8 \tau_{1,10} \tau_{2,13} l_{11}^2 t^3 + 8 \tau_{1,8} \tau_{3,8} l_{11}^2 t^3 - 8 \tau_{1,10} \tau_{3,8} l_{11}^2 t^3 - \\
& 8 \tau_{2,10} \tau_{3,13} l_{11}^2 t^3 + 8 \tau_{1,9} \tau_{2,9} l_{13}^2 t^3 + 16 \tau_{1,10} \tau_{2,9} l_{13}^2 t^3 + 8 \tau_{1,10} \tau_{2,10} l_{13}^2 t^3 + 8 \tau_{2,9} \tau_{2,10} l_{13}^2 t^3 - 8 \tau_{1,9} \tau_{3,6} l_{13}^2 t^3 - \\
& 16 \tau_{1,10} \tau_{3,6} l_{13}^2 t^3 - 8 \tau_{2,10} \tau_{3,9} l_{13}^2 t^3 + 4 \tau_{1,6}^4 t^2 + 12 (-s^2 + t^2 + u^2) \tau_{9,15} l_7^2 t^2 + 4 (-s^2 + t^2 + u^2) \tau_{8,13} l_{11}^2 t^2 + \\
& 10 (-s^2 + t^2 + u^2) l_7^2 l_{11}^2 t^2 + 10 (-s^2 + t^2 + u^2) l_6^2 l_{13}^2 t^2 - 4 (-s^2 + t^2 + u^2) l_{11}^2 l_{14}^2 t^2 + (-s^2 + t^2 + u^2) l_{11}^2 l_{15}^2 t^2 - \\
& 8 \tau_{1,6}^3 (t \tau_{2,5} + (t - u) \tau_{2,7} + s \tau_{3,6}) t + 10 (-s^2 + t^2 + u^2) \tau_{1,8}^2 l_6^2 t - 4 (-s^2 + t^2 + u^2) \tau_{1,10}^2 l_6^2 t + \\
& 8 (-s^2 + t^2 + u^2) \tau_{2,8}^2 l_6^2 t - 4 (-s^2 + t^2 + u^2) \tau_{2,10}^2 l_6^2 t - 6 (-s^2 + t^2 + u^2) \tau_{1,8} \tau_{1,10} l_6^2 t + 18 (-s^2 + t^2 + u^2) \tau_{1,8} \tau_{2,8} l_6^2 t - \\
& 6 (-s^2 + t^2 + u^2) \tau_{1,10} \tau_{2,8} l_6^2 t - 4 (-s^2 + t^2 + u^2) \tau_{1,8} \tau_{2,10} l_6^2 t - 8 (-s^2 + t^2 + u^2) \tau_{1,10} \tau_{2,10} l_6^2 t - \\
& 4 (-s^2 + t^2 + u^2) \tau_{2,8} \tau_{2,10} l_6^2 t - 2 (-s^2 + t^2 + u^2) \tau_{1,8} \tau_{2,13} l_6^2 t + 2 (-s^2 + t^2 + u^2) \tau_{1,10} \tau_{2,13} l_6^2 t + \\
& 14 (-s^2 + t^2 + u^2) \tau_{1,8} \tau_{3,8} l_6^2 t - 14 (-s^2 + t^2 + u^2) \tau_{1,10} \tau_{3,8} l_6^2 t + 12 (-s^2 + t^2 + u^2) \tau_{2,8} \tau_{3,8} l_6^2 t - \\
& 12 (-s^2 + t^2 + u^2) \tau_{2,10} \tau_{3,8} l_6^2 t + 10 (-s^2 + t^2 + u^2) \tau_{1,8} \tau_{3,13} l_6^2 t - 10 (-s^2 + t^2 + u^2) \tau_{1,10} \tau_{3,13} l_6^2 t + \\
& 12 (-s^2 + t^2 + u^2) \tau_{2,8} \tau_{3,13} l_6^2 t - 12 (-s^2 + t^2 + u^2) \tau_{2,10} \tau_{3,13} l_6^2 t + 6 (-s^2 + t^2 + u^2) \tau_{1,14}^2 l_7^2 t + \\
& (-s^2 + t^2 + u^2) \tau_{3,11}^2 l_7^2 t + 10 (-s^2 + t^2 + u^2) \tau_{3,14}^2 l_7^2 t + 9 (-s^2 + t^2 + u^2) \tau_{3,15}^2 l_7^2 t + 12 (-s^2 + t^2 + u^2) \tau_{4,9}^2 l_7^2 t - \\
& 5 (-s^2 + t^2 + u^2) \tau_{4,11}^2 l_7^2 t + 10 (-s^2 + t^2 + u^2) \tau_{4,14}^2 l_7^2 t + 6 (-s^2 + t^2 + u^2) \tau_{1,14} \tau_{1,15} l_7^2 t - 6 (-s^2 + t^2 + u^2) \tau_{1,14} \tau_{3,9} l_7^2 t + \\
& 4 (-s^2 + t^2 + u^2) \tau_{1,14} \tau_{3,11} l_7^2 t + 10 (-s^2 + t^2 + u^2) \tau_{1,15} \tau_{3,11} l_7^2 t + 2 (-s^2 + t^2 + u^2) \tau_{3,9} \tau_{3,11} l_7^2 t + \\
& 16 (-s^2 + t^2 + u^2) \tau_{1,14} \tau_{3,14} l_7^2 t + 12 (-s^2 + t^2 + u^2) \tau_{1,15} \tau_{3,14} l_7^2 t - 2 (-s^2 + t^2 + u^2) \tau_{3,9} \tau_{3,14} l_7^2 t + \\
& 8 (-s^2 + t^2 + u^2) \tau_{3,11} \tau_{3,14} l_7^2 t + 18 (-s^2 + t^2 + u^2) \tau_{1,14} \tau_{3,15} l_7^2 t + 20 (-s^2 + t^2 + u^2) \tau_{1,15} \tau_{3,15} l_7^2 t + \\
& 4 (-s^2 + t^2 + u^2) \tau_{3,9} \tau_{3,15} l_7^2 t + 12 (-s^2 + t^2 + u^2) \tau_{3,11} \tau_{3,15} l_7^2 t + 18 (-s^2 + t^2 + u^2) \tau_{3,14} \tau_{3,15} l_7^2 t - \\
& 24 (-s^2 + t^2 + u^2) \tau_{1,14} \tau_{4,9} l_7^2 t - 6 (-s^2 + t^2 + u^2) \tau_{1,15} \tau_{4,9} l_7^2 t + 6 (-s^2 + t^2 + u^2) \tau_{3,9} \tau_{4,9} l_7^2 t + \\
& 2 (-s^2 + t^2 + u^2) \tau_{3,11} \tau_{4,9} l_7^2 t - 16 (-s^2 + t^2 + u^2) \tau_{3,14} \tau_{4,9} l_7^2 t + 2 (-s^2 + t^2 + u^2) \tau_{3,15} \tau_{4,9} l_7^2 t -
\end{aligned}$$

$$\begin{aligned}
& 8(-s^2 + t^2 + u^2) \tau_{1,14} \tau_{4,11} l_7^2 t + 4(-s^2 + t^2 + u^2) \tau_{1,15} \tau_{4,11} l_7^2 t + 8(-s^2 + t^2 + u^2) \tau_{3,9} \tau_{4,11} l_7^2 t - \\
& 2(-s^2 + t^2 + u^2) \tau_{3,14} \tau_{4,11} l_7^2 t + 2(-s^2 + t^2 + u^2) \tau_{3,15} \tau_{4,11} l_7^2 t + 14(-s^2 + t^2 + u^2) \tau_{4,9} \tau_{4,11} l_7^2 t + \\
& 18(-s^2 + t^2 + u^2) \tau_{1,14} \tau_{4,14} l_7^2 t + 14(-s^2 + t^2 + u^2) \tau_{1,15} \tau_{4,14} l_7^2 t - 4(-s^2 + t^2 + u^2) \tau_{3,9} \tau_{4,14} l_7^2 t + \\
& 6(-s^2 + t^2 + u^2) \tau_{3,11} \tau_{4,14} l_7^2 t + 22(-s^2 + t^2 + u^2) \tau_{3,14} \tau_{4,14} l_7^2 t + 16(-s^2 + t^2 + u^2) \tau_{3,15} \tau_{4,14} l_7^2 t - \\
& 18(-s^2 + t^2 + u^2) \tau_{4,9} \tau_{4,14} l_7^2 t - 10(-s^2 + t^2 + u^2) \tau_{4,11} \tau_{4,14} l_7^2 t + 12u(-s^2 + t^2 + u^2) \tau_{9,15} l_7^2 t - \\
& 12(-s^2 + t^2 + u^2) \tau_{4,6}^2 l_8^2 t + 4(-s^2 + t^2 + u^2) \tau_{4,13}^2 l_8^2 t - 8(-s^2 + t^2 + u^2) \tau_{2,6} \tau_{4,6} l_8^2 t - 8(-s^2 + t^2 + u^2) \tau_{2,10} \tau_{4,6} l_8^2 t + \\
& 4(-s^2 + t^2 + u^2) \tau_{3,6} \tau_{4,6} l_8^2 t - 4(-s^2 + t^2 + u^2) \tau_{3,13} \tau_{4,6} l_8^2 t + 8(-s^2 + t^2 + u^2) \tau_{2,6} \tau_{4,10} l_8^2 t + \\
& 8(-s^2 + t^2 + u^2) \tau_{3,6} \tau_{4,10} l_8^2 t - 8(-s^2 + t^2 + u^2) \tau_{3,13} \tau_{4,10} l_8^2 t - 16(-s^2 + t^2 + u^2) \tau_{4,6} \tau_{4,10} l_8^2 t - \\
& 16(-s^2 + t^2 + u^2) \tau_{2,6} \tau_{4,13} l_8^2 t - 8(-s^2 + t^2 + u^2) \tau_{2,10} \tau_{4,13} l_8^2 t - 4(-s^2 + t^2 + u^2) \tau_{3,6} \tau_{4,13} l_8^2 t + \\
& 4(-s^2 + t^2 + u^2) \tau_{3,13} \tau_{4,13} l_8^2 t - 8(-s^2 + t^2 + u^2) \tau_{4,6} \tau_{4,13} l_8^2 t - 16(-s^2 + t^2 + u^2) \tau_{4,10} \tau_{4,13} l_8^2 t - \\
& 4(-s^2 + t^2 + u^2) \tau_{1,8}^2 l_{11}^2 t + 4(-s^2 + t^2 + u^2) \tau_{1,8} \tau_{1,10} l_{11}^2 t - 4(-s^2 + t^2 + u^2) \tau_{1,8} \tau_{2,10} l_{11}^2 t + \\
& 4(-s^2 + t^2 + u^2) \tau_{1,8} \tau_{2,13} l_{11}^2 t - 4(-s^2 + t^2 + u^2) \tau_{1,10} \tau_{2,13} l_{11}^2 t + 4(-s^2 + t^2 + u^2) \tau_{2,10} \tau_{2,13} l_{11}^2 t - \\
& 8(-s^2 + t^2 + u^2) \tau_{1,8} \tau_{3,8} l_{11}^2 t + 8(-s^2 + t^2 + u^2) \tau_{1,10} \tau_{3,8} l_{11}^2 t + 8(-s^2 + t^2 + u^2) \tau_{2,10} \tau_{3,13} l_{11}^2 t + \\
& 2u(-s^2 + t^2 + u^2) \tau_{8,13} l_{11}^2 t + 12u(-s^2 + t^2 + u^2) l_7^2 l_{11}^2 t - 4(-s^2 + t^2 + u^2) \tau_{1,10}^2 l_{13}^2 t - 4(-s^2 + t^2 + u^2) \tau_{2,10}^2 l_{13}^2 t - \\
& 4(-s^2 + t^2 + u^2) \tau_{1,9} \tau_{2,9} l_{13}^2 t - 8(-s^2 + t^2 + u^2) \tau_{1,10} \tau_{2,9} l_{13}^2 t - 16(-s^2 + t^2 + u^2) \tau_{1,10} \tau_{2,10} l_{13}^2 t + \\
& 8(-s^2 + t^2 + u^2) \tau_{1,9} \tau_{3,6} l_{13}^2 t + 16(-s^2 + t^2 + u^2) \tau_{1,10} \tau_{3,6} l_{13}^2 t + 8(-s^2 + t^2 + u^2) \tau_{2,10} \tau_{3,9} l_{13}^2 t + \\
& 22u(-s^2 + t^2 + u^2) l_6^2 l_{13}^2 t - 2u(-s^2 + t^2 + u^2) l_{11}^2 l_{14}^2 t + 4u^2 \tau_{2,7}^4 + 4u^2 \tau_{2,5}^2 \tau_{2,7}^2 + 4s^2 \tau_{2,7}^2 (\tau_{3,5} + \tau_{3,6})^2 + \\
& 4\tau_{1,5}^2 (t(-\tau_{1,6} + \tau_{2,5} + \tau_{2,7}) + s\tau_{3,6})^2 - 8su\tau_{2,7}^3 (\tau_{3,5} + \tau_{3,6}) + 8u\tau_{2,5} \tau_{2,7}^2 (u\tau_{2,7} - s(\tau_{3,5} + \tau_{3,6})) + \\
& 8\tau_{1,5} (t\tau_{1,6} - t(\tau_{2,5} + \tau_{2,7}) - s\tau_{3,6}) (t\tau_{1,6}^2 - (t\tau_{2,5} + (t-u)\tau_{2,7} + s\tau_{3,6}) \tau_{1,6} + \tau_{2,7} (s(\tau_{3,5} + \tau_{3,6}) - u(\tau_{2,5} + \tau_{2,7}))) + \\
& 6u(-s^2 + t^2 + u^2) \tau_{1,8}^2 l_6^2 + 4u^3 \tau_{1,10}^2 l_6^2 - 6u(-s^2 + t^2 + u^2) \tau_{1,10}^2 l_6^2 + 4u^3 \tau_{2,8}^2 l_6^2 + 2u(-s^2 + t^2 + u^2) \tau_{2,8}^2 l_6^2 + \\
& 8u^3 \tau_{2,10}^2 l_6^2 - 8u(-s^2 + t^2 + u^2) \tau_{2,10}^2 l_6^2 - 2u(-s^2 + t^2 + u^2) \tau_{1,8} \tau_{1,10} l_6^2 + 4u^3 \tau_{1,8} \tau_{2,8} l_6^2 + 8u(-s^2 + t^2 + u^2) \tau_{1,8} \tau_{2,8} l_6^2 - \\
& 4u^3 \tau_{1,10} \tau_{2,8} l_6^2 - 12u^3 \tau_{1,8} \tau_{2,10} l_6^2 + 6u(-s^2 + t^2 + u^2) \tau_{1,8} \tau_{2,10} l_6^2 + 12u^3 \tau_{1,10} \tau_{2,10} l_6^2 - 14u(-s^2 + t^2 + u^2) \tau_{1,10} \tau_{2,10} l_6^2 - \\
& 12u^3 \tau_{2,8} \tau_{2,10} l_6^2 + 6u(-s^2 + t^2 + u^2) \tau_{2,8} \tau_{2,10} l_6^2 - 2u(-s^2 + t^2 + u^2) \tau_{1,8} \tau_{2,13} l_6^2 + 2u(-s^2 + t^2 + u^2) \tau_{1,10} \tau_{2,13} l_6^2 - \\
& 4u^3 \tau_{2,8} \tau_{2,13} l_6^2 + 2u(-s^2 + t^2 + u^2) \tau_{2,8} \tau_{2,13} l_6^2 + 4u^3 \tau_{2,10} \tau_{2,13} l_6^2 - 2u(-s^2 + t^2 + u^2) \tau_{2,10} \tau_{2,13} l_6^2 - \\
& 12u^3 \tau_{1,8} \tau_{3,8} l_6^2 + 16u(-s^2 + t^2 + u^2) \tau_{1,8} \tau_{3,8} l_6^2 + 12u^3 \tau_{1,10} \tau_{3,8} l_6^2 - 16u(-s^2 + t^2 + u^2) \tau_{1,10} \tau_{3,8} l_6^2 - \\
& 8u^3 \tau_{2,8} \tau_{3,8} l_6^2 + 12u(-s^2 + t^2 + u^2) \tau_{2,8} \tau_{3,8} l_6^2 + 8u^3 \tau_{2,10} \tau_{3,8} l_6^2 - 12u(-s^2 + t^2 + u^2) \tau_{2,10} \tau_{3,8} l_6^2 - \\
& 4u^3 \tau_{1,8} \tau_{3,13} l_6^2 + 8u(-s^2 + t^2 + u^2) \tau_{1,8} \tau_{3,13} l_6^2 + 4u^3 \tau_{1,10} \tau_{3,13} l_6^2 - 8u(-s^2 + t^2 + u^2) \tau_{1,10} \tau_{3,13} l_6^2 - \\
& 8u^3 \tau_{2,8} \tau_{3,13} l_6^2 + 12u(-s^2 + t^2 + u^2) \tau_{2,8} \tau_{3,13} l_6^2 + 8u^3 \tau_{2,10} \tau_{3,13} l_6^2 - 12u(-s^2 + t^2 + u^2) \tau_{2,10} \tau_{3,13} l_6^2 - \\
& 4u^3 \tau_{1,14}^2 l_7^2 + 6u(-s^2 + t^2 + u^2) \tau_{1,14}^2 l_7^2 - 6u^3 \tau_{3,11}^2 l_7^2 + 3u(-s^2 + t^2 + u^2) \tau_{3,11}^2 l_7^2 - 12u^3 \tau_{3,14}^2 l_7^2 + \\
& 14u(-s^2 + t^2 + u^2) \tau_{3,14}^2 l_7^2 - 10u^3 \tau_{3,15}^2 l_7^2 + 11u(-s^2 + t^2 + u^2) \tau_{3,15}^2 l_7^2 - 8u^3 \tau_{4,9}^2 l_7^2 + 12u(-s^2 + t^2 + u^2) \tau_{4,9}^2 l_7^2 - \\
& 2u^3 \tau_{4,11}^2 l_7^2 - 7u(-s^2 + t^2 + u^2) \tau_{4,11}^2 l_7^2 - 16u^3 \tau_{4,14}^2 l_7^2 + 16u(-s^2 + t^2 + u^2) \tau_{4,14}^2 l_7^2 - 4u^3 \tau_{1,14} \tau_{1,15} l_7^2 + \\
& 6u(-s^2 + t^2 + u^2) \tau_{1,14} \tau_{1,15} l_7^2 + 4u^3 \tau_{1,14} \tau_{3,9} l_7^2 - 6u(-s^2 + t^2 + u^2) \tau_{1,14} \tau_{3,9} l_7^2 - 16u^3 \tau_{1,14} \tau_{3,11} l_7^2 + \\
& 14u(-s^2 + t^2 + u^2) \tau_{1,14} \tau_{3,11} l_7^2 - 12u^3 \tau_{1,15} \tau_{3,11} l_7^2 + 14u(-s^2 + t^2 + u^2) \tau_{1,15} \tau_{3,11} l_7^2 + 4u^3 \tau_{3,9} \tau_{3,11} l_7^2 -
\end{aligned}$$

$$\begin{aligned}
& 2u(-s^2 + t^2 + u^2)\tau_{3,9}\tau_{3,11}l_7^2 - 16u^3\tau_{1,14}\tau_{3,14}l_7^2 + 20u(-s^2 + t^2 + u^2)\tau_{1,14}\tau_{3,14}l_7^2 - 16u^3\tau_{1,15}\tau_{3,14}l_7^2 + \\
& 18u(-s^2 + t^2 + u^2)\tau_{1,15}\tau_{3,14}l_7^2 + 4u^3\tau_{3,9}\tau_{3,14}l_7^2 - 4u(-s^2 + t^2 + u^2)\tau_{3,9}\tau_{3,14}l_7^2 - 20u^3\tau_{3,11}\tau_{3,14}l_7^2 + \\
& 18u(-s^2 + t^2 + u^2)\tau_{3,11}\tau_{3,14}l_7^2 - 20u^3\tau_{1,14}\tau_{3,15}l_7^2 + 24u(-s^2 + t^2 + u^2)\tau_{1,14}\tau_{3,15}l_7^2 - 16u^3\tau_{1,15}\tau_{3,15}l_7^2 + \\
& 22u(-s^2 + t^2 + u^2)\tau_{1,15}\tau_{3,15}l_7^2 + 2u(-s^2 + t^2 + u^2)\tau_{3,9}\tau_{3,15}l_7^2 - 20u^3\tau_{3,11}\tau_{3,15}l_7^2 + 18u(-s^2 + t^2 + u^2)\tau_{3,11}\tau_{3,15}l_7^2 - \\
& 24u^3\tau_{3,14}\tau_{3,15}l_7^2 + 28u(-s^2 + t^2 + u^2)\tau_{3,14}\tau_{3,15}l_7^2 + 16u^3\tau_{1,14}\tau_{4,9}l_7^2 - 24u(-s^2 + t^2 + u^2)\tau_{1,14}\tau_{4,9}l_7^2 + \\
& 4u^3\tau_{1,15}\tau_{4,9}l_7^2 - 6u(-s^2 + t^2 + u^2)\tau_{1,15}\tau_{4,9}l_7^2 - 4u^3\tau_{3,9}\tau_{4,9}l_7^2 + 6u(-s^2 + t^2 + u^2)\tau_{3,9}\tau_{4,9}l_7^2 + 12u^3\tau_{3,11}\tau_{4,9}l_7^2 - \\
& 8u(-s^2 + t^2 + u^2)\tau_{3,11}\tau_{4,9}l_7^2 + 16u^3\tau_{3,14}\tau_{4,9}l_7^2 - 20u(-s^2 + t^2 + u^2)\tau_{3,14}\tau_{4,9}l_7^2 + 12u^3\tau_{3,15}\tau_{4,9}l_7^2 - \\
& 8u(-s^2 + t^2 + u^2)\tau_{3,15}\tau_{4,9}l_7^2 - 16u^3\tau_{1,14}\tau_{4,11}l_7^2 + 8u(-s^2 + t^2 + u^2)\tau_{1,14}\tau_{4,11}l_7^2 - 8u^3\tau_{1,15}\tau_{4,11}l_7^2 + \\
& 8u(-s^2 + t^2 + u^2)\tau_{1,15}\tau_{4,11}l_7^2 + 4u(-s^2 + t^2 + u^2)\tau_{3,9}\tau_{4,11}l_7^2 - 8u^3\tau_{3,11}\tau_{4,11}l_7^2 - 12u^3\tau_{3,14}\tau_{4,11}l_7^2 + \\
& 8u(-s^2 + t^2 + u^2)\tau_{3,14}\tau_{4,11}l_7^2 - 12u^3\tau_{3,15}\tau_{4,11}l_7^2 + 4u(-s^2 + t^2 + u^2)\tau_{3,15}\tau_{4,11}l_7^2 + 12u^3\tau_{4,9}\tau_{4,11}l_7^2 - \\
& 2u(-s^2 + t^2 + u^2)\tau_{4,9}\tau_{4,11}l_7^2 - 20u^3\tau_{1,14}\tau_{4,14}l_7^2 + 24u(-s^2 + t^2 + u^2)\tau_{1,14}\tau_{4,14}l_7^2 - 12u^3\tau_{1,15}\tau_{4,14}l_7^2 + \\
& 16u(-s^2 + t^2 + u^2)\tau_{1,15}\tau_{4,14}l_7^2 - 2u(-s^2 + t^2 + u^2)\tau_{3,9}\tau_{4,14}l_7^2 - 24u^3\tau_{3,11}\tau_{4,14}l_7^2 + 18u(-s^2 + t^2 + u^2)\tau_{3,11}\tau_{4,14}l_7^2 - \\
& 24u^3\tau_{3,14}\tau_{4,14}l_7^2 + 30u(-s^2 + t^2 + u^2)\tau_{3,14}\tau_{4,14}l_7^2 - 24u^3\tau_{3,15}\tau_{4,14}l_7^2 + 24u(-s^2 + t^2 + u^2)\tau_{3,15}\tau_{4,14}l_7^2 + \\
& 20u^3\tau_{4,9}\tau_{4,14}l_7^2 - 24u(-s^2 + t^2 + u^2)\tau_{4,9}\tau_{4,14}l_7^2 - 20u^3\tau_{4,11}\tau_{4,14}l_7^2 + 4u(-s^2 + t^2 + u^2)\tau_{4,11}\tau_{4,14}l_7^2 + \\
& 4u^2(-s^2 + t^2 + u^2)\tau_{9,15}l_7^2 - 4u(-s^2 + t^2 + u^2)\tau_{2,6}\tau_{4,6}l_8^2 - 4u(-s^2 + t^2 + u^2)\tau_{2,10}\tau_{4,6}l_8^2 + 4u(-s^2 + t^2 + u^2)\tau_{3,6}\tau_{4,6}l_8^2 + \\
& 4u(-s^2 + t^2 + u^2)\tau_{2,6}\tau_{4,10}l_8^2 + 8u(-s^2 + t^2 + u^2)\tau_{3,6}\tau_{4,10}l_8^2 - 8u(-s^2 + t^2 + u^2)\tau_{2,6}\tau_{4,13}l_8^2 - \\
& 4u(-s^2 + t^2 + u^2)\tau_{2,10}\tau_{4,13}l_8^2 - 4u(-s^2 + t^2 + u^2)\tau_{3,6}\tau_{4,13}l_8^2 - 4u(-s^2 + t^2 + u^2)\tau_{1,8}\tau_{2,10}l_{11}^2 + \\
& 4u(-s^2 + t^2 + u^2)\tau_{2,10}\tau_{2,13}l_{11}^2 - 4u(-s^2 + t^2 + u^2)\tau_{1,8}\tau_{3,8}l_{11}^2 + 4u(-s^2 + t^2 + u^2)\tau_{1,10}\tau_{3,8}l_{11}^2 + \\
& 4u(-s^2 + t^2 + u^2)\tau_{2,10}\tau_{3,13}l_{11}^2 - 4u^4l_7^2l_{11}^2 + 6u^2(-s^2 + t^2 + u^2)l_7^2l_{11}^2 - 4u(-s^2 + t^2 + u^2)\tau_{1,10}^2l_{13}^2 - \\
& 4u(-s^2 + t^2 + u^2)\tau_{2,10}^2l_{13}^2 - 12u(-s^2 + t^2 + u^2)\tau_{1,10}\tau_{2,10}l_{13}^2 + 4u(-s^2 + t^2 + u^2)\tau_{2,9}\tau_{2,10}l_{13}^2 + \\
& 4u(-s^2 + t^2 + u^2)\tau_{1,9}\tau_{3,6}l_{13}^2 + 8u(-s^2 + t^2 + u^2)\tau_{1,10}\tau_{3,6}l_{13}^2 + 4u(-s^2 + t^2 + u^2)\tau_{2,10}\tau_{3,9}l_{13}^2 + 2u^4l_6^2l_{13}^2 + \\
& 10u^2(-s^2 + t^2 + u^2)l_6^2l_{13}^2 + 8\tau_{1,6}(\tau_{2,7}(t\tau_{2,5} + (t-u)\tau_{2,7} + s\tau_{3,6}))(u(\tau_{2,5} + \tau_{2,7}) - s(\tau_{3,5} + \tau_{3,6})) + \\
& st(t\tau_{1,9} + 2(t-u)\tau_{1,10} - 2t\tau_{2,9} - (t+4u)\tau_{2,10} - 2s\tau_{3,6})l_{13}^2 + 4\tau_{1,6}^2(t^2\tau_{2,5}^2 + 2t((t-2u)\tau_{2,7} + s\tau_{3,6})\tau_{2,5} + \\
& (3(t^2 + u^2) - 2s^2)\tau_{2,7}^2 + 2s\tau_{2,7}(t\tau_{3,5} + (2t-u)\tau_{3,6}) + s(s\tau_{3,6}^2 + 2t(2t-u)l_{13}^2)))
\end{aligned}$$

■  $N_{36}^{(5)}$

$$\begin{aligned}
& \frac{1}{4} \left( 4l_7^2((\tau_{1,15} + \tau_{3,9} + \tau_{3,11} + 2\tau_{4,9} + \tau_{4,11})\tau_{9,15} - (\tau_{1,14} + 2\tau_{1,17} + \tau_{3,6} - 2\tau_{3,12} + 2\tau_{3,14} - \tau_{3,17} + \tau_{4,6} - 2\tau_{4,12} + 2\tau_{4,14})l_{11}^2) + \right. \\
& (18\tau_{1,7} + 2\tau_{1,8} + 4\tau_{2,7} + 6\tau_{2,8} + 17\tau_{2,9} + 6\tau_{4,8})l_6^2l_{13}^2 + \\
& 14\tau_{4,9}l_6^2l_{13}^2 - (\tau_{2,10} - 3\tau_{3,6} + 2(\tau_{3,13} + \tau_{4,6} + \tau_{4,10}))l_{11}^2l_{15}^2)t^3 - \\
& 2(2l_8^2\tau_{2,6}^3 + 2\tau_{1,8}^2(\tau_{2,13} + 2\tau_{3,13})l_6^2 - 4\tau_{1,8}(\tau_{1,10} - \tau_{2,8} + \tau_{2,10})(\tau_{2,13} + 2\tau_{3,13})l_6^2 - \\
& 2\tau_{1,14}^2(\tau_{3,11} + \tau_{3,14} + \tau_{3,15} + 2\tau_{4,11})l_7^2 - 2\tau_{1,14}(2\tau_{3,14}^2 + 2(2\tau_{3,15} - \tau_{4,9} + \tau_{4,11} + \tau_{4,14})\tau_{3,14} + 2\tau_{3,15}^2 + \\
& \tau_{1,15}(2(\tau_{3,11} + \tau_{3,14} + \tau_{3,15}) + 3\tau_{4,11}) - \tau_{3,9}(\tau_{4,11} - 2\tau_{4,14}) - 2\tau_{4,11}(2\tau_{4,9} + \tau_{4,11} - \tau_{4,14}) +
\end{aligned}$$

$$\begin{aligned}
& 2 \tau_{3,11} (\tau_{3,14} + \tau_{3,15} - \tau_{4,9} - \tau_{4,11} + \tau_{4,14}) + \tau_{3,15} (-2 \tau_{4,9} + \tau_{4,11} + 2 \tau_{4,14})) l_7^2 - \\
& (2 \tau_{3,14}^3 + (6 \tau_{3,15} - 4 \tau_{4,9} + 4 \tau_{4,14}) \tau_{3,14}^2 + (5 \tau_{3,15}^2 + 8 (\tau_{4,14} - \tau_{4,9}) \tau_{3,15} + \\
& 2 (\tau_{4,9}^2 - 2 (\tau_{4,11} + \tau_{4,14}) \tau_{4,9} - 2 \tau_{4,11}^2 + \tau_{4,14}^2)) \tau_{3,14} + \tau_{3,15}^3 + 4 \tau_{3,15} \tau_{4,9}^2 - \tau_{3,15} \tau_{4,11}^2 + 4 \tau_{4,9} \tau_{4,11}^2 + \\
& 2 \tau_{3,15} \tau_{4,14}^2 + \tau_{3,11}^2 \tau_{3,15} - 2 \tau_{3,15}^2 \tau_{4,9} + 4 \tau_{4,9}^2 \tau_{4,11} + 2 \tau_{3,15} \tau_{4,9} \tau_{4,11} + \tau_{1,15}^2 (3 \tau_{3,11} + \tau_{3,14} + 4 \tau_{4,11}) + \\
& 4 \tau_{3,15}^2 \tau_{4,14} - 4 \tau_{4,11}^2 \tau_{4,14} - 4 \tau_{3,15} \tau_{4,9} \tau_{4,14} - 4 \tau_{4,9} \tau_{4,11} \tau_{4,14} - \tau_{3,9}^2 (\tau_{3,11} + \tau_{3,14} + 2 \tau_{4,14}) + \\
& 2 \tau_{3,9} (2 \tau_{4,14}^2 + (2 \tau_{3,14} + \tau_{3,15} - 2 \tau_{4,9}) \tau_{4,14} + (\tau_{3,15} + \tau_{4,11}) (\tau_{3,11} + \tau_{4,9} + \tau_{4,11})) + \tau_{3,11} \\
& (2 \tau_{3,14}^2 + 4 (\tau_{3,15} - \tau_{4,9} - \tau_{4,11} + \tau_{4,14}) \tau_{3,14} + \tau_{3,15}^2 + 2 (\tau_{4,9} - \tau_{4,14}) (\tau_{4,9} + 2 \tau_{4,11} - \tau_{4,14}) + 4 \tau_{3,15} \tau_{4,14})) + \\
& 2 \tau_{1,15} (\tau_{3,11}^2 + (2 \tau_{3,14} + \tau_{3,15} + \tau_{4,11} + 2 \tau_{4,14}) \tau_{3,11} + 2 \tau_{3,14}^2 + \tau_{3,9} (\tau_{3,11} + \tau_{4,14}) + (\tau_{3,15} + \tau_{4,11}) \\
& (\tau_{3,15} - \tau_{4,9} + 2 \tau_{4,14}) + \tau_{3,14} (3 \tau_{3,15} + 2 (-\tau_{4,9} + \tau_{4,11} + \tau_{4,14})))) l_7^2 - 2 \tau_{1,6}^2 (2 \tau_{1,6} + \tau_{1,9}) l_{13}^2 + \\
& 2 (l_8^2 \tau_{2,10}^3 + ((\tau_{2,13} + 2 \tau_{3,13}) l_6^2 + (3 \tau_{2,6} + 4 (\tau_{4,6} + \tau_{4,10})) l_8^2 + (\tau_{1,9} + 2 \tau_{3,9}) l_{13}^2) \tau_{2,10}^2 - 2 \tau_{2,8} (\tau_{2,13} + 2 \tau_{3,13}) \\
& l_6^2 \tau_{2,10} + ((3 \tau_{2,6}^2 + 8 (\tau_{4,6} + \tau_{4,10}) \tau_{2,6} + 5 \tau_{4,6}^2 + 6 \tau_{4,10}^2 + \tau_{4,13}^2 + 10 \tau_{4,6} \tau_{4,10} - 2 \tau_{4,10} \tau_{4,13})) l_8^2 + \\
& 2 (\tau_{1,6}^2 + (\tau_{3,6} - \tau_{3,9}) \tau_{1,6} - \tau_{1,9} \tau_{2,9} + \tau_{3,6} (\tau_{2,9} - \tau_{3,9})) l_{13}^2) \tau_{2,10} + \\
& \tau_{1,10}^2 (\tau_{2,13} + 2 \tau_{3,13}) l_6^2 + \tau_{2,8}^2 (\tau_{2,13} + 2 \tau_{3,13}) l_6^2 + 2 \tau_{4,6}^3 l_8^2 + 4 \tau_{4,10}^3 l_8^2 - 2 \tau_{3,13} \tau_{4,10}^2 l_8^2 + \\
& 8 \tau_{4,6} \tau_{4,10}^2 l_8^2 + 2 \tau_{4,6} \tau_{4,13}^2 l_8^2 + 2 \tau_{4,10} \tau_{4,13}^2 l_8^2 + 6 \tau_{4,6}^2 \tau_{4,10} l_8^2 - 2 \tau_{3,13} \tau_{4,6} \tau_{4,10} l_8^2 + \\
& 4 \tau_{2,6}^2 (\tau_{4,6} + \tau_{4,10}) l_8^2 - 4 \tau_{4,10}^2 \tau_{4,13} l_8^2 + 2 \tau_{3,13} \tau_{4,6} \tau_{4,13} l_8^2 + 2 \tau_{3,13} \tau_{4,10} \tau_{4,13} l_8^2 - \\
& 4 \tau_{4,6} \tau_{4,10} \tau_{4,13} l_8^2 + \tau_{2,6} (5 \tau_{4,6}^2 + 10 \tau_{4,10} \tau_{4,6} + 7 \tau_{4,10}^2 + 2 \tau_{4,13}^2 - 4 \tau_{4,10} \tau_{4,13}) l_8^2 - \\
& 2 \tau_{1,6} \tau_{3,6}^2 l_{13}^2 - \tau_{1,9} \tau_{3,6}^2 l_{13}^2 + \tau_{1,6} (4 \tau_{1,6} + 2 \tau_{1,9} - \tau_{2,9}) \tau_{2,9} l_{13}^2 - 4 \tau_{1,6}^2 \tau_{3,6} l_{13}^2 - \\
& 2 \tau_{1,6} \tau_{1,9} \tau_{3,6} l_{13}^2 + 4 \tau_{1,6} \tau_{2,9} \tau_{3,6} l_{13}^2 + 2 \tau_{1,9} \tau_{2,9} \tau_{3,6} l_{13}^2 - 2 \tau_{1,10} (\tau_{2,8} (\tau_{2,13} + 2 \tau_{3,13}) l_6^2 + \\
& (\tau_{1,6} + \tau_{3,6}) (\tau_{1,6} - 2 \tau_{2,9} + \tau_{3,6}) l_{13}^2 - \tau_{2,10} ((\tau_{2,13} + 2 \tau_{3,13}) l_6^2 + (\tau_{1,6} - \tau_{2,9} + \tau_{3,6}) l_{13}^2))) t^2 - \\
& \frac{1}{2} (-s^2 + t^2 + u^2) ((12 \tau_{1,7} - 6 \tau_{1,8} + 8 \tau_{1,9} - 2 \tau_{2,7} - 2 \tau_{2,8} + 25 \tau_{2,9} + 14 \tau_{4,8}) l_6^2 l_{13}^2 + \\
& 2 (6 \tau_{1,15} \tau_{9,15} l_7^2 + 6 \tau_{3,9} \tau_{9,15} l_7^2 + 4 \tau_{3,11} \tau_{9,15} l_7^2 - 2 \tau_{3,15} \tau_{9,15} l_7^2 + 12 \tau_{4,9} \tau_{9,15} l_7^2 + 2 \tau_{4,11} \tau_{9,15} l_7^2 - 2 \tau_{4,14} \tau_{9,15} l_7^2 - \\
& 2 \tau_{1,14} l_{11}^2 l_7^2 - 12 \tau_{1,17} l_{11}^2 l_7^2 - 2 \tau_{3,6} l_{11}^2 l_7^2 + 4 \tau_{3,12} l_{11}^2 l_7^2 - 4 \tau_{3,14} l_{11}^2 l_7^2 - 2 \tau_{4,6} l_{11}^2 l_7^2 + 2 \tau_{4,12} l_{11}^2 l_7^2 - \\
& 4 \tau_{4,14} l_{11}^2 l_7^2 + 19 \tau_{4,9} l_6^2 l_{13}^2 + (-2 \tau_{2,10} + 2 \tau_{3,6} - \tau_{4,10} + \tau_{4,13}) l_{11}^2 l_{15}^2)) t - \frac{1}{2} u (-s^2 + t^2 + u^2) \\
& (4 l_7^2 ((3 \tau_{1,15} + 3 \tau_{3,9} + \tau_{3,11} - 2 \tau_{3,15} + 6 \tau_{4,9} - \tau_{4,11} - 2 \tau_{4,14}) \tau_{9,15} - (\tau_{1,14} + 4 \tau_{1,17} - \tau_{3,6} + \tau_{3,17} - \tau_{4,6} + 2 \tau_{4,12}) l_{11}^2) + \\
& (-2 \tau_{1,7} - 2 \tau_{1,8} + 25 \tau_{1,9} + 12 \tau_{2,7} - 6 \tau_{2,8} + 8 \tau_{2,9} + 14 \tau_{4,8} + 38 \tau_{4,9}) l_6^2 l_{13}^2) + \\
& u^3 (4 l_7^2 ((\tau_{1,15} + \tau_{3,9} - \tau_{3,15} + 2 \tau_{4,9} - \tau_{4,11} - \tau_{4,14}) \tau_{9,15} + (-\tau_{1,14} + \tau_{3,6} + \tau_{4,6} - \tau_{4,12}) l_{11}^2) + \\
& (4 \tau_{1,7} + 6 \tau_{1,8} + 17 \tau_{1,9} + 2 (9 \tau_{2,7} + \tau_{2,8} + 3 \tau_{4,8} + 7 \tau_{4,9})) l_6^2 l_{13}^2) - \\
& 2 u^2 (2 l_{13}^2 \tau_{1,6}^3 + 4 \tau_{3,6} l_{13}^2 \tau_{1,6}^2 - 4 \tau_{3,6}^2 l_{13}^2 \tau_{1,6} - \tau_{2,8}^3 l_6^2 + 2 \tau_{1,8}^2 (2 \tau_{2,10} - \tau_{2,13} + 2 \tau_{3,8}) l_6^2 + \\
& \tau_{2,8}^2 (2 \tau_{2,10} + 3 \tau_{2,13} + 4 \tau_{3,13}) l_6^2 - \tau_{2,8} \tau_{2,10} (\tau_{2,10} + 6 \tau_{2,13} + 8 \tau_{3,13}) l_6^2 - \\
& 2 \tau_{1,8} ((\tau_{2,8} - \tau_{2,10}) (\tau_{2,8} - \tau_{2,10} - 2 \tau_{2,13} - \tau_{3,8} - 3 \tau_{3,13}) + \tau_{1,10} (\tau_{2,8} + \tau_{2,10} + 3 \tau_{3,8} + \tau_{3,13})) l_6^2 - \\
& 2 \tau_{1,14}^2 (\tau_{3,11} + \tau_{3,14} + \tau_{3,15} + 2 \tau_{4,11}) l_7^2 - \tau_{1,15}^2 (3 \tau_{3,11} + \tau_{3,14} + 4 \tau_{4,11}) l_7^2 -
\end{aligned}$$



$$\begin{aligned}
& 2 \tau_{1,14} (2 \tau_{3,11}^2 + (4 \tau_{3,14} + 4 \tau_{3,15} - 2 \tau_{4,9} + 3 \tau_{4,11} + 4 \tau_{4,14}) \tau_{3,11} + 2 \tau_{3,14}^2 + 2 \tau_{3,15}^2 + \\
& \quad \tau_{1,15} (2 (\tau_{3,11} + \tau_{3,14} + \tau_{3,15}) + 3 \tau_{4,11}) - \tau_{3,9} (\tau_{4,11} - 2 \tau_{4,14}) + 2 \tau_{3,15} (-\tau_{4,9} + 2 \tau_{4,11} + \tau_{4,14}) + \\
& \quad 2 \tau_{3,14} (2 \tau_{3,15} - \tau_{4,9} + 2 \tau_{4,11} + \tau_{4,14}) + \tau_{4,11} (-4 \tau_{4,9} + 2 \tau_{4,11} + 5 \tau_{4,14})) l_7^2 - \\
& 2 \tau_{1,15} (2 \tau_{3,11}^2 + (4 \tau_{3,14} + 2 \tau_{3,15} + 3 (\tau_{4,11} + \tau_{4,14})) \tau_{3,11} + 2 \tau_{3,14}^2 + \tau_{3,15}^2 + \tau_{3,9} (\tau_{3,11} + \tau_{4,14}) + \\
& \quad \tau_{4,11} (-\tau_{4,9} + \tau_{4,11} + 3 \tau_{4,14}) + \tau_{3,14} (4 \tau_{3,15} - 2 \tau_{4,9} + 5 \tau_{4,11} + 3 \tau_{4,14}) + \tau_{3,15} (2 (\tau_{4,11} + \tau_{4,14}) - \tau_{4,9})) l_7^2 + \\
& (-\tau_{3,11}^3 - (5 \tau_{3,14} + 5 \tau_{3,15} - 4 \tau_{4,9} + 2 \tau_{4,11} + 6 \tau_{4,14}) \tau_{3,11}^2 - (6 \tau_{3,14}^2 + 2 (6 \tau_{3,15} - 4 \tau_{4,9} + 3 \tau_{4,11} + 6 \tau_{4,14}) \tau_{3,14} + \\
& \quad 7 \tau_{4,14}^2 + 2 (\tau_{3,15} - \tau_{4,9}) (2 \tau_{3,15} - \tau_{4,9} + 3 \tau_{4,11}) + 4 (3 \tau_{3,15} - 2 \tau_{4,9} + 2 \tau_{4,11}) \tau_{4,14}) \tau_{3,11} - \\
& \quad 2 \tau_{3,14}^3 - \tau_{3,15}^3 + 2 \tau_{3,15}^2 (2 \tau_{4,9} - \tau_{4,11} - 2 \tau_{4,14}) + \tau_{3,9}^2 (\tau_{3,11} + \tau_{3,14} + 2 \tau_{4,14}) + \\
& \quad 2 \tau_{4,11} (\tau_{4,9} - \tau_{4,14}) (-2 \tau_{4,9} + 2 \tau_{4,11} + 3 \tau_{4,14}) + 2 \tau_{3,9} \\
& \quad (\tau_{3,11}^2 + (\tau_{3,14} + \tau_{4,11}) \tau_{3,11} - 3 \tau_{4,14}^2 - \tau_{3,15} \tau_{4,9} + (\tau_{3,14} - \tau_{4,9}) \tau_{4,11} - (2 (\tau_{3,14} + \tau_{3,15} - \tau_{4,9}) + \tau_{4,11}) \tau_{4,14}) - \\
& \quad \tau_{3,14} (\tau_{4,14}^2 + 2 (4 \tau_{3,15} - 2 \tau_{4,9} + 3 \tau_{4,11}) \tau_{4,14} + 2 (\tau_{3,15} - \tau_{4,9}) (3 \tau_{3,15} - \tau_{4,9} + 4 \tau_{4,11})) - 2 \tau_{3,14}^2 \\
& \quad (3 \tau_{3,15} + 2 (-\tau_{4,9} + \tau_{4,11} + \tau_{4,14})) - \tau_{3,15} (4 \tau_{4,9}^2 - 2 (4 \tau_{4,11} + 3 \tau_{4,14}) \tau_{4,9} + \tau_{4,11}^2 + 2 \tau_{4,14}^2 + 8 \tau_{4,11} \tau_{4,14})) \\
& \quad l_7^2 - 2 \tau_{2,6} \tau_{4,6}^2 l_8^2 + 2 \tau_{2,6} \tau_{4,10}^2 l_8^2 + 4 \tau_{3,6} \tau_{4,10}^2 l_8^2 + 4 \tau_{2,6} \tau_{4,13}^2 l_8^2 - 4 \tau_{2,6} \tau_{4,6} \tau_{4,10} l_8^2 + \\
& \quad 4 \tau_{3,6} \tau_{4,6} \tau_{4,10} l_8^2 - 4 \tau_{3,6} \tau_{4,6} \tau_{4,13} l_8^2 - 8 \tau_{2,6} \tau_{4,10} \tau_{4,13} l_8^2 - 4 \tau_{3,6} \tau_{4,10} \tau_{4,13} l_8^2 - \\
& \quad 2 \tau_{1,9} \tau_{3,6}^2 l_{13}^2 + \tau_{1,10}^2 ((\tau_{2,8} + \tau_{2,13} + 2 (\tau_{3,8} + \tau_{3,13})) l_6^2 + 2 (\tau_{1,6} + 2 \tau_{3,6}) l_{13}^2) + \\
& \quad 2 \tau_{1,10} (2 (\tau_{1,6}^2 + (\tau_{2,10} + 2 \tau_{3,6}) \tau_{1,6} + (3 \tau_{2,10} - \tau_{3,6}) \tau_{3,6}) l_{13}^2 - (\tau_{2,8} - \tau_{2,10}) (2 \tau_{2,13} + \tau_{3,8} + 3 \tau_{3,13}) l_6^2) + \\
& \quad 2 \tau_{2,10} (2 (\tau_{1,6}^2 + 4 \tau_{3,6} \tau_{1,6} - \tau_{3,6} (\tau_{2,9} + \tau_{3,9})) l_{13}^2 - (\tau_{4,6} + 2 \tau_{4,10} - \tau_{4,13}) (\tau_{4,6} + \tau_{4,13}) l_8^2) + \\
& \quad \tau_{2,10}^2 ((3 \tau_{2,13} + 4 \tau_{3,13}) l_6^2 + 2 (-\tau_{1,6} + \tau_{1,9} + 2 (\tau_{2,9} + \tau_{3,6} + \tau_{3,9})) l_{13}^2)) - \\
& 2 (s^2 - t^2 - u^2) (2 l_{13}^2 \tau_{1,6}^3 + 2 \tau_{1,8}^3 l_6^2 + \tau_{1,8}^2 (-3 \tau_{1,10} + 3 \tau_{2,8} - \tau_{2,10} + 2 (\tau_{3,8} + \tau_{3,13})) l_6^2 + \\
& \quad \tau_{1,8} (\tau_{1,10}^2 - (4 \tau_{2,8} - \tau_{2,10} + \tau_{2,13} + 3 \tau_{3,8} + 5 \tau_{3,13}) \tau_{1,10} + (\tau_{2,8} - \tau_{2,10}) (\tau_{2,8} + 3 \tau_{2,13} + \tau_{3,8} + 7 \tau_{3,13})) l_6^2 - \\
& \quad 2 \tau_{1,14}^2 (\tau_{3,11} + \tau_{3,14} + \tau_{3,15} + 2 \tau_{4,11}) l_7^2 - \tau_{1,15}^2 (3 \tau_{3,11} + \tau_{3,14} + 4 \tau_{4,11}) l_7^2 - \\
& \quad \tau_{1,15} (3 \tau_{3,11}^2 + (6 \tau_{3,14} + 3 \tau_{3,15} + 4 \tau_{4,11} + 5 \tau_{4,14}) \tau_{3,11} + 4 \tau_{3,14}^2 + 2 \tau_{3,15}^2 + 2 \tau_{3,9} (\tau_{3,11} + \tau_{4,14}) + \\
& \quad \tau_{3,15} (-2 \tau_{4,9} + 3 \tau_{4,11} + 4 \tau_{4,14}) + \tau_{4,11} (-2 \tau_{4,9} + \tau_{4,11} + 5 \tau_{4,14}) + \tau_{3,14} (7 \tau_{3,15} - 4 \tau_{4,9} + 7 \tau_{4,11} + 5 \tau_{4,14})) l_7^2 - \\
& \quad \tau_{1,14} (2 \tau_{3,11}^2 + (6 \tau_{3,14} + 6 \tau_{3,15} - 4 \tau_{4,9} + \tau_{4,11} + 6 \tau_{4,14}) \tau_{3,11} + 4 \tau_{3,14}^2 + 4 \tau_{3,15}^2 + \\
& \quad \tau_{1,15} (4 (\tau_{3,11} + \tau_{3,14} + \tau_{3,15}) + 6 \tau_{4,11}) - 2 \tau_{3,9} (\tau_{4,11} - 2 \tau_{4,14}) + \tau_{3,15} (-4 \tau_{4,9} + 5 \tau_{4,11} + 4 \tau_{4,14}) + \\
& \quad \tau_{3,14} (8 \tau_{3,15} - 4 \tau_{4,9} + 6 \tau_{4,11} + 4 \tau_{4,14}) + \tau_{4,11} (7 \tau_{4,14} - 8 \tau_{4,9})) l_7^2 + \\
& (-2 \tau_{3,14}^3 - 2 (3 \tau_{3,15} - 2 \tau_{4,9} + \tau_{4,11} + 2 \tau_{4,14}) \tau_{3,14}^2 - (6 \tau_{3,15}^2 + (-8 \tau_{4,9} + 5 \tau_{4,11} + 9 \tau_{4,14}) \tau_{3,15} + \\
& \quad 2 (\tau_{4,9}^2 - 3 \tau_{4,11} \tau_{4,9} - \tau_{4,11}^2 + \tau_{4,14}^2 + 2 (\tau_{4,11} - \tau_{4,9}) \tau_{4,14})) \tau_{3,14} - \tau_{3,15}^3 + \\
& \quad \tau_{3,11} (-4 \tau_{3,14}^2 + (-8 \tau_{3,15} + 6 \tau_{4,9} - 8 \tau_{4,14}) \tau_{3,14} - 2 \tau_{3,15}^2 + \tau_{3,15} (3 \tau_{4,9} - 7 \tau_{4,14}) - \\
& \quad (2 \tau_{4,9} - 3 \tau_{4,11} - 4 \tau_{4,14}) (\tau_{4,9} + \tau_{4,11} - \tau_{4,14})) + \tau_{3,15}^2 (3 \tau_{4,9} - 4 \tau_{4,14}) + \\
& \quad \tau_{3,11}^2 (-2 \tau_{3,14} - 2 \tau_{3,15} + 2 \tau_{4,9} + \tau_{4,11} - 2 \tau_{4,14}) + \tau_{3,9}^2 (\tau_{3,11} + \tau_{3,14} + 2 \tau_{4,14}) + \\
& \quad \tau_{3,9} (\tau_{3,11}^2 + (\tau_{3,14} - \tau_{3,15}) \tau_{3,11} - 5 \tau_{4,14}^2 - (\tau_{3,15} + \tau_{4,11}) (2 \tau_{4,9} + \tau_{4,11}) + \tau_{3,14} (\tau_{4,11} - 4 \tau_{4,14}) - \\
& \quad (3 \tau_{3,15} - 4 \tau_{4,9} + \tau_{4,11}) \tau_{4,14}) + \tau_{3,15} (-4 \tau_{4,9}^2 + 3 \tau_{4,11} \tau_{4,9} + 3 \tau_{4,11}^2 - 2 \tau_{4,14}^2 + (5 \tau_{4,9} - 2 \tau_{4,11}) \tau_{4,14}) +
\end{aligned}$$

$$\begin{aligned}
& \tau_{4,11} \left( -4 \tau_{4,9}^2 + 2 \tau_{4,11}^2 - 2 \tau_{4,14}^2 + (7 \tau_{4,9} + 3 \tau_{4,11}) \tau_{4,14} \right) l_7^2 - \\
& 2 \tau_{2,6} \tau_{4,6}^2 l_8^2 + \tau_{1,10}^2 \left( (\tau_{2,8} + \tau_{2,13} + \tau_{3,8} + 3 \tau_{3,13}) l_6^2 + 2 (\tau_{1,6} + \tau_{3,6}) l_{13}^2 \right) + \\
& \tau_{1,10} \left( 2 \left( 2 \tau_{1,6}^2 + 3 \tau_{2,10} \tau_{1,6} - 2 \tau_{3,6}^2 - \tau_{2,9} \tau_{2,10} + 2 (\tau_{2,9} + 2 \tau_{2,10}) \tau_{3,6} \right) l_{13}^2 - \right. \\
& \quad (\tau_{2,8} - \tau_{2,10}) (\tau_{2,8} + 3 \tau_{2,13} + \tau_{3,8} + 7 \tau_{3,13}) l_6^2 + 2 \left( (\tau_{2,13} + 2 \tau_{3,13}) l_6^2 \tau_{2,8}^2 - 2 \tau_{2,10} (\tau_{2,13} + 2 \tau_{3,13}) l_6^2 \tau_{2,8} - \right. \\
& \quad \left. (\tau_{4,6}^3 + 3 \tau_{4,10} \tau_{4,6}^2 + (-\tau_{4,13}^2 + (\tau_{3,6} - \tau_{3,13} + 2 \tau_{4,10}) \tau_{4,13} + \tau_{4,10} (2 \tau_{2,6} - \tau_{3,6} + \tau_{3,13} + 2 \tau_{4,10})) \tau_{4,6} - \right. \\
& \quad \left. (\tau_{2,6} + \tau_{3,6} - \tau_{3,13}) \tau_{4,10}^2 - (2 \tau_{2,6} + \tau_{4,10}) \tau_{4,13}^2 + \tau_{4,10} (4 \tau_{2,6} + \tau_{3,6} - \tau_{3,13} + 2 \tau_{4,10}) \tau_{4,13} \right) l_8^2 - \\
& \quad \tau_{3,6} (\tau_{1,6}^2 + (\tau_{1,9} - 2 \tau_{2,9} + 2 \tau_{3,6}) \tau_{1,6} + \tau_{1,9} (\tau_{3,6} - \tau_{2,9})) l_{13}^2 + \\
& \quad \tau_{2,10}^2 \left( (\tau_{2,13} + 2 \tau_{3,13}) l_6^2 + (\tau_{1,9} + \tau_{2,9} + \tau_{3,6} + 2 \tau_{3,9}) l_{13}^2 \right) + \\
& \quad \left. \tau_{2,10} \left( (4 \tau_{1,6}^2 - (2 \tau_{2,9} - 5 \tau_{3,6} + \tau_{3,9}) \tau_{1,6} - \tau_{1,9} \tau_{2,9} - 2 \tau_{3,6} \tau_{3,9}) l_{13}^2 - (\tau_{4,6} + 2 \tau_{4,10} - \tau_{4,13}) (\tau_{4,6} + \tau_{4,13}) l_8^2 \right) \right)
\end{aligned}$$

■  $N_{36}^{(6)}$

$$\begin{aligned}
& \frac{1}{8} \left( s l_7^2 (4 l_8^2 (3 (s^2 + 3 (t^2 + u^2)) l_9^2 + (19 s^2 - 31 t^2 - 9 u^2) l_{13}^2) + (-24 l_{16}^2 s^2 + 4 (8 s^2 + 5 (t^2 + u^2)) l_9^2 + (4 s^2 + 3 (t^2 + u^2)) l_{13}^2) l_{17}^2) - \right. \\
& \quad l_{13}^2 (32 l_6^2 l_{12}^2 t^3 + 2 (4 \tau_{1,8}^2 - (12 \tau_{2,7} + 2 \tau_{2,8} + 3 \tau_{2,9} - 4 \tau_{4,8}) \tau_{1,8} + 8 \tau_{2,7}^2 - 4 \tau_{2,8}^2 - \tau_{1,9} (4 \tau_{2,8} + 5 \tau_{2,9}) - \\
& \quad 2 \tau_{2,7} (\tau_{2,8} - 5 \tau_{2,9} + 3 \tau_{4,8} - 5 \tau_{4,9}) + 4 \tau_{2,8} (2 \tau_{2,9} - \tau_{4,8} + \tau_{4,9}) + 4 \tau_{4,8} (3 \tau_{2,9} + 2 \tau_{4,9})) l_6^2 t^2 + \\
& \quad s l_5^2 l_{17}^2 t^2 - 76 (-s^2 + t^2 + u^2) l_6^2 l_{12}^2 t + 2 (5 s^2 + t^2 + 3 u^2) \tau_{1,7}^2 l_6^2 - \\
& \quad 2 \tau_{1,7} (-4 \tau_{2,9} s^2 + 7 \tau_{4,8} s^2 - 9 \tau_{4,9} s^2 + (3 s^2 + 9 t^2 - u^2) \tau_{1,8} - 2 u (4 t + 5 u) \tau_{1,9} - 2 (9 s^2 + 2 (t^2 + u^2)) \tau_{2,7} + \\
& \quad 2 (3 s^2 + t^2 + 3 u^2) \tau_{2,8} - 6 t^2 \tau_{2,9} + 4 u^2 \tau_{2,9} + t^2 \tau_{4,8} - u^2 \tau_{4,8} + t^2 \tau_{4,9} - u^2 \tau_{4,9}) l_6^2 + \\
& \quad 2 (s^2 - t^2 - u^2) (2 \tau_{1,8}^2 + 2 (\tau_{1,9} - 3 \tau_{2,7} + 2 \tau_{2,9} + \tau_{4,9}) \tau_{1,8} + 5 \tau_{2,7}^2 + \tau_{1,9} (4 (\tau_{2,7} + \tau_{2,8} - \tau_{2,9}) + 6 \tau_{4,8}) + \\
& \quad \tau_{2,7} (-3 \tau_{2,8} + 4 \tau_{2,9} - 7 \tau_{4,8} + 9 \tau_{4,9}) + 2 (\tau_{2,8}^2 + (\tau_{2,9} + \tau_{4,9}) \tau_{2,8} + \tau_{4,8} (3 \tau_{2,9} + 4 \tau_{4,9}))) l_6^2 - \\
& \quad 2 u^2 (4 \tau_{1,8}^2 + 2 (-4 \tau_{1,9} + 4 \tau_{2,7} + \tau_{2,8} + 2 (\tau_{2,9} + \tau_{4,8} - \tau_{4,9})) \tau_{1,8} + \tau_{1,9} (-10 \tau_{2,7} + 3 \tau_{2,8} + 5 \tau_{2,9} - 12 \tau_{4,8}) - \\
& \quad 2 (3 \tau_{2,7}^2 + (-6 \tau_{2,8} - 4 \tau_{4,8} + 4 \tau_{4,9}) \tau_{2,7} + 2 \tau_{2,8} (\tau_{2,8} + \tau_{4,8}) + 4 \tau_{4,8} \tau_{4,9})) \\
& \quad \left. l_6^2 + 32 u^3 l_6^2 l_{12}^2 - 76 u (-s^2 + t^2 + u^2) l_6^2 l_{12}^2 \right)
\end{aligned}$$

■  $N_{36}^{(7)}$

$$\begin{aligned}
& \frac{1}{8} \left( (-32 \tau_{2,13} l_7^2 l_8^2 l_9^2 + 16 \tau_{2,15} l_7^2 l_8^2 l_9^2 + 8 \tau_{3,10} l_7^2 l_8^2 l_9^2 - 58 \tau_{3,12} l_7^2 l_8^2 l_9^2 + 8 \tau_{3,13} l_7^2 l_8^2 l_9^2 - 4 \tau_{4,10} l_7^2 l_8^2 l_9^2 - \right. \\
& 44 \tau_{4,12} l_7^2 l_8^2 l_9^2 + 12 \tau_{4,13} l_7^2 l_8^2 l_9^2 - 8 \tau_{2,17} l_7^2 l_8^2 l_{13}^2 - 8 \tau_{3,5} l_7^2 l_8^2 l_{13}^2 + 8 \tau_{3,10} l_7^2 l_8^2 l_{13}^2 + 72 \tau_{3,12} l_7^2 l_8^2 l_{13}^2 + \\
& 8 \tau_{3,17} l_7^2 l_8^2 l_{13}^2 + 32 \tau_{4,5} l_7^2 l_8^2 l_{13}^2 + 64 \tau_{4,10} l_7^2 l_8^2 l_{13}^2 + 48 \tau_{4,12} l_7^2 l_8^2 l_{13}^2 + 12 \tau_{1,7} l_6^2 l_{12}^2 l_{13}^2 - 20 \tau_{1,9} l_6^2 l_{12}^2 l_{13}^2 - \\
& 14 \tau_{1,11} l_6^2 l_{12}^2 l_{13}^2 - 4 \tau_{2,7} l_6^2 l_{12}^2 l_{13}^2 - 48 \tau_{2,9} l_6^2 l_{12}^2 l_{13}^2 - 34 \tau_{2,11} l_6^2 l_{12}^2 l_{13}^2 - 52 \tau_{4,9} l_6^2 l_{12}^2 l_{13}^2 - \\
& 20 \tau_{4,11} l_6^2 l_{12}^2 l_{13}^2 - 52 \tau_{4,16} l_6^2 l_{12}^2 l_{13}^2 + 4 \tau_{2,12} l_7^2 l_8^2 (7 l_{13}^2 - 6 l_9^2) + 4 \tau_{2,10} l_7^2 l_8^2 (19 l_9^2 + 28 l_{13}^2) + \\
& l_7^2 ((8 \tau_{2,11} + 28 \tau_{2,15} - 2 \tau_{2,16} + 7 \tau_{3,8} + 48 \tau_{3,11} + 19 \tau_{3,15} - 3 \tau_{3,16} - 23 \tau_{4,8} + 32 \tau_{4,11} + 15 \tau_{4,15} - 7 \tau_{4,16}) l_9^2 + \\
& (17 \tau_{2,9} + 6 \tau_{2,15} + 22 \tau_{2,16} + 45 \tau_{3,8} + 61 \tau_{3,9} - 4 \tau_{3,15} + 9 \tau_{3,16} + 35 \tau_{4,8} + 51 \tau_{4,9} - 12 \tau_{4,15} + 2 \tau_{4,16}) l_{13}^2) l_{17}^2) \\
& t^2 + (s^2 - t^2 - u^2) (2 \tau_{2,13} l_7^2 l_8^2 l_9^2 + 16 \tau_{2,15} l_7^2 l_8^2 l_9^2 + 4 \tau_{3,10} l_7^2 l_8^2 l_9^2 - 52 \tau_{3,12} l_7^2 l_8^2 l_9^2 + 8 \tau_{3,13} l_7^2 l_8^2 l_9^2 + \\
& 4 \tau_{3,15} l_7^2 l_8^2 l_9^2 - 26 \tau_{4,10} l_7^2 l_8^2 l_9^2 + 4 \tau_{4,12} l_7^2 l_8^2 l_9^2 + 6 \tau_{4,13} l_7^2 l_8^2 l_9^2 - 28 \tau_{2,5} l_7^2 l_8^2 l_{13}^2 - 8 \tau_{2,17} l_7^2 l_8^2 l_{13}^2 - \\
& 8 \tau_{3,5} l_7^2 l_8^2 l_{13}^2 + 4 \tau_{3,10} l_7^2 l_8^2 l_{13}^2 + 32 \tau_{3,12} l_7^2 l_8^2 l_{13}^2 + 12 \tau_{3,17} l_7^2 l_8^2 l_{13}^2 + 24 \tau_{4,5} l_7^2 l_8^2 l_{13}^2 + 84 \tau_{4,10} l_7^2 l_8^2 l_{13}^2 - \\
& 68 \tau_{4,12} l_7^2 l_8^2 l_{13}^2 - 56 \tau_{1,9} l_6^2 l_{12}^2 l_{13}^2 - 34 \tau_{1,11} l_6^2 l_{12}^2 l_{13}^2 - 56 \tau_{2,9} l_6^2 l_{12}^2 l_{13}^2 - 34 \tau_{2,11} l_6^2 l_{12}^2 l_{13}^2 - 48 \tau_{4,9} l_6^2 l_{12}^2 l_{13}^2 - \\
& 24 \tau_{4,11} l_6^2 l_{12}^2 l_{13}^2 - 56 \tau_{4,16} l_6^2 l_{12}^2 l_{13}^2 + 2 \tau_{2,12} l_7^2 l_8^2 (2 l_{13}^2 - 11 l_9^2) + 2 \tau_{2,10} l_7^2 l_8^2 (27 l_9^2 + 46 l_{13}^2) + \\
& l_7^2 ((16 \tau_{2,11} + 44 \tau_{2,15} + 14 \tau_{2,16} + 16 \tau_{3,8} + 32 \tau_{3,11} + 13 \tau_{3,15} - 9 \tau_{3,16} + 16 \tau_{4,8} + 32 \tau_{4,11} + 13 \tau_{4,15} - 9 \tau_{4,16}) l_9^2 + \\
& (20 \tau_{2,9} + 6 \tau_{2,15} + 22 \tau_{2,16} + 37 \tau_{3,8} + 53 \tau_{3,9} - 5 \tau_{3,15} + 7 \tau_{3,16} + 37 \tau_{4,8} + 53 \tau_{4,9} - 5 \tau_{4,15} + 7 \tau_{4,16}) l_{13}^2) l_{17}^2) + \\
& u^2 (24 \tau_{2,13} l_7^2 l_8^2 l_9^2 + 16 \tau_{2,15} l_7^2 l_8^2 l_9^2 + 48 \tau_{3,10} l_7^2 l_8^2 l_9^2 - 116 \tau_{3,12} l_7^2 l_8^2 l_9^2 + 8 \tau_{3,13} l_7^2 l_8^2 l_9^2 + 8 \tau_{3,15} l_7^2 l_8^2 l_9^2 - \\
& 56 \tau_{4,12} l_7^2 l_8^2 l_9^2 + 2 \tau_{2,10} l_7^2 l_8^2 (59 l_9^2 - 4 l_{13}^2) + 8 \tau_{2,5} l_7^2 l_8^2 l_{13}^2 - 8 \tau_{2,17} l_7^2 l_8^2 l_{13}^2 + 8 \tau_{3,5} l_7^2 l_8^2 l_{13}^2 - \\
& 80 \tau_{3,10} l_7^2 l_8^2 l_{13}^2 + 72 \tau_{3,12} l_7^2 l_8^2 l_{13}^2 + 16 \tau_{3,17} l_7^2 l_8^2 l_{13}^2 + 32 \tau_{4,5} l_7^2 l_8^2 l_{13}^2 + 24 \tau_{4,10} l_7^2 l_8^2 l_{13}^2 - 24 \tau_{4,12} l_7^2 l_8^2 l_{13}^2 - \\
& 4 \tau_{1,7} l_6^2 l_{12}^2 l_{13}^2 - 48 \tau_{1,9} l_6^2 l_{12}^2 l_{13}^2 - 34 \tau_{1,11} l_6^2 l_{12}^2 l_{13}^2 + 12 \tau_{2,7} l_6^2 l_{12}^2 l_{13}^2 - 20 \tau_{2,9} l_6^2 l_{12}^2 l_{13}^2 - \\
& 14 \tau_{2,11} l_6^2 l_{12}^2 l_{13}^2 - 52 \tau_{4,9} l_6^2 l_{12}^2 l_{13}^2 - 20 \tau_{4,11} l_6^2 l_{12}^2 l_{13}^2 - 52 \tau_{4,16} l_6^2 l_{12}^2 l_{13}^2 + 4 \tau_{2,12} l_7^2 l_8^2 (5 l_{13}^2 - 13 l_9^2) + \\
& l_7^2 ((8 \tau_{2,11} + 28 \tau_{2,15} - 2 \tau_{2,16} - 23 \tau_{3,8} + 32 \tau_{3,11} + 15 \tau_{3,15} - 7 \tau_{3,16} + 7 \tau_{4,8} + 48 \tau_{4,11} + 19 \tau_{4,15} - 3 \tau_{4,16}) l_9^2 + \\
& (17 \tau_{2,9} + 6 \tau_{2,15} + 22 \tau_{2,16} + 35 \tau_{3,8} + 51 \tau_{3,9} - 12 \tau_{3,15} + 2 \tau_{3,16} + 45 \tau_{4,8} + 61 \tau_{4,9} - 4 \tau_{4,15} + 9 \tau_{4,16}) l_{13}^2) l_{17}^2))
\end{aligned}$$

■  $N_{36}^{(8)}$

0
