# Supplementary material for: The Ultraviolet Behavior of N=8 Supergravity at Four Loops
Source: arXiv:0905.2326 ancillary file (2012-01-08)
Supplement: Supplementary file 33 [file SUGRA38.pdf]

## Integral 38: $\mathcal{I}_{38}$

$\mathcal{N} = 8$  four-point four-loop amplitude.

### ■ 2D plot of graph associated with $\mathcal{I}_{38}$

This fixes the labelling associated with the numerator expressions given below.

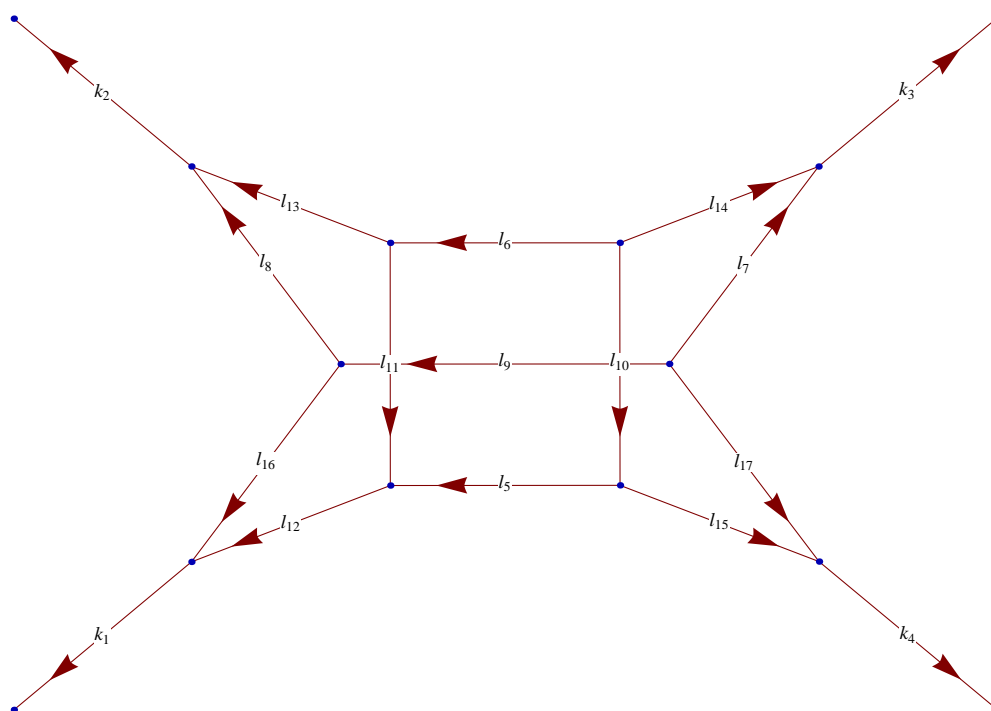

When using MathPlayer, by clicking three times (holding the click on the third click) directly on a vertex, one is able to move that vertex around, and its associated edges follow elastically. This functionality is absent when viewing as a pdf.

*Note: propagators for certain graphs were relabeled in the manuscript due to size constraints. The labels given in `aux/rawData/Neq8FourLoops.m` should be used for verification purposes.*

### ■ 3D plot of graph associated with $\mathcal{I}_{38}$

3D PLOT UNAVAILABLE FOR PDF. Please see .nb version for the 3D figure.

When using MathPlayer, by clicking anywhere in the image and dragging one should be able to rotate this 3D image. By holding (ALT) or (COMMAND) while clicking and moving the mouse up/down one should be able to zoom in/out. This functionality is absent when viewing as a pdf.

### ■ "Vertex Form" of graph associated with $\mathcal{I}_{38}$

This function returns the graph associated with the integral object in a vertex representation. This can be used as a way of specifying the topology of a graph using trivalent (cubic) vertices,  $\text{gVertex}[p_a, p_b, p_c]$ , where  $\{p_a, p_b, p_c\}$  are momenta labeling the propagators (edges) of the graph, and is understood that the edge labelled by  $p_a$  flows into the edge labelled by  $-p_a$ . Additionally, each vertex represents the manifest conservation of ( $D$  - dimensional) momenta :

$$\text{gVertex}[\{p_1, p_2, p_3\}] \iff (p_1 + p_2 + p_3 = 0)$$

$$\{\text{gVertex}(\{k_1, -l_{16}, -l_{12}\}), \text{gVertex}(\{k_2, -l_{13}, -l_8\}), \text{gVertex}(\{k_3, -l_{14}, -l_7\}), \text{gVertex}(\{k_4, -l_{17}, -l_{15}\}), \text{gVertex}(\{-l_5, -l_{11}, l_{12}\}), \\ \text{gVertex}(\{l_5, l_{15}, -l_{10}\}), \text{gVertex}(\{-l_6, l_{13}, l_{11}\}), \text{gVertex}(\{l_6, l_{10}, l_{14}\}), \text{gVertex}(\{l_7, l_{17}, l_9\}), \text{gVertex}(\{l_8, -l_9, l_{16}\})\}$$

### ■ Numerator expression for integral 38:

The following notation is used:  $\tau_{i,j} \equiv \begin{cases} 2 k_i \cdot l_j & \text{if } i \leq 4, j > 4 \\ 2 l_i \cdot l_j & \text{if } i, j > 4 \end{cases}$ .

$$s \equiv 2 k_1 \cdot k_2 = 2 k_3 \cdot k_4$$

We use  $s, t, u$  to represent the traditional Mandelstam variables for massless external four-point momenta:  $t \equiv 2 k_1 \cdot k_4 = 2 k_2 \cdot k_3$ .

$$u \equiv 2 k_1 \cdot k_3 = 2 k_2 \cdot k_4$$

Furthermore we use the shorthand  $(l_i)^2$  to represent the lorentz square:  $(l_i)^2 = l_i \cdot l_i$ .

The total numerator  $\mathcal{N}_{38}$  is given by summing over the following terms, distinguished here by explicit dependence on loop momenta:  $\mathcal{N}_{38} = \sum_{i=0}^8 \mathcal{N}_{38}^{(i)}$ :

$$\blacksquare \mathcal{N}_{38}^{(0)}$$

$$16 s^4 t^2$$

$$\blacksquare \mathcal{N}_{38}^{(1)}$$

$$-8 s^3 t$$

$$(2 t \tau_{1,5} + 2 t \tau_{1,6} - t (\tau_{1,17} - 2 \tau_{2,5} - 2 \tau_{2,6} + \tau_{2,7} + 2 \tau_{3,5} + 2 \tau_{3,6} + \tau_{3,8} + 2 (\tau_{4,5} + \tau_{4,6}) + \tau_{4,16}) - u (\tau_{1,17} + \tau_{2,7} + \tau_{3,8} + \tau_{4,16}))$$

■  $N_{38}^{(2)}$

$$\begin{aligned}
& 2s^2 \left( 2(\tau_{7,8} + \tau_{16,17})t^3 + 6\tau_{1,5}^2 t^2 + 6\tau_{1,6}^2 t^2 + \right. \\
& \quad (\tau_{1,17}^2 + (-3\tau_{2,5} - 3\tau_{2,6} + 3(\tau_{3,5} + \tau_{3,6} + \tau_{4,5} + \tau_{4,6}) + 2\tau_{4,16})\tau_{1,17} + 6\tau_{2,5}^2 + 6\tau_{2,6}^2 + \tau_{2,7}^2 + 6\tau_{3,5}^2 + 6\tau_{3,6}^2 + \\
& \quad \tau_{3,8}^2 + 6\tau_{4,5}^2 + 6\tau_{4,6}^2 + \tau_{4,16}^2 + 12\tau_{3,5}\tau_{3,6} + 3\tau_{3,5}\tau_{3,8} + 3\tau_{3,6}\tau_{3,8} + 12\tau_{3,5}\tau_{4,5} + 12\tau_{3,6}\tau_{4,5} + 3\tau_{3,8}\tau_{4,5} + \\
& \quad 12\tau_{3,5}\tau_{4,6} + 12\tau_{3,6}\tau_{4,6} + 3\tau_{3,8}\tau_{4,6} + 12\tau_{4,5}\tau_{4,6} + \tau_{2,7}(3\tau_{3,5} + 3\tau_{3,6} + 2\tau_{3,8} + 3(\tau_{4,5} + \tau_{4,6})) + \\
& \quad 3\tau_{2,5}(4\tau_{2,6} - \tau_{2,7} - \tau_{3,8} - \tau_{4,16}) + 3\tau_{3,5}\tau_{4,16} + 3\tau_{3,6}\tau_{4,16} + 3\tau_{4,5}\tau_{4,16} + 3\tau_{4,6}\tau_{4,16} - 3\tau_{2,6}(\tau_{2,7} + \tau_{3,8} + \tau_{4,16}))t^2 + \\
& \quad 3\tau_{1,6}(4t(\tau_{2,5} + \tau_{2,6}) + s(\tau_{1,17} + \tau_{2,7} + \tau_{3,8} + \tau_{4,16}))t + 3\tau_{1,5}(4t(\tau_{1,6} + \tau_{2,5} + \tau_{2,6}) + s(\tau_{1,17} + \tau_{2,7} + \tau_{3,8} + \tau_{4,16}))t - \\
& \quad 2(-s^2 + t^2 + u^2)(\tau_{7,8} + \tau_{16,17})t + u^2((\tau_{2,7} + \tau_{3,8})^2 + (\tau_{1,17} + \tau_{4,16})^2) + \\
& \quad \frac{1}{2}(-s^2 - t^2 - u^2)(2\tau_{1,17}^2 + (-3\tau_{2,5} - 3\tau_{2,6} + 3(\tau_{3,5} + \tau_{3,6} + \tau_{4,5} + \tau_{4,6}) + 4\tau_{4,16})\tau_{1,17} + \\
& \quad 2\tau_{4,16}^2 + (\tau_{2,7} + \tau_{3,8})(-3\tau_{2,5} - 3\tau_{2,6} + 2\tau_{2,7} + 3\tau_{3,5} + 3\tau_{3,6} + 2\tau_{3,8} + 3(\tau_{4,5} + \tau_{4,6})) + \\
& \quad \left. 3(-\tau_{2,5} - \tau_{2,6} + \tau_{3,5} + \tau_{3,6} + \tau_{4,5} + \tau_{4,6})\tau_{4,16}) - u(-s^2 + t^2 + u^2)(\tau_{7,8} + \tau_{16,17}) \right)
\end{aligned}$$

■  $N_{38}^{(3)}$ 

$$\begin{aligned}
& -s \left( 2 \left( (\tau_{1,5} + \tau_{1,6} + \tau_{2,5} + \tau_{2,6} - \tau_{2,7} - \tau_{3,5} - \tau_{3,6} - \tau_{3,8} - \tau_{4,5} - \tau_{4,6}) \tau_{7,8} + \right. \right. \\
& \quad (\tau_{1,5} + \tau_{1,6} - \tau_{1,17} + \tau_{2,5} + \tau_{2,6} - \tau_{3,5} - \tau_{3,6} - \tau_{4,5} - \tau_{4,6} - \tau_{4,16}) \tau_{16,17} \Big) t^3 + \\
& \quad (4 \tau_{1,5}^3 + 3 (4 \tau_{1,6} - \tau_{1,17} + 4 \tau_{2,5} + 4 \tau_{2,6} - \tau_{2,7} - \tau_{3,8} - \tau_{4,16}) \tau_{1,5}^2 + \\
& \quad (12 \tau_{1,6}^2 - 6 (\tau_{1,17} - 4 \tau_{2,5} - 4 \tau_{2,6} + \tau_{2,7} + \tau_{3,8} + \tau_{4,16}) \tau_{1,6} + \tau_{1,17}^2 + 12 \tau_{2,5}^2 + 12 \tau_{2,6}^2 + \tau_{2,7}^2 + \tau_{3,8}^2 + \tau_{4,16}^2 + \\
& \quad 2 \tau_{2,7} \tau_{3,8} + 6 \tau_{2,5} (4 \tau_{2,6} - \tau_{2,7} - \tau_{3,8} - \tau_{4,16}) + 2 \tau_{1,17} (\tau_{4,16} - 3 (\tau_{2,5} + \tau_{2,6})) - 6 \tau_{2,6} (\tau_{2,7} + \tau_{3,8} + \tau_{4,16})) \tau_{1,5} + \\
& \quad 4 \tau_{1,6}^3 + 4 \tau_{2,5}^3 + 4 \tau_{2,6}^3 - 4 \tau_{3,5}^3 - 4 \tau_{3,6}^3 - 4 \tau_{4,5}^3 - 4 \tau_{4,6}^3 + 12 \tau_{2,5} \tau_{2,6}^2 - 3 \tau_{1,17} (\tau_{2,5} + \tau_{2,6})^2 + \\
& \quad \tau_{2,5} \tau_{2,7}^2 + \tau_{2,6} \tau_{2,7}^2 - 3 \tau_{2,7} \tau_{3,5}^2 - 3 \tau_{2,7} \tau_{3,6}^2 - 12 \tau_{3,5} \tau_{3,6}^2 + \tau_{2,5} \tau_{3,8}^2 + \tau_{2,6} \tau_{3,8}^2 - \tau_{3,5} \tau_{3,8}^2 - \tau_{3,6} \tau_{3,8}^2 - \\
& \quad 3 \tau_{2,7} \tau_{4,5}^2 - 12 \tau_{3,5} \tau_{4,5}^2 - 12 \tau_{3,6} \tau_{4,5}^2 - 3 \tau_{3,8} \tau_{4,5}^2 - 3 \tau_{2,7} \tau_{4,6}^2 - 12 \tau_{3,5} \tau_{4,6}^2 - 12 \tau_{3,6} \tau_{4,6}^2 - 3 \tau_{3,8} \tau_{4,6}^2 - \\
& \quad 12 \tau_{4,5} \tau_{4,6}^2 - 3 \tau_{1,17} (\tau_{3,5} + \tau_{3,6} + \tau_{4,5} + \tau_{4,6})^2 + (\tau_{2,5} + \tau_{2,6} - \tau_{3,5} - \tau_{3,6} - \tau_{4,5} - \tau_{4,6}) \tau_{4,16}^2 + 12 \tau_{2,5}^2 \tau_{2,6} - \\
& \quad 3 \tau_{2,5}^2 \tau_{2,7} - 3 \tau_{2,6}^2 \tau_{2,7} - 6 \tau_{2,5} \tau_{2,6} \tau_{2,7} - \tau_{2,7}^2 \tau_{3,5} - \tau_{2,7}^2 \tau_{3,6} - 12 \tau_{3,5}^2 \tau_{3,6} - 6 \tau_{2,7} \tau_{3,5} \tau_{3,6} - 3 \tau_{2,5}^2 \tau_{3,8} - \\
& \quad 3 \tau_{2,6}^2 \tau_{3,8} - 3 \tau_{3,5}^2 \tau_{3,8} - 3 \tau_{3,6}^2 \tau_{3,8} - 6 \tau_{2,5} \tau_{2,6} \tau_{3,8} + 2 \tau_{2,5} \tau_{2,7} \tau_{3,8} + 2 \tau_{2,6} \tau_{2,7} \tau_{3,8} - 2 \tau_{2,7} \tau_{3,5} \tau_{3,8} - \\
& \quad 2 \tau_{2,7} \tau_{3,6} \tau_{3,8} - 6 \tau_{3,5} \tau_{3,6} \tau_{3,8} - \tau_{2,7}^2 \tau_{4,5} - 12 \tau_{3,5}^2 \tau_{4,5} - 12 \tau_{3,6}^2 \tau_{4,5} - \tau_{3,8}^2 \tau_{4,5} - 6 \tau_{2,7} \tau_{3,5} \tau_{4,5} - 6 \tau_{2,7} \tau_{3,6} \tau_{4,5} - \\
& \quad 24 \tau_{3,5} \tau_{3,6} \tau_{4,5} - 2 \tau_{2,7} \tau_{3,8} \tau_{4,5} - 6 \tau_{3,5} \tau_{3,8} \tau_{4,5} - 6 \tau_{3,6} \tau_{3,8} \tau_{4,5} + \tau_{1,17}^2 (\tau_{2,5} + \tau_{2,6} - \tau_{3,5} - \tau_{3,6} - \tau_{4,5} - \tau_{4,6}) - \\
& \quad \tau_{2,7}^2 \tau_{4,6} - 12 \tau_{3,5}^2 \tau_{4,6} - 12 \tau_{3,6}^2 \tau_{4,6} - \tau_{3,8}^2 \tau_{4,6} - 12 \tau_{4,5}^2 \tau_{4,6} - 6 \tau_{2,7} \tau_{3,5} \tau_{4,6} - 6 \tau_{2,7} \tau_{3,6} \tau_{4,6} - 24 \tau_{3,5} \tau_{3,6} \tau_{4,6} - \\
& \quad 2 \tau_{2,7} \tau_{3,8} \tau_{4,6} - 6 \tau_{3,5} \tau_{3,8} \tau_{4,6} - 6 \tau_{3,6} \tau_{3,8} \tau_{4,6} - 6 \tau_{2,7} \tau_{4,5} \tau_{4,6} - 24 \tau_{3,5} \tau_{4,5} \tau_{4,6} - 24 \tau_{3,6} \tau_{4,5} \tau_{4,6} - \\
& \quad 6 \tau_{3,8} \tau_{4,5} \tau_{4,6} + (2 \tau_{1,17} (\tau_{2,5} + \tau_{2,6} - \tau_{3,5} - \tau_{3,6} - \tau_{4,5} - \tau_{4,6}) - 3 ((\tau_{2,5} + \tau_{2,6})^2 + (\tau_{3,5} + \tau_{3,6} + \tau_{4,5} + \tau_{4,6})^2)) \tau_{4,16} - \\
& \quad 3 \tau_{1,6}^2 (\tau_{1,17} - 4 \tau_{2,5} - 4 \tau_{2,6} + \tau_{2,7} + \tau_{3,8} + \tau_{4,16}) + \tau_{1,6} (\tau_{1,17}^2 + 2 (\tau_{4,16} - 3 (\tau_{2,5} + \tau_{2,6})) \tau_{1,17} + 12 \tau_{2,5}^2 + 12 \tau_{2,6}^2 + \\
& \quad \tau_{2,7}^2 + \tau_{3,8}^2 + \tau_{4,16}^2 + 2 \tau_{2,7} \tau_{3,8} + 6 \tau_{2,5} (4 \tau_{2,6} - \tau_{2,7} - \tau_{3,8} - \tau_{4,16}) - 6 \tau_{2,6} (\tau_{2,7} + \tau_{3,8} + \tau_{4,16})) t^2 + \\
& \quad (s^2 - t^2 - u^2) ((2 \tau_{1,5} + 2 \tau_{1,6} + 2 \tau_{2,5} + 2 \tau_{2,6} - 3 \tau_{2,7} - 2 \tau_{3,5} - 2 \tau_{3,6} - 3 \tau_{3,8} - 2 \tau_{4,5} - 2 \tau_{4,6}) \tau_{7,8} + \\
& \quad (2 \tau_{1,5} + 2 \tau_{1,6} - 3 \tau_{1,17} + 2 \tau_{2,5} + 2 \tau_{2,6} - 2 (\tau_{3,5} + \tau_{3,6} + \tau_{4,5} + \tau_{4,6}) - 3 \tau_{4,16}) \tau_{16,17} \Big) t + \\
& \quad u^2 (\tau_{1,5} + \tau_{1,6} + \tau_{2,5} + \tau_{2,6} - \tau_{3,5} - \tau_{3,6} - \tau_{4,5} - \tau_{4,6}) ((\tau_{2,7} + \tau_{3,8})^2 + (\tau_{1,17} + \tau_{4,16})^2) - \\
& \quad \frac{1}{2} (s^2 - t^2 - u^2) (3 (\tau_{1,17} + \tau_{2,7} + \tau_{3,8} + \tau_{4,16}) \tau_{1,5}^2 + 2 (-\tau_{1,17}^2 + (3 (\tau_{2,5} + \tau_{2,6}) - 2 \tau_{4,16}) \tau_{1,17} - \tau_{4,16}^2 + \\
& \quad (3 \tau_{2,5} + 3 \tau_{2,6} - \tau_{2,7} - \tau_{3,8}) (\tau_{2,7} + \tau_{3,8}) + 3 (\tau_{2,5} + \tau_{2,6}) \tau_{4,16} + 3 \tau_{1,6} (\tau_{1,17} + \tau_{2,7} + \tau_{3,8} + \tau_{4,16})) \tau_{1,5} + \\
& \quad 3 \tau_{1,17} (\tau_{2,5} + \tau_{2,6})^2 - 2 \tau_{2,6} \tau_{2,7}^2 + 3 \tau_{2,7} \tau_{3,5}^2 + 3 \tau_{2,7} \tau_{3,6}^2 - 2 \tau_{2,6} \tau_{3,8}^2 + 2 \tau_{3,5} \tau_{3,8}^2 + 2 \tau_{3,6} \tau_{3,8}^2 + \\
& \quad 3 \tau_{2,7} \tau_{4,5}^2 + 3 \tau_{3,8} \tau_{4,5}^2 + 3 \tau_{2,7} \tau_{4,6}^2 + 3 \tau_{3,8} \tau_{4,6}^2 + 3 \tau_{1,17} (\tau_{3,5} + \tau_{3,6} + \tau_{4,5} + \tau_{4,6})^2 + \\
& \quad 2 (-\tau_{2,5} - \tau_{2,6} + \tau_{3,5} + \tau_{3,6} + \tau_{4,5} + \tau_{4,6}) \tau_{4,16}^2 + 3 \tau_{2,5}^2 \tau_{2,7} + 3 \tau_{2,6}^2 \tau_{2,7} + 2 \tau_{2,7}^2 \tau_{3,5} + 2 \tau_{2,7}^2 \tau_{3,6} + 6 \tau_{2,7} \tau_{3,5} \tau_{3,6} + \\
& \quad 3 \tau_{2,5}^2 \tau_{3,8} + 3 \tau_{2,6}^2 \tau_{3,8} + 3 \tau_{3,5}^2 \tau_{3,8} + 3 \tau_{3,6}^2 \tau_{3,8} - 4 \tau_{2,6} \tau_{2,7} \tau_{3,8} + 4 \tau_{2,7} \tau_{3,5} \tau_{3,8} + 4 \tau_{2,7} \tau_{3,6} \tau_{3,8} + 6 \tau_{3,5} \tau_{3,6} \tau_{3,8} + \\
& \quad 2 \tau_{2,5} (3 \tau_{2,6} - \tau_{2,7} - \tau_{3,8}) (\tau_{2,7} + \tau_{3,8}) + 2 \tau_{2,7}^2 \tau_{4,5} + 2 \tau_{3,8}^2 \tau_{4,5} + 6 \tau_{2,7} \tau_{3,5} \tau_{4,5} + 6 \tau_{2,7} \tau_{3,6} \tau_{4,5} + 4 \tau_{2,7} \tau_{3,8} \tau_{4,5} + \\
& \quad 6 \tau_{3,5} \tau_{3,8} \tau_{4,5} + 6 \tau_{3,6} \tau_{3,8} \tau_{4,5} + 2 \tau_{2,7}^2 \tau_{4,6} + 2 \tau_{3,8}^2 \tau_{4,6} + 6 \tau_{2,7} \tau_{3,5} \tau_{4,6} + 6 \tau_{2,7} \tau_{3,6} \tau_{4,6} + 4 \tau_{2,7} \tau_{3,8} \tau_{4,6} + \\
& \quad 6 \tau_{3,5} \tau_{3,8} \tau_{4,6} + 6 \tau_{3,6} \tau_{3,8} \tau_{4,6} + 6 \tau_{2,7} \tau_{4,5} \tau_{4,6} + 6 \tau_{3,8} \tau_{4,5} \tau_{4,6} + 2 \tau_{1,17}^2 (-\tau_{2,5} - \tau_{2,6} + \tau_{3,5} + \tau_{3,6} + \tau_{4,5} + \tau_{4,6}) + \\
& \quad (4 \tau_{1,17} (-\tau_{2,5} - \tau_{2,6} + \tau_{3,5} + \tau_{3,6} + \tau_{4,5} + \tau_{4,6}) + 3 ((\tau_{2,5} + \tau_{2,6})^2 + (\tau_{3,5} + \tau_{3,6} + \tau_{4,5} + \tau_{4,6})^2)) \tau_{4,16} + \\
& \quad 3 \tau_{1,6}^2 (\tau_{1,17} + \tau_{2,7} + \tau_{3,8} + \tau_{4,16}) - 2 \tau_{1,6} \\
& \quad (\tau_{1,17}^2 + (2 \tau_{4,16} - 3 (\tau_{2,5} + \tau_{2,6})) \tau_{1,17} + \tau_{4,16}^2 - (3 \tau_{2,5} + 3 \tau_{2,6} - \tau_{2,7} - \tau_{3,8}) (\tau_{2,7} + \tau_{3,8}) - 3 (\tau_{2,5} + \tau_{2,6}) \tau_{4,16})) + \\
& \quad u (s^2 - t^2 - u^2) ((\tau_{1,5} + \tau_{1,6} + \tau_{2,5} + \tau_{2,6} - 3 \tau_{2,7} - \tau_{3,5} - \tau_{3,6} - 3 \tau_{3,8} - \tau_{4,5} - \tau_{4,6}) \tau_{7,8} + \\
& \quad (\tau_{1,5} + \tau_{1,6} - 3 \tau_{1,17} + \tau_{2,5} + \tau_{2,6} - \tau_{3,5} - \tau_{3,6} - \tau_{4,5} - \tau_{4,6} - 3 \tau_{4,16}) \tau_{16,17} \Big) + \\
& \quad 2 u^3 (-(\tau_{2,7} + \tau_{3,8}) \tau_{7,8} - (\tau_{1,17} + \tau_{4,16}) \tau_{16,17} \Big) \Big)
\end{aligned}$$

■  $N_{38}^{(4)}$

$$\begin{aligned}
& \frac{1}{4} \left( 2 (\tau_{7,8}^2 + \tau_{16,17}^2) t^4 + \right. \\
& 2 ((\tau_{7,8} + \tau_{16,17}) \tau_{1,5}^2 + ((2 \tau_{1,6} + 2 \tau_{2,5} + 2 \tau_{2,6} - \tau_{2,7} - \tau_{3,8}) \tau_{7,8} + (2 \tau_{1,6} - \tau_{1,17} + 2 (\tau_{2,5} + \tau_{2,6}) - \tau_{4,16}) \tau_{16,17}) \tau_{1,5} + \\
& \tau_{1,6}^2 (\tau_{7,8} + \tau_{16,17}) + \tau_{2,5}^2 (\tau_{7,8} + \tau_{16,17}) + \tau_{2,6}^2 (\tau_{7,8} + \tau_{16,17}) - \tau_{2,6} ((\tau_{2,7} + \tau_{3,8}) \tau_{7,8} + (\tau_{1,17} + \tau_{4,16}) \tau_{16,17}) + \\
& \tau_{2,5} (-(-2 \tau_{2,6} + \tau_{2,7} + \tau_{3,8}) \tau_{7,8} - (\tau_{1,17} - 2 \tau_{2,6} + \tau_{4,16}) \tau_{16,17}) + \\
& \tau_{1,6} ((2 \tau_{2,5} + 2 \tau_{2,6} - \tau_{2,7} - \tau_{3,8}) \tau_{7,8} - (\tau_{1,17} - 2 (\tau_{2,5} + \tau_{2,6}) + \tau_{4,16}) \tau_{16,17}) + \\
& \left. (\tau_{3,5} + \tau_{3,6} + \tau_{4,5} + \tau_{4,6}) ((\tau_{2,7} + \tau_{3,5} + \tau_{3,6} + \tau_{3,8} + \tau_{4,5} + \tau_{4,6}) \tau_{7,8} + (\tau_{1,17} + \tau_{3,5} + \tau_{3,6} + \tau_{4,5} + \tau_{4,6} + \tau_{4,16}) \tau_{16,17}) \right) \\
& t^3 + (2 \tau_{1,5}^4 + (8 \tau_{1,6} - 2 (\tau_{1,17} - 4 \tau_{2,5} - 4 \tau_{2,6} + \tau_{2,7} + \tau_{3,8} + \tau_{4,16})) \tau_{1,5}^3 + \\
& (12 \tau_{1,6}^2 - 6 (\tau_{1,17} - 4 \tau_{2,5} - 4 \tau_{2,6} + \tau_{2,7} + \tau_{3,8} + \tau_{4,16}) \tau_{1,6} + \tau_{1,17}^2 + 12 \tau_{2,5}^2 + 12 \tau_{2,6}^2 + \tau_{2,7}^2 + \tau_{3,8}^2 + \tau_{4,16}^2 + \\
& 2 \tau_{2,7} \tau_{3,8} + 6 \tau_{2,5} (4 \tau_{2,6} - \tau_{2,7} - \tau_{3,8} - \tau_{4,16}) + 2 \tau_{1,17} (\tau_{4,16} - 3 (\tau_{2,5} + \tau_{2,6})) - 6 \tau_{2,6} (\tau_{2,7} + \tau_{3,8} + \tau_{4,16})) \tau_{1,5}^2 + \\
& 2 (\tau_{1,6} + \tau_{2,5} + \tau_{2,6}) (4 \tau_{1,6}^2 - (3 \tau_{1,17} - 8 \tau_{2,5} - 8 \tau_{2,6} + 3 (\tau_{2,7} + \tau_{3,8} + \tau_{4,16})) \tau_{1,6} + \tau_{1,17}^2 + 4 \tau_{2,5}^2 + \\
& 4 \tau_{2,6}^2 + \tau_{2,7}^2 + \tau_{3,8}^2 + \tau_{4,16}^2 + 2 \tau_{2,7} \tau_{3,8} - 3 \tau_{2,6} (\tau_{2,7} + \tau_{3,8} + \tau_{4,16}) + \tau_{1,17} (2 \tau_{4,16} - 3 (\tau_{2,5} + \tau_{2,6})) + \\
& \tau_{2,5} (8 \tau_{2,6} - 3 (\tau_{2,7} + \tau_{3,8} + \tau_{4,16}))) \tau_{1,5} + 2 \tau_{1,6}^4 + 2 \tau_{2,5}^4 + 2 \tau_{2,6}^4 + 2 \tau_{3,5}^4 + 2 \tau_{3,6}^4 + 2 \tau_{4,5}^4 + \\
& 2 \tau_{4,6}^4 + 2 \tau_{2,7} \tau_{3,5}^3 + 2 \tau_{2,7} \tau_{3,6}^3 + 8 \tau_{3,5} \tau_{3,6}^3 + 2 \tau_{2,7} \tau_{4,5}^3 + 8 \tau_{3,5} \tau_{4,5}^3 + 8 \tau_{3,6} \tau_{4,5}^3 + 2 \tau_{3,8} \tau_{4,5}^3 + \\
& 2 \tau_{2,7} \tau_{4,6}^3 + 8 \tau_{3,5} \tau_{4,6}^3 + 8 \tau_{3,6} \tau_{4,6}^3 + 2 \tau_{3,8} \tau_{4,6}^3 + 8 \tau_{4,5} \tau_{4,6}^3 + \tau_{2,6}^2 \tau_{2,7}^2 + \tau_{2,7}^2 \tau_{3,5}^2 + \tau_{2,7}^2 \tau_{3,6}^2 + \\
& 12 \tau_{3,5}^2 \tau_{3,6}^2 + 6 \tau_{2,7} \tau_{3,5} \tau_{3,6}^2 + \tau_{2,6}^2 \tau_{3,8}^2 + \tau_{3,5}^2 \tau_{3,8}^2 + \tau_{3,6}^2 \tau_{3,8}^2 + 2 \tau_{3,5} \tau_{3,6} \tau_{3,8}^2 + \tau_{2,7}^2 \tau_{4,5}^2 + 12 \tau_{3,5}^2 \tau_{4,5}^2 + \\
& 12 \tau_{3,6}^2 \tau_{4,5}^2 + \tau_{3,8}^2 \tau_{4,5}^2 + 6 \tau_{2,7} \tau_{3,5} \tau_{4,5}^2 + 6 \tau_{2,7} \tau_{3,6} \tau_{4,5}^2 + 24 \tau_{3,5} \tau_{3,6} \tau_{4,5}^2 + 2 \tau_{2,7} \tau_{3,8} \tau_{4,5}^2 + 6 \tau_{3,5} \tau_{3,8} \tau_{4,5}^2 + \\
& 6 \tau_{3,6} \tau_{3,8} \tau_{4,5}^2 + \tau_{2,7}^2 \tau_{4,6}^2 + 12 \tau_{3,5}^2 \tau_{4,6}^2 + 12 \tau_{3,6}^2 \tau_{4,6}^2 + \tau_{3,8}^2 \tau_{4,6}^2 + 12 \tau_{4,5}^2 \tau_{4,6}^2 + 6 \tau_{2,7} \tau_{3,5} \tau_{4,6}^2 + \\
& 6 \tau_{2,7} \tau_{3,6} \tau_{4,6}^2 + 24 \tau_{3,5} \tau_{3,6} \tau_{4,6}^2 + 2 \tau_{2,7} \tau_{3,8} \tau_{4,6}^2 + 6 \tau_{3,5} \tau_{3,8} \tau_{4,6}^2 + 6 \tau_{3,6} \tau_{3,8} \tau_{4,6}^2 + 6 \tau_{2,7} \tau_{4,5} \tau_{4,6}^2 + \\
& 24 \tau_{3,5} \tau_{4,5} \tau_{4,6}^2 + 24 \tau_{3,6} \tau_{4,5} \tau_{4,6}^2 + 6 \tau_{3,8} \tau_{4,5} \tau_{4,6}^2 + \tau_{2,6}^2 \tau_{4,16}^2 + \tau_{3,5}^2 \tau_{4,16}^2 + \tau_{3,6}^2 \tau_{4,16}^2 + \tau_{4,5}^2 \tau_{4,16}^2 + \\
& \tau_{4,6}^2 \tau_{4,16}^2 + 2 \tau_{3,5} \tau_{3,6} \tau_{4,16}^2 + 2 \tau_{3,5} \tau_{4,5} \tau_{4,16}^2 + 2 \tau_{3,6} \tau_{4,5} \tau_{4,16}^2 + 2 \tau_{3,5} \tau_{4,6} \tau_{4,16}^2 + 2 \tau_{3,6} \tau_{4,6} \tau_{4,16}^2 + \\
& 2 \tau_{4,5} \tau_{4,6} \tau_{4,16}^2 - 2 \tau_{2,6}^3 \tau_{2,7} + 8 \tau_{3,5}^3 \tau_{3,6} + 6 \tau_{2,7} \tau_{3,5}^2 \tau_{3,6} + 2 \tau_{2,7}^2 \tau_{3,5} \tau_{3,6} - 2 \tau_{2,6}^3 \tau_{3,8} + 2 \tau_{3,5}^3 \tau_{3,8} + \\
& 2 \tau_{3,6}^3 \tau_{3,8} + 2 \tau_{2,7} \tau_{3,5}^2 \tau_{3,8} + 2 \tau_{2,7} \tau_{3,6}^2 \tau_{3,8} + 6 \tau_{3,5} \tau_{3,6}^2 \tau_{3,8} + 2 \tau_{2,6}^2 \tau_{2,7} \tau_{3,8} + 6 \tau_{3,5}^2 \tau_{3,6} \tau_{3,8} + \\
& 4 \tau_{2,7} \tau_{3,5} \tau_{3,6} \tau_{3,8} + 8 \tau_{3,5}^3 \tau_{4,5} + 8 \tau_{3,6}^3 \tau_{4,5} + 6 \tau_{2,7} \tau_{3,5}^2 \tau_{4,5} + 6 \tau_{2,7} \tau_{3,6}^2 \tau_{4,5} + 24 \tau_{3,5} \tau_{3,6}^2 \tau_{4,5} + \\
& 2 \tau_{3,5} \tau_{3,8}^2 \tau_{4,5} + 2 \tau_{3,6} \tau_{3,8}^2 \tau_{4,5} + 2 \tau_{2,7}^2 \tau_{3,5} \tau_{4,5} + 2 \tau_{2,7}^2 \tau_{3,6} \tau_{4,5} + 24 \tau_{3,5}^2 \tau_{3,6} \tau_{4,5} + 12 \tau_{2,7} \tau_{3,5} \tau_{3,6} \tau_{4,5} + \\
& 6 \tau_{3,5}^2 \tau_{3,8} \tau_{4,5} + 6 \tau_{3,6}^2 \tau_{3,8} \tau_{4,5} + 4 \tau_{2,7} \tau_{3,5} \tau_{3,8} \tau_{4,5} + 4 \tau_{2,7} \tau_{3,6} \tau_{3,8} \tau_{4,5} + 12 \tau_{3,5} \tau_{3,6} \tau_{3,8} \tau_{4,5} + \\
& 8 \tau_{3,5}^3 \tau_{4,6} + 8 \tau_{3,6}^3 \tau_{4,6} + 8 \tau_{4,5}^3 \tau_{4,6} + 6 \tau_{2,7} \tau_{3,5}^2 \tau_{4,6} + 6 \tau_{2,7} \tau_{3,6}^2 \tau_{4,6} + 24 \tau_{3,5} \tau_{3,6}^2 \tau_{4,6} + 2 \tau_{3,5} \tau_{3,8}^2 \tau_{4,6} + \\
& 2 \tau_{3,6} \tau_{3,8}^2 \tau_{4,6} + 6 \tau_{2,7} \tau_{4,5}^2 \tau_{4,6} + 24 \tau_{3,5} \tau_{4,5}^2 \tau_{4,6} + 24 \tau_{3,6} \tau_{4,5}^2 \tau_{4,6} + 6 \tau_{3,8} \tau_{4,5}^2 \tau_{4,6} + 2 \tau_{2,7}^2 \tau_{3,5} \tau_{4,6} + \\
& 2 \tau_{2,7}^2 \tau_{3,6} \tau_{4,6} + 24 \tau_{3,5}^2 \tau_{3,6} \tau_{4,6} + 12 \tau_{2,7} \tau_{3,5} \tau_{3,6} \tau_{4,6} + 6 \tau_{3,5}^2 \tau_{3,8} \tau_{4,6} + 6 \tau_{3,6}^2 \tau_{3,8} \tau_{4,6} + 4 \tau_{2,7} \tau_{3,5} \tau_{3,8} \tau_{4,6} + \\
& 4 \tau_{2,7} \tau_{3,6} \tau_{3,8} \tau_{4,6} + 12 \tau_{3,5} \tau_{3,6} \tau_{3,8} \tau_{4,6} + 2 \tau_{2,7}^2 \tau_{4,5} \tau_{4,6} + 24 \tau_{3,5}^2 \tau_{4,5} \tau_{4,6} + 24 \tau_{3,6}^2 \tau_{4,5} \tau_{4,6} + \\
& 2 \tau_{3,8}^2 \tau_{4,5} \tau_{4,6} + 12 \tau_{2,7} \tau_{3,5} \tau_{4,5} \tau_{4,6} + 12 \tau_{2,7} \tau_{3,6} \tau_{4,5} \tau_{4,6} + 48 \tau_{3,5} \tau_{3,6} \tau_{4,5} \tau_{4,6} + 4 \tau_{2,7} \tau_{3,8} \tau_{4,5} \tau_{4,6} + \\
& 12 \tau_{3,5} \tau_{3,8} \tau_{4,5} \tau_{4,6} + 12 \tau_{3,6} \tau_{3,8} \tau_{4,5} \tau_{4,6} + \tau_{1,17}^2 ((\tau_{2,5} + \tau_{2,6})^2 + (\tau_{3,5} + \tau_{3,6} + \tau_{4,5} + \tau_{4,6})^2) - 2 \tau_{2,6}^3 \tau_{4,16} + \\
& 2 \tau_{3,5}^3 \tau_{4,16} + 2 \tau_{3,6}^3 \tau_{4,16} + 2 \tau_{4,5}^3 \tau_{4,16} + 2 \tau_{4,6}^3 \tau_{4,16} + 6 \tau_{3,5} \tau_{3,6}^2 \tau_{4,16} + 6 \tau_{3,5} \tau_{4,5}^2 \tau_{4,16} + 6 \tau_{3,6} \tau_{4,5}^2 \tau_{4,16} +
\end{aligned}$$

$$\begin{aligned}
& 6 \tau_{3,5} \tau_{4,6}^2 \tau_{4,16} + 6 \tau_{3,6} \tau_{4,6}^2 \tau_{4,16} + 6 \tau_{4,5} \tau_{4,6}^2 \tau_{4,16} + 6 \tau_{3,5}^2 \tau_{3,6} \tau_{4,16} + 6 \tau_{3,5}^2 \tau_{4,5} \tau_{4,16} + 6 \tau_{3,6}^2 \tau_{4,5} \tau_{4,16} + \\
& 12 \tau_{3,5} \tau_{3,6} \tau_{4,5} \tau_{4,16} + 6 \tau_{3,5}^2 \tau_{4,6} \tau_{4,16} + 6 \tau_{3,6}^2 \tau_{4,6} \tau_{4,16} + 6 \tau_{4,5}^2 \tau_{4,6} \tau_{4,16} + 12 \tau_{3,5} \tau_{3,6} \tau_{4,6} \tau_{4,16} + \\
& 12 \tau_{3,5} \tau_{4,5} \tau_{4,6} \tau_{4,16} + 12 \tau_{3,6} \tau_{4,5} \tau_{4,6} \tau_{4,16} - 2 \tau_{1,6}^3 (\tau_{1,17} - 4 \tau_{2,5} - 4 \tau_{2,6} + \tau_{2,7} + \tau_{3,8} + \tau_{4,16}) + \\
& \tau_{2,5}^3 (8 \tau_{2,6} - 2 (\tau_{2,7} + \tau_{3,8} + \tau_{4,16})) + \tau_{2,5}^2 (12 \tau_{2,6}^2 - 6 (\tau_{2,7} + \tau_{3,8} + \tau_{4,16}) \tau_{2,6} + (\tau_{2,7} + \tau_{3,8})^2 + \tau_{4,16}^2) + \\
& \tau_{1,6}^2 (\tau_{1,17}^2 + 2 (\tau_{4,16} - 3 (\tau_{2,5} + \tau_{2,6})) \tau_{1,17} + 12 \tau_{2,5}^2 + 12 \tau_{2,6}^2 + \tau_{2,7}^2 + \tau_{3,8}^2 + \\
& \tau_{4,16}^2 + 2 \tau_{2,7} \tau_{3,8} + 6 \tau_{2,5} (4 \tau_{2,6} - \tau_{2,7} - \tau_{3,8} - \tau_{4,16}) - 6 \tau_{2,6} (\tau_{2,7} + \tau_{3,8} + \tau_{4,16})) + \\
& 2 \tau_{2,5} \tau_{2,6} (4 \tau_{2,6}^2 - 3 (\tau_{2,7} + \tau_{3,8} + \tau_{4,16}) \tau_{2,6} + (\tau_{2,7} + \tau_{3,8})^2 + \tau_{4,16}^2) + 2 \tau_{1,17} (-\tau_{2,5}^3 + (\tau_{4,16} - 3 \tau_{2,6}) \tau_{2,5}^2 + \\
& \tau_{2,6} (2 \tau_{4,16} - 3 \tau_{2,6}) \tau_{2,5} - \tau_{2,6}^3 + \tau_{2,6}^2 \tau_{4,16} + (\tau_{3,5} + \tau_{3,6} + \tau_{4,5} + \tau_{4,6})^2 (\tau_{3,5} + \tau_{3,6} + \tau_{4,5} + \tau_{4,6} + \tau_{4,16})) + \\
& 2 \tau_{1,6} (\tau_{2,5} + \tau_{2,6}) (\tau_{1,17}^2 + (2 \tau_{4,16} - 3 (\tau_{2,5} + \tau_{2,6})) \tau_{1,17} + 4 \tau_{2,5}^2 + 4 \tau_{2,6}^2 + \tau_{2,7}^2 + \tau_{3,8}^2 + \tau_{4,16}^2 + \\
& 2 \tau_{2,7} \tau_{3,8} - 3 \tau_{2,6} (\tau_{2,7} + \tau_{3,8} + \tau_{4,16}) + \tau_{2,5} (8 \tau_{2,6} - 3 (\tau_{2,7} + \tau_{3,8} + \tau_{4,16}))) t^2 - \\
& 4 (-s^2 + t^2 + u^2) (\tau_{7,8}^2 + \tau_{16,17}^2) t^2 - 6 u (-s^2 + t^2 + u^2) (\tau_{7,8}^2 + \tau_{16,17}^2) t + \\
& (s^2 - t^2 - u^2) \\
& (2 (\tau_{7,8} + \tau_{16,17}) \tau_{1,5}^2 + ((4 \tau_{1,6} + 4 \tau_{2,5} + 4 \tau_{2,6} - 3 (\tau_{2,7} + \tau_{3,8})) \tau_{7,8} + (4 \tau_{1,6} - 3 \tau_{1,17} + 4 (\tau_{2,5} + \tau_{2,6}) - 3 \tau_{4,16}) \tau_{16,17}) \\
& \tau_{1,5} + 2 \tau_{1,6}^2 (\tau_{7,8} + \tau_{16,17}) + 2 \tau_{2,5}^2 (\tau_{7,8} + \tau_{16,17}) + 2 \tau_{2,6}^2 (\tau_{7,8} + \tau_{16,17}) + \\
& \tau_{2,5} ((4 \tau_{2,6} - 3 (\tau_{2,7} + \tau_{3,8})) \tau_{7,8} + (-3 \tau_{1,17} + 4 \tau_{2,6} - 3 \tau_{4,16}) \tau_{16,17}) + \\
& \tau_{1,6} ((4 \tau_{2,5} + 4 \tau_{2,6} - 3 (\tau_{2,7} + \tau_{3,8})) \tau_{7,8} + (-3 \tau_{1,17} + 4 (\tau_{2,5} + \tau_{2,6}) - 3 \tau_{4,16}) \tau_{16,17}) - \\
& 3 \tau_{2,6} ((\tau_{2,7} + \tau_{3,8}) \tau_{7,8} + (\tau_{1,17} + \tau_{4,16}) \tau_{16,17}) + (\tau_{3,5} + \tau_{3,6} + \tau_{4,5} + \tau_{4,6}) \\
& ((3 \tau_{2,7} + 2 \tau_{3,5} + 2 \tau_{3,6} + 3 \tau_{3,8} + 2 (\tau_{4,5} + \tau_{4,6})) \tau_{7,8} + (3 \tau_{1,17} + 2 (\tau_{3,5} + \tau_{3,6} + \tau_{4,5} + \tau_{4,6}) + 3 \tau_{4,16}) \tau_{16,17})) t + \\
& u^2 ((\tau_{1,5} + \tau_{1,6} + \tau_{2,5} + \tau_{2,6})^2 + (\tau_{3,5} + \tau_{3,6} + \tau_{4,5} + \tau_{4,6})^2) ((\tau_{2,7} + \tau_{3,8})^2 + (\tau_{1,17} + \tau_{4,16})^2) + \\
& (s^2 - t^2 - u^2) (- (\tau_{1,17} + \tau_{2,7} + \tau_{3,8} + \tau_{4,16}) \tau_{1,5}^3 + (\tau_{1,17}^2 + (2 \tau_{4,16} - 3 (\tau_{2,5} + \tau_{2,6})) \tau_{1,17} + \tau_{4,16}^2 - \\
& (3 \tau_{2,5} + 3 \tau_{2,6} - \tau_{2,7} - \tau_{3,8}) (\tau_{2,7} + \tau_{3,8}) - 3 (\tau_{2,5} + \tau_{2,6}) \tau_{4,16} - 3 \tau_{1,6} (\tau_{1,17} + \tau_{2,7} + \tau_{3,8} + \tau_{4,16})) \tau_{1,5}^2 - \\
& (\tau_{1,6} + \tau_{2,5} + \tau_{2,6}) (-2 \tau_{1,17}^2 + (3 (\tau_{2,5} + \tau_{2,6}) - 4 \tau_{4,16}) \tau_{1,17} - 2 \tau_{4,16}^2 + (\tau_{2,7} + \tau_{3,8}) (3 \tau_{2,5} + 3 \tau_{2,6} - 2 (\tau_{2,7} + \tau_{3,8}))) + \\
& 3 (\tau_{2,5} + \tau_{2,6}) \tau_{4,16} + 3 \tau_{1,6} (\tau_{1,17} + \tau_{2,7} + \tau_{3,8} + \tau_{4,16})) \tau_{1,5} + \tau_{2,7} \tau_{3,5}^3 + \tau_{2,7} \tau_{3,6}^3 + \tau_{2,7} \tau_{4,5}^3 + \\
& \tau_{3,8} \tau_{4,5}^3 + \tau_{2,7} \tau_{4,6}^3 + \tau_{3,8} \tau_{4,6}^3 + \tau_{2,6}^2 \tau_{2,7}^2 + \tau_{2,7}^2 \tau_{3,5}^2 + \tau_{2,7}^2 \tau_{3,6}^2 + 3 \tau_{2,7} \tau_{3,5} \tau_{3,6}^2 + \tau_{2,6}^2 \tau_{3,8}^2 + \\
& \tau_{3,5}^2 \tau_{3,8}^2 + \tau_{3,6}^2 \tau_{3,8}^2 + 2 \tau_{3,5} \tau_{3,6} \tau_{3,8}^2 + \tau_{2,7}^2 \tau_{4,5}^2 + \tau_{3,8}^2 \tau_{4,5}^2 + 3 \tau_{2,7} \tau_{3,5} \tau_{4,5}^2 + 3 \tau_{2,7} \tau_{3,6} \tau_{4,5}^2 + \\
& 2 \tau_{2,7} \tau_{3,8} \tau_{4,5}^2 + 3 \tau_{3,5} \tau_{3,8} \tau_{4,5}^2 + 3 \tau_{3,6} \tau_{3,8} \tau_{4,5}^2 + \tau_{2,7}^2 \tau_{4,6}^2 + \tau_{3,8}^2 \tau_{4,6}^2 + 3 \tau_{2,7} \tau_{3,5} \tau_{4,6}^2 + \\
& 3 \tau_{2,7} \tau_{3,6} \tau_{4,6}^2 + 2 \tau_{2,7} \tau_{3,8} \tau_{4,6}^2 + 3 \tau_{3,5} \tau_{3,8} \tau_{4,6}^2 + 3 \tau_{3,6} \tau_{3,8} \tau_{4,6}^2 + 3 \tau_{2,7} \tau_{4,5} \tau_{4,6}^2 + 3 \tau_{3,8} \tau_{4,5} \tau_{4,6}^2 + \\
& \tau_{2,6}^2 \tau_{4,16}^2 + \tau_{3,5}^2 \tau_{4,16}^2 + \tau_{3,6}^2 \tau_{4,16}^2 + \tau_{4,5}^2 \tau_{4,16}^2 + \tau_{4,6}^2 \tau_{4,16}^2 + 2 \tau_{3,5} \tau_{3,6} \tau_{4,16}^2 + 2 \tau_{3,5} \tau_{4,5} \tau_{4,16}^2 + \\
& 2 \tau_{3,6} \tau_{4,5} \tau_{4,16}^2 + 2 \tau_{3,5} \tau_{4,6} \tau_{4,16}^2 + 2 \tau_{3,6} \tau_{4,6} \tau_{4,16}^2 + 2 \tau_{4,5} \tau_{4,6} \tau_{4,16}^2 - \tau_{2,6}^3 \tau_{2,7} + 3 \tau_{2,7} \tau_{3,5}^2 \tau_{3,6} + \\
& 2 \tau_{2,7}^2 \tau_{3,5} \tau_{3,6} - \tau_{2,6}^3 \tau_{3,8} + \tau_{3,5}^3 \tau_{3,8} + \tau_{3,6}^3 \tau_{3,8} + 2 \tau_{2,7} \tau_{3,5}^2 \tau_{3,8} + 2 \tau_{2,7} \tau_{3,6}^2 \tau_{3,8} + 3 \tau_{3,5} \tau_{3,6}^2 \tau_{3,8} + \\
& 2 \tau_{2,6}^2 \tau_{2,7} \tau_{3,8} + 3 \tau_{3,5}^2 \tau_{3,6} \tau_{3,8} + 4 \tau_{2,7} \tau_{3,5} \tau_{3,6} \tau_{3,8} + 3 \tau_{2,7} \tau_{3,5}^2 \tau_{4,5} + 3 \tau_{2,7} \tau_{3,6}^2 \tau_{4,5} + 2 \tau_{3,5} \tau_{3,8}^2 \tau_{4,5} + \\
& 2 \tau_{3,6} \tau_{3,8}^2 \tau_{4,5} + 2 \tau_{2,7}^2 \tau_{3,5} \tau_{4,5} + 2 \tau_{2,7}^2 \tau_{3,6} \tau_{4,5} + 6 \tau_{2,7} \tau_{3,5} \tau_{3,6} \tau_{4,5} + 3 \tau_{3,5}^2 \tau_{3,8} \tau_{4,5} + 3 \tau_{3,6}^2 \tau_{3,8} \tau_{4,5} + \\
& 4 \tau_{2,7} \tau_{3,5} \tau_{3,8} \tau_{4,5} + 4 \tau_{2,7} \tau_{3,6} \tau_{3,8} \tau_{4,5} + 6 \tau_{3,5} \tau_{3,6} \tau_{3,8} \tau_{4,5} + 3 \tau_{2,7} \tau_{3,5}^2 \tau_{4,6} + 3 \tau_{2,7} \tau_{3,6}^2 \tau_{4,6} + 2 \tau_{3,5} \tau_{3,8}^2 \tau_{4,6} + \\
& 2 \tau_{3,6} \tau_{3,8}^2 \tau_{4,6} + 3 \tau_{2,7} \tau_{4,5}^2 \tau_{4,6} + 3 \tau_{3,8} \tau_{4,5}^2 \tau_{4,6} + 2 \tau_{2,7}^2 \tau_{3,5} \tau_{4,6} + 2 \tau_{2,7}^2 \tau_{3,6} \tau_{4,6} + 6 \tau_{2,7} \tau_{3,5} \tau_{3,6} \tau_{4,6} + \\
& 3 \tau_{3,5}^2 \tau_{3,8} \tau_{4,6} + 3 \tau_{3,6}^2 \tau_{3,8} \tau_{4,6} + 4 \tau_{2,7} \tau_{3,5} \tau_{3,8} \tau_{4,6} + 4 \tau_{2,7} \tau_{3,6} \tau_{3,8} \tau_{4,6} + 6 \tau_{3,5} \tau_{3,6} \tau_{3,8} \tau_{4,6} +
\end{aligned}$$

$$\begin{aligned}
& 2 \tau_{2,7}^2 \tau_{4,5} \tau_{4,6} + 2 \tau_{3,8}^2 \tau_{4,5} \tau_{4,6} + 6 \tau_{2,7} \tau_{3,5} \tau_{4,5} \tau_{4,6} + 6 \tau_{2,7} \tau_{3,6} \tau_{4,5} \tau_{4,6} + 4 \tau_{2,7} \tau_{3,8} \tau_{4,5} \tau_{4,6} + \\
& 6 \tau_{3,5} \tau_{3,8} \tau_{4,5} \tau_{4,6} + 6 \tau_{3,6} \tau_{3,8} \tau_{4,5} \tau_{4,6} + \tau_{1,17}^2 ((\tau_{2,5} + \tau_{2,6})^2 + (\tau_{3,5} + \tau_{3,6} + \tau_{4,5} + \tau_{4,6})^2) - \tau_{2,6}^3 \tau_{4,16} + \\
& \tau_{3,5}^3 \tau_{4,16} + \tau_{3,6}^3 \tau_{4,16} + \tau_{4,5}^3 \tau_{4,16} + \tau_{4,6}^3 \tau_{4,16} + 3 \tau_{3,5} \tau_{3,6}^2 \tau_{4,16} + 3 \tau_{3,5} \tau_{4,5}^2 \tau_{4,16} + 3 \tau_{3,6} \tau_{4,5}^2 \tau_{4,16} + \\
& 3 \tau_{3,5} \tau_{4,6}^2 \tau_{4,16} + 3 \tau_{3,6} \tau_{4,6}^2 \tau_{4,16} + 3 \tau_{4,5} \tau_{4,6}^2 \tau_{4,16} + 3 \tau_{3,5}^2 \tau_{3,6} \tau_{4,16} + 3 \tau_{3,5}^2 \tau_{4,5} \tau_{4,16} + 3 \tau_{3,6}^2 \tau_{4,5} \tau_{4,16} + \\
& 6 \tau_{3,5} \tau_{3,6} \tau_{4,5} \tau_{4,16} + 3 \tau_{3,5}^2 \tau_{4,6} \tau_{4,16} + 3 \tau_{3,6}^2 \tau_{4,6} \tau_{4,16} + 3 \tau_{4,5}^2 \tau_{4,6} \tau_{4,16} + 6 \tau_{3,5} \tau_{3,6} \tau_{4,6} \tau_{4,16} + \\
& 6 \tau_{3,5} \tau_{4,5} \tau_{4,6} \tau_{4,16} + 6 \tau_{3,6} \tau_{4,5} \tau_{4,6} \tau_{4,16} - \tau_{2,5}^3 (\tau_{2,7} + \tau_{3,8} + \tau_{4,16}) - \tau_{1,6}^3 (\tau_{1,17} + \tau_{2,7} + \tau_{3,8} + \tau_{4,16}) - \\
& \tau_{1,6} (\tau_{2,5} + \tau_{2,6}) (-2 \tau_{1,17}^2 + (3 (\tau_{2,5} + \tau_{2,6}) - 4 \tau_{4,16}) \tau_{1,17} - 2 \tau_{4,16}^2 + (\tau_{2,7} + \tau_{3,8}) (3 \tau_{2,5} + 3 \tau_{2,6} - 2 (\tau_{2,7} + \tau_{3,8})) + \\
& 3 (\tau_{2,5} + \tau_{2,6}) \tau_{4,16}) + \tau_{2,5}^2 ((\tau_{2,7} + \tau_{3,8})^2 + \tau_{4,16}^2 - 3 \tau_{2,6} (\tau_{2,7} + \tau_{3,8} + \tau_{4,16})) + \\
& \tau_{1,6}^2 (\tau_{1,17}^2 + (2 \tau_{4,16} - 3 (\tau_{2,5} + \tau_{2,6})) \tau_{1,17} + \tau_{4,16}^2 - (3 \tau_{2,5} + 3 \tau_{2,6} - \tau_{2,7} - \tau_{3,8}) (\tau_{2,7} + \tau_{3,8}) - 3 (\tau_{2,5} + \tau_{2,6}) \tau_{4,16}) + \\
& \tau_{1,17} (-\tau_{2,5}^3 + (2 \tau_{4,16} - 3 \tau_{2,6}) \tau_{2,5}^2 + \tau_{2,6} (4 \tau_{4,16} - 3 \tau_{2,6}) \tau_{2,5} - \tau_{2,6}^3 + 2 \tau_{2,6}^2 \tau_{4,16} + (\tau_{3,5} + \tau_{3,6} + \tau_{4,5} + \tau_{4,6})^2 \\
& (\tau_{3,5} + \tau_{3,6} + \tau_{4,5} + \tau_{4,6} + 2 \tau_{4,16})) + \tau_{2,5} \tau_{2,6} (2 ((\tau_{2,7} + \tau_{3,8})^2 + \tau_{4,16}^2) - 3 \tau_{2,6} (\tau_{2,7} + \tau_{3,8} + \tau_{4,16})) - \\
& 2 u^3 (\tau_{1,5} + \tau_{1,6} + \tau_{2,5} + \tau_{2,6} - \tau_{3,5} - \tau_{3,6} - \tau_{4,5} - \tau_{4,6}) ((\tau_{2,7} + \tau_{3,8}) \tau_{7,8} + (\tau_{1,17} + \tau_{4,16}) \tau_{16,17}) + \\
& 2 u^4 (\tau_{7,8}^2 + \tau_{16,17}^2) - \\
& 4 u^2 (-s^2 + t^2 + u^2) (\tau_{7,8}^2 + \tau_{16,17}^2) + \\
& u (s^2 - t^2 - u^2) \\
& ((\tau_{7,8} + \tau_{16,17}) \tau_{1,5}^2 + ((2 \tau_{1,6} + 2 \tau_{2,5} + 2 \tau_{2,6} - 3 (\tau_{2,7} + \tau_{3,8})) \tau_{7,8} + (2 \tau_{1,6} - 3 \tau_{1,17} + 2 (\tau_{2,5} + \tau_{2,6}) - 3 \tau_{4,16}) \tau_{16,17}) \tau_{1,5} + \\
& \tau_{1,6}^2 (\tau_{7,8} + \tau_{16,17}) + \tau_{2,5}^2 (\tau_{7,8} + \tau_{16,17}) + \tau_{2,6}^2 (\tau_{7,8} + \tau_{16,17}) + \\
& \tau_{2,5} ((2 \tau_{2,6} - 3 (\tau_{2,7} + \tau_{3,8})) \tau_{7,8} + (-3 \tau_{1,17} + 2 \tau_{2,6} - 3 \tau_{4,16}) \tau_{16,17}) + \\
& \tau_{1,6} ((2 \tau_{2,5} + 2 \tau_{2,6} - 3 (\tau_{2,7} + \tau_{3,8})) \tau_{7,8} + (-3 \tau_{1,17} + 2 (\tau_{2,5} + \tau_{2,6}) - 3 \tau_{4,16}) \tau_{16,17}) - \\
& 3 \tau_{2,6} ((\tau_{2,7} + \tau_{3,8}) \tau_{7,8} + (\tau_{1,17} + \tau_{4,16}) \tau_{16,17}) + (\tau_{3,5} + \tau_{3,6} + \tau_{4,5} + \tau_{4,6}) \\
& ((3 \tau_{2,7} + \tau_{3,5} + \tau_{3,6} + 3 \tau_{3,8} + \tau_{4,5} + \tau_{4,6}) \tau_{7,8} + (3 \tau_{1,17} + \tau_{3,5} + \tau_{3,6} + \tau_{4,5} + \tau_{4,6} + 3 \tau_{4,16}) \tau_{16,17})))
\end{aligned}$$

■  $N_{38}^{(5)}$

0

■  $N_{38}^{(6)}$

0

■  $N_{38}^{(7)}$

0

■  $N_{38}^{(8)}$

0
