# Supplementary material for: The Ultraviolet Behavior of N=8 Supergravity at Four Loops
Source: arXiv:0905.2326 ancillary file (2012-01-08)
Supplement: Supplementary file 34 [file SUGRA39.pdf]

## Integral 39: $\mathcal{I}_{39}$

$\mathcal{N} = 8$  four-point four-loop amplitude.

### ■ 2D plot of graph associated with $\mathcal{I}_{39}$

This fixes the labelling associated with the numerator expressions given below.

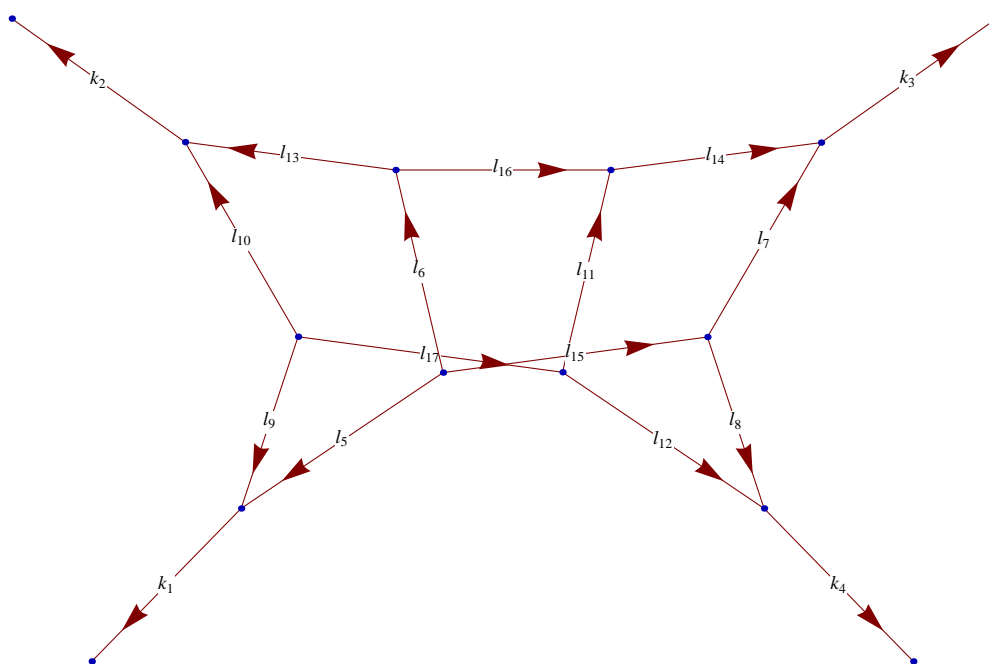

When using MathPlayer, by clicking three times (holding the click on the third click) directly on a vertex, one is able to move that vertex around, and its associated edges follow elastically. This functionality is absent when viewing as a pdf.

*Note: propagators for certain graphs were relabeled in the manuscript due to size constraints. The labels given in `aux/rawData/Neq8FourLoops.m` should be used for verification purposes.*

### ■ 3D plot of graph associated with $\mathcal{I}_{39}$

3D PLOT UNAVAILABLE FOR PDF. Please see .nb version for the 3D figure.

When using MathPlayer, by clicking anywhere in the image and dragging one should be able to rotate this 3D image. By holding (ALT) or (COMMAND) while clicking and moving the mouse up/down one should be able to zoom in/out. This functionality is absent when viewing as a pdf.

### "Vertex Form" of graph associated with $I_{39}$

This function returns the graph associated with the integral object in a vertex representation. This can be used as a way of specifying the topology of a graph using trivalent (cubic) vertices,  $\text{gVertex}[p_a, p_b, p_c]$ , where  $\{p_a, p_b, p_c\}$  are momenta labeling the propagators (edges) of the graph, and is understood that the edge labelled by  $p_a$  flows into the edge labelled by  $-p_a$ . Additionally, each vertex represents the manifest conservation of ( $D$  - dimensional) momenta :

$$\text{gVertex}[\{p_1, p_2, p_3\}] \iff (p_1 + p_2 + p_3 = 0)$$

$$\{\text{gVertex}(\{k_1, -l_9, -l_5\}), \text{gVertex}(\{k_2, -l_{13}, -l_{10}\}), \text{gVertex}(\{k_3, -l_7, -l_{14}\}), \text{gVertex}(\{k_4, -l_{12}, -l_8\}), \text{gVertex}(\{l_5, l_{15}, l_6\}), \\ \text{gVertex}(\{-l_6, l_{16}, l_{13}\}), \text{gVertex}(\{l_7, -l_{15}, l_8\}), \text{gVertex}(\{l_9, l_{10}, l_{17}\}), \text{gVertex}(\{-l_{11}, -l_{16}, l_{14}\}), \text{gVertex}(\{l_{11}, l_{12}, -l_{17}\})\}$$

### ■ Numerator expression for integral 39:

The following notation is used:  $\tau_{i,j} \equiv \begin{cases} 2 k_i \cdot l_j & \text{if } i \leq 4, j > 4 \\ 2 l_i \cdot l_j & \text{if } i, j > 4 \end{cases}$ .

$$s \equiv 2 k_1 \cdot k_2 = 2 k_3 \cdot k_4$$

We use  $s, t, u$  to represent the traditional Mandelstam variables for massless external four-point momenta:  $t \equiv 2 k_1 \cdot k_4 = 2 k_2 \cdot k_3$ .

$$u \equiv 2 k_1 \cdot k_3 = 2 k_2 \cdot k_4$$

Furthermore we use the shorthand  $(l_i)^2$  to represent the lorentz square:  $(l_i)^2 = l_i \cdot l_i$ .

**The total numerator  $N_{39}$  is given by summing over the following terms, distinguished here by explicit dependence on loop momenta:  $N_{39} = \sum_{i=0}^8 N_{39}^{(i)}$ :**

■  $N_{39}^{(0)}$

$$0$$

■  $N_{39}^{(1)}$

$$0$$

■  $N_{39}^{(2)}$

$$\frac{1}{2} s^2 t^2 (\tau_{1,6}^2 + \tau_{4,11}^2)$$

■  $N_{39}^{(3)}$

$$s t \left( \tau_{1,6} \left( s^2 \tau_{5,7} + \tau_{1,10} (t (\tau_{2,5} + \tau_{2,6}) - s \tau_{2,7}) + (\tau_{2,5} + \tau_{2,6}) (u \tau_{2,5} - s \tau_{3,5}) - s \tau_{1,7} \tau_{2,5} \right) + \right. \\ \left. \tau_{4,11} \left( s^2 \tau_{10,12} + \tau_{3,12} (-s \tau_{4,10} + t \tau_{4,7} + u \tau_{4,11}) - s \tau_{2,12} (\tau_{3,11} + \tau_{3,12}) - s \tau_{3,10} \tau_{4,7} + \right. \right. \\ \left. \left. \tau_{3,11} (t \tau_{4,7} + u \tau_{3,12}) + \tau_{2,7} \tau_{4,11} (t + u) + t \tau_{4,7} \tau_{4,11} + u \tau_{3,12}^2 \right) + \tau_{1,6}^2 (-s \tau_{3,10} + t \tau_{1,10} + u \tau_{2,5}) \right)$$

■  $N_{39}^{(4)}$ 

$$\begin{aligned}
& \frac{1}{8} (4 \tau_{5,7}^2 t^4 + 4 \tau_{10,12}^2 t^4 + 8 l_8^2 l_9^2 t^4 + 2 l_7^2 l_{10}^2 t^4 + 8 \tau_{2,6} \tau_{3,5} \tau_{5,7} t^3 + 8 \tau_{2,12} \tau_{3,11} \tau_{10,12} t^3 + 8 \tau_{2,12} \tau_{3,12} \tau_{10,12} t^3 + \\
& 8 \tau_{3,10} \tau_{4,7} \tau_{10,12} t^3 + 8 \tau_{3,11} \tau_{4,7} \tau_{10,12} t^3 + 8 \tau_{3,12} \tau_{4,7} \tau_{10,12} t^3 + 8 \tau_{3,12} \tau_{4,10} \tau_{10,12} t^3 + 8 \tau_{2,7} \tau_{4,11} \tau_{10,12} t^3 + \\
& 8 \tau_{4,7} \tau_{4,11} \tau_{10,12} t^3 + 4 \tau_{2,6}^2 \tau_{3,5}^2 t^2 + 4 \tau_{2,12}^2 \tau_{3,11}^2 t^2 + 4 \tau_{2,12}^2 \tau_{3,12}^2 t^2 + 4 \tau_{3,10}^2 \tau_{4,7}^2 t^2 + 4 \tau_{3,11}^2 \tau_{4,7}^2 t^2 + \\
& 4 \tau_{3,12}^2 \tau_{4,7}^2 t^2 + 8 \tau_{3,10} \tau_{3,11} \tau_{4,7}^2 t^2 + 8 \tau_{3,10} \tau_{3,12} \tau_{4,7}^2 t^2 + 8 \tau_{3,11} \tau_{3,12} \tau_{4,7}^2 t^2 + 4 \tau_{3,12}^2 \tau_{4,10}^2 t^2 + 4 \tau_{2,7}^2 \tau_{4,11}^2 t^2 + \\
& 4 \tau_{4,7}^2 \tau_{4,11}^2 t^2 + 8 \tau_{2,7} \tau_{4,7} \tau_{4,11}^2 t^2 - 8 (-s^2 + t^2 + u^2) \tau_{5,7}^2 t^2 - 8 (-s^2 + t^2 + u^2) \tau_{10,12}^2 t^2 + 8 \tau_{2,12}^2 \tau_{3,11} \tau_{3,12} t^2 + \\
& 8 \tau_{2,12} \tau_{3,11}^2 \tau_{4,7} t^2 + 8 \tau_{2,12} \tau_{3,12}^2 \tau_{4,7} t^2 + 8 \tau_{2,12} \tau_{3,10} \tau_{3,11} \tau_{4,7} t^2 + 8 \tau_{2,12} \tau_{3,10} \tau_{3,12} \tau_{4,7} t^2 + 16 \tau_{2,12} \tau_{3,11} \tau_{3,12} \tau_{4,7} t^2 + \\
& 8 \tau_{2,12} \tau_{3,12}^2 \tau_{4,10} t^2 + 8 \tau_{2,12} \tau_{3,11} \tau_{3,12} \tau_{4,10} t^2 + 8 \tau_{3,12}^2 \tau_{4,7} \tau_{4,10} t^2 + 8 \tau_{3,10} \tau_{3,12} \tau_{4,7} \tau_{4,10} t^2 + 8 \tau_{3,11} \tau_{3,12} \tau_{4,7} \tau_{4,10} t^2 + \\
& 8 \tau_{3,10} \tau_{4,7}^2 \tau_{4,11} t^2 + 8 \tau_{3,11} \tau_{4,7}^2 \tau_{4,11} t^2 + 8 \tau_{3,12} \tau_{4,7}^2 \tau_{4,11} t^2 + 8 \tau_{2,7} \tau_{2,12} \tau_{3,11} \tau_{4,11} t^2 + 8 \tau_{2,7} \tau_{2,12} \tau_{3,12} \tau_{4,11} t^2 + \\
& 8 \tau_{2,7} \tau_{3,10} \tau_{4,7} \tau_{4,11} t^2 + 8 \tau_{2,7} \tau_{3,11} \tau_{4,7} \tau_{4,11} t^2 + 8 \tau_{2,12} \tau_{3,11} \tau_{4,7} \tau_{4,11} t^2 + 8 \tau_{2,7} \tau_{3,12} \tau_{4,7} \tau_{4,11} t^2 + \\
& 8 \tau_{2,12} \tau_{3,12} \tau_{4,7} \tau_{4,11} t^2 + 8 \tau_{2,7} \tau_{3,12} \tau_{4,10} \tau_{4,11} t^2 + 8 \tau_{3,12} \tau_{4,7} \tau_{4,10} \tau_{4,11} t^2 - 32 (-s^2 + t^2 + u^2) l_8^2 l_9^2 t^2 - \\
& 12 (-s^2 + t^2 + u^2) l_7^2 l_{10}^2 t^2 - 12 u (-s^2 + t^2 + u^2) \tau_{5,7}^2 t - 12 u (-s^2 + t^2 + u^2) \tau_{10,12}^2 t - 12 (-s^2 + t^2 + u^2) \tau_{2,6} \tau_{3,5} \tau_{5,7} t - \\
& 4 (-s^2 + t^2 + u^2) \tau_{3,12}^2 \tau_{10,12} t - 12 (-s^2 + t^2 + u^2) \tau_{2,12} \tau_{3,11} \tau_{10,12} t - 12 (-s^2 + t^2 + u^2) \tau_{2,12} \tau_{3,12} \tau_{10,12} t - \\
& 4 (-s^2 + t^2 + u^2) \tau_{3,11} \tau_{3,12} \tau_{10,12} t - 12 (-s^2 + t^2 + u^2) \tau_{3,10} \tau_{4,7} \tau_{10,12} t - 8 (-s^2 + t^2 + u^2) \tau_{3,11} \tau_{4,7} \tau_{10,12} t - \\
& 8 (-s^2 + t^2 + u^2) \tau_{3,12} \tau_{4,7} \tau_{10,12} t - 12 (-s^2 + t^2 + u^2) \tau_{3,12} \tau_{4,10} \tau_{10,12} t - 12 (-s^2 + t^2 + u^2) \tau_{2,7} \tau_{4,11} \tau_{10,12} t - \\
& 4 (-s^2 + t^2 + u^2) \tau_{3,12} \tau_{4,11} \tau_{10,12} t - 8 (-s^2 + t^2 + u^2) \tau_{4,7} \tau_{4,11} \tau_{10,12} t - 40 u (-s^2 + t^2 + u^2) l_8^2 l_9^2 t - \\
& 23 u (-s^2 + t^2 + u^2) l_7^2 l_{10}^2 t + 4 u^2 \tau_{2,5}^4 + 4 u^2 \tau_{3,12}^4 + 8 u^2 \tau_{2,12} \tau_{3,12}^3 + 4 (s^2 - t^2 - u^2) \tau_{2,12} \tau_{3,12}^3 + \\
& 8 u^2 \tau_{3,11} \tau_{3,12}^3 + 4 s^2 \tau_{1,7}^2 \tau_{2,5}^2 + 4 \tau_{1,10}^2 (t (\tau_{2,5} + \tau_{2,6}) - s \tau_{2,7})^2 + 4 u^2 \tau_{2,6}^2 \tau_{3,5}^2 + 4 (s^2 - t^2 - u^2) \tau_{2,6}^2 \tau_{3,5}^2 + \\
& 4 \tau_{1,6}^2 (t \tau_{1,10} + u \tau_{2,5} - s \tau_{3,10})^2 + 4 u^2 \tau_{2,12}^2 \tau_{3,11}^2 + 4 (s^2 - t^2 - u^2) \tau_{2,12}^2 \tau_{3,11}^2 + 4 u^2 \tau_{2,12}^2 \tau_{3,12}^2 + \\
& 4 (s^2 - t^2 - u^2) \tau_{2,12}^2 \tau_{3,12}^2 + 4 u^2 \tau_{3,11}^2 \tau_{3,12}^2 + 16 u^2 \tau_{2,12} \tau_{3,11} \tau_{3,12}^2 + 8 (s^2 - t^2 - u^2) \tau_{2,12} \tau_{3,11} \tau_{3,12}^2 + \\
& 4 u^2 \tau_{3,10}^2 \tau_{4,7}^2 + 4 (s^2 - t^2 - u^2) \tau_{3,10}^2 \tau_{4,7}^2 + 4 (s^2 - t^2 - u^2) \tau_{3,10} \tau_{3,11} \tau_{4,7}^2 + 4 (s^2 - t^2 - u^2) \tau_{3,10} \tau_{3,12} \tau_{4,7}^2 + \\
& 4 u^2 \tau_{3,12}^2 \tau_{4,10}^2 + 4 (s^2 - t^2 - u^2) \tau_{3,12}^2 \tau_{4,10}^2 + 4 u^2 \tau_{2,7}^2 \tau_{4,11}^2 + 4 (s^2 - t^2 - u^2) \tau_{2,7}^2 \tau_{4,11}^2 + 4 u^2 \tau_{3,12}^2 \tau_{4,11}^2 + \\
& 8 u^2 \tau_{2,7} \tau_{3,12} \tau_{4,11}^2 + 4 (s^2 - t^2 - u^2) \tau_{2,7} \tau_{3,12} \tau_{4,11}^2 + 4 (s^2 - t^2 - u^2) \tau_{2,7} \tau_{4,7} \tau_{4,11}^2 + 4 (s^2 - t^2 - u^2) \tau_{3,12} \tau_{4,7} \tau_{4,11}^2 + \\
& 4 u^4 \tau_{5,7}^2 - 8 u^2 (-s^2 + t^2 + u^2) \tau_{5,7}^2 + 4 u^4 \tau_{10,12}^2 - 8 u^2 (-s^2 + t^2 + u^2) \tau_{10,12}^2 + 8 u \tau_{2,5}^3 (u \tau_{2,6} - s \tau_{3,5}) + \\
& 8 u^2 \tau_{2,12} \tau_{3,11}^2 \tau_{3,12} + 4 (s^2 - t^2 - u^2) \tau_{2,12} \tau_{3,11}^2 \tau_{3,12} + 8 u^2 \tau_{2,12}^2 \tau_{3,11} \tau_{3,12} + 8 (s^2 - t^2 - u^2) \tau_{2,12}^2 \tau_{3,11} \tau_{3,12} + \\
& 4 (s^2 - t^2 - u^2) \tau_{3,12}^3 \tau_{4,7} + 4 (s^2 - t^2 - u^2) \tau_{2,12} \tau_{3,11}^2 \tau_{4,7} + 4 (s^2 - t^2 - u^2) \tau_{2,12} \tau_{3,12}^2 \tau_{4,7} + \\
& 8 u^2 \tau_{3,10} \tau_{3,12}^2 \tau_{4,7} + 4 (s^2 - t^2 - u^2) \tau_{3,10} \tau_{3,12}^2 \tau_{4,7} + 8 (s^2 - t^2 - u^2) \tau_{3,11} \tau_{3,12}^2 \tau_{4,7} + 8 u^2 \tau_{2,12} \tau_{3,10} \tau_{3,11} \tau_{4,7} + \\
& 8 (s^2 - t^2 - u^2) \tau_{2,12} \tau_{3,10} \tau_{3,11} \tau_{4,7} + 4 (s^2 - t^2 - u^2) \tau_{3,11}^2 \tau_{3,12} \tau_{4,7} + 8 u^2 \tau_{2,12} \tau_{3,10} \tau_{3,12} \tau_{4,7} + \\
& 8 (s^2 - t^2 - u^2) \tau_{2,12} \tau_{3,10} \tau_{3,12} \tau_{4,7} + 8 (s^2 - t^2 - u^2) \tau_{2,12} \tau_{3,11} \tau_{3,12} \tau_{4,7} + 8 u^2 \tau_{3,10} \tau_{3,11} \tau_{3,12} \tau_{4,7} + \\
& 4 (s^2 - t^2 - u^2) \tau_{3,10} \tau_{3,11} \tau_{3,12} \tau_{4,7} + 8 u^2 \tau_{3,12}^3 \tau_{4,10} + 4 (s^2 - t^2 - u^2) \tau_{3,12}^3 \tau_{4,10} + 8 u^2 \tau_{2,12} \tau_{3,12}^2 \tau_{4,10} + \\
& 8 (s^2 - t^2 - u^2) \tau_{2,12} \tau_{3,12}^2 \tau_{4,10} + 8 u^2 \tau_{3,11} \tau_{3,12}^2 \tau_{4,10} + 4 (s^2 - t^2 - u^2) \tau_{3,11} \tau_{3,12}^2 \tau_{4,10} + 8 u^2 \tau_{2,12} \tau_{3,11} \tau_{3,12} \tau_{4,10} +
\end{aligned}$$

$$\begin{aligned}
& 8(s^2 - t^2 - u^2) \tau_{2,12} \tau_{3,11} \tau_{3,12} \tau_{4,10} + 4(s^2 - t^2 - u^2) \tau_{3,12}^2 \tau_{4,7} \tau_{4,10} + 8u^2 \tau_{3,10} \tau_{3,12} \tau_{4,7} \tau_{4,10} + \\
& 8(s^2 - t^2 - u^2) \tau_{3,10} \tau_{3,12} \tau_{4,7} \tau_{4,10} + 4(s^2 - t^2 - u^2) \tau_{3,11} \tau_{3,12} \tau_{4,7} \tau_{4,10} + 8u^2 \tau_{3,12}^3 \tau_{4,11} + 8u^2 \tau_{2,7} \tau_{3,12}^2 \tau_{4,11} + \\
& 4(s^2 - t^2 - u^2) \tau_{2,7} \tau_{3,12}^2 \tau_{4,11} + 8u^2 \tau_{2,12} \tau_{3,12}^2 \tau_{4,11} + 4(s^2 - t^2 - u^2) \tau_{2,12} \tau_{3,12}^2 \tau_{4,11} + 8u^2 \tau_{3,11} \tau_{3,12}^2 \tau_{4,11} + \\
& 4(s^2 - t^2 - u^2) \tau_{3,10} \tau_{4,7}^2 \tau_{4,11} + 8u^2 \tau_{2,7} \tau_{2,12} \tau_{3,11} \tau_{4,11} + 8(s^2 - t^2 - u^2) \tau_{2,7} \tau_{2,12} \tau_{3,11} \tau_{4,11} + 8u^2 \tau_{2,7} \tau_{2,12} \tau_{3,12} \tau_{4,11} + \\
& 8(s^2 - t^2 - u^2) \tau_{2,7} \tau_{2,12} \tau_{3,12} \tau_{4,11} + 8u^2 \tau_{2,7} \tau_{3,11} \tau_{3,12} \tau_{4,11} + 4(s^2 - t^2 - u^2) \tau_{2,7} \tau_{3,11} \tau_{3,12} \tau_{4,11} + \\
& 8u^2 \tau_{2,12} \tau_{3,11} \tau_{3,12} \tau_{4,11} + 4(s^2 - t^2 - u^2) \tau_{2,12} \tau_{3,11} \tau_{3,12} \tau_{4,11} + 8(s^2 - t^2 - u^2) \tau_{3,12}^2 \tau_{4,7} \tau_{4,11} + \\
& 8u^2 \tau_{2,7} \tau_{3,10} \tau_{4,7} \tau_{4,11} + 8(s^2 - t^2 - u^2) \tau_{2,7} \tau_{3,10} \tau_{4,7} \tau_{4,11} + 4(s^2 - t^2 - u^2) \tau_{2,7} \tau_{3,11} \tau_{4,7} \tau_{4,11} + \\
& 4(s^2 - t^2 - u^2) \tau_{2,12} \tau_{3,11} \tau_{4,7} \tau_{4,11} + 4(s^2 - t^2 - u^2) \tau_{2,7} \tau_{3,12} \tau_{4,7} \tau_{4,11} + 4(s^2 - t^2 - u^2) \tau_{2,12} \tau_{3,12} \tau_{4,7} \tau_{4,11} + \\
& 8u^2 \tau_{3,10} \tau_{3,12} \tau_{4,7} \tau_{4,11} + 4(s^2 - t^2 - u^2) \tau_{3,10} \tau_{3,12} \tau_{4,7} \tau_{4,11} + 8(s^2 - t^2 - u^2) \tau_{3,11} \tau_{3,12} \tau_{4,7} \tau_{4,11} + \\
& 8u^2 \tau_{3,12}^2 \tau_{4,10} \tau_{4,11} + 4(s^2 - t^2 - u^2) \tau_{3,12}^2 \tau_{4,10} \tau_{4,11} + 8u^2 \tau_{2,7} \tau_{3,12} \tau_{4,10} \tau_{4,11} + 8(s^2 - t^2 - u^2) \tau_{2,7} \tau_{3,12} \tau_{4,10} \tau_{4,11} + \\
& 4(s^2 - t^2 - u^2) \tau_{3,12} \tau_{4,7} \tau_{4,10} \tau_{4,11} + 8u^3 \tau_{2,6} \tau_{3,5} \tau_{5,7} - 12u(-s^2 + t^2 + u^2) \tau_{2,6} \tau_{3,5} \tau_{5,7} - \\
& 8s \tau_{2,5} (s \tau_{3,5} - u \tau_{2,6}) (s \tau_{5,7} - \tau_{2,6} \tau_{3,5}) + 8 \tau_{1,10} (t(\tau_{2,5} + \tau_{2,6}) - s \tau_{2,7}) (\tau_{5,7} s^2 + (\tau_{2,5} + \tau_{2,6})(u \tau_{2,5} - s \tau_{3,5})) - \\
& 8s \tau_{1,7} \tau_{2,5} (\tau_{5,7} s^2 + \tau_{1,10} (t(\tau_{2,5} + \tau_{2,6}) - s \tau_{2,7}) + (\tau_{2,5} + \tau_{2,6})(u \tau_{2,5} - s \tau_{3,5})) + \\
& 8 \tau_{1,6} (t \tau_{1,10} + u \tau_{2,5} - s \tau_{3,10}) (\tau_{5,7} s^2 - \tau_{1,7} \tau_{2,5} s + \tau_{1,10} (t(\tau_{2,5} + \tau_{2,6}) - s \tau_{2,7}) + (\tau_{2,5} + \tau_{2,6})(u \tau_{2,5} - s \tau_{3,5})) + \\
& 4 \tau_{2,5}^2 ((\tau_{3,5}^2 + 2u \tau_{5,7}) s^2 - 4u \tau_{2,6} \tau_{3,5} s + u^2 \tau_{2,6}^2) + 8u^3 \tau_{3,12}^2 \tau_{10,12} - 8u(-s^2 + t^2 + u^2) \tau_{3,12}^2 \tau_{10,12} + \\
& 8u^3 \tau_{2,12} \tau_{3,11} \tau_{10,12} - 12u(-s^2 + t^2 + u^2) \tau_{2,12} \tau_{3,11} \tau_{10,12} + 8u^3 \tau_{2,12} \tau_{3,12} \tau_{10,12} - 12u(-s^2 + t^2 + u^2) \tau_{2,12} \tau_{3,12} \tau_{10,12} + \\
& 8u^3 \tau_{3,11} \tau_{3,12} \tau_{10,12} - 8u(-s^2 + t^2 + u^2) \tau_{3,11} \tau_{3,12} \tau_{10,12} + 8u^3 \tau_{3,10} \tau_{4,7} \tau_{10,12} - 12u(-s^2 + t^2 + u^2) \tau_{3,10} \tau_{4,7} \tau_{10,12} - \\
& 4u(-s^2 + t^2 + u^2) \tau_{3,11} \tau_{4,7} \tau_{10,12} - 4u(-s^2 + t^2 + u^2) \tau_{3,12} \tau_{4,7} \tau_{10,12} + 8u^3 \tau_{3,12} \tau_{4,10} \tau_{10,12} - \\
& 12u(-s^2 + t^2 + u^2) \tau_{3,12} \tau_{4,10} \tau_{10,12} + 8u^3 \tau_{2,7} \tau_{4,11} \tau_{10,12} - 12u(-s^2 + t^2 + u^2) \tau_{2,7} \tau_{4,11} \tau_{10,12} + 8u^3 \tau_{3,12} \tau_{4,11} \tau_{10,12} - \\
& 8u(-s^2 + t^2 + u^2) \tau_{3,12} \tau_{4,11} \tau_{10,12} - 4u(-s^2 + t^2 + u^2) \tau_{4,7} \tau_{4,11} \tau_{10,12} - 24u^4 l_8^2 l_9^2 + 4u^4 l_7^2 l_{10}^2 - 14u^2(-s^2 + t^2 + u^2) l_7^2 l_{10}^2)
\end{aligned}$$

■  $N_{39}^{(5)}$

$$\begin{aligned}
& \frac{1}{8} s (6 \tau_{1,12} l_8^2 l_9^2 s^2 + 6 \tau_{2,5} l_8^2 l_9^2 s^2 + 16 \tau_{2,7} l_8^2 l_9^2 s^2 - 10 \tau_{2,12} l_8^2 l_9^2 s^2 - 10 \tau_{3,5} l_8^2 l_9^2 s^2 + 16 \tau_{3,10} l_8^2 l_9^2 s^2 + \\
& 6 \tau_{3,12} l_8^2 l_9^2 s^2 + 6 \tau_{4,5} l_8^2 l_9^2 s^2 + 2 \tau_{4,12} l_8^2 l_9^2 s^2 + 2(s^2 + 9t^2 - 7u^2) \tau_{1,5} l_8^2 l_9^2 + 12(t^2 - u^2) \tau_{1,7} l_8^2 l_9^2 - \\
& 12t^2 \tau_{1,10} l_8^2 l_9^2 + 12u^2 \tau_{1,10} l_8^2 l_9^2 - 18t^2 \tau_{1,12} l_8^2 l_9^2 + 14u^2 \tau_{1,12} l_8^2 l_9^2 - 2t^2 \tau_{2,5} l_8^2 l_9^2 - 2u^2 \tau_{2,5} l_8^2 l_9^2 - \\
& 20t^2 \tau_{2,7} l_8^2 l_9^2 + 20u^2 \tau_{2,7} l_8^2 l_9^2 + 14t^2 \tau_{2,12} l_8^2 l_9^2 - 18u^2 \tau_{2,12} l_8^2 l_9^2 + 14t^2 \tau_{3,5} l_8^2 l_9^2 - 18u^2 \tau_{3,5} l_8^2 l_9^2 - \\
& 20t^2 \tau_{3,10} l_8^2 l_9^2 + 20u^2 \tau_{3,10} l_8^2 l_9^2 - 2t^2 \tau_{3,12} l_8^2 l_9^2 - 2u^2 \tau_{3,12} l_8^2 l_9^2 - 18t^2 \tau_{4,5} l_8^2 l_9^2 + 14u^2 \tau_{4,5} l_8^2 l_9^2 - \\
& 12t^2 \tau_{4,7} l_8^2 l_9^2 + 12u^2 \tau_{4,7} l_8^2 l_9^2 + 12t^2 \tau_{4,10} l_8^2 l_9^2 - 12u^2 \tau_{4,10} l_8^2 l_9^2 + 18t^2 \tau_{4,12} l_8^2 l_9^2 - 14u^2 \tau_{4,12} l_8^2 l_9^2 + \\
& (-4 \tau_{2,9} s^2 - 4 \tau_{2,12} s^2 - 4 \tau_{2,13} s^2 + 4 \tau_{2,14} s^2 - 4 \tau_{3,5} s^2 - 4 \tau_{3,8} s^2 + 4 \tau_{3,13} s^2 - 4 \tau_{3,14} s^2 + 6 \tau_{4,5} s^2 - 5 \tau_{4,9} s^2 + \\
& 3 \tau_{4,13} s^2 + 2(4t + u) \tau_{1,8} s + 2(3s^2 - 2(t^2 + u^2)) \tau_{1,12} - 4(5s^2 - t^2 + u^2) \tau_{1,13} + (3s^2 - t^2 - 7u^2) \tau_{1,14} + \\
& 4u^2 \tau_{2,9} - 4t^2 \tau_{2,12} + 4u^2 \tau_{2,12} - 4u^2 \tau_{2,13} - 4t^2 \tau_{2,14} + 4u^2 \tau_{2,14} - 4t^2 \tau_{3,5} + 4u^2 \tau_{3,5} + 4u^2 \tau_{3,8} - 4t^2 \tau_{3,13} + \\
& 4u^2 \tau_{3,13} - 4u^2 \tau_{3,14} - 4t^2 \tau_{4,5} - 4u^2 \tau_{4,5} - 3t^2 \tau_{4,9} + 3u^2 \tau_{4,9} - t^2 \tau_{4,13} - 7u^2 \tau_{4,13} - 4(5s^2 - t^2 + u^2) \tau_{4,14}) l_7^2 l_{10}^2)
\end{aligned}$$

■  $N_{39}^{(6)}$

$$\begin{aligned}
& \frac{1}{8} (8 \tau_{5,7} l_8^2 l_9^2 s^3 + 8 \tau_{10,12} l_8^2 l_9^2 s^3 - 8 \tau_{5,8} l_7^2 l_{10}^2 s^3 - 8 \tau_{9,12} l_7^2 l_{10}^2 s^3 - 8 \tau_{1,5}^2 l_8^2 l_9^2 s^2 - 8 \tau_{1,7}^2 l_8^2 l_9^2 s^2 - 8 \tau_{1,10}^2 l_8^2 l_9^2 s^2 - \\
& 6 \tau_{2,7}^2 l_8^2 l_9^2 s^2 + 6 \tau_{2,12}^2 l_8^2 l_9^2 s^2 + 6 \tau_{3,5}^2 l_8^2 l_9^2 s^2 - 6 \tau_{3,10}^2 l_8^2 l_9^2 s^2 - 8 \tau_{4,5}^2 l_8^2 l_9^2 s^2 - 8 \tau_{4,7}^2 l_8^2 l_9^2 s^2 - 8 \tau_{4,10}^2 l_8^2 l_9^2 s^2 - \\
& 8 \tau_{4,12}^2 l_8^2 l_9^2 s^2 + 20 \tau_{2,5} \tau_{2,7} l_8^2 l_9^2 s^2 - 20 \tau_{2,5} \tau_{2,12} l_8^2 l_9^2 s^2 + 10 \tau_{2,5} \tau_{3,5} l_8^2 l_9^2 s^2 + 34 \tau_{2,7} \tau_{3,5} l_8^2 l_9^2 s^2 - 48 \tau_{2,12} \tau_{3,5} l_8^2 l_9^2 s^2 - \\
& 10 \tau_{2,5} \tau_{3,10} l_8^2 l_9^2 s^2 - 20 \tau_{2,7} \tau_{3,10} l_8^2 l_9^2 s^2 + 34 \tau_{2,12} \tau_{3,10} l_8^2 l_9^2 s^2 - 10 \tau_{2,7} \tau_{3,12} l_8^2 l_9^2 s^2 + 10 \tau_{2,12} \tau_{3,12} l_8^2 l_9^2 s^2 - \\
& 20 \tau_{3,5} \tau_{3,12} l_8^2 l_9^2 s^2 + 20 \tau_{3,10} \tau_{3,12} l_8^2 l_9^2 s^2 - 8 \tau_{2,5} \tau_{4,5} l_8^2 l_9^2 s^2 - 16 \tau_{2,7} \tau_{4,5} l_8^2 l_9^2 s^2 + 8 \tau_{2,12} \tau_{4,5} l_8^2 l_9^2 s^2 - \\
& 2 \tau_{3,5} \tau_{4,5} l_8^2 l_9^2 s^2 + 2 \tau_{3,10} \tau_{4,5} l_8^2 l_9^2 s^2 - 8 \tau_{3,12} \tau_{4,5} l_8^2 l_9^2 s^2 - 4 \tau_{2,5} \tau_{4,7} l_8^2 l_9^2 s^2 - 10 \tau_{2,7} \tau_{4,7} l_8^2 l_9^2 s^2 + 10 \tau_{2,12} \tau_{4,7} l_8^2 l_9^2 s^2 + \\
& 2 \tau_{3,5} \tau_{4,7} l_8^2 l_9^2 s^2 - 10 \tau_{3,10} \tau_{4,7} l_8^2 l_9^2 s^2 + 8 \tau_{3,12} \tau_{4,7} l_8^2 l_9^2 s^2 - 4 \tau_{4,5} \tau_{4,7} l_8^2 l_9^2 s^2 + 8 \tau_{2,5} \tau_{4,10} l_8^2 l_9^2 s^2 + 14 \tau_{2,7} \tau_{4,10} l_8^2 l_9^2 s^2 - \\
& 6 \tau_{2,12} \tau_{4,10} l_8^2 l_9^2 s^2 + 6 \tau_{3,5} \tau_{4,10} l_8^2 l_9^2 s^2 - 6 \tau_{3,10} \tau_{4,10} l_8^2 l_9^2 s^2 + 16 \tau_{4,5} \tau_{4,10} l_8^2 l_9^2 s^2 + 4 \tau_{4,7} \tau_{4,10} l_8^2 l_9^2 s^2 + \\
& 8 \tau_{2,5} \tau_{4,12} l_8^2 l_9^2 s^2 + 14 \tau_{2,7} \tau_{4,12} l_8^2 l_9^2 s^2 - 14 \tau_{2,12} \tau_{4,12} l_8^2 l_9^2 s^2 - 8 \tau_{3,5} \tau_{4,12} l_8^2 l_9^2 s^2 + 12 \tau_{3,10} \tau_{4,12} l_8^2 l_9^2 s^2 - \\
& 8 \tau_{3,12} \tau_{4,12} l_8^2 l_9^2 s^2 + 16 \tau_{4,7} \tau_{4,12} l_8^2 l_9^2 s^2 - 4 \tau_{4,10} \tau_{4,12} l_8^2 l_9^2 s^2 + \tau_{1,8}^2 l_7^2 l_{10}^2 s^2 + 8 \tau_{1,13}^2 l_7^2 l_{10}^2 s^2 + 2 \tau_{1,14}^2 l_7^2 l_{10}^2 s^2 + \\
& \tau_{4,5}^2 l_7^2 l_{10}^2 s^2 + \tau_{4,9}^2 l_7^2 l_{10}^2 s^2 + 2 \tau_{4,13}^2 l_7^2 l_{10}^2 s^2 + 8 \tau_{4,14}^2 l_7^2 l_{10}^2 s^2 + 12 \tau_{1,8} \tau_{1,13} l_7^2 l_{10}^2 s^2 - 2 \tau_{1,8} \tau_{1,14} l_7^2 l_{10}^2 s^2 - \\
& 8 \tau_{1,13} \tau_{1,14} l_7^2 l_{10}^2 s^2 - 4 \tau_{1,14} \tau_{2,9} l_7^2 l_{10}^2 s^2 + 8 \tau_{1,13} \tau_{2,12} l_7^2 l_{10}^2 s^2 - 4 \tau_{2,9} \tau_{2,12} l_7^2 l_{10}^2 s^2 + 4 \tau_{2,12} \tau_{2,13} l_7^2 l_{10}^2 s^2 - \\
& 4 \tau_{2,9} \tau_{2,14} l_7^2 l_{10}^2 s^2 - 8 \tau_{1,8} \tau_{3,5} l_7^2 l_{10}^2 s^2 + 4 \tau_{1,13} \tau_{3,8} l_7^2 l_{10}^2 s^2 - 4 \tau_{3,5} \tau_{3,8} l_7^2 l_{10}^2 s^2 - 8 \tau_{1,8} \tau_{3,13} l_7^2 l_{10}^2 s^2 - \\
& 4 \tau_{3,8} \tau_{3,13} l_7^2 l_{10}^2 s^2 + 4 \tau_{3,5} \tau_{3,14} l_7^2 l_{10}^2 s^2 - 4 \tau_{1,8} \tau_{4,5} l_7^2 l_{10}^2 s^2 - 4 \tau_{1,14} \tau_{4,5} l_7^2 l_{10}^2 s^2 + 4 \tau_{3,8} \tau_{4,5} l_7^2 l_{10}^2 s^2 - \\
& 4 \tau_{3,14} \tau_{4,5} l_7^2 l_{10}^2 s^2 - 4 \tau_{1,14} \tau_{4,9} l_7^2 l_{10}^2 s^2 - 8 \tau_{2,12} \tau_{4,9} l_7^2 l_{10}^2 s^2 - 8 \tau_{2,14} \tau_{4,9} l_7^2 l_{10}^2 s^2 - 4 \tau_{1,8} \tau_{4,13} l_7^2 l_{10}^2 s^2 - \\
& 8 \tau_{1,14} \tau_{4,13} l_7^2 l_{10}^2 s^2 - 4 \tau_{3,8} \tau_{4,13} l_7^2 l_{10}^2 s^2 + 2 \tau_{4,5} \tau_{4,13} l_7^2 l_{10}^2 s^2 - 2 \tau_{4,9} \tau_{4,13} l_7^2 l_{10}^2 s^2 + 4 \tau_{2,9} \tau_{4,14} l_7^2 l_{10}^2 s^2 + \\
& 8 \tau_{3,5} \tau_{4,14} l_7^2 l_{10}^2 s^2 - 12 \tau_{4,5} \tau_{4,14} l_7^2 l_{10}^2 s^2 + 12 \tau_{4,9} \tau_{4,14} l_7^2 l_{10}^2 s^2 - 8 \tau_{4,13} \tau_{4,14} l_7^2 l_{10}^2 s^2 + \tau_{1,12}^2 (l_7^2 l_{10}^2 - 8 l_8^2 l_9^2) s^2 + \\
& 4 \tau_{1,10} ((3t - u) \tau_{1,12} + 5u \tau_{2,7} + (2t - 3u) \tau_{2,12} - (3t + 2u) (\tau_{3,5} - \tau_{3,10}) + s(2\tau_{2,5} - \tau_{3,12})) l_8^2 l_9^2 s + \\
& 4 \tau_{1,7} ((u - 3t) \tau_{1,10} + 4s \tau_{1,12} + 2(t - u) \tau_{2,5} + (t + 2u) \tau_{2,7} - (t + 2u) \tau_{2,12} + t \tau_{3,5} + 2u \tau_{3,5} - 3t \tau_{3,10} - 4u \tau_{3,10} - \\
& 2t \tau_{3,12} - 2u \tau_{3,12}) l_8^2 l_9^2 s + 4 \tau_{1,5} ((3t - u) \tau_{1,7} + 4s \tau_{1,10} + 2(u - t) \tau_{1,12} - 2s \tau_{2,5} - t \tau_{2,7} - 5u \tau_{2,7} + \\
& 4u \tau_{2,12} + 4t \tau_{3,5} + 3u \tau_{3,5} - 4t \tau_{3,10} - 3u \tau_{3,10} - 2(t + u) \tau_{3,12}) l_8^2 l_9^2 s + 2t^2 \tau_{2,7}^2 l_8^2 l_9^2 s - 2u^2 \tau_{2,7}^2 l_8^2 l_9^2 s + \\
& 2t^2 \tau_{2,12}^2 l_8^2 l_9^2 s - 2u^2 \tau_{2,12}^2 l_8^2 l_9^2 s + 2t^2 \tau_{3,5}^2 l_8^2 l_9^2 s - 2u^2 \tau_{3,5}^2 l_8^2 l_9^2 s + 2t^2 \tau_{3,10}^2 l_8^2 l_9^2 s - 2u^2 \tau_{3,10}^2 l_8^2 l_9^2 s - \\
& 12t^2 \tau_{2,5} \tau_{2,7} l_8^2 l_9^2 s + 12u^2 \tau_{2,5} \tau_{2,7} l_8^2 l_9^2 s + 12t^2 \tau_{2,5} \tau_{2,12} l_8^2 l_9^2 s - 12u^2 \tau_{2,5} \tau_{2,12} l_8^2 l_9^2 s - 4t^2 \tau_{2,7} \tau_{2,12} l_8^2 l_9^2 s + \\
& 4u^2 \tau_{2,7} \tau_{2,12} l_8^2 l_9^2 s - 2t^2 \tau_{2,5} \tau_{3,5} l_8^2 l_9^2 s + 2u^2 \tau_{2,5} \tau_{3,5} l_8^2 l_9^2 s + 2t^2 \tau_{2,7} \tau_{3,5} l_8^2 l_9^2 s - 2u^2 \tau_{2,7} \tau_{3,5} l_8^2 l_9^2 s + 2t^2 \tau_{2,5} \tau_{3,10} l_8^2 l_9^2 s - \\
& 2u^2 \tau_{2,5} \tau_{3,10} l_8^2 l_9^2 s - 4t^2 \tau_{2,7} \tau_{3,10} l_8^2 l_9^2 s + 4u^2 \tau_{2,7} \tau_{3,10} l_8^2 l_9^2 s + 2t^2 \tau_{2,12} \tau_{3,10} l_8^2 l_9^2 s - 2u^2 \tau_{2,12} \tau_{3,10} l_8^2 l_9^2 s - \\
& 4t^2 \tau_{3,5} \tau_{3,10} l_8^2 l_9^2 s + 4u^2 \tau_{3,5} \tau_{3,10} l_8^2 l_9^2 s + 2t^2 \tau_{2,7} \tau_{3,12} l_8^2 l_9^2 s - 2u^2 \tau_{2,7} \tau_{3,12} l_8^2 l_9^2 s - 2t^2 \tau_{2,12} \tau_{3,12} l_8^2 l_9^2 s + \\
& 2u^2 \tau_{2,12} \tau_{3,12} l_8^2 l_9^2 s + 12t^2 \tau_{3,5} \tau_{3,12} l_8^2 l_9^2 s - 12u^2 \tau_{3,5} \tau_{3,12} l_8^2 l_9^2 s - 12t^2 \tau_{3,10} \tau_{3,12} l_8^2 l_9^2 s + 12u^2 \tau_{3,10} \tau_{3,12} l_8^2 l_9^2 s + \\
& 2t^2 \tau_{3,5} \tau_{4,5} l_8^2 l_9^2 s - 2u^2 \tau_{3,5} \tau_{4,5} l_8^2 l_9^2 s - 2t^2 \tau_{3,10} \tau_{4,5} l_8^2 l_9^2 s + 2u^2 \tau_{3,10} \tau_{4,5} l_8^2 l_9^2 s + 8t^2 \tau_{3,12} \tau_{4,5} l_8^2 l_9^2 s - 8u^2 \tau_{3,12} \tau_{4,5} l_8^2 l_9^2 s - \\
& 2t^2 \tau_{2,7} \tau_{4,7} l_8^2 l_9^2 s + 2u^2 \tau_{2,7} \tau_{4,7} l_8^2 l_9^2 s + 2t^2 \tau_{2,12} \tau_{4,7} l_8^2 l_9^2 s - 2u^2 \tau_{2,12} \tau_{4,7} l_8^2 l_9^2 s - 10t^2 \tau_{3,5} \tau_{4,7} l_8^2 l_9^2 s + 10u^2 \tau_{3,5} \tau_{4,7} l_8^2 l_9^2 s + \\
& 10t^2 \tau_{3,10} \tau_{4,7} l_8^2 l_9^2 s - 10u^2 \tau_{3,10} \tau_{4,7} l_8^2 l_9^2 s - 8t^2 \tau_{4,5} \tau_{4,7} l_8^2 l_9^2 s + 8u^2 \tau_{4,5} \tau_{4,7} l_8^2 l_9^2 s - 2t^2 \tau_{2,7} \tau_{4,10} l_8^2 l_9^2 s + \\
& 2u^2 \tau_{2,7} \tau_{4,10} l_8^2 l_9^2 s + 2t^2 \tau_{2,12} \tau_{4,10} l_8^2 l_9^2 s - 2u^2 \tau_{2,12} \tau_{4,10} l_8^2 l_9^2 s - 2t^2 \tau_{3,5} \tau_{4,10} l_8^2 l_9^2 s + 2u^2 \tau_{3,5} \tau_{4,10} l_8^2 l_9^2 s +
\end{aligned}$$

$$\begin{aligned}
& 2t^2 \tau_{3,10} \tau_{4,10} l_8^2 l_9^2 - 2u^2 \tau_{3,10} \tau_{4,10} l_8^2 l_9^2 - 8t^2 \tau_{3,12} \tau_{4,10} l_8^2 l_9^2 + 8u^2 \tau_{3,12} \tau_{4,10} l_8^2 l_9^2 + 8t^2 \tau_{4,7} \tau_{4,10} l_8^2 l_9^2 - \\
& 8u^2 \tau_{4,7} \tau_{4,10} l_8^2 l_9^2 + 2t^2 \tau_{2,7} \tau_{4,12} l_8^2 l_9^2 - 2u^2 \tau_{2,7} \tau_{4,12} l_8^2 l_9^2 - 2t^2 \tau_{2,12} \tau_{4,12} l_8^2 l_9^2 + 2u^2 \tau_{2,12} \tau_{4,12} l_8^2 l_9^2 + \\
& 8t^2 \tau_{3,5} \tau_{4,12} l_8^2 l_9^2 - 8u^2 \tau_{3,5} \tau_{4,12} l_8^2 l_9^2 - 8t^2 \tau_{3,10} \tau_{4,12} l_8^2 l_9^2 + 8u^2 \tau_{3,10} \tau_{4,12} l_8^2 l_9^2 + 8t^2 \tau_{4,5} \tau_{4,12} l_8^2 l_9^2 - \\
& 8u^2 \tau_{4,5} \tau_{4,12} l_8^2 l_9^2 - 8t^2 \tau_{4,10} \tau_{4,12} l_8^2 l_9^2 + 8u^2 \tau_{4,10} \tau_{4,12} l_8^2 l_9^2 - 6u^2 \tau_{1,13}^2 l_7^2 l_{10}^2 - 6u^2 \tau_{4,14}^2 l_7^2 l_{10}^2 + 4t^2 \tau_{1,8} \tau_{1,13} l_7^2 l_{10}^2 - \\
& 4u^2 \tau_{1,8} \tau_{1,13} l_7^2 l_{10}^2 - 8t^2 \tau_{1,13} \tau_{1,14} l_7^2 l_{10}^2 + 4u^2 \tau_{1,14} \tau_{2,9} l_7^2 l_{10}^2 - 8u^2 \tau_{1,13} \tau_{2,12} l_7^2 l_{10}^2 + 4u^2 \tau_{2,9} \tau_{2,12} l_7^2 l_{10}^2 - \\
& 4u^2 \tau_{1,14} \tau_{2,13} l_7^2 l_{10}^2 - 4u^2 \tau_{2,12} \tau_{2,13} l_7^2 l_{10}^2 - 8u^2 \tau_{1,13} \tau_{2,14} l_7^2 l_{10}^2 + 4u^2 \tau_{2,9} \tau_{2,14} l_7^2 l_{10}^2 - 4u^2 \tau_{2,13} \tau_{2,14} l_7^2 l_{10}^2 - \\
& 4u^2 \tau_{1,13} \tau_{3,8} l_7^2 l_{10}^2 + 4u^2 \tau_{3,5} \tau_{3,8} l_7^2 l_{10}^2 + 4u^2 \tau_{3,8} \tau_{3,13} l_7^2 l_{10}^2 + 4u^2 \tau_{1,13} \tau_{3,14} l_7^2 l_{10}^2 - 4u^2 \tau_{3,5} \tau_{3,14} l_7^2 l_{10}^2 - \\
& 4u^2 \tau_{3,13} \tau_{3,14} l_7^2 l_{10}^2 - 4t^2 \tau_{1,8} \tau_{4,5} l_7^2 l_{10}^2 + 4u^2 \tau_{1,8} \tau_{4,5} l_7^2 l_{10}^2 + 4t^2 \tau_{1,14} \tau_{4,5} l_7^2 l_{10}^2 - 4u^2 \tau_{1,14} \tau_{4,5} l_7^2 l_{10}^2 + \\
& 4u^2 \tau_{3,8} \tau_{4,5} l_7^2 l_{10}^2 - 4u^2 \tau_{3,14} \tau_{4,5} l_7^2 l_{10}^2 - 4t^2 \tau_{1,14} \tau_{4,9} l_7^2 l_{10}^2 + 4u^2 \tau_{1,14} \tau_{4,9} l_7^2 l_{10}^2 - 4t^2 \tau_{1,8} \tau_{4,13} l_7^2 l_{10}^2 + \\
& 4u^2 \tau_{1,8} \tau_{4,13} l_7^2 l_{10}^2 + 8t^2 \tau_{1,14} \tau_{4,13} l_7^2 l_{10}^2 - 8u^2 \tau_{1,14} \tau_{4,13} l_7^2 l_{10}^2 + 4u^2 \tau_{3,8} \tau_{4,13} l_7^2 l_{10}^2 - 4u^2 \tau_{3,14} \tau_{4,13} l_7^2 l_{10}^2 + \\
& 16u^2 \tau_{1,13} \tau_{4,14} l_7^2 l_{10}^2 - 4u^2 \tau_{2,9} \tau_{4,14} l_7^2 l_{10}^2 + 4u^2 \tau_{2,13} \tau_{4,14} l_7^2 l_{10}^2 - 8u^2 \tau_{3,5} \tau_{4,14} l_7^2 l_{10}^2 - 8u^2 \tau_{3,13} \tau_{4,14} l_7^2 l_{10}^2 - \\
& 4t^2 \tau_{4,5} \tau_{4,14} l_7^2 l_{10}^2 - 4u^2 \tau_{4,5} \tau_{4,14} l_7^2 l_{10}^2 + 4t^2 \tau_{4,9} \tau_{4,14} l_7^2 l_{10}^2 - 4u^2 \tau_{4,9} \tau_{4,14} l_7^2 l_{10}^2 - 8t^2 \tau_{4,13} \tau_{4,14} l_7^2 l_{10}^2 + \\
& 2\tau_{1,12} (2s(u(4\tau_{2,5} - \tau_{2,7} + \tau_{2,12}) + 2s(\tau_{3,5} - 2\tau_{3,10} - \tau_{3,12})) l_8^2 l_9^2 + (\tau_{1,14} s^2 - 2(3s^2 + t^2 + u^2) \tau_{1,13} + \\
& 2((s^2 + u^2) \tau_{2,9} - (s^2 + u^2) \tau_{2,13} + 2s(t\tau_{4,9} + u\tau_{4,13}))) l_7^2 l_{10}^2) - u(s^2 - t^2 + u^2) l_7^2 l_{10}^2 l_{16}^2)
\end{aligned}$$

■  $N_{39}^{(7)}$

0

■  $N_{39}^{(8)}$

$$-\frac{1}{4} l_7^2 l_8^2 l_9^2 l_{10}^2 (16s^2 + t^2 + u^2)$$
