# Supplementary material for: The Ultraviolet Behavior of N=8 Supergravity at Four Loops
Source: arXiv:0905.2326 ancillary file (2012-01-08)
Supplement: Supplementary file 38 [file SUGRA42.pdf]

## Integral 42: $\mathcal{I}_{42}$

$\mathcal{N} = 8$  four-point four-loop amplitude.

### ■ 2D plot of graph associated with $\mathcal{I}_{42}$

This fixes the labelling associated with the numerator expressions given below.

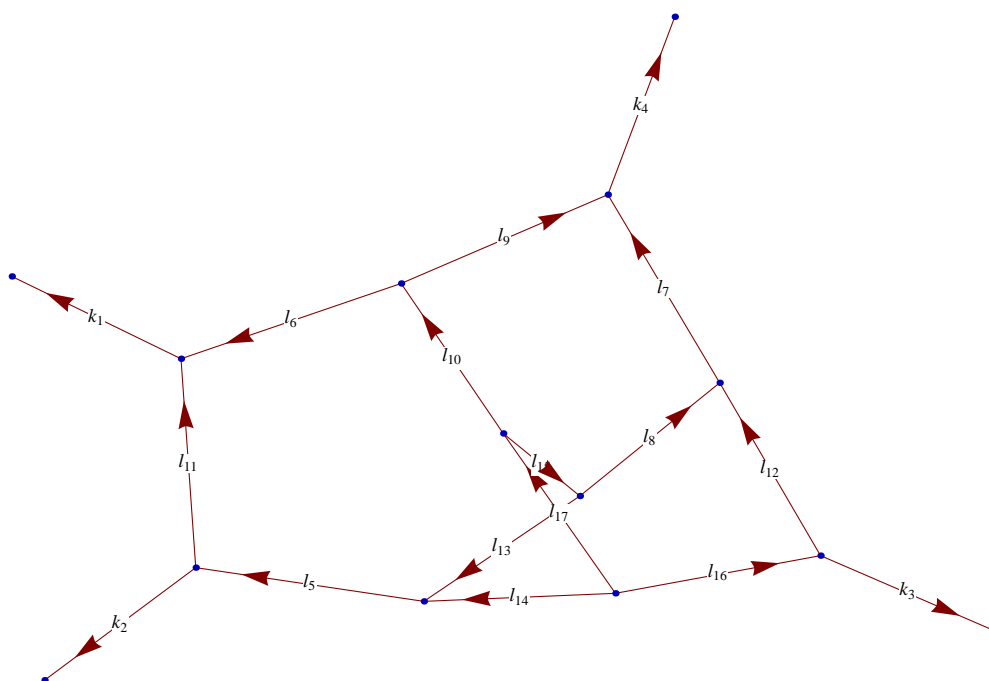

When using MathPlayer, by clicking three times (holding the click on the third click) directly on a vertex, one is able to move that vertex around, and its associated edges follow elastically. This functionality is absent when viewing as a pdf.

*Note: propagators for certain graphs were relabeled in the manuscript due to size constraints. The labels given in `aux/rawData/Neq8FourLoops.m` should be used for verification purposes.*

### ■ 3D plot of graph associated with $\mathcal{I}_{42}$

3D PLOT UNAVAILABLE FOR PDF. Please see .nb version for the 3D figure.

When using MathPlayer, by clicking anywhere in the image and dragging one should be able to rotate this 3D image. By holding (ALT) or (COMMAND) while clicking and moving the mouse up/down one should be able to zoom in/out. This functionality is absent when viewing as a pdf.

### "Vertex Form" of graph associated with $I_{42}$

This function returns the graph associated with the integral object in a vertex representation. This can be used as a way of specifying the topology of a graph using trivalent (cubic) vertices,  $\text{gVertex}[p_a, p_b, p_c]$ , where  $\{p_a, p_b, p_c\}$  are momenta labeling the propagators (edges) of the graph, and is understood that the edge labelled by  $p_a$  flows into the edge labelled by  $-p_a$ . Additionally, each vertex represents the manifest conservation of ( $D$  - dimensional) momenta :

$$\text{gVertex}[\{p_1, p_2, p_3\}] \iff (p_1 + p_2 + p_3 = 0)$$

$$\{\text{gVertex}(\{k_1, -l_{11}, -l_6\}), \text{gVertex}(\{k_2, -l_5, l_{11}\}), \text{gVertex}(\{k_3, -l_{16}, l_{12}\}), \text{gVertex}(\{k_4, -l_9, -l_7\}), \text{gVertex}(\{l_5, -l_{13}, -l_{14}\}), \\ \text{gVertex}(\{l_6, -l_{10}, l_9\}), \text{gVertex}(\{l_7, -l_{12}, -l_8\}), \text{gVertex}(\{l_8, -l_{15}, l_{13}\}), \text{gVertex}(\{l_{10}, l_{15}, -l_{17}\}), \text{gVertex}(\{l_{14}, l_{16}, l_{17}\})\}$$

### ■ Numerator expression for integral 42:

The following notation is used:  $\tau_{i,j} \equiv \begin{cases} 2 k_i \cdot l_j & \text{if } i \leq 4, j > 4 \\ 2 l_i \cdot l_j & \text{if } i, j > 4 \end{cases}$ .

$$s \equiv 2 k_1 \cdot k_2 = 2 k_3 \cdot k_4$$

We use  $s, t, u$  to represent the traditional Mandelstam variables for massless external four-point momenta:  $t \equiv 2 k_1 \cdot k_4 = 2 k_2 \cdot k_3$ .

$$u \equiv 2 k_1 \cdot k_3 = 2 k_2 \cdot k_4$$

Furthermore we use the shorthand  $(l_i)^2$  to represent the lorentz square:  $(l_i)^2 = l_i \cdot l_i$ .

**The total numerator  $\mathcal{N}_{42}$  is given by summing over the following terms, distinguished here by explicit dependence on loop momenta:  $\mathcal{N}_{42} = \sum_{i=0}^8 \mathcal{N}_{42}^{(i)}$ :**

■  $\mathcal{N}_{42}^{(0)}$

$$0$$

■  $\mathcal{N}_{42}^{(1)}$

$$0$$

■  $\mathcal{N}_{42}^{(2)}$

$$-\frac{1}{4} s^3 (4 l_{10}^2 (u^2 - t^2) + l_5^2 (t + 2u) (3t + 2u))$$

■  $\mathcal{N}_{42}^{(3)}$

$$\frac{1}{8} s^2 (l_5^2 (\tau_{1,10} (-19 s^2 + 5 t^2 + 3 u^2) + 4 \tau_{2,6} (3 s^2 - 2 t^2 - u^2) + \\ 8 \tau_{2,10} (t^2 - 2 s^2) - 12 s^2 \tau_{3,6} + 2 t^2 \tau_{1,14} + t^2 \tau_{2,14} + 4 t^2 \tau_{3,6} - 4 u^2 \tau_{3,6}) + \\ 4 l_{10}^2 s (s (\tau_{1,13} + 2 \tau_{3,13}) + \tau_{1,8} (u - t) + 2 \tau_{1,16} (u - t) - \tau_{2,13} (t + u) - 2 t \tau_{2,8} - 2 t \tau_{2,16} + 4 t \tau_{3,11} + 2 u \tau_{2,16} + 4 u \tau_{3,11}))$$

■  $N_{42}^{(4)}$

$$\begin{aligned}
& \frac{1}{16} \left( (4 \tau_{6,16} l_5^2 - (8 l_8^2 - 44 l_{10}^2 + l_{11}^2 + 2 (l_{12}^2 - 6 l_{13}^2 + 5 l_{15}^2 + 12 l_{17}^2)) l_5^2 + \right. \\
& \quad 4 (2 \tau_{8,11} l_{10}^2 - l_6^2 (4 l_{10}^2 + 3 l_{11}^2) + 2 (l_{10}^2 (2 l_{12}^2 - l_{13}^2) + l_7^2 (l_{10}^2 + l_{13}^2 + l_{17}^2))) t^4 + \\
& \quad 4 ((2 \tau_{1,10}^2 + (\tau_{1,14} - \tau_{2,6} + 5 \tau_{2,10} - \tau_{2,14} + 12 \tau_{3,6} - \tau_{3,14}) \tau_{1,10} + \tau_{1,16} \tau_{2,6} - (\tau_{2,6} - \tau_{2,10}) (3 \tau_{2,6} + \tau_{2,10} + \tau_{2,14}) - \\
& \quad (8 \tau_{2,6} - 8 \tau_{2,10} + \tau_{2,16}) \tau_{3,6}) l_5^2 + 4 (\tau_{1,8} + 2 \tau_{1,16} + \tau_{2,8} + 2 \tau_{2,16}) \tau_{3,11} l_{10}^2) t^3 + \\
& \quad 16 (\tau_{1,7} + \tau_{2,7})^2 \tau_{3,5}^2 t^2 + 2 (s^2 - t^2 - u^2) (2 \tau_{6,16} l_5^2 - (4 l_8^2 - 30 l_{10}^2 + 2 l_{11}^2 + l_{12}^2 - 6 l_{13}^2 + 5 l_{15}^2 + 12 l_{17}^2) l_5^2 + \\
& \quad l_6^2 (l_9^2 - 2 (2 l_{10}^2 + l_{11}^2)) + 8 (\tau_{8,11} l_{10}^2 + (2 l_{12}^2 - l_{13}^2) l_{10}^2 + l_7^2 (l_{10}^2 + l_{13}^2 + l_{17}^2))) t^2 + 2 (s^2 - t^2 - u^2) \\
& \quad ((9 \tau_{1,10}^2 + (2 \tau_{1,14} - 8 \tau_{2,6} + 24 \tau_{2,10} - 3 \tau_{2,14} + 44 \tau_{3,6} - 2 \tau_{3,14}) \tau_{1,10} - 3 \tau_{2,6}^2 + 9 \tau_{2,10}^2 + \tau_{1,16} \tau_{2,6} - 2 \tau_{2,16} \tau_{3,6} + \\
& \quad \tau_{2,10} (\tau_{2,14} + 32 \tau_{3,6}) - \tau_{2,6} (6 \tau_{2,10} + \tau_{2,14} + \tau_{2,16} + 32 \tau_{3,6})) l_5^2 + 12 (\tau_{1,8} + 2 \tau_{1,16} + \tau_{2,8} + 2 \tau_{2,16}) \tau_{3,11} l_{10}^2) t + \\
& \quad u (s^2 - t^2 - u^2) (2 \tau_{6,16} l_5^2 - (4 l_8^2 - 58 l_{10}^2 + 7 l_{11}^2 + l_{12}^2 - 6 l_{13}^2 + 5 l_{15}^2 + 12 l_{17}^2) l_5^2 + \\
& \quad 2 (l_6^2 (l_9^2 + 8 l_{10}^2 - 4 l_{11}^2) + 12 (\tau_{8,11} l_{10}^2 + (2 l_{12}^2 - l_{13}^2) l_{10}^2 + l_7^2 (l_{10}^2 + l_{13}^2 + l_{17}^2)))) t + \\
& \quad 16 u^2 (\tau_{1,7} + \tau_{2,7})^2 \tau_{3,5}^2 + 16 (s^2 - t^2 - u^2) (\tau_{1,7} + \tau_{2,7})^2 \tau_{3,5}^2 + \\
& \quad 8 u^3 ((\tau_{1,10}^2 + 2 (\tau_{2,6} + 2 \tau_{2,10} + 5 \tau_{3,6}) \tau_{1,10} - 2 (\tau_{2,6} - \tau_{2,10}) (\tau_{2,6} + \tau_{2,10} + 4 \tau_{3,6})) l_5^2 + \\
& \quad 2 (\tau_{1,8} + 2 \tau_{1,16} + \tau_{2,8} + 2 \tau_{2,16}) \tau_{3,11} l_{10}^2) + \\
& \quad 2 u (s^2 - t^2 - u^2) ((9 \tau_{1,10}^2 + (\tau_{1,14} - 3 \tau_{2,6} + 27 \tau_{2,10} - 2 \tau_{2,14} + 52 \tau_{3,6} - \tau_{3,14}) \tau_{1,10} - 4 \tau_{2,6}^2 + 12 \tau_{2,10}^2 + \\
& \quad (40 \tau_{2,10} - \tau_{2,16}) \tau_{3,6} - \tau_{2,6} (8 \tau_{2,10} + \tau_{2,16} + 40 \tau_{3,6})) l_5^2 + 12 (\tau_{1,8} + 2 \tau_{1,16} + \tau_{2,8} + 2 \tau_{2,16}) \tau_{3,11} l_{10}^2) + \\
& \quad 4 u^2 (s^2 - t^2 - u^2) (4 \tau_{8,11} l_{10}^2 + l_5^2 (6 l_{10}^2 - l_{11}^2) + l_6^2 (6 l_{10}^2 - l_{11}^2) + 4 (l_{10}^2 (2 l_{12}^2 - l_{13}^2) + l_7^2 (l_{10}^2 + l_{13}^2 + l_{17}^2))) + \\
& \quad u^4 (8 \tau_{8,11} l_{10}^2 + l_5^2 (8 l_{10}^2 - l_{11}^2) + 4 (l_6^2 (4 l_{10}^2 - 3 l_{11}^2) + 2 (l_{10}^2 (2 l_{12}^2 - l_{13}^2) + l_7^2 (l_{10}^2 + l_{13}^2 + l_{17}^2))))
\end{aligned}$$

■  $N_{42}^{(5)}$ 

$$\frac{1}{16}$$

$$\begin{aligned}
& \left( (8 \tau_{1,7} l_5^2 l_8^2 - 8 \tau_{2,7} l_5^2 l_8^2 - 16 \tau_{3,11} l_5^2 l_8^2 - 8 \tau_{3,14} l_5^2 l_8^2 + 20 \tau_{3,7} l_6^2 l_9^2 + 16 \tau_{3,10} l_6^2 l_9^2 + 24 \tau_{1,8} l_5^2 l_{10}^2 + 24 \tau_{1,12} l_5^2 l_{10}^2 + 8 \tau_{1,14} l_5^2 l_{10}^2 - \right. \\
& \quad 16 \tau_{2,11} l_5^2 l_{10}^2 + 16 \tau_{2,12} l_5^2 l_{10}^2 - 32 \tau_{4,11} l_5^2 l_{10}^2 - 16 \tau_{3,11} l_6^2 l_{10}^2 + 16 \tau_{4,12} l_6^2 l_{10}^2 - 4 \tau_{2,6} l_5^2 (\tau_{6,16} - 2 l_{11}^2) + \\
& \quad 12 \tau_{1,7} l_6^2 (l_9^2 - l_{11}^2) + 20 \tau_{1,6} l_5^2 l_{11}^2 - 20 \tau_{1,7} l_5^2 l_{11}^2 + 6 \tau_{1,12} l_5^2 l_{11}^2 + 20 \tau_{1,13} l_5^2 l_{11}^2 - 14 \tau_{2,7} l_5^2 l_{11}^2 + \\
& \quad 8 \tau_{2,12} l_5^2 l_{11}^2 + 11 \tau_{2,13} l_5^2 l_{11}^2 + 15 \tau_{3,6} l_5^2 l_{11}^2 + 19 \tau_{3,13} l_5^2 l_{11}^2 - 8 \tau_{3,10} l_6^2 l_{11}^2 - 4 \tau_{2,7} l_6^2 (l_9^2 + 4 l_{10}^2 + 9 l_{11}^2) + \\
& \quad 4 \tau_{2,10} (\tau_{6,16} l_5^2 - 4 l_6^2 l_{11}^2) + 2 \tau_{1,7} l_5^2 l_{12}^2 + 2 \tau_{3,8} l_5^2 l_{12}^2 + 2 \tau_{3,13} l_5^2 l_{12}^2 - 2 \tau_{3,17} l_5^2 l_{12}^2 + 8 \tau_{2,11} l_5^2 l_{13}^2 + \\
& \quad 8 \tau_{3,11} l_5^2 l_{13}^2 + 4 \tau_{1,9} l_5^2 l_{15}^2 - 4 \tau_{1,12} l_5^2 l_{15}^2 + 2 \tau_{2,9} l_5^2 l_{15}^2 + 2 \tau_{2,11} l_5^2 l_{15}^2 - 2 \tau_{2,12} l_5^2 l_{15}^2 + \\
& \quad 4 \tau_{4,11} l_5^2 l_{15}^2 - 8 (-3 \tau_{1,7} + 3 \tau_{1,8} + 3 \tau_{2,7} + 3 \tau_{2,8} + 2 (\tau_{2,11} - \tau_{2,14} + \tau_{3,11})) l_5^2 l_{17}^2) t^3 + \\
& \quad 2 (4 (\tau_{1,9}^3 - 2 \tau_{2,10}^2 \tau_{1,9} - 4 (\tau_{1,9} + \tau_{2,10})^2 \tau_{4,10}) l_6^2 - (\tau_{2,6} - \tau_{2,10}) \\
& \quad (2 \tau_{1,16} \tau_{2,6} + 2 \tau_{1,14} (\tau_{2,6} - \tau_{2,10}) + (\tau_{2,6} - \tau_{2,10}) (4 \tau_{2,6} + \tau_{2,14}) + 2 (4 \tau_{2,6} - 4 \tau_{2,10} - \tau_{2,16}) \tau_{3,6}) l_5^2) t^2 + \\
& \quad \frac{1}{2} (s^2 - t^2 - u^2) (-16 \tau_{2,11} l_5^2 l_8^2 - 32 \tau_{3,11} l_5^2 l_8^2 - 16 \tau_{3,14} l_5^2 l_8^2 + 20 \tau_{3,7} l_6^2 l_9^2 + 8 \tau_{3,10} l_6^2 l_9^2 + 80 \tau_{1,8} l_5^2 l_{10}^2 + \\
& \quad 96 \tau_{1,12} l_5^2 l_{10}^2 + 24 \tau_{1,14} l_5^2 l_{10}^2 + 16 \tau_{2,8} l_5^2 l_{10}^2 - 32 \tau_{2,11} l_5^2 l_{10}^2 + 64 \tau_{2,12} l_5^2 l_{10}^2 - 96 \tau_{4,11} l_5^2 l_{10}^2 - \\
& \quad 16 \tau_{3,7} l_6^2 l_{10}^2 - 48 \tau_{3,11} l_6^2 l_{10}^2 + 49 \tau_{1,6} l_5^2 l_{11}^2 + 12 \tau_{1,12} l_5^2 l_{11}^2 + 54 \tau_{1,13} l_5^2 l_{11}^2 + 14 \tau_{2,12} l_5^2 l_{11}^2 + \\
& \quad 45 \tau_{2,13} l_5^2 l_{11}^2 + 45 \tau_{3,6} l_5^2 l_{11}^2 + 57 \tau_{3,13} l_5^2 l_{11}^2 - 24 \tau_{3,10} l_6^2 l_{11}^2 + \tau_{2,6} l_5^2 (37 l_{11}^2 - 4 \tau_{6,16}) + \\
& \quad 4 \tau_{2,10} (\tau_{6,16} l_5^2 - 6 l_6^2 l_{11}^2) + 2 \tau_{3,8} l_5^2 l_{12}^2 + 2 \tau_{3,13} l_5^2 l_{12}^2 - 2 \tau_{3,17} l_5^2 l_{12}^2 - 2 \tau_{4,8} l_5^2 l_{12}^2 - 2 \tau_{4,13} l_5^2 l_{12}^2 + \\
& \quad 2 \tau_{4,17} l_5^2 l_{12}^2 + 16 \tau_{2,11} l_5^2 l_{13}^2 + 16 \tau_{3,11} l_5^2 l_{13}^2 + 6 \tau_{1,9} l_5^2 l_{15}^2 - 4 \tau_{1,12} l_5^2 l_{15}^2 + 2 \tau_{2,9} l_5^2 l_{15}^2 + 2 \tau_{2,11} l_5^2 l_{15}^2 + \\
& \quad 2 \tau_{2,14} l_5^2 l_{15}^2 + 8 \tau_{4,11} l_5^2 l_{15}^2 - 24 \tau_{1,8} l_5^2 l_{17}^2 - 24 \tau_{2,8} l_5^2 l_{17}^2 - 32 \tau_{2,11} l_5^2 l_{17}^2 + 16 \tau_{2,14} l_5^2 l_{17}^2 - 32 \tau_{3,11} l_5^2 l_{17}^2 - \\
& \quad 8 \tau_{2,7} (l_6^2 (2 l_9^2 + 8 l_{10}^2 - l_{11}^2) + l_5^2 (l_8^2 + 7 l_{11}^2 + 3 l_{17}^2)) + 2 \tau_{1,7} (2 l_6^2 (2 l_{11}^2 - 3 l_9^2) + l_5^2 (12 l_8^2 - 31 l_{11}^2 + 2 l_{12}^2 + 36 l_{17}^2))) t - \\
& \quad 2 \tau_{1,10}^2 (2 t (2 t + u) \tau_{1,14} + 4 (3 s^2 - t^2 + 2 u^2) \tau_{2,6} + (s^2 + t^2) \tau_{2,14} - 2 s (4 (2 t + 3 u) \tau_{3,6} + (2 t + u) \tau_{3,14})) l_5^2 + \\
& \quad 2 (s^2 - t^2 - u^2) (8 (\tau_{1,9} + \tau_{2,10})^2 (\tau_{1,9} - \tau_{2,10} - 2 \tau_{4,10}) l_6^2 - \\
& \quad (\tau_{2,6} - \tau_{2,10}) (4 \tau_{2,6}^2 - (4 \tau_{2,10} + \tau_{2,16} - 12 \tau_{3,6}) \tau_{2,6} - (12 \tau_{2,10} + \tau_{2,16}) \tau_{3,6}) l_5^2) + \\
& \quad 16 u^2 (2 (\tau_{1,9} + \tau_{2,10})^2 (\tau_{1,9} - \tau_{4,10}) l_6^2 - (\tau_{2,6} - \tau_{2,10})^2 (\tau_{2,6} + 2 \tau_{3,6}) l_5^2) + \\
& \quad u^3 (16 ((2 \tau_{1,8} + 3 \tau_{1,12} + \tau_{1,14} + \tau_{2,8} + 2 \tau_{2,12} - 2 \tau_{4,11}) l_5^2 - (2 (\tau_{2,7} + \tau_{3,7}) + \tau_{3,11}) l_6^2) l_{10}^2 + \\
& \quad ((8 \tau_{1,6} - 14 \tau_{1,7} + 8 \tau_{1,12} + 11 \tau_{1,13} + 20 \tau_{2,6} - 20 \tau_{2,7} + 6 \tau_{2,12} + 20 \tau_{2,13} + 15 \tau_{3,6} + 19 \tau_{3,13}) l_5^2 - \\
& \quad 4 (9 \tau_{1,7} + 3 \tau_{2,7} + 2 (\tau_{2,10} + \tau_{3,10})) l_6^2) l_{11}^2) + \\
& \quad 4 \tau_{1,10} \left( t (3 t + u) \tau_{1,14} (\tau_{2,6} - \tau_{2,10}) l_5^2 + \frac{1}{2} (\tau_{6,16} l_5^2 t^3 + 10 l_6^2 l_9^2 t^3 - u \tau_{6,16} l_5^2 t^2 + 2 u l_6^2 l_9^2 t^2 + 2 (2 t + u) \tau_{1,16} \tau_{2,6} l_5^2 t + 3 s^2 \right. \\
& \quad \left. \tau_{6,16} l_5^2 t - 3 u^2 \tau_{6,16} l_5^2 t - 2 s^2 l_6^2 l_9^2 t + 2 u^2 l_6^2 l_9^2 t + 4 (3 s^2 - t^2 + 3 u^2) \tau_{2,6}^2 l_5^2 + (-3 s^2 - t^2 + u^2) \tau_{2,16} \tau_{3,6} l_5^2 - \right.
\end{aligned}$$

$$\begin{aligned}
& 2\tau_{2,6}(-\tau_{2,14}t^2 + (6s^2 - 2t^2 + 6u^2)\tau_{2,10} + u(2t + u)\tau_{2,16} + s(4(3t + 5u)\tau_{3,6} + t\tau_{3,14}))l_5^2 - u^3\tau_{6,16}l_5^2 + \\
& s^2u\tau_{6,16}l_5^2 - 8s^2\tau_{1,9}^2l_6^2 - 8s^2\tau_{2,10}^2l_6^2 + 2\tau_{2,10}(s((4(3t + 5u)\tau_{3,6} + t\tau_{3,14})l_5^2 - 8s\tau_{1,9}l_6^2) - t^2\tau_{2,14}l_5^2) + \\
& 2u^3l_6^2l_9^2 - 2s^2ul_6^2l_9^2 - 2(-2t^3 - 3ut^2 - 4u^2t + u^3 + s^2(4t + 3u))l_6^2l_{11}^2) + \\
& \frac{1}{2}u(s^2 - t^2 - u^2)(-8\tau_{3,14}l_5^2l_8^2 - 4(\tau_{2,7} - \tau_{3,7} + 2\tau_{3,10})l_6^2l_9^2 + 88\tau_{1,8}l_5^2l_{10}^2 + 120\tau_{1,12}l_5^2l_{10}^2 + 32\tau_{1,14}l_5^2l_{10}^2 + \\
& 32\tau_{2,8}l_5^2l_{10}^2 + 80\tau_{2,12}l_5^2l_{10}^2 - 96\tau_{4,11}l_5^2l_{10}^2 - 80\tau_{2,7}l_6^2l_{10}^2 - 48\tau_{3,7}l_6^2l_{10}^2 - 16\tau_{4,12}l_6^2l_{10}^2 + 37\tau_{1,6}l_5^2l_{11}^2 + \\
& 14\tau_{1,12}l_5^2l_{11}^2 + 45\tau_{1,13}l_5^2l_{11}^2 + 49\tau_{2,6}l_5^2l_{11}^2 - 62\tau_{2,7}l_5^2l_{11}^2 + 12\tau_{2,12}l_5^2l_{11}^2 + 54\tau_{2,13}l_5^2l_{11}^2 + 45\tau_{3,6}l_5^2l_{11}^2 + \\
& 57\tau_{3,13}l_5^2l_{11}^2 + 8\tau_{2,7}l_6^2l_{11}^2 - 32\tau_{2,10}l_6^2l_{11}^2 - 24\tau_{3,10}l_6^2l_{11}^2 - 2\tau_{4,8}l_5^2l_{12}^2 - 2\tau_{4,13}l_5^2l_{12}^2 + 2\tau_{4,17}l_5^2l_{12}^2 + \\
& 2\tau_{1,9}l_5^2l_{15}^2 + 2\tau_{2,12}l_5^2l_{15}^2 + 2\tau_{2,14}l_5^2l_{15}^2 + 4\tau_{4,11}l_5^2l_{15}^2 - 8\tau_{2,11}l_5^2(2l_8^2 + 2l_{10}^2 - l_{13}^2 + 2l_{17}^2) - \\
& 8\tau_{3,11}(6l_6^2l_{10}^2 + l_5^2(2l_8^2 - l_{13}^2 + 2l_{17}^2)) + 2\tau_{1,7}(l_6^2(4l_{11}^2 - 3l_9^2) + l_5^2(8l_8^2 - 28l_{11}^2 + l_{12}^2 + 24l_{17}^2)))
\end{aligned}$$

■  $N_{42}^{(6)}$

$$\begin{aligned}
& \frac{1}{32}(-2l_6^2l_9^2l_{10}^2t^3 + 16l_5^2l_8^2l_{11}^2t^3 - 10l_5^2l_9^2l_{11}^2t^3 - 26l_5^2l_{11}^2l_{13}^2t^3 - 7l_5^2l_{11}^2l_{15}^2t^3 - 4\tau_{3,10}^2l_6^2l_9^2t^2 + 2ul_6^2l_9^2l_{10}^2t^2 + 7\tau_{1,6}^2l_5^2l_{11}^2t^2 - \\
& 6\tau_{1,12}^2l_5^2l_{11}^2t^2 + 8\tau_{1,13}^2l_5^2l_{11}^2t^2 - 3\tau_{2,6}^2l_5^2l_{11}^2t^2 - 2\tau_{2,12}^2l_5^2l_{11}^2t^2 - 4\tau_{2,13}^2l_5^2l_{11}^2t^2 - \tau_{1,6}\tau_{1,12}l_5^2l_{11}^2t^2 + \\
& 13\tau_{1,6}\tau_{1,13}l_5^2l_{11}^2t^2 - 2\tau_{1,12}\tau_{1,13}l_5^2l_{11}^2t^2 - 6\tau_{1,6}\tau_{2,6}l_5^2l_{11}^2t^2 + 21\tau_{1,12}\tau_{2,6}l_5^2l_{11}^2t^2 - 3\tau_{1,13}\tau_{2,6}l_5^2l_{11}^2t^2 - \\
& 5\tau_{1,6}\tau_{2,12}l_5^2l_{11}^2t^2 - 8\tau_{1,12}\tau_{2,12}l_5^2l_{11}^2t^2 - 4\tau_{1,13}\tau_{2,12}l_5^2l_{11}^2t^2 + 17\tau_{2,6}\tau_{2,12}l_5^2l_{11}^2t^2 - 3\tau_{1,6}\tau_{2,13}l_5^2l_{11}^2t^2 + \\
& 16\tau_{1,12}\tau_{2,13}l_5^2l_{11}^2t^2 - 2\tau_{1,13}\tau_{2,13}l_5^2l_{11}^2t^2 - 9\tau_{2,6}\tau_{2,13}l_5^2l_{11}^2t^2 + 14\tau_{2,12}\tau_{2,13}l_5^2l_{11}^2t^2 + 10\tau_{1,6}\tau_{3,6}l_5^2l_{11}^2t^2 + \\
& 5\tau_{1,13}\tau_{3,6}l_5^2l_{11}^2t^2 - 10\tau_{2,6}\tau_{3,6}l_5^2l_{11}^2t^2 - 5\tau_{2,13}\tau_{3,6}l_5^2l_{11}^2t^2 + 5\tau_{1,6}\tau_{3,13}l_5^2l_{11}^2t^2 + 6\tau_{1,13}\tau_{3,13}l_5^2l_{11}^2t^2 - \\
& 5\tau_{2,6}\tau_{3,13}l_5^2l_{11}^2t^2 - 6\tau_{2,13}\tau_{3,13}l_5^2l_{11}^2t^2 - 16\tau_{2,10}^2l_6^2l_{11}^2t^2 + 52ul_5^2l_8^2l_{11}^2t^2 - 122ul_5^2l_9^2l_{11}^2t^2 - 14ul_5^2l_9^2l_{12}^2t^2 - \\
& 42ul_5^2l_{11}^2l_{13}^2t^2 - 17ul_5^2l_{11}^2l_{15}^2t^2 - 2s^2l_6^2l_9^2l_{10}^2t + 2u^2l_6^2l_9^2l_{10}^2t - 52s^2l_5^2l_8^2l_{11}^2t + 52u^2l_5^2l_8^2l_{11}^2t + 122s^2l_5^2l_9^2l_{11}^2t - \\
& 122u^2l_5^2l_9^2l_{11}^2t + 28s^2l_5^2l_9^2l_{12}^2t - 28u^2l_5^2l_9^2l_{12}^2t + 42s^2l_5^2l_{11}^2l_{13}^2t - 42u^2l_5^2l_{11}^2l_{13}^2t + 17s^2l_5^2l_{11}^2l_{15}^2t - \\
& 17u^2l_5^2l_{11}^2l_{15}^2t - 28s^2\tau_{3,10}^2l_6^2l_9^2 + 4u^2\tau_{3,10}^2l_6^2l_9^2 + 2u^3l_6^2l_9^2l_{10}^2 - 2s^2ul_6^2l_9^2l_{10}^2 + 19s^2\tau_{1,6}^2l_5^2l_{11}^2 - 3u^2\tau_{1,6}^2l_5^2l_{11}^2 + \\
& 18s^2\tau_{1,12}^2l_5^2l_{11}^2 - 2u^2\tau_{1,12}^2l_5^2l_{11}^2 + 24s^2\tau_{1,13}^2l_5^2l_{11}^2 - 4u^2\tau_{1,13}^2l_5^2l_{11}^2 + 19s^2\tau_{2,6}^2l_5^2l_{11}^2 + 7u^2\tau_{2,6}^2l_5^2l_{11}^2 + \\
& 18s^2\tau_{2,12}^2l_5^2l_{11}^2 - 6u^2\tau_{2,12}^2l_5^2l_{11}^2 + 24s^2\tau_{2,13}^2l_5^2l_{11}^2 + 8u^2\tau_{2,13}^2l_5^2l_{11}^2 - 65s^2\tau_{1,6}\tau_{1,12}l_5^2l_{11}^2 + 17u^2\tau_{1,6}\tau_{1,12}l_5^2l_{11}^2 + \\
& 41s^2\tau_{1,6}\tau_{1,13}l_5^2l_{11}^2 - 9u^2\tau_{1,6}\tau_{1,13}l_5^2l_{11}^2 - 78s^2\tau_{1,12}\tau_{1,13}l_5^2l_{11}^2 + 14u^2\tau_{1,12}\tau_{1,13}l_5^2l_{11}^2 - 10s^2\tau_{1,6}\tau_{2,6}l_5^2l_{11}^2 - \\
& 6u^2\tau_{1,6}\tau_{2,6}l_5^2l_{11}^2 - 51s^2\tau_{1,12}\tau_{2,6}l_5^2l_{11}^2 - 5u^2\tau_{1,12}\tau_{2,6}l_5^2l_{11}^2 + 17s^2\tau_{1,13}\tau_{2,6}l_5^2l_{11}^2 - 3u^2\tau_{1,13}\tau_{2,6}l_5^2l_{11}^2 - \\
& 51s^2\tau_{1,6}\tau_{2,12}l_5^2l_{11}^2 + 21u^2\tau_{1,6}\tau_{2,12}l_5^2l_{11}^2 + 36s^2\tau_{1,12}\tau_{2,12}l_5^2l_{11}^2 - 8u^2\tau_{1,12}\tau_{2,12}l_5^2l_{11}^2 - 64s^2\tau_{1,13}\tau_{2,12}l_5^2l_{11}^2 + \\
& 16u^2\tau_{1,13}\tau_{2,12}l_5^2l_{11}^2 - 65s^2\tau_{2,6}\tau_{2,12}l_5^2l_{11}^2 - u^2\tau_{2,6}\tau_{2,12}l_5^2l_{11}^2 + 17s^2\tau_{1,6}\tau_{2,13}l_5^2l_{11}^2 - 3u^2\tau_{1,6}\tau_{2,13}l_5^2l_{11}^2 - \\
& 64s^2\tau_{1,12}\tau_{2,13}l_5^2l_{11}^2 - 4u^2\tau_{1,12}\tau_{2,13}l_5^2l_{11}^2 + 16s^2\tau_{1,13}\tau_{2,13}l_5^2l_{11}^2 - 2u^2\tau_{1,13}\tau_{2,13}l_5^2l_{11}^2 + 41s^2\tau_{2,6}\tau_{2,13}l_5^2l_{11}^2 + \\
& 13u^2\tau_{2,6}\tau_{2,13}l_5^2l_{11}^2 - 78s^2\tau_{2,12}\tau_{2,13}l_5^2l_{11}^2 - 2u^2\tau_{2,12}\tau_{2,13}l_5^2l_{11}^2 - 10u^2\tau_{1,6}\tau_{3,6}l_5^2l_{11}^2 - 80s^2\tau_{1,12}\tau_{3,6}l_5^2l_{11}^2 +
\end{aligned}$$

$$\begin{aligned}
& 21 s^2 \tau_{1,13} \tau_{3,6} l_5^2 l_{11}^2 - 5 u^2 \tau_{1,13} \tau_{3,6} l_5^2 l_{11}^2 + 10 u^2 \tau_{2,6} \tau_{3,6} l_5^2 l_{11}^2 - 80 s^2 \tau_{2,12} \tau_{3,6} l_5^2 l_{11}^2 + 21 s^2 \tau_{2,13} \tau_{3,6} l_5^2 l_{11}^2 + \\
& 5 u^2 \tau_{2,13} \tau_{3,6} l_5^2 l_{11}^2 + 23 s^2 \tau_{1,6} \tau_{3,13} l_5^2 l_{11}^2 - 5 u^2 \tau_{1,6} \tau_{3,13} l_5^2 l_{11}^2 - 92 s^2 \tau_{1,12} \tau_{3,13} l_5^2 l_{11}^2 + 22 s^2 \tau_{1,13} \tau_{3,13} l_5^2 l_{11}^2 - \\
& 6 u^2 \tau_{1,13} \tau_{3,13} l_5^2 l_{11}^2 + 23 s^2 \tau_{2,6} \tau_{3,13} l_5^2 l_{11}^2 + 5 u^2 \tau_{2,6} \tau_{3,13} l_5^2 l_{11}^2 - 92 s^2 \tau_{2,12} \tau_{3,13} l_5^2 l_{11}^2 + 22 s^2 \tau_{2,13} \tau_{3,13} l_5^2 l_{11}^2 + \\
& 6 u^2 \tau_{2,13} \tau_{3,13} l_5^2 l_{11}^2 - 16 s^2 \tau_{2,10}^2 l_6^2 l_{11}^2 - 16 u^2 \tau_{2,10}^2 l_6^2 l_{11}^2 - 32 s^2 \tau_{2,10} \tau_{3,10} l_6^2 l_{11}^2 + 16 u^3 l_5^2 l_8^2 l_{11}^2 - 52 s^2 u l_5^2 l_8^2 l_{11}^2 - \\
& 10 u^3 l_5^2 l_9^2 l_{11}^2 + 122 s^2 u l_5^2 l_9^2 l_{11}^2 - 16 \tau_{1,10}^2 l_6^2 ((t-u)(2t+u) l_9^2 + (s^2 + t^2 + u^2) l_{11}^2) + \tau_{2,7} (-8 s (3t+4u) \tau_{3,7} l_6^2 l_9^2 + \\
& ((8 \tau_{2,12} s^2 + \tau_{2,13} s^2 + 80 \tau_{3,6} s^2 - 12 \tau_{3,13} s^2 + (29 s^2 + 21 t^2 - 5 u^2) \tau_{1,6} + 4 (s^2 + t^2 + u^2) \tau_{1,12} + (s^2 + 5 t^2 - u^2) \\
& \tau_{1,13} + (15 s^2 - t^2 + 17 u^2) \tau_{2,6} + 4 t^2 \tau_{2,12} + 4 u^2 \tau_{2,12} + t^2 \tau_{2,13} + 3 u^2 \tau_{2,13}) l_5^2 - 16 (t^2 + u^2) \tau_{2,10} l_6^2) \\
& l_{11}^2 + 8 \tau_{3,10} l_6^2 ((3 s^2 - t^2) l_9^2 - 2 s^2 l_{11}^2) + 2 \tau_{2,7}^2 ((9 s^2 - 3 t^2 - u^2) l_5^2 l_{11}^2 + l_6^2 ((8 s^2 - 4 t^2) l_9^2 - 8 (5 t^2 + u^2) l_{11}^2)) + \\
& 2 \tau_{1,7}^2 ((9 s^2 - t^2 - 3 u^2) l_5^2 l_{11}^2 + 4 l_6^2 ((4 s^2 - 5 t^2 + 4 u^2) l_9^2 - 2 (t^2 + 5 u^2) l_{11}^2)) + \\
& 4 \tau_{1,10} l_6^2 ((4 s^2 + t^2 - 5 u^2) \tau_{2,7} l_9^2 + (-8 s^2 - 9 t^2 + 11 u^2) \tau_{3,7} l_9^2 - 4 s (2 s \tau_{2,10} l_{11}^2 + \tau_{3,10} ((u-4t) l_9^2 + 2 s l_{11}^2))) - \\
& 14 u^3 l_5^2 l_9^2 l_{12}^2 + 14 s^2 u l_5^2 l_9^2 l_{12}^2 + 8 \tau_{3,7}^2 (l_5^2 l_{12}^2 t^2 + 3 s (2t+u) l_6^2 l_9^2) + \\
& 8 \tau_{3,7} (s (8t+7u) \tau_{3,10} l_6^2 l_9^2 + t (u (\tau_{4,8} + \tau_{4,13} - \tau_{4,17}) - t (\tau_{3,8} + \tau_{3,13} - \tau_{3,17}))) l_5^2 l_{12}^2) + \\
& \tau_{1,7} (-4 \tau_{3,10} l_6^2 (4 l_{11}^2 s^2 + (5 s^2 + 9 t^2 - 8 u^2) l_9^2) + 4 \tau_{1,10} l_6^2 (3 (s^2 - 6 t^2 + u^2) l_9^2 - 4 (t^2 + u^2) l_{11}^2) + \\
& 4 \tau_{2,7} ((9 s^2 - 2 (t^2 + u^2)) l_5^2 l_{11}^2 + l_6^2 ((15 s^2 - t^2 - 2 u^2) l_9^2 + 2 (2 s^2 - 9 (t^2 + u^2)) l_{11}^2)) + \\
& l_5^2 ((4 \tau_{2,12} s^2 + \tau_{2,13} s^2 + 80 \tau_{3,6} s^2 - 12 \tau_{3,13} s^2 + (15 s^2 + 17 t^2 - u^2) \tau_{1,6} + 4 (2 s^2 + t^2 + u^2) \tau_{1,12} + \\
& (s^2 + 3 t^2 + u^2) \tau_{1,13} + (29 s^2 - 5 t^2 + 21 u^2) \tau_{2,6} + 4 t^2 \tau_{2,12} + 4 u^2 \tau_{2,12} - t^2 \tau_{2,13} + 5 u^2 \tau_{2,13}) l_{11}^2 + \\
& 8 s (t (\tau_{3,8} + \tau_{3,13} - \tau_{3,17}) - u (\tau_{4,8} + \tau_{4,13} - \tau_{4,17})) l_{12}^2) - 8 \tau_{3,7} ((2 s^2 + 5 (t^2 - 2 u^2)) l_6^2 l_9^2 + s t l_5^2 l_{12}^2)) - \\
& 26 u^3 l_5^2 l_{11}^2 l_{13}^2 + 42 s^2 u l_5^2 l_{11}^2 l_{13}^2 - 7 u^3 l_5^2 l_{11}^2 l_{15}^2 + 17 s^2 u l_5^2 l_{11}^2 l_{15}^2)
\end{aligned}$$

■  $N_{42}^{(7)}$

$$\begin{aligned}
& -\frac{1}{32} l_5^2 l_9^2 (2 l_{11}^2 \tau_{1,6} (17 s^2 + 10 t^2 + 21 u^2) + \\
& 2 l_{12}^2 (\tau_{3,7} (s^2 + t^2 - 23 u^2) + \tau_{3,8} (5 s^2 + t^2 + 25 u^2) + \tau_{3,13} (5 s^2 + t^2 + 25 u^2) - \tau_{3,17} (5 s^2 + t^2 + 25 u^2) - \\
& 18 s^2 \tau_{4,7} + 26 s^2 \tau_{4,8} + 26 s^2 \tau_{4,13} - 26 s^2 \tau_{4,17} + 24 t^2 \tau_{4,7} - 24 t^2 \tau_{4,8} - \\
& 24 t^2 \tau_{4,13} + 24 t^2 \tau_{4,17} - 50 u^2 \tau_{4,7} + 50 u^2 \tau_{4,8} + 50 u^2 \tau_{4,13} - 50 u^2 \tau_{4,17}) + \\
& 2 \tau_{1,7} (l_{11}^2 (10 s^2 + 9 t^2 + 5 u^2) - 4 l_{12}^2 s (4t+3u)) - 27 l_{11}^2 s^2 \tau_{1,12} + 28 l_{11}^2 s^2 \tau_{1,13} + 34 l_{11}^2 s^2 \tau_{2,6} + \\
& 20 l_{11}^2 s^2 \tau_{2,7} - 27 l_{11}^2 s^2 \tau_{2,12} + 28 l_{11}^2 s^2 \tau_{2,13} + 82 l_{11}^2 s^2 \tau_{3,6} + 38 l_{11}^2 s^2 \tau_{3,7} + 62 l_{11}^2 s^2 \tau_{3,13} + \\
& l_{11}^2 t^2 \tau_{1,12} - 6 l_{11}^2 t^2 \tau_{1,13} + 42 l_{11}^2 t^2 \tau_{2,6} + 10 l_{11}^2 t^2 \tau_{2,7} - 13 l_{11}^2 t^2 \tau_{2,12} + 64 l_{11}^2 t^2 \tau_{2,13} + \\
& 108 l_{11}^2 t^2 \tau_{3,6} - 14 l_{11}^2 t^2 \tau_{3,7} + 128 l_{11}^2 t^2 \tau_{3,13} - 13 l_{11}^2 u^2 \tau_{1,12} + 64 l_{11}^2 u^2 \tau_{1,13} + 20 l_{11}^2 u^2 \tau_{2,6} + \\
& 18 l_{11}^2 u^2 \tau_{2,7} + l_{11}^2 u^2 \tau_{2,12} - 6 l_{11}^2 u^2 \tau_{2,13} + 108 l_{11}^2 u^2 \tau_{3,6} - 14 l_{11}^2 u^2 \tau_{3,7} + 128 l_{11}^2 u^2 \tau_{3,13})
\end{aligned}$$

■  $N_{42}^{(8)}$

$$\begin{aligned}
& \frac{1}{32} l_5^2 l_6^2 l_9^2 l_{12}^2 (93 s^2 - 22 t^2 + 93 u^2)
\end{aligned}$$
