# Supplementary material for: The Ultraviolet Behavior of N=8 Supergravity at Four Loops
Source: arXiv:0905.2326 ancillary file (2012-01-08)
Supplement: Supplementary file 39 [file SUGRA43.pdf]

## Integral 43: $\mathcal{I}_{43}$

$\mathcal{N} = 8$  four-point four-loop amplitude.

### ■ 2D plot of graph associated with $\mathcal{I}_{43}$

This fixes the labelling associated with the numerator expressions given below.

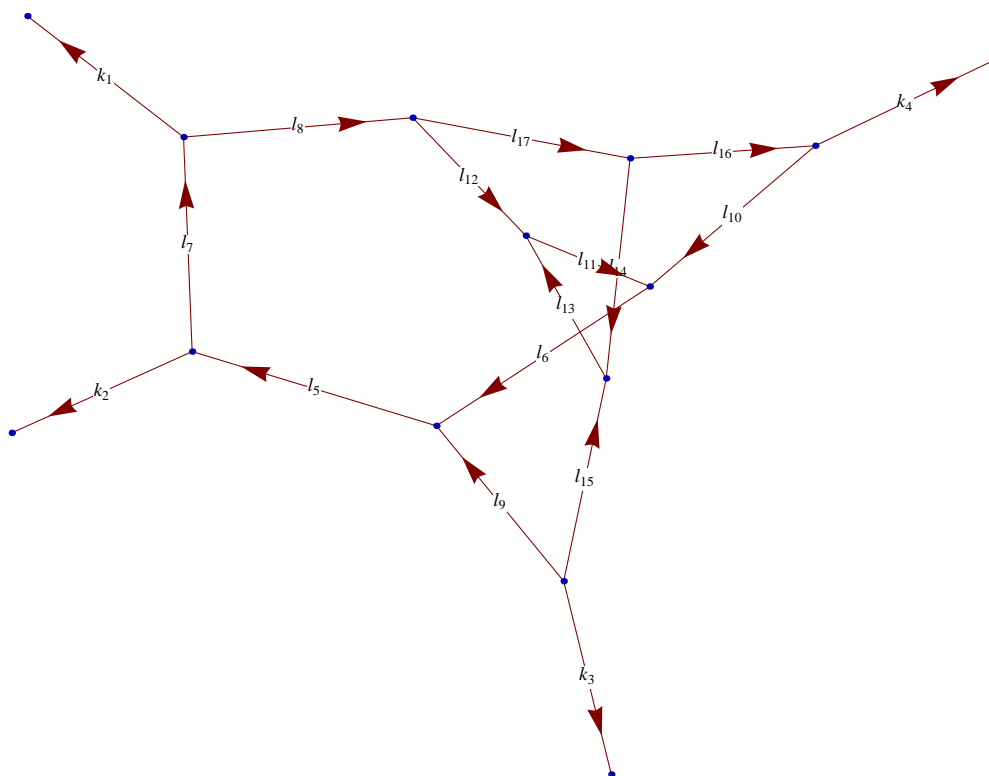

When using MathPlayer, by clicking three times (holding the click on the third click) directly on a vertex, one is able to move that vertex around, and its associated edges follow elastically. This functionality is absent when viewing as a pdf.

*Note: propagators for certain graphs were relabeled in the manuscript due to size constraints. The labels given in `aux/rawData/Neq8FourLoops.m` should be used for verification purposes.*

### ■ 3D plot of graph associated with $\mathcal{I}_{43}$

3D PLOT UNAVAILABLE FOR PDF. Please see .nb version for the 3D figure.

When using MathPlayer, by clicking anywhere in the image and dragging one should be able to rotate this 3D image. By holding (ALT) or (COMMAND) while clicking and moving the mouse up/down one should be able to zoom in/out. This functionality is absent when viewing as a pdf.

### ■ "Vertex Form" of graph associated with $\mathcal{I}_{43}$

This function returns the graph associated with the integral object in a vertex representation. This can be used as a way of specifying the topology of a graph using trivalent (cubic) vertices,  $\text{gVertex}[p_a, p_b, p_c]$ , where  $\{p_a, p_b, p_c\}$  are momenta labeling the propagators (edges) of the graph, and is understood that the edge labelled by  $p_a$  flows into the edge labelled by  $-p_a$ . Additionally, each vertex represents the manifest conservation of ( $D$  - dimensional) momenta :

$$\text{gVertex}[\{p_1, p_2, p_3\}] \iff (p_1 + p_2 + p_3 = 0)$$

$$\{\text{gVertex}(\{k_1, -l_7, l_8\}), \text{gVertex}(\{k_2, -l_5, l_7\}), \text{gVertex}(\{k_3, l_{15}, l_9\}), \\ \text{gVertex}(\{k_4, -l_{16}, l_{10}\}), \text{gVertex}(\{l_5, -l_6, -l_9\}), \text{gVertex}(\{l_6, -l_{10}, -l_{11}\}), \text{gVertex}(\{-l_8, l_{12}, l_{17}\}), \\ \text{gVertex}(\{l_{11}, -l_{12}, -l_{13}\}), \text{gVertex}(\{l_{13}, -l_{14}, -l_{15}\}), \text{gVertex}(\{l_{14}, l_{16}, -l_{17}\})\}$$

### ■ Numerator expression for integral 43:

The following notation is used:  $\tau_{i,j} \equiv \begin{cases} 2 k_i \cdot l_j & \text{if } i \leq 4, j > 4 \\ 2 l_i \cdot l_j & \text{if } i, j > 4 \end{cases}$ .

$$s \equiv 2 k_1 \cdot k_2 = 2 k_3 \cdot k_4$$

We use  $s, t, u$  to represent the traditional Mandelstam variables for massless external four-point momenta:  $t \equiv 2 k_1 \cdot k_4 = 2 k_2 \cdot k_3$ .

$$u \equiv 2 k_1 \cdot k_3 = 2 k_2 \cdot k_4$$

Furthermore we use the shorthand  $(l_i)^2$  to represent the lorentz square:  $(l_i)^2 = l_i \cdot l_i$ .

The total numerator  $\mathcal{N}_{43}$  is given by summing over the following terms, distinguished here by explicit dependence on loop momenta:  $\mathcal{N}_{43} = \sum_{i=0}^8 \mathcal{N}_{43}^{(i)}$ :

#### ■ $\mathcal{N}_{43}^{(0)}$

$$0$$

#### ■ $\mathcal{N}_{43}^{(1)}$

$$0$$

#### ■ $\mathcal{N}_{43}^{(2)}$

$$\frac{1}{2} s^2 t \left( (l_8^2 + 2 l_9^2) t^2 - 4 l_6^2 s u \right)$$

#### ■ $\mathcal{N}_{43}^{(3)}$

$$\frac{1}{4} s \left( -2 l_{15}^2 s^3 \tau_{1,13} - 2 l_{15}^2 s^3 \tau_{2,13} + 4 l_{15}^2 s^3 \tau_{4,8} + 2 l_{15}^2 s^3 \tau_{4,13} + \tau_{3,7} \left( 4 l_6^2 (t - u) (s^2 + (t + u)^2) - 6 l_9^2 t (s^2 + t^2 - u^2) \right) + \right. \\ \left. 4 l_6^2 s^2 \tau_{2,9} (u - t) - 8 l_6^2 s^2 t \tau_{1,9} - 5 l_8^2 s^2 t \tau_{1,10} - 4 l_8^2 s^2 t \tau_{1,11} - l_8^2 s^2 t \tau_{1,14} - 2 l_8^2 s^2 t \tau_{4,7} - 8 l_8^2 s^2 t \tau_{4,11} - \right. \\ \left. 6 l_8^2 s^2 t \tau_{4,14} + 12 l_8^2 t^3 \tau_{1,7} - 5 l_8^2 t^3 \tau_{1,10} - 4 l_8^2 t^3 \tau_{1,11} - l_8^2 t^3 \tau_{1,14} - 2 l_8^2 t^3 \tau_{4,7} + 4 l_8^2 t^3 \tau_{4,11} - \right. \\ \left. 6 l_8^2 t^3 \tau_{4,14} + 5 l_8^2 t u^2 \tau_{1,10} + 4 l_8^2 t u^2 \tau_{1,11} + l_8^2 t u^2 \tau_{1,14} + 2 l_8^2 t u^2 \tau_{4,7} + 8 l_8^2 t u^2 \tau_{4,11} + 6 l_8^2 t u^2 \tau_{4,14} \right)$$

$N_{43}^{(4)}$ 

$$\begin{aligned}
& -\tau_{7,9} l_6^2 t^4 + 3 \tau_{7,10} l_8^2 t^4 - 3 l_6^2 l_8^2 t^4 - \frac{5}{4} l_7^2 l_8^2 t^4 - 2 l_6^2 l_{10}^2 t^4 - \frac{3}{2} l_8^2 l_{10}^2 t^4 + \frac{7}{2} l_8^2 l_{11}^2 t^4 + \frac{1}{4} l_8^2 l_{12}^2 t^4 - l_8^2 l_{13}^2 t^4 + l_8^2 l_{14}^2 t^4 - \tau_{13,17} l_{15}^2 t^4 + \\
& \frac{3}{2} l_6^2 l_{15}^2 t^4 - \frac{5}{2} l_9^2 l_{15}^2 t^4 - l_{11}^2 l_{15}^2 t^4 + \frac{3}{2} l_{12}^2 l_{15}^2 t^4 - \frac{5}{4} l_8^2 l_{16}^2 t^4 - 2 \tau_{3,7}^2 l_6^2 t^3 + 2 \tau_{2,9} \tau_{3,7} l_6^2 t^3 + \frac{5}{2} \tau_{1,7}^2 l_8^2 t^3 + \frac{5}{2} \tau_{1,10}^2 l_8^2 t^3 + \\
& \frac{1}{2} \tau_{1,11}^2 l_8^2 t^3 - \frac{1}{2} \tau_{4,7}^2 l_8^2 t^3 - \frac{1}{2} \tau_{4,11}^2 l_8^2 t^3 - 5 \tau_{1,7} \tau_{1,10} l_8^2 t^3 - 3 \tau_{1,7} \tau_{1,11} l_8^2 t^3 + 3 \tau_{1,10} \tau_{1,11} l_8^2 t^3 - 2 \tau_{1,7} \tau_{1,14} l_8^2 t^3 + \\
& 2 \tau_{1,10} \tau_{1,14} l_8^2 t^3 + 2 \tau_{1,11} \tau_{1,14} l_8^2 t^3 + 3 \tau_{1,7} \tau_{2,10} l_8^2 t^3 - 2 \tau_{1,10} \tau_{4,7} l_8^2 t^3 + \tau_{1,14} \tau_{4,7} l_8^2 t^3 - 4 \tau_{1,7} \tau_{4,11} l_8^2 t^3 + 4 \tau_{1,10} \tau_{4,11} l_8^2 t^3 + \\
& 2 \tau_{1,11} \tau_{4,11} l_8^2 t^3 + 2 \tau_{1,14} \tau_{4,11} l_8^2 t^3 + 3 \tau_{2,10} \tau_{4,11} l_8^2 t^3 + 3 \tau_{2,14} \tau_{4,11} l_8^2 t^3 - \tau_{4,7} \tau_{4,11} l_8^2 t^3 - 4 \tau_{1,7} \tau_{4,14} l_8^2 t^3 + \\
& 4 \tau_{1,10} \tau_{4,14} l_8^2 t^3 + 4 \tau_{1,11} \tau_{4,14} l_8^2 t^3 - \tau_{4,7} \tau_{4,14} l_8^2 t^3 + 4 \tau_{4,11} \tau_{4,14} l_8^2 t^3 + 3 \tau_{3,7}^2 l_9^2 t^3 - \tau_{4,8}^2 l_{15}^2 t^3 + \tau_{1,13} \tau_{4,8} l_{15}^2 t^3 - \\
& \tau_{1,14} \tau_{4,8} l_{15}^2 t^3 - \tau_{1,17} \tau_{4,8} l_{15}^2 t^3 + \tau_{2,13} \tau_{4,8} l_{15}^2 t^3 - \tau_{2,14} \tau_{4,8} l_{15}^2 t^3 - \tau_{2,17} \tau_{4,8} l_{15}^2 t^3 + 2(-s^2 + t^2 + u^2) \tau_{7,9} l_6^2 t^2 - \\
& 3(-s^2 + t^2 + u^2) \tau_{7,10} l_8^2 t^2 + 5(-s^2 + t^2 + u^2) l_6^2 l_8^2 t^2 + \frac{15}{8}(-s^2 + t^2 + u^2) l_7^2 l_8^2 t^2 + 4(-s^2 + t^2 + u^2) l_6^2 l_{10}^2 t^2 - \\
& \frac{7}{2}(-s^2 + t^2 + u^2) l_8^2 l_{11}^2 t^2 - (-s^2 + t^2 + u^2) l_8^2 l_{12}^2 t^2 + (-s^2 + t^2 + u^2) l_8^2 l_{13}^2 t^2 - (-s^2 + t^2 + u^2) l_8^2 l_{14}^2 t^2 + \\
& 2(-s^2 + t^2 + u^2) \tau_{13,17} l_{15}^2 t^2 - 3(-s^2 + t^2 + u^2) l_6^2 l_{15}^2 t^2 + 5(-s^2 + t^2 + u^2) l_9^2 l_{15}^2 t^2 + 2(-s^2 + t^2 + u^2) l_{11}^2 l_{15}^2 t^2 - \\
& 3(-s^2 + t^2 + u^2) l_{12}^2 l_{15}^2 t^2 + \frac{13}{8}(-s^2 + t^2 + u^2) l_8^2 l_{16}^2 t^2 + 3(-s^2 + t^2 + u^2) \tau_{3,7}^2 l_6^2 t - 3(-s^2 + t^2 + u^2) \tau_{2,9} \tau_{3,7} l_6^2 t + \\
& 3 u(-s^2 + t^2 + u^2) \tau_{7,9} l_6^2 t - (-s^2 + t^2 + u^2) \tau_{1,7}^2 l_8^2 t - \frac{5}{2}(-s^2 + t^2 + u^2) \tau_{1,10}^2 l_8^2 t - \frac{1}{2}(-s^2 + t^2 + u^2) \tau_{1,11}^2 l_8^2 t + \\
& \frac{1}{2}(-s^2 + t^2 + u^2) \tau_{4,7}^2 l_8^2 t - (-s^2 + t^2 + u^2) \tau_{4,11}^2 l_8^2 t + \frac{9}{2}(-s^2 + t^2 + u^2) \tau_{1,7} \tau_{1,10} l_8^2 t + \frac{5}{2}(-s^2 + t^2 + u^2) \tau_{1,7} \tau_{1,11} l_8^2 t - \\
& 3(-s^2 + t^2 + u^2) \tau_{1,10} \tau_{1,11} l_8^2 t + \frac{1}{2}(-s^2 + t^2 + u^2) \tau_{1,7} \tau_{1,14} l_8^2 t - 2(-s^2 + t^2 + u^2) \tau_{1,10} \tau_{1,14} l_8^2 t - \\
& 2(-s^2 + t^2 + u^2) \tau_{1,11} \tau_{1,14} l_8^2 t - \frac{3}{2}(-s^2 + t^2 + u^2) \tau_{1,7} \tau_{2,10} l_8^2 t + \frac{1}{2}(-s^2 + t^2 + u^2) \tau_{1,7} \tau_{4,7} l_8^2 t + \\
& 2(-s^2 + t^2 + u^2) \tau_{1,10} \tau_{4,7} l_8^2 t - (-s^2 + t^2 + u^2) \tau_{1,14} \tau_{4,7} l_8^2 t + 4(-s^2 + t^2 + u^2) \tau_{1,7} \tau_{4,11} l_8^2 t - \frac{9}{2}(-s^2 + t^2 + u^2) \tau_{1,10} \tau_{4,11} l_8^2 t - \\
& \frac{5}{2}(-s^2 + t^2 + u^2) \tau_{1,11} \tau_{4,11} l_8^2 t - 2(-s^2 + t^2 + u^2) \tau_{1,14} \tau_{4,11} l_8^2 t - \frac{3}{2}(-s^2 + t^2 + u^2) \tau_{2,10} \tau_{4,11} l_8^2 t - \\
& \frac{3}{2}(-s^2 + t^2 + u^2) \tau_{2,14} \tau_{4,11} l_8^2 t + \frac{3}{2}(-s^2 + t^2 + u^2) \tau_{4,7} \tau_{4,11} l_8^2 t + \frac{5}{2}(-s^2 + t^2 + u^2) \tau_{1,7} \tau_{4,14} l_8^2 t -
\end{aligned}$$

$$\begin{aligned}
& 4(-s^2 + t^2 + u^2) \tau_{1,10} \tau_{4,14} l_8^2 t - 4(-s^2 + t^2 + u^2) \tau_{1,11} \tau_{4,14} l_8^2 t + (-s^2 + t^2 + u^2) \tau_{4,7} \tau_{4,14} l_8^2 t - 4(-s^2 + t^2 + u^2) \tau_{4,11} \tau_{4,14} l_8^2 t - \\
& \frac{3}{2} u(-s^2 + t^2 + u^2) \tau_{7,10} l_8^2 t + \frac{13}{2} u(-s^2 + t^2 + u^2) l_6^2 l_8^2 t + \frac{5}{2} u(-s^2 + t^2 + u^2) l_7^2 l_8^2 t - 3(-s^2 + t^2 + u^2) \tau_{3,7}^2 l_9^2 t + \\
& 6u(-s^2 + t^2 + u^2) l_6^2 l_{10}^2 t - \frac{3}{4} u(-s^2 + t^2 + u^2) l_8^2 l_{10}^2 t - \frac{7}{4} u(-s^2 + t^2 + u^2) l_8^2 l_{11}^2 t - \frac{1}{2} u(-s^2 + t^2 + u^2) l_8^2 l_{12}^2 t + \\
& \frac{1}{2} u(-s^2 + t^2 + u^2) l_8^2 l_{13}^2 t - \frac{1}{2} u(-s^2 + t^2 + u^2) l_8^2 l_{14}^2 t + \frac{3}{2} (-s^2 + t^2 + u^2) \tau_{4,8}^2 l_{15}^2 t - \frac{3}{2} (-s^2 + t^2 + u^2) \tau_{1,13} \tau_{4,8} l_{15}^2 t + \\
& \frac{3}{2} (-s^2 + t^2 + u^2) \tau_{1,14} \tau_{4,8} l_{15}^2 t + \frac{3}{2} (-s^2 + t^2 + u^2) \tau_{1,17} \tau_{4,8} l_{15}^2 t - \frac{3}{2} (-s^2 + t^2 + u^2) \tau_{2,13} \tau_{4,8} l_{15}^2 t + \\
& \frac{3}{2} (-s^2 + t^2 + u^2) \tau_{2,14} \tau_{4,8} l_{15}^2 t + \frac{3}{2} (-s^2 + t^2 + u^2) \tau_{2,17} \tau_{4,8} l_{15}^2 t + 3u(-s^2 + t^2 + u^2) \tau_{13,17} l_{15}^2 t - \frac{9}{2} u(-s^2 + t^2 + u^2) l_6^2 l_{15}^2 t + \\
& \frac{5}{2} u(-s^2 + t^2 + u^2) l_8^2 l_{15}^2 t + \frac{15}{2} u(-s^2 + t^2 + u^2) l_9^2 l_{15}^2 t + 3u(-s^2 + t^2 + u^2) l_{11}^2 l_{15}^2 t - \frac{9}{2} u(-s^2 + t^2 + u^2) l_{12}^2 l_{15}^2 t + \\
& \frac{19}{16} u(-s^2 + t^2 + u^2) l_8^2 l_{16}^2 t + s^2 \tau_{3,5}^4 + 2s^2 \tau_{2,6} \tau_{3,5}^3 + s^2 \tau_{1,6}^2 \tau_{3,5}^2 + s^2 \tau_{2,6}^2 \tau_{3,5}^2 + 2s^2 \tau_{1,6} \tau_{3,5}^2 (\tau_{2,6} + \tau_{3,5}) - \\
& 2u^3 \tau_{3,7}^2 l_6^2 + 3u(-s^2 + t^2 + u^2) \tau_{3,7}^2 l_6^2 - 2s^3 \tau_{1,9} \tau_{3,7} l_6^2 + 2u^3 \tau_{2,9} \tau_{3,7} l_6^2 - 3u(-s^2 + t^2 + u^2) \tau_{2,9} \tau_{3,7} l_6^2 - u^4 \tau_{7,9} l_6^2 + \\
& 2u^2(-s^2 + t^2 + u^2) \tau_{7,9} l_6^2 + \frac{1}{4} u(-s^2 + t^2 + u^2) \tau_{1,7}^2 l_8^2 - \frac{5}{4} u(-s^2 + t^2 + u^2) \tau_{1,10}^2 l_8^2 - \frac{1}{4} u(-s^2 + t^2 + u^2) \tau_{1,11}^2 l_8^2 + \\
& \frac{1}{4} u(-s^2 + t^2 + u^2) \tau_{4,7}^2 l_8^2 - \frac{5}{4} u(-s^2 + t^2 + u^2) \tau_{4,11}^2 l_8^2 + 2u(-s^2 + t^2 + u^2) \tau_{1,7} \tau_{1,10} l_8^2 + u(-s^2 + t^2 + u^2) \tau_{1,7} \tau_{1,11} l_8^2 - \\
& \frac{3}{2} u(-s^2 + t^2 + u^2) \tau_{1,10} \tau_{1,11} l_8^2 - \frac{1}{2} u(-s^2 + t^2 + u^2) \tau_{1,7} \tau_{1,14} l_8^2 - u(-s^2 + t^2 + u^2) \tau_{1,10} \tau_{1,14} l_8^2 - \\
& u(-s^2 + t^2 + u^2) \tau_{1,11} \tau_{1,14} l_8^2 + \frac{1}{2} u(-s^2 + t^2 + u^2) \tau_{1,7} \tau_{4,7} l_8^2 + u(-s^2 + t^2 + u^2) \tau_{1,10} \tau_{4,7} l_8^2 - \frac{1}{2} u(-s^2 + t^2 + u^2) \tau_{1,14} \tau_{4,7} l_8^2 + \\
& 2u(-s^2 + t^2 + u^2) \tau_{1,7} \tau_{4,11} l_8^2 - \frac{5}{2} u(-s^2 + t^2 + u^2) \tau_{1,10} \tau_{4,11} l_8^2 - \frac{3}{2} u(-s^2 + t^2 + u^2) \tau_{1,11} \tau_{4,11} l_8^2 - \\
& u(-s^2 + t^2 + u^2) \tau_{1,14} \tau_{4,11} l_8^2 + u(-s^2 + t^2 + u^2) \tau_{4,7} \tau_{4,11} l_8^2 + \frac{1}{2} u(-s^2 + t^2 + u^2) \tau_{1,7} \tau_{4,14} l_8^2 - 2u(-s^2 + t^2 + u^2) \tau_{1,10} \tau_{4,14} l_8^2 - \\
& 2u(-s^2 + t^2 + u^2) \tau_{1,11} \tau_{4,14} l_8^2 + \frac{1}{2} u(-s^2 + t^2 + u^2) \tau_{4,7} \tau_{4,14} l_8^2 - 2u(-s^2 + t^2 + u^2) \tau_{4,11} \tau_{4,14} l_8^2 - 2u^4 l_6^2 l_8^2 + \\
& 4u^2(-s^2 + t^2 + u^2) l_6^2 l_8^2 - \frac{5}{4} u^4 l_7^2 l_8^2 + \frac{15}{8} u^2(-s^2 + t^2 + u^2) l_7^2 l_8^2 - \frac{3}{2} u(-s^2 + t^2 + u^2) \tau_{3,7}^2 l_9^2 - 2u^4 l_6^2 l_{10}^2 +
\end{aligned}$$

$$\begin{aligned}
& 4u^2(-s^2+t^2+u^2)l_6^2l_{10}^2 - u^3\tau_{4,8}^2l_{15}^2 + \frac{3}{2}u(-s^2+t^2+u^2)\tau_{4,8}^2l_{15}^2 + u^3\tau_{1,13}\tau_{4,8}l_{15}^2 - \frac{3}{2}u(-s^2+t^2+u^2)\tau_{1,13}\tau_{4,8}l_{15}^2 - \\
& u^3\tau_{1,14}\tau_{4,8}l_{15}^2 + \frac{3}{2}u(-s^2+t^2+u^2)\tau_{1,14}\tau_{4,8}l_{15}^2 - u^3\tau_{1,17}\tau_{4,8}l_{15}^2 + \frac{3}{2}u(-s^2+t^2+u^2)\tau_{1,17}\tau_{4,8}l_{15}^2 + \\
& u^3\tau_{2,13}\tau_{4,8}l_{15}^2 - \frac{3}{2}u(-s^2+t^2+u^2)\tau_{2,13}\tau_{4,8}l_{15}^2 - u^3\tau_{2,14}\tau_{4,8}l_{15}^2 + \frac{3}{2}u(-s^2+t^2+u^2)\tau_{2,14}\tau_{4,8}l_{15}^2 - \\
& u^3\tau_{2,17}\tau_{4,8}l_{15}^2 + \frac{3}{2}u(-s^2+t^2+u^2)\tau_{2,17}\tau_{4,8}l_{15}^2 - u^4\tau_{13,17}l_{15}^2 + 2u^2(-s^2+t^2+u^2)\tau_{13,17}l_{15}^2 + \frac{3}{2}u^4l_6^2l_{15}^2 - \\
& 3u^2(-s^2+t^2+u^2)l_6^2l_{15}^2 - u^4l_8^2l_{15}^2 + 3u^2(-s^2+t^2+u^2)l_8^2l_{15}^2 - \frac{5}{2}u^4l_9^2l_{15}^2 + 5u^2(-s^2+t^2+u^2)l_9^2l_{15}^2 - u^4l_{11}^2l_{15}^2 + \\
& 2u^2(-s^2+t^2+u^2)l_{11}^2l_{15}^2 + \frac{3}{2}u^4l_{12}^2l_{15}^2 - 3u^2(-s^2+t^2+u^2)l_{12}^2l_{15}^2 + \frac{3}{8}u^4l_8^2l_{16}^2 + \frac{1}{2}(s^4l_{15}^2 - 2t^3(t+2u)l_8^2)l_{17}^2
\end{aligned}$$

■  $N_{43}^{(5)}$

$$\begin{aligned}
& \frac{1}{8} \left( l_8^2(-16\tau_{2,9}l_6^2 + 24\tau_{3,5}l_6^2 - 16\tau_{3,10}l_6^2 - 8\tau_{2,5}l_7^2 + 5\tau_{2,6}l_7^2 - 7\tau_{2,10}l_7^2 + 7\tau_{2,12}l_7^2 - 2\tau_{3,5}l_7^2 + 9\tau_{3,12}l_7^2 + \tau_{1,6}(3l_7^2 - 32l_{10}^2) + \right. \\
& 4\tau_{2,12}l_{10}^2 - 16\tau_{2,12}l_{11}^2 - 16\tau_{2,13}l_{11}^2 + 8\tau_{2,15}l_{11}^2 + 4\tau_{2,11}l_{12}^2 - 10\tau_{2,15}l_{12}^2 + 6\tau_{3,5}l_{12}^2 - 8\tau_{3,7}l_{13}^2 - 8\tau_{4,9}l_{14}^2 + \\
& 4(2\tau_{1,14} - \tau_{1,17})l_{15}^2 + 12\tau_{2,9}l_{15}^2 + 4\tau_{2,14}l_{15}^2 - 6\tau_{2,17}l_{15}^2 - 2(\tau_{3,10} - 11\tau_{3,12} - 8\tau_{4,5} + 8\tau_{4,10})l_{16}^2 - \\
& 2\tau_{1,9}(8l_6^2 + 4l_{14}^2 - 10l_{15}^2 + l_{16}^2) + 2\tau_{1,5}(4l_6^2 - 3l_7^2 + 2l_{12}^2 + 5l_{16}^2) + 2\tau_{1,12}(3l_7^2 + l_{10}^2 + 12l_{16}^2) + \\
& 4(2\tau_{1,11}\tau_{7,10} + 2\tau_{4,11}(\tau_{7,10} - l_{10}^2) - 2\tau_{4,9}l_{15}^2 + \tau_{4,7}(-2\tau_{7,10} + 3l_{10}^2 - 4l_{11}^2 + 5l_{15}^2) + \tau_{4,12}(l_{10}^2 + l_{16}^2))t^3 - \\
& 8\tau_{1,7}^3l_8^2t^2 + 4(2l_9^2\tau_{3,7}^3 + ((\tau_{1,14} + 2\tau_{4,14})\tau_{1,11}^2 + 2((\tau_{1,14} + \tau_{2,10} + \tau_{2,14} - 2\tau_{4,7})\tau_{4,11} - (\tau_{4,7} - 2\tau_{4,11})\tau_{4,14})\tau_{1,11} - \\
& (\tau_{4,7} - \tau_{4,11})(\tau_{1,14}(\tau_{4,7} + \tau_{4,11}) + 2\tau_{4,11}(\tau_{2,10} + \tau_{2,14} + \tau_{4,14})))l_8^2)t^2 + \\
& \frac{1}{2}(s^2 - t^2 - u^2)l_8^2(-48\tau_{2,9}l_6^2 + 48\tau_{3,5}l_6^2 - 16\tau_{3,10}l_6^2 + 9\tau_{1,12}l_7^2 - 12\tau_{2,5}l_7^2 + 13\tau_{2,6}l_7^2 - 3\tau_{2,10}l_7^2 + \\
& 10\tau_{2,12}l_7^2 + 6\tau_{3,5}l_7^2 + 15\tau_{3,12}l_7^2 + \tau_{1,6}(11l_7^2 - 40l_{10}^2) + 4\tau_{1,12}l_{10}^2 + 24\tau_{2,6}l_{10}^2 + 4\tau_{2,12}l_{10}^2 + \\
& 16(\tau_{1,12} + \tau_{1,13} - \tau_{1,15} - \tau_{2,12} - \tau_{2,13})l_{11}^2 - 16\tau_{3,7}l_{13}^2 - 16\tau_{4,9}l_{14}^2 + 20\tau_{1,14}l_{15}^2 - 4\tau_{1,17}l_{15}^2 + 12\tau_{2,9}l_{15}^2 + 8\tau_{2,14}l_{15}^2 - \\
& 10\tau_{2,17}l_{15}^2 + 2(8\tau_{4,11}(\tau_{7,10} - l_{10}^2) + \tau_{1,11}(8\tau_{7,10} - 2l_{12}^2) + 4(\tau_{3,5} - \tau_{2,15})l_{12}^2 - 2\tau_{4,7}(4\tau_{7,10} + 6l_{10}^2 + 8l_{11}^2 - l_{15}^2) + \\
& 2\tau_{4,17}l_{15}^2 + \tau_{4,12}(4l_{10}^2 - 8l_{11}^2 - 13l_{16}^2)) + 2(6\tau_{1,12} + 16\tau_{3,12} + 8\tau_{4,5} + 3\tau_{4,9} - 11\tau_{4,10})l_{16}^2 + \\
& 2\tau_{1,5}(4l_6^2 - 5l_7^2 + 4l_{12}^2 + l_{16}^2) + 2\tau_{1,9}(-24l_6^2 - 8l_{14}^2 + 14l_{15}^2 + 11l_{16}^2))t + \\
& 4s^2\tau_{1,10}^3l_8^2 + 4s^2\tau_{1,10}^2(2\tau_{1,11} + \tau_{1,14} + 2(-\tau_{4,7} + \tau_{4,11} + \tau_{4,14}))l_8^2 + \\
& 4\tau_{1,7}^2(-s(5t+u)\tau_{1,10} - 4st\tau_{1,11} + (t^2 - u^2)\tau_{1,14} + 2t(s\tau_{2,10} + 2(t+2u)\tau_{4,11} - s\tau_{4,14}))l_8^2 + \\
& 4u^2(2l_9^2\tau_{3,7}^3 + (\tau_{1,14}\tau_{1,11}^2 + 2\tau_{1,14}\tau_{4,11}\tau_{1,11} - 4\tau_{4,7}\tau_{4,11}\tau_{1,11} - \tau_{1,14}\tau_{4,7}^2 + \\
& \tau_{1,14}\tau_{4,11}^2 - 4\tau_{4,7}\tau_{4,11}^2 + 2(\tau_{1,11} + \tau_{4,11})(\tau_{1,11} - \tau_{4,7} + \tau_{4,11})\tau_{4,14}))l_8^2) +
\end{aligned}$$

$$\begin{aligned}
& 4(s^2 - t^2 - u^2) \left( 2l_9^2 \tau_{3,7}^3 + ((\tau_{1,14} + 2\tau_{4,14}) \tau_{1,11}^2 + ((2\tau_{1,14} + \tau_{2,10} + \tau_{2,14} - 4\tau_{4,7}) \tau_{4,11} - 2(\tau_{4,7} - 2\tau_{4,11}) \tau_{4,14}) \tau_{1,11} + \right. \\
& \quad \left. \tau_{1,14} (\tau_{4,11}^2 - \tau_{4,7}^2) + \tau_{4,11} (\tau_{2,10} (\tau_{4,11} - \tau_{4,7}) + \tau_{2,14} (\tau_{4,11} - \tau_{4,7}) - 2(\tau_{4,7} (\tau_{4,11} + \tau_{4,14}) - \tau_{4,11} \tau_{4,14})) \right) l_8^2 - \\
& 2\tau_{1,7} l_8^2 \left( (4\tau_{7,10} - 21l_{10}^2 + 4l_{13}^2 - 7l_{15}^2) t^3 + 4(\tau_{2,10} \tau_{4,7} + (\tau_{1,14} + \tau_{2,14} - 2\tau_{4,7}) \tau_{4,11} - (\tau_{4,7} - 2\tau_{4,11}) \tau_{4,14}) t^2 - \right. \\
& \quad \frac{1}{2} (-s^2 + t^2 + u^2) (8\tau_{7,10} - 14l_{10}^2 + 16l_{11}^2 + 4l_{13}^2 - l_{15}^2) t + 8s^2 \tau_{1,10}^2 + \\
& \quad 4s^2 \tau_{1,11}^2 - 4s \tau_{1,11} (t \tau_{1,14} - t \tau_{2,10} + 2(t + 2u) \tau_{4,11} + (2t + u) \tau_{4,14}) - \\
& \quad 4s \tau_{1,10} (-3s \tau_{1,11} + t \tau_{1,14} - t \tau_{2,10} + s \tau_{4,7} + (3t + 5u) \tau_{4,11} + (2t + u) \tau_{4,14}) + \\
& \quad 2(s^2 - t^2 - u^2) (\tau_{2,10} \tau_{4,7} + \tau_{1,14} (\tau_{4,7} + \tau_{4,11}) + \tau_{4,11} (\tau_{2,14} - 2\tau_{4,7} + 2\tau_{4,11}) - (\tau_{4,7} - 3\tau_{4,11}) \tau_{4,14}) + \\
& \quad \left. 4u^2 (\tau_{1,14} \tau_{4,7} + \tau_{4,11} (3\tau_{4,11} + \tau_{4,14})) - 11u^3 l_{15}^2 - \frac{1}{2} u (-s^2 + t^2 + u^2) (4\tau_{7,10} + 13l_{10}^2 + 16l_{11}^2 + 3l_{15}^2) \right) - \\
& s \tau_{1,10} l_8^2 (-8l_6^2 s^2 + 2l_7^2 s^2 - 4\tau_{1,11}^2 s - 4\tau_{4,7}^2 s + 8\tau_{4,7} (3\tau_{4,11} + \tau_{4,14}) s - 8\tau_{1,11} (\tau_{1,14} - \tau_{4,7} + \tau_{4,11} + 2\tau_{4,14}) s + \\
& \quad 4(t + u) \tau_{4,11}^2 + 8((t + u) \tau_{1,14} + t(\tau_{2,10} + \tau_{2,14})) \tau_{4,11} + 16(t + u) \tau_{4,11} \tau_{4,14} + \\
& \quad 4(s^2 + t^2 - u^2) \tau_{7,10} - 8t^2 l_6^2 + 8u^2 l_6^2 - 3t^2 l_7^2 - 9u^2 l_7^2 - 2t^2 l_{16}^2 + 2u^2 l_{16}^2) + \\
& u^3 l_8^2 (-16(\tau_{1,9} + \tau_{2,9} - \tau_{3,10}) l_6^2 + (5\tau_{1,6} + 7\tau_{1,12} - 6\tau_{2,5} + 3\tau_{2,6} - \tau_{2,10} + 6\tau_{2,12} - 2\tau_{3,5} + 9\tau_{3,12}) l_7^2 + \\
& \quad 2(2\tau_{1,9} + 2\tau_{1,14} + 2\tau_{1,17} + 2\tau_{2,9} + \tau_{2,17} + 14\tau_{4,7} + 2\tau_{4,17}) l_{15}^2 + \\
& \quad (26\tau_{1,9} + 7\tau_{1,12} - 11\tau_{4,5} + 26\tau_{4,9} + 13\tau_{4,10} + 5\tau_{4,12}) l_{16}^2 - \tau_{1,5} (8l_7^2 + 5l_{16}^2)) + \frac{1}{2} u (s^2 - t^2 - u^2) l_8^2 \\
& (8\tau_{1,11} \tau_{7,10} + 10\tau_{1,12} l_7^2 - 10\tau_{2,5} l_7^2 + 11\tau_{2,6} l_7^2 + 3\tau_{2,10} l_7^2 + 9\tau_{2,12} l_7^2 + 15\tau_{3,12} l_7^2 + \tau_{1,6} (13l_7^2 - 8l_{10}^2) + \\
& \quad 8\tau_{4,11} (\tau_{7,10} - l_{10}^2) + 2\tau_{1,12} l_{10}^2 + 24\tau_{2,6} l_{10}^2 + 8(2(\tau_{1,12} + \tau_{1,13} - \tau_{1,15}) - \tau_{2,15}) l_{11}^2 + \tau_{3,5} (24l_6^2 + 6l_7^2 + 8l_{12}^2) - \\
& \quad 8\tau_{4,9} l_{14}^2 - 4\tau_{4,7} (2\tau_{7,10} + 9l_{10}^2 + 4l_{11}^2 - 3l_{15}^2) + 2(8\tau_{1,14} + 2(\tau_{1,17} + \tau_{2,14}) - \tau_{2,17}) l_{15}^2 + 8(\tau_{4,9} + \tau_{4,17}) l_{15}^2 + \\
& \quad 4\tau_{2,9} (l_{15}^2 - 12l_6^2) + \tau_{4,12} (4l_{10}^2 - 16l_{11}^2 - 25l_{16}^2) - 5\tau_{1,12} l_{16}^2 + 10\tau_{3,12} l_{16}^2 - 11\tau_{4,5} l_{16}^2 + (32\tau_{4,9} + 7\tau_{4,10}) l_{16}^2 + \\
& \quad \left. 2\tau_{3,10} (8l_6^2 + l_{16}^2) - \tau_{1,5} (12l_7^2 + 13l_{16}^2) + 2\tau_{1,9} (-24l_6^2 - 4l_{14}^2 + 6l_{15}^2 + 25l_{16}^2) + 8\tau_{3,7} (l_{17}^2 - l_{13}^2) \right)
\end{aligned}$$

■  $N_{43}^{(6)}$

$$\begin{aligned}
& \frac{1}{8} \left( 2l_8^2 (-2l_6^2 l_{10}^2 + (4l_6^2 + 3l_{11}^2 + l_{12}^2 - 7l_{14}^2) l_{15}^2 + 2\tau_{5,10} (l_7^2 + 3l_{16}^2) - l_{16}^2 (10l_6^2 - 2l_{11}^2 + 10l_{12}^2 + 8l_{13}^2 - 4l_{14}^2 + l_{17}^2)) t^3 + \right. \\
& \quad l_8^2 (16l_{16}^2 \tau_{1,5}^2 + ((8\tau_{1,6} + 2\tau_{1,10} - 4\tau_{2,5} + 8\tau_{2,6} + 6\tau_{2,10} + 5\tau_{2,12} + 16\tau_{3,5}) l_7^2 + \\
& \quad 2(4\tau_{1,9} - 6\tau_{1,10} + 14\tau_{1,12} - 6\tau_{3,10} + 22\tau_{3,12} + 17\tau_{4,5} - 6\tau_{4,9} - 7\tau_{4,10} + 15\tau_{4,12}) l_{16}^2) \tau_{1,5} - \\
& \quad 2\tau_{1,6}^2 (l_7^2 + 2l_{10}^2) + 2\tau_{1,6} ((\tau_{1,10} - \tau_{1,12} + \tau_{2,5} - \tau_{2,6} - 2\tau_{2,10} - 2\tau_{2,12} + \tau_{3,5} - 3\tau_{3,12}) l_7^2 + \\
& \quad (11\tau_{1,7} + \tau_{1,12} + 2(\tau_{2,12} + 5\tau_{4,7} - 2\tau_{4,11} + \tau_{4,12})) l_{10}^2) - 2\tau_{1,12}^2 (l_7^2 + 2l_{16}^2) + \\
& \quad \left. \tau_{1,12} (5\tau_{2,5} l_7^2 - (5\tau_{2,12} + 6\tau_{3,5} + 4\tau_{3,12}) l_7^2 - 2(\tau_{1,7} + \tau_{4,7} - 2\tau_{4,11}) l_{10}^2 + 2\tau_{2,6} (l_{10}^2 - 2l_7^2) - \right.
\end{aligned}$$

$$\begin{aligned}
& 4(\tau_{1,10} + \tau_{3,10})l_{16}^2 + 2(6\tau_{3,12} + 4\tau_{4,5} - 4\tau_{4,9} - 3\tau_{4,10} + 7\tau_{4,12})l_{16}^2) + \\
& 2(-9l_{10}^2\tau_{1,7}^2 - 3l_{15}^2\tau_{1,7}^2 - \tau_{2,6}l_{10}^2\tau_{1,7} - 2\tau_{2,12}l_{10}^2\tau_{1,7} - 9\tau_{4,7}l_{10}^2\tau_{1,7} + 3\tau_{4,11}l_{10}^2\tau_{1,7} - 2\tau_{4,12}l_{10}^2\tau_{1,7} - \\
& 8\tau_{1,9}l_{15}^2\tau_{1,7} + 2\tau_{1,14}l_{15}^2\tau_{1,7} + 4\tau_{1,17}l_{15}^2\tau_{1,7} - 2\tau_{2,14}l_{15}^2\tau_{1,7} + 6\tau_{2,17}l_{15}^2\tau_{1,7} - 8\tau_{4,7}l_{15}^2\tau_{1,7} + \\
& 2\tau_{4,17}l_{15}^2\tau_{1,7} - \tau_{2,5}^2l_7^2 - \tau_{2,10}^2l_7^2 - 2\tau_{2,12}^2l_7^2 + 6\tau_{3,5}^2l_7^2 - 2\tau_{3,12}^2l_7^2 + \tau_{2,6}\tau_{2,10}l_7^2 - 2\tau_{2,6}\tau_{2,12}l_7^2 + \\
& 3\tau_{2,10}\tau_{2,12}l_7^2 + 3\tau_{2,6}\tau_{3,5}l_7^2 + \tau_{2,10}\tau_{3,5}l_7^2 - 4\tau_{2,6}\tau_{3,12}l_7^2 + 2\tau_{2,10}\tau_{3,12}l_7^2 - 5\tau_{2,12}\tau_{3,12}l_7^2 - 6\tau_{3,5}\tau_{3,12}l_7^2 + \\
& \tau_{2,5}(\tau_{2,6} - 2\tau_{2,10} + 3\tau_{2,12} + 4\tau_{3,12})l_7^2 - 2\tau_{2,6}^2l_{10}^2 - 4\tau_{4,11}^2l_{10}^2 + 2\tau_{2,6}\tau_{2,12}l_{10}^2 + 4\tau_{2,6}\tau_{4,7}l_{10}^2 - \\
& 2\tau_{2,12}\tau_{4,7}l_{10}^2 - 4\tau_{2,6}\tau_{4,11}l_{10}^2 + 4\tau_{2,12}\tau_{4,11}l_{10}^2 + 2\tau_{4,7}\tau_{4,11}l_{10}^2 + 2\tau_{2,6}\tau_{4,12}l_{10}^2 - 2\tau_{4,7}\tau_{4,12}l_{10}^2 + \\
& 4\tau_{4,11}\tau_{4,12}l_{10}^2 - 4\tau_{1,17}^2l_{15}^2 - 4\tau_{2,14}^2l_{15}^2 - 11\tau_{2,17}^2l_{15}^2 - 4\tau_{4,7}^2l_{15}^2 - 4\tau_{4,17}^2l_{15}^2 + 2\tau_{1,9}\tau_{1,17}l_{15}^2 - \\
& 4\tau_{1,14}\tau_{1,17}l_{15}^2 - 2\tau_{1,17}\tau_{2,9}l_{15}^2 + 4\tau_{1,17}\tau_{2,14}l_{15}^2 - 4\tau_{1,14}\tau_{2,17}l_{15}^2 - 12\tau_{1,17}\tau_{2,17}l_{15}^2 - 4\tau_{2,9}\tau_{2,17}l_{15}^2 + \\
& 12\tau_{2,14}\tau_{2,17}l_{15}^2 - 8\tau_{1,9}\tau_{4,7}l_{15}^2 - 4\tau_{1,14}\tau_{4,7}l_{15}^2 - 8\tau_{2,14}\tau_{4,7}l_{15}^2 + 4\tau_{2,17}\tau_{4,7}l_{15}^2 + 2\tau_{1,17}\tau_{4,9}l_{15}^2 + \\
& 4\tau_{2,17}\tau_{4,9}l_{15}^2 + 4\tau_{1,9}\tau_{4,17}l_{15}^2 - 4\tau_{1,14}\tau_{4,17}l_{15}^2 - 4\tau_{1,17}\tau_{4,17}l_{15}^2 - 4\tau_{2,9}\tau_{4,17}l_{15}^2 - 8\tau_{2,17}\tau_{4,17}l_{15}^2 - \\
& 4\tau_{4,7}\tau_{4,17}l_{15}^2 + 4\tau_{4,9}\tau_{4,17}l_{15}^2 + (4\tau_{1,9}^2 + (-4\tau_{3,12} - 4\tau_{4,5} + 8(\tau_{4,9} + \tau_{4,10}) + 6\tau_{4,12})\tau_{1,9} + \\
& 12\tau_{4,5}^2 + 4(\tau_{4,9} + \tau_{4,10})^2 + 8\tau_{4,12}^2 - \tau_{3,10}\tau_{4,5} + \tau_{3,12}(23\tau_{4,5} - 10\tau_{4,9} - 4\tau_{4,10} + 8\tau_{4,12}) + \\
& \tau_{4,5}(-14\tau_{4,9} - 9\tau_{4,10} + 11\tau_{4,12}))l_{16}^2 + \tau_{1,10}((-\tau_{2,10} + 2\tau_{2,12} + 3\tau_{3,5} + \tau_{3,12})l_7^2 - 7\tau_{4,5}l_{16}^2)))t^2 + \\
& \frac{1}{2}(s^2 - t^2 - u^2)(l_5^2(2l_7^2l_9^2 - 75l_8^2l_{15}^2) + 2\tau_{5,10}l_8^2(6l_7^2 + 11l_{16}^2) - 2l_8^2(12\tau_{7,14}l_{15}^2 + 7l_{14}^2(3l_{15}^2 - l_{16}^2) - \\
& l_{11}^2(13l_{15}^2 + 3l_{16}^2) + l_{12}^2(l_{15}^2 + 4l_{16}^2) + l_6^2(20l_{10}^2 - 4l_{15}^2 + 7l_{16}^2) + l_{16}^2(11l_{13}^2 + l_{17}^2)))t + \\
& u^3l_8^2(4\tau_{5,10}l_7^2 + (-24\tau_{7,14} - 27l_5^2 + 2(7l_{11}^2 - 3l_{12}^2 + l_{14}^2))l_{15}^2 + 8l_6^2(l_{16}^2 - 4l_{10}^2)) + \\
& (s^2 - t^2 - u^2) \\
& l_8^2 \\
& ((l_7^2 - 14l_{16}^2)\tau_{1,5}^2 + ((2\tau_{1,6} + 2\tau_{1,10} + \tau_{1,12} + 2(\tau_{2,5} + \tau_{2,6} + 3\tau_{2,10} + \tau_{2,12} + 4\tau_{3,5}) + \tau_{3,12})l_7^2 - \\
& (-14\tau_{1,9} + 11\tau_{1,10} + 9\tau_{1,12} + 5\tau_{3,10} + 5\tau_{3,12} + 16\tau_{4,5} - 3\tau_{4,9} + 5\tau_{4,10} + 9\tau_{4,12})l_{16}^2)\tau_{1,5} + \\
& \tau_{1,10}^2l_7^2 + \tau_{2,5}^2l_7^2 + \tau_{2,6}^2l_7^2 + \tau_{2,10}^2l_7^2 - 2\tau_{2,12}^2l_7^2 + 16\tau_{3,5}^2l_7^2 - 2\tau_{3,12}^2l_7^2 + 2\tau_{2,5}\tau_{2,6}l_7^2 + \\
& 2\tau_{2,5}\tau_{2,10}l_7^2 + 2\tau_{2,6}\tau_{2,10}l_7^2 + \tau_{2,5}\tau_{2,12}l_7^2 - 3\tau_{2,6}\tau_{2,12}l_7^2 + 8\tau_{2,5}\tau_{3,5}l_7^2 + 8\tau_{2,6}\tau_{3,5}l_7^2 + \\
& 8\tau_{2,10}\tau_{3,5}l_7^2 - 6\tau_{2,12}\tau_{3,5}l_7^2 + \tau_{2,5}\tau_{3,12}l_7^2 - 7\tau_{2,6}\tau_{3,12}l_7^2 - \tau_{2,10}\tau_{3,12}l_7^2 - \\
& 4\tau_{2,12}\tau_{3,12}l_7^2 - 16\tau_{3,5}\tau_{3,12}l_7^2 + \tau_{1,6}^2(l_7^2 - 4l_{10}^2) - 6\tau_{1,7}^2l_{10}^2 - 4\tau_{2,6}^2l_{10}^2 + 12\tau_{4,7}^2l_{10}^2 - \\
& 8\tau_{4,11}^2l_{10}^2 - 10\tau_{1,7}\tau_{2,6}l_{10}^2 - 2\tau_{1,7}\tau_{2,12}l_{10}^2 + 2\tau_{2,6}\tau_{2,12}l_{10}^2 + 14\tau_{1,7}\tau_{4,7}l_{10}^2 - \\
& 4\tau_{2,6}\tau_{4,7}l_{10}^2 - 2\tau_{2,12}\tau_{4,7}l_{10}^2 + 6\tau_{1,7}\tau_{4,11}l_{10}^2 - 8\tau_{2,6}\tau_{4,11}l_{10}^2 + 4\tau_{2,12}\tau_{4,11}l_{10}^2 + \\
& 4\tau_{4,7}\tau_{4,11}l_{10}^2 - 4\tau_{1,7}\tau_{4,12}l_{10}^2 + 4\tau_{2,6}\tau_{4,12}l_{10}^2 - 4\tau_{4,7}\tau_{4,12}l_{10}^2 + 8\tau_{4,11}\tau_{4,12}l_{10}^2 + \\
& \tau_{1,6}((2\tau_{1,10} - 3\tau_{1,12} + 2(\tau_{2,5} + \tau_{2,6} - \tau_{2,10} - 2\tau_{2,12} + 4\tau_{3,5}) - 7\tau_{3,12})l_7^2 + \\
& 2(9\tau_{1,7} + \tau_{1,12} + \tau_{2,12} + 4\tau_{4,7} - 4\tau_{4,11} + 2\tau_{4,12})l_{10}^2) - 8\tau_{1,7}^2l_{15}^2 + 2\tau_{1,17}^2l_{15}^2 + \\
& 4\tau_{2,14}^2l_{15}^2 + 18\tau_{2,17}^2l_{15}^2 + 8\tau_{4,7}^2l_{15}^2 - 12\tau_{4,17}^2l_{15}^2 - 16\tau_{1,7}\tau_{1,9}l_{15}^2 + 6\tau_{1,7}\tau_{1,14}l_{15}^2 + 4\tau_{1,7}\tau_{1,17}l_{15}^2 + \\
& 4\tau_{1,9}\tau_{1,17}l_{15}^2 - 14\tau_{1,14}\tau_{1,17}l_{15}^2 + 8\tau_{1,7}\tau_{2,9}l_{15}^2 - 4\tau_{1,17}\tau_{2,9}l_{15}^2 - 14\tau_{1,7}\tau_{2,14}l_{15}^2 +
\end{aligned}$$

$$\begin{aligned}
& 12 \tau_{1,14} \tau_{2,14} l_{15}^2 - 10 \tau_{1,17} \tau_{2,14} l_{15}^2 + 12 \tau_{1,7} \tau_{2,17} l_{15}^2 - 20 \tau_{1,14} \tau_{2,17} l_{15}^2 + 12 \tau_{1,17} \tau_{2,17} l_{15}^2 - \\
& 4 \tau_{2,9} \tau_{2,17} l_{15}^2 - 16 \tau_{2,14} \tau_{2,17} l_{15}^2 - 4 \tau_{1,7} \tau_{4,7} l_{15}^2 - 8 \tau_{1,9} \tau_{4,7} l_{15}^2 + 4 \tau_{1,14} \tau_{4,7} l_{15}^2 - \\
& 12 \tau_{1,17} \tau_{4,7} l_{15}^2 + 8 \tau_{2,9} \tau_{4,7} l_{15}^2 - 4 \tau_{2,14} \tau_{4,7} l_{15}^2 - 12 \tau_{2,17} \tau_{4,7} l_{15}^2 - 8 \tau_{1,7} \tau_{4,9} l_{15}^2 + \\
& 4 \tau_{1,17} \tau_{4,9} l_{15}^2 + 4 \tau_{2,17} \tau_{4,9} l_{15}^2 - 8 \tau_{4,7} \tau_{4,9} l_{15}^2 + 6 \tau_{1,7} \tau_{4,17} l_{15}^2 + 8 \tau_{1,9} \tau_{4,17} l_{15}^2 - \\
& 12 \tau_{1,14} \tau_{4,17} l_{15}^2 - 14 \tau_{1,17} \tau_{4,17} l_{15}^2 - 8 \tau_{2,9} \tau_{4,17} l_{15}^2 + 8 \tau_{2,14} \tau_{4,17} l_{15}^2 - 24 \tau_{2,17} \tau_{4,17} l_{15}^2 + \\
& 4 \tau_{4,7} \tau_{4,17} l_{15}^2 + 8 \tau_{4,9} \tau_{4,17} l_{15}^2 + 8 \tau_{1,9}^2 l_{16}^2 - 3 \tau_{4,5}^2 l_{16}^2 + 8 \tau_{4,9}^2 l_{16}^2 + 8 \tau_{4,10}^2 l_{16}^2 + 8 \tau_{4,12}^2 l_{16}^2 - \\
& 4 \tau_{1,9} \tau_{3,12} l_{16}^2 - 7 \tau_{1,9} \tau_{4,5} l_{16}^2 - \tau_{3,10} \tau_{4,5} l_{16}^2 - 5 \tau_{3,12} \tau_{4,5} l_{16}^2 + 16 \tau_{1,9} \tau_{4,9} l_{16}^2 - 9 \tau_{3,12} \tau_{4,9} l_{16}^2 - \\
& 9 \tau_{4,5} \tau_{4,9} l_{16}^2 + 16 \tau_{1,9} \tau_{4,10} l_{16}^2 - 4 \tau_{3,12} \tau_{4,10} l_{16}^2 - 10 \tau_{4,5} \tau_{4,10} l_{16}^2 + 16 \tau_{4,9} \tau_{4,10} l_{16}^2 + \\
& 15 \tau_{1,9} \tau_{4,12} l_{16}^2 - 2 \tau_{4,5} \tau_{4,12} l_{16}^2 + 10 \tau_{4,9} \tau_{4,12} l_{16}^2 + 4 \tau_{4,10} \tau_{4,12} l_{16}^2 - \tau_{1,12}^2 (2 l_7^2 + 3 l_{16}^2) + \\
& \tau_{1,10} ((6 \tau_{2,5} - 2 \tau_{2,6} + 2 \tau_{2,10} - \tau_{2,12} + 8 \tau_{3,5} - \tau_{3,12}) l_7^2 - (3 \tau_{1,12} + 13 \tau_{4,5}) l_{16}^2) + \\
& \tau_{1,12} (2 \tau_{2,5} l_7^2 - (\tau_{2,10} + 2 \tau_{2,12} + 6 \tau_{3,5} + 4 \tau_{3,12}) l_7^2 - 2 (\tau_{1,7} + \tau_{4,7} - 2 \tau_{4,11}) l_{10}^2 + \\
& 2 \tau_{2,6} (l_{10}^2 - 2 l_7^2) + (4 \tau_{1,9} - \tau_{3,10}) l_{16}^2 - (5 \tau_{3,12} + 9 \tau_{4,5} + \tau_{4,10} + 5 \tau_{4,12}) l_{16}^2) + \\
& u^2 l_8^2 (-2 (l_7^2 + 3 l_{16}^2) \tau_{1,5}^2 + ((2 \tau_{1,6} - 4 \tau_{1,10} + 6 \tau_{1,12} - 4 \tau_{2,5} + 2 \tau_{2,6} + 5 \tau_{2,12} + 8 \tau_{3,12}) l_7^2 + \\
& (20 \tau_{1,9} - 10 \tau_{1,10} - 8 \tau_{1,12} - 23 \tau_{4,5} + 36 \tau_{4,9} + 11 \tau_{4,10} + 19 \tau_{4,12}) l_{16}^2) \tau_{1,5} - 2 \tau_{1,10}^2 l_7^2 - 4 \tau_{1,6}^2 l_{10}^2 + \\
& 2 \tau_{1,6} ((\tau_{1,10} - 2 \tau_{1,12} + 4 \tau_{2,5} - \tau_{2,6} - 2 \tau_{2,12} + 3 \tau_{3,5} - 4 \tau_{3,12}) l_7^2 + (\tau_{1,7} + \tau_{1,12} - 2 \tau_{4,7} - 4 \tau_{4,11} + 2 \tau_{4,12}) l_{10}^2) - \\
& 2 \tau_{1,12}^2 (2 l_7^2 + l_{16}^2) + 2 \tau_{1,10} ((3 \tau_{1,12} + 3 \tau_{2,5} - 2 \tau_{2,6} - \tau_{2,10} + \tau_{3,5} + 2 \tau_{3,12}) l_7^2 - (\tau_{1,12} + 6 \tau_{4,5}) l_{16}^2) + \\
& \tau_{1,12} ((5 \tau_{2,5} - 4 \tau_{2,6} + 4 \tau_{2,10} - 5 (\tau_{2,12} + 2 \tau_{3,12})) l_7^2 - 2 \tau_{1,7} l_{10}^2 + 2 (\tau_{2,6} - \tau_{4,7} + 2 \tau_{4,11}) l_{10}^2 + \\
& (8 \tau_{1,9} - 15 \tau_{4,5} + 8 \tau_{4,9} + 3 (\tau_{4,10} + \tau_{4,12})) l_{16}^2) + 2 ((17 l_{10}^2 - 5 l_{15}^2) \tau_{1,7}^2 + \\
& ((29 \tau_{4,7} + 3 \tau_{4,11} - 2 \tau_{4,12}) l_{10}^2 + 2 (-2 \tau_{1,9} + 8 \tau_{1,14} - 4 \tau_{1,17} + 6 \tau_{2,9} - 9 \tau_{2,17} + 6 \tau_{4,7} - 6 \tau_{4,9} + 8 \tau_{4,17}) l_{15}^2) \\
& \tau_{1,7} + \tau_{2,5} (4 \tau_{2,6} + \tau_{2,10} + 8 \tau_{3,5}) l_7^2 - \\
& (\tau_{2,12}^2 + 3 \tau_{3,5} \tau_{2,12} - 6 \tau_{3,5}^2 + 2 \tau_{3,12}^2 + 2 (\tau_{2,12} + 3 \tau_{3,5}) \tau_{3,12} - \tau_{2,10} (3 \tau_{3,5} + \tau_{3,12})) l_7^2 - 4 \tau_{4,11}^2 l_{10}^2 + 4 \tau_{4,11} \\
& \tau_{4,12} l_{10}^2 - \tau_{2,6}^2 (l_7^2 + 2 l_{10}^2) + \tau_{2,6} ((\tau_{2,10} - \tau_{2,12} + \tau_{3,5} - 3 \tau_{3,12}) l_7^2 - (15 \tau_{1,7} + 8 \tau_{4,7} + 4 \tau_{4,11} - 2 \tau_{4,12}) l_{10}^2) - \\
& 8 \tau_{1,14}^2 l_{15}^2 - 2 \tau_{1,17}^2 l_{15}^2 + \tau_{2,17}^2 l_{15}^2 - 16 \tau_{4,17}^2 l_{15}^2 + 2 \tau_{1,9} \tau_{1,17} l_{15}^2 + 2 \tau_{1,14} \tau_{1,17} l_{15}^2 - 2 \tau_{1,17} \tau_{2,9} l_{15}^2 - \\
& 4 \tau_{1,14} \tau_{2,14} l_{15}^2 - 2 \tau_{1,17} \tau_{2,14} l_{15}^2 + 12 \tau_{1,14} \tau_{2,17} l_{15}^2 + 2 \tau_{1,17} \tau_{4,9} l_{15}^2 + 4 \tau_{1,9} \tau_{4,17} l_{15}^2 - 24 \tau_{1,14} \tau_{4,17} l_{15}^2 + \\
& 2 \tau_{1,17} \tau_{4,17} l_{15}^2 - 4 \tau_{2,9} \tau_{4,17} l_{15}^2 - 8 \tau_{2,14} \tau_{4,17} l_{15}^2 + 12 \tau_{2,17} \tau_{4,17} l_{15}^2 + 4 \tau_{4,9} \tau_{4,17} l_{15}^2 + 12 \tau_{4,7}^2 (l_{10}^2 + l_{15}^2) + \\
& 2 \tau_{4,7} ((\tau_{4,11} - \tau_{4,12}) l_{10}^2 + 2 (2 \tau_{1,14} - 3 \tau_{1,17} + 2 \tau_{2,9} + \tau_{2,14} - 4 \tau_{2,17} - 2 \tau_{4,9} + 2 \tau_{4,17}) l_{15}^2) + \\
& (4 \tau_{1,9}^2 + (-3 \tau_{4,5} + 8 (\tau_{4,9} + \tau_{4,10}) + 9 \tau_{4,12}) \tau_{1,9} - 7 \tau_{4,5}^2 + 4 (\tau_{4,9} + \tau_{4,10})^2 + \\
& 8 \tau_{4,12}^2 + (9 \tau_{4,9} + 4 \tau_{4,10}) \tau_{4,12} + \tau_{4,5} (5 \tau_{4,9} - \tau_{4,10} + 7 \tau_{4,12})) l_{16}^2) + \\
& \frac{1}{2} u (s^2 - t^2 - u^2) (l_5^2 (2 l_7^2 l_9^2 - 75 l_8^2 l_{15}^2) + 2 \tau_{5,10} l_8^2 (6 l_7^2 + 5 l_{16}^2) - 2 l_8^2 ((24 \tau_{7,14} - 17 l_{11}^2 + 11 l_{12}^2 + 13 l_{14}^2) l_{15}^2 + \\
& l_6^2 (34 l_{10}^2 - 7 l_{16}^2) + l_{16}^2 (-l_{11}^2 + 2 l_{12}^2 + 3 l_{13}^2 - 3 l_{14}^2 + l_{17}^2))) \Big)
\end{aligned}$$

■  $N_{43}^{(7)}$

$$\begin{aligned}
& \frac{1}{48} l_5^2 (l_7^2 l_9^2 (\tau_{4,6} (15 (s^2 + t^2) - 17 u^2) + 32 \tau_{1,6} (t^2 - u^2) + 32 t \tau_{3,6} (t + 2 u)) + \\
& 3 l_8^2 l_{15}^2 (-4 \tau_{2,7} (-6 s^2 + t^2 + 9 u^2) + \tau_{2,9} (27 s^2 + 17 t^2 + 3 u^2) + \\
& (-52 \tau_{2,14} + 20 \tau_{2,17} + 41 \tau_{3,7} + 23 \tau_{3,9} - 24 \tau_{3,14} - 39 \tau_{4,7} + 64 \tau_{4,9} + 12 \tau_{4,14}) (s^2 - t^2 - u^2) - \\
& 8 t^2 (9 \tau_{2,14} - 6 \tau_{2,17} - 8 \tau_{3,7} - 8 \tau_{3,9} + 3 \tau_{3,14} + 3 \tau_{3,17} + 10 \tau_{4,7} - 18 \tau_{4,9} + 3 \tau_{4,14}) + \\
& 2 u^2 (-18 \tau_{2,14} + 8 \tau_{2,17} + 4 \tau_{3,7} - 5 \tau_{3,9} - 6 \tau_{3,14} + 6 \tau_{3,17} - 34 \tau_{4,7} + 30 \tau_{4,9} + 12 \tau_{4,14}))) \Big)
\end{aligned}$$



$$N_{43}^{(8)}$$

$$0$$
