# Supplementary material for: The Ultraviolet Behavior of N=8 Supergravity at Four Loops
Source: arXiv:0905.2326 ancillary file (2012-01-08)
Supplement: Supplementary file 40 [file SUGRA44.pdf]

## Integral 44: $\mathcal{I}_{44}$

$\mathcal{N} = 8$  four-point four-loop amplitude.

### ■ 2D plot of graph associated with $\mathcal{I}_{44}$

This fixes the labelling associated with the numerator expressions given below.

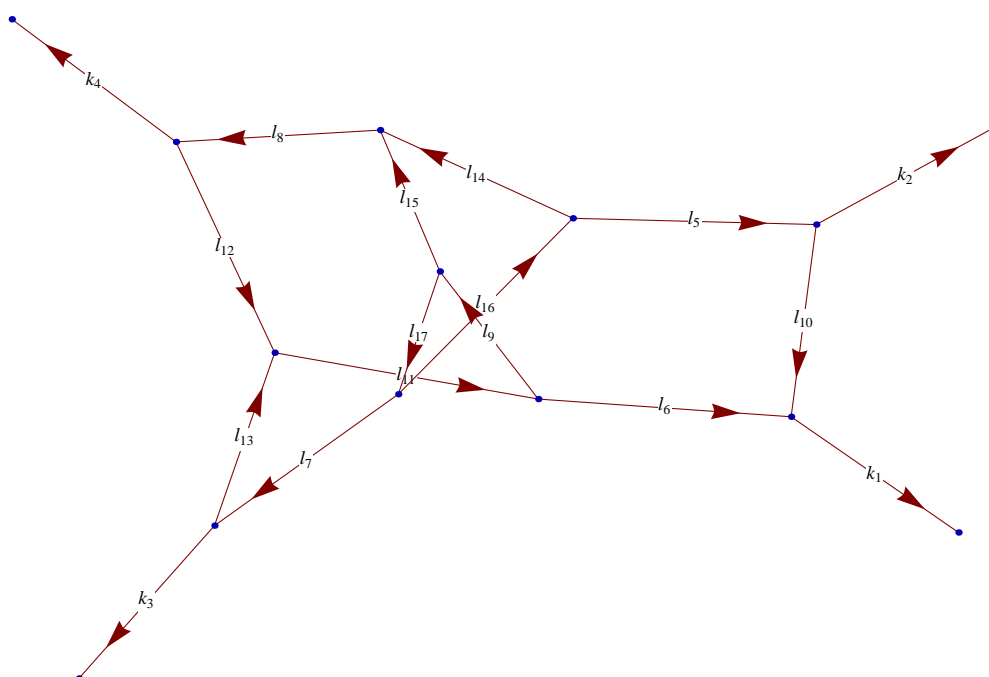

When using MathPlayer, by clicking three times (holding the click on the third click) directly on a vertex, one is able to move that vertex around, and its associated edges follow elastically. This functionality is absent when viewing as a pdf.

*Note: propagators for certain graphs were relabeled in the manuscript due to size constraints. The labels given in `aux/rawData/Neq8FourLoops.m` should be used for verification purposes.*

### ■ 3D plot of graph associated with $\mathcal{I}_{44}$

3D PLOT UNAVAILABLE FOR PDF. Please see .nb version for the 3D figure.

When using MathPlayer, by clicking anywhere in the image and dragging one should be able to rotate this 3D image. By holding (ALT) or (COMMAND) while clicking and moving the mouse up/down one should be able to zoom in/out. This functionality is absent when viewing as a pdf.

### "Vertex Form" of graph associated with $I_{44}$

This function returns the graph associated with the integral object in a vertex representation. This can be used as a way of specifying the topology of a graph using trivalent (cubic) vertices,  $\text{gVertex}[p_a, p_b, p_c]$ , where  $\{p_a, p_b, p_c\}$  are momenta labeling the propagators (edges) of the graph, and is understood that the edge labelled by  $p_a$  flows into the edge labelled by  $-p_a$ . Additionally, each vertex represents the manifest conservation of ( $D$  - dimensional) momenta :

$$\text{gVertex}[\{p_1, p_2, p_3\}] \iff (p_1 + p_2 + p_3 = 0)$$

$$\{\text{gVertex}(\{k_1, -l_6, -l_{10}\}), \text{gVertex}(\{k_2, l_{10}, -l_5\}), \text{gVertex}(\{k_3, -l_7, l_{13}\}), \text{gVertex}(\{k_4, -l_8, l_{12}\}), \text{gVertex}(\{l_5, -l_{16}, l_{14}\}), \\ \text{gVertex}(\{l_6, -l_{11}, l_9\}), \text{gVertex}(\{l_7, -l_{17}, l_{16}\}), \text{gVertex}(\{l_8, -l_{14}, -l_{15}\}), \text{gVertex}(\{-l_9, l_{17}, l_{15}\}), \text{gVertex}(\{l_{11}, -l_{12}, -l_{13}\})\}$$

### ■ Numerator expression for integral 44:

The following notation is used:  $\tau_{i,j} \equiv \begin{cases} 2 k_i \cdot l_j & \text{if } i \leq 4, j > 4 \\ 2 l_i \cdot l_j & \text{if } i, j > 4 \end{cases}$ .

$$s \equiv 2 k_1 \cdot k_2 = 2 k_3 \cdot k_4$$

We use  $s, t, u$  to represent the traditional Mandelstam variables for massless external four-point momenta:  $t \equiv 2 k_1 \cdot k_4 = 2 k_2 \cdot k_3$ .

$$u \equiv 2 k_1 \cdot k_3 = 2 k_2 \cdot k_4$$

Furthermore we use the shorthand  $(l_i)^2$  to represent the lorentz square:  $(l_i)^2 = l_i \cdot l_i$ .

**The total numerator  $\mathcal{N}_{44}$  is given by summing over the following terms, distinguished here by explicit dependence on loop momenta:  $\mathcal{N}_{44} = \sum_{i=0}^8 \mathcal{N}_{44}^{(i)}$ :**

#### ■ $\mathcal{N}_{44}^{(0)}$

$$0$$

#### ■ $\mathcal{N}_{44}^{(1)}$

$$0$$

#### ■ $\mathcal{N}_{44}^{(2)}$

$$\frac{1}{4} s^3 (2 s \tau_{3,5}^2 + 2 s \tau_{4,5}^2 + l_5^2 (5 (t^2 + u^2) - 6 s^2) - 6 l_9^2 s^2)$$

#### ■ $\mathcal{N}_{44}^{(3)}$

$$\frac{1}{4} s^2 (4 \tau_{3,5} \tau_{5,7} s^2 + 4 \tau_{4,5} \tau_{5,8} s^2 + 6 \tau_{1,9} l_5^2 s^2 - \tau_{1,14} l_5^2 s^2 + \tau_{1,16} l_5^2 s^2 + 4 \tau_{2,6} l_5^2 s^2 + 6 \tau_{2,9} l_5^2 s^2 - \tau_{2,14} l_5^2 s^2 + \tau_{2,16} l_5^2 s^2 - \\ 3 \tau_{3,6} l_5^2 s^2 - 3 \tau_{4,6} l_5^2 s^2 + 4 \tau_{1,11} l_9^2 s^2 + 2 \tau_{1,15} l_9^2 s^2 + 2 \tau_{1,17} l_9^2 s^2 + 2 \tau_{2,11} l_9^2 s^2 + 2 \tau_{2,15} l_9^2 s^2 + 2 \tau_{2,17} l_9^2 s^2 - \\ 6 \tau_{3,10} l_9^2 s^2 + 4 \tau_{3,15} l_9^2 s^2 - 6 \tau_{4,10} l_9^2 s^2 + 4 \tau_{4,17} l_9^2 s^2 + 2 (\tau_{1,12} + \tau_{1,13} + \tau_{2,12} + \tau_{2,13} + \tau_{3,6} + \tau_{4,6}) l_{11}^2 s^2 - \\ 6 t^2 \tau_{1,9} l_5^2 - 6 u^2 \tau_{1,9} l_5^2 + t^2 \tau_{1,14} l_5^2 + 3 u^2 \tau_{1,14} l_5^2 - 3 t^2 \tau_{1,16} l_5^2 - u^2 \tau_{1,16} l_5^2 - 7 t^2 \tau_{2,6} l_5^2 - 7 u^2 \tau_{2,6} l_5^2 - 6 t^2 \tau_{2,9} l_5^2 - \\ 6 u^2 \tau_{2,9} l_5^2 + 2 t^2 \tau_{2,14} l_5^2 + 2 u^2 \tau_{2,14} l_5^2 - 2 t^2 \tau_{2,16} l_5^2 - 2 u^2 \tau_{2,16} l_5^2 - t^2 \tau_{3,6} l_5^2 + u^2 \tau_{3,6} l_5^2 + t^2 \tau_{4,6} l_5^2 - u^2 \tau_{4,6} l_5^2 + \\ \tau_{1,8} (4 s \tau_{3,5}^2 + 4 s \tau_{4,5}^2 + (3 (t^2 + u^2) - 5 s^2) l_5^2 + 4 s t l_9^2) + \tau_{1,7} (4 s \tau_{3,5}^2 + 4 s \tau_{4,5}^2 + (3 (t^2 + u^2) - 5 s^2) l_5^2 + 4 s u l_9^2) + \\ \tau_{2,8} (-4 (t + u) \tau_{3,5}^2 - 4 (t + u) \tau_{4,5}^2 + (-5 s^2 + t^2 + 5 u^2) l_5^2 - 2 (s^2 + t^2 - u^2) l_9^2) + \\ \tau_{2,7} (-4 (t + u) \tau_{3,5}^2 - 4 (t + u) \tau_{4,5}^2 + (-5 s^2 + 5 t^2 + u^2) l_5^2 - 2 (s^2 - t^2 + u^2) l_9^2))$$

$N_{44}^{(4)}$ 

$$\begin{aligned}
& -\frac{1}{4}s \left( (2(\tau_{5,7}^2 + \tau_{5,8}^2 + (\tau_{6,7} + \tau_{6,8})l_5^2 - 2l_7^2 l_8^2 - \tau_{10,11}l_9^2) + (l_5^2 - 2\tau_{6,9})l_{11}^2)t^3 + \right. \\
& (2l_5^2 \tau_{1,7}^2 + 2(-2\tau_{3,5}\tau_{5,7} - 2\tau_{4,5}\tau_{5,8} + (\tau_{1,16} + \tau_{2,6} + \tau_{2,7} + 2\tau_{3,6})l_5^2 + 2\tau_{3,10}l_9^2)\tau_{1,7} + \tau_{1,8}^2 l_5^2 + 3\tau_{2,8}^2 l_5^2 + \\
& 2\tau_{2,7}(-2\tau_{3,5}\tau_{5,7} - 2\tau_{4,5}\tau_{5,8} + (\tau_{1,9} + 2\tau_{1,16} + 3\tau_{2,6} + \tau_{2,9} + \tau_{2,16} + 3\tau_{3,6})l_5^2 + 2\tau_{3,10}l_9^2) - \\
& 2\tau_{2,8}(2\tau_{3,5}\tau_{5,7} + 2\tau_{4,5}\tau_{5,8} + (\tau_{1,9} - \tau_{1,14} + \tau_{2,6} + \tau_{2,9})l_5^2 - 2\tau_{4,10}l_9^2) - \\
& 2\tau_{1,8}(2\tau_{3,5}\tau_{5,7} + 2\tau_{4,5}\tau_{5,8} + (\tau_{1,9} - 2\tau_{2,8} + \tau_{2,9} + \tau_{2,14} - \tau_{4,6})l_5^2 - 2\tau_{4,10}l_9^2) - \\
& 2((\tau_{2,6} + \tau_{2,9})(2\tau_{1,16} + 3\tau_{2,6} + \tau_{2,16} + 3\tau_{3,6} + 2\tau_{4,6}) + \tau_{1,9}(2\tau_{1,16} + 3\tau_{2,6} + \tau_{2,16} + 3\tau_{3,6} + \tau_{3,16} + 2\tau_{4,6} + \tau_{4,14})) \\
& l_5^2 + (\tau_{1,11} + \tau_{2,11})(\tau_{3,10} + \tau_{4,10})l_9^2 - \\
& \left. (-2\tau_{4,6}^2 + (\tau_{1,9} - 2\tau_{1,13} + \tau_{2,9} - 2\tau_{2,13})\tau_{4,6} + \tau_{3,6}(\tau_{1,9} - 2\tau_{1,12} + \tau_{2,9} - 2(\tau_{2,12} + \tau_{3,6})))l_{11}^2 \right) t^2 + \\
& 2(\tau_{1,7} + \tau_{1,8} + \tau_{2,7} + \tau_{2,8})^2 (\tau_{3,5}^2 + \tau_{4,5}^2) t - \frac{1}{2}(-s^2 + t^2 + u^2) \\
& (6\tau_{5,7}^2 + 6\tau_{5,8}^2 + l_5^2(10(\tau_{6,7} + \tau_{6,8}) - 11l_{11}^2) - 6(2l_7^2 l_8^2 + \tau_{10,11}l_9^2 + \tau_{6,9}l_{11}^2))t + \\
& 2u(\tau_{1,7} + \tau_{1,8} + \tau_{2,7} + \tau_{2,8})^2 (\tau_{3,5}^2 + \tau_{4,5}^2) + \\
& (s^2 - t^2 - u^2) \left( 2l_5^2 \tau_{1,7}^2 - (4\tau_{3,5}\tau_{5,7} + 4\tau_{4,5}\tau_{5,8} + (3\tau_{1,9} + \tau_{1,16} - 4\tau_{2,7} + 3\tau_{2,9} + \tau_{2,16} - 3\tau_{3,6})l_5^2 - 4\tau_{3,10}l_9^2)\tau_{1,7} + \right. \\
& 2\tau_{1,8}^2 l_5^2 + 2\tau_{2,7}^2 l_5^2 + 2\tau_{2,8}^2 l_5^2 + 2\tau_{2,9}^2 l_5^2 + (2\tau_{1,9} - \tau_{1,14} + \tau_{1,16} - 4\tau_{2,6})(\tau_{1,9} + \tau_{2,6})l_5^2 + \\
& 4\tau_{1,9}\tau_{2,9}l_5^2 - \tau_{1,14}\tau_{2,9}l_5^2 + \tau_{1,16}\tau_{2,9}l_5^2 - 2\tau_{2,6}\tau_{2,9}l_5^2 - \tau_{1,9}\tau_{2,14}l_5^2 - \tau_{2,6}\tau_{2,14}l_5^2 - \tau_{2,9}\tau_{2,14}l_5^2 + \\
& \tau_{1,9}\tau_{2,16}l_5^2 + \tau_{2,6}\tau_{2,16}l_5^2 + \tau_{2,9}\tau_{2,16}l_5^2 - 5\tau_{1,9}\tau_{3,6}l_5^2 - 5\tau_{2,6}\tau_{3,6}l_5^2 - 5\tau_{2,9}\tau_{3,6}l_5^2 - 5\tau_{1,9}\tau_{4,6}l_5^2 - \\
& 5\tau_{2,6}\tau_{4,6}l_5^2 - 5\tau_{2,9}\tau_{4,6}l_5^2 - 2\tau_{1,11}\tau_{3,10}l_9^2 - 2\tau_{2,11}\tau_{3,10}l_9^2 - 2\tau_{1,11}\tau_{4,10}l_9^2 - 2\tau_{2,11}\tau_{4,10}l_9^2 - \\
& \tau_{2,7}(4\tau_{3,5}\tau_{5,7} + 4\tau_{4,5}\tau_{5,8} + (2\tau_{1,9} + \tau_{1,16} - \tau_{2,6} + 2\tau_{2,9} + \tau_{2,16} - 3\tau_{3,6})l_5^2 - 4\tau_{3,10}l_9^2) + \\
& \tau_{1,8}(-4\tau_{3,5}\tau_{5,7} - 4\tau_{4,5}\tau_{5,8} + (-3\tau_{1,9} + \tau_{1,14} + 4\tau_{2,8} - 3\tau_{2,9} + \tau_{2,14} + 3\tau_{4,6})l_5^2 + 4\tau_{4,10}l_9^2) + \\
& \tau_{2,8}(-4\tau_{3,5}\tau_{5,7} - 4\tau_{4,5}\tau_{5,8} + (-2\tau_{1,9} + \tau_{1,14} + \tau_{2,6} - 2\tau_{2,9} + \tau_{2,14} + 3\tau_{4,6})l_5^2 + 4\tau_{4,10}l_9^2) + \\
& \left. 2(-2\tau_{4,6}^2 + (\tau_{1,9} - 2\tau_{1,13} + \tau_{2,9} - 2\tau_{2,13})\tau_{4,6} + \tau_{3,6}(\tau_{1,9} - 2\tau_{1,12} + \tau_{2,9} - 2(\tau_{2,12} + \tau_{3,6})))l_{11}^2 \right) + \\
& u^3 (2(\tau_{5,7}^2 + \tau_{5,8}^2 + (\tau_{6,7} + \tau_{6,8})l_5^2 - 2l_7^2 l_8^2 - \tau_{10,11}l_9^2) + (l_5^2 - 2\tau_{6,9})l_{11}^2) + \\
& u^2 (l_5^2 \tau_{1,7}^2 + 2(-2\tau_{3,5}\tau_{5,7} - 2\tau_{4,5}\tau_{5,8} + (-\tau_{1,9} + 2\tau_{2,7} - \tau_{2,9} + \tau_{2,16} + \tau_{3,6})l_5^2 + 2\tau_{3,10}l_9^2)\tau_{1,7} + \\
& 2\tau_{1,8}^2 l_5^2 + 3\tau_{2,7}^2 l_5^2 - 2\tau_{2,7}(2\tau_{3,5}\tau_{5,7} + 2\tau_{4,5}\tau_{5,8} + (\tau_{1,9} + \tau_{1,16} + \tau_{2,6} + \tau_{2,9})l_5^2 - 2\tau_{3,10}l_9^2) + \\
& 2\tau_{1,8}(-2\tau_{3,5}\tau_{5,7} - 2\tau_{4,5}\tau_{5,8} + (-\tau_{1,14} + \tau_{2,6} + \tau_{2,8} + 2\tau_{4,6})l_5^2 + 2\tau_{4,10}l_9^2) - \\
& 2(-((\tau_{2,6} + \tau_{2,9})(2\tau_{1,14} - 3\tau_{2,6} + \tau_{2,14} - 2\tau_{3,6} - 3\tau_{4,6}) + \tau_{1,9}(2\tau_{1,14} - 3\tau_{2,6} + \tau_{2,14} - 2\tau_{3,6} + \tau_{3,16} - 3\tau_{4,6} + \tau_{4,14})) \\
& l_5^2 + (\tau_{1,11} + \tau_{2,11})(\tau_{3,10} + \tau_{4,10})l_9^2 + \\
& \tau_{2,8}(2\tau_{3,5}\tau_{5,7} + 2\tau_{4,5}\tau_{5,8} - (\tau_{1,9} - 2\tau_{1,14} + 3\tau_{2,6} + \tau_{2,9} - \tau_{2,14} + 3\tau_{4,6})l_5^2 - 2\tau_{4,10}l_9^2) - \\
& \left. (-2\tau_{4,6}^2 + (\tau_{1,9} - 2\tau_{1,13} + \tau_{2,9} - 2\tau_{2,13})\tau_{4,6} + \tau_{3,6}(\tau_{1,9} - 2\tau_{1,12} + \tau_{2,9} - 2(\tau_{2,12} + \tau_{3,6})))l_{11}^2 \right) - \\
& \left. \frac{1}{2}u(-s^2 + t^2 + u^2)(6\tau_{5,7}^2 + 6\tau_{5,8}^2 + l_5^2(10(\tau_{6,7} + \tau_{6,8}) - 11l_{11}^2) - 6(2l_7^2 l_8^2 + \tau_{10,11}l_9^2 + \tau_{6,9}l_{11}^2)) \right)
\end{aligned}$$

■  $N_{44}^{(5)}$ 

$$\begin{aligned}
& \frac{1}{4} l_5^2 \left( (-2(\tau_{1,7} + \tau_{2,7}) \tau_{6,7} + 2(\tau_{2,6} - \tau_{2,8} + \tau_{2,9}) \tau_{6,8} - (\tau_{1,10} + 2(\tau_{1,11} + \tau_{2,11}) - \tau_{2,13}) l_6^2 + \right. \\
& \quad 2(3\tau_{3,12} + 2\tau_{4,13}) l_9^2 + (-2\tau_{2,7} + 2\tau_{2,8} + 3\tau_{2,9} - 5\tau_{2,10} + 3\tau_{3,8} + 4\tau_{3,10} - 3\tau_{4,7} - 4\tau_{4,10}) l_{11}^2) t^3 + \\
& \quad (-2\tau_{2,6}^3 - (-4\tau_{2,7} - 2\tau_{2,8} + 4\tau_{2,9} + \tau_{2,16} + 2(\tau_{3,6} + \tau_{4,6})) \tau_{2,6}^2 + \\
& \quad (-2\tau_{2,7}^2 + 2(2\tau_{2,9} + \tau_{2,16} + 3\tau_{3,6}) \tau_{2,7} + \tau_{2,8}^2 + 2\tau_{2,8}(\tau_{2,9} + \tau_{4,6}) - 2\tau_{2,9}(\tau_{2,9} + \tau_{2,16} + 2(\tau_{3,6} + \tau_{4,6}))) \tau_{2,6} - \\
& \quad 2\tau_{1,14} \tau_{2,8}^2 - 2\tau_{1,16}(\tau_{2,6} - \tau_{2,7} + \tau_{2,9})^2 - \tau_{2,8}^2 \tau_{2,14} + \tau_{1,7}^2 \tau_{2,16} - \tau_{2,7}^2 \tau_{2,16} - \\
& \quad \tau_{2,9}^2 \tau_{2,16} + 2\tau_{2,7} \tau_{2,9} \tau_{2,16} - 2\tau_{2,7}^2 \tau_{3,6} - 2\tau_{2,9}^2 \tau_{3,6} + 6\tau_{2,7} \tau_{2,9} \tau_{3,6} + \\
& \quad 2\tau_{1,7}((\tau_{1,16} + \tau_{2,6})(\tau_{2,6} - \tau_{2,7} + \tau_{2,9}) + (2\tau_{2,6} - \tau_{2,7} + 2\tau_{2,9}) \tau_{3,6}) + 2\tau_{2,8}^2 \tau_{4,6} - 2\tau_{2,9}^2 \tau_{4,6} + 2\tau_{2,8} \tau_{2,9} \tau_{4,6}) t^2 + \\
& \quad \frac{1}{2} (s^2 - t^2 - u^2) (2(-5\tau_{1,7} + 2\tau_{2,6} - 5\tau_{2,7} + 2\tau_{2,9}) \tau_{6,7} + 2(3\tau_{2,6} - 5\tau_{2,8} + 3\tau_{2,9}) \tau_{6,8} + (-\tau_{1,10} + \tau_{2,12} + 2\tau_{2,13}) l_6^2 + \\
& \quad 2(7\tau_{3,12} + 6\tau_{4,13}) l_9^2 + (-2\tau_{2,7} + 2\tau_{2,8} + 7\tau_{2,9} - 5\tau_{2,10} + 3\tau_{3,8} + 4\tau_{3,10} - 3\tau_{4,7} - 4\tau_{4,10}) l_{11}^2) t - \\
& \quad \tau_{1,8}^2 (t(t + 4u) \tau_{2,6} + (u^2 - t^2) \tau_{2,14}) - (s^2 - t^2 - u^2) \\
& \quad (2\tau_{2,6} \tau_{1,7}^2 + (-3\tau_{2,6}^2 + (4\tau_{2,7} - 3\tau_{2,9} + \tau_{2,16} - 3\tau_{3,6}) \tau_{2,6} + \tau_{1,16}(\tau_{2,6} + \tau_{2,9}) + \tau_{2,9}(\tau_{2,16} - 3\tau_{3,6})) \tau_{1,7} + \\
& \quad 2(\tau_{2,6}^3 + (-2\tau_{2,7} - 2\tau_{2,8} + 2\tau_{2,9} + \tau_{3,6} + \tau_{4,6}) \tau_{2,6}^2 + (\tau_{2,7}^2 - 2(\tau_{2,9} + \tau_{3,6}) \tau_{2,7} + \tau_{2,8}^2 - 2\tau_{2,8}(\tau_{2,9} + \tau_{4,6}) + \\
& \quad \tau_{2,9}(\tau_{2,9} + 2(\tau_{3,6} + \tau_{4,6}))) \tau_{2,6} + \tau_{2,9}((\tau_{2,9} - 2\tau_{2,7}) \tau_{3,6} + (\tau_{2,9} - 2\tau_{2,8}) \tau_{4,6}))) + \\
& \quad u^2 (-2\tau_{2,6}^3 + (2\tau_{2,7} + 4\tau_{2,8} - 4\tau_{2,9} + \tau_{2,14} - 2(\tau_{3,6} + \tau_{4,6})) \tau_{2,6}^2 + \\
& \quad (\tau_{2,7}^2 + 2(\tau_{2,9} + \tau_{3,6}) \tau_{2,7} - 2(\tau_{2,8}^2 + (-2\tau_{2,9} + \tau_{2,14} - 3\tau_{4,6}) \tau_{2,8} + \tau_{2,9}(\tau_{2,9} - \tau_{2,14} + 2(\tau_{3,6} + \tau_{4,6})))) \tau_{2,6} + \\
& \quad 2\tau_{1,16} \tau_{2,7}^2 + 2\tau_{1,14}(\tau_{2,6} - \tau_{2,8} + \tau_{2,9})^2 + \tau_{2,8}^2 \tau_{2,14} + \tau_{2,9}^2 \tau_{2,14} - 2\tau_{2,8} \tau_{2,9} \tau_{2,14} + \\
& \quad \tau_{2,7}^2 \tau_{2,16} - \tau_{1,7}^2(\tau_{2,6} + \tau_{2,16}) + 2\tau_{2,7}^2 \tau_{3,6} - 2\tau_{2,9}^2 \tau_{3,6} + 2\tau_{2,7} \tau_{2,9} \tau_{3,6} + \\
& \quad 2\tau_{1,7}(\tau_{1,16} \tau_{2,7} + \tau_{2,6}(\tau_{2,6} + \tau_{2,9}) + (\tau_{2,6} + \tau_{2,7} + \tau_{2,9}) \tau_{3,6}) - 2\tau_{2,8}^2 \tau_{4,6} - 2\tau_{2,9}^2 \tau_{4,6} + 6\tau_{2,8} \tau_{2,9} \tau_{4,6}) - \\
& \quad \tau_{1,9}^2 (2\tau_{3,6} s^2 + 2\tau_{4,6} s^2 - 2t \tau_{3,16} s + 2u \tau_{4,14} s - 2u^2 \tau_{1,14} + 2t^2 \tau_{1,16} + 2(t + u)^2 \tau_{2,6} - u^2 \tau_{2,14} + t^2 \tau_{2,16}) + \\
& \quad \tau_{1,8} (-(-3s^2 + t^2 + u^2) \tau_{2,6}^2 - (2u(4t + u) \tau_{2,8} + (-3s^2 + t^2 + u^2) \tau_{2,9} + (-s^2 + t^2 + u^2) \tau_{2,14} + 2s(t + 2u) \tau_{4,6}) \tau_{2,6} + \\
& \quad 2(t - u) \tau_{1,14} (s \tau_{2,8} + u(\tau_{2,6} + \tau_{2,9})) + \tau_{2,9} ((s^2 - t^2 - u^2) \tau_{2,14} - 2s(t + 2u) \tau_{4,6}) - \\
& \quad \tau_{1,9} (2u(u - t) \tau_{1,14} + (-3s^2 + t^2 + u^2) \tau_{2,6} + (-s^2 + t^2 + u^2) \tau_{2,14} + 2s((t + 2u) \tau_{4,6} + (t - u) \tau_{4,14})) + \\
& \quad 2s((u - t) \tau_{2,8} \tau_{4,6} - (-2s^2 + t^2 + u^2) \tau_{6,8})) + \\
& \quad u^3 (2(-\tau_{1,7} + \tau_{2,6} - \tau_{2,7} + \tau_{2,9}) \tau_{6,7} - 2\tau_{2,8} \tau_{6,8} - (\tau_{1,10} + 2(\tau_{1,11} + \tau_{2,11}) - \tau_{2,12}) l_6^2 + 2(2\tau_{3,12} + 3\tau_{4,13}) l_9^2 + \\
& \quad (2\tau_{2,7} - 2\tau_{2,8} + 3\tau_{2,9} - 5\tau_{2,10} - 3\tau_{3,8} - 4\tau_{3,10} + 3\tau_{4,7} + 4\tau_{4,10}) l_{11}^2) + \\
& \quad \frac{1}{2} u (s^2 - t^2 - u^2) (2(-5\tau_{1,7} + 3\tau_{2,6} - 5\tau_{2,7} + 3\tau_{2,9}) \tau_{6,7} + 2(2\tau_{2,6} - 5\tau_{2,8} + 2\tau_{2,9}) \tau_{6,8} + (-\tau_{1,10} + 2\tau_{2,12} + \tau_{2,13}) l_6^2 + \\
& \quad 2(6\tau_{3,12} + 7\tau_{4,13}) l_9^2 + (2\tau_{2,7} - 2\tau_{2,8} + 7\tau_{2,9} - 5\tau_{2,10} - 3\tau_{3,8} - 4\tau_{3,10} + 3\tau_{4,7} + 4\tau_{4,10}) l_{11}^2) +
\end{aligned}$$

$$\begin{aligned}
& \tau_{1,9} \left( (2\tau_{6,8} + 5l_{11}^2)t^3 - 2(2\tau_{2,6}^2 + (-2\tau_{2,7} - \tau_{2,8} + 2\tau_{2,9} + \tau_{2,16} + 2\tau_{3,6} + \tau_{3,16} + 2\tau_{4,6})\tau_{2,6} + \right. \\
& \quad 2\tau_{1,16}(\tau_{2,6} - \tau_{2,7} + \tau_{2,9}) - \tau_{2,7}(\tau_{2,16} + 3\tau_{3,6} + \tau_{3,16}) + \tau_{2,9}(\tau_{2,16} + 2\tau_{3,6} + \tau_{3,16} + 2\tau_{4,6}) - \tau_{2,8}(\tau_{4,6} + \tau_{4,14})) \\
& \quad t^2 - \frac{1}{2}(-s^2 + t^2 + u^2)(4\tau_{6,7} + 6\tau_{6,8} + 13l_{11}^2)t + \\
& \quad 2\tau_{1,7} \left( t(t-u)\tau_{1,16} - \frac{1}{2}(-3s^2 + t^2 + u^2)\tau_{2,6} + \frac{1}{2}(-s^2 + t^2 + u^2)\tau_{2,16} - s((2t+u)\tau_{3,6} + (t-u)\tau_{3,16}) \right) - \\
& \quad (s^2 - t^2 - u^2)(4\tau_{2,6}^2 + (-4\tau_{2,7} - 4\tau_{2,8} + 4\tau_{2,9} + 4\tau_{3,6} + \tau_{3,16} + 4\tau_{4,6} - \tau_{4,14})\tau_{2,6} - 4\tau_{2,7}\tau_{3,6} - 4\tau_{2,8}\tau_{4,6} + \\
& \quad \tau_{2,9}(4\tau_{3,6} + \tau_{3,16} + 4\tau_{4,6} - \tau_{4,14})) + 2u^2(-2\tau_{2,6}^2 + (\tau_{2,7} + 2\tau_{2,8} - 2\tau_{2,9} + \tau_{2,14} - 2(\tau_{3,6} + \tau_{4,6}) + \tau_{4,14})\tau_{2,6} + \\
& \quad 2\tau_{1,14}(\tau_{2,6} - \tau_{2,8} + \tau_{2,9}) + \tau_{2,7}(\tau_{3,6} - \tau_{3,16}) - \tau_{2,8}(\tau_{2,14} - 3\tau_{4,6} + \tau_{4,14}) + \tau_{2,9}(\tau_{2,14} - 2(\tau_{3,6} + \tau_{4,6}) + \tau_{4,14})) + \\
& \quad \left. u^3(2\tau_{6,7} + 5l_{11}^2) - \frac{1}{2}u(-s^2 + t^2 + u^2)(6\tau_{6,7} + 4\tau_{6,8} + 13l_{11}^2) \right) \Big)
\end{aligned}$$

■  $N_{44}^{(6)}$

$$\begin{aligned}
& \frac{1}{16} \left( (-4\tau_{10,12}l_5^2l_6^2 + 4\tau_{10,13}l_5^2l_6^2 + 25l_7^2l_8^2l_6^2 + l_5^2(25l_7^2l_8^2 + 4l_6^2(7l_{11}^2 - 6l_9^2)))t^3 - \right. \\
& \quad 2(6\tau_{1,10}^2 + (10\tau_{1,11} - 4\tau_{1,13} + 2\tau_{1,14} + \tau_{2,10} + 8\tau_{2,11} + 2\tau_{2,12} - 6\tau_{2,13} + \tau_{2,14} - \tau_{2,16} + 2(\tau_{3,10} + \tau_{3,14} - \tau_{4,16}))\tau_{1,10} + \\
& \quad 2(-\tau_{1,11}^2 + (\tau_{1,14} + 3\tau_{2,10} - 3\tau_{2,11} + 2\tau_{2,13} + \tau_{2,14} - \tau_{2,16} + 3\tau_{3,10} + \tau_{3,14} + 2\tau_{4,10} - 3\tau_{4,16})\tau_{1,11} - \\
& \quad 2\tau_{2,11}^2 - 2\tau_{2,12}^2 - 2\tau_{2,13}^2 + 3\tau_{2,10}\tau_{2,11} + 3\tau_{1,14}\tau_{2,12} - \tau_{2,10}\tau_{2,12} + \tau_{2,11}\tau_{2,12} + \tau_{1,16}(\tau_{2,11} - \tau_{2,13}) - \\
& \quad 2\tau_{2,10}\tau_{2,13} + 3\tau_{2,11}\tau_{2,13} + 2\tau_{2,12}\tau_{2,14} + 3\tau_{2,11}\tau_{3,10} - 3\tau_{2,12}\tau_{3,10} + 2\tau_{2,12}\tau_{3,14} + \\
& \quad \tau_{1,12}(2\tau_{1,14} - \tau_{2,10} + \tau_{2,11} - 2\tau_{2,12} + \tau_{2,14} - 2\tau_{3,10} + 2\tau_{3,14}) + 2\tau_{2,11}\tau_{4,10} - 5\tau_{2,13}\tau_{4,10} - \\
& \quad \left. 2\tau_{2,11}\tau_{4,16} + 2\tau_{2,13}\tau_{4,16} + \tau_{1,13}(-2\tau_{2,10} + \tau_{2,11} - 2\tau_{2,13} + \tau_{2,16} - 4\tau_{4,10} + 2\tau_{4,16}))l_5^2l_6^2t^2 + \right. \\
& \quad \frac{1}{2}(-s^2 + t^2 + u^2)(4\tau_{10,12}l_5^2l_6^2 - 4\tau_{10,13}l_5^2l_6^2 + 41l_7^2l_8^2l_6^2 + l_5^2(4l_6^2(28l_9^2 - 29l_{11}^2) - 13l_7^2l_8^2))t - \\
& \quad 2(s^2 - t^2 - u^2)(4\tau_{1,10}^2 + \\
& \quad (10\tau_{1,11} - 4\tau_{1,12} - 4\tau_{1,13} + \tau_{1,14} - \tau_{1,16} + 8\tau_{2,11} - 4\tau_{2,12} - 4\tau_{2,13} + \tau_{2,14} - \tau_{2,16} + \tau_{3,10} + 2\tau_{3,14} + \tau_{4,10} - 2\tau_{4,16}) \\
& \quad \tau_{1,10} - 2\tau_{2,11}^2 - 4\tau_{2,12}^2 - 4\tau_{2,13}^2 + \tau_{1,14}\tau_{2,11} - \tau_{1,16}\tau_{2,11} + 8\tau_{2,10}\tau_{2,11} - \\
& \quad 4\tau_{2,10}\tau_{2,12} + 4\tau_{2,11}\tau_{2,12} - 4\tau_{2,10}\tau_{2,13} + 4\tau_{2,11}\tau_{2,13} + \tau_{2,11}\tau_{2,14} - \tau_{2,11}\tau_{2,16} + 5\tau_{2,11}\tau_{3,10} - \\
& \quad 8\tau_{2,12}\tau_{3,10} - 2\tau_{1,12}(\tau_{1,14} + 2\tau_{2,10} - \tau_{2,11} + 2\tau_{2,12} + \tau_{2,14} + 3\tau_{3,10}) + 2\tau_{2,11}\tau_{3,14} + \\
& \quad 2\tau_{1,13}(\tau_{1,16} - 2\tau_{2,10} + \tau_{2,11} - 2\tau_{2,13} + \tau_{2,16} - 3\tau_{4,10}) + 5\tau_{2,11}\tau_{4,10} - 8\tau_{2,13}\tau_{4,10} + \\
& \quad \tau_{1,11}(3\tau_{1,14} - 3\tau_{1,16} + 8\tau_{2,10} - 2\tau_{2,11} + 2\tau_{2,12} + 2\tau_{2,13} + 3\tau_{2,14} - 3\tau_{2,16} + 5\tau_{3,10} + 4\tau_{3,14} + 5\tau_{4,10} - 4\tau_{4,16}) - \\
& \quad \left. 2\tau_{2,11}\tau_{4,16})l_5^2l_6^2 - \right. \\
& \quad \left. 2u^2(6\tau_{1,10}^2 + (10\tau_{1,11} - 4\tau_{1,12} - 2\tau_{1,16} + \tau_{2,10} + 8\tau_{2,11} - 6\tau_{2,12} + 2\tau_{2,13} + \tau_{2,14} - \tau_{2,16} + 2(\tau_{3,14} + \tau_{4,10} - \tau_{4,16}))\tau_{1,10} - \right. \\
& \quad \left. 2(\tau_{1,11}^2 + (\tau_{1,16} - 3\tau_{2,10} + 3\tau_{2,11} - 2\tau_{2,12} - \tau_{2,14} + \tau_{2,16} - 2\tau_{3,10} - 3(\tau_{3,14} + \tau_{4,10}) + \tau_{4,16})\tau_{1,11} + \right.
\end{aligned}$$

$$\begin{aligned}
& 2 \tau_{2,11}^2 + 2 \tau_{2,12}^2 + 2 \tau_{2,13}^2 + \tau_{1,14} (\tau_{2,11} - \tau_{2,12}) - 3 \tau_{2,11} \tau_{2,12} + 3 \tau_{1,16} \tau_{2,13} - \tau_{2,11} \tau_{2,13} + \\
& \tau_{2,10} (-3 \tau_{2,11} + 2 \tau_{2,12} + \tau_{2,13}) + 2 \tau_{2,13} \tau_{2,16} - 2 \tau_{2,11} \tau_{3,10} + 5 \tau_{2,12} \tau_{3,10} - 2 \tau_{2,11} \tau_{3,14} + \\
& 2 \tau_{2,12} \tau_{3,14} + \tau_{1,12} (2 \tau_{2,10} - \tau_{2,11} + 2 \tau_{2,12} + \tau_{2,14} + 4 \tau_{3,10} + 2 \tau_{3,14}) - 3 \tau_{2,11} \tau_{4,10} + \\
& 3 \tau_{2,13} \tau_{4,10} + 2 \tau_{2,13} \tau_{4,16} + \tau_{1,13} (2 \tau_{1,16} + \tau_{2,10} - \tau_{2,11} + 2 \tau_{2,13} + \tau_{2,16} + 2 (\tau_{4,10} + \tau_{4,16})) \Big) l_5^2 l_6^2 + \\
& u^3 (4 \tau_{10,12} l_5^2 l_6^2 - 4 \tau_{10,13} l_5^2 l_6^2 + 25 l_7^2 l_8^2 l_6^2 + l_5^2 (25 l_7^2 l_8^2 + 4 l_6^2 (7 l_{11}^2 - 6 l_9^2))) - \\
& \frac{1}{2} u (-s^2 + t^2 + u^2) \\
& (4 \tau_{10,12} l_5^2 l_6^2 - 4 \tau_{10,13} l_5^2 l_6^2 - 41 l_7^2 l_8^2 l_6^2 + l_5^2 (13 l_7^2 l_8^2 + 4 l_6^2 (29 l_{11}^2 - 28 l_9^2))) \Big)
\end{aligned}$$

■  $N_{44}^{(7)}$

$$\begin{aligned}
& \frac{1}{16} l_7^2 l_8^2 \\
& (l_5^2 (\tau_{2,14} (16 s^2 - 47 t^2 - 35 u^2) + \tau_{2,16} (-16 s^2 + 35 t^2 + 47 u^2) + \tau_{3,14} (2 s^2 - 9 t^2 - 13 u^2) - 2 s^2 \tau_{4,16} + 13 \tau_{3,16} (t^2 - u^2) + \\
& 13 t^2 \tau_{4,14} + 13 t^2 \tau_{4,16} - 13 u^2 \tau_{4,14} + 9 u^2 \tau_{4,16}) + \\
& l_6^2 (4 \tau_{1,10} (s^2 + 22 (t^2 + u^2)) + (t - u) (\tau_{1,14} (7 t + 11 u) + \tau_{1,16} (11 t + 7 u) - \tau_{2,14} (5 t + u) - \tau_{2,16} (t + 5 u) + \\
& 37 t \tau_{3,10} + 4 t \tau_{3,16} - 41 t \tau_{4,10} - 4 t \tau_{4,14} + 41 u \tau_{3,10} - 4 u \tau_{3,16} - 37 u \tau_{4,10} + 4 u \tau_{4,14})))
\end{aligned}$$

■  $N_{44}^{(8)}$

$$\frac{1}{2} l_5^2 l_6^2 l_7^2 l_8^2 (s^2 + t^2 + u^2)$$
