# Supplementary material for: The Ultraviolet Behavior of N=8 Supergravity at Four Loops
Source: arXiv:0905.2326 ancillary file (2012-01-08)
Supplement: Supplementary file 41 [file SUGRA45.pdf]

## Integral 45: $\mathcal{I}_{45}$

$\mathcal{N} = 8$  four-point four-loop amplitude.

### ■ 2D plot of graph associated with $\mathcal{I}_{45}$

This fixes the labelling associated with the numerator expressions given below.

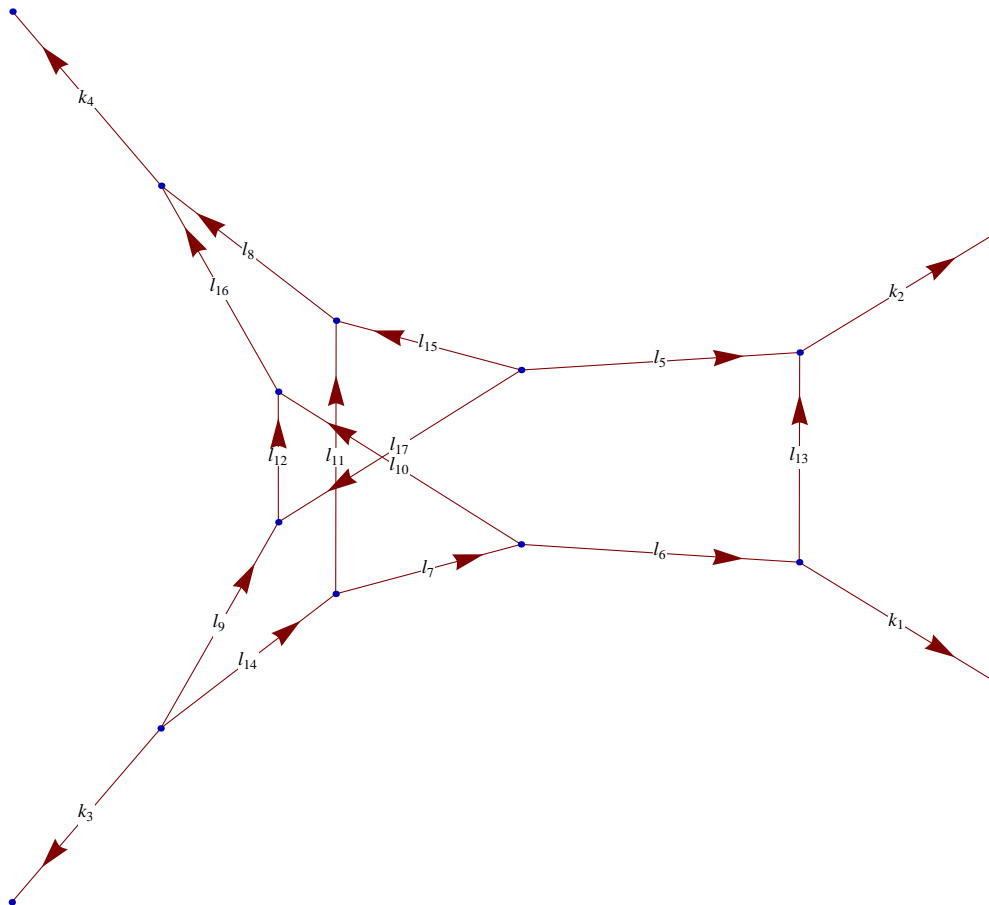

When using MathPlayer, by clicking three times (holding the click on the third click) directly on a vertex, one is able to move that vertex around, and its associated edges follow elastically. This functionality is absent when viewing as a pdf.

*Note: propagators for certain graphs were relabeled in the manuscript due to size constraints. The labels given in `aux/rawData/Neq8FourLoops.m` should be used for verification purposes.*

### ■ 3D plot of graph associated with $\mathcal{I}_{45}$

3D PLOT UNAVAILABLE FOR PDF. Please see .nb version for the 3D figure.

When using MathPlayer, by clicking anywhere in the image and dragging one should be able to rotate this 3D image. By holding (ALT) or (COMMAND) while clicking and moving the mouse up/down one should be able to zoom in/out. This functionality is absent when viewing as a pdf.

### ■ "Vertex Form" of graph associated with $\mathcal{I}_{45}$

This function returns the graph associated with the integral object in a vertex representation. This can be used as a way of specifying the topology of a graph using trivalent (cubic) vertices, `gVertex[ $p_a, p_b, p_c$ ]`, where  $\{p_a, p_b, p_c\}$  are momenta labeling the propagators (edges) of the graph, and is understood that the edge labelled by  $p_a$  flows into the edge labelled by  $-p_a$ . Additionally, each vertex represents the manifest conservation of ( $D$  - dimensional) momenta :

$$\text{gVertex}[\{p_1, p_2, p_3\}] \iff (p_1 + p_2 + p_3 = 0)$$

$$\{\text{gVertex}(\{k_1, l_{13}, -l_6\}), \text{gVertex}(\{k_2, -l_5, -l_{13}\}), \text{gVertex}(\{k_3, l_9, l_{14}\}), \text{gVertex}(\{k_4, -l_{16}, -l_8\}), \text{gVertex}(\{l_5, l_{17}, l_{15}\}), \\ \text{gVertex}(\{l_6, l_{10}, -l_7\}), \text{gVertex}(\{l_7, l_{11}, -l_{14}\}), \text{gVertex}(\{l_8, -l_{15}, -l_{11}\}), \text{gVertex}(\{-l_9, -l_{17}, l_{12}\}), \text{gVertex}(\{-l_{10}, -l_{12}, l_{16}\})\}$$

### ■ Numerator expression for integral 45:

The following notation is used:  $\tau_{i,j} \equiv \begin{cases} 2 k_i \cdot l_j & \text{if } i \leq 4, j > 4 \\ 2 l_i \cdot l_j & \text{if } i, j > 4 \end{cases}$ .

$$s \equiv 2 k_1 \cdot k_2 = 2 k_3 \cdot k_4$$

We use  $s, t, u$  to represent the traditional Mandelstam variables for massless external four-point momenta:  $t \equiv 2 k_1 \cdot k_4 = 2 k_2 \cdot k_3$ .

$$u \equiv 2 k_1 \cdot k_3 = 2 k_2 \cdot k_4$$

Furthermore we use the shorthand  $(l_i)^2$  to represent the lorentz square:  $(l_i)^2 = l_i \cdot l_i$ .

The total numerator  $\mathcal{N}_{45}$  is given by summing over the following terms, distinguished here by explicit dependence on loop momenta:  $\mathcal{N}_{45} = \sum_{i=0}^8 \mathcal{N}_{45}^{(i)}$ :

#### ■ $\mathcal{N}_{45}^{(0)}$

$$0$$

#### ■ $\mathcal{N}_{45}^{(1)}$

$$0$$

■  $N_{45}^{(2)}$

$$\begin{aligned}
& \frac{1}{4} \left( -2 l_5^2 t^5 - 3 u l_5^2 t^4 + 2 s^2 l_5^2 t^3 - 6 u^2 l_5^2 t^3 + s u l_5^2 t^3 - 5 u^3 l_5^2 t^2 + s u^2 l_5^2 t^2 + 3 s^2 u l_5^2 t^2 - 2 u^4 l_5^2 t - s u^3 l_5^2 t + 2 s^2 u^2 l_5^2 t + \right. \\
& s^3 u l_5^2 t + s^4 \tau_{1,7}^2 + s^4 \tau_{1,8}^2 + s^4 \tau_{1,9}^2 + s^4 \tau_{1,10}^2 + s^4 \tau_{1,14}^2 + s^4 \tau_{1,15}^2 + s^4 \tau_{1,16}^2 + s^4 \tau_{1,17}^2 + s^4 \tau_{2,7}^2 + s^4 \tau_{2,8}^2 + s^4 \tau_{2,9}^2 + \\
& s^4 \tau_{2,10}^2 + s^4 \tau_{2,14}^2 + s^4 \tau_{2,15}^2 + s^4 \tau_{2,16}^2 + s^4 \tau_{2,17}^2 + 4 s^4 \tau_{3,5}^2 + 4 s^4 \tau_{3,6}^2 + s^4 \tau_{3,7}^2 + s^4 \tau_{3,17}^2 + 4 s^4 \tau_{4,5}^2 + 4 s^4 \tau_{4,6}^2 + \\
& s^4 \tau_{4,10}^2 + s^4 \tau_{4,15}^2 - 2 s^4 \tau_{1,14} \tau_{1,15} + 2 s^4 \tau_{1,16} \tau_{1,17} - 2 s^4 \tau_{2,7} \tau_{2,8} - 2 s^4 \tau_{2,9} \tau_{2,10} + 2 s^4 \tau_{1,14} \tau_{2,14} - 2 s^4 \tau_{1,15} \tau_{2,14} - \\
& 2 s^4 \tau_{1,14} \tau_{2,15} + 2 s^4 \tau_{1,15} \tau_{2,15} - 2 s^4 \tau_{2,14} \tau_{2,15} + 2 s^4 \tau_{1,16} \tau_{2,16} + 2 s^4 \tau_{1,17} \tau_{2,16} + 2 s^4 \tau_{1,16} \tau_{2,17} + 2 s^4 \tau_{1,17} \tau_{2,17} + \\
& 2 s^4 \tau_{2,16} \tau_{2,17} + 4 s^4 \tau_{2,7} \tau_{3,5} - 4 s^4 \tau_{2,8} \tau_{3,5} - 4 s^4 \tau_{1,16} \tau_{3,6} - 4 s^4 \tau_{1,17} \tau_{3,6} - 4 s^4 \tau_{2,16} \tau_{3,6} - 4 s^4 \tau_{2,17} \tau_{3,6} + 2 s^4 \tau_{2,7} \tau_{3,7} - \\
& 2 s^4 \tau_{2,8} \tau_{3,7} + 4 s^4 \tau_{3,5} \tau_{3,7} - 2 s^4 \tau_{1,8} (\tau_{2,7} - \tau_{2,8} + 2 \tau_{3,5} + \tau_{3,7}) + 2 s^4 \tau_{1,7} (-\tau_{1,8} + \tau_{2,7} - \tau_{2,8} + 2 \tau_{3,5} + \tau_{3,7}) + \\
& 2 s^4 \tau_{1,16} \tau_{3,17} + 2 s^4 \tau_{1,17} \tau_{3,17} + 2 s^4 \tau_{2,16} \tau_{3,17} + 2 s^4 \tau_{2,17} \tau_{3,17} - 4 s^4 \tau_{3,6} \tau_{3,17} + 4 s^4 \tau_{2,9} \tau_{4,5} - 4 s^4 \tau_{2,10} \tau_{4,5} + \\
& 4 s^4 \tau_{1,14} \tau_{4,6} - 4 s^4 \tau_{1,15} \tau_{4,6} + 4 s^4 \tau_{2,14} \tau_{4,6} - 4 s^4 \tau_{2,15} \tau_{4,6} - 2 s^4 \tau_{2,9} \tau_{4,10} + 2 s^4 \tau_{2,10} \tau_{4,10} - 4 s^4 \tau_{4,5} \tau_{4,10} + \\
& 2 s^4 \tau_{1,10} (-\tau_{2,9} + \tau_{2,10} - 2 \tau_{4,5} + \tau_{4,10}) - 2 s^4 \tau_{1,9} (\tau_{1,10} - \tau_{2,9} + \tau_{2,10} - 2 \tau_{4,5} + \tau_{4,10}) - 2 s^4 \tau_{1,14} \tau_{4,15} + 2 s^4 \tau_{1,15} \tau_{4,15} - \\
& \left. 2 s^4 \tau_{2,14} \tau_{4,15} + 2 s^4 \tau_{2,15} \tau_{4,15} - 4 s^4 \tau_{4,6} \tau_{4,15} - 2 u^5 l_5^2 - s u^4 l_5^2 + 2 s^2 u^3 l_5^2 + s^3 u^2 l_5^2 + s (t - u)^2 (-s^2 + t^2 + u^2) l_6^2 \right)
\end{aligned}$$

■  $N_{45}^{(3)}$

$$\begin{aligned}
& \frac{1}{16} (8 \tau_{2,7} \tau_{5,8} s^4 - 8 \tau_{2,8} \tau_{5,8} s^4 + 16 \tau_{3,5} \tau_{5,8} s^4 + 8 \tau_{3,7} \tau_{5,8} s^4 + 8 \tau_{1,10} \tau_{5,9} s^4 - 8 \tau_{2,9} \tau_{5,9} s^4 + 8 \tau_{2,10} \tau_{5,9} s^4 - 16 \tau_{4,5} \tau_{5,9} s^4 + \\
& 8 \tau_{4,10} \tau_{5,9} s^4 - 8 \tau_{1,14} \tau_{6,14} s^4 + 8 \tau_{1,15} \tau_{6,14} s^4 - 8 \tau_{2,14} \tau_{6,14} s^4 + 8 \tau_{2,15} \tau_{6,14} s^4 - 16 \tau_{4,6} \tau_{6,14} s^4 + 8 \tau_{4,15} \tau_{6,14} s^4 - \\
& 8 \tau_{1,16} \tau_{6,16} s^4 - 8 \tau_{1,17} \tau_{6,16} s^4 - 8 \tau_{2,16} \tau_{6,16} s^4 - 8 \tau_{2,17} \tau_{6,16} s^4 + 16 \tau_{3,6} \tau_{6,16} s^4 - 8 \tau_{3,17} \tau_{6,16} s^4 + 4 \tau_{1,10} l_5^2 s^4 + \\
& 8 \tau_{1,15} l_5^2 s^4 + 8 \tau_{1,17} l_5^2 s^4 - 4 \tau_{2,7} l_5^2 s^4 - 4 \tau_{2,8} l_5^2 s^4 + 4 \tau_{2,9} l_5^2 s^4 + 4 \tau_{2,10} l_5^2 s^4 + 8 \tau_{2,13} l_5^2 s^4 + 8 \tau_{2,15} l_5^2 s^4 + \\
& 8 \tau_{2,17} l_5^2 s^4 + 4 \tau_{3,17} l_5^2 s^4 + 4 \tau_{4,15} l_5^2 s^4 + 16 \tau_{3,5}^3 s^3 + 16 \tau_{3,6}^3 s^3 + 16 \tau_{4,5}^3 s^3 + 16 \tau_{4,6}^3 s^3 + 8 \tau_{2,7} \tau_{3,5}^2 s^3 - \\
& 24 \tau_{2,8} \tau_{3,5}^2 s^3 - 16 \tau_{2,9} \tau_{3,5}^2 s^3 - 16 \tau_{1,14} \tau_{3,6}^2 s^3 - 24 \tau_{1,16} \tau_{3,6}^2 s^3 - 8 \tau_{1,17} \tau_{3,6}^2 s^3 - 16 \tau_{2,14} \tau_{3,6}^2 s^3 - \\
& 24 \tau_{2,16} \tau_{3,6}^2 s^3 - 8 \tau_{2,17} \tau_{3,6}^2 s^3 - 8 \tau_{1,10} \tau_{4,5}^2 s^3 + 16 \tau_{2,8} \tau_{4,5}^2 s^3 + 24 \tau_{2,9} \tau_{4,5}^2 s^3 - 8 \tau_{2,10} \tau_{4,5}^2 s^3 + 24 \tau_{1,14} \tau_{4,6}^2 s^3 - \\
& 8 \tau_{1,15} \tau_{4,6}^2 s^3 + 16 \tau_{1,16} \tau_{4,6}^2 s^3 + 24 \tau_{2,14} \tau_{4,6}^2 s^3 - 8 \tau_{2,15} \tau_{4,6}^2 s^3 + 16 \tau_{2,16} \tau_{4,6}^2 s^3 + 8 \tau_{1,8}^2 \tau_{3,5} s^3 + 8 \tau_{2,8}^2 \tau_{3,5} s^3 - \\
& 8 \tau_{2,7} \tau_{2,8} \tau_{3,5} s^3 - 8 \tau_{2,7} \tau_{2,9} \tau_{3,5} s^3 + 8 \tau_{2,8} \tau_{2,9} \tau_{3,5} s^3 + 8 \tau_{1,16}^2 \tau_{3,6} s^3 + 8 \tau_{2,16}^2 \tau_{3,6} s^3 + 8 \tau_{1,14} \tau_{1,16} \tau_{3,6} s^3 + \\
& 8 \tau_{1,14} \tau_{1,17} \tau_{3,6} s^3 + 8 \tau_{1,16} \tau_{1,17} \tau_{3,6} s^3 + 8 \tau_{1,16} \tau_{2,14} \tau_{3,6} s^3 + 8 \tau_{1,17} \tau_{2,14} \tau_{3,6} s^3 + 8 \tau_{1,14} \tau_{2,16} \tau_{3,6} s^3 + \\
& 16 \tau_{1,16} \tau_{2,16} \tau_{3,6} s^3 + 8 \tau_{1,17} \tau_{2,16} \tau_{3,6} s^3 + 8 \tau_{2,14} \tau_{2,16} \tau_{3,6} s^3 + 8 \tau_{1,14} \tau_{2,17} \tau_{3,6} s^3 + 8 \tau_{1,16} \tau_{2,17} \tau_{3,6} s^3 + \\
& 8 \tau_{2,14} \tau_{2,17} \tau_{3,6} s^3 + 8 \tau_{2,16} \tau_{2,17} \tau_{3,6} s^3 + 8 \tau_{3,5}^2 \tau_{3,7} s^3 - 8 \tau_{2,8} \tau_{3,5} \tau_{3,7} s^3 - 8 \tau_{2,9} \tau_{3,5} \tau_{3,7} s^3 - 8 \tau_{3,6}^2 \tau_{3,17} s^3 + \\
& 8 \tau_{1,14} \tau_{3,6} \tau_{3,17} s^3 + 8 \tau_{1,16} \tau_{3,6} \tau_{3,17} s^3 + 8 \tau_{2,14} \tau_{3,6} \tau_{3,17} s^3 + 8 \tau_{2,16} \tau_{3,6} \tau_{3,17} s^3 + 8 \tau_{1,9}^2 \tau_{4,5} s^3 + 8 \tau_{2,9}^2 \tau_{4,5} s^3 - \\
& 8 \tau_{1,10} \tau_{2,8} \tau_{4,5} s^3 - 8 \tau_{1,10} \tau_{2,9} \tau_{4,5} s^3 + 8 \tau_{2,8} \tau_{2,9} \tau_{4,5} s^3 - 8 \tau_{2,8} \tau_{2,10} \tau_{4,5} s^3 - 8 \tau_{2,9} \tau_{2,10} \tau_{4,5} s^3 + 8 \tau_{1,14}^2 \tau_{4,6} s^3 + \\
& 8 \tau_{2,14}^2 \tau_{4,6} s^3 - 8 \tau_{1,14} \tau_{1,15} \tau_{4,6} s^3 + 8 \tau_{1,14} \tau_{1,16} \tau_{4,6} s^3 - 8 \tau_{1,15} \tau_{1,16} \tau_{4,6} s^3 + 16 \tau_{1,14} \tau_{2,14} \tau_{4,6} s^3 - 8 \tau_{1,15} \tau_{2,14} \tau_{4,6} s^3 + \\
& 8 \tau_{1,16} \tau_{2,14} \tau_{4,6} s^3 - 8 \tau_{1,14} \tau_{2,15} \tau_{4,6} s^3 - 8 \tau_{1,16} \tau_{2,15} \tau_{4,6} s^3 - 8 \tau_{2,14} \tau_{2,15} \tau_{4,6} s^3 + 8 \tau_{1,14} \tau_{2,16} \tau_{4,6} s^3 - 8 \tau_{1,15} \tau_{2,16} \tau_{4,6} s^3 + \\
& 8 \tau_{2,14} \tau_{2,16} \tau_{4,6} s^3 - 8 \tau_{2,15} \tau_{2,16} \tau_{4,6} s^3 - 8 \tau_{4,5}^2 \tau_{4,10} s^3 - 8 \tau_{2,8} \tau_{4,5} \tau_{4,10} s^3 - 8 \tau_{2,9} \tau_{4,5} \tau_{4,10} s^3 - 8 \tau_{4,6}^2 \tau_{4,15} s^3 - \\
& 8 \tau_{1,14} \tau_{4,6} \tau_{4,15} s^3 - 8 \tau_{1,16} \tau_{4,6} \tau_{4,15} s^3 - 8 \tau_{2,14} \tau_{4,6} \tau_{4,15} s^3 - 8 \tau_{2,16} \tau_{4,6} \tau_{4,15} s^3 - 9 (s^2 - t^2 + u^2) \tau_{1,10} l_5^2 s^2 - \\
& 14 (s^2 + t^2 - u^2) \tau_{1,15} l_5^2 s^2 - 14 (s^2 - t^2 + u^2) \tau_{1,17} l_5^2 s^2 + 9 (s^2 + t^2 - u^2) \tau_{2,7} l_5^2 s^2 - (s^2 - t^2 + u^2) \tau_{2,7} l_5^2 s^2 + \\
& 9 (s^2 + t^2 - u^2) \tau_{2,8} l_5^2 s^2 - (s^2 - t^2 + u^2) \tau_{2,8} l_5^2 s^2 - 9 (s^2 - t^2 + u^2) \tau_{2,9} l_5^2 s^2 - 9 (s^2 - t^2 + u^2) \tau_{2,10} l_5^2 s^2 + \\
& 5 (s^2 + t^2 - u^2) \tau_{2,13} l_5^2 s^2 + 5 (s^2 - t^2 + u^2) \tau_{2,13} l_5^2 s^2 - 11 (s^2 + t^2 - u^2) \tau_{2,15} l_5^2 s^2 - (s^2 - t^2 + u^2) \tau_{2,15} l_5^2 s^2 - \\
& (s^2 + t^2 - u^2) \tau_{2,17} l_5^2 s^2 - 11 (s^2 - t^2 + u^2) \tau_{2,17} l_5^2 s^2 - 2 (s^2 + t^2 - u^2) \tau_{3,13} l_5^2 s^2 + 6 (s^2 - t^2 + u^2) \tau_{3,13} l_5^2 s^2 - \\
& 9 (s^2 - t^2 + u^2) \tau_{3,17} l_5^2 s^2 + 6 (s^2 + t^2 - u^2) \tau_{4,13} l_5^2 s^2 - 2 (s^2 - t^2 + u^2) \tau_{4,13} l_5^2 s^2 - 9 (s^2 + t^2 - u^2) \tau_{4,15} l_5^2 s^2 - \\
& 8 u (s^2 - t^2 + u^2) \tau_{1,10} l_5^2 s - 8 t (s^2 + t^2 - u^2) \tau_{1,15} l_5^2 s - 8 u (s^2 - t^2 + u^2) \tau_{1,17} l_5^2 s + 8 t (s^2 + t^2 - u^2) \tau_{2,7} l_5^2 s + \\
& 4 t (s^2 + t^2 - u^2) \tau_{2,8} l_5^2 s - 4 u (s^2 - t^2 + u^2) \tau_{2,9} l_5^2 s - 8 u (s^2 - t^2 + u^2) \tau_{2,10} l_5^2 s + 4 t (s^2 + t^2 - u^2) \tau_{2,13} l_5^2 s + \\
& 4 u (s^2 - t^2 + u^2) \tau_{2,13} l_5^2 s - 6 t (s^2 + t^2 - u^2) \tau_{2,15} l_5^2 s - 6 u (s^2 - t^2 + u^2) \tau_{2,17} l_5^2 s + 8 u (s^2 - t^2 + u^2) \tau_{3,13} l_5^2 s - \\
& 4 u (s^2 - t^2 + u^2) \tau_{3,17} l_5^2 s + 8 t (s^2 + t^2 - u^2) \tau_{4,13} l_5^2 s - 4 t (s^2 + t^2 - u^2) \tau_{4,15} l_5^2 s + 4 t^4 \tau_{1,10} l_5^2 + 16 u^4 \tau_{1,10} l_5^2 + \\
& u^2 (-s^2 - t^2 + u^2) \tau_{1,10} l_5^2 + 9 t^2 (s^2 - t^2 + u^2) \tau_{1,10} l_5^2 - 9 u^2 (s^2 - t^2 + u^2) \tau_{1,10} l_5^2 - 4 t^2 (-s^2 + t^2 + u^2) \tau_{1,10} l_5^2 - \\
& u^2 (-s^2 + t^2 + u^2) \tau_{1,10} l_5^2 + 5 t u (-s^2 + t^2 + u^2) \tau_{1,10} l_5^2 + 32 t^4 \tau_{1,15} l_5^2 - 14 t^2 (s^2 + t^2 - u^2) \tau_{1,15} l_5^2 + \\
& 14 u^2 (s^2 + t^2 - u^2) \tau_{1,15} l_5^2 + 8 t u (-s^2 + t^2 + u^2) \tau_{1,15} l_5^2 + 32 u^4 \tau_{1,17} l_5^2 + 14 t^2 (s^2 - t^2 + u^2) \tau_{1,17} l_5^2 - \\
& 14 u^2 (s^2 - t^2 + u^2) \tau_{1,17} l_5^2 + 8 t u (-s^2 + t^2 + u^2) \tau_{1,17} l_5^2 - 16 t^4 \tau_{2,7} l_5^2 + 9 t^2 (s^2 + t^2 - u^2) \tau_{2,7} l_5^2 +
\end{aligned}$$

$$\begin{aligned}
& 9u^2(-s^2-t^2+u^2)\tau_{2,7}l_5^2 - u^2(s^2-t^2+u^2)\tau_{2,7}l_5^2 - t^2(-s^2+t^2+u^2)\tau_{2,7}l_5^2 - 9tu(-s^2+t^2+u^2)\tau_{2,7}l_5^2 - \\
& 8t^4\tau_{2,8}l_5^2 + 9t^2(s^2+t^2-u^2)\tau_{2,8}l_5^2 + 9u^2(-s^2-t^2+u^2)\tau_{2,8}l_5^2 - u^2(s^2-t^2+u^2)\tau_{2,8}l_5^2 - t^2(-s^2+t^2+u^2)\tau_{2,8}l_5^2 - \\
& 5tu(-s^2+t^2+u^2)\tau_{2,9}l_5^2 + 4t^4\tau_{2,9}l_5^2 + 8u^4\tau_{2,9}l_5^2 + u^2(-s^2-t^2+u^2)\tau_{2,9}l_5^2 + 9t^2(s^2-t^2+u^2)\tau_{2,9}l_5^2 - \\
& 9u^2(s^2-t^2+u^2)\tau_{2,9}l_5^2 - 4t^2(-s^2+t^2+u^2)\tau_{2,9}l_5^2 - u^2(-s^2+t^2+u^2)\tau_{2,9}l_5^2 + tu(-s^2+t^2+u^2)\tau_{2,9}l_5^2 + \\
& 4t^4\tau_{2,10}l_5^2 + 16u^4\tau_{2,10}l_5^2 + u^2(-s^2-t^2+u^2)\tau_{2,10}l_5^2 + 9t^2(s^2-t^2+u^2)\tau_{2,10}l_5^2 - 9u^2(s^2-t^2+u^2)\tau_{2,10}l_5^2 - \\
& 4t^2(-s^2+t^2+u^2)\tau_{2,10}l_5^2 - u^2(-s^2+t^2+u^2)\tau_{2,10}l_5^2 + 5tu(-s^2+t^2+u^2)\tau_{2,10}l_5^2 - 8t^4\tau_{2,13}l_5^2 - 8u^4\tau_{2,13}l_5^2 + \\
& 5t^2(-s^2+t^2-u^2)\tau_{2,13}l_5^2 + 5t^2(s^2+t^2-u^2)\tau_{2,13}l_5^2 + 5u^2(-s^2-t^2+u^2)\tau_{2,13}l_5^2 + 5u^2(s^2-t^2+u^2)\tau_{2,13}l_5^2 - \\
& 8tu(-s^2+t^2+u^2)\tau_{2,13}l_5^2 + 20t^4\tau_{2,15}l_5^2 - 11t^2(s^2+t^2-u^2)\tau_{2,15}l_5^2 + 11u^2(s^2+t^2-u^2)\tau_{2,15}l_5^2 - \\
& u^2(s^2-t^2+u^2)\tau_{2,15}l_5^2 - t^2(-s^2+t^2+u^2)\tau_{2,15}l_5^2 + 5tu(-s^2+t^2+u^2)\tau_{2,15}l_5^2 + 20u^4\tau_{2,17}l_5^2 - \\
& t^2(s^2+t^2-u^2)\tau_{2,17}l_5^2 + 11t^2(s^2-t^2+u^2)\tau_{2,17}l_5^2 - 11u^2(s^2-t^2+u^2)\tau_{2,17}l_5^2 - u^2(-s^2+t^2+u^2)\tau_{2,17}l_5^2 + \\
& 5tu(-s^2+t^2+u^2)\tau_{2,17}l_5^2 - 16u^4\tau_{3,13}l_5^2 + 6t^2(-s^2+t^2-u^2)\tau_{3,13}l_5^2 - 2t^2(s^2+t^2-u^2)\tau_{3,13}l_5^2 + \\
& 2u^2(s^2+t^2-u^2)\tau_{3,13}l_5^2 + 6u^2(s^2-t^2+u^2)\tau_{3,13}l_5^2 - 8tu(-s^2+t^2+u^2)\tau_{3,13}l_5^2 + 4t^4\tau_{3,17}l_5^2 + 8u^4\tau_{3,17}l_5^2 + \\
& u^2(-s^2-t^2+u^2)\tau_{3,17}l_5^2 + 9t^2(s^2-t^2+u^2)\tau_{3,17}l_5^2 - 9u^2(s^2-t^2+u^2)\tau_{3,17}l_5^2 - 4t^2(-s^2+t^2+u^2)\tau_{3,17}l_5^2 - \\
& u^2(-s^2+t^2+u^2)\tau_{3,17}l_5^2 + tu(-s^2+t^2+u^2)\tau_{3,17}l_5^2 - 16t^4\tau_{4,13}l_5^2 + 6t^2(s^2+t^2-u^2)\tau_{4,13}l_5^2 + \\
& 6u^2(-s^2-t^2+u^2)\tau_{4,13}l_5^2 + 2t^2(s^2-t^2+u^2)\tau_{4,13}l_5^2 - 2u^2(s^2-t^2+u^2)\tau_{4,13}l_5^2 - 8tu(-s^2+t^2+u^2)\tau_{4,13}l_5^2 + \\
& 8t^4\tau_{4,15}l_5^2 + 4u^4\tau_{4,15}l_5^2 + t^2(-s^2+t^2-u^2)\tau_{4,15}l_5^2 - 9t^2(s^2+t^2-u^2)\tau_{4,15}l_5^2 + 9u^2(s^2+t^2-u^2)\tau_{4,15}l_5^2 - \\
& t^2(-s^2+t^2+u^2)\tau_{4,15}l_5^2 - 4u^2(-s^2+t^2+u^2)\tau_{4,15}l_5^2 + tu(-s^2+t^2+u^2)\tau_{4,15}l_5^2 + 8\tau_{1,9}(su(s^2-t^2-u^2)l_5^2 - \\
& s^3(\tau_{2,7}\tau_{3,5} + (2\tau_{3,5} + \tau_{3,7})\tau_{3,5} - \tau_{2,8}(\tau_{3,5} + \tau_{4,5}) + \tau_{4,5}(\tau_{1,10} - 2\tau_{2,9} + \tau_{2,10} - 3\tau_{4,5} + \tau_{4,10}) + s\tau_{5,9})) + \\
& 8\tau_{1,8}(-(3\tau_{3,5}^2 + \tau_{2,7}\tau_{3,5} - 2\tau_{2,8}\tau_{3,5} + \tau_{3,7}\tau_{3,5} - 2\tau_{4,5}^2 + \tau_{1,10}\tau_{4,5} + \tau_{2,10}\tau_{4,5} - \tau_{1,9}(\tau_{3,5} + \tau_{4,5}) - \\
& \tau_{2,9}(\tau_{3,5} + \tau_{4,5}) + \tau_{4,5}\tau_{4,10} + s\tau_{5,8})s^3 - t(t+u)(-s^2+t^2+u^2)l_5^2) + \\
& 4(2(-\tau_{1,16} + \tau_{1,17} + \tau_{2,10} + \tau_{2,17} + 2\tau_{3,7} + \tau_{3,13} + \tau_{4,10} + \tau_{4,13})t^4 + (-s^2+t^2+u^2) \\
& (3\tau_{1,16} - 3\tau_{1,17} - 6\tau_{2,7} - 4\tau_{2,10} + 2\tau_{2,14} + 3\tau_{2,15} - 3\tau_{2,17} - 5\tau_{3,7} + 2\tau_{3,13} - 3\tau_{4,10} - 2\tau_{4,13})t^2 - \\
& u(-s^2+t^2+u^2)(\tau_{1,16} - \tau_{1,17} + \tau_{2,7} - \tau_{2,10} - 2\tau_{2,14} - \tau_{2,15} + 2\tau_{2,16} - \tau_{2,17} + \tau_{3,7} - 2\tau_{3,13} - \tau_{4,10} - 2\tau_{4,13})t + \\
& (-2t^4 + u^2t^2 + 3u^4 + s^2(3t^2 - 4u^2))\tau_{1,10} + s^2(-4s^2 + t^2 + u^2)\tau_{1,13} + s((3t - 2u)s^2 + t(t - u)(t + 3u))\tau_{1,14} - \\
& 2su(u - t)(3t + u)\tau_{1,15} - u^2(-s^2+t^2+u^2)(5\tau_{1,16} - 3\tau_{1,17} - 4\tau_{2,7} - 6\tau_{2,10} + 3\tau_{2,15} + 2\tau_{2,16} - 3\tau_{2,17} - \\
& 3\tau_{3,7} + 2\tau_{3,13} - 5\tau_{4,10} - 2\tau_{4,13}) + 2u^4(2\tau_{1,16} - \tau_{2,7} + \tau_{2,15} - \tau_{3,7} + \tau_{3,13} - 2\tau_{4,10} + \tau_{4,13}))l_6^2 - \\
& 4\tau_{1,7}(2\tau_{5,8}t^4 + 3l_5^2t^4 - \tau_{3,5}^2t^3 + 6u\tau_{5,8}t^3 + ul_5^2t^3 - 3u\tau_{3,5}^2t^2 - 4s^2\tau_{5,8}t^2 + 8u^2\tau_{5,8}t^2 - 3s^2l_5^2t^2 + 3s^2\tau_{3,5}^2t - \\
& 3u^2\tau_{3,5}^2t + 6u^3\tau_{5,8}t - 6s^2u\tau_{5,8}t + u^3l_5^2t - s^2ul_5^2t - u^3\tau_{3,5}^2 + 3s^2u\tau_{3,5}^2 + 2s^3\tau_{1,8}\tau_{3,5} + 2s^3\tau_{1,9}\tau_{3,5} + \\
& 2s^3\tau_{2,8}\tau_{3,5} + 2s^3\tau_{2,9}\tau_{3,5} + 2u^4\tau_{5,8} - 4s^2u^2\tau_{5,8} - u^4l_5^2 + 3s^2u^2l_5^2 + (3t^4 + u^2t^2 - 2u^4 + s^2(3u^2 - 4t^2))l_6^2)
\end{aligned}$$

■  $N_{45}^{(4)}$

$$\begin{aligned}
& \frac{1}{16} \left( 4 (\tau_{5,8}^2 + \tau_{5,9}^2 + \tau_{6,14}^2 + \tau_{6,16}^2 - 2 (\tau_{8,13} + \tau_{9,13}) l_5^2 + (29 l_5^2 - 2 (\tau_{13,14} + \tau_{13,16})) l_6^2) t^4 + \right. \\
& 8 (2 l_5^2 \tau_{2,8}^2 + \tau_{3,5} \tau_{5,8} \tau_{2,8} + \tau_{4,5} \tau_{5,9} \tau_{2,8} + \tau_{1,7} l_5^2 \tau_{2,8} - 4 \tau_{1,15} l_5^2 \tau_{2,8} + \tau_{2,7} l_5^2 \tau_{2,8} + 2 \tau_{2,13} l_5^2 \tau_{2,8} - \\
& 5 \tau_{2,15} l_5^2 \tau_{2,8} + 3 \tau_{4,13} l_5^2 \tau_{2,8} - 4 \tau_{4,15} l_5^2 \tau_{2,8} - \tau_{3,5}^2 \tau_{5,8} + \tau_{2,9} \tau_{3,5} \tau_{5,8} + \tau_{4,5}^2 \tau_{5,9} + \tau_{2,9} \tau_{4,5} \tau_{5,9} + \\
& \tau_{4,6} (\tau_{1,14} + \tau_{1,16} + \tau_{2,14} + \tau_{2,16} + \tau_{4,6}) \tau_{6,14} + (\tau_{1,14} + \tau_{1,16} + \tau_{2,14} + \tau_{2,16} - \tau_{3,6}) \tau_{3,6} \tau_{6,16} - \tau_{2,10}^2 l_5^2 + \\
& 2 \tau_{2,13}^2 l_5^2 + 2 \tau_{2,15}^2 l_5^2 - \tau_{2,17}^2 l_5^2 - \tau_{4,13}^2 l_5^2 + 2 \tau_{4,15}^2 l_5^2 - (\tau_{1,10} + \tau_{1,17}) (\tau_{1,10} + 2 \tau_{1,17}) l_5^2 - \tau_{1,10} \tau_{2,9} l_5^2 - \\
& 2 \tau_{1,17} \tau_{2,9} l_5^2 - 2 \tau_{1,10} \tau_{2,10} l_5^2 - 3 \tau_{1,17} \tau_{2,10} l_5^2 - \tau_{2,9} \tau_{2,10} l_5^2 - \tau_{1,7} \tau_{2,13} l_5^2 + \tau_{1,10} \tau_{2,13} l_5^2 + \tau_{1,15} \tau_{2,13} l_5^2 + \\
& \tau_{1,17} \tau_{2,13} l_5^2 - \tau_{2,7} \tau_{2,13} l_5^2 + \tau_{2,9} \tau_{2,13} l_5^2 + \tau_{2,10} \tau_{2,13} l_5^2 + 2 \tau_{1,15} \tau_{2,15} l_5^2 - \tau_{2,13} \tau_{2,15} l_5^2 - 2 \tau_{1,10} \tau_{2,17} l_5^2 - \\
& 3 \tau_{1,17} \tau_{2,17} l_5^2 - \tau_{2,9} \tau_{2,17} l_5^2 - 2 \tau_{2,10} \tau_{2,17} l_5^2 + \tau_{2,13} \tau_{2,17} l_5^2 + \tau_{1,10} \tau_{3,13} l_5^2 + 2 \tau_{1,17} \tau_{3,13} l_5^2 + \tau_{2,9} \tau_{3,13} l_5^2 + \\
& \tau_{2,10} \tau_{3,13} l_5^2 - \tau_{2,13} \tau_{3,13} l_5^2 + 2 \tau_{2,17} \tau_{3,13} l_5^2 - 2 \tau_{1,10} \tau_{3,17} l_5^2 - 2 \tau_{1,17} \tau_{3,17} l_5^2 - \tau_{2,10} \tau_{3,17} l_5^2 + \\
& \tau_{2,13} \tau_{3,17} l_5^2 - \tau_{2,17} \tau_{3,17} l_5^2 + \tau_{3,13} \tau_{3,17} l_5^2 - 2 \tau_{1,7} \tau_{4,13} l_5^2 + 2 \tau_{1,15} \tau_{4,13} l_5^2 - 2 \tau_{2,7} \tau_{4,13} l_5^2 + 2 \tau_{2,13} \tau_{4,13} l_5^2 - \\
& 2 \tau_{1,7} \tau_{4,15} l_5^2 + 4 \tau_{1,15} \tau_{4,15} l_5^2 - \tau_{2,7} \tau_{4,15} l_5^2 - 2 \tau_{2,13} \tau_{4,15} l_5^2 + 5 \tau_{2,15} \tau_{4,15} l_5^2 - 3 \tau_{4,13} \tau_{4,15} l_5^2 + \\
& \tau_{1,9} (\tau_{3,5} \tau_{5,8} + \tau_{4,5} \tau_{5,9} + (\tau_{2,17} - \tau_{2,13}) l_5^2) + \tau_{1,8} (\tau_{3,5} \tau_{5,8} + \tau_{4,5} \tau_{5,9} + (2 \tau_{2,8} - \tau_{2,15} - 2 \tau_{4,15}) l_5^2) + \\
& (2 \tau_{1,7}^2 - (\tau_{1,13} + 5 \tau_{1,14} - 2 \tau_{2,7} + \tau_{2,14} - 5 \tau_{3,7}) \tau_{1,7} - \tau_{1,10}^2 + 2 \tau_{1,13}^2 + 2 \tau_{1,14}^2 - \tau_{1,17}^2 - 2 \tau_{2,10}^2 - \tau_{2,17}^2 + \\
& 2 \tau_{3,7}^2 - \tau_{3,13}^2 + \tau_{1,16} \tau_{1,17} + 2 \tau_{1,16} \tau_{2,10} - 3 \tau_{1,17} \tau_{2,10} + \tau_{1,16} \tau_{2,17} - 2 \tau_{1,17} \tau_{2,17} - 3 \tau_{2,10} \tau_{2,17} - \\
& \tau_{1,15} \tau_{3,7} + 4 \tau_{2,7} \tau_{3,7} - 2 \tau_{2,14} \tau_{3,7} - 2 \tau_{2,15} \tau_{3,7} - 2 \tau_{1,15} \tau_{3,13} + 2 \tau_{2,7} \tau_{3,13} - 2 \tau_{2,15} \tau_{3,13} - 3 \tau_{3,7} \tau_{3,13} + \\
& \tau_{1,14} (\tau_{1,15} - 4 \tau_{2,7} + 2 \tau_{2,14} + \tau_{2,15} - 4 \tau_{3,7} + 3 \tau_{3,13}) - \tau_{1,17} \tau_{4,10} - 2 \tau_{2,10} \tau_{4,10} - 2 \tau_{2,17} \tau_{4,10} + \\
& \tau_{1,13} (2 \tau_{1,14} - \tau_{1,15} + \tau_{1,16} - \tau_{1,17} + \tau_{2,7} - \tau_{2,10} - \tau_{2,15} - \tau_{2,16} - \tau_{2,17} - 2 \tau_{3,7} + 2 \tau_{3,13} - \tau_{4,10} - \tau_{4,13}) + \\
& \tau_{1,16} \tau_{4,13} - \tau_{1,17} \tau_{4,13} - 2 \tau_{2,10} \tau_{4,13} - \tau_{2,17} \tau_{4,13} - \tau_{4,10} \tau_{4,13} - \\
& \tau_{1,10} (\tau_{1,13} - \tau_{1,16} + 2 \tau_{1,17} + 3 \tau_{2,10} + \tau_{2,16} + 2 \tau_{2,17} + \tau_{4,10} + 2 \tau_{4,13})) l_6^2) t^3 + \\
& 4 (\tau_{4,5}^4 + 2 (\tau_{1,8} + \tau_{1,9} + \tau_{2,8} + \tau_{2,9}) \tau_{4,5}^3 + (\tau_{1,8} + \tau_{1,9} + \tau_{2,8} + \tau_{2,9})^2 \tau_{4,5}^2 + \tau_{4,6}^4 + \\
& 2 (\tau_{1,14} + \tau_{1,16} + \tau_{2,14} + \tau_{2,16}) \tau_{4,6}^3 + (\tau_{1,8} + \tau_{1,9} + \tau_{2,8} + \tau_{2,9} - \tau_{3,5})^2 \tau_{3,5}^2 + \\
& (\tau_{1,14} + \tau_{1,16} + \tau_{2,14} + \tau_{2,16} - \tau_{3,6})^2 \tau_{3,6}^2 + (\tau_{1,14} + \tau_{1,16} + \tau_{2,14} + \tau_{2,16})^2 \tau_{4,6}^2) t^2 + \\
& (s^2 - t^2 - u^2) (8 (\tau_{5,8}^2 + \tau_{5,9}^2 + \tau_{6,14}^2 + \tau_{6,16}^2 - (2 \tau_{8,13} + \tau_{9,13}) l_5^2) + (219 l_5^2 - 8 (2 \tau_{13,14} + \tau_{13,16})) l_6^2) t^2 + \\
& 4 (s^2 - t^2 - u^2) \\
& (4 l_5^2 \tau_{2,8}^2 + 3 \tau_{3,5} \tau_{5,8} \tau_{2,8} + 3 \tau_{4,5} \tau_{5,9} \tau_{2,8} + 3 \tau_{1,7} l_5^2 \tau_{2,8} - 8 \tau_{1,15} l_5^2 \tau_{2,8} + 3 \tau_{2,7} l_5^2 \tau_{2,8} - 4 \tau_{2,13} l_5^2 \tau_{2,8} - \\
& 7 \tau_{2,15} l_5^2 \tau_{2,8} + 3 \tau_{4,13} l_5^2 \tau_{2,8} - 8 \tau_{4,15} l_5^2 \tau_{2,8} - 3 \tau_{3,5}^2 \tau_{5,8} + 3 \tau_{2,9} \tau_{3,5} \tau_{5,8} + 3 \tau_{4,5}^2 \tau_{5,9} + 3 \tau_{2,9} \tau_{4,5} \tau_{5,9} + \\
& 3 \tau_{4,6} (\tau_{1,14} + \tau_{1,16} + \tau_{2,14} + \tau_{2,16} + \tau_{4,6}) \tau_{6,14} + 3 (\tau_{1,14} + \tau_{1,16} + \tau_{2,14} + \tau_{2,16} - \tau_{3,6}) \tau_{3,6} \tau_{6,16} + \\
& 2 \tau_{2,9}^2 l_5^2 + 6 \tau_{2,13}^2 l_5^2 + 3 \tau_{2,15}^2 l_5^2 - 2 \tau_{2,17}^2 l_5^2 + \tau_{3,13}^2 l_5^2 + 2 \tau_{3,17}^2 l_5^2 + 4 \tau_{4,15}^2 l_5^2 + \\
& ((\tau_{1,7} - 3 \tau_{1,15} + \tau_{2,7}) (\tau_{1,7} - 2 \tau_{1,15} + \tau_{2,7}) - 2 \tau_{1,17} (\tau_{1,10} + \tau_{1,17})) l_5^2 + \tau_{1,10} \tau_{2,9} l_5^2 - 2 \tau_{1,17} \tau_{2,9} l_5^2 - \\
& 2 \tau_{1,17} \tau_{2,10} l_5^2 + \tau_{2,9} \tau_{2,10} l_5^2 - \tau_{1,7} \tau_{2,13} l_5^2 + \tau_{1,10} \tau_{2,13} l_5^2 - \tau_{1,15} \tau_{2,13} l_5^2 + \tau_{1,17} \tau_{2,13} l_5^2 - \tau_{2,7} \tau_{2,13} l_5^2 + 5 \tau_{2,9} \tau_{2,13} l_5^2 + \\
& \tau_{2,10} \tau_{2,13} l_5^2 - 3 \tau_{1,7} \tau_{2,15} l_5^2 + 9 \tau_{1,15} \tau_{2,15} l_5^2 - 3 \tau_{2,7} \tau_{2,15} l_5^2 - \tau_{1,10} \tau_{2,17} l_5^2 - 4 \tau_{1,17} \tau_{2,17} l_5^2 - \tau_{2,9} \tau_{2,17} l_5^2 - \\
& \tau_{2,10} \tau_{2,17} l_5^2 + 2 \tau_{2,13} \tau_{2,17} l_5^2 + \tau_{2,9} \tau_{3,13} l_5^2 + 2 \tau_{2,13} \tau_{3,13} l_5^2 + \tau_{2,17} \tau_{3,13} l_5^2 - 2 \tau_{1,10} \tau_{3,17} l_5^2 - 2 \tau_{1,17} \tau_{3,17} l_5^2 + \\
& 4 \tau_{2,9} \tau_{3,17} l_5^2 + \tau_{2,10} \tau_{3,17} l_5^2 + 5 \tau_{2,13} \tau_{3,17} l_5^2 - \tau_{2,17} \tau_{3,17} l_5^2 + \tau_{3,13} \tau_{3,17} l_5^2 - \tau_{1,7} \tau_{4,13} l_5^2 - 4 \tau_{1,15} \tau_{4,13} l_5^2 -
\end{aligned}$$

$$\begin{aligned}
& \tau_{2,7} \tau_{4,13} l_5^2 + 5 \tau_{2,13} \tau_{4,13} l_5^2 - 3 \tau_{2,15} \tau_{4,13} l_5^2 - 2 \tau_{1,7} \tau_{4,15} l_5^2 + 8 \tau_{1,15} \tau_{4,15} l_5^2 - 3 \tau_{2,7} \tau_{4,15} l_5^2 + 4 \tau_{2,13} \tau_{4,15} l_5^2 + \\
& 7 \tau_{2,15} \tau_{4,15} l_5^2 - 3 \tau_{4,13} \tau_{4,15} l_5^2 + \tau_{1,9} (3 \tau_{3,5} \tau_{5,8} + 3 \tau_{4,5} \tau_{5,9} + (2 \tau_{1,10} + 2 \tau_{2,9} + 2 \tau_{2,10} + \tau_{2,13} + \tau_{2,17} + 2 \tau_{3,17}) l_5^2) + \\
& \tau_{1,8} (3 \tau_{3,5} \tau_{5,8} + 3 \tau_{4,5} \tau_{5,9} + (2 \tau_{1,7} - 4 \tau_{1,15} + 2 \tau_{2,7} + 4 \tau_{2,8} - 4 \tau_{2,13} - 3 \tau_{2,15} - 4 \tau_{4,15}) l_5^2) + \\
& (3 \tau_{1,7}^2 - (7 \tau_{1,14} + 3 \tau_{1,15} - 9 \tau_{2,7} + 3 \tau_{2,14} + 3 \tau_{2,15} - 7 \tau_{3,7} + 3 \tau_{3,13}) \tau_{1,7} - 2 \tau_{1,10}^2 + 6 \tau_{1,13}^2 + \\
& 4 \tau_{1,14}^2 + \tau_{1,15}^2 + 2 \tau_{1,16}^2 + 6 \tau_{2,7}^2 - 2 \tau_{2,10}^2 + \tau_{2,15}^2 + 4 \tau_{3,7}^2 + 2 \tau_{4,10}^2 + \tau_{4,13}^2 - 4 \tau_{2,7} \tau_{2,14} - \\
& 5 \tau_{2,7} \tau_{2,15} + 2 \tau_{2,14} \tau_{2,15} - 2 \tau_{2,10} \tau_{2,17} - 2 \tau_{2,16} \tau_{2,17} + 8 \tau_{2,7} \tau_{3,7} - 4 \tau_{2,14} \tau_{3,7} - 2 \tau_{2,15} \tau_{3,7} - \\
& 4 \tau_{2,7} \tau_{3,13} - \tau_{2,15} \tau_{3,13} - 3 \tau_{3,7} \tau_{3,13} - \tau_{1,15} (5 \tau_{2,7} - 2 \tau_{2,14} - 2 \tau_{2,15} + 3 \tau_{3,7} + \tau_{3,13}) + \\
& \tau_{1,14} (3 \tau_{1,15} - 8 \tau_{2,7} + 4 \tau_{2,14} + 3 \tau_{2,15} - 8 \tau_{3,7} + 3 \tau_{3,13}) - 2 \tau_{2,10} \tau_{4,10} - 2 \tau_{2,16} \tau_{4,10} - 2 \tau_{2,17} \tau_{4,10} + \\
& \tau_{1,17} (\tau_{4,10} - 2 (\tau_{2,10} + \tau_{2,16})) - \tau_{1,13} (4 \tau_{1,14} + \tau_{1,15} - 5 \tau_{1,16} + \tau_{1,17} + \tau_{2,7} + \tau_{2,10} + 4 \tau_{2,14} + \tau_{2,15} - \tau_{2,16} + \\
& \tau_{2,17} - 4 \tau_{3,7} - 5 \tau_{3,13} + 5 \tau_{4,10} - 2 \tau_{4,13}) - \tau_{1,16} (\tau_{1,17} - 2 \tau_{2,10} - 2 \tau_{2,16} + \tau_{2,17} + 4 \tau_{4,10} - \tau_{4,13}) - \\
& \tau_{4,10} \tau_{4,13} - \tau_{1,10} (2 \tau_{1,13} - \tau_{1,16} + \tau_{1,17} + 4 \tau_{2,10} + \tau_{2,16} + \tau_{2,17} + \tau_{4,10} + \tau_{4,13})) l_5^2) t + \\
& 2 u (s^2 - t^2 - u^2) (6 (\tau_{5,8}^2 + \tau_{5,9}^2 + \tau_{6,14}^2 + \tau_{6,16}^2) + 4 (\tau_{9,13} - \tau_{8,13}) l_5^2 + (-4 \tau_{13,14} + 4 \tau_{13,16} + 16 l_5^2) l_6^2) t + \\
& 4 u^2 (\tau_{4,5}^4 + 2 (\tau_{1,8} + \tau_{1,9} + \tau_{2,8} + \tau_{2,9}) \tau_{4,5}^3 + (\tau_{1,8} + \tau_{1,9} + \tau_{2,8} + \tau_{2,9})^2 \tau_{4,5}^2 + \\
& \tau_{4,6}^4 + 2 (\tau_{1,14} + \tau_{1,16} + \tau_{2,14} + \tau_{2,16}) \tau_{4,6}^3 + (\tau_{1,8} + \tau_{1,9} + \tau_{2,8} + \tau_{2,9} - \tau_{3,5})^2 \tau_{3,5}^2 + \\
& (\tau_{1,14} + \tau_{1,16} + \tau_{2,14} + \tau_{2,16} - \tau_{3,6})^2 \tau_{3,6}^2 + (\tau_{1,14} + \tau_{1,16} + \tau_{2,14} + \tau_{2,16})^2 \tau_{4,6}^2) + \\
& 4 (s^2 - t^2 - u^2) (\tau_{4,5}^4 + 2 (\tau_{1,8} + \tau_{1,9} + \tau_{2,8} + \tau_{2,9}) \tau_{4,5}^3 + (\tau_{1,8} + \tau_{1,9} + \tau_{2,8} + \tau_{2,9})^2 \tau_{4,5}^2 + \tau_{4,6}^4 + \\
& 2 (\tau_{1,14} + \tau_{1,16} + \tau_{2,14} + \tau_{2,16}) \tau_{4,6}^3 + (\tau_{1,8} + \tau_{1,9} + \tau_{2,8} + \tau_{2,9} - \tau_{3,5})^2 \tau_{3,5}^2 + \\
& (\tau_{1,14} + \tau_{1,16} + \tau_{2,14} + \tau_{2,16} - \tau_{3,6})^2 \tau_{3,6}^2 + (\tau_{1,14} + \tau_{1,16} + \tau_{2,14} + \tau_{2,16})^2 \tau_{4,6}^2) + \\
& 4 u (s^2 - t^2 - u^2) (2 l_5^2 \tau_{2,8}^2 + 3 \tau_{3,5} \tau_{5,8} \tau_{2,8} + 3 \tau_{4,5} \tau_{5,9} \tau_{2,8} + \tau_{1,7} l_5^2 \tau_{2,8} + 2 \tau_{1,15} l_5^2 \tau_{2,8} + \tau_{2,7} l_5^2 \tau_{2,8} - \\
& 5 \tau_{2,13} l_5^2 \tau_{2,8} + \tau_{2,15} l_5^2 \tau_{2,8} - \tau_{4,13} l_5^2 \tau_{2,8} - 4 \tau_{4,15} l_5^2 \tau_{2,8} - 3 \tau_{3,5}^2 \tau_{5,8} + 3 \tau_{2,9} \tau_{3,5} \tau_{5,8} + 3 \tau_{4,5}^2 \tau_{5,9} + \\
& 3 \tau_{2,9} \tau_{4,5} \tau_{5,9} + 3 \tau_{4,6} (\tau_{1,14} + \tau_{1,16} + \tau_{2,14} + \tau_{2,16} + \tau_{4,6}) \tau_{6,14} + 3 (\tau_{1,14} + \tau_{1,16} + \tau_{2,14} + \tau_{2,16} - \tau_{3,6}) \tau_{3,6} \tau_{6,16} + \\
& 4 \tau_{2,9}^2 l_5^2 + \tau_{2,10}^2 l_5^2 + 6 \tau_{2,13}^2 l_5^2 - 2 \tau_{2,15}^2 l_5^2 + 3 \tau_{2,17}^2 l_5^2 + 4 \tau_{3,17}^2 l_5^2 + \tau_{4,13}^2 l_5^2 + 2 \tau_{4,15}^2 l_5^2 + \\
& ((\tau_{1,10} + 2 \tau_{1,17}) (\tau_{1,10} + 3 \tau_{1,17}) + 2 \tau_{1,15} (\tau_{1,7} - \tau_{1,15} + \tau_{2,7})) l_5^2 + 3 \tau_{1,10} \tau_{2,9} l_5^2 + 8 \tau_{1,17} \tau_{2,9} l_5^2 + \\
& 2 \tau_{1,10} \tau_{2,10} l_5^2 + 5 \tau_{1,17} \tau_{2,10} l_5^2 + 3 \tau_{2,9} \tau_{2,10} l_5^2 - \tau_{1,7} \tau_{2,13} l_5^2 + \tau_{1,10} \tau_{2,13} l_5^2 + \tau_{1,15} \tau_{2,13} l_5^2 - \tau_{1,17} \tau_{2,13} l_5^2 - \\
& \tau_{2,7} \tau_{2,13} l_5^2 + 4 \tau_{2,9} \tau_{2,13} l_5^2 + \tau_{2,10} \tau_{2,13} l_5^2 + \tau_{1,7} \tau_{2,15} l_5^2 - 4 \tau_{1,15} \tau_{2,15} l_5^2 + \tau_{2,7} \tau_{2,15} l_5^2 + 2 \tau_{2,13} \tau_{2,15} l_5^2 + \\
& 3 \tau_{1,10} \tau_{2,17} l_5^2 + 9 \tau_{1,17} \tau_{2,17} l_5^2 + 7 \tau_{2,9} \tau_{2,17} l_5^2 + 3 \tau_{2,10} \tau_{2,17} l_5^2 + \tau_{1,10} \tau_{3,13} l_5^2 - 4 \tau_{1,17} \tau_{3,13} l_5^2 - \\
& 3 \tau_{2,9} \tau_{3,13} l_5^2 + \tau_{2,10} \tau_{3,13} l_5^2 + 5 \tau_{2,13} \tau_{3,13} l_5^2 - 3 \tau_{2,17} \tau_{3,13} l_5^2 + 2 \tau_{1,10} \tau_{3,17} l_5^2 + 8 \tau_{1,17} \tau_{3,17} l_5^2 + \\
& 8 \tau_{2,9} \tau_{3,17} l_5^2 + 3 \tau_{2,10} \tau_{3,17} l_5^2 + 4 \tau_{2,13} \tau_{3,17} l_5^2 + 7 \tau_{2,17} \tau_{3,17} l_5^2 - 3 \tau_{3,13} \tau_{3,17} l_5^2 + 2 \tau_{2,13} \tau_{4,13} l_5^2 + \\
& \tau_{2,15} \tau_{4,13} l_5^2 + 2 \tau_{1,7} \tau_{4,15} l_5^2 - 2 \tau_{1,15} \tau_{4,15} l_5^2 - \tau_{2,7} \tau_{4,15} l_5^2 + 5 \tau_{2,13} \tau_{4,15} l_5^2 - \tau_{2,15} \tau_{4,15} l_5^2 + \tau_{4,13} \tau_{4,15} l_5^2 + \\
& \tau_{1,9} (3 \tau_{3,5} \tau_{5,8} + 3 \tau_{4,5} \tau_{5,9} + (2 \tau_{1,10} + 4 \tau_{1,17} + 4 \tau_{2,9} + 2 \tau_{2,10} + 4 \tau_{2,13} + 3 \tau_{2,17} + 4 \tau_{3,17}) l_5^2) + \\
& \tau_{1,8} (3 \tau_{3,5} \tau_{5,8} + 3 \tau_{4,5} \tau_{5,9} + (2 \tau_{1,7} + 2 \tau_{2,7} + 2 \tau_{2,8} - \tau_{2,13} - \tau_{2,15} - 2 \tau_{4,15}) l_5^2) + \\
& (-2 \tau_{1,7}^2 + (2 \tau_{1,13} + \tau_{1,14} + \tau_{1,15} - 4 \tau_{2,7} - \tau_{2,14} + \tau_{2,15} - \tau_{3,7} + \tau_{3,13}) \tau_{1,7} + 6 \tau_{1,13}^2 + 2 \tau_{1,14}^2 + 4 \tau_{1,16}^2 + \\
& \tau_{1,17}^2 - 2 \tau_{2,7}^2 + 6 \tau_{2,10}^2 + \tau_{2,17}^2 + 2 \tau_{3,7}^2 + \tau_{3,13}^2 + 4 \tau_{4,10}^2 + 2 \tau_{2,7} \tau_{2,15} + 2 \tau_{2,14} \tau_{2,15} - 4 \tau_{2,10} \tau_{2,16} + \\
& 5 \tau_{2,10} \tau_{2,17} - 2 \tau_{2,16} \tau_{2,17} + \tau_{1,15} (2 (\tau_{2,7} + \tau_{2,14}) - \tau_{3,7}) - 2 \tau_{2,7} \tau_{3,7} - 2 \tau_{2,14} \tau_{3,7} + 2 \tau_{2,15} \tau_{3,7} +
\end{aligned}$$

$$\begin{aligned}
& \tau_{1,14} (\tau_{1,15} + 2\tau_{2,7} + 2\tau_{2,14} + \tau_{2,15} - 4\tau_{3,7} - \tau_{3,13}) + \tau_{3,7} \tau_{3,13} + 8\tau_{2,10} \tau_{4,10} - 4\tau_{2,16} \tau_{4,10} + 2\tau_{2,17} \tau_{4,10} - \\
& \tau_{1,13} (5\tau_{1,14} + \tau_{1,15} - 4\tau_{1,16} + \tau_{1,17} - \tau_{2,7} - \tau_{2,10} + \tau_{2,14} + \tau_{2,15} - 4\tau_{2,16} + \tau_{2,17} - 5\tau_{3,7} - 2\tau_{3,13} + \\
& \quad 4\tau_{4,10} - 5\tau_{4,13}) + \tau_{1,17} (5\tau_{2,10} - 2\tau_{2,16} + 2\tau_{2,17} + 3\tau_{4,10} - \tau_{4,13}) + 4\tau_{2,10} \tau_{4,13} - \tau_{2,17} \tau_{4,13} + \\
& \quad 3\tau_{4,10} \tau_{4,13} + \tau_{1,10} (3\tau_{1,10} - 7\tau_{1,16} + 3\tau_{1,17} + 9\tau_{2,10} - 3\tau_{2,16} + 3\tau_{2,17} + 7\tau_{4,10} + 3\tau_{4,13}) - \\
& \quad \tau_{1,16} (3\tau_{1,17} + 8\tau_{2,10} - 4\tau_{2,16} + 3\tau_{2,17} + 8\tau_{4,10} + 3\tau_{4,13})) l_6^2) + \\
& 8u^3 (2l_5^2 \tau_{2,9}^2 + \tau_{3,5} \tau_{5,8} \tau_{2,9} + \tau_{4,5} \tau_{5,9} \tau_{2,9} + \tau_{1,10} l_5^2 \tau_{2,9} + 4\tau_{1,17} l_5^2 \tau_{2,9} + \tau_{2,10} l_5^2 \tau_{2,9} - 2\tau_{2,13} l_5^2 \tau_{2,9} + \\
& \quad 5\tau_{2,17} l_5^2 \tau_{2,9} - 3\tau_{3,13} l_5^2 \tau_{2,9} + 4\tau_{3,17} l_5^2 \tau_{2,9} - \tau_{3,5}^2 \tau_{5,8} + \tau_{2,8} \tau_{3,5} \tau_{5,8} + \tau_{4,5}^2 \tau_{5,9} + \tau_{2,8} \tau_{4,5} \tau_{5,9} + \\
& \quad \tau_{4,6} (\tau_{1,14} + \tau_{1,16} + \tau_{2,14} + \tau_{2,16} + \tau_{4,6}) \tau_{6,14} + (\tau_{1,14} + \tau_{1,16} + \tau_{2,14} + \tau_{2,16} - \tau_{3,6}) \tau_{3,6} \tau_{6,16} + \\
& \quad 2\tau_{2,13}^2 l_5^2 - \tau_{2,15}^2 l_5^2 + 2\tau_{2,17}^2 l_5^2 - \tau_{3,13}^2 l_5^2 + 2\tau_{3,17}^2 l_5^2 - (\tau_{1,7} - 2\tau_{1,15} + \tau_{2,7}) (\tau_{1,7} - \tau_{1,15} + \tau_{2,7}) l_5^2 - \\
& \quad \tau_{1,7} \tau_{2,8} l_5^2 + 2\tau_{1,15} \tau_{2,8} l_5^2 - \tau_{2,7} \tau_{2,8} l_5^2 - \tau_{1,7} \tau_{2,13} l_5^2 + \tau_{1,10} \tau_{2,13} l_5^2 + \tau_{1,15} \tau_{2,13} l_5^2 + \tau_{1,17} \tau_{2,13} l_5^2 - \\
& \quad \tau_{2,7} \tau_{2,13} l_5^2 - \tau_{2,8} \tau_{2,13} l_5^2 + \tau_{2,10} \tau_{2,13} l_5^2 + 2\tau_{1,7} \tau_{2,15} l_5^2 - 3\tau_{1,15} \tau_{2,15} l_5^2 + 2\tau_{2,7} \tau_{2,15} l_5^2 + \tau_{2,8} \tau_{2,15} l_5^2 + \\
& \quad \tau_{2,13} \tau_{2,15} l_5^2 + 2\tau_{1,17} \tau_{2,17} l_5^2 - \tau_{2,13} \tau_{2,17} l_5^2 + 2\tau_{1,10} \tau_{3,13} l_5^2 + 2\tau_{1,17} \tau_{3,13} l_5^2 + 2\tau_{2,10} \tau_{3,13} l_5^2 + \\
& \quad 2\tau_{2,13} \tau_{3,13} l_5^2 + 2\tau_{1,10} \tau_{3,17} l_5^2 + 4\tau_{1,17} \tau_{3,17} l_5^2 + \tau_{2,10} \tau_{3,17} l_5^2 - 2\tau_{2,13} \tau_{3,17} l_5^2 + 5\tau_{2,17} \tau_{3,17} l_5^2 - \\
& \quad 3\tau_{3,13} \tau_{3,17} l_5^2 - \tau_{1,7} \tau_{4,13} l_5^2 + 2\tau_{1,15} \tau_{4,13} l_5^2 - \tau_{2,7} \tau_{4,13} l_5^2 - \tau_{2,8} \tau_{4,13} l_5^2 - \tau_{2,13} \tau_{4,13} l_5^2 + 2\tau_{2,15} \tau_{4,13} l_5^2 + \\
& \quad 2\tau_{1,7} \tau_{4,15} l_5^2 - 2\tau_{1,15} \tau_{4,15} l_5^2 + \tau_{2,7} \tau_{4,15} l_5^2 + \tau_{2,13} \tau_{4,15} l_5^2 - \tau_{2,15} \tau_{4,15} l_5^2 + \tau_{4,13} \tau_{4,15} l_5^2 + \\
& \quad \tau_{1,8} (\tau_{3,5} \tau_{5,8} + \tau_{4,5} \tau_{5,9} + (\tau_{2,13} - \tau_{2,15}) l_5^2) + \tau_{1,9} (\tau_{3,5} \tau_{5,8} + \tau_{4,5} \tau_{5,9} + (2\tau_{2,9} + \tau_{2,17} + 2\tau_{3,17}) l_5^2) - \\
& \quad (\tau_{1,7}^2 - (\tau_{1,13} + \tau_{1,14} + 2\tau_{1,15} - 3\tau_{2,7} - \tau_{2,14} + 2\tau_{2,15} - \tau_{3,7} + 2\tau_{3,13}) \tau_{1,7} - 2\tau_{1,10}^2 - 2\tau_{1,13}^2 + \tau_{1,15}^2 - 2\tau_{1,16}^2 + \\
& \quad 2\tau_{2,7}^2 + \tau_{2,15}^2 - 2\tau_{4,10}^2 + \tau_{4,13}^2 + \tau_{1,16} \tau_{1,17} - 3\tau_{1,15} \tau_{2,7} + 4\tau_{1,16} \tau_{2,10} + 2\tau_{1,15} \tau_{2,15} - 3\tau_{2,7} \tau_{2,15} - \\
& \quad 2\tau_{1,16} \tau_{2,16} + \tau_{1,16} \tau_{2,17} - \tau_{1,15} \tau_{3,7} + 2\tau_{2,7} \tau_{3,7} - 2\tau_{2,15} \tau_{3,7} + \tau_{1,15} \tau_{3,13} - 2\tau_{2,7} \tau_{3,13} + \tau_{2,15} \tau_{3,13} - \tau_{3,7} \tau_{3,13} + \\
& \quad \tau_{1,14} (\tau_{1,15} - 2\tau_{2,7} + \tau_{2,15} + \tau_{3,13}) + \tau_{1,10} (-\tau_{1,13} + 5\tau_{1,16} - 2\tau_{2,10} + \tau_{2,16} - 5\tau_{4,10}) + 4\tau_{1,16} \tau_{4,10} - \tau_{1,17} \tau_{4,10} - \\
& \quad 4\tau_{2,10} \tau_{4,10} + 2\tau_{2,16} \tau_{4,10} - 2\tau_{2,17} \tau_{4,10} + 3\tau_{1,16} \tau_{4,13} + 2\tau_{1,17} \tau_{4,13} + 2\tau_{2,10} \tau_{4,13} + 2\tau_{2,17} \tau_{4,13} - 3\tau_{4,10} \tau_{4,13} + \\
& \quad \tau_{1,13} (\tau_{1,14} + \tau_{1,15} + 2\tau_{1,16} + \tau_{1,17} - \tau_{2,7} + \tau_{2,10} - \tau_{2,14} + \tau_{2,15} + \tau_{2,17} - \tau_{3,7} + \tau_{3,13} - 2(\tau_{4,10} + \tau_{4,13}))) l_6^2) + \\
& 4u^4 (\tau_{5,8}^2 + \tau_{5,9}^2 + \tau_{6,14}^2 + \tau_{6,16}^2 + 2(\tau_{8,13} + \tau_{9,13}) l_5^2 + (2(\tau_{13,14} + \tau_{13,16}) + 29l_5^2) l_6^2) + \\
& u^2 (s^2 - t^2 - u^2) \\
& (8(\tau_{5,8}^2 + \tau_{5,9}^2 + \tau_{6,14}^2 + \tau_{6,16}^2 + (\tau_{8,13} + 2\tau_{9,13}) l_5^2) + (8\tau_{13,14} + 16\tau_{13,16} + 219l_5^2) l_6^2))
\end{aligned}$$

■  $N_{45}^{(5)}$

$$\begin{aligned}
& \frac{1}{16} (-8\tau_{1,7} \tau_{8,13} l_5^2 t^3 + 8\tau_{1,15} \tau_{8,13} l_5^2 t^3 - 8\tau_{2,7} \tau_{8,13} l_5^2 t^3 + 8\tau_{2,13} \tau_{8,13} l_5^2 t^3 + 8\tau_{2,15} \tau_{8,13} l_5^2 t^3 + 8\tau_{1,10} \tau_{9,13} l_5^2 t^3 + \\
& 8\tau_{1,17} \tau_{9,13} l_5^2 t^3 + 8\tau_{2,10} \tau_{9,13} l_5^2 t^3 - 8\tau_{2,13} \tau_{9,13} l_5^2 t^3 + 8\tau_{2,17} \tau_{9,13} l_5^2 t^3 + 16\tau_{1,17}^3 l_5^2 t^2 + 8\tau_{2,13}^3 l_5^2 t^2 - 8\tau_{2,15}^3 l_5^2 t^2 + \\
& 8\tau_{2,17}^3 l_5^2 t^2 + 16\tau_{1,9} \tau_{1,17}^2 l_5^2 t^2 + 32\tau_{1,10} \tau_{1,17}^2 l_5^2 t^2 - 16\tau_{1,15} \tau_{2,8}^2 l_5^2 t^2 + 16\tau_{1,17} \tau_{2,9}^2 l_5^2 t^2 + 16\tau_{1,17} \tau_{2,10}^2 l_5^2 t^2 + \\
& 8\tau_{1,7} \tau_{2,13}^2 l_5^2 t^2 - 8\tau_{1,10} \tau_{2,13}^2 l_5^2 t^2 - 8\tau_{1,15} \tau_{2,13}^2 l_5^2 t^2 - 8\tau_{1,17} \tau_{2,13}^2 l_5^2 t^2 + 8\tau_{2,7} \tau_{2,13}^2 l_5^2 t^2 + 16\tau_{2,8} \tau_{2,13}^2 l_5^2 t^2 - \\
& 8\tau_{2,10} \tau_{2,13}^2 l_5^2 t^2 - 16\tau_{1,15} \tau_{2,15}^2 l_5^2 t^2 + 16\tau_{2,8} \tau_{2,15}^2 l_5^2 t^2 + 12\tau_{2,13} \tau_{2,15}^2 l_5^2 t^2 + 16\tau_{1,10} \tau_{2,17}^2 l_5^2 t^2 + 32\tau_{1,17} \tau_{2,17}^2 l_5^2 t^2 + \\
& 16\tau_{2,9} \tau_{2,17}^2 l_5^2 t^2 + 16\tau_{2,10} \tau_{2,17}^2 l_5^2 t^2 - 4\tau_{2,13} \tau_{2,17}^2 l_5^2 t^2 + 16\tau_{1,9} \tau_{3,13}^2 l_5^2 t^2 + 8\tau_{1,10} \tau_{3,13}^2 l_5^2 t^2 + 8\tau_{1,17} \tau_{3,13}^2 l_5^2 t^2 +
\end{aligned}$$

$$\begin{aligned}
& 16 \tau_{2,9} \tau_{3,13}^2 l_5^2 t^2 + 8 \tau_{2,10} \tau_{3,13}^2 l_5^2 t^2 + 16 \tau_{2,13} \tau_{3,13}^2 l_5^2 t^2 + 8 \tau_{2,17} \tau_{3,13}^2 l_5^2 t^2 + 16 \tau_{1,10} \tau_{3,17}^2 l_5^2 t^2 + 16 \tau_{1,17} \tau_{3,17}^2 l_5^2 t^2 - \\
& 8 \tau_{2,13} \tau_{3,17}^2 l_5^2 t^2 + 8 \tau_{2,17} \tau_{3,17}^2 l_5^2 t^2 - 16 \tau_{3,13} \tau_{3,17}^2 l_5^2 t^2 - 8 \tau_{1,7} \tau_{4,13}^2 l_5^2 t^2 + 8 \tau_{1,15} \tau_{4,13}^2 l_5^2 t^2 - 8 \tau_{2,7} \tau_{4,13}^2 l_5^2 t^2 + \\
& 16 \tau_{2,8} \tau_{4,13}^2 l_5^2 t^2 + 16 \tau_{2,13} \tau_{4,13}^2 l_5^2 t^2 + 16 \tau_{1,7} \tau_{4,15}^2 l_5^2 t^2 - 16 \tau_{1,15} \tau_{4,15}^2 l_5^2 t^2 + 16 \tau_{2,13} \tau_{4,15}^2 l_5^2 t^2 - 8 \tau_{2,15} \tau_{4,15}^2 l_5^2 t^2 + \\
& 16 \tau_{4,13} \tau_{4,15}^2 l_5^2 t^2 + 16 \tau_{1,10}^2 \tau_{1,17} l_5^2 t^2 + 16 \tau_{1,9} \tau_{1,10} \tau_{1,17} l_5^2 t^2 + 16 \tau_{1,15}^2 \tau_{2,8} l_5^2 t^2 + 32 \tau_{1,17}^2 \tau_{2,9} l_5^2 t^2 + \\
& 16 \tau_{1,9} \tau_{1,17} \tau_{2,9} l_5^2 t^2 + 32 \tau_{1,10} \tau_{1,17} \tau_{2,9} l_5^2 t^2 + 32 \tau_{1,17}^2 \tau_{2,10} l_5^2 t^2 + 16 \tau_{1,9} \tau_{1,17} \tau_{2,10} l_5^2 t^2 + 32 \tau_{1,10} \tau_{1,17} \tau_{2,10} l_5^2 t^2 + \\
& 32 \tau_{1,17} \tau_{2,9} \tau_{2,10} l_5^2 t^2 + 8 \tau_{1,9}^2 \tau_{2,13} l_5^2 t^2 - 4 \tau_{1,10}^2 \tau_{2,13} l_5^2 t^2 - 4 \tau_{1,15}^2 \tau_{2,13} l_5^2 t^2 - 4 \tau_{1,17}^2 \tau_{2,13} l_5^2 t^2 - 4 \tau_{2,7}^2 \tau_{2,13} l_5^2 t^2 + \\
& 16 \tau_{2,8}^2 \tau_{2,13} l_5^2 t^2 - 8 \tau_{2,9}^2 \tau_{2,13} l_5^2 t^2 - 4 \tau_{2,10}^2 \tau_{2,13} l_5^2 t^2 + 8 \tau_{1,7} \tau_{1,15} \tau_{2,13} l_5^2 t^2 - 8 \tau_{1,10} \tau_{1,17} \tau_{2,13} l_5^2 t^2 - \\
& 8 \tau_{1,7} \tau_{2,7} \tau_{2,13} l_5^2 t^2 + 8 \tau_{1,15} \tau_{2,7} \tau_{2,13} l_5^2 t^2 - 32 \tau_{1,15} \tau_{2,8} \tau_{2,13} l_5^2 t^2 - 16 \tau_{1,10} \tau_{2,9} \tau_{2,13} l_5^2 t^2 - 16 \tau_{1,17} \tau_{2,9} \tau_{2,13} l_5^2 t^2 - \\
& 8 \tau_{1,10} \tau_{2,10} \tau_{2,13} l_5^2 t^2 - 8 \tau_{1,17} \tau_{2,10} \tau_{2,13} l_5^2 t^2 - 16 \tau_{2,9} \tau_{2,10} \tau_{2,13} l_5^2 t^2 - 8 \tau_{1,15}^2 \tau_{2,15} l_5^2 t^2 - 8 \tau_{2,8}^2 \tau_{2,15} l_5^2 t^2 - \\
& 16 \tau_{2,13}^2 \tau_{2,15} l_5^2 t^2 + 32 \tau_{1,15} \tau_{2,8} \tau_{2,15} l_5^2 t^2 + 8 \tau_{1,7} \tau_{2,13} \tau_{2,15} l_5^2 t^2 + 8 \tau_{1,15} \tau_{2,13} \tau_{2,15} l_5^2 t^2 + 8 \tau_{2,7} \tau_{2,13} \tau_{2,15} l_5^2 t^2 - \\
& 32 \tau_{2,8} \tau_{2,13} \tau_{2,15} l_5^2 t^2 - 8 \tau_{1,9}^2 \tau_{2,17} l_5^2 t^2 + 8 \tau_{1,10}^2 \tau_{2,17} l_5^2 t^2 + 40 \tau_{1,17}^2 \tau_{2,17} l_5^2 t^2 + 8 \tau_{2,9}^2 \tau_{2,17} l_5^2 t^2 + 8 \tau_{2,10}^2 \tau_{2,17} l_5^2 t^2 - \\
& 8 \tau_{2,13}^2 \tau_{2,17} l_5^2 t^2 + 16 \tau_{1,9} \tau_{1,17} \tau_{2,17} l_5^2 t^2 + 48 \tau_{1,10} \tau_{1,17} \tau_{2,17} l_5^2 t^2 + 16 \tau_{1,10} \tau_{2,9} \tau_{2,17} l_5^2 t^2 + 48 \tau_{1,17} \tau_{2,9} \tau_{2,17} l_5^2 t^2 + \\
& 16 \tau_{1,10} \tau_{2,10} \tau_{2,17} l_5^2 t^2 + 48 \tau_{1,17} \tau_{2,10} \tau_{2,17} l_5^2 t^2 + 16 \tau_{2,9} \tau_{2,10} \tau_{2,17} l_5^2 t^2 - 8 \tau_{1,10} \tau_{2,13} \tau_{2,17} l_5^2 t^2 - 8 \tau_{1,17} \tau_{2,13} \tau_{2,17} l_5^2 t^2 - \\
& 16 \tau_{2,9} \tau_{2,13} \tau_{2,17} l_5^2 t^2 - 8 \tau_{2,10} \tau_{2,13} \tau_{2,17} l_5^2 t^2 - 8 \tau_{1,10}^2 \tau_{3,13} l_5^2 t^2 - 24 \tau_{1,17}^2 \tau_{3,13} l_5^2 t^2 - 16 \tau_{2,9}^2 \tau_{3,13} l_5^2 t^2 - \\
& 8 \tau_{2,10}^2 \tau_{3,13} l_5^2 t^2 + 16 \tau_{2,13}^2 \tau_{3,13} l_5^2 t^2 - 24 \tau_{2,17}^2 \tau_{3,13} l_5^2 t^2 - 16 \tau_{1,9} \tau_{1,10} \tau_{3,13} l_5^2 t^2 - 32 \tau_{1,9} \tau_{1,17} \tau_{3,13} l_5^2 t^2 - \\
& 32 \tau_{1,10} \tau_{1,17} \tau_{3,13} l_5^2 t^2 - 16 \tau_{1,9} \tau_{2,9} \tau_{3,13} l_5^2 t^2 - 32 \tau_{1,10} \tau_{2,9} \tau_{3,13} l_5^2 t^2 - 48 \tau_{1,17} \tau_{2,9} \tau_{3,13} l_5^2 t^2 - 16 \tau_{1,9} \tau_{2,10} \tau_{3,13} l_5^2 t^2 - \\
& 16 \tau_{1,10} \tau_{2,10} \tau_{3,13} l_5^2 t^2 - 32 \tau_{1,17} \tau_{2,10} \tau_{3,13} l_5^2 t^2 - 32 \tau_{2,9} \tau_{2,10} \tau_{3,13} l_5^2 t^2 + 16 \tau_{1,9} \tau_{2,13} \tau_{3,13} l_5^2 t^2 - 8 \tau_{1,10} \tau_{2,13} \tau_{3,13} l_5^2 t^2 - \\
& 8 \tau_{1,17} \tau_{2,13} \tau_{3,13} l_5^2 t^2 + 16 \tau_{2,9} \tau_{2,13} \tau_{3,13} l_5^2 t^2 - 8 \tau_{2,10} \tau_{2,13} \tau_{3,13} l_5^2 t^2 - 32 \tau_{1,9} \tau_{2,17} \tau_{3,13} l_5^2 t^2 - 32 \tau_{1,10} \tau_{2,17} \tau_{3,13} l_5^2 t^2 - \\
& 48 \tau_{1,17} \tau_{2,17} \tau_{3,13} l_5^2 t^2 - 48 \tau_{2,9} \tau_{2,17} \tau_{3,13} l_5^2 t^2 - 32 \tau_{2,10} \tau_{2,17} \tau_{3,13} l_5^2 t^2 - 8 \tau_{2,13} \tau_{2,17} \tau_{3,13} l_5^2 t^2 + 16 \tau_{1,10}^2 \tau_{3,17} l_5^2 t^2 + \\
& 32 \tau_{1,17}^2 \tau_{3,17} l_5^2 t^2 + 16 \tau_{2,17}^2 \tau_{3,17} l_5^2 t^2 + 16 \tau_{3,13}^2 \tau_{3,17} l_5^2 t^2 + 16 \tau_{1,9} \tau_{1,10} \tau_{3,17} l_5^2 t^2 + 16 \tau_{1,9} \tau_{1,17} \tau_{3,17} l_5^2 t^2 + \\
& 48 \tau_{1,10} \tau_{1,17} \tau_{3,17} l_5^2 t^2 + 16 \tau_{1,10} \tau_{2,9} \tau_{3,17} l_5^2 t^2 + 32 \tau_{1,17} \tau_{2,9} \tau_{3,17} l_5^2 t^2 + 16 \tau_{1,10} \tau_{2,10} \tau_{3,17} l_5^2 t^2 + 32 \tau_{1,17} \tau_{2,10} \tau_{3,17} l_5^2 t^2 - \\
& 16 \tau_{1,10} \tau_{2,13} \tau_{3,17} l_5^2 t^2 - 16 \tau_{1,17} \tau_{2,13} \tau_{3,17} l_5^2 t^2 - 16 \tau_{2,9} \tau_{2,13} \tau_{3,17} l_5^2 t^2 - 16 \tau_{2,10} \tau_{2,13} \tau_{3,17} l_5^2 t^2 + 32 \tau_{1,10} \tau_{2,17} \tau_{3,17} l_5^2 t^2 + \\
& 48 \tau_{1,17} \tau_{2,17} \tau_{3,17} l_5^2 t^2 + 16 \tau_{2,9} \tau_{2,17} \tau_{3,17} l_5^2 t^2 + 16 \tau_{2,10} \tau_{2,17} \tau_{3,17} l_5^2 t^2 - 16 \tau_{2,13} \tau_{2,17} \tau_{3,17} l_5^2 t^2 - 16 \tau_{1,9} \tau_{3,13} \tau_{3,17} l_5^2 t^2 - \\
& 32 \tau_{1,10} \tau_{3,13} \tau_{3,17} l_5^2 t^2 - 48 \tau_{1,17} \tau_{3,13} \tau_{3,17} l_5^2 t^2 - 32 \tau_{2,9} \tau_{3,13} \tau_{3,17} l_5^2 t^2 - 32 \tau_{2,10} \tau_{3,13} \tau_{3,17} l_5^2 t^2 + 16 \tau_{2,13} \tau_{3,13} \tau_{3,17} l_5^2 t^2 - \\
& 48 \tau_{2,17} \tau_{3,13} \tau_{3,17} l_5^2 t^2 - 8 \tau_{1,7}^2 \tau_{4,13} l_5^2 t^2 - 8 \tau_{1,15}^2 \tau_{4,13} l_5^2 t^2 - 8 \tau_{2,7}^2 \tau_{4,13} l_5^2 t^2 + 16 \tau_{2,8}^2 \tau_{4,13} l_5^2 t^2 + 16 \tau_{2,13}^2 \tau_{4,13} l_5^2 t^2 + \\
& 8 \tau_{2,15}^2 \tau_{4,13} l_5^2 t^2 + 16 \tau_{1,7} \tau_{1,15} \tau_{4,13} l_5^2 t^2 - 16 \tau_{1,7} \tau_{2,7} \tau_{4,13} l_5^2 t^2 + 16 \tau_{1,15} \tau_{2,7} \tau_{4,13} l_5^2 t^2 - 32 \tau_{1,15} \tau_{2,8} \tau_{4,13} l_5^2 t^2 + \\
& 8 \tau_{1,7} \tau_{2,13} \tau_{4,13} l_5^2 t^2 - 8 \tau_{1,15} \tau_{2,13} \tau_{4,13} l_5^2 t^2 + 8 \tau_{2,7} \tau_{2,13} \tau_{4,13} l_5^2 t^2 + 32 \tau_{2,8} \tau_{2,13} \tau_{4,13} l_5^2 t^2 + 16 \tau_{1,7} \tau_{2,15} \tau_{4,13} l_5^2 t^2 + \\
& 16 \tau_{2,7} \tau_{2,15} \tau_{4,13} l_5^2 t^2 - 32 \tau_{2,8} \tau_{2,15} \tau_{4,13} l_5^2 t^2 - 24 \tau_{2,13} \tau_{2,15} \tau_{4,13} l_5^2 t^2 + 16 \tau_{1,8} (\tau_{2,13} + \tau_{4,13}) (\tau_{2,8} - \tau_{4,15}) l_5^2 t^2 - \\
& 16 \tau_{1,15}^2 \tau_{4,15} l_5^2 t^2 - 16 \tau_{2,13}^2 \tau_{4,15} l_5^2 t^2 - 16 \tau_{2,15}^2 \tau_{4,15} l_5^2 t^2 - 16 \tau_{4,13}^2 \tau_{4,15} l_5^2 t^2 - 16 \tau_{1,7} \tau_{1,8} \tau_{4,15} l_5^2 t^2 + \\
& 16 \tau_{1,7} \tau_{1,15} \tau_{4,15} l_5^2 t^2 - 16 \tau_{1,7} \tau_{2,8} \tau_{4,15} l_5^2 t^2 + 32 \tau_{1,15} \tau_{2,8} \tau_{4,15} l_5^2 t^2 - 16 \tau_{1,7} \tau_{2,13} \tau_{4,15} l_5^2 t^2 + 32 \tau_{1,15} \tau_{2,13} \tau_{4,15} l_5^2 t^2 - \\
& 32 \tau_{2,8} \tau_{2,13} \tau_{4,15} l_5^2 t^2 + 16 \tau_{1,7} \tau_{2,15} \tau_{4,15} l_5^2 t^2 - 32 \tau_{1,15} \tau_{2,15} \tau_{4,15} l_5^2 t^2 + 16 \tau_{2,8} \tau_{2,15} \tau_{4,15} l_5^2 t^2 + 32 \tau_{2,13} \tau_{2,15} \tau_{4,15} l_5^2 t^2 - \\
& 16 \tau_{1,7} \tau_{4,13} \tau_{4,15} l_5^2 t^2 + 32 \tau_{1,15} \tau_{4,13} \tau_{4,15} l_5^2 t^2 - 32 \tau_{2,8} \tau_{4,13} \tau_{4,15} l_5^2 t^2 - 32 \tau_{2,13} \tau_{4,13} \tau_{4,15} l_5^2 t^2 + 32 \tau_{2,15} \tau_{4,13} \tau_{4,15} l_5^2 t^2 + \\
& 12 (-s^2 + t^2 + u^2) \tau_{1,7} \tau_{8,13} l_5^2 t + 16 (-s^2 + t^2 + u^2) \tau_{1,8} \tau_{8,13} l_5^2 t - 20 (-s^2 + t^2 + u^2) \tau_{1,15} \tau_{8,13} l_5^2 t +
\end{aligned}$$

$$\begin{aligned}
& 12(-s^2 + t^2 + u^2) \tau_{2,7} \tau_{8,13} l_5^2 t + 16(-s^2 + t^2 + u^2) \tau_{2,8} \tau_{8,13} l_5^2 t - 4(-s^2 + t^2 + u^2) \tau_{2,13} \tau_{8,13} l_5^2 t - \\
& 20(-s^2 + t^2 + u^2) \tau_{2,15} \tau_{8,13} l_5^2 t + 8(-s^2 + t^2 + u^2) \tau_{4,13} \tau_{8,13} l_5^2 t - 16(-s^2 + t^2 + u^2) \tau_{4,15} \tau_{8,13} l_5^2 t + \\
& 16(-s^2 + t^2 + u^2) \tau_{1,9} \tau_{9,13} l_5^2 t + 4(-s^2 + t^2 + u^2) \tau_{1,10} \tau_{9,13} l_5^2 t + 12(-s^2 + t^2 + u^2) \tau_{1,17} \tau_{9,13} l_5^2 t + \\
& 16(-s^2 + t^2 + u^2) \tau_{2,9} \tau_{9,13} l_5^2 t + 4(-s^2 + t^2 + u^2) \tau_{2,10} \tau_{9,13} l_5^2 t + 4(-s^2 + t^2 + u^2) \tau_{2,13} \tau_{9,13} l_5^2 t + \\
& 12(-s^2 + t^2 + u^2) \tau_{2,17} \tau_{9,13} l_5^2 t - 8(-s^2 + t^2 + u^2) \tau_{3,13} \tau_{9,13} l_5^2 t + 16(-s^2 + t^2 + u^2) \tau_{3,17} \tau_{9,13} l_5^2 t + 16u^2 \tau_{1,15}^3 l_5^2 + \\
& 8(-s^2 + t^2 + u^2) \tau_{1,15}^3 l_5^2 + 8(-s^2 + t^2 + u^2) \tau_{1,17}^3 l_5^2 + 8u^2 \tau_{2,13}^3 l_5^2 + 8(s^2 - t^2 - u^2) \tau_{2,13}^3 l_5^2 + 8u^2 \tau_{2,15}^3 l_5^2 - \\
& 8u^2 \tau_{2,17}^3 l_5^2 - 32u^2 \tau_{1,7} \tau_{1,15}^2 l_5^2 + 8(s^2 - t^2 - u^2) \tau_{1,7} \tau_{1,15}^2 l_5^2 + 16(t - u) u \tau_{1,8} \tau_{1,15}^2 l_5^2 + 8(-s^2 + t^2 + u^2) \tau_{1,9} \tau_{1,17}^2 l_5^2 + \\
& 8(-s^2 + t^2 + u^2) \tau_{1,10} \tau_{1,17}^2 l_5^2 + 16u^2 \tau_{1,15} \tau_{2,7}^2 l_5^2 + 16u^2 \tau_{1,15} \tau_{2,8}^2 l_5^2 - 16u^2 \tau_{1,17} \tau_{2,9}^2 l_5^2 + 8u^2 \tau_{1,7} \tau_{2,13}^2 l_5^2 + \\
& 8(s^2 - t^2 - u^2) \tau_{1,7} \tau_{2,13}^2 l_5^2 + 8(s^2 - t^2 - u^2) \tau_{1,9} \tau_{2,13}^2 l_5^2 - 8u^2 \tau_{1,10} \tau_{2,13}^2 l_5^2 + 8(-s^2 + t^2 + u^2) \tau_{1,10} \tau_{2,13}^2 l_5^2 - \\
& 8u^2 \tau_{1,15} \tau_{2,13}^2 l_5^2 + 8(-s^2 + t^2 + u^2) \tau_{1,15} \tau_{2,13}^2 l_5^2 - 8u^2 \tau_{1,17} \tau_{2,13}^2 l_5^2 + 8(-s^2 + t^2 + u^2) \tau_{1,17} \tau_{2,13}^2 l_5^2 + \\
& 8u^2 \tau_{2,7} \tau_{2,13}^2 l_5^2 + 8(s^2 - t^2 - u^2) \tau_{2,7} \tau_{2,13}^2 l_5^2 - 16u^2 \tau_{2,9} \tau_{2,13}^2 l_5^2 - 8u^2 \tau_{2,10} \tau_{2,13}^2 l_5^2 + 8(-s^2 + t^2 + u^2) \tau_{2,10} \tau_{2,13}^2 l_5^2 - \\
& 16u^2 \tau_{1,7} \tau_{2,15}^2 l_5^2 + 32u^2 \tau_{1,15} \tau_{2,15}^2 l_5^2 + 8(-s^2 + t^2 + u^2) \tau_{1,15} \tau_{2,15}^2 l_5^2 - 16u^2 \tau_{2,7} \tau_{2,15}^2 l_5^2 - 16u^2 \tau_{2,8} \tau_{2,15}^2 l_5^2 - \\
& 4u^2 \tau_{2,13} \tau_{2,15}^2 l_5^2 + 4(-s^2 + t^2 + u^2) \tau_{2,13} \tau_{2,15}^2 l_5^2 - 16u^2 \tau_{1,17} \tau_{2,17}^2 l_5^2 + 8(-s^2 + t^2 + u^2) \tau_{1,17} \tau_{2,17}^2 l_5^2 - \\
& 16u^2 \tau_{2,9} \tau_{2,17}^2 l_5^2 + 12u^2 \tau_{2,13} \tau_{2,17}^2 l_5^2 + 4(-s^2 + t^2 + u^2) \tau_{2,13} \tau_{2,17}^2 l_5^2 + 8(s^2 - t^2 - u^2) \tau_{1,9} \tau_{3,13}^2 l_5^2 + 8u^2 \tau_{1,10} \tau_{3,13}^2 l_5^2 + \\
& 8(s^2 - t^2 - u^2) \tau_{1,10} \tau_{3,13}^2 l_5^2 + 8u^2 \tau_{1,17} \tau_{3,13}^2 l_5^2 - 16u^2 \tau_{2,9} \tau_{3,13}^2 l_5^2 + 8u^2 \tau_{2,10} \tau_{3,13}^2 l_5^2 + 8(s^2 - t^2 - u^2) \tau_{2,10} \tau_{3,13}^2 l_5^2 + \\
& 16u^2 \tau_{2,13} \tau_{3,13}^2 l_5^2 + 16(s^2 - t^2 - u^2) \tau_{2,13} \tau_{3,13}^2 l_5^2 - 16u^2 \tau_{1,10} \tau_{3,17}^2 l_5^2 - 16u^2 \tau_{1,17} \tau_{3,17}^2 l_5^2 + \\
& 16u^2 \tau_{2,13} \tau_{3,17}^2 l_5^2 + 8(-s^2 + t^2 + u^2) \tau_{2,13} \tau_{3,17}^2 l_5^2 - 8u^2 \tau_{2,17} \tau_{3,17}^2 l_5^2 + 16u^2 \tau_{3,13} \tau_{3,17}^2 l_5^2 - 8u^2 \tau_{1,7} \tau_{4,13}^2 l_5^2 + \\
& 8(-s^2 + t^2 + u^2) \tau_{1,7} \tau_{4,13}^2 l_5^2 + 8u^2 \tau_{1,15} \tau_{4,13}^2 l_5^2 - 8u^2 \tau_{2,7} \tau_{4,13}^2 l_5^2 + 8(-s^2 + t^2 + u^2) \tau_{2,7} \tau_{4,13}^2 l_5^2 - 16u^2 \tau_{2,8} \tau_{4,13}^2 l_5^2 + \\
& 16u^2 \tau_{2,13} \tau_{4,13}^2 l_5^2 + 16(s^2 - t^2 - u^2) \tau_{2,13} \tau_{4,13}^2 l_5^2 + 8u^2 \tau_{2,15} \tau_{4,13}^2 l_5^2 - 16u^2 \tau_{1,7} \tau_{4,15}^2 l_5^2 + 16u^2 \tau_{1,15} \tau_{4,15}^2 l_5^2 - \\
& 8u^2 \tau_{2,13} \tau_{4,15}^2 l_5^2 + 8(-s^2 + t^2 + u^2) \tau_{2,13} \tau_{4,15}^2 l_5^2 + 8u^2 \tau_{2,15} \tau_{4,15}^2 l_5^2 - 16u^2 \tau_{4,13} \tau_{4,15}^2 l_5^2 + 16u^2 \tau_{1,7}^2 \tau_{1,15} l_5^2 + \\
& 8(-s^2 + t^2 + u^2) \tau_{1,9} \tau_{1,10} \tau_{1,17} l_5^2 - 32u^2 \tau_{1,15}^2 \tau_{2,7} l_5^2 + 8(s^2 - t^2 - u^2) \tau_{1,15}^2 \tau_{2,7} l_5^2 + 32u^2 \tau_{1,7} \tau_{1,15} \tau_{2,7} l_5^2 - \\
& 32u^2 \tau_{1,15}^2 \tau_{2,8} l_5^2 + 8(s^2 - t^2 - u^2) \tau_{1,15}^2 \tau_{2,8} l_5^2 + 32u^2 \tau_{1,7} \tau_{1,15} \tau_{2,8} l_5^2 + 32u^2 \tau_{1,15} \tau_{2,7} \tau_{2,8} l_5^2 - 16u^2 \tau_{1,17}^2 \tau_{2,9} l_5^2 + \\
& 8(-s^2 + t^2 + u^2) \tau_{1,17}^2 \tau_{2,9} l_5^2 - 16u^2 \tau_{1,9} \tau_{1,17} \tau_{2,9} l_5^2 + 8(-s^2 + t^2 + u^2) \tau_{1,17}^2 \tau_{2,10} l_5^2 + 8(-s^2 + t^2 + u^2) \tau_{1,9} \tau_{1,17} \tau_{2,10} l_5^2 - \\
& 4s^2 \tau_{1,7}^2 \tau_{2,13} l_5^2 + 8(-s^2 + t^2 + u^2) \tau_{1,9}^2 \tau_{2,13} l_5^2 - 4u^2 \tau_{1,10}^2 \tau_{2,13} l_5^2 + 4(-s^2 + t^2 + u^2) \tau_{1,10}^2 \tau_{2,13} l_5^2 - \\
& 4u^2 \tau_{1,15}^2 \tau_{2,13} l_5^2 + 4(s^2 - t^2 - u^2) \tau_{1,15}^2 \tau_{2,13} l_5^2 - 4u^2 \tau_{1,17}^2 \tau_{2,13} l_5^2 + 4(s^2 - t^2 - u^2) \tau_{1,17}^2 \tau_{2,13} l_5^2 - 4u^2 \tau_{2,7}^2 \tau_{2,13} l_5^2 + \\
& 4(-s^2 + t^2 + u^2) \tau_{2,7}^2 \tau_{2,13} l_5^2 - 8u^2 \tau_{2,8}^2 \tau_{2,13} l_5^2 + 8(-s^2 + t^2 + u^2) \tau_{2,8}^2 \tau_{2,13} l_5^2 + 16u^2 \tau_{2,9}^2 \tau_{2,13} l_5^2 + \\
& 8(-s^2 + t^2 + u^2) \tau_{2,9}^2 \tau_{2,13} l_5^2 - 4u^2 \tau_{2,10}^2 \tau_{2,13} l_5^2 + 4(-s^2 + t^2 + u^2) \tau_{2,10}^2 \tau_{2,13} l_5^2 + 8(-s^2 + t^2 + u^2) \tau_{1,9} \tau_{1,10} \tau_{2,13} l_5^2 + \\
& 8u^2 \tau_{1,7} \tau_{1,15} \tau_{2,13} l_5^2 + 16(-s^2 + t^2 + u^2) \tau_{1,9} \tau_{1,17} \tau_{2,13} l_5^2 - 8u^2 \tau_{1,10} \tau_{1,17} \tau_{2,13} l_5^2 - 8u^2 \tau_{1,7} \tau_{2,7} \tau_{2,13} l_5^2 + \\
& 8(-s^2 + t^2 + u^2) \tau_{1,7} \tau_{2,7} \tau_{2,13} l_5^2 + 8u^2 \tau_{1,15} \tau_{2,7} \tau_{2,13} l_5^2 - 16u^2 \tau_{1,7} \tau_{2,8} \tau_{2,13} l_5^2 + 16(-s^2 + t^2 + u^2) \tau_{1,7} \tau_{2,8} \tau_{2,13} l_5^2 + \\
& 16u^2 \tau_{1,15} \tau_{2,8} \tau_{2,13} l_5^2 + 8(s^2 - t^2 - u^2) \tau_{1,15} \tau_{2,8} \tau_{2,13} l_5^2 - 16u^2 \tau_{2,7} \tau_{2,8} \tau_{2,13} l_5^2 + 16(-s^2 + t^2 + u^2) \tau_{2,7} \tau_{2,8} \tau_{2,13} l_5^2 + \\
& 16u^2 \tau_{1,9} \tau_{2,9} \tau_{2,13} l_5^2 + 16(-s^2 + t^2 + u^2) \tau_{1,9} \tau_{2,9} \tau_{2,13} l_5^2 + 16(-s^2 + t^2 + u^2) \tau_{1,10} \tau_{2,9} \tau_{2,13} l_5^2 + \\
& 32u^2 \tau_{1,17} \tau_{2,9} \tau_{2,13} l_5^2 + 8(-s^2 + t^2 + u^2) \tau_{1,17} \tau_{2,9} \tau_{2,13} l_5^2 + 8(-s^2 + t^2 + u^2) \tau_{1,9} \tau_{2,10} \tau_{2,13} l_5^2 - 8u^2 \tau_{1,10} \tau_{2,10} \tau_{2,13} l_5^2 + \\
& 8(-s^2 + t^2 + u^2) \tau_{1,10} \tau_{2,10} \tau_{2,13} l_5^2 - 8u^2 \tau_{1,17} \tau_{2,10} \tau_{2,13} l_5^2 + 16(-s^2 + t^2 + u^2) \tau_{2,9} \tau_{2,10} \tau_{2,13} l_5^2 +
\end{aligned}$$

$$\begin{aligned}
& 8u^2 \tau_{1,7}^2 \tau_{2,15} l_5^2 + 40u^2 \tau_{1,15}^2 \tau_{2,15} l_5^2 + 16(-s^2 + t^2 + u^2) \tau_{1,15}^2 \tau_{2,15} l_5^2 + 8u^2 \tau_{2,7}^2 \tau_{2,15} l_5^2 + 8u^2 \tau_{2,8}^2 \tau_{2,15} l_5^2 - \\
& 8u^2 \tau_{2,13}^2 \tau_{2,15} l_5^2 + 8(-s^2 + t^2 + u^2) \tau_{2,13}^2 \tau_{2,15} l_5^2 - 48u^2 \tau_{1,7} \tau_{1,15} \tau_{2,15} l_5^2 + 8(s^2 - t^2 - u^2) \tau_{1,7} \tau_{1,15} \tau_{2,15} l_5^2 + \\
& 16u^2 \tau_{1,7} \tau_{2,7} \tau_{2,15} l_5^2 - 48u^2 \tau_{1,15} \tau_{2,7} \tau_{2,15} l_5^2 + 8(s^2 - t^2 - u^2) \tau_{1,15} \tau_{2,7} \tau_{2,15} l_5^2 + 16u^2 \tau_{1,7} \tau_{2,8} \tau_{2,15} l_5^2 - \\
& 48u^2 \tau_{1,15} \tau_{2,8} \tau_{2,15} l_5^2 + 8(s^2 - t^2 - u^2) \tau_{1,15} \tau_{2,8} \tau_{2,15} l_5^2 + 16u^2 \tau_{2,7} \tau_{2,8} \tau_{2,15} l_5^2 + 8u^2 \tau_{1,7} \tau_{2,13} \tau_{2,15} l_5^2 + \\
& 8(s^2 - t^2 - u^2) \tau_{1,7} \tau_{2,13} \tau_{2,15} l_5^2 - 8u^2 \tau_{1,15} \tau_{2,13} \tau_{2,15} l_5^2 + 8u^2 \tau_{2,7} \tau_{2,13} \tau_{2,15} l_5^2 + 8(s^2 - t^2 - u^2) \tau_{2,7} \tau_{2,13} \tau_{2,15} l_5^2 + \\
& 16u^2 \tau_{2,8} \tau_{2,13} \tau_{2,15} l_5^2 + 16(s^2 - t^2 - u^2) \tau_{2,8} \tau_{2,13} \tau_{2,15} l_5^2 + 8\tau_{1,8}^2 (u(u-2t) \tau_{2,13} + (t^2 - u^2) \tau_{2,15}) l_5^2 + \\
& 8u^2 \tau_{1,9}^2 \tau_{2,17} l_5^2 - 8u^2 \tau_{1,17}^2 \tau_{2,17} l_5^2 + 16(-s^2 + t^2 + u^2) \tau_{1,17}^2 \tau_{2,17} l_5^2 - 8u^2 \tau_{2,9}^2 \tau_{2,17} l_5^2 - 16u^2 \tau_{2,13}^2 \tau_{2,17} l_5^2 + \\
& 8(-s^2 + t^2 + u^2) \tau_{2,13}^2 \tau_{2,17} l_5^2 + 8(-s^2 + t^2 + u^2) \tau_{1,9} \tau_{1,10} \tau_{2,17} l_5^2 + 8(-s^2 + t^2 + u^2) \tau_{1,9} \tau_{1,17} \tau_{2,17} l_5^2 + \\
& 8(-s^2 + t^2 + u^2) \tau_{1,10} \tau_{1,17} \tau_{2,17} l_5^2 - 32u^2 \tau_{1,17} \tau_{2,9} \tau_{2,17} l_5^2 + 8(-s^2 + t^2 + u^2) \tau_{1,17} \tau_{2,9} \tau_{2,17} l_5^2 + \\
& 8(-s^2 + t^2 + u^2) \tau_{1,9} \tau_{2,10} \tau_{2,17} l_5^2 + 8(-s^2 + t^2 + u^2) \tau_{1,17} \tau_{2,10} \tau_{2,17} l_5^2 + 24(-s^2 + t^2 + u^2) \tau_{1,9} \tau_{2,13} \tau_{2,17} l_5^2 - \\
& 8u^2 \tau_{1,10} \tau_{2,13} \tau_{2,17} l_5^2 + 8(-s^2 + t^2 + u^2) \tau_{1,10} \tau_{2,13} \tau_{2,17} l_5^2 + 8u^2 \tau_{1,17} \tau_{2,13} \tau_{2,17} l_5^2 + 32u^2 \tau_{2,9} \tau_{2,13} \tau_{2,17} l_5^2 + \\
& 16(-s^2 + t^2 + u^2) \tau_{2,9} \tau_{2,13} \tau_{2,17} l_5^2 - 8u^2 \tau_{2,10} \tau_{2,13} \tau_{2,17} l_5^2 + 8(-s^2 + t^2 + u^2) \tau_{2,10} \tau_{2,13} \tau_{2,17} l_5^2 - 8u^2 \tau_{1,10}^2 \tau_{3,13} l_5^2 + \\
& 8(-s^2 + t^2 + u^2) \tau_{1,10}^2 \tau_{3,13} l_5^2 - 8u^2 \tau_{1,17}^2 \tau_{3,13} l_5^2 + 8(s^2 - t^2 - u^2) \tau_{1,17}^2 \tau_{3,13} l_5^2 + 16u^2 \tau_{2,9}^2 \tau_{3,13} l_5^2 - \\
& 8u^2 \tau_{2,10}^2 \tau_{3,13} l_5^2 + 8(-s^2 + t^2 + u^2) \tau_{2,10}^2 \tau_{3,13} l_5^2 + 16u^2 \tau_{2,13}^2 \tau_{3,13} l_5^2 + 16(s^2 - t^2 - u^2) \tau_{2,13}^2 \tau_{3,13} l_5^2 + \\
& 8u^2 \tau_{2,17}^2 \tau_{3,13} l_5^2 + 8(-s^2 + t^2 + u^2) \tau_{1,9} \tau_{1,10} \tau_{3,13} l_5^2 - 16u^2 \tau_{1,10} \tau_{1,17} \tau_{3,13} l_5^2 + 8(-s^2 + t^2 + u^2) \tau_{1,10} \tau_{1,17} \tau_{3,13} l_5^2 + \\
& 16u^2 \tau_{1,9} \tau_{2,9} \tau_{3,13} l_5^2 + 16(-s^2 + t^2 + u^2) \tau_{1,10} \tau_{2,9} \tau_{3,13} l_5^2 + 32u^2 \tau_{1,17} \tau_{2,9} \tau_{3,13} l_5^2 + 8(s^2 - t^2 - u^2) \tau_{1,17} \tau_{2,9} \tau_{3,13} l_5^2 + \\
& 8(-s^2 + t^2 + u^2) \tau_{1,9} \tau_{2,10} \tau_{3,13} l_5^2 - 16u^2 \tau_{1,10} \tau_{2,10} \tau_{3,13} l_5^2 + 16(-s^2 + t^2 + u^2) \tau_{1,10} \tau_{2,10} \tau_{3,13} l_5^2 - 16u^2 \tau_{1,17} \tau_{2,10} \tau_{3,13} l_5^2 + \\
& 8(-s^2 + t^2 + u^2) \tau_{1,17} \tau_{2,10} \tau_{3,13} l_5^2 + 16(-s^2 + t^2 + u^2) \tau_{2,9} \tau_{2,10} \tau_{3,13} l_5^2 + 16(s^2 - t^2 - u^2) \tau_{1,9} \tau_{2,13} \tau_{3,13} l_5^2 - \\
& 8u^2 \tau_{1,10} \tau_{2,13} \tau_{3,13} l_5^2 + 8(-s^2 + t^2 + u^2) \tau_{1,10} \tau_{2,13} \tau_{3,13} l_5^2 - 8u^2 \tau_{1,17} \tau_{2,13} \tau_{3,13} l_5^2 + 16(-s^2 + t^2 + u^2) \tau_{1,17} \tau_{2,13} \tau_{3,13} l_5^2 - \\
& 32u^2 \tau_{2,9} \tau_{2,13} \tau_{3,13} l_5^2 - 8u^2 \tau_{2,10} \tau_{2,13} \tau_{3,13} l_5^2 + 8(-s^2 + t^2 + u^2) \tau_{2,10} \tau_{2,13} \tau_{3,13} l_5^2 + 8(-s^2 + t^2 + u^2) \tau_{1,9} \tau_{2,17} \tau_{3,13} l_5^2 - \\
& 16u^2 \tau_{1,10} \tau_{2,17} \tau_{3,13} l_5^2 + 16(-s^2 + t^2 + u^2) \tau_{1,10} \tau_{2,17} \tau_{3,13} l_5^2 + 8(s^2 - t^2 - u^2) \tau_{1,17} \tau_{2,17} \tau_{3,13} l_5^2 + \\
& 32u^2 \tau_{2,9} \tau_{2,17} \tau_{3,13} l_5^2 - 16u^2 \tau_{2,10} \tau_{2,17} \tau_{3,13} l_5^2 + 16(-s^2 + t^2 + u^2) \tau_{2,10} \tau_{2,17} \tau_{3,13} l_5^2 - 24u^2 \tau_{2,13} \tau_{2,17} \tau_{3,13} l_5^2 + \\
& 16(-s^2 + t^2 + u^2) \tau_{2,13} \tau_{2,17} \tau_{3,13} l_5^2 + 8(s^2 - t^2 - u^2) \tau_{1,10}^2 \tau_{3,17} l_5^2 - 16u^2 \tau_{1,17}^2 \tau_{3,17} l_5^2 + 8(-s^2 + t^2 + u^2) \tau_{1,17}^2 \tau_{3,17} l_5^2 - \\
& 16u^2 \tau_{2,13}^2 \tau_{3,17} l_5^2 - 16u^2 \tau_{2,17}^2 \tau_{3,17} l_5^2 - 16u^2 \tau_{3,13}^2 \tau_{3,17} l_5^2 - 16u^2 \tau_{1,9} \tau_{1,10} \tau_{3,17} l_5^2 - 16u^2 \tau_{1,9} \tau_{1,17} \tau_{3,17} l_5^2 - \\
& 16u^2 \tau_{1,10} \tau_{1,17} \tau_{3,17} l_5^2 - 16u^2 \tau_{1,10} \tau_{2,9} \tau_{3,17} l_5^2 - 32u^2 \tau_{1,17} \tau_{2,9} \tau_{3,17} l_5^2 + 8(s^2 - t^2 - u^2) \tau_{1,10} \tau_{2,10} \tau_{3,17} l_5^2 + \\
& 16u^2 \tau_{1,9} \tau_{2,13} \tau_{3,17} l_5^2 + 16(-s^2 + t^2 + u^2) \tau_{1,9} \tau_{2,13} \tau_{3,17} l_5^2 + 16u^2 \tau_{1,10} \tau_{2,13} \tau_{3,17} l_5^2 + 8(-s^2 + t^2 + u^2) \tau_{1,10} \tau_{2,13} \tau_{3,17} l_5^2 + \\
& 32u^2 \tau_{1,17} \tau_{2,13} \tau_{3,17} l_5^2 + 8(-s^2 + t^2 + u^2) \tau_{1,17} \tau_{2,13} \tau_{3,17} l_5^2 + 32u^2 \tau_{2,9} \tau_{2,13} \tau_{3,17} l_5^2 + 16(-s^2 + t^2 + u^2) \tau_{2,9} \tau_{2,13} \tau_{3,17} l_5^2 + \\
& 16(-s^2 + t^2 + u^2) \tau_{2,10} \tau_{2,13} \tau_{3,17} l_5^2 - 16u^2 \tau_{1,10} \tau_{2,17} \tau_{3,17} l_5^2 - 32u^2 \tau_{1,17} \tau_{2,17} \tau_{3,17} l_5^2 + 8(-s^2 + t^2 + u^2) \tau_{1,17} \tau_{2,17} \tau_{3,17} l_5^2 - \\
& 16u^2 \tau_{2,9} \tau_{2,17} \tau_{3,17} l_5^2 + 32u^2 \tau_{2,13} \tau_{2,17} \tau_{3,17} l_5^2 + 16(-s^2 + t^2 + u^2) \tau_{2,13} \tau_{2,17} \tau_{3,17} l_5^2 + 16u^2 \tau_{1,9} \tau_{3,13} \tau_{3,17} l_5^2 + \\
& 16u^2 \tau_{1,10} \tau_{3,13} \tau_{3,17} l_5^2 + 8(-s^2 + t^2 + u^2) \tau_{1,10} \tau_{3,13} \tau_{3,17} l_5^2 + 32u^2 \tau_{1,17} \tau_{3,13} \tau_{3,17} l_5^2 + 8(s^2 - t^2 - u^2) \tau_{1,17} \tau_{3,13} \tau_{3,17} l_5^2 + \\
& 32u^2 \tau_{2,9} \tau_{3,13} \tau_{3,17} l_5^2 + 16(-s^2 + t^2 + u^2) \tau_{2,10} \tau_{3,13} \tau_{3,17} l_5^2 - 32u^2 \tau_{2,13} \tau_{3,13} \tau_{3,17} l_5^2 + 32u^2 \tau_{2,17} \tau_{3,13} \tau_{3,17} l_5^2 - \\
& 8u^2 \tau_{1,7}^2 \tau_{4,13} l_5^2 + 8(-s^2 + t^2 + u^2) \tau_{1,7}^2 \tau_{4,13} l_5^2 - 24u^2 \tau_{1,15}^2 \tau_{4,13} l_5^2 + 8(s^2 - t^2 - u^2) \tau_{1,15}^2 \tau_{4,13} l_5^2 - 8u^2 \tau_{2,7}^2 \tau_{4,13} l_5^2 + \\
& 8(-s^2 + t^2 + u^2) \tau_{2,7}^2 \tau_{4,13} l_5^2 - 16u^2 \tau_{2,8}^2 \tau_{4,13} l_5^2 + 16u^2 \tau_{2,13}^2 \tau_{4,13} l_5^2 + 16(s^2 - t^2 - u^2) \tau_{2,13}^2 \tau_{4,13} l_5^2 -
\end{aligned}$$

$$\begin{aligned}
& 24u^2 \tau_{2,15}^2 \tau_{4,13} l_5^2 + 32u^2 \tau_{1,7} \tau_{1,15} \tau_{4,13} l_5^2 + 8(s^2 - t^2 - u^2) \tau_{1,7} \tau_{1,15} \tau_{4,13} l_5^2 - 16u^2 \tau_{1,7} \tau_{2,7} \tau_{4,13} l_5^2 + \\
& 16(-s^2 + t^2 + u^2) \tau_{1,7} \tau_{2,7} \tau_{4,13} l_5^2 + 32u^2 \tau_{1,15} \tau_{2,7} \tau_{4,13} l_5^2 + 8(s^2 - t^2 - u^2) \tau_{1,15} \tau_{2,7} \tau_{4,13} l_5^2 - 32u^2 \tau_{1,7} \tau_{2,8} \tau_{4,13} l_5^2 + \\
& 16(-s^2 + t^2 + u^2) \tau_{1,7} \tau_{2,8} \tau_{4,13} l_5^2 + 48u^2 \tau_{1,15} \tau_{2,8} \tau_{4,13} l_5^2 + 8(-s^2 + t^2 + u^2) \tau_{1,15} \tau_{2,8} \tau_{4,13} l_5^2 - 32u^2 \tau_{2,7} \tau_{2,8} \tau_{4,13} l_5^2 + \\
& 16(-s^2 + t^2 + u^2) \tau_{2,7} \tau_{2,8} \tau_{4,13} l_5^2 + 8u^2 \tau_{1,7} \tau_{2,13} \tau_{4,13} l_5^2 + 8(s^2 - t^2 - u^2) \tau_{1,7} \tau_{2,13} \tau_{4,13} l_5^2 - 8u^2 \tau_{1,15} \tau_{2,13} \tau_{4,13} l_5^2 + \\
& 16(-s^2 + t^2 + u^2) \tau_{1,15} \tau_{2,13} \tau_{4,13} l_5^2 + 8u^2 \tau_{2,7} \tau_{2,13} \tau_{4,13} l_5^2 + 8(s^2 - t^2 - u^2) \tau_{2,7} \tau_{2,13} \tau_{4,13} l_5^2 - 16u^2 \tau_{2,8} \tau_{2,13} \tau_{4,13} l_5^2 + \\
& 32u^2 \tau_{1,7} \tau_{2,15} \tau_{4,13} l_5^2 + 16(s^2 - t^2 - u^2) \tau_{1,7} \tau_{2,15} \tau_{4,13} l_5^2 - 48u^2 \tau_{1,15} \tau_{2,15} \tau_{4,13} l_5^2 + 8(s^2 - t^2 - u^2) \tau_{1,15} \tau_{2,15} \tau_{4,13} l_5^2 + \\
& 32u^2 \tau_{2,7} \tau_{2,15} \tau_{4,13} l_5^2 + 16(s^2 - t^2 - u^2) \tau_{2,7} \tau_{2,15} \tau_{4,13} l_5^2 + 48u^2 \tau_{2,8} \tau_{2,15} \tau_{4,13} l_5^2 - 8u^2 \tau_{2,13} \tau_{2,15} \tau_{4,13} l_5^2 + \\
& 16(-s^2 + t^2 + u^2) \tau_{2,13} \tau_{2,15} \tau_{4,13} l_5^2 - 8(s^2 - t^2 - u^2) \tau_{1,7} \tau_{1,8} (\tau_{1,15} + \tau_{2,13} + \tau_{2,15} + \tau_{4,13}) l_5^2 - 8(s^2 - t^2 - u^2) \tau_{1,8} \\
& (\tau_{2,13}^2 + 2\tau_{2,8} \tau_{2,13} + (-3\tau_{2,15} + 2\tau_{4,13} - 2\tau_{4,15}) \tau_{2,13} + \tau_{4,13} (\tau_{4,13} - \tau_{2,15}) + \tau_{2,7} (\tau_{2,13} + \tau_{2,15} + \tau_{4,13})) l_5^2 - \\
& 16u^2 \tau_{1,8} \tau_{4,13} (\tau_{2,7} + \tau_{2,8} + \tau_{2,13} - 2\tau_{2,15} + \tau_{4,13} - \tau_{4,15}) l_5^2 + 16u^2 \tau_{1,7}^2 \tau_{4,15} l_5^2 + 8(s^2 - t^2 - u^2) \tau_{1,7}^2 \tau_{4,15} l_5^2 + \\
& 32u^2 \tau_{1,15}^2 \tau_{4,15} l_5^2 + 8(-s^2 + t^2 + u^2) \tau_{1,15}^2 \tau_{4,15} l_5^2 + 16u^2 \tau_{2,15}^2 \tau_{4,15} l_5^2 + 16u^2 \tau_{4,13}^2 \tau_{4,15} l_5^2 - 48u^2 \tau_{1,7} \tau_{1,15} \tau_{4,15} l_5^2 + \\
& 16u^2 \tau_{1,7} \tau_{2,7} \tau_{4,15} l_5^2 + 8(s^2 - t^2 - u^2) \tau_{1,7} \tau_{2,7} \tau_{4,15} l_5^2 - 32u^2 \tau_{1,15} \tau_{2,7} \tau_{4,15} l_5^2 + 16u^2 \tau_{1,7} \tau_{2,8} \tau_{4,15} l_5^2 - \\
& 32u^2 \tau_{1,15} \tau_{2,8} \tau_{4,15} l_5^2 + 16u^2 \tau_{1,7} \tau_{2,13} \tau_{4,15} l_5^2 + 8(s^2 - t^2 - u^2) \tau_{1,7} \tau_{2,13} \tau_{4,15} l_5^2 - 16u^2 \tau_{1,15} \tau_{2,13} \tau_{4,15} l_5^2 + \\
& 8(-s^2 + t^2 + u^2) \tau_{1,15} \tau_{2,13} \tau_{4,15} l_5^2 + 16u^2 \tau_{2,7} \tau_{2,13} \tau_{4,15} l_5^2 + 16(s^2 - t^2 - u^2) \tau_{2,7} \tau_{2,13} \tau_{4,15} l_5^2 + \\
& 16u^2 \tau_{2,8} \tau_{2,13} \tau_{4,15} l_5^2 + 16(s^2 - t^2 - u^2) \tau_{2,8} \tau_{2,13} \tau_{4,15} l_5^2 - 32u^2 \tau_{1,7} \tau_{2,15} \tau_{4,15} l_5^2 + 48u^2 \tau_{1,15} \tau_{2,15} \tau_{4,15} l_5^2 + \\
& 8(-s^2 + t^2 + u^2) \tau_{1,15} \tau_{2,15} \tau_{4,15} l_5^2 - 16u^2 \tau_{2,7} \tau_{2,15} \tau_{4,15} l_5^2 - 16u^2 \tau_{2,8} \tau_{2,15} \tau_{4,15} l_5^2 - 16u^2 \tau_{2,13} \tau_{2,15} \tau_{4,15} l_5^2 + \\
& 16(-s^2 + t^2 + u^2) \tau_{2,13} \tau_{2,15} \tau_{4,15} l_5^2 + 32u^2 \tau_{1,7} \tau_{4,13} \tau_{4,15} l_5^2 + 8(s^2 - t^2 - u^2) \tau_{1,7} \tau_{4,13} \tau_{4,15} l_5^2 - \\
& 48u^2 \tau_{1,15} \tau_{4,13} \tau_{4,15} l_5^2 + 8(s^2 - t^2 - u^2) \tau_{1,15} \tau_{4,13} \tau_{4,15} l_5^2 + 32u^2 \tau_{2,7} \tau_{4,13} \tau_{4,15} l_5^2 + 16(s^2 - t^2 - u^2) \tau_{2,7} \tau_{4,13} \tau_{4,15} l_5^2 + \\
& 32u^2 \tau_{2,8} \tau_{4,13} \tau_{4,15} l_5^2 + 16u^2 \tau_{2,13} \tau_{4,13} \tau_{4,15} l_5^2 - 48u^2 \tau_{2,15} \tau_{4,13} \tau_{4,15} l_5^2 + 16u^2 \tau_{1,7} \tau_{1,8} (\tau_{1,15} - \tau_{4,13} + \tau_{4,15}) l_5^2 + \\
& 16\tau_{1,8} \tau_{1,15} (u(u-t) \tau_{2,7} + (u^2 - t^2) \tau_{2,8} + u(2t \tau_{2,13} + (t-u) \tau_{2,15} + 2u \tau_{4,13}) + (t^2 - u^2) \tau_{4,15}) l_5^2 + \\
& 8u^3 \tau_{1,7} \tau_{8,13} l_5^2 + 4u(-s^2 + t^2 + u^2) \tau_{1,7} \tau_{8,13} l_5^2 + 16u(-s^2 + t^2 + u^2) \tau_{1,8} \tau_{8,13} l_5^2 - 8u^3 \tau_{1,15} \tau_{8,13} l_5^2 - \\
& 12u(-s^2 + t^2 + u^2) \tau_{1,15} \tau_{8,13} l_5^2 + 8u^3 \tau_{2,7} \tau_{8,13} l_5^2 + 4u(-s^2 + t^2 + u^2) \tau_{2,7} \tau_{8,13} l_5^2 + 16u(-s^2 + t^2 + u^2) \tau_{2,8} \tau_{8,13} l_5^2 + \\
& 8u^3 \tau_{2,13} \tau_{8,13} l_5^2 - 4u(-s^2 + t^2 + u^2) \tau_{2,13} \tau_{8,13} l_5^2 - 8u^3 \tau_{2,15} \tau_{8,13} l_5^2 - 12u(-s^2 + t^2 + u^2) \tau_{2,15} \tau_{8,13} l_5^2 + \\
& 8u(-s^2 + t^2 + u^2) \tau_{4,13} \tau_{8,13} l_5^2 - 16u(-s^2 + t^2 + u^2) \tau_{4,15} \tau_{8,13} l_5^2 + 16u(-s^2 + t^2 + u^2) \tau_{1,9} \tau_{9,13} l_5^2 - \\
& 8u^3 \tau_{1,10} \tau_{9,13} l_5^2 + 12u(-s^2 + t^2 + u^2) \tau_{1,10} \tau_{9,13} l_5^2 - 8u^3 \tau_{1,17} \tau_{9,13} l_5^2 + 20u(-s^2 + t^2 + u^2) \tau_{1,17} \tau_{9,13} l_5^2 + \\
& 16u(-s^2 + t^2 + u^2) \tau_{2,9} \tau_{9,13} l_5^2 - 8u^3 \tau_{2,10} \tau_{9,13} l_5^2 + 12u(-s^2 + t^2 + u^2) \tau_{2,10} \tau_{9,13} l_5^2 - 8u^3 \tau_{2,13} \tau_{9,13} l_5^2 + \\
& 4u(-s^2 + t^2 + u^2) \tau_{2,13} \tau_{9,13} l_5^2 - 8u^3 \tau_{2,17} \tau_{9,13} l_5^2 + 20u(-s^2 + t^2 + u^2) \tau_{2,17} \tau_{9,13} l_5^2 - 8u(-s^2 + t^2 + u^2) \tau_{3,13} \tau_{9,13} l_5^2 + \\
& 16u(-s^2 + t^2 + u^2) \tau_{3,17} \tau_{9,13} l_5^2 - ((8(\tau_{1,7} + \tau_{1,13} - \tau_{1,15} + \tau_{2,7} - \tau_{2,15}) \tau_{13,14} - 8(\tau_{1,10} + \tau_{1,13} + \tau_{1,17} + \tau_{2,10} + \tau_{2,17}) \tau_{13,16} + \\
& (52\tau_{1,7} + 28\tau_{1,8} - 44\tau_{1,9} - 38\tau_{1,10} + 27\tau_{1,11} - 27\tau_{1,12} - 27\tau_{1,14} + \tau_{1,15} + 41\tau_{1,16} + 13\tau_{1,17} - \\
& \tau_{2,7} + 27\tau_{2,8} - 41\tau_{2,9} + 13\tau_{2,10} - 27\tau_{2,11} + 27\tau_{2,12} - 28\tau_{2,14} - 52\tau_{2,15} + 44\tau_{2,16} - \\
& 38\tau_{2,17} + 32\tau_{3,7} - 60\tau_{3,10} - 60\tau_{3,15} - 22\tau_{3,17} + 60\tau_{4,7} - 22\tau_{4,10} - 32\tau_{4,15} - 60\tau_{4,17}) l_5^2) \\
& t^3 - 4(2\tau_{1,7}^3 + (-3\tau_{1,13} - 4\tau_{1,14} + 4(\tau_{2,7} + \tau_{3,7}) - 2\tau_{3,13}) \tau_{1,7}^2 + \\
& 2(2\tau_{1,13}^2 + (4\tau_{1,14} - \tau_{1,15} - \tau_{2,7} - \tau_{2,15} - 4\tau_{3,7} + 3\tau_{3,13}) \tau_{1,13} + \tau_{1,14}^2 + \tau_{2,7}^2 - \tau_{2,14}^2 + \tau_{3,7}^2 + 4\tau_{2,7} \tau_{3,7} -
\end{aligned}$$

$$\begin{aligned}
& 2 \tau_{2,15} \tau_{3,7} - 2 \tau_{1,14} (2 \tau_{2,7} + \tau_{3,7} - 2 \tau_{3,13}) - 2 (\tau_{1,15} + \tau_{2,15} + 2 \tau_{3,7}) \tau_{3,13} \tau_{1,7} + 2 \tau_{1,10}^3 - 2 \tau_{1,13}^3 + \\
& \tau_{1,10}^2 (\tau_{1,13} - 4 \tau_{1,16} + 4 (\tau_{1,17} + 2 \tau_{2,10} + \tau_{2,17} + \tau_{4,10}) + 6 \tau_{4,13}) - 2 \tau_{1,13}^2 (2 \tau_{1,14} + \tau_{1,15} + \tau_{1,17} - \tau_{2,7} + \tau_{2,10} + \\
& \tau_{2,15} + \tau_{2,17} + 2 (-\tau_{3,7} + \tau_{3,13} + \tau_{4,13})) + \tau_{1,13} (-4 \tau_{1,14}^2 + (8 \tau_{2,7} - 4 \tau_{2,14} + 8 \tau_{3,7} - 8 \tau_{3,13}) \tau_{1,14} + \\
& \tau_{1,15}^2 + 2 \tau_{1,16}^2 + \tau_{1,17}^2 + \tau_{2,7}^2 + \tau_{2,10}^2 + \tau_{2,15}^2 - 2 \tau_{2,16}^2 + \tau_{2,17}^2 - 4 \tau_{3,7}^2 - 4 \tau_{3,13}^2 + 2 \tau_{4,10}^2 - \\
& 4 \tau_{4,13}^2 + 2 \tau_{2,10} \tau_{2,17} + 4 \tau_{2,14} \tau_{3,7} + \tau_{2,15} (4 \tau_{3,7} - 2 \tau_{3,13}) - 2 \tau_{2,7} (\tau_{2,15} + 4 \tau_{3,7} - \tau_{3,13}) + 8 \tau_{3,7} \tau_{3,13} - \\
& 2 \tau_{1,15} (\tau_{2,7} - \tau_{2,15} + \tau_{3,13}) + 4 \tau_{2,10} \tau_{4,10} + 4 \tau_{2,17} \tau_{4,10} + 2 \tau_{1,17} (\tau_{2,10} + \tau_{2,17} + 2 \tau_{4,10} - \tau_{4,13}) - \\
& 2 (\tau_{2,10} + 2 \tau_{2,16} + \tau_{2,17} - 2 \tau_{4,10}) \tau_{4,13} - 4 \tau_{1,16} (\tau_{1,17} + \tau_{2,10} + \tau_{2,17} + \tau_{4,10} + \tau_{4,13})) + 2 \tau_{1,10} \\
& (-\tau_{1,13}^2 + (-2 \tau_{1,16} + \tau_{1,17} + \tau_{2,10} + \tau_{2,17} + 2 \tau_{4,10} - \tau_{4,13}) \tau_{1,13} + \tau_{1,16}^2 + \tau_{1,17}^2 + 5 \tau_{2,10}^2 - \tau_{2,16}^2 + \tau_{2,17}^2 + \\
& \tau_{4,10}^2 + \tau_{4,13}^2 + 4 \tau_{2,17} \tau_{4,10} - 4 \tau_{2,16} \tau_{4,13} + 4 \tau_{2,17} \tau_{4,13} + 6 \tau_{4,10} \tau_{4,13} + 2 \tau_{1,17} (3 \tau_{2,10} + \tau_{2,17} + \tau_{4,10} + 2 \\
& \tau_{4,13}) - 2 \tau_{1,16} (\tau_{1,17} + 3 \tau_{2,10} + \tau_{2,17} + \tau_{4,10} + 3 \tau_{4,13}) + \tau_{2,10} (6 (\tau_{2,17} + \tau_{4,10} + \tau_{4,13}) - 2 \tau_{2,16})) + \\
& 2 (2 (\tau_{2,10} + \tau_{4,13}) \tau_{1,16}^2 - 2 (2 \tau_{2,10}^2 + (-\tau_{2,16} + 2 (\tau_{2,17} + \tau_{4,10}) + 3 \tau_{4,13}) \tau_{2,10} + 2 \tau_{1,17} \\
& (\tau_{2,10} + \tau_{4,13}) + \tau_{4,13} (-\tau_{2,16} + 2 \tau_{4,10} + \tau_{4,13}) + \tau_{2,17} (\tau_{4,10} + 2 \tau_{4,13})) \tau_{1,16} + \\
& (-2 \tau_{1,14} + \tau_{1,15} - \tau_{2,7} + \tau_{2,15} + 2 \tau_{3,7}) \tau_{3,13}^2 + 2 (\tau_{1,14} - \tau_{2,7} + \tau_{2,14} - \tau_{3,7}) \\
& (\tau_{1,14} \tau_{2,7} + (\tau_{2,15} - \tau_{2,7}) \tau_{3,7}) + (-2 \tau_{1,14}^2 + (4 \tau_{2,7} - 2 \tau_{2,14} + 4 \tau_{3,7}) \tau_{1,14} + (\tau_{1,15} - \tau_{2,7} + \tau_{2,15})^2 - 2 \\
& \tau_{3,7}^2 + 2 (-2 \tau_{2,7} + \tau_{2,14} + \tau_{2,15}) \tau_{3,7}) \tau_{3,13} + \tau_{1,17}^2 (2 \tau_{2,10} + \tau_{4,13}) + (\tau_{2,10} + \tau_{2,17} + \tau_{4,13}) \\
& (2 (\tau_{2,10} + \tau_{4,10}) (\tau_{2,10} - \tau_{2,16} + \tau_{2,17} + \tau_{4,10}) + (\tau_{2,10} - 2 \tau_{2,16} + \tau_{2,17} + 2 \tau_{4,10}) \tau_{4,13}) + \tau_{1,17} (4 \tau_{2,10}^2 + \\
& (4 (\tau_{2,17} + \tau_{4,10} + \tau_{4,13}) - 2 \tau_{2,16}) \tau_{2,10} + 2 \tau_{2,17} (\tau_{4,10} + \tau_{4,13}) + \tau_{4,13} (-2 \tau_{2,16} + 4 \tau_{4,10} + \tau_{4,13}))) \\
& t^2 + (s^2 - t^2 - u^2) (4 ((5 \tau_{1,7} + \tau_{1,13} - 4 \tau_{1,14} - 3 \tau_{1,15} + 5 \tau_{2,7} - 4 \tau_{2,14} - 3 \tau_{2,15} + 4 \tau_{3,7} - 2 \tau_{3,13}) \tau_{13,14} + \\
& (3 \tau_{1,10} - \tau_{1,13} - 4 \tau_{1,16} + \tau_{1,17} + 3 \tau_{2,10} - 4 \tau_{2,16} + \tau_{2,17} + 4 \tau_{4,10} + 2 \tau_{4,13}) \tau_{13,16}) + \\
& (79 \tau_{1,7} + 41 \tau_{1,8} - 52 \tau_{1,9} - 71 \tau_{1,10} + 43 \tau_{1,11} - 43 \tau_{1,12} - 38 \tau_{1,14} + 2 \tau_{1,15} + 46 \tau_{1,16} + 11 \tau_{1,17} - \\
& 2 \tau_{2,7} + 38 \tau_{2,8} - 46 \tau_{2,9} + 11 \tau_{2,10} - 43 \tau_{2,11} + 43 \tau_{2,12} - 41 \tau_{2,14} - 79 \tau_{2,15} + 52 \tau_{2,16} - \\
& 71 \tau_{2,17} + 38 \tau_{3,7} - 84 \tau_{3,10} - 85 \tau_{3,15} - 36 \tau_{3,17} + 85 \tau_{4,7} - 36 \tau_{4,10} - 38 \tau_{4,15} - 84 \tau_{4,17}) l_5^2) t + \\
& 4 u^2 (2 \tau_{1,7}^3 - (\tau_{1,13} + 4 (\tau_{1,14} + \tau_{1,15} - 2 \tau_{2,7} + \tau_{2,15} - \tau_{3,7}) + 6 \tau_{3,13}) \tau_{1,7}^2 - \\
& 2 (\tau_{1,13}^2 + (-2 \tau_{1,14} - \tau_{1,15} + \tau_{2,7} - \tau_{2,15} + 2 \tau_{3,7} + \tau_{3,13}) \tau_{1,13} - \tau_{1,14}^2 - \tau_{1,15}^2 - 5 \tau_{2,7}^2 + \tau_{2,14}^2 - \tau_{2,15}^2 - \\
& \tau_{3,7}^2 - \tau_{3,13}^2 + 4 \tau_{2,15} \tau_{3,7} + 2 \tau_{1,15} (3 \tau_{2,7} - \tau_{2,15} + \tau_{3,7} - 2 \tau_{3,13}) - 4 \tau_{2,14} \tau_{3,13} - 4 \tau_{2,15} \tau_{3,13} + \\
& 6 \tau_{3,7} \tau_{3,13} - 2 \tau_{1,14} (\tau_{1,15} - 3 \tau_{2,7} + \tau_{2,15} - \tau_{3,7} + 3 \tau_{3,13}) + 2 \tau_{2,7} (\tau_{2,14} + 3 (\tau_{2,15} - \tau_{3,7} + \tau_{3,13}))) \tau_{1,7} + \\
& 2 \tau_{1,10}^3 + 2 \tau_{1,13}^3 + \tau_{1,10}^2 (3 \tau_{1,13} - 4 \tau_{1,16} + 4 (\tau_{2,10} + \tau_{4,10}) + 2 \tau_{4,13}) + 2 (-2 \tau_{1,14} + \tau_{1,15} - \tau_{2,7} + 2 \tau_{2,14} + \\
& \tau_{2,15} - 2 \tau_{3,7}) \tau_{3,13}^2 - (2 \tau_{1,14}^2 + 2 (2 \tau_{1,15} - 3 \tau_{2,7} + \tau_{2,14} + 2 \tau_{2,15} - 2 \tau_{3,7}) \tau_{1,14} + \tau_{1,15}^2 + 3 \\
& \tau_{2,7}^2 + \tau_{2,15}^2 + 2 \tau_{3,7}^2 + 2 \tau_{1,15} (-2 \tau_{2,7} + \tau_{2,14} + \tau_{2,15} - 2 \tau_{3,7}) + 2 \tau_{2,14} (\tau_{2,15} - \tau_{3,7}) - 4 \tau_{2,15} \\
& \tau_{3,7} + \tau_{2,7} (6 \tau_{3,7} - 4 (\tau_{2,14} + \tau_{2,15}))) \tau_{3,13} - (2 \tau_{1,16} + \tau_{1,17} + \tau_{2,10} + \tau_{2,17} - 2 \tau_{4,10}) \tau_{4,13}^2 + \\
& 2 (\tau_{1,14} + \tau_{1,15} - \tau_{2,7} + \tau_{2,14} + \tau_{2,15} - \tau_{3,7}) (\tau_{1,14} \tau_{2,7} + \tau_{1,15} \tau_{2,7} - (\tau_{2,7} - \tau_{2,15}) (\tau_{2,7} + \tau_{3,7})) + \\
& 2 (\tau_{1,16} - \tau_{2,10} + \tau_{2,16} - \tau_{4,10}) (\tau_{1,16} \tau_{2,10} - (\tau_{2,10} + \tau_{2,17}) \tau_{4,10}) + (2 \tau_{1,16}^2 + 2 (-2 \tau_{2,10} + \tau_{2,16} - 2 \tau_{4,10}) \\
& \tau_{1,16} - (\tau_{1,17} + \tau_{2,10} + \tau_{2,17})^2 + 2 \tau_{4,10}^2 + 2 (2 \tau_{2,10} - \tau_{2,16} + \tau_{2,17}) \tau_{4,10}) \tau_{4,13}) + \\
& 2 \tau_{1,13}^2 (\tau_{1,15} - 2 \tau_{1,16} + \tau_{1,17} - \tau_{2,7} + \tau_{2,10} + \tau_{2,15} + \tau_{2,17} + 2 (\tau_{3,13} + \tau_{4,10} + \tau_{4,13})) +
\end{aligned}$$

$$\begin{aligned}
& 2 \tau_{1,10} (2 \tau_{1,13}^2 - (4 \tau_{1,16} + \tau_{1,17} - \tau_{2,10} + \tau_{2,17} - 4 \tau_{4,10} - 3 \tau_{4,13}) \tau_{1,13} + \tau_{1,16}^2 + \tau_{2,10}^2 - \tau_{2,16}^2 + \tau_{4,10}^2 + \\
& \quad 4 \tau_{2,10} \tau_{4,10} + 2 \tau_{2,17} \tau_{4,10} - 2 (\tau_{1,17} + \tau_{2,17} - 2 \tau_{4,10}) \tau_{4,13} - 2 \tau_{1,16} (2 \tau_{2,10} + \tau_{4,10} + 2 \tau_{4,13})) - \\
& \tau_{1,13} (2 \tau_{1,14}^2 + 4 (\tau_{1,15} - \tau_{2,7} + \tau_{2,15} - \tau_{3,7} + \tau_{3,13}) \tau_{1,14} + \tau_{1,15}^2 - 4 \tau_{1,16}^2 + \tau_{1,17}^2 + \tau_{2,7}^2 + \\
& \quad \tau_{2,10}^2 - 2 \tau_{2,14}^2 + \tau_{2,15}^2 + \tau_{2,17}^2 + 2 \tau_{3,7}^2 - 4 \tau_{3,13}^2 - 4 \tau_{4,10}^2 - 4 \tau_{4,13}^2 - 2 \tau_{2,7} \tau_{2,15} + 4 \tau_{2,7} \tau_{3,7} - \\
& \quad 4 \tau_{2,15} \tau_{3,7} + 2 (\tau_{2,7} + 2 \tau_{2,14} - \tau_{2,15} - 2 \tau_{3,7}) \tau_{3,13} - 2 \tau_{1,15} (\tau_{2,7} - \tau_{2,15} + 2 \tau_{3,7} + \tau_{3,13}) + \\
& \quad 4 \tau_{2,16} \tau_{4,10} + 2 \tau_{1,17} (\tau_{2,10} + \tau_{2,17} - \tau_{4,13}) + 2 \tau_{2,10} (\tau_{2,17} - 4 \tau_{4,10} - \tau_{4,13}) - \\
& \quad 8 \tau_{4,10} \tau_{4,13} - 2 \tau_{2,17} (2 \tau_{4,10} + \tau_{4,13}) + 4 \tau_{1,16} (2 \tau_{2,10} - \tau_{2,16} + 2 (\tau_{4,10} + \tau_{4,13}))) - \\
& 4 (s^2 - t^2 - u^2) (-2 \tau_{1,13}^3 - 2 (\tau_{1,15} + \tau_{1,17} - \tau_{2,7} + \tau_{2,10} - \tau_{2,14} + \tau_{2,15} + \tau_{2,16} + \tau_{2,17} + 2 (\tau_{3,13} + \tau_{4,13})) \tau_{1,13}^2 + \\
& \quad (2 \tau_{1,14}^2 + 2 (2 \tau_{1,15} - \tau_{2,7} + 2 (\tau_{2,14} + \tau_{2,15} - \tau_{3,7})) \tau_{1,14} + \tau_{1,15}^2 + 2 \tau_{1,16}^2 + \tau_{1,17}^2 - \tau_{2,7}^2 - \tau_{2,10}^2 + \\
& \quad 2 \tau_{2,14}^2 + \tau_{2,15}^2 + 2 \tau_{2,16}^2 + \tau_{2,17}^2 + 2 \tau_{3,7}^2 - 4 \tau_{3,13}^2 + 2 \tau_{4,10}^2 - 4 \tau_{4,13}^2 - 2 \tau_{2,15} \tau_{3,7} + \\
& \quad 2 \tau_{1,15} (\tau_{2,14} + \tau_{2,15} - 2 \tau_{3,7} - \tau_{3,13}) - 2 \tau_{2,15} \tau_{3,13} + 2 \tau_{2,14} (\tau_{2,15} - 2 \tau_{3,7} + 2 \tau_{3,13}) + \\
& \quad 2 \tau_{2,7} (-2 \tau_{2,14} + \tau_{3,7} + 2 \tau_{3,13}) + 2 \tau_{2,17} \tau_{4,10} - 2 \tau_{1,16} (2 \tau_{1,17} + \tau_{2,10} + 2 (-\tau_{2,16} + \tau_{2,17} + \tau_{4,10})) + \\
& \quad 2 \tau_{2,10} (-2 \tau_{2,16} + \tau_{4,10} - 2 \tau_{4,13}) - 2 \tau_{2,17} \tau_{4,13} - 2 \tau_{1,17} (\tau_{2,16} - \tau_{2,17} - 2 \tau_{4,10} + \tau_{4,13}) - \\
& \quad 2 \tau_{2,16} (\tau_{2,17} + 2 (\tau_{4,10} + \tau_{4,13}))) \tau_{1,13} + \tau_{1,7}^2 (\tau_{1,13} + 2 \tau_{2,7}) + \tau_{1,10}^2 (\tau_{1,13} - 2 \tau_{2,10}) + \\
& \quad 2 \tau_{1,7} (\tau_{1,13}^2 - (2 \tau_{1,14} + \tau_{1,15} + 3 \tau_{2,14} + \tau_{2,15} - 2 (\tau_{3,7} + \tau_{3,13})) \tau_{1,13} + 2 \tau_{2,7}^2 - \tau_{1,14} \tau_{2,7} + \\
& \quad \tau_{2,14} \tau_{2,15} + \tau_{1,15} (-\tau_{2,7} + \tau_{2,14} - 2 \tau_{3,13}) - \tau_{2,14} \tau_{3,13} - 2 \tau_{2,15} \tau_{3,13} - \tau_{2,7} (\tau_{2,14} + \tau_{2,15} - \tau_{3,7} + \tau_{3,13})) - \\
& \quad 2 \tau_{1,10} (\tau_{1,13}^2 + (2 \tau_{1,16} - \tau_{1,17} + 3 \tau_{2,16} - \tau_{2,17} - 2 \tau_{4,10} + 2 \tau_{4,13}) \tau_{1,13} + 2 \tau_{2,10}^2 - \tau_{1,16} \tau_{2,10} - \tau_{2,16} \tau_{2,17} + \\
& \quad \tau_{1,17} (\tau_{2,10} - \tau_{2,16} - 2 \tau_{4,13}) + \tau_{2,16} \tau_{4,13} - 2 \tau_{2,17} \tau_{4,13} + \tau_{2,10} (-\tau_{2,16} + \tau_{2,17} + \tau_{4,10} + \tau_{4,13})) + \\
& \quad 2 (\tau_{3,13} \tau_{1,15}^2 + (-\tau_{2,7}^2 + (\tau_{2,14} - \tau_{3,13}) \tau_{2,7} - \tau_{2,15} \tau_{3,7} + \tau_{3,13} (\tau_{2,14} + 2 \tau_{2,15} - 2 \tau_{3,7} + \tau_{3,13})) \tau_{1,15} + \\
& \quad (\tau_{2,7} - \tau_{2,15} - \tau_{3,13}) (\tau_{2,7}^2 + (\tau_{3,7} - \tau_{2,14}) \tau_{2,7} + \tau_{2,15} \tau_{3,7} - (\tau_{2,14} + \tau_{2,15}) \tau_{3,13}) + \tau_{1,14} \\
& \quad ((2 \tau_{1,15} + \tau_{2,7} + 2 \tau_{2,15}) \tau_{3,13} - \tau_{2,7}^2) + \tau_{1,17}^2 \tau_{4,13} + \tau_{1,16} (\tau_{2,10}^2 + (-2 \tau_{1,17} + \tau_{2,10} - 2 \tau_{2,17}) \tau_{4,13}) - \\
& \quad (\tau_{2,10} + \tau_{2,17} + \tau_{4,13}) (\tau_{2,10}^2 + (\tau_{4,10} - \tau_{2,16}) \tau_{2,10} + \tau_{2,16} \tau_{4,13} - \tau_{2,17} (\tau_{4,10} + \tau_{4,13})) + \\
& \quad \tau_{1,17} (-\tau_{2,10}^2 + (\tau_{2,16} + \tau_{4,13}) \tau_{2,10} + \tau_{2,17} \tau_{4,10} + \tau_{4,13} (-\tau_{2,16} + 2 (\tau_{2,17} + \tau_{4,10}) + \tau_{4,13})))) + \\
& u (s^2 - t^2 - u^2) (4 ((3 \tau_{1,7} + \tau_{1,13} - 4 \tau_{1,14} - \tau_{1,15} + 3 \tau_{2,7} - 4 \tau_{2,14} - \tau_{2,15} + 4 \tau_{3,7} - 2 \tau_{3,13}) \tau_{13,14} + \\
& \quad (5 \tau_{1,10} - \tau_{1,13} - 4 \tau_{1,16} + 3 \tau_{1,17} + 5 \tau_{2,10} - 4 \tau_{2,16} + 3 \tau_{2,17} + 4 \tau_{4,10} + 2 \tau_{4,13}) \tau_{13,16}) + \\
& \quad (71 \tau_{1,7} + 52 \tau_{1,8} - 41 \tau_{1,9} - 79 \tau_{1,10} + 43 \tau_{1,11} - 43 \tau_{1,12} - 46 \tau_{1,14} + 11 \tau_{1,15} + 38 \tau_{1,16} + \\
& \quad 2 \tau_{1,17} - 11 \tau_{2,7} + 46 \tau_{2,8} - 38 \tau_{2,9} + 2 \tau_{2,10} - 43 \tau_{2,11} + 43 \tau_{2,12} - 52 \tau_{2,14} - 71 \tau_{2,15} + 41 \tau_{2,16} - \\
& \quad 79 \tau_{2,17} + 36 \tau_{3,7} - 85 \tau_{3,10} - 84 \tau_{3,15} - 38 \tau_{3,17} + 84 \tau_{4,7} - 38 \tau_{4,10} - 36 \tau_{4,15} - 85 \tau_{4,17}) l_5^2) + \\
& u^3 (8 (-\tau_{1,7} + \tau_{1,13} + \tau_{1,15} - \tau_{2,7} + \tau_{2,15}) \tau_{13,14} + 8 (\tau_{1,10} - \tau_{1,13} + \tau_{1,17} + \tau_{2,10} + \tau_{2,17}) \tau_{13,16} + \\
& \quad (38 \tau_{1,7} + 44 \tau_{1,8} - 28 \tau_{1,9} - 52 \tau_{1,10} + 27 \tau_{1,11} - 27 \tau_{1,12} - 41 \tau_{1,14} + 13 \tau_{1,15} + 27 \tau_{1,16} + \tau_{1,17} - \\
& \quad 13 \tau_{2,7} + 41 \tau_{2,8} - 27 \tau_{2,9} + \tau_{2,10} - 27 \tau_{2,11} + 27 \tau_{2,12} - 44 \tau_{2,14} - 38 \tau_{2,15} + 28 \tau_{2,16} - \\
& \quad 52 \tau_{2,17} + 22 \tau_{3,7} - 60 \tau_{3,10} - 60 \tau_{3,15} - 32 \tau_{3,17} + 60 \tau_{4,7} - 32 \tau_{4,10} - 22 \tau_{4,15} - 60 \tau_{4,17}) l_5^2) l_6^2)
\end{aligned}$$

■  $N_{45}^{(6)}$

$$\begin{aligned}
& \frac{1}{16} (20 \tau_{7,8} l_5^2 l_6^2 t^3 + 20 \tau_{9,10} l_5^2 l_6^2 t^3 + 20 \tau_{14,15} l_5^2 l_6^2 t^3 - 20 \tau_{16,17} l_5^2 l_6^2 t^3 + 16 l_5^2 l_6^2 l_{13}^2 t^3 - 36 l_5^2 l_8^2 l_{14}^2 t^3 - 36 l_6^2 l_8^2 l_{14}^2 t^3 + \\
& (40 \tau_{1,7}^2 + 2 (12 \tau_{1,8} - 24 \tau_{1,9} - 13 \tau_{1,10} + 22 \tau_{1,11} + 4 \tau_{1,12} + 6 \tau_{2,7} - 4 \tau_{2,8} - 19 \tau_{2,9} + 6 \tau_{2,10} + 4 \tau_{2,11} + 15 \tau_{2,12} - \\
& \quad 2 (8 \tau_{3,7} + 7 \tau_{3,10} - 15 \tau_{4,7} + 6 \tau_{4,10})) \tau_{1,7} + 6 \tau_{1,8}^2 + 40 \tau_{1,9}^2 + 28 \tau_{1,10}^2 + 61 \tau_{1,11}^2 + 27 \tau_{1,12}^2 + \\
& \quad 21 \tau_{1,14}^2 + 21 \tau_{1,15}^2 + 21 \tau_{1,16}^2 + 27 \tau_{1,17}^2 + 21 \tau_{2,7}^2 + 21 \tau_{2,8}^2 + 21 \tau_{2,9}^2 + 27 \tau_{2,10}^2 + 61 \tau_{2,11}^2 + \\
& \quad 27 \tau_{2,12}^2 + 6 \tau_{2,14}^2 + 40 \tau_{2,15}^2 + 40 \tau_{2,16}^2 + 28 \tau_{2,17}^2 + 56 \tau_{3,7}^2 + 46 \tau_{3,10}^2 + 56 \tau_{3,15}^2 + 46 \tau_{3,17}^2 + 56 \tau_{4,7}^2 + \\
& \quad 46 \tau_{4,10}^2 + 56 \tau_{4,15}^2 + 46 \tau_{4,17}^2 - 42 \tau_{1,11} \tau_{1,14} + 6 \tau_{1,11} \tau_{1,15} + 24 \tau_{1,12} \tau_{1,15} - 2 \tau_{1,14} \tau_{1,15} - 42 \tau_{1,12} \tau_{1,16} - \\
& \quad 28 \tau_{1,15} \tau_{1,16} - 6 \tau_{1,11} \tau_{1,17} - 18 \tau_{1,12} \tau_{1,17} + 10 \tau_{1,14} \tau_{1,17} + 2 \tau_{1,15} \tau_{1,17} + 10 \tau_{1,16} \tau_{1,17} - 10 \tau_{1,11} \tau_{2,7} + \\
& \quad 12 \tau_{1,12} \tau_{2,7} - 42 \tau_{1,11} \tau_{2,8} - 2 \tau_{2,7} \tau_{2,8} - 12 \tau_{1,12} \tau_{2,9} - 28 \tau_{2,7} \tau_{2,9} + 2 \tau_{1,11} \tau_{2,10} - 20 \tau_{1,12} \tau_{2,10} - 2 \tau_{2,7} \tau_{2,10} - \\
& \quad 10 \tau_{2,8} \tau_{2,10} - 10 \tau_{2,9} \tau_{2,10} + 68 \tau_{1,11} \tau_{2,11} - 42 \tau_{1,14} \tau_{2,11} - 10 \tau_{1,15} \tau_{2,11} - 2 \tau_{1,17} \tau_{2,11} + 6 \tau_{2,7} \tau_{2,11} - \\
& \quad 42 \tau_{2,8} \tau_{2,11} + 6 \tau_{2,10} \tau_{2,11} + 16 \tau_{1,12} \tau_{2,12} + 12 \tau_{1,15} \tau_{2,12} - 12 \tau_{1,16} \tau_{2,12} + 20 \tau_{1,17} \tau_{2,12} + 24 \tau_{2,7} \tau_{2,12} - \\
& \quad 42 \tau_{2,9} \tau_{2,12} + 18 \tau_{2,10} \tau_{2,12} - 12 \tau_{1,11} \tau_{2,14} + 8 \tau_{1,14} \tau_{2,14} + 4 \tau_{1,15} \tau_{2,14} + 16 \tau_{1,17} \tau_{2,14} + 4 \tau_{2,11} \tau_{2,14} + \\
& \quad 8 \tau_{1,11} \tau_{2,15} + 30 \tau_{1,12} \tau_{2,15} - 8 \tau_{1,14} \tau_{2,15} + 12 \tau_{1,15} \tau_{2,15} - 38 \tau_{1,16} \tau_{2,15} - 12 \tau_{1,17} \tau_{2,15} + 44 \tau_{2,11} \tau_{2,15} + \\
& \quad 8 \tau_{2,12} \tau_{2,15} + 24 \tau_{2,14} \tau_{2,15} - 42 \tau_{1,12} \tau_{2,16} - 40 \tau_{1,15} \tau_{2,16} + 34 \tau_{1,16} \tau_{2,16} + 40 \tau_{1,17} \tau_{2,16} + 4 \tau_{2,12} \tau_{2,16} - \\
& \quad 48 \tau_{2,15} \tau_{2,16} - 22 \tau_{1,11} \tau_{2,17} + 26 \tau_{1,14} \tau_{2,17} - 14 \tau_{1,15} \tau_{2,17} - 4 \tau_{1,16} \tau_{2,17} + 4 \tau_{1,17} \tau_{2,17} + 2 \tau_{2,11} \tau_{2,17} - \\
& \quad 4 \tau_{2,12} \tau_{2,17} + 36 \tau_{2,14} \tau_{2,17} + 26 \tau_{2,15} \tau_{2,17} - 10 \tau_{2,16} \tau_{2,17} - 84 \tau_{1,11} \tau_{3,7} - 4 \tau_{2,7} \tau_{3,7} + 64 \tau_{2,8} \tau_{3,7} - \\
& \quad 24 \tau_{2,10} \tau_{3,7} - 64 \tau_{2,11} \tau_{3,7} + 4 \tau_{1,11} \tau_{3,10} + 14 \tau_{2,7} \tau_{3,10} - 34 \tau_{2,8} \tau_{3,10} + 30 \tau_{2,10} \tau_{3,10} + 38 \tau_{2,11} \tau_{3,10} - \\
& \quad 56 \tau_{3,7} \tau_{3,10} - 4 \tau_{1,8} (9 \tau_{1,10} - \tau_{1,11} - \tau_{2,7} - 2 \tau_{2,8} + 4 \tau_{2,10} + 3 \tau_{2,11} - 7 \tau_{3,7} + 11 \tau_{3,10}) + 64 \tau_{1,12} \tau_{3,15} + \\
& \quad 52 \tau_{1,15} \tau_{3,15} - 64 \tau_{1,16} \tau_{3,15} - 32 \tau_{1,17} \tau_{3,15} + 28 \tau_{2,12} \tau_{3,15} + 60 \tau_{2,15} \tau_{3,15} - 84 \tau_{2,16} \tau_{3,15} - 4 \tau_{2,17} \tau_{3,15} + \\
& \quad 34 \tau_{1,12} \tau_{3,17} + 32 \tau_{1,15} \tau_{3,17} - 38 \tau_{1,16} \tau_{3,17} + 28 \tau_{1,17} \tau_{3,17} + 44 \tau_{2,12} \tau_{3,17} + 24 \tau_{2,15} \tau_{3,17} - 4 \tau_{2,16} \tau_{3,17} - \\
& \quad 14 \tau_{2,17} \tau_{3,17} + 56 \tau_{3,15} \tau_{3,17} + 28 \tau_{1,12} \tau_{4,7} + 52 \tau_{2,7} \tau_{4,7} - 64 \tau_{2,9} \tau_{4,7} + 32 \tau_{2,10} \tau_{4,7} + 64 \tau_{2,12} \tau_{4,7} + \\
& \quad 2 \tau_{1,10} (-\tau_{1,11} + 2 \tau_{1,12} + 7 \tau_{2,7} - 13 \tau_{2,8} + 2 \tau_{2,9} + 2 \tau_{2,10} + 11 \tau_{2,11} - 16 \tau_{3,7} + 31 \tau_{3,10} + 2 \tau_{4,7} - 7 \tau_{4,10}) - \\
& \quad 44 \tau_{1,12} \tau_{4,10} - 32 \tau_{2,7} \tau_{4,10} + 38 \tau_{2,9} \tau_{4,10} + 28 \tau_{2,10} \tau_{4,10} - 34 \tau_{2,12} \tau_{4,10} - 56 \tau_{4,7} \tau_{4,10} + \\
& \quad 2 \tau_{1,9} (5 \tau_{1,10} + 2 \tau_{1,12} - 20 \tau_{2,7} + 17 \tau_{2,9} - 20 \tau_{2,10} - 21 (\tau_{2,12} + 2 \tau_{4,7}) + 2 \tau_{4,10}) - 64 \tau_{1,11} \tau_{4,15} + \\
& \quad 64 \tau_{1,14} \tau_{4,15} - 4 \tau_{1,15} \tau_{4,15} + 24 \tau_{1,17} \tau_{4,15} - 84 \tau_{2,11} \tau_{4,15} + 28 \tau_{2,14} \tau_{4,15} - 32 \tau_{2,15} \tau_{4,15} + 32 \tau_{2,17} \tau_{4,15} + \\
& \quad 2 (-19 \tau_{1,11} + 17 \tau_{1,14} - 7 \tau_{1,15} + 15 \tau_{1,17} - 2 \tau_{2,11} + 22 \tau_{2,14} + 14 \tau_{2,15} + 31 \tau_{2,17} + 28 \tau_{4,15}) \tau_{4,17} l_5^2 l_6^2 t^2 - \\
& 24 (-s^2 + t^2 + u^2) \tau_{7,8} l_5^2 l_6^2 t - 24 (-s^2 + t^2 + u^2) \tau_{9,10} l_5^2 l_6^2 t - 24 (-s^2 + t^2 + u^2) \tau_{14,15} l_5^2 l_6^2 t + \\
& 24 (-s^2 + t^2 + u^2) \tau_{16,17} l_5^2 l_6^2 t + \\
& 48 (-s^2 + t^2 + u^2) l_5^2 l_6^2 l_{13}^2 t - \\
& 10 (-s^2 + t^2 + u^2) l_5^2 l_8^2 l_{14}^2 t - \\
& 10 (-s^2 + t^2 + u^2) l_6^2 l_8^2 l_{14}^2 t + \\
& (s^2 - t^2 - u^2) (24 \tau_{1,7}^2 + (36 \tau_{1,8} - 41 \tau_{1,9} - 24 \tau_{1,10} + 5 \tau_{1,11} + 4 \tau_{1,12} - 5 \tau_{2,7} + 14 \tau_{2,8} - 30 \tau_{2,9} + 6 \tau_{2,10} - 10 \tau_{2,11} + \\
& \quad 26 \tau_{2,12} - 17 \tau_{3,7} - 20 \tau_{3,10} + 61 \tau_{4,7} - 28 \tau_{4,10}) \tau_{1,7} + 10 \tau_{1,8}^2 + 10 \tau_{1,9}^2 + 24 \tau_{1,10}^2 + 22 \tau_{1,11}^2 + 22 \tau_{1,12}^2 + \\
& \quad 12 \tau_{1,14}^2 + 13 \tau_{1,15}^2 + 12 \tau_{1,16}^2 + 13 \tau_{1,17}^2 + 13 \tau_{2,7}^2 + 12 \tau_{2,8}^2 + 12 \tau_{2,9}^2 + 13 \tau_{2,10}^2 + 22 \tau_{2,11}^2 + \\
& \quad 22 \tau_{2,12}^2 + 10 \tau_{2,14}^2 + 24 \tau_{2,15}^2 + 10 \tau_{2,16}^2 + 24 \tau_{2,17}^2 + 50 \tau_{3,7}^2 + 50 \tau_{3,10}^2 + 50 \tau_{3,15}^2 + 50 \tau_{3,17}^2 + 50 \tau_{4,7}^2 + \\
& \quad 50 \tau_{4,10}^2 + 50 \tau_{4,15}^2 + 50 \tau_{4,17}^2 - 24 \tau_{1,11} \tau_{1,14} - 4 \tau_{1,11} \tau_{1,15} + 13 \tau_{1,12} \tau_{1,15} + 8 \tau_{1,14} \tau_{1,15} - 24 \tau_{1,12} \tau_{1,16} -
\end{aligned}$$

$$\begin{aligned}
& 13 \tau_{1,15} \tau_{1,16} - 13 \tau_{1,11} \tau_{1,17} + 4 \tau_{1,12} \tau_{1,17} + 13 \tau_{1,14} \tau_{1,17} + 6 \tau_{1,15} \tau_{1,17} - 8 \tau_{1,16} \tau_{1,17} - 32 \tau_{1,11} \tau_{2,7} + 4 \tau_{1,12} \tau_{2,7} - \\
& 5 \tau_{1,11} \tau_{2,8} + 8 \tau_{2,7} \tau_{2,8} - 5 \tau_{1,12} \tau_{2,9} - 13 \tau_{2,7} \tau_{2,9} + 4 \tau_{1,11} \tau_{2,10} - 32 \tau_{1,12} \tau_{2,10} - 6 \tau_{2,7} \tau_{2,10} - 13 \tau_{2,8} \tau_{2,10} + \\
& 8 \tau_{2,9} \tau_{2,10} + 2 \tau_{1,11} \tau_{2,11} - 5 \tau_{1,14} \tau_{2,11} - 32 \tau_{1,15} \tau_{2,11} - 4 \tau_{1,17} \tau_{2,11} - 4 \tau_{2,7} \tau_{2,11} - 24 \tau_{2,8} \tau_{2,11} + 13 \tau_{2,10} \tau_{2,11} + \\
& 2 \tau_{1,12} \tau_{2,12} + 4 \tau_{1,15} \tau_{2,12} - 5 \tau_{1,16} \tau_{2,12} + 32 \tau_{1,17} \tau_{2,12} + 13 \tau_{2,7} \tau_{2,12} - 24 \tau_{2,9} \tau_{2,12} - 4 \tau_{2,10} \tau_{2,12} - 5 \tau_{1,11} \tau_{2,14} + \\
& \tau_{1,14} \tau_{2,14} - \tau_{1,15} \tau_{2,14} + 23 \tau_{1,17} \tau_{2,14} + 32 \tau_{2,11} \tau_{2,14} - 10 \tau_{1,11} \tau_{2,15} + 26 \tau_{1,12} \tau_{2,15} + 14 \tau_{1,14} \tau_{2,15} - 5 \tau_{1,15} \tau_{2,15} - \\
& 30 \tau_{1,16} \tau_{2,15} - 6 \tau_{1,17} \tau_{2,15} + 5 \tau_{2,11} \tau_{2,15} + 4 \tau_{2,12} \tau_{2,15} + 36 \tau_{2,14} \tau_{2,15} - 5 \tau_{1,12} \tau_{2,16} - 23 \tau_{1,15} \tau_{2,16} + \tau_{1,16} \tau_{2,16} + \\
& \tau_{1,17} \tau_{2,16} + 32 \tau_{2,12} \tau_{2,16} - 41 \tau_{2,15} \tau_{2,16} - 26 \tau_{1,11} \tau_{2,17} + 10 \tau_{1,12} \tau_{2,17} + 30 \tau_{1,14} \tau_{2,17} - 6 \tau_{1,15} \tau_{2,17} - 14 \tau_{1,16} \tau_{2,17} - \\
& 5 \tau_{1,17} \tau_{2,17} - 4 \tau_{2,11} \tau_{2,17} - 5 \tau_{2,12} \tau_{2,17} + 41 \tau_{2,14} \tau_{2,17} + 24 \tau_{2,15} \tau_{2,17} - 36 \tau_{2,16} \tau_{2,17} - 56 \tau_{1,11} \tau_{3,7} + 20 \tau_{2,7} \tau_{3,7} + \\
& 45 \tau_{2,8} \tau_{3,7} - 28 \tau_{2,10} \tau_{3,7} - 41 \tau_{2,11} \tau_{3,7} + 8 \tau_{1,11} \tau_{3,10} + 17 \tau_{2,7} \tau_{3,10} - 41 \tau_{2,8} \tau_{3,10} + 39 \tau_{2,10} \tau_{3,10} + 45 \tau_{2,11} \tau_{3,10} - \\
& 56 \tau_{3,7} \tau_{3,10} - \tau_{1,8} (41 \tau_{1,10} - 32 \tau_{1,11} + \tau_{2,7} - \tau_{2,8} + 23 \tau_{2,10} + 5 \tau_{2,11} - 8 \tau_{3,7} + 56 \tau_{3,10}) + 45 \tau_{1,12} \tau_{3,15} + \\
& 39 \tau_{1,15} \tau_{3,15} - 41 \tau_{1,16} \tau_{3,15} - 17 \tau_{1,17} \tau_{3,15} + 8 \tau_{2,12} \tau_{3,15} + 61 \tau_{2,15} \tau_{3,15} - 56 \tau_{2,16} \tau_{3,15} + 20 \tau_{2,17} \tau_{3,15} + \\
& 41 \tau_{1,12} \tau_{3,17} + 28 \tau_{1,15} \tau_{3,17} - 45 \tau_{1,16} \tau_{3,17} + 20 \tau_{1,17} \tau_{3,17} + 56 \tau_{2,12} \tau_{3,17} + 28 \tau_{2,15} \tau_{3,17} - 8 \tau_{2,16} \tau_{3,17} - \\
& 17 \tau_{2,17} \tau_{3,17} + 56 \tau_{3,15} \tau_{3,17} + 8 \tau_{1,12} \tau_{4,7} + 39 \tau_{2,7} \tau_{4,7} - 41 \tau_{2,9} \tau_{4,7} + 17 \tau_{2,10} \tau_{4,7} + 45 \tau_{2,12} \tau_{4,7} + \tau_{1,10} \\
& (4 \tau_{1,11} + 5 \tau_{1,12} + 6 \tau_{2,7} - 30 \tau_{2,8} + 14 \tau_{2,9} - 5 \tau_{2,10} + 26 \tau_{2,11} - 10 \tau_{2,12} - 28 \tau_{3,7} + 61 \tau_{3,10} - 20 \tau_{4,7} - 17 \tau_{4,10}) - \\
& 56 \tau_{1,12} \tau_{4,10} - 28 \tau_{2,7} \tau_{4,10} + 45 \tau_{2,9} \tau_{4,10} + 20 \tau_{2,10} \tau_{4,10} - 41 \tau_{2,12} \tau_{4,10} - 56 \tau_{4,7} \tau_{4,10} + \\
& \tau_{1,9} (36 \tau_{1,10} + 32 \tau_{1,12} - 23 \tau_{2,7} + \tau_{2,9} - \tau_{2,10} - 5 \tau_{2,12} - 56 \tau_{4,7} + 8 \tau_{4,10}) - 41 \tau_{1,11} \tau_{4,15} + \\
& 45 \tau_{1,14} \tau_{4,15} + 20 \tau_{1,15} \tau_{4,15} + 28 \tau_{1,17} \tau_{4,15} - 56 \tau_{2,11} \tau_{4,15} + 8 \tau_{2,14} \tau_{4,15} - 17 \tau_{2,15} \tau_{4,15} + 28 \tau_{2,17} \tau_{4,15} + \\
& (-45 \tau_{1,11} + 41 \tau_{1,14} - 17 \tau_{1,15} + 39 \tau_{1,17} - 8 \tau_{2,11} + 56 \tau_{2,14} + 20 \tau_{2,15} + 61 \tau_{2,17} + 56 \tau_{4,15}) l_5^2 l_6^2 + \\
& u^2 (28 \tau_{1,7}^2 + 2 (5 \tau_{1,8} - 18 \tau_{1,9} - 13 \tau_{1,10} + 2 \tau_{1,11} - \tau_{1,12} + 2 \tau_{2,7} + 2 \tau_{2,8} - 13 \tau_{2,9} + 7 \tau_{2,10} + 11 \tau_{2,12} - 7 \tau_{3,7} + \\
& 2 \tau_{3,10} + 31 \tau_{4,7} - 16 \tau_{4,10}) \tau_{1,7} + 40 \tau_{1,8}^2 + 6 \tau_{1,9}^2 + 40 \tau_{1,10}^2 + 27 \tau_{1,11}^2 + 61 \tau_{1,12}^2 + 21 \tau_{1,14}^2 + \\
& 27 \tau_{1,15}^2 + 21 \tau_{1,16}^2 + 21 \tau_{1,17}^2 + 27 \tau_{2,7}^2 + 21 \tau_{2,8}^2 + 21 \tau_{2,9}^2 + 21 \tau_{2,10}^2 + 27 \tau_{2,11}^2 + 61 \tau_{2,12}^2 + \\
& 40 \tau_{2,14}^2 + 28 \tau_{2,15}^2 + 6 \tau_{2,16}^2 + 40 \tau_{2,17}^2 + 46 \tau_{3,7}^2 + 56 \tau_{3,10}^2 + 46 \tau_{3,15}^2 + 56 \tau_{3,17}^2 + 46 \tau_{4,7}^2 + 56 \tau_{4,10}^2 + \\
& 46 \tau_{4,15}^2 + 56 \tau_{4,17}^2 - 42 \tau_{1,11} \tau_{1,14} + 18 \tau_{1,11} \tau_{1,15} + 6 \tau_{1,12} \tau_{1,15} - 10 \tau_{1,14} \tau_{1,15} - 42 \tau_{1,12} \tau_{1,16} - 10 \tau_{1,15} \tau_{1,16} - \\
& 24 \tau_{1,11} \tau_{1,17} - 6 \tau_{1,12} \tau_{1,17} + 28 \tau_{1,14} \tau_{1,17} + 2 \tau_{1,15} \tau_{1,17} + 2 \tau_{1,16} \tau_{1,17} - 20 \tau_{1,11} \tau_{2,7} + 2 \tau_{1,12} \tau_{2,7} - 12 \tau_{1,11} \tau_{2,8} - \\
& 10 \tau_{2,7} \tau_{2,8} - 42 \tau_{1,12} \tau_{2,9} - 10 \tau_{2,7} \tau_{2,9} + 12 \tau_{1,11} \tau_{2,10} - 10 \tau_{1,12} \tau_{2,10} - 2 \tau_{2,7} \tau_{2,10} - 28 \tau_{2,8} \tau_{2,10} - 2 \tau_{2,9} \tau_{2,10} + \\
& 16 \tau_{1,11} \tau_{2,11} - 12 \tau_{1,14} \tau_{2,11} - 20 \tau_{1,15} \tau_{2,11} - 12 \tau_{1,17} \tau_{2,11} + 18 \tau_{2,7} \tau_{2,11} - 42 \tau_{2,8} \tau_{2,11} + 24 \tau_{2,10} \tau_{2,11} + \\
& 68 \tau_{1,12} \tau_{2,12} + 2 \tau_{1,15} \tau_{2,12} - 42 \tau_{1,16} \tau_{2,12} + 10 \tau_{1,17} \tau_{2,12} + 6 \tau_{2,7} \tau_{2,12} - 42 \tau_{2,9} \tau_{2,12} + 6 \tau_{2,10} \tau_{2,12} - 42 \tau_{1,11} \tau_{2,14} + \\
& 34 \tau_{1,14} \tau_{2,14} - 40 \tau_{1,15} \tau_{2,14} + 40 \tau_{1,17} \tau_{2,14} + 4 \tau_{2,11} \tau_{2,14} + 22 \tau_{1,12} \tau_{2,15} + 4 \tau_{1,14} \tau_{2,15} + 4 \tau_{1,15} \tau_{2,15} - 26 \tau_{1,16} \tau_{2,15} - \\
& 14 \tau_{1,17} \tau_{2,15} + 4 \tau_{2,11} \tau_{2,15} - 2 \tau_{2,12} \tau_{2,15} + 10 \tau_{2,14} \tau_{2,15} - 12 \tau_{1,12} \tau_{2,16} - 16 \tau_{1,15} \tau_{2,16} + 8 \tau_{1,16} \tau_{2,16} - 4 \tau_{1,17} \tau_{2,16} + \\
& 4 \tau_{2,12} \tau_{2,16} - 36 \tau_{2,15} \tau_{2,16} - 30 \tau_{1,11} \tau_{2,17} - 8 \tau_{1,12} \tau_{2,17} + 38 \tau_{1,14} \tau_{2,17} - 12 \tau_{1,15} \tau_{2,17} + 8 \tau_{1,16} \tau_{2,17} + 12 \tau_{1,17} \tau_{2,17} - \\
& 8 \tau_{2,11} \tau_{2,17} - 44 \tau_{2,12} \tau_{2,17} + 48 \tau_{2,14} \tau_{2,17} + 26 \tau_{2,15} \tau_{2,17} - 24 \tau_{2,16} \tau_{2,17} - 44 \tau_{1,11} \tau_{3,7} + 28 \tau_{2,7} \tau_{3,7} + 38 \tau_{2,8} \tau_{3,7} - \\
& 32 \tau_{2,10} \tau_{3,7} - 34 \tau_{2,11} \tau_{3,7} + 28 \tau_{1,11} \tau_{3,10} + 32 \tau_{2,7} \tau_{3,10} - 64 \tau_{2,8} \tau_{3,10} + 52 \tau_{2,10} \tau_{3,10} + 64 \tau_{2,11} \tau_{3,10} - \\
& 56 \tau_{3,7} \tau_{3,10} - 2 \tau_{1,8} (24 \tau_{1,10} - 2 \tau_{1,11} + 20 \tau_{2,7} - 17 \tau_{2,8} + 20 \tau_{2,10} + 21 \tau_{2,11} - 2 \tau_{3,7} + 42 \tau_{3,10}) + 38 \tau_{1,12} \tau_{3,15} + \\
& 30 \tau_{1,15} \tau_{3,15} - 34 \tau_{1,16} \tau_{3,15} - 14 \tau_{1,17} \tau_{3,15} + 4 \tau_{2,12} \tau_{3,15} + 62 \tau_{2,15} \tau_{3,15} - 44 \tau_{2,16} \tau_{3,15} + 28 \tau_{2,17} \tau_{3,15} + \\
& 64 \tau_{1,12} \tau_{3,17} + 24 \tau_{1,15} \tau_{3,17} - 64 \tau_{1,16} \tau_{3,17} - 4 \tau_{1,17} \tau_{3,17} + 84 \tau_{2,12} \tau_{3,17} + 32 \tau_{2,15} \tau_{3,17} - 28 \tau_{2,16} \tau_{3,17} - \\
& 32 \tau_{2,17} \tau_{3,17} + 56 \tau_{3,15} \tau_{3,17} + 4 \tau_{1,12} \tau_{4,7} + 30 \tau_{2,7} \tau_{4,7} - 34 \tau_{2,9} \tau_{4,7} + 14 \tau_{2,10} \tau_{4,7} + 38 \tau_{2,12} \tau_{4,7} + 2 \tau_{1,10} \\
& (4 \tau_{1,11} + 22 \tau_{1,12} + 6 \tau_{2,7} - 19 \tau_{2,8} - 4 \tau_{2,9} + 6 \tau_{2,10} + 15 \tau_{2,11} + 4 \tau_{2,12} - 12 \tau_{3,7} + 30 \tau_{3,10} - 14 \tau_{4,7} - 16 \tau_{4,10}) - \\
& 84 \tau_{1,12} \tau_{4,10} - 24 \tau_{2,7} \tau_{4,10} + 64 \tau_{2,9} \tau_{4,10} - 4 \tau_{2,10} \tau_{4,10} - 64 \tau_{2,12} \tau_{4,10} - 56 \tau_{4,7} \tau_{4,10} +
\end{aligned}$$

$$\begin{aligned}
& 4 \tau_{1,9} (6 \tau_{1,10} + \tau_{1,12} - 4 \tau_{2,7} + 2 \tau_{2,9} + \tau_{2,10} - 3 \tau_{2,12} - 11 \tau_{4,7} + 7 \tau_{4,10}) - 34 \tau_{1,11} \tau_{4,15} + 38 \tau_{1,14} \tau_{4,15} + \\
& 28 \tau_{1,15} \tau_{4,15} + 32 \tau_{1,17} \tau_{4,15} - 44 \tau_{2,11} \tau_{4,15} + 4 \tau_{2,14} \tau_{4,15} - 14 \tau_{2,15} \tau_{4,15} + 24 \tau_{2,17} \tau_{4,15} - \\
& 4 (16 \tau_{1,11} - 16 \tau_{1,14} + 8 \tau_{1,15} - 13 \tau_{1,17} + 7 \tau_{2,11} - 21 \tau_{2,14} + \tau_{2,15} - 15 \tau_{2,17} - 14 \tau_{4,15}) \tau_{4,17} l_5^2 l_6^2 + \\
& 20 u^3 \tau_{7,8} l_5^2 l_6^2 - 24 u (-s^2 + t^2 + u^2) \tau_{7,8} l_5^2 l_6^2 + 20 u^3 \tau_{9,10} l_5^2 l_6^2 - \\
& 24 u (-s^2 + t^2 + u^2) \tau_{9,10} l_5^2 l_6^2 + \\
& 20 u^3 \tau_{14,15} l_5^2 l_6^2 - \\
& 24 u (-s^2 + t^2 + u^2) \tau_{14,15} l_5^2 l_6^2 - \\
& 20 u^3 \tau_{16,17} l_5^2 l_6^2 + \\
& 24 u (-s^2 + t^2 + u^2) \tau_{16,17} l_5^2 l_6^2 + \\
& 16 u^3 l_5^2 l_6^2 l_{13}^2 + \\
& 48 u (-s^2 + t^2 + u^2) l_5^2 l_6^2 l_{13}^2 + \\
& 16 u^3 l_5^2 l_8^2 l_{14}^2 - \\
& 36 u (-s^2 + t^2 + u^2) l_5^2 l_8^2 l_{14}^2 + \\
& 16 u^3 l_6^2 l_8^2 l_{14}^2 - \\
& 36 u (-s^2 + t^2 + u^2) l_6^2 l_8^2 l_{14}^2 - \\
& 4 s (7 s^2 - 3 t^2 - 16 u^2) (l_5^2 + l_6^2) l_9^2 l_{16}^2
\end{aligned}$$

■  $N_{45}^{(7)}$

$$\begin{aligned}
& \frac{1}{16} (14 \tau_{2,12} l_5^2 l_8^2 l_{14}^2 s^2 + 2 \tau_{3,9} l_5^2 l_8^2 l_{14}^2 s^2 - 56 \tau_{3,10} l_5^2 l_8^2 l_{14}^2 s^2 - 32 \tau_{3,11} l_5^2 l_8^2 l_{14}^2 s^2 - 62 \tau_{3,12} l_5^2 l_8^2 l_{14}^2 s^2 + 10 \tau_{4,9} l_5^2 l_8^2 l_{14}^2 s^2 - \\
& 85 \tau_{4,10} l_5^2 l_8^2 l_{14}^2 s^2 - 64 \tau_{4,11} l_5^2 l_8^2 l_{14}^2 s^2 - 89 \tau_{4,12} l_5^2 l_8^2 l_{14}^2 s^2 + 4 \tau_{1,11} l_6^2 l_8^2 l_{14}^2 s^2 - 14 \tau_{1,12} l_6^2 l_8^2 l_{14}^2 s^2 + \\
& 10 \tau_{1,16} l_6^2 l_8^2 l_{14}^2 s^2 + 64 \tau_{3,11} l_6^2 l_8^2 l_{14}^2 s^2 + 89 \tau_{3,12} l_6^2 l_8^2 l_{14}^2 s^2 - 10 \tau_{3,16} l_6^2 l_8^2 l_{14}^2 s^2 - 85 \tau_{3,17} l_6^2 l_8^2 l_{14}^2 s^2 + \\
& 32 \tau_{4,11} l_6^2 l_8^2 l_{14}^2 s^2 + 62 \tau_{4,12} l_6^2 l_8^2 l_{14}^2 s^2 - 2 \tau_{4,16} l_6^2 l_8^2 l_{14}^2 s^2 - 56 \tau_{4,17} l_6^2 l_8^2 l_{14}^2 s^2 + 20 t (2 t - u) \tau_{2,9} l_5^2 l_8^2 l_{14}^2 - \\
& 54 t^2 \tau_{2,12} l_5^2 l_8^2 l_{14}^2 - 6 u^2 \tau_{2,12} l_5^2 l_8^2 l_{14}^2 - 6 t^2 \tau_{3,9} l_5^2 l_8^2 l_{14}^2 + 32 u^2 \tau_{3,9} l_5^2 l_8^2 l_{14}^2 - 100 t^2 \tau_{3,10} l_5^2 l_8^2 l_{14}^2 + 8 u^2 \tau_{3,10} l_5^2 l_8^2 l_{14}^2 - \\
& 76 t^2 \tau_{3,11} l_5^2 l_8^2 l_{14}^2 + 50 u^2 \tau_{3,11} l_5^2 l_8^2 l_{14}^2 - 90 t^2 \tau_{3,12} l_5^2 l_8^2 l_{14}^2 - 30 u^2 \tau_{3,12} l_5^2 l_8^2 l_{14}^2 + 22 t^2 \tau_{4,9} l_5^2 l_8^2 l_{14}^2 + 2 u^2 \tau_{4,9} l_5^2 l_8^2 l_{14}^2 - \\
& 119 t^2 \tau_{4,10} l_5^2 l_8^2 l_{14}^2 - 5 u^2 \tau_{4,10} l_5^2 l_8^2 l_{14}^2 - 100 t^2 \tau_{4,11} l_5^2 l_8^2 l_{14}^2 + 8 u^2 \tau_{4,11} l_5^2 l_8^2 l_{14}^2 - 147 t^2 \tau_{4,12} l_5^2 l_8^2 l_{14}^2 - \\
& 5 u^2 \tau_{4,12} l_5^2 l_8^2 l_{14}^2 + 28 t^2 \tau_{1,11} l_6^2 l_8^2 l_{14}^2 - 28 u^2 \tau_{1,11} l_6^2 l_8^2 l_{14}^2 + 54 t^2 \tau_{1,12} l_6^2 l_8^2 l_{14}^2 + 6 u^2 \tau_{1,12} l_6^2 l_8^2 l_{14}^2 - 50 t^2 \tau_{1,16} l_6^2 l_8^2 l_{14}^2 - \\
& 10 u^2 \tau_{1,16} l_6^2 l_8^2 l_{14}^2 + 100 t^2 \tau_{3,11} l_6^2 l_8^2 l_{14}^2 - 8 u^2 \tau_{3,11} l_6^2 l_8^2 l_{14}^2 + 147 t^2 \tau_{3,12} l_6^2 l_8^2 l_{14}^2 + 5 u^2 \tau_{3,12} l_6^2 l_8^2 l_{14}^2 - \\
& 22 t^2 \tau_{3,16} l_6^2 l_8^2 l_{14}^2 - 2 u^2 \tau_{3,16} l_6^2 l_8^2 l_{14}^2 - 119 t^2 \tau_{3,17} l_6^2 l_8^2 l_{14}^2 - 5 u^2 \tau_{3,17} l_6^2 l_8^2 l_{14}^2 + 76 t^2 \tau_{4,11} l_6^2 l_8^2 l_{14}^2 - 50 u^2 \tau_{4,11} l_6^2 l_8^2 l_{14}^2 + \\
& 90 t^2 \tau_{4,12} l_6^2 l_8^2 l_{14}^2 + 30 u^2 \tau_{4,12} l_6^2 l_8^2 l_{14}^2 + 6 t^2 \tau_{4,16} l_6^2 l_8^2 l_{14}^2 - 32 u^2 \tau_{4,16} l_6^2 l_8^2 l_{14}^2 - 100 t^2 \tau_{4,17} l_6^2 l_8^2 l_{14}^2 + 8 u^2 \tau_{4,17} l_6^2 l_8^2 l_{14}^2 + \\
& (85 \tau_{3,7} l_5^2 s^2 - 10 \tau_{3,8} l_5^2 s^2 + 89 \tau_{3,11} l_5^2 s^2 + 64 \tau_{3,12} l_5^2 s^2 + 56 \tau_{4,7} l_5^2 s^2 - 2 \tau_{4,8} l_5^2 s^2 + 62 \tau_{4,11} l_5^2 s^2 + \\
& 32 \tau_{4,12} l_5^2 s^2 + 10 (s^2 - t^2 - 5 u^2) \tau_{2,8} l_5^2 + 4 (s^2 - 7 t^2 + 7 u^2) \tau_{2,12} l_5^2 + 5 t^2 \tau_{3,7} l_5^2 + 119 u^2 \tau_{3,7} l_5^2 - \\
& 2 t^2 \tau_{3,8} l_5^2 - 22 u^2 \tau_{3,8} l_5^2 + 5 t^2 \tau_{3,11} l_5^2 + 147 u^2 \tau_{3,11} l_5^2 - 8 t^2 \tau_{3,12} l_5^2 + 100 u^2 \tau_{3,12} l_5^2 - 8 t^2 \tau_{4,7} l_5^2 + \\
& 100 u^2 \tau_{4,7} l_5^2 - 32 t^2 \tau_{4,8} l_5^2 + 6 u^2 \tau_{4,8} l_5^2 + 30 t^2 \tau_{4,11} l_5^2 + 90 u^2 \tau_{4,11} l_5^2 - 50 t^2 \tau_{4,12} l_5^2 + \\
& 76 u^2 \tau_{4,12} l_5^2 + (-32 \tau_{3,12} s^2 + 2 \tau_{3,14} s^2 - 56 \tau_{3,15} s^2 - 89 \tau_{4,11} s^2 - 64 \tau_{4,12} s^2 + 10 \tau_{4,14} s^2 - \\
& 85 \tau_{4,15} s^2 + 2 (7 s^2 - 3 (t^2 + 9 u^2)) \tau_{1,11} - 4 (s^2 - 7 t^2 + 7 u^2) \tau_{1,12} + 10 (-s^2 + t^2 + 5 u^2) \tau_{1,14} - \\
& 2 (31 s^2 + 15 (t^2 + 3 u^2)) \tau_{3,11} + 50 t^2 \tau_{3,12} - 76 u^2 \tau_{3,12} + 32 t^2 \tau_{3,14} - 6 u^2 \tau_{3,14} + 8 t^2 \tau_{3,15} - 100 u^2 \tau_{3,15} - \\
& 5 t^2 \tau_{4,11} - 147 u^2 \tau_{4,11} + 8 t^2 \tau_{4,12} - 100 u^2 \tau_{4,12} + 2 t^2 \tau_{4,14} + 22 u^2 \tau_{4,14} - 5 t^2 \tau_{4,15} - 119 u^2 \tau_{4,15}) l_6^2) \\
& l_9^2 l_{16}^2 + 2 \tau_{2,11} l_5^2 (4 s (4 t - 3 u) l_8^2 l_{14}^2 + (3 (t^2 + 9 u^2) - 7 s^2) l_9^2 l_{16}^2)
\end{aligned}$$

■  $N_{45}^{(8)}$

$$-\frac{1}{16} \left( l_5^2 + l_6^2 \right) l_{13}^2 \left( l_8^2 l_{14}^2 + l_9^2 l_{16}^2 \right) \left( 14 s^2 + 23 \left( t^2 + u^2 \right) \right)$$
