# Supplementary material for: The Ultraviolet Behavior of N=8 Supergravity at Four Loops
Source: arXiv:0905.2326 ancillary file (2012-01-08)
Supplement: Supplementary file 42 [file SUGRA46.pdf]

## Integral 46: $\mathcal{I}_{46}$

$\mathcal{N} = 8$  four-point four-loop amplitude.

### ■ 2D plot of graph associated with $\mathcal{I}_{46}$

This fixes the labelling associated with the numerator expressions given below.

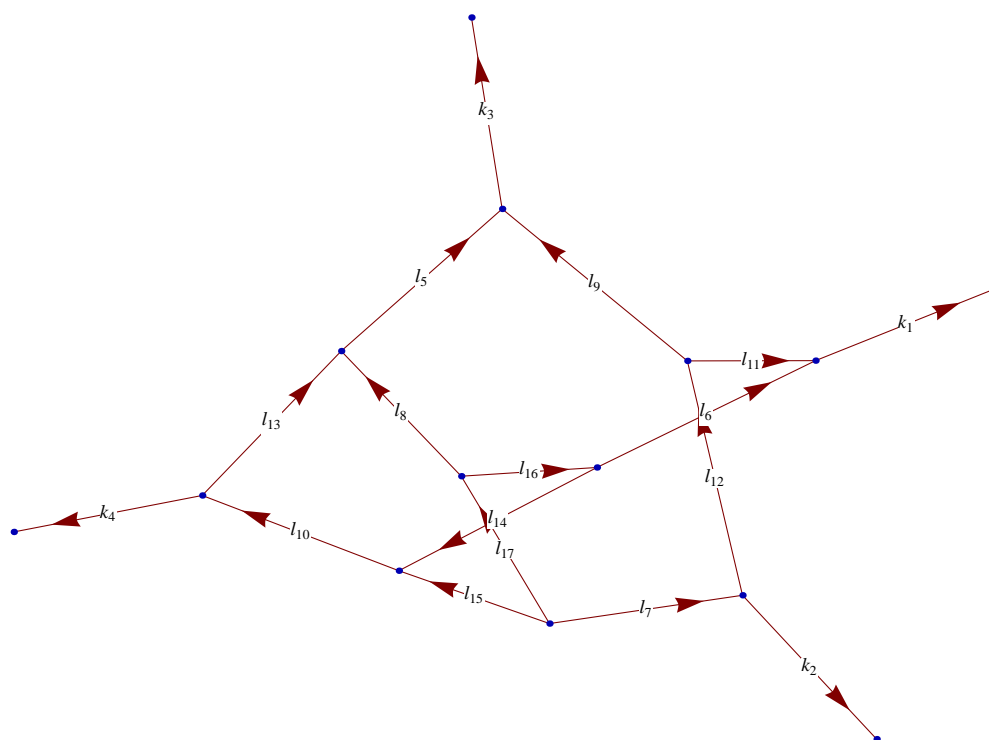

When using MathPlayer, by clicking three times (holding the click on the third click) directly on a vertex, one is able to move that vertex around, and its associated edges follow elastically. This functionality is absent when viewing as a pdf.

*Note: propagators for certain graphs were relabeled in the manuscript due to size constraints. The labels given in `aux/rawData/Neq8FourLoops.m` should be used for verification purposes.*

### ■ 3D plot of graph associated with $\mathcal{I}_{46}$

3D PLOT UNAVAILABLE FOR PDF. Please see .nb version for the 3D figure.

When using MathPlayer, by clicking anywhere in the image and dragging one should be able to rotate this 3D image. By holding (ALT) or (COMMAND) while clicking and moving the mouse up/down one should be able to zoom in/out. This functionality is absent when viewing as a pdf.

### ■ "Vertex Form" of graph associated with $\mathcal{I}_{46}$

This function returns the graph associated with the integral object in a vertex representation. This can be used as a way of specifying the topology of a graph using trivalent (cubic) vertices,  $\text{gVertex}[p_a, p_b, p_c]$ , where  $\{p_a, p_b, p_c\}$  are momenta labeling the propagators (edges) of the graph, and is understood that the edge labelled by  $p_a$  flows into the edge labelled by  $-p_a$ . Additionally, each vertex represents the manifest conservation of ( $D$  - dimensional) momenta :

$$\text{gVertex}[\{p_1, p_2, p_3\}] \iff (p_1 + p_2 + p_3 = 0)$$

$$\{\text{gVertex}(\{k_1, -l_{11}, -l_6\}), \text{gVertex}(\{k_2, -l_7, l_{12}\}), \text{gVertex}(\{k_3, -l_5, -l_9\}), \text{gVertex}(\{k_4, -l_{10}, l_{13}\}), \text{gVertex}(\{l_5, -l_{13}, -l_8\}), \\ \text{gVertex}(\{l_6, -l_{16}, l_{14}\}), \text{gVertex}(\{l_7, l_{17}, l_{15}\}), \text{gVertex}(\{l_8, l_{16}, -l_{17}\}), \text{gVertex}(\{l_9, -l_{12}, l_{11}\}), \text{gVertex}(\{l_{10}, -l_{14}, -l_{15}\})\}$$

### ■ Numerator expression for integral 46:

The following notation is used:  $\tau_{i,j} \equiv \begin{cases} 2 k_i \cdot l_j & \text{if } i \leq 4, j > 4 \\ 2 l_i \cdot l_j & \text{if } i, j > 4 \end{cases}$ .

$$s \equiv 2 k_1 \cdot k_2 = 2 k_3 \cdot k_4$$

We use  $s, t, u$  to represent the traditional Mandelstam variables for massless external four-point momenta:  $t \equiv 2 k_1 \cdot k_4 = 2 k_2 \cdot k_3$ .

$$u \equiv 2 k_1 \cdot k_3 = 2 k_2 \cdot k_4$$

Furthermore we use the shorthand  $(l_i)^2$  to represent the lorentz square:  $(l_i)^2 = l_i \cdot l_i$ .

The total numerator  $\mathcal{N}_{46}$  is given by summing over the following terms, distinguished here by explicit dependence on loop momenta:  $\mathcal{N}_{46} = \sum_{i=0}^8 \mathcal{N}_{46}^{(i)}$ :

$$\blacksquare \mathcal{N}_{46}^{(0)}$$

$$0$$

$$\blacksquare \mathcal{N}_{46}^{(1)}$$

$$0$$

$$\blacksquare \mathcal{N}_{46}^{(2)}$$

$$-\frac{1}{2} s \left( -s (\tau_{1,5} + \tau_{2,5})^2 (t^2 + u^2) - \frac{1}{2} l_9^2 (t - u)^2 (-s^2 + t^2 + u^2) \right)$$

$$\blacksquare \mathcal{N}_{46}^{(3)}$$

$$\frac{1}{4} \left( l_5^2 s^4 \tau_{3,8} + 2 \tau_{1,5} (-4 s^2 \tau_{2,5} (t \tau_{3,7} + u \tau_{3,6}) - 2 s \tau_{2,5}^2 (t - 2u) (t - u) + l_9^2 t^3 (t + 7u)) + \right. \\ l_9^2 (-3 u \tau_{1,12} (t - u) (-s^2 + t^2 + u^2) - 3 t \tau_{2,11} (t - u) (-s^2 + t^2 + u^2) + 4 s (s^2 - t^2 - u^2) (t \tau_{3,11} - u \tau_{3,12}) + \\ \tau_{3,5} (s^2 (5 t^2 + 7 t u + 5 u^2) - 4 t^4 - 7 t^3 u - 10 t^2 u^2 - 7 t u^3 - 4 u^4)) + 2 l_9^2 u^3 \tau_{2,5} (7 t + u) + \\ \left. 2 s \tau_{1,5}^2 (\tau_{2,5} (3 s^2 - 7 t^2 - 5 u^2) - 2 s (t \tau_{3,7} + u \tau_{3,6})) - 4 s^2 \tau_{2,5}^2 (t \tau_{3,7} + u \tau_{3,6}) + 4 t \tau_{1,5}^3 (t^2 - u^2) + 4 u \tau_{2,5}^3 (u^2 - t^2) \right)$$

$N_{46}^{(4)}$ 

$$\begin{aligned}
& \frac{1}{16} \left( (4 \tau_{6,8} l_5^2 + 4 \tau_{7,8} l_5^2 + (-16 l_8^2 + 3 l_9^2 + 2 l_{13}^2) l_5^2 + 8 l_6^2 l_9^2) t^4 + \right. \\
& 4 (2 (\tau_{2,11} \tau_{3,5} + 2 (\tau_{3,5} - \tau_{3,11}) \tau_{3,11} + \tau_{1,5} (2 \tau_{2,11} + \tau_{3,5} + 4 \tau_{3,11})) l_9^2 - \\
& (\tau_{1,8} + \tau_{2,8} - \tau_{3,6} - \tau_{3,7} - \tau_{3,13} + \tau_{4,8}) (\tau_{3,13} + \tau_{4,8}) l_5^2) t^3 + 8 (\tau_{1,5} + \tau_{2,5})^2 \\
& (2 \tau_{1,5}^2 + 2 (\tau_{3,6} - \tau_{3,7}) \tau_{1,5} + \tau_{3,6}^2 + \tau_{3,7}^2) t^2 + (s^2 - t^2 - u^2) (8 \tau_{6,8} l_5^2 + 8 \tau_{7,8} l_5^2 + (4 l_{13}^2 - 13 l_9^2) l_5^2 - 16 l_6^2 l_9^2) t^2 + \\
& 2 (s^2 - t^2 - u^2) (2 (7 \tau_{1,5}^2 + 2 (7 \tau_{2,11} + 4 \tau_{3,5}) \tau_{1,5} - 3 \tau_{1,12}^2 + \tau_{2,5}^2 + 3 \tau_{2,11}^2 + 4 \tau_{3,5}^2 - 4 \tau_{3,11}^2 - 2 \tau_{3,12}^2 + \\
& (5 \tau_{2,5} - 7 \tau_{1,12}) \tau_{3,5} + 2 \tau_{2,11} (5 \tau_{3,5} - 4 \tau_{3,11}) + 2 \tau_{3,5} \tau_{3,11} + 4 (\tau_{2,5} - 2 \tau_{1,12}) \tau_{3,12}) l_9^2 - \\
& 3 (\tau_{1,8} + \tau_{2,8} - \tau_{3,6} - \tau_{3,7} - \tau_{3,13} + \tau_{4,8}) (\tau_{3,13} + \tau_{4,8}) l_5^2) t + \\
& u (s^2 - t^2 - u^2) (12 \tau_{6,8} l_5^2 + 12 \tau_{7,8} l_5^2 + (16 l_8^2 - 23 l_9^2 + 6 l_{13}^2) l_5^2 - 16 (l_6^2 + l_7^2) l_9^2) t + \\
& 8 u^2 (\tau_{1,5} + \tau_{2,5})^2 (2 \tau_{2,5}^2 + 2 (\tau_{3,7} - \tau_{3,6}) \tau_{2,5} + \tau_{3,6}^2 + \tau_{3,7}^2) - \\
& 8 (s^2 - t^2 - u^2) (\tau_{1,5} + \tau_{2,5})^2 (-\tau_{3,6}^2 - \tau_{3,7}^2 + \tau_{2,5} (\tau_{3,6} - \tau_{3,7}) + \tau_{1,5} (2 \tau_{2,5} - \tau_{3,6} + \tau_{3,7})) + \\
& 4 u^3 (- (\tau_{1,8} + \tau_{2,8} - \tau_{3,6} - \tau_{3,7} - \tau_{3,13} + \tau_{4,8}) (\tau_{3,13} + \tau_{4,8}) l_5^2 - \\
& 2 (\tau_{1,12} (2 \tau_{2,5} + \tau_{3,5}) - \tau_{2,5} (\tau_{3,5} - 4 \tau_{3,12}) + 2 \tau_{3,12} (\tau_{3,5} + \tau_{3,12})) l_9^2) + \\
& 2 u (s^2 - t^2 - u^2) (2 (\tau_{1,5}^2 + (5 \tau_{3,5} - 4 \tau_{3,11}) \tau_{1,5} + 3 \tau_{1,12}^2 + 7 \tau_{2,5}^2 - 3 \tau_{2,11}^2 + 8 \tau_{2,5} \tau_{3,5} + \tau_{2,11} (7 \tau_{3,5} - 8 \tau_{3,11}) - \\
& 2 \tau_{1,12} (7 \tau_{2,5} + 5 \tau_{3,5} + 4 \tau_{3,12}) - 2 (-2 \tau_{3,5}^2 + \tau_{3,12} \tau_{3,5} + \tau_{3,11}^2 + 2 \tau_{3,12}^2)) l_9^2 - \\
& 3 (\tau_{1,8} + \tau_{2,8} - \tau_{3,6} - \tau_{3,7} - \tau_{3,13} + \tau_{4,8}) (\tau_{3,13} + \tau_{4,8}) l_5^2) + u^4 (4 \tau_{6,8} l_5^2 + 4 \tau_{7,8} l_5^2 + (-16 l_8^2 + 3 l_9^2 + 2 l_{13}^2) l_5^2 + 8 l_7^2 l_9^2) + \\
& u^2 (s^2 - t^2 - u^2) (8 \tau_{6,8} l_5^2 + 8 \tau_{7,8} l_5^2 + (4 l_{13}^2 - 13 l_9^2) l_5^2 - 16 l_7^2 l_9^2)
\end{aligned}$$

■  $N_{46}^{(5)}$ 

$$\frac{1}{16}$$

$$\begin{aligned}
& \left( (-8 \tau_{3,6} \tau_{6,8} l_5^2 + 12 \tau_{4,8} \tau_{6,8} l_5^2 - 8 \tau_{3,7} \tau_{7,8} l_5^2 - 4 \tau_{4,8} \tau_{7,8} l_5^2 - 16 \tau_{1,13} l_8^2 l_5^2 + 16 \tau_{2,13} l_8^2 l_5^2 + 16 \tau_{3,9} l_8^2 l_5^2 + 32 \tau_{4,9} l_8^2 l_5^2 + 16 \tau_{4,11} \right. \\
& \quad l_8^2 l_5^2 + 16 \tau_{4,12} l_8^2 l_5^2 - 7 \tau_{1,12} l_9^2 l_5^2 + 5 \tau_{1,13} l_9^2 l_5^2 + 13 \tau_{2,11} l_9^2 l_5^2 + 15 \tau_{2,13} l_9^2 l_5^2 + 14 \tau_{3,11} l_9^2 l_5^2 + \\
& \quad 14 \tau_{3,12} l_9^2 l_5^2 + 4 \tau_{3,13} (\tau_{6,8} - 3 \tau_{7,8} - 4 l_8^2 + 2 l_9^2) l_5^2 + 2 \tau_{3,8} (2 \tau_{6,8} - 2 \tau_{7,8} + 9 l_9^2) l_5^2 + \\
& \quad (2 \tau_{3,10} - \tau_{3,11} - \tau_{3,12} + 2 \tau_{4,10} + \tau_{4,11} + \tau_{4,12}) l_{13}^2 l_5^2 - 20 \tau_{2,11} l_6^2 l_9^2 - 8 \tau_{2,14} l_6^2 l_9^2 + 8 \tau_{2,15} l_6^2 l_9^2 + \\
& \quad 16 \tau_{3,7} l_6^2 l_9^2 - 12 \tau_{3,11} l_6^2 l_9^2 + 8 \tau_{3,14} l_6^2 l_9^2 + 8 \tau_{3,15} l_6^2 l_9^2 + 24 \tau_{4,7} l_6^2 l_9^2 - 36 \tau_{4,11} l_6^2 l_9^2 - 8 \tau_{4,15} l_6^2 l_9^2) t^3 - \\
& \quad 4 ((\tau_{3,8}^3 + 3 (\tau_{3,13} + \tau_{4,8}) \tau_{3,8}^2 + (4 \tau_{3,13}^2 + 6 \tau_{4,8} \tau_{3,13} + 4 \tau_{4,8}^2) \tau_{3,8} + 3 \tau_{3,13}^3 + 3 \tau_{4,8}^3 + 5 \tau_{3,13} \tau_{4,8}^2 + \\
& \quad 5 \tau_{3,13}^2 \tau_{4,8} + \tau_{3,6} (-(\tau_{3,8} + \tau_{3,13})^2 - 5 \tau_{4,8}^2 - 2 (2 \tau_{3,8} + 3 \tau_{3,13}) \tau_{4,8}) + \tau_{3,6}^2 (\tau_{3,8} + 2 (\tau_{3,13} + \tau_{4,8})) + \\
& \quad \tau_{3,7}^2 (\tau_{3,8} + 2 (\tau_{3,13} + \tau_{4,8})) + \tau_{3,7} (\tau_{3,8}^2 + 2 (2 \tau_{3,13} + \tau_{4,8}) \tau_{3,8} + (\tau_{3,13} + \tau_{4,8}) (5 \tau_{3,13} + \tau_{4,8}))) l_5^2 + \\
& \quad (2 \tau_{1,5}^3 + (\tau_{3,5} - 8 \tau_{3,11}) \tau_{1,5}^2 - 2 (-2 \tau_{3,11}^2 + 4 (\tau_{2,11} + \tau_{3,5}) \tau_{3,11} + \tau_{2,11} (\tau_{2,11} + \tau_{3,5})) \tau_{1,5} - 2 \tau_{1,12}^3 - \\
& \quad \tau_{2,5}^2 \tau_{3,5} - \tau_{2,11}^2 \tau_{3,5} + 4 \tau_{2,11} \tau_{3,11} (\tau_{3,11} - \tau_{3,5}) + 4 \tau_{2,5} \tau_{3,12} (\tau_{3,5} + \tau_{3,12}) - \tau_{1,12}^2 (7 \tau_{3,5} + 8 \tau_{3,12}) + \\
& \quad 2 \tau_{3,5} (\tau_{3,11}^2 + \tau_{3,12}^2 + \tau_{3,5} (\tau_{3,12} - \tau_{3,11})) + 2 \tau_{1,12} (\tau_{2,5}^2 + (5 \tau_{3,5} + 4 \tau_{3,12}) \tau_{2,5} + 2 (\tau_{3,5}^2 - \tau_{3,12}^2))) l_9^2) t^2 + \\
& \quad \frac{1}{2} (s^2 - t^2 - u^2) (-4 \tau_{3,13} \tau_{6,8} l_5^2 + 20 \tau_{4,8} \tau_{6,8} l_5^2 - 24 \tau_{3,7} \tau_{7,8} l_5^2 - 20 \tau_{3,13} \tau_{7,8} l_5^2 + 4 \tau_{4,8} \tau_{7,8} l_5^2 - 16 \tau_{1,13} l_8^2 l_5^2 + \\
& \quad 16 \tau_{2,13} l_8^2 l_5^2 + 16 \tau_{3,9} l_8^2 l_5^2 + 16 \tau_{3,13} l_8^2 l_5^2 + 32 \tau_{4,9} l_8^2 l_5^2 + 16 \tau_{4,11} l_8^2 l_5^2 + 16 \tau_{4,12} l_8^2 l_5^2 + \\
& \quad 2 \tau_{3,8} (2 \tau_{6,8} - 2 \tau_{7,8} - 15 l_9^2) l_5^2 + 23 \tau_{1,12} l_9^2 l_5^2 - 37 \tau_{1,13} l_9^2 l_5^2 - 13 \tau_{2,11} l_9^2 l_5^2 + \tau_{2,13} l_9^2 l_5^2 + 2 \tau_{3,11} l_9^2 l_5^2 + \\
& \quad 2 \tau_{3,12} l_9^2 l_5^2 - 8 \tau_{3,13} l_9^2 l_5^2 + (-4 \tau_{3,9} + 2 \tau_{3,10} - \tau_{3,11} - \tau_{3,12} - 4 \tau_{4,9} + 2 \tau_{4,10} + \tau_{4,11} + \tau_{4,12}) l_{13}^2 l_5^2 - 8 \tau_{2,11} l_6^2 l_9^2 - \\
& \quad 16 \tau_{2,14} l_6^2 l_9^2 - 16 \tau_{2,15} l_6^2 l_9^2 - 32 \tau_{3,7} l_6^2 l_9^2 + 40 \tau_{3,11} l_6^2 l_9^2 - 16 \tau_{3,15} l_6^2 l_9^2 - 80 \tau_{4,7} l_6^2 l_9^2 + 56 \tau_{4,11} l_6^2 l_9^2 + 20 \tau_{1,12} l_7^2 l_9^2 + \\
& \quad 8 \tau_{1,15} l_7^2 l_9^2 - 4 \tau_{3,12} l_7^2 l_9^2 + 8 \tau_{3,15} l_7^2 l_9^2 - 40 \tau_{4,6} l_7^2 l_9^2 - 36 \tau_{4,12} l_7^2 l_9^2 + 8 \tau_{4,14} l_7^2 l_9^2 + 8 \tau_{3,6} (l_7^2 l_9^2 - 3 \tau_{6,8} l_5^2)) t - \\
& \quad 4 s^2 \tau_{1,8}^2 (\tau_{3,8} + 2 (\tau_{3,13} + \tau_{4,8})) l_5^2 - 4 s^2 \tau_{2,8}^2 (\tau_{3,8} + 2 (\tau_{3,13} + \tau_{4,8})) l_5^2 + \\
& \quad \tau_{1,8} l_5^2 \left( 8 \tau_{3,7} (\tau_{3,8} + 2 (\tau_{3,13} + \tau_{4,8})) s^2 - \right. \\
& \quad 4 (2 \tau_{7,8} s^2 + (t - u) \tau_{3,8}^2 + (\tau_{3,13} + \tau_{4,8}) ((5 t - u) \tau_{3,13} + (t - 5 u) \tau_{4,8}) + 2 \tau_{3,8} ((2 t - u) \tau_{3,13} + (t - 2 u) \tau_{4,8})) s + \\
& \quad \left. \frac{1}{2} (37 t^3 + 13 u t^2 + 23 u^2 t + 39 u^3 - s^2 (23 t + 13 u)) l_9^2 \right) + \tau_{2,8} l_5^2 \left( 8 \tau_{3,6} (\tau_{3,8} + 2 (\tau_{3,13} + \tau_{4,8})) s^2 - \right. \\
& \quad 4 (2 \tau_{6,8} s^2 + (u - t) \tau_{3,8}^2 - (\tau_{3,13} + \tau_{4,8}) ((t - 5 u) \tau_{3,13} + (5 t - u) \tau_{4,8}) + 2 \tau_{3,8} ((u - 2 t) \tau_{4,8} - (t - 2 u) \tau_{3,13})) s + \\
& \quad \left. \frac{1}{2} (39 t^3 + 23 u t^2 + 13 u^2 t + 37 u^3 - s^2 (13 t + 23 u)) l_9^2 \right) + \\
& \quad 4 (s^2 - t^2 - u^2) ((\tau_{4,8}^3 + (2 \tau_{3,8} + 7 \tau_{3,13}) \tau_{4,8}^2 + (\tau_{3,8}^2 + 6 \tau_{3,13} \tau_{3,8} + 7 \tau_{3,13}^2) \tau_{4,8} + \tau_{3,13} (\tau_{3,8} + \tau_{3,13})^2 -
\end{aligned}$$

$$\begin{aligned}
& \tau_{3,6}^2 (\tau_{3,8} + 2 (\tau_{3,13} + \tau_{4,8})) - \tau_{3,7}^2 (\tau_{3,8} + 2 (\tau_{3,13} + \tau_{4,8})) - \\
& \tau_{3,6} (\tau_{3,13} - \tau_{4,8}) (\tau_{3,8} + 2 (\tau_{3,13} + \tau_{4,8})) - \tau_{3,7} (\tau_{3,13} - \tau_{4,8}) (\tau_{3,8} + 2 (\tau_{3,13} + \tau_{4,8})) \Big) l_5^2 + \\
& (\tau_{1,5}^3 + (7 \tau_{2,11} + \tau_{3,5} + 4 \tau_{3,11}) \tau_{1,5}^2 + (7 \tau_{2,11}^2 + 8 \tau_{3,5} \tau_{2,11} - 4 \tau_{3,11}^2 + 6 \tau_{3,5} \tau_{3,11}) \tau_{1,5} + \tau_{2,11}^3 + \\
& 2 (2 \tau_{1,12} - 2 \tau_{2,5} - \tau_{3,5}) \tau_{3,12}^2 - (\tau_{1,12} - \tau_{2,5}) (\tau_{1,12}^2 - 6 \tau_{2,5} \tau_{1,12} + \tau_{2,5}^2) + \tau_{2,11}^2 (5 \tau_{3,5} - 4 \tau_{3,11}) + \\
& 2 \tau_{2,11} (\tau_{3,5} - \tau_{3,11}) (\tau_{3,5} + 2 \tau_{3,11}) + \tau_{3,5} (5 \tau_{1,12}^2 - 2 (4 \tau_{2,5} + \tau_{3,5}) \tau_{1,12} + \tau_{2,5}^2 + 2 (\tau_{3,5} - \tau_{3,11}) \tau_{3,11}) + \\
& 2 (2 \tau_{1,12} - 2 \tau_{2,5} - \tau_{3,5}) (\tau_{1,12} + \tau_{2,5} + \tau_{3,5}) \tau_{3,12} \Big) l_9^2) - \\
& 4 u^2 \Big( (\tau_{3,8}^3 + 3 (\tau_{3,13} + \tau_{4,8}) \tau_{3,8}^2 + (4 \tau_{3,13}^2 + 6 \tau_{4,8} \tau_{3,13} + 4 \tau_{4,8}^2) \tau_{3,8} + 3 \tau_{3,13}^3 + 3 \tau_{4,8}^3 + 5 \tau_{3,13} \tau_{4,8}^2 + \\
& 5 \tau_{3,13}^2 \tau_{4,8} - \tau_{3,7} ((\tau_{3,8} + \tau_{3,13})^2 + 5 \tau_{4,8}^2 + 2 (2 \tau_{3,8} + 3 \tau_{3,13}) \tau_{4,8}) + \tau_{3,6}^2 (\tau_{3,8} + 2 (\tau_{3,13} + \tau_{4,8})) + \\
& \tau_{3,7}^2 (\tau_{3,8} + 2 (\tau_{3,13} + \tau_{4,8})) + \tau_{3,6} (\tau_{3,8}^2 + 2 (2 \tau_{3,13} + \tau_{4,8}) \tau_{3,8} + (\tau_{3,13} + \tau_{4,8}) (5 \tau_{3,13} + \tau_{4,8})) \Big) l_5^2 + \\
& (2 \tau_{2,5}^3 + (\tau_{3,5} + 8 \tau_{3,12}) \tau_{2,5}^2 + 4 \tau_{3,12} (2 \tau_{3,5} + \tau_{3,12}) \tau_{2,5} + 2 \tau_{2,11}^3 - \tau_{1,12}^2 (2 \tau_{2,5} + \tau_{3,5}) - \tau_{1,5}^2 (2 \tau_{2,11} + \tau_{3,5}) + \\
& \tau_{2,11}^2 (8 \tau_{3,11} - 7 \tau_{3,5}) + 4 \tau_{2,11} (\tau_{3,11}^2 - \tau_{3,5}^2) + 2 \tau_{1,5} (2 \tau_{3,11} (\tau_{3,11} - \tau_{3,5}) + \tau_{2,11} (4 \tau_{3,11} - 5 \tau_{3,5})) + \\
& 2 \tau_{1,12} (\tau_{2,5} (\tau_{3,5} - 4 \tau_{3,12}) - 2 \tau_{3,12} (\tau_{3,5} + \tau_{3,12})) + 2 \tau_{3,5} (\tau_{3,11}^2 + \tau_{3,12}^2 + \tau_{3,5} (\tau_{3,12} - \tau_{3,11})) \Big) l_9^2) + \\
& u^3 \Big( -4 \tau_{4,8} \tau_{6,8} l_5^2 - 8 \tau_{3,7} \tau_{7,8} l_5^2 + 12 \tau_{4,8} \tau_{7,8} l_5^2 + 16 \tau_{1,13} l_8^2 l_5^2 - 16 \tau_{2,13} l_8^2 l_5^2 + 16 \tau_{3,9} l_8^2 l_5^2 + 32 \tau_{4,9} l_8^2 l_5^2 - \\
& 16 \tau_{4,11} l_8^2 l_5^2 - 16 \tau_{4,12} l_8^2 l_5^2 - 13 \tau_{1,12} l_9^2 l_5^2 + 15 \tau_{1,13} l_9^2 l_5^2 + 7 \tau_{2,11} l_9^2 l_5^2 + 5 \tau_{2,13} l_9^2 l_5^2 - 14 \tau_{3,11} l_9^2 l_5^2 - \\
& 14 \tau_{3,12} l_9^2 l_5^2 + 4 \tau_{3,13} (-3 \tau_{6,8} + \tau_{7,8} - 4 l_8^2 + 2 l_9^2) l_5^2 + 2 \tau_{3,8} (-2 \tau_{6,8} + 2 \tau_{7,8} + 9 l_9^2) l_5^2 + \\
& (2 \tau_{3,10} + \tau_{3,11} + \tau_{3,12} + 2 \tau_{4,10} - \tau_{4,11} - \tau_{4,12}) l_{13}^2 l_5^2 + 20 \tau_{1,12} l_7^2 l_9^2 + 8 \tau_{1,14} l_7^2 l_9^2 - 8 \tau_{1,15} l_7^2 l_9^2 + \\
& 12 \tau_{3,12} l_7^2 l_9^2 + 8 \tau_{3,14} l_7^2 l_9^2 + 8 \tau_{3,15} l_7^2 l_9^2 + 24 \tau_{4,6} l_7^2 l_9^2 + 36 \tau_{4,12} l_7^2 l_9^2 - 8 \tau_{4,14} l_7^2 l_9^2 - 8 \tau_{3,6} (\tau_{6,8} l_5^2 - 2 l_7^2 l_9^2) \Big) - \\
& \frac{1}{2} u (s^2 - t^2 - u^2) \Big( 20 \tau_{3,13} \tau_{6,8} l_5^2 - 4 \tau_{4,8} \tau_{6,8} l_5^2 + 24 \tau_{3,7} \tau_{7,8} l_5^2 + 4 \tau_{3,13} \tau_{7,8} l_5^2 - 20 \tau_{4,8} \tau_{7,8} l_5^2 - 16 \tau_{1,13} l_8^2 l_5^2 + \\
& 16 \tau_{2,13} l_8^2 l_5^2 - 16 \tau_{3,9} l_8^2 l_5^2 - 16 \tau_{3,13} l_8^2 l_5^2 - 32 \tau_{4,9} l_8^2 l_5^2 + 16 \tau_{4,11} l_8^2 l_5^2 + 16 \tau_{4,12} l_8^2 l_5^2 - 13 \tau_{1,12} l_9^2 l_5^2 - \tau_{1,13} l_9^2 l_5^2 + \\
& 23 \tau_{2,11} l_9^2 l_5^2 + 37 \tau_{2,13} l_9^2 l_5^2 + 2 \tau_{3,11} l_9^2 l_5^2 + 2 \tau_{3,12} l_9^2 l_5^2 + 8 \tau_{3,13} l_9^2 l_5^2 + 2 \tau_{3,8} (2 \tau_{6,8} - 2 \tau_{7,8} + 15 l_9^2) l_5^2 + \\
& (4 \tau_{3,9} - 2 \tau_{3,10} - \tau_{3,11} - \tau_{3,12} + 4 \tau_{4,9} - 2 \tau_{4,10} + \tau_{4,11} + \tau_{4,12}) l_{13}^2 l_5^2 + 20 \tau_{2,11} l_6^2 l_9^2 - 8 \tau_{2,14} l_6^2 l_9^2 - \\
& 8 \tau_{3,7} l_6^2 l_9^2 - 4 \tau_{3,11} l_6^2 l_9^2 - 8 \tau_{3,14} l_6^2 l_9^2 + 40 \tau_{4,7} l_6^2 l_9^2 - 36 \tau_{4,11} l_6^2 l_9^2 - 8 \tau_{4,15} l_6^2 l_9^2 - 8 \tau_{1,12} l_7^2 l_9^2 + 16 \tau_{1,14} l_7^2 l_9^2 + \\
& 16 \tau_{1,15} l_7^2 l_9^2 + 40 \tau_{3,12} l_7^2 l_9^2 + 16 \tau_{3,14} l_7^2 l_9^2 + 80 \tau_{4,6} l_7^2 l_9^2 + 56 \tau_{4,12} l_7^2 l_9^2 + 8 \tau_{3,6} (3 \tau_{6,8} l_5^2 + 4 l_7^2 l_9^2) \Big)
\end{aligned}$$

■  $N_{46}^{(6)}$

$$\begin{aligned}
& \frac{1}{16} \Big( l_9^2 (16 \tau_{7,14} l_6^2 + l_5^2 (55 l_6^2 + 29 l_7^2 - 8 l_{13}^2)) t^3 + \\
& (-24 l_7^2 l_9^2 \tau_{1,12}^2 + 16 \tau_{1,14} l_7^2 l_9^2 \tau_{1,12} - 28 \tau_{3,6} l_7^2 l_9^2 \tau_{1,12} - 36 \tau_{3,12} l_7^2 l_9^2 \tau_{1,12} + 16 \tau_{3,14} l_7^2 l_9^2 \tau_{1,12} + 32 \tau_{4,6} l_7^2 l_9^2 \tau_{1,12} + \\
& 8 \tau_{4,12} l_7^2 l_9^2 \tau_{1,12} - 16 \tau_{4,14} l_7^2 l_9^2 \tau_{1,12} + 16 \tau_{3,7}^2 l_6^2 l_9^2 + 12 \tau_{3,11}^2 l_6^2 l_9^2 + 88 \tau_{4,7}^2 l_6^2 l_9^2 + 40 \tau_{4,11}^2 l_6^2 l_9^2 + \\
& 8 \tau_{3,11} \tau_{3,14} l_6^2 l_9^2 - 80 \tau_{3,11} \tau_{4,7} l_6^2 l_9^2 + 16 \tau_{3,14} \tau_{4,7} l_6^2 l_9^2 + 16 \tau_{3,15} \tau_{4,7} l_6^2 l_9^2 + 36 \tau_{3,11} \tau_{4,11} l_6^2 l_9^2 - \\
& 120 \tau_{4,7} \tau_{4,11} l_6^2 l_9^2 - 16 \tau_{2,15} (\tau_{3,11} - \tau_{4,7} + \tau_{4,11}) l_6^2 l_9^2 + 8 \tau_{3,11} \tau_{4,15} l_6^2 l_9^2 - 16 \tau_{4,7} \tau_{4,15} l_6^2 l_9^2 + 16 \tau_{4,11} \tau_{4,15} l_6^2 l_9^2 -
\end{aligned}$$

$$\begin{aligned}
& 4 \tau_{3,7} (9 \tau_{3,11} + 2 \tau_{3,14} - 18 \tau_{4,7} + 11 \tau_{4,11} + 2 \tau_{4,15}) l_6^2 l_9^2 + 8 \tau_{3,6}^2 l_7^2 l_9^2 - 4 \tau_{3,12}^2 l_7^2 l_9^2 - 8 \tau_{1,15} \tau_{3,6} l_7^2 l_9^2 + \\
& 16 \tau_{1,14} \tau_{3,12} l_7^2 l_9^2 + 8 \tau_{1,15} \tau_{3,12} l_7^2 l_9^2 - 12 \tau_{3,6} \tau_{3,12} l_7^2 l_9^2 + 16 \tau_{3,12} \tau_{3,14} l_7^2 l_9^2 - 8 \tau_{3,6} \tau_{3,15} l_7^2 l_9^2 + \\
& 8 \tau_{3,12} \tau_{3,15} l_7^2 l_9^2 + 8 \tau_{3,6} \tau_{4,6} l_7^2 l_9^2 + 24 \tau_{3,12} \tau_{4,6} l_7^2 l_9^2 - 4 \tau_{3,6} \tau_{4,12} l_7^2 l_9^2 + 12 \tau_{3,12} \tau_{4,12} l_7^2 l_9^2 - 8 \tau_{3,6} \tau_{4,14} l_7^2 l_9^2 - \\
& 8 \tau_{3,12} \tau_{4,14} l_7^2 l_9^2 + (4 \tau_{1,10}^2 + (\tau_{3,9} + 10 \tau_{3,10} - 4 \tau_{3,11} - 5 \tau_{4,9} - 2 \tau_{4,10} - 4 \tau_{4,11}) \tau_{1,10} + 4 \tau_{2,10}^2 + 8 \tau_{3,9}^2 + \\
& 6 \tau_{3,10}^2 + 2 \tau_{3,11}^2 + 2 \tau_{3,12}^2 + 8 \tau_{4,9}^2 + 6 \tau_{4,10}^2 + 2 \tau_{4,11}^2 + 2 \tau_{4,12}^2 - 3 \tau_{3,11} \tau_{4,9} - 3 \tau_{3,12} \tau_{4,9} + \\
& \tau_{3,11} \tau_{4,10} + 5 \tau_{3,12} \tau_{4,10} + 2 \tau_{4,9} \tau_{4,10} + 8 \tau_{4,9} \tau_{4,11} + \tau_{4,10} \tau_{4,11} + 4 \tau_{4,9} \tau_{4,12} + 5 \tau_{4,10} \tau_{4,12} - \\
& \tau_{3,10} (5 \tau_{3,11} + \tau_{3,12} + 4 \tau_{4,9} + 5 \tau_{4,11} + \tau_{4,12}) + \tau_{2,10} (-5 \tau_{3,9} - 2 \tau_{3,10} + 4 \tau_{3,12} + \tau_{4,9} + 10 \tau_{4,10} + 4 \tau_{4,12}) + \\
& \tau_{3,9} (2 \tau_{3,10} - 4 \tau_{3,11} - 8 \tau_{3,12} + 10 \tau_{4,9} - 4 \tau_{4,10} + 3 (\tau_{4,11} + \tau_{4,12}))) l_5^2 l_{13}^2) t^2 + \\
& \frac{1}{2} (s^2 - t^2 - u^2) ((32 \tau_{7,14} + 65 l_5^2) l_6^2 + (16 \tau_{6,15} + 99 l_5^2) l_7^2) l_9^2 t - 8 (2t + u) (t + 3u) \tau_{2,11}^2 l_6^2 l_9^2 - \\
& 8 s^2 \tau_{2,14} (\tau_{3,7} + \tau_{3,11}) l_6^2 l_9^2 - \\
& 4 \tau_{2,11} (4 \tau_{2,15} s^2 + 9 \tau_{4,7} s^2 - 4 \tau_{4,15} s^2 + 4 t \tau_{3,14} s - 4 u \tau_{3,15} s + 2 u \tau_{4,11} s + \\
& (2 s^2 - t^2 - 9 u^2) \tau_{3,7} + (6 s^2 - t^2 + 3 u^2) \tau_{3,11} - 7 t^2 \tau_{4,7} - u^2 \tau_{4,7}) l_6^2 l_9^2 + \\
& \frac{1}{2} u (s^2 - t^2 - u^2) ((16 \tau_{7,14} + 99 l_5^2) l_6^2 + (32 \tau_{6,15} + 65 l_5^2) l_7^2) l_9^2 + \\
& u^3 l_9^2 (16 \tau_{6,15} l_7^2 + l_5^2 (29 l_6^2 + 55 l_7^2 - 8 l_{13}^2)) + \\
& 2 (s^2 - t^2 - u^2) (-14 l_7^2 l_9^2 \tau_{1,12}^2 + 8 \tau_{1,14} l_7^2 l_9^2 \tau_{1,12} + 4 \tau_{3,6} l_7^2 l_9^2 \tau_{1,12} - 12 \tau_{3,12} l_7^2 l_9^2 \tau_{1,12} + 4 \tau_{3,14} l_7^2 l_9^2 \tau_{1,12} - \\
& 4 \tau_{3,15} l_7^2 l_9^2 \tau_{1,12} + 18 \tau_{4,6} l_7^2 l_9^2 \tau_{1,12} + 2 \tau_{4,12} l_7^2 l_9^2 \tau_{1,12} - 8 \tau_{4,14} l_7^2 l_9^2 \tau_{1,12} - 2 \tau_{3,7}^2 l_6^2 l_9^2 - 2 \tau_{4,7}^2 l_6^2 l_9^2 - \\
& 2 \tau_{4,11}^2 l_6^2 l_9^2 - 4 \tau_{3,11} \tau_{3,15} l_6^2 l_9^2 - 14 \tau_{3,11} \tau_{4,7} l_6^2 l_9^2 + 4 \tau_{3,14} \tau_{4,7} l_6^2 l_9^2 + 4 \tau_{3,15} \tau_{4,7} l_6^2 l_9^2 + 2 \tau_{3,11} \tau_{4,11} l_6^2 l_9^2 + \\
& 2 \tau_{4,7} \tau_{4,11} l_6^2 l_9^2 - 4 \tau_{2,15} (2 \tau_{3,11} - \tau_{4,7} + \tau_{4,11}) l_6^2 l_9^2 + 4 \tau_{3,11} \tau_{4,15} l_6^2 l_9^2 - 4 \tau_{4,7} \tau_{4,15} l_6^2 l_9^2 + 4 \tau_{4,11} \tau_{4,15} l_6^2 l_9^2 - \\
& 4 \tau_{3,7} (\tau_{3,14} + 2 \tau_{4,7} - 2 \tau_{4,11} + \tau_{4,15}) l_6^2 l_9^2 - 2 \tau_{3,6}^2 l_7^2 l_9^2 - 2 \tau_{4,6}^2 l_7^2 l_9^2 - 2 \tau_{4,12}^2 l_7^2 l_9^2 - 4 \tau_{1,15} \tau_{3,6} l_7^2 l_9^2 + \\
& 8 \tau_{1,14} \tau_{3,12} l_7^2 l_9^2 + 4 \tau_{1,15} \tau_{3,12} l_7^2 l_9^2 + 4 \tau_{3,12} \tau_{3,14} l_7^2 l_9^2 - 4 \tau_{3,6} \tau_{3,15} l_7^2 l_9^2 + 4 \tau_{1,14} \tau_{4,6} l_7^2 l_9^2 - \\
& 8 \tau_{3,6} \tau_{4,6} l_7^2 l_9^2 + 14 \tau_{3,12} \tau_{4,6} l_7^2 l_9^2 + 4 \tau_{3,14} \tau_{4,6} l_7^2 l_9^2 + 4 \tau_{3,15} \tau_{4,6} l_7^2 l_9^2 + 4 \tau_{1,14} \tau_{4,12} l_7^2 l_9^2 - 8 \tau_{3,6} \tau_{4,12} l_7^2 l_9^2 + \\
& 2 \tau_{3,12} \tau_{4,12} l_7^2 l_9^2 - 2 \tau_{4,6} \tau_{4,12} l_7^2 l_9^2 - 4 \tau_{3,6} \tau_{4,14} l_7^2 l_9^2 - 4 \tau_{3,12} \tau_{4,14} l_7^2 l_9^2 - 4 \tau_{4,6} \tau_{4,14} l_7^2 l_9^2 - 4 \tau_{4,12} \tau_{4,14} l_7^2 l_9^2 + \\
& (2 \tau_{1,10}^2 - (\tau_{3,9} - 2 \tau_{3,10} + 2 \tau_{3,11} + \tau_{4,9} - 2 \tau_{4,10} + 2 \tau_{4,11}) \tau_{1,10} + 2 \tau_{2,10}^2 - 4 \tau_{3,9}^2 - \tau_{3,10}^2 + \tau_{3,11}^2 + \tau_{3,12}^2 - 4 \tau_{4,9}^2 - \\
& \tau_{4,10}^2 + \tau_{4,11}^2 + \tau_{4,12}^2 - \tau_{3,11} \tau_{4,10} + \tau_{3,12} \tau_{4,10} - 3 \tau_{4,9} \tau_{4,10} + \tau_{3,9} (-3 \tau_{3,10} + \tau_{3,11} - \tau_{3,12} - 7 \tau_{4,9} + \tau_{4,10}) + \\
& \tau_{4,9} \tau_{4,11} - \tau_{4,10} \tau_{4,11} - \tau_{4,9} \tau_{4,12} + \tau_{4,10} \tau_{4,12} + \tau_{3,10} (-\tau_{3,11} + \tau_{3,12} + \tau_{4,9} + 6 \tau_{4,10} - \tau_{4,11} + \tau_{4,12}) - \\
& \tau_{2,10} (\tau_{3,9} - 2 \tau_{3,10} - 2 \tau_{3,12} + \tau_{4,9} - 2 (\tau_{4,10} + \tau_{4,12}))) l_5^2 l_{13}^2) + \\
& u^2 (-16 l_7^2 l_9^2 \tau_{1,12}^2 + 16 \tau_{1,14} l_7^2 l_9^2 \tau_{1,12} + 4 \tau_{3,6} l_7^2 l_9^2 \tau_{1,12} - 20 \tau_{3,12} l_7^2 l_9^2 \tau_{1,12} - 16 \tau_{3,15} l_7^2 l_9^2 \tau_{1,12} + 8 \tau_{4,6} l_7^2 l_9^2 \tau_{1,12} - \\
& 16 \tau_{4,14} l_7^2 l_9^2 \tau_{1,12} + 8 \tau_{3,7}^2 l_6^2 l_9^2 - 4 \tau_{3,11}^2 l_6^2 l_9^2 - 16 \tau_{2,15} \tau_{3,11} l_6^2 l_9^2 - 8 \tau_{3,11} \tau_{3,14} l_6^2 l_9^2 - 16 \tau_{3,11} \tau_{3,15} l_6^2 l_9^2 - \\
& 24 \tau_{3,11} \tau_{4,7} l_6^2 l_9^2 + 12 \tau_{3,11} \tau_{4,11} l_6^2 l_9^2 + 4 \tau_{3,7} (3 \tau_{3,11} - 2 \tau_{3,14} + 2 \tau_{4,7} + \tau_{4,11} - 2 \tau_{4,15}) l_6^2 l_9^2 + 8 \tau_{3,11} \tau_{4,15} l_6^2 l_9^2 + \\
& 16 \tau_{3,6}^2 l_7^2 l_9^2 + 12 \tau_{3,12}^2 l_7^2 l_9^2 + 88 \tau_{4,6}^2 l_7^2 l_9^2 + 40 \tau_{4,12}^2 l_7^2 l_9^2 - 8 \tau_{1,15} \tau_{3,6} l_7^2 l_9^2 + 16 \tau_{1,14} \tau_{3,12} l_7^2 l_9^2 + \\
& 8 \tau_{1,15} \tau_{3,12} l_7^2 l_9^2 + 36 \tau_{3,6} \tau_{3,12} l_7^2 l_9^2 - 8 \tau_{3,6} \tau_{3,15} l_7^2 l_9^2 - 8 \tau_{3,12} \tau_{3,15} l_7^2 l_9^2 + 16 \tau_{1,14} \tau_{4,6} l_7^2 l_9^2 + 72 \tau_{3,6} \tau_{4,6} l_7^2 l_9^2 + \\
& 80 \tau_{3,12} \tau_{4,6} l_7^2 l_9^2 + 16 \tau_{3,14} \tau_{4,6} l_7^2 l_9^2 + 16 \tau_{3,15} \tau_{4,6} l_7^2 l_9^2 + 16 \tau_{1,14} \tau_{4,12} l_7^2 l_9^2 + 44 \tau_{3,6} \tau_{4,12} l_7^2 l_9^2 +
\end{aligned}$$

$$\begin{aligned}
& 36 \tau_{3,12} \tau_{4,12} l_7^2 l_9^2 + 120 \tau_{4,6} \tau_{4,12} l_7^2 l_9^2 - 8 \tau_{3,6} \tau_{4,14} l_7^2 l_9^2 - 8 \tau_{3,12} \tau_{4,14} l_7^2 l_9^2 - 16 \tau_{4,6} \tau_{4,14} l_7^2 l_9^2 - \\
& 16 \tau_{4,12} \tau_{4,14} l_7^2 l_9^2 + \left( 4 \tau_{1,10}^2 + (-5 \tau_{3,9} - 2 \tau_{3,10} - 4 \tau_{3,11} + \tau_{4,9} + 10 \tau_{4,10} - 4 \tau_{4,11}) \tau_{1,10} + 4 \tau_{2,10}^2 + 8 \tau_{3,9}^2 + \right. \\
& \quad 6 \tau_{3,10}^2 + 2 \tau_{3,11}^2 + 2 \tau_{3,12}^2 + 8 \tau_{4,9}^2 + 6 \tau_{4,10}^2 + 2 \tau_{4,11}^2 + 2 \tau_{4,12}^2 + 3 \tau_{3,11} \tau_{4,9} + 3 \tau_{3,12} \tau_{4,9} - \\
& \quad 5 \tau_{3,11} \tau_{4,10} - \tau_{3,12} \tau_{4,10} + 2 \tau_{4,9} \tau_{4,10} - 4 \tau_{4,9} \tau_{4,11} - 5 \tau_{4,10} \tau_{4,11} - 8 \tau_{4,9} \tau_{4,12} - \tau_{4,10} \tau_{4,12} + \\
& \quad \tau_{2,10} (\tau_{3,9} + 10 \tau_{3,10} + 4 \tau_{3,12} - 5 \tau_{4,9} - 2 \tau_{4,10} + 4 \tau_{4,12}) + \tau_{3,10} (\tau_{3,11} + 5 \tau_{3,12} - 4 \tau_{4,9} + \tau_{4,11} + 5 \tau_{4,12}) + \\
& \quad \left. \tau_{3,9} (2 \tau_{3,10} + 8 \tau_{3,11} + 4 \tau_{3,12} + 10 \tau_{4,9} - 4 \tau_{4,10} - 3 (\tau_{4,11} + \tau_{4,12})) \right) l_5^2 l_{13}^2 \Big)
\end{aligned}$$

■  $N_{46}^{(7)}$

0

■  $N_{46}^{(8)}$

$$-\frac{3}{4} l_5^2 l_{11}^2 l_{12}^2 l_{13}^2 s^2$$
