# Supplementary material for: The Ultraviolet Behavior of N=8 Supergravity at Four Loops
Source: arXiv:0905.2326 ancillary file (2012-01-08)
Supplement: Supplementary file 43 [file SUGRA47.pdf]

## Integral 47: $\mathcal{I}_{47}$

$\mathcal{N} = 8$  four-point four-loop amplitude.

### ■ 2D plot of graph associated with $\mathcal{I}_{47}$

This fixes the labelling associated with the numerator expressions given below.

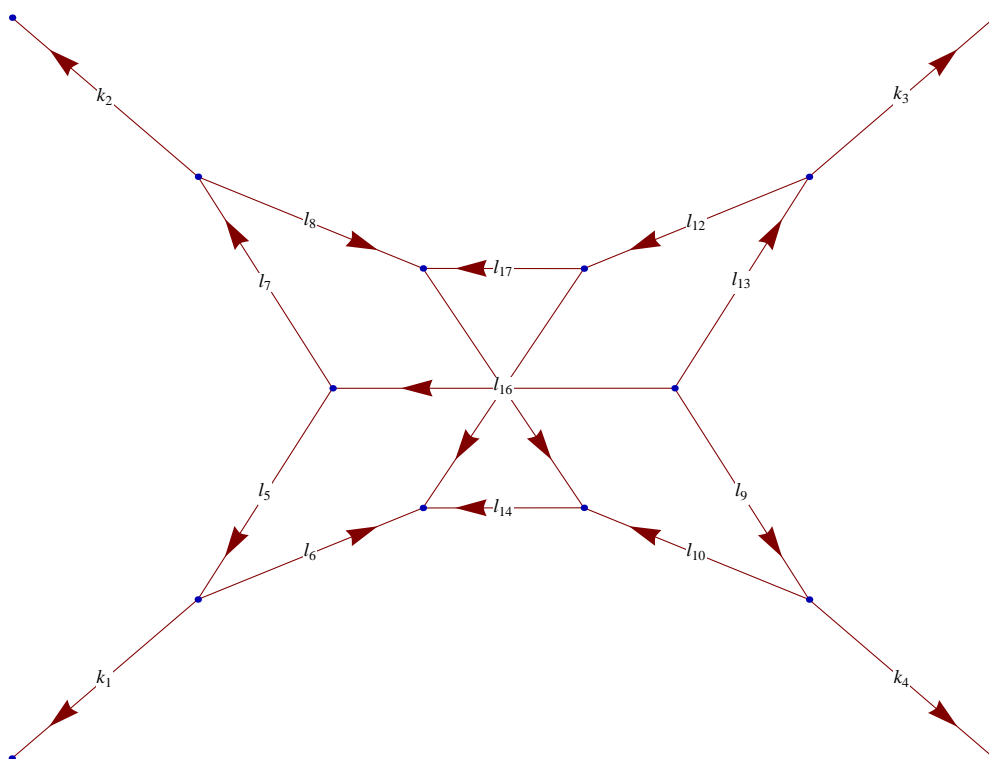

When using MathPlayer, by clicking three times (holding the click on the third click) directly on a vertex, one is able to move that vertex around, and its associated edges follow elastically. This functionality is absent when viewing as a pdf.

*Note: propagators for certain graphs were relabeled in the manuscript due to size constraints. The labels given in `aux/rawData/Neq8FourLoops.m` should be used for verification purposes.*

### ■ 3D plot of graph associated with $\mathcal{I}_{47}$

3D PLOT UNAVAILABLE FOR PDF. Please see .nb version for the 3D figure.

When using MathPlayer, by clicking anywhere in the image and dragging one should be able to rotate this 3D image. By holding (ALT) or (COMMAND) while clicking and moving the mouse up/down one should be able to zoom in/out. This functionality is absent when viewing as a pdf.

### ■ "Vertex Form" of graph associated with $\mathcal{I}_{47}$

This function returns the graph associated with the integral object in a vertex representation. This can be used as a way of specifying the topology of a graph using trivalent (cubic) vertices,  $\text{gVertex}[p_a, p_b, p_c]$ , where  $\{p_a, p_b, p_c\}$  are momenta labeling the propagators (edges) of the graph, and is understood that the edge labelled by  $p_a$  flows into the edge labelled by  $-p_a$ . Additionally, each vertex represents the manifest conservation of ( $D$  - dimensional) momenta :

$$\text{gVertex}[\{p_1, p_2, p_3\}] \iff (p_1 + p_2 + p_3 = 0)$$

$$\{\text{gVertex}(\{k_1, l_6, -l_5\}), \text{gVertex}(\{k_2, l_8, -l_7\}), \text{gVertex}(\{k_3, l_{12}, -l_{13}\}), \text{gVertex}(\{k_4, -l_9, l_{10}\}), \text{gVertex}(\{l_5, l_7, -l_{11}\}), \\ \text{gVertex}(\{-l_6, -l_{14}, -l_{15}\}), \text{gVertex}(\{-l_8, -l_{17}, l_{16}\}), \text{gVertex}(\{l_9, l_{11}, l_{13}\}), \text{gVertex}(\{-l_{10}, -l_{16}, l_{14}\}), \text{gVertex}(\{-l_{12}, l_{17}, l_{15}\})\}$$

### ■ Numerator expression for integral 47:

The following notation is used:  $\tau_{i,j} \equiv \begin{cases} 2 k_i \cdot l_j & \text{if } i \leq 4, j > 4 \\ 2 l_i \cdot l_j & \text{if } i, j > 4 \end{cases}$ .

$$s \equiv 2 k_1 \cdot k_2 = 2 k_3 \cdot k_4$$

We use  $s, t, u$  to represent the traditional Mandelstam variables for massless external four-point momenta:  $t \equiv 2 k_1 \cdot k_4 = 2 k_2 \cdot k_3$ .

$$u \equiv 2 k_1 \cdot k_3 = 2 k_2 \cdot k_4$$

Furthermore we use the shorthand  $(l_i)^2$  to represent the lorentz square:  $(l_i)^2 = l_i \cdot l_i$ .

The total numerator  $\mathcal{N}_{47}$  is given by summing over the following terms, distinguished here by explicit dependence on loop momenta:  $\mathcal{N}_{47} = \sum_{i=0}^8 \mathcal{N}_{47}^{(i)}$ :

$$\blacksquare \mathcal{N}_{47}^{(0)}$$

$$0$$

$$\blacksquare \mathcal{N}_{47}^{(1)}$$

$$0$$

$$\blacksquare \mathcal{N}_{47}^{(2)}$$

$$0$$

■  $N_{47}^{(3)}$

$$\begin{aligned}
& \frac{1}{8} \left( (2((-3\tau_{3,9} + \tau_{3,14} - 3\tau_{4,12} + 3\tau_{4,15})l_6^2 + \right. \\
& \quad (-2\tau_{2,7} - 3(\tau_{3,10} + \tau_{3,16} + \tau_{4,13}) + \tau_{4,17})l_8^2 - (3\tau_{1,8} - 3\tau_{1,16} + 3\tau_{2,5} + \tau_{2,14} + 2\tau_{4,9})l_{10}^2) - \\
& \quad (\tau_{1,7} - 2\tau_{1,12} + \tau_{2,5} - 2\tau_{2,10} - 2\tau_{3,6} + \tau_{3,9} - 2\tau_{4,8} + \tau_{4,13})l_{11}^2 - 2(3\tau_{1,7} + \tau_{1,17} + 3(\tau_{2,6} + \tau_{2,15}) + 2\tau_{3,13})l_{12}^2) t^4 - \\
& \quad (s^2 - t^2 - u^2) \left( -6\tau_{3,14}l_6^2 + 7\tau_{4,12}l_6^2 + \tau_{4,13}l_6^2 - 10\tau_{4,15}l_6^2 + 10\tau_{2,7}l_8^2 + 10\tau_{3,16}l_8^2 + \tau_{4,12}l_8^2 + 7\tau_{4,13}l_8^2 - \right. \\
& \quad 6\tau_{4,17}l_8^2 + \tau_{3,10}(l_6^2 + 7l_8^2) + 7\tau_{1,8}l_{10}^2 - 10\tau_{1,16}l_{10}^2 + 7\tau_{2,5}l_{10}^2 + \tau_{2,6}l_{10}^2 + 6\tau_{2,14}l_{10}^2 + 10\tau_{4,9}l_{10}^2 + \\
& \quad (\tau_{1,10} - 3\tau_{1,12})l_{11}^2 + \tau_{2,5}l_{11}^2 - 3\tau_{2,10}l_{11}^2 + \tau_{2,12}l_{11}^2 - 3\tau_{3,6}l_{11}^2 + \tau_{3,8}l_{11}^2 + (\tau_{4,6} - 3\tau_{4,8} + \tau_{4,13})l_{11}^2 + \\
& \quad \tau_{3,9}(7l_6^2 + l_8^2 + l_{11}^2) + (\tau_{1,8} + 6\tau_{1,17} + \tau_{2,5} + 7\tau_{2,6} + 10(\tau_{2,15} + \tau_{3,13}))l_{12}^2 + \tau_{1,7}(l_{10}^2 + l_{11}^2 + 7l_{12}^2) \Big) t^2 - \\
& \quad u \left( s^2 - t^2 - u^2 \right) \left( (5\tau_{3,9} + 5\tau_{3,10} - 12\tau_{3,14} + 5(\tau_{4,12} + \tau_{4,13}) - 12\tau_{4,15})l_6^2 + 16\tau_{2,7}l_8^2 + \right. \\
& \quad (5\tau_{3,9} + 5\tau_{3,10} + 12\tau_{3,16} + 5(\tau_{4,12} + \tau_{4,13}) - 12\tau_{4,17})l_8^2 + \\
& \quad (5\tau_{1,7} + 5\tau_{1,8} - 12\tau_{1,16} + 5\tau_{2,5} + 5\tau_{2,6} + 12\tau_{2,14} + 16\tau_{4,9})l_{10}^2 + \\
& \quad 3(\tau_{1,10} + \tau_{1,12} + \tau_{2,10} + \tau_{2,12} + \tau_{3,6} + \tau_{3,8} + \tau_{4,6} + \tau_{4,8})l_{11}^2 + \\
& \quad (5\tau_{1,7} + 5\tau_{1,8} + 12\tau_{1,17} + 5\tau_{2,5} + 5\tau_{2,6} + 12\tau_{2,15} + 16\tau_{3,13})l_{12}^2 \Big) t + 2s^2(-3s^2 + t^2 + u^2)\tau_{1,5}l_6^2 + \\
& \quad u^4 \left( 2(\tau_{4,15} - 3(\tau_{3,10} - \tau_{3,14} + \tau_{4,13}))l_6^2 - 2(2\tau_{2,7} + 3\tau_{3,9} + \tau_{3,16} + 3\tau_{4,12} - 3\tau_{4,17})l_8^2 - \right. \\
& \quad 2(3\tau_{1,7} - \tau_{1,16} + 3(\tau_{2,6} + \tau_{2,14}) + 2\tau_{4,9})l_{10}^2 - (\tau_{1,7} - 2\tau_{1,10} + \tau_{2,5} - 2\tau_{2,12} - 2\tau_{3,8} + \tau_{3,9} - 2\tau_{4,6} + \tau_{4,13})l_{11}^2 - \\
& \quad 2(3\tau_{1,8} + 3\tau_{1,17} + 3\tau_{2,5} + \tau_{2,15} + 2\tau_{3,13})l_{12}^2 \Big) - \\
& \quad u^2 \left( s^2 - t^2 - u^2 \right) \left( -10\tau_{3,14}l_6^2 + \tau_{4,12}l_6^2 + 7\tau_{4,13}l_6^2 - 6\tau_{4,15}l_6^2 + 10\tau_{2,7}l_8^2 + 6\tau_{3,16}l_8^2 + 7\tau_{4,12}l_8^2 + \tau_{4,13}l_8^2 - \right. \\
& \quad 10\tau_{4,17}l_8^2 + \tau_{3,10}(7l_6^2 + l_8^2) + \tau_{1,8}l_{10}^2 - 6\tau_{1,16}l_{10}^2 + \tau_{2,5}l_{10}^2 + 7\tau_{2,6}l_{10}^2 + 10\tau_{2,14}l_{10}^2 + 10\tau_{4,9}l_{10}^2 + \\
& \quad (\tau_{1,12} - 3\tau_{1,10})l_{11}^2 + \tau_{2,5}l_{11}^2 + \tau_{2,10}l_{11}^2 - 3\tau_{2,12}l_{11}^2 + \tau_{3,6}l_{11}^2 - 3\tau_{3,8}l_{11}^2 + (-3\tau_{4,6} + \tau_{4,8} + \tau_{4,13})l_{11}^2 + \\
& \quad \tau_{3,9}(l_6^2 + 7l_8^2 + l_{11}^2) + (7\tau_{1,8} + 10\tau_{1,17} + 7\tau_{2,5} + \tau_{2,6} + 6\tau_{2,15} + 10\tau_{3,13})l_{12}^2 + \tau_{1,7}(7l_{10}^2 + l_{11}^2 + l_{12}^2) \Big) \Big)
\end{aligned}$$

■  $N_{47}^{(4)}$ 

$$\begin{aligned}
& \frac{1}{8} \left( (2\tau_{5,9}^2 + 2\tau_{5,13}^2 + 2\tau_{7,9}^2 + 2\tau_{7,13}^2 - 2(\tau_{9,17} - 3\tau_{13,16})l_8^2 - 2l_6^2(3\tau_{9,15} + \tau_{13,14} + 2l_8^2) + \right. \\
& (\tau_{5,10} - \tau_{5,12} + \tau_{6,9} - \tau_{6,13} - \tau_{7,10} + \tau_{7,12} - \tau_{8,9} + \tau_{8,13})l_{11}^2 + 2l_{10}^2(-3\tau_{5,16} + \tau_{7,14} - 2l_{12}^2) + 2(\tau_{5,17} + 3\tau_{7,15})l_{12}^2) t^4 - \\
& (-2l_{11}^2\tau_{1,12}^2 + 10\tau_{4,12}l_6^2\tau_{1,12} - 4\tau_{4,15}l_6^2\tau_{1,12} - 2\tau_{1,10}l_{11}^2\tau_{1,12} - \tau_{3,5}l_{11}^2\tau_{1,12} - 2\tau_{4,13}^2\tau_{5,9} + 2\tau_{4,13}^2\tau_{5,13} + \\
& 2\tau_{2,13}\tau_{4,13}\tau_{5,13} - 2\tau_{3,5}\tau_{4,13}\tau_{5,13} - 2\tau_{4,7}\tau_{4,13}\tau_{7,9} + 2\tau_{1,13}\tau_{4,13}\tau_{7,13} - 2\tau_{3,7}\tau_{4,13}\tau_{7,13} + 2\tau_{3,10}^2l_6^2 - \\
& 6\tau_{4,12}^2l_6^2 + 2\tau_{4,13}^2l_6^2 + 4\tau_{1,5}\tau_{3,10}l_6^2 + 2\tau_{1,10}\tau_{3,10}l_6^2 - 4\tau_{1,10}\tau_{3,14}l_6^2 - 2\tau_{3,10}\tau_{3,14}l_6^2 + 4\tau_{1,5}\tau_{4,12}l_6^2 + \\
& 10\tau_{3,5}\tau_{4,12}l_6^2 + 12\tau_{1,5}\tau_{4,13}l_6^2 + 2\tau_{1,10}\tau_{4,13}l_6^2 + 4\tau_{3,10}\tau_{4,13}l_6^2 - 10\tau_{3,14}\tau_{4,13}l_6^2 - 4\tau_{1,5}\tau_{4,15}l_6^2 - 4\tau_{3,5}\tau_{4,15}l_6^2 + \\
& 6\tau_{4,12}\tau_{4,15}l_6^2 - 6\tau_{3,10}^2l_8^2 + 2\tau_{4,12}^2l_8^2 + 2\tau_{4,13}^2l_8^2 + 4\tau_{2,7}\tau_{3,7}l_8^2 + 4\tau_{2,7}\tau_{3,10}l_8^2 + 10\tau_{2,10}\tau_{3,10}l_8^2 + 4\tau_{2,7}\tau_{3,16}l_8^2 + \\
& 4\tau_{2,10}\tau_{3,16}l_8^2 - 6\tau_{3,10}\tau_{3,16}l_8^2 + 10\tau_{3,10}\tau_{4,7}l_8^2 + 4\tau_{3,16}\tau_{4,7}l_8^2 + 4\tau_{2,7}\tau_{4,12}l_8^2 + 2\tau_{2,12}\tau_{4,12}l_8^2 + 2\tau_{3,7}\tau_{4,12}l_8^2 + \\
& 12\tau_{2,7}\tau_{4,13}l_8^2 + 10\tau_{2,10}\tau_{4,13}l_8^2 - 4\tau_{3,10}\tau_{4,13}l_8^2 + 2\tau_{3,16}\tau_{4,13}l_8^2 + 10\tau_{4,7}\tau_{4,13}l_8^2 - 4\tau_{2,12}\tau_{4,17}l_8^2 - 4\tau_{3,7}\tau_{4,17}l_8^2 - \\
& 2\tau_{4,12}\tau_{4,17}l_8^2 + \tau_{3,9}^2(2(\tau_{7,9} - \tau_{7,13} + l_6^2 + l_8^2) - l_{11}^2) - 2\tau_{2,10}^2l_{11}^2 - 2\tau_{3,6}^2l_{11}^2 - 2\tau_{4,8}^2l_{11}^2 - \tau_{4,13}^2l_{11}^2 - \\
& 2\tau_{2,10}\tau_{2,12}l_{11}^2 - \tau_{1,10}\tau_{3,5}l_{11}^2 - \tau_{1,13}\tau_{3,6}l_{11}^2 + \tau_{2,13}\tau_{3,6}l_{11}^2 + \tau_{2,10}\tau_{3,7}l_{11}^2 + \tau_{2,12}\tau_{3,7}l_{11}^2 - \tau_{1,13}\tau_{3,8}l_{11}^2 + \\
& \tau_{2,13}\tau_{3,8}l_{11}^2 - 2\tau_{3,6}\tau_{3,8}l_{11}^2 - \tau_{2,10}\tau_{4,7}l_{11}^2 - \tau_{2,12}\tau_{4,7}l_{11}^2 - 2\tau_{4,6}\tau_{4,8}l_{11}^2 + \tau_{1,13}\tau_{4,13}l_{11}^2 - \tau_{2,13}\tau_{4,13}l_{11}^2 + \\
& 3\tau_{3,6}\tau_{4,13}l_{11}^2 + \tau_{3,8}\tau_{4,13}l_{11}^2 + \tau_{4,5}(2(2\tau_{1,5} + \tau_{3,10} - 2\tau_{3,14})l_6^2 + 2\tau_{4,13}(l_6^2 - \tau_{5,9}) + (\tau_{1,10} + \tau_{1,12})l_{11}^2) + \\
& \tau_{2,9}(2(\tau_{3,9} + \tau_{4,13})\tau_{5,9} + 2(5\tau_{1,8} - 2\tau_{1,16})l_{10}^2 + (\tau_{3,9} - \tau_{4,6} - \tau_{4,8})l_{11}^2) + \\
& \tau_{3,9}(-2\tau_{4,5}\tau_{5,9} + 2\tau_{2,13}\tau_{5,13} + 2\tau_{4,13}(-\tau_{5,9} + \tau_{5,13} + \tau_{7,9} - \tau_{7,13}) - 2(\tau_{3,5}\tau_{5,13} + \tau_{4,7}\tau_{7,9} + (\tau_{3,7} - \tau_{1,13})\tau_{7,13}) + \\
& 2(6\tau_{1,5} + 5\tau_{1,12} + 5\tau_{3,5} - 2\tau_{4,12} - \tau_{4,15})l_6^2 + 2(6\tau_{2,7} + \tau_{2,12} + \tau_{3,7} + 2\tau_{4,12} - 5\tau_{4,17})l_8^2 + (\tau_{4,6} + 3\tau_{4,8})l_{11}^2) + \\
& 2(-3\tau_{2,6}^2 + (-3\tau_{2,15} + 5\tau_{3,6} + 2\tau_{3,13})\tau_{2,6} + \tau_{1,13}(5\tau_{2,6} + 2\tau_{2,15}) + 2\tau_{2,15}\tau_{3,6} + (\tau_{1,8} + 2\tau_{1,17})(\tau_{2,13} + \tau_{3,8}) + \\
& 2(\tau_{1,8} + \tau_{2,13} + \tau_{2,15} + \tau_{3,8})\tau_{3,13})l_{12}^2 + \tau_{2,5}^2(2\tau_{5,13} - 2\tau_{7,13} + 2l_{10}^2 - l_{11}^2 + 2l_{12}^2) + \\
& \tau_{2,5}(2(\tau_{4,5} - \tau_{1,13})\tau_{5,13} + 2(\tau_{3,7} - \tau_{2,9})\tau_{7,9} + 2\tau_{4,7}\tau_{7,13} - 2(2\tau_{1,8} + \tau_{1,16})l_{10}^2 + 2(5(\tau_{2,9} + \tau_{4,8}) + 6\tau_{4,9})l_{10}^2 + \\
& (\tau_{1,10} + 3\tau_{1,12})l_{11}^2 - \tau_{4,5}l_{11}^2 + \tau_{3,5}(2\tau_{5,9} + l_{11}^2) + 2(2\tau_{1,8} + 5\tau_{1,17} + \tau_{3,8} + 6\tau_{3,13})l_{12}^2 + 2\tau_{2,13}(l_{12}^2 - \tau_{7,13})) + \\
& 2((l_{12}^2 - 3l_{10}^2)\tau_{1,8}^2 + ((3\tau_{1,16} + 5\tau_{4,8} + 2\tau_{4,9})l_{10}^2 + \tau_{1,17}l_{12}^2)\tau_{1,8} + 2\tau_{1,5}\tau_{1,10}l_6^2 + 2\tau_{2,7}\tau_{2,12}l_8^2 + \\
& (\tau_{2,6}^2 + (\tau_{2,14} + \tau_{4,6} + 2\tau_{4,9})\tau_{2,6} + 2\tau_{4,6}(\tau_{2,14} + \tau_{4,9}) - 2\tau_{1,16}(\tau_{4,8} + \tau_{4,9}))l_{10}^2))t^3 + \\
& (2\tau_{2,5}^4 + 2(\tau_{2,13} + \tau_{4,5} - \tau_{4,7})\tau_{2,5}^3 + (\tau_{3,5}^2 + (\tau_{2,9} - \tau_{3,7})^2 + \tau_{4,5}^2 + (\tau_{2,13} - \tau_{4,7})^2)\tau_{2,5}^2 + (\tau_{3,9} + \tau_{4,13})^2((\tau_{2,13} - \tau_{3,5})^2 + \\
& \tau_{3,7}^2 + 2\tau_{3,9}^2 + (\tau_{2,9} - \tau_{4,5})^2 + \tau_{4,7}^2 + 2\tau_{4,13}^2 + 2\tau_{3,7}\tau_{3,9} - 2\tau_{3,9}\tau_{4,7} + 2(-\tau_{2,9} + \tau_{2,13} - \tau_{3,5} + \tau_{4,5})\tau_{4,13}) + \\
& \tau_{1,13}^2(\tau_{2,5}^2 + (\tau_{3,9} + \tau_{4,13})^2) - 2\tau_{1,13}((\tau_{2,5} + \tau_{4,5})\tau_{2,5}^2 + (\tau_{3,7} + \tau_{3,9})(\tau_{3,9} + \tau_{4,13})^2))t^2 + \\
& (s^2 - t^2 - u^2)(4\tau_{5,9}^2 + 4\tau_{5,13}^2 + 4\tau_{7,9}^2 + 4\tau_{7,13}^2 - l_6^2(10\tau_{9,15} + 6\tau_{13,14} + 5l_8^2) + \\
& 2((5\tau_{13,16} - 3\tau_{9,17})l_8^2 + (3\tau_{7,14} - 5\tau_{5,16})l_{10}^2 + (\tau_{5,10} - \tau_{5,12} + \tau_{6,9} - \tau_{6,13} - \tau_{7,10} + \tau_{7,12} - \tau_{8,9} + \tau_{8,13})l_{11}^2) + \\
& (6\tau_{5,17} + 10\tau_{7,15} - 5l_{10}^2)l_{12}^2)t^2 + \\
& u(s^2 - t^2 - u^2)(6\tau_{5,9}^2 + 6\tau_{5,13}^2 + 6\tau_{7,9}^2 + 6\tau_{7,13}^2 - 12\tau_{9,15}l_6^2 - 12\tau_{13,14}l_6^2 - 14l_6^2l_8^2 + 3l_6^2l_{11}^2 + \\
& 3l_8^2l_{11}^2 + 3l_{10}^2l_{11}^2 + (3l_{11}^2 - 14l_{10}^2)l_{12}^2 + 3(4(\tau_{13,16} - \tau_{9,17})l_8^2 + 4(\tau_{7,14} - \tau_{5,16})l_{10}^2 +
\end{aligned}$$

$$\begin{aligned}
& (\tau_{5,10} + \tau_{5,12} + \tau_{6,9} + \tau_{6,13} + \tau_{7,10} + \tau_{7,12} + \tau_{8,9} + \tau_{8,13}) l_{11}^2 + 4(\tau_{5,17} + \tau_{7,15}) l_{12}^2)) t - \\
& \frac{1}{2} (s^2 - t^2 - u^2) (2 l_{11}^2 \tau_{1,10}^2 + 14 \tau_{3,10} l_6^2 \tau_{1,10} - 12 \tau_{3,14} l_6^2 \tau_{1,10} + 14 \tau_{4,13} l_6^2 \tau_{1,10} - 2 \tau_{1,12} l_{11}^2 \tau_{1,10} - \\
& 3 \tau_{3,5} l_{11}^2 \tau_{1,10} - 4 \tau_{4,13}^2 \tau_{5,9} + 4 \tau_{4,13}^2 \tau_{5,13} + 6 \tau_{2,13} \tau_{4,13} \tau_{5,13} - 6 \tau_{3,5} \tau_{4,13} \tau_{5,13} - 2 \tau_{4,13}^2 \tau_{7,9} - 6 \tau_{4,7} \tau_{4,13} \tau_{7,9} + \\
& 2 \tau_{4,13}^2 \tau_{7,13} + 6 \tau_{1,13} \tau_{4,13} \tau_{7,13} - 6 \tau_{3,7} \tau_{4,13} \tau_{7,13} + 10 \tau_{3,10}^2 l_6^2 + 2 \tau_{4,12}^2 l_6^2 + 18 \tau_{4,13}^2 l_6^2 + 4 \tau_{1,5} \tau_{3,5} l_6^2 - \\
& 4 \tau_{1,5} \tau_{3,14} l_6^2 + 2 \tau_{3,10} \tau_{3,14} l_6^2 + 22 \tau_{1,12} \tau_{4,12} l_6^2 + 22 \tau_{3,5} \tau_{4,12} l_6^2 + 24 \tau_{1,5} \tau_{4,13} l_6^2 + 28 \tau_{3,10} \tau_{4,13} l_6^2 - \\
& 22 \tau_{3,14} \tau_{4,13} l_6^2 - 8 \tau_{1,5} \tau_{4,15} l_6^2 - 12 \tau_{1,12} \tau_{4,15} l_6^2 - 12 \tau_{3,5} \tau_{4,15} l_6^2 + 10 \tau_{4,12} \tau_{4,15} l_6^2 + 2 \tau_{3,10}^2 l_8^2 + 10 \tau_{4,12}^2 l_8^2 + \\
& 18 \tau_{4,13}^2 l_8^2 + 8 \tau_{2,7} \tau_{3,7} l_8^2 + 22 \tau_{2,10} \tau_{3,10} l_8^2 + 8 \tau_{2,7} \tau_{3,16} l_8^2 + 12 \tau_{2,10} \tau_{3,16} l_8^2 - 10 \tau_{3,10} \tau_{3,16} l_8^2 + 4 \tau_{2,7} \tau_{4,7} l_8^2 + \\
& 22 \tau_{3,10} \tau_{4,7} l_8^2 + 12 \tau_{3,16} \tau_{4,7} l_8^2 + 14 \tau_{2,12} \tau_{4,12} l_8^2 + 14 \tau_{3,7} \tau_{4,12} l_8^2 + 24 \tau_{2,7} \tau_{4,13} l_8^2 + 22 \tau_{2,10} \tau_{4,13} l_8^2 + \\
& 20 \tau_{3,10} \tau_{4,13} l_8^2 + 14 \tau_{3,16} \tau_{4,13} l_8^2 + 22 \tau_{4,7} \tau_{4,13} l_8^2 - 4 \tau_{2,7} \tau_{4,17} l_8^2 - 12 \tau_{2,12} \tau_{4,17} l_8^2 - 12 \tau_{3,7} \tau_{4,17} l_8^2 + \\
& 2 \tau_{4,12} \tau_{4,17} l_8^2 + 4 \tau_{1,12}^2 l_{11}^2 + 4 \tau_{1,13}^2 l_{11}^2 + 4 \tau_{2,9}^2 l_{11}^2 + 4 \tau_{2,10}^2 l_{11}^2 + 2 \tau_{2,12}^2 l_{11}^2 + 4 \tau_{2,13}^2 l_{11}^2 + 4 \tau_{3,5}^2 l_{11}^2 + \\
& 4 \tau_{3,6}^2 l_{11}^2 + 4 \tau_{3,7}^2 l_{11}^2 + 2 \tau_{3,8}^2 l_{11}^2 + 4 \tau_{4,5}^2 l_{11}^2 + 2 \tau_{4,6}^2 l_{11}^2 + 4 \tau_{4,7}^2 l_{11}^2 + 4 \tau_{4,8}^2 l_{11}^2 + 3 \tau_{4,13}^2 l_{11}^2 - \\
& 2 \tau_{2,10} \tau_{2,12} l_{11}^2 + 5 \tau_{1,12} \tau_{3,5} l_{11}^2 + 5 \tau_{1,13} \tau_{3,6} l_{11}^2 - 5 \tau_{2,13} \tau_{3,6} l_{11}^2 - 5 \tau_{2,10} \tau_{3,7} l_{11}^2 + 3 \tau_{2,12} \tau_{3,7} l_{11}^2 - 3 \tau_{1,13} \tau_{3,8} l_{11}^2 + \\
& 3 \tau_{2,13} \tau_{3,8} l_{11}^2 - 2 \tau_{3,6} \tau_{3,8} l_{11}^2 + 5 \tau_{2,10} \tau_{4,7} l_{11}^2 - 3 \tau_{2,12} \tau_{4,7} l_{11}^2 - 2 \tau_{4,6} \tau_{4,8} l_{11}^2 + 3 \tau_{1,13} \tau_{4,13} l_{11}^2 + 5 \tau_{2,13} \tau_{4,13} l_{11}^2 - \\
& 3 \tau_{3,6} \tau_{4,13} l_{11}^2 - \tau_{3,8} \tau_{4,13} l_{11}^2 + \tau_{4,5} (2(4 \tau_{1,5} + 7 \tau_{3,10} - 6 \tau_{3,14}) l_6^2 + 2 \tau_{4,13} (7 l_6^2 - 3 \tau_{5,9}) + (3 \tau_{1,10} - 5 \tau_{1,12}) l_{11}^2) + \\
& \tau_{3,9} (-2(3 \tau_{4,5} \tau_{5,9} + \tau_{4,13} (\tau_{5,9} - \tau_{5,13} - \tau_{7,9} + \tau_{7,13}))) + \\
& 2(3 \tau_{2,13} \tau_{5,13} - 3 \tau_{4,7} \tau_{7,9} + 3(\tau_{1,13} - \tau_{3,7}) \tau_{7,13} + (12 \tau_{1,5} + 11 \tau_{1,12} + 10 \tau_{4,12} - 7 \tau_{4,15}) l_6^2 + \\
& \tau_{3,5} (11 l_6^2 - 3 \tau_{5,13}) + (12 \tau_{2,7} + 7 \tau_{2,12}) l_8^2 + (7 \tau_{3,7} + 14 \tau_{4,12} - 11 \tau_{4,17}) l_8^2) - (\tau_{4,6} + 3 \tau_{4,8}) l_{11}^2) + \\
& \tau_{2,9} (6(\tau_{3,9} + \tau_{4,13}) \tau_{5,9} + 2(11 \tau_{1,8} - 6 \tau_{1,16} + 2 \tau_{4,9}) l_{10}^2 + (3 \tau_{3,9} - 3 \tau_{4,6} + 5 \tau_{4,8}) l_{11}^2) + \\
& \tau_{3,9}^2 (2 \tau_{5,9} - 2 \tau_{5,13} + 4 \tau_{7,9} - 4 \tau_{7,13} + 3(l_6^2 + l_8^2) + l_{11}^2) + \\
& 2(\tau_{2,6}^2 + (11 \tau_{3,6} - 5 \tau_{2,15}) \tau_{2,6} + (7 \tau_{1,8} + 6 \tau_{1,17}) (\tau_{2,13} + \tau_{3,8}) + \tau_{1,13} (11 \tau_{2,6} + 6 \tau_{2,15} + 2 \tau_{3,13}) + \\
& \tau_{2,15} (6 \tau_{3,6} + 4 \tau_{3,13}) + 2 \tau_{3,13} (\tau_{1,17} + 2 \tau_{2,13} + \tau_{3,6} + 2(\tau_{3,8} + \tau_{3,13}))) l_{12}^2 + \\
& \tau_{2,5} (6(\tau_{4,5} - \tau_{1,13}) \tau_{5,13} + 6 \tau_{3,7} \tau_{7,9} + 6(\tau_{4,7} - \tau_{2,13}) \tau_{7,13} + 2(10 \tau_{1,8} - 7 \tau_{1,16} + 11 \tau_{4,8} + 12 \tau_{4,9}) l_{10}^2 + \\
& \tau_{2,9} (22 l_{10}^2 - 6 \tau_{7,9}) - (\tau_{1,10} + 3 \tau_{1,12}) l_{11}^2 + 5 \tau_{4,5} l_{11}^2 + 3 \tau_{3,5} (2 \tau_{5,9} + l_{11}^2) + \\
& 2(14 \tau_{1,8} + 11 \tau_{1,17}) l_{12}^2 + 2(7(\tau_{2,13} + \tau_{3,8}) + 12 \tau_{3,13}) l_{12}^2) + \\
& \tau_{2,5}^2 (2 \tau_{5,9} + 4 \tau_{5,13} - 2 \tau_{7,9} - 4 \tau_{7,13} + 3(6 l_{10}^2 + l_{11}^2 + 6 l_{12}^2)) + 2((l_{10}^2 + 5 l_{12}^2) \tau_{1,8}^2 + \\
& ((5 \tau_{1,16} + 11 \tau_{4,8}) l_{10}^2 - \tau_{1,17} l_{12}^2) \tau_{1,8} + 2 \tau_{1,5} (2(\tau_{1,5} + \tau_{1,10}) + \tau_{1,12}) l_6^2 + 2 \tau_{2,7} (2 \tau_{2,7} + \tau_{2,10} + 2 \tau_{2,12}) l_8^2 + \\
& (5 \tau_{2,6}^2 - (\tau_{2,14} - 7 \tau_{4,6}) \tau_{2,6} + 2(\tau_{2,14} (3 \tau_{4,6} + \tau_{4,9}) + \tau_{4,9} (2 \tau_{4,6} + \tau_{4,8} + 2 \tau_{4,9}) - \tau_{1,16} (3 \tau_{4,8} + 2 \tau_{4,9}))) l_{10}^2)) \\
& t + 2(t^2 + u^2) \tau_{1,7}^4 + 2 \tau_{1,7}^3 (2 \tau_{2,5} (t - u)^2 - s t \tau_{1,9} - s u \tau_{1,13} + s(t(\tau_{2,9} + \tau_{3,5} - \tau_{3,7}) + u(\tau_{2,13} + \tau_{4,5} - \tau_{4,7}))) + \\
& u^2 (2 \tau_{2,5}^4 + 2(\tau_{2,9} + \tau_{3,5} - \tau_{3,7}) \tau_{2,5}^3 + (\tau_{3,5}^2 + (\tau_{2,9} - \tau_{3,7})^2 + \tau_{4,5}^2 + (\tau_{2,13} - \tau_{4,7})^2) \tau_{2,5}^2 + \\
& (\tau_{3,9} + \tau_{4,13})^2 (\tau_{2,9}^2 + 2(\tau_{3,9} - \tau_{4,5}) \tau_{2,9} + (\tau_{2,13} - \tau_{3,5})^2 + \tau_{3,7}^2 + \tau_{4,5}^2 + \tau_{4,7}^2 + \\
& 2 \tau_{4,13}^2 + 2 \tau_{3,9} (-\tau_{2,13} + \tau_{3,5} + \tau_{3,9}) - 2 \tau_{3,9} \tau_{4,5} + 2(\tau_{4,7} - \tau_{3,7}) \tau_{4,13}) + \\
& \tau_{1,13}^2 (\tau_{2,5}^2 + (\tau_{3,9} + \tau_{4,13})^2) - 2 \tau_{1,13} (\tau_{4,5} \tau_{2,5}^2 + (\tau_{3,7} - \tau_{4,13}) (\tau_{3,9} + \tau_{4,13})^2)) +
\end{aligned}$$

$$\begin{aligned}
& (s^2 - t^2 - u^2) \left( (\tau_{2,9} + \tau_{2,13} + \tau_{3,5} - \tau_{3,7} + \tau_{4,5} - \tau_{4,7}) \tau_{2,5}^3 + (\tau_{3,5}^2 + (\tau_{2,9} - \tau_{3,7})^2 + \tau_{4,5}^2 + (\tau_{2,13} - \tau_{4,7})^2) \tau_{2,5}^2 + \right. \\
& (\tau_{3,9} + \tau_{4,13})^2 (\tau_{2,9}^2 + (\tau_{3,9} - 2\tau_{4,5} - \tau_{4,13}) \tau_{2,9} + (\tau_{2,13} - \tau_{3,5})^2 + \tau_{3,7}^2 + \tau_{4,5}^2 + \tau_{4,7}^2 - \tau_{2,13} \tau_{3,9} + \\
& \tau_{3,5} \tau_{3,9} + \tau_{3,7} \tau_{3,9} - \tau_{3,9} \tau_{4,5} - \tau_{3,9} \tau_{4,7} + (\tau_{2,13} - \tau_{3,5} - \tau_{3,7} - 4\tau_{3,9} + \tau_{4,5} + \tau_{4,7}) \tau_{4,13}) + \\
& \left. \tau_{1,13}^2 (\tau_{2,5}^2 + (\tau_{3,9} + \tau_{4,13})^2) - \tau_{1,13} (\tau_{2,5}^3 + 2\tau_{4,5} \tau_{2,5}^2 + (2\tau_{3,7} + \tau_{3,9} - \tau_{4,13}) (\tau_{3,9} + \tau_{4,13})^2) \right) - \\
& s \tau_{1,9}^2 (2(-s^2 + t^2 + u^2) l_{11}^2 - s(\tau_{2,5}^2 + (\tau_{3,9} + \tau_{4,13})^2)) + \\
& \frac{1}{2} \tau_{1,9} (((7t^3 + 3ut^2 + 5u^2t + u^3 - s^2(5t + 3u)) \tau_{3,9} + (t^3 + 5ut^2 + 3u^2t + 7u^3 - s^2(3t + 5u)) \tau_{4,6} - \\
& (7t^3 + 3ut^2 + 5u^2t + u^3 - s^2(5t + 3u)) \tau_{4,8}) l_{11}^2 - 4s(-u\tau_{2,5}^3 + s\tau_{3,5} \tau_{2,5}^2 + s^2 \tau_{5,9} \tau_{2,5} + \\
& (\tau_{3,9} + \tau_{4,13}) ((\tau_{3,9} + \tau_{4,13}) (t \tau_{3,9} + s \tau_{4,7} - u \tau_{4,13}) - s^2 \tau_{7,9}) + s((t + 5u) \tau_{2,6} - 2s \tau_{2,14} + 2t \tau_{4,9}) l_{10}^2)) + \\
& u^2 (s^2 - t^2 - u^2) (4\tau_{5,9}^2 + 4\tau_{5,13}^2 + 4\tau_{7,9}^2 + 4\tau_{7,13}^2 - l_6^2 (6\tau_{9,15} + 5(2\tau_{13,14} + l_8^2)) + \\
& 2((3\tau_{13,16} - 5\tau_{9,17}) l_8^2 + (5\tau_{7,14} - 3\tau_{5,16}) l_{10}^2 + (-\tau_{5,10} + \tau_{5,12} - \tau_{6,9} + \tau_{6,13} + \tau_{7,10} - \tau_{7,12} + \tau_{8,9} - \tau_{8,13}) l_{11}^2) + \\
& (10\tau_{5,17} + 6\tau_{7,15} - 5l_{10}^2) l_{12}^2) + \\
& u^4 (2\tau_{5,9}^2 + 2\tau_{5,13}^2 + 2\tau_{7,9}^2 + 2\tau_{7,13}^2 + 2(\tau_{13,16} - 3\tau_{9,17}) l_8^2 - 2l_6^2 (\tau_{9,15} + 3\tau_{13,14} + 2l_8^2) + \\
& (-\tau_{5,10} + \tau_{5,12} - \tau_{6,9} + \tau_{6,13} + \tau_{7,10} - \tau_{7,12} + \tau_{8,9} - \tau_{8,13}) l_{11}^2 + 2(3\tau_{5,17} + \tau_{7,15}) l_{12}^2 - 2l_{10}^2 (\tau_{5,16} - 3\tau_{7,14} + 2l_{12}^2)) - \\
& u^3 (-2l_{11}^2 \tau_{1,10}^2 + 10\tau_{3,10} l_6^2 \tau_{1,10} - 4\tau_{3,14} l_6^2 \tau_{1,10} + 10\tau_{4,13} l_6^2 \tau_{1,10} - 2\tau_{1,12} l_{11}^2 \tau_{1,10} + \tau_{3,5} l_{11}^2 \tau_{1,10} + \\
& 2\tau_{2,13} \tau_{4,13} \tau_{5,13} - 2\tau_{3,5} \tau_{4,13} \tau_{5,13} - 2\tau_{4,13}^2 \tau_{7,9} - 2\tau_{4,7} \tau_{4,13} \tau_{7,9} + 2\tau_{4,13}^2 \tau_{7,13} + 2\tau_{1,13} \tau_{4,13} \tau_{7,13} - \\
& 2\tau_{3,7} \tau_{4,13} \tau_{7,13} - 6\tau_{3,10}^2 l_6^2 + 2\tau_{4,12}^2 l_6^2 + 2\tau_{4,13}^2 l_6^2 + 4\tau_{1,5} \tau_{1,12} l_6^2 + 4\tau_{1,5} \tau_{3,5} l_6^2 + 4\tau_{1,5} \tau_{3,10} l_6^2 - 4\tau_{1,5} \tau_{3,14} l_6^2 + \\
& 6\tau_{3,10} \tau_{3,14} l_6^2 + 4\tau_{1,5} \tau_{4,12} l_6^2 + 2\tau_{1,12} \tau_{4,12} l_6^2 + 2\tau_{3,5} \tau_{4,12} l_6^2 + 12\tau_{1,5} \tau_{4,13} l_6^2 - 4\tau_{3,10} \tau_{4,13} l_6^2 - 2\tau_{3,14} \tau_{4,13} l_6^2 - \\
& 4\tau_{1,12} \tau_{4,15} l_6^2 - 4\tau_{3,5} \tau_{4,15} l_6^2 - 2\tau_{4,12} \tau_{4,15} l_6^2 + 2\tau_{3,10}^2 l_8^2 - 6\tau_{4,12}^2 l_8^2 + 2\tau_{4,13}^2 l_8^2 + 4\tau_{2,7} \tau_{2,10} l_8^2 + 4\tau_{2,7} \tau_{3,10} l_8^2 + \\
& 2\tau_{2,10} \tau_{3,10} l_8^2 + 4\tau_{2,10} \tau_{3,16} l_8^2 + 2\tau_{3,10} \tau_{3,16} l_8^2 + 4\tau_{2,7} \tau_{4,7} l_8^2 + 2\tau_{3,10} \tau_{4,7} l_8^2 + 4\tau_{3,16} \tau_{4,7} l_8^2 + 4\tau_{2,7} \tau_{4,12} l_8^2 + \\
& 10\tau_{2,12} \tau_{4,12} l_8^2 + 10\tau_{3,7} \tau_{4,12} l_8^2 + 12\tau_{2,7} \tau_{4,13} l_8^2 + 2\tau_{2,10} \tau_{4,13} l_8^2 + 4\tau_{3,10} \tau_{4,13} l_8^2 + 10\tau_{3,16} \tau_{4,13} l_8^2 + \\
& 2\tau_{4,7} \tau_{4,13} l_8^2 - 4\tau_{2,7} \tau_{4,17} l_8^2 - 4\tau_{2,12} \tau_{4,17} l_8^2 - 4\tau_{3,7} \tau_{4,17} l_8^2 + 6\tau_{4,12} \tau_{4,17} l_8^2 + 2\tau_{1,8} (\tau_{1,8} - \tau_{1,16}) l_{10}^2 + \\
& 2(-3\tau_{2,6}^2 + (-3\tau_{2,14} + 5\tau_{4,6} + 2\tau_{4,9}) \tau_{2,6} + (\tau_{1,8} - 2\tau_{1,16}) \tau_{4,8} + 2(\tau_{1,8} + \tau_{4,8}) \tau_{4,9} + 2\tau_{2,14} (\tau_{4,6} + \tau_{4,9})) l_{10}^2 + \\
& \tau_{3,9}^2 (2(\tau_{5,9} - \tau_{5,13} + l_6^2 + l_8^2) - l_{11}^2) - 2\tau_{2,12}^2 l_{11}^2 - 2\tau_{3,8}^2 l_{11}^2 - 2\tau_{4,6}^2 l_{11}^2 - \tau_{4,13}^2 l_{11}^2 - 2\tau_{2,10} \tau_{2,12} l_{11}^2 + \\
& \tau_{1,12} \tau_{3,5} l_{11}^2 + \tau_{1,13} \tau_{3,6} l_{11}^2 - \tau_{2,13} \tau_{3,6} l_{11}^2 - \tau_{2,10} \tau_{3,7} l_{11}^2 - \tau_{2,12} \tau_{3,7} l_{11}^2 + \tau_{1,13} \tau_{3,8} l_{11}^2 - \tau_{2,13} \tau_{3,8} l_{11}^2 - \\
& 2\tau_{3,6} \tau_{3,8} l_{11}^2 + \tau_{2,10} \tau_{4,7} l_{11}^2 + \tau_{2,12} \tau_{4,7} l_{11}^2 - 2\tau_{4,6} \tau_{4,8} l_{11}^2 - \tau_{1,13} \tau_{4,13} l_{11}^2 + \tau_{2,13} \tau_{4,13} l_{11}^2 + \\
& \tau_{3,6} \tau_{4,13} l_{11}^2 + 3\tau_{3,8} \tau_{4,13} l_{11}^2 - \tau_{4,5} (2\tau_{4,13} (\tau_{5,9} - 5l_6^2) + 2(2\tau_{3,14} - 5\tau_{3,10}) l_6^2 + (\tau_{1,10} + \tau_{1,12}) l_{11}^2) + \\
& \tau_{2,9} (2(\tau_{3,9} + \tau_{4,13}) \tau_{5,9} + 2(\tau_{1,8} - 2\tau_{1,16} + 2\tau_{4,9}) l_{10}^2 + (-\tau_{3,9} + \tau_{4,6} + \tau_{4,8}) l_{11}^2) + \\
& \tau_{3,9} (-2(\tau_{4,5} \tau_{5,9} + \tau_{4,13} (-\tau_{5,9} + \tau_{5,13} + \tau_{7,9} - \tau_{7,13}))) + \\
& 2(\tau_{2,13} \tau_{5,13} - \tau_{4,7} \tau_{7,9} + (\tau_{1,13} - \tau_{3,7}) \tau_{7,13} + (6\tau_{1,5} + \tau_{1,12} + 2\tau_{4,12} - 5\tau_{4,15}) l_6^2 + \\
& \tau_{3,5} (l_6^2 - \tau_{5,13}) + (6\tau_{2,7} + 5\tau_{2,12}) l_8^2 + (5\tau_{3,7} - 2\tau_{4,12} - \tau_{4,17}) l_8^2) + (3\tau_{4,6} + \tau_{4,8}) l_{11}^2) - \\
& 6\tau_{1,8} (\tau_{1,8} + \tau_{1,17}) l_{12}^2 + 2(\tau_{2,6}^2 + (\tau_{2,15} + \tau_{3,6} + 2\tau_{3,13}) \tau_{2,6} + 2\tau_{2,15} \tau_{3,6} + (5\tau_{1,8} + 2\tau_{1,17}) (\tau_{2,13} + \tau_{3,8}) + \\
& 2(\tau_{1,8} + \tau_{1,17} + \tau_{3,6}) \tau_{3,13} + \tau_{1,13} (\tau_{2,6} + 2(\tau_{2,15} + \tau_{3,13}))) l_{12}^2 + \tau_{2,5}^2 (2\tau_{5,9} - 2\tau_{7,9} + 2l_{10}^2 - l_{11}^2 + 2l_{12}^2) +
\end{aligned}$$

$$\begin{aligned}
& \tau_{2,5} (2 (\tau_{4,5} - \tau_{1,13}) \tau_{5,13} + 2 \tau_{3,7} \tau_{7,9} + 2 \tau_{4,7} \tau_{7,13} + 2 (2 \tau_{1,8} - 5 \tau_{1,16} + \tau_{4,8} + 6 \tau_{4,9}) l_{10}^2 + 2 \tau_{2,9} (l_{10}^2 - \tau_{7,9}) + \tau_{3,5} \\
& \quad (2 \tau_{5,9} - l_{11}^2) + (3 \tau_{1,10} + \tau_{1,12}) l_{11}^2 + \tau_{4,5} l_{11}^2 - 2 \tau_{2,13} (\tau_{7,13} - 5 l_{12}^2) + 2 (-2 \tau_{1,8} + \tau_{1,17} + 5 \tau_{3,8} + 6 \tau_{3,13}) l_{12}^2) + \\
& \frac{1}{2} \tau_{1,7} (4 \tau_{3,5} \tau_{5,9} s^3 + 4 \tau_{1,9}^2 \tau_{2,5} s^2 + 4 \tau_{1,13}^2 \tau_{2,5} s^2 + 4 \tau_{2,5} (\tau_{3,5}^2 + (\tau_{2,9} - \tau_{3,7})^2 + \tau_{4,5}^2 + \\
& \quad (\tau_{2,13} - \tau_{4,7})^2 + (t - u) (\tau_{5,9} - \tau_{5,13} - \tau_{7,9} + \tau_{7,13})) s^2 + \\
& \quad 4 \tau_{2,5}^2 ((t - 2u) \tau_{2,9} + (u - 2t) \tau_{2,13} + (t - 2u) \tau_{3,5} - (t - 2u) \tau_{3,7} - (2t - u) (\tau_{4,5} - \tau_{4,7})) s - \\
& \quad 4 \tau_{1,9} ((t - 2u) \tau_{2,5}^2 + 2s \tau_{3,5} \tau_{2,5} + s (s \tau_{5,9} + (t + 5u) l_{10}^2)) s - \\
& \quad 4 ((-6s^2 + 8t^2 + 4u^2) \tau_{2,6} + s(t + 5u) \tau_{2,15} + s(5t + u) \tau_{3,6} - 3(s^2 + t^2 + u^2) \tau_{3,13}) l_{12}^2 s - \\
& \quad 4 \tau_{1,13} ((u - 2t) \tau_{2,5}^2 + 2s \tau_{4,5} \tau_{2,5} + s(s \tau_{5,13} + (5t + u) l_{12}^2)) s + 8(t - u)^2 \tau_{2,5}^3 - 4t^3 \tau_{4,5} \tau_{5,13} - \\
& \quad 4u^3 \tau_{4,5} \tau_{5,13} + 6t(-s^2 + t^2 + u^2) \tau_{4,5} \tau_{5,13} + 6u(-s^2 + t^2 + u^2) \tau_{4,5} \tau_{5,13} + 4t^3 \tau_{2,9} \tau_{7,9} + 4u^3 \tau_{2,9} \tau_{7,9} - \\
& \quad 6t(-s^2 + t^2 + u^2) \tau_{2,9} \tau_{7,9} - 6u(-s^2 + t^2 + u^2) \tau_{2,9} \tau_{7,9} - 4t^3 \tau_{3,7} \tau_{7,9} - 4u^3 \tau_{3,7} \tau_{7,9} + 6t(-s^2 + t^2 + u^2) \tau_{3,7} \tau_{7,9} + \\
& \quad 6u(-s^2 + t^2 + u^2) \tau_{3,7} \tau_{7,9} + 4t^3 \tau_{2,13} \tau_{7,13} + 4u^3 \tau_{2,13} \tau_{7,13} - 6t(-s^2 + t^2 + u^2) \tau_{2,13} \tau_{7,13} - \\
& \quad 6u(-s^2 + t^2 + u^2) \tau_{2,13} \tau_{7,13} - 4t^3 \tau_{4,7} \tau_{7,13} - 4u^3 \tau_{4,7} \tau_{7,13} + 6t(-s^2 + t^2 + u^2) \tau_{4,7} \tau_{7,13} + \\
& \quad 6u(-s^2 + t^2 + u^2) \tau_{4,7} \tau_{7,13} - 8t^3 \tau_{2,6} l_{10}^2 + 8u^3 \tau_{2,6} l_{10}^2 + 28t(-s^2 + t^2 + u^2) \tau_{2,6} l_{10}^2 + 20u(-s^2 + t^2 + u^2) \tau_{2,6} l_{10}^2 - \\
& \quad 20t^3 \tau_{2,14} l_{10}^2 - 4u^3 \tau_{2,14} l_{10}^2 + 22t(-s^2 + t^2 + u^2) \tau_{2,14} l_{10}^2 + 14u(-s^2 + t^2 + u^2) \tau_{2,14} l_{10}^2 - \\
& \quad 4t^3 \tau_{4,6} l_{10}^2 - 20u^3 \tau_{4,6} l_{10}^2 + 14t(-s^2 + t^2 + u^2) \tau_{4,6} l_{10}^2 + 22u(-s^2 + t^2 + u^2) \tau_{4,6} l_{10}^2 - 24t^3 \tau_{4,9} l_{10}^2 - \\
& \quad 24u^3 \tau_{4,9} l_{10}^2 + 24t(-s^2 + t^2 + u^2) \tau_{4,9} l_{10}^2 + 24u(-s^2 + t^2 + u^2) \tau_{4,9} l_{10}^2 - 6t^3 \tau_{2,10} l_{11}^2 - \\
& \quad 2u^3 \tau_{2,10} l_{11}^2 - 3t(-s^2 + t^2 + u^2) \tau_{2,10} l_{11}^2 - u(-s^2 + t^2 + u^2) \tau_{2,10} l_{11}^2 - 2t^3 \tau_{2,12} l_{11}^2 - 6u^3 \tau_{2,12} l_{11}^2 - \\
& \quad t(-s^2 + t^2 + u^2) \tau_{2,12} l_{11}^2 - 3u(-s^2 + t^2 + u^2) \tau_{2,12} l_{11}^2 + 2t^3 \tau_{3,7} l_{11}^2 - 2u^3 \tau_{3,7} l_{11}^2 + 5t(-s^2 + t^2 + u^2) \tau_{3,7} l_{11}^2 + \\
& \quad 3u(-s^2 + t^2 + u^2) \tau_{3,7} l_{11}^2 - 2t^3 \tau_{4,7} l_{11}^2 + 2u^3 \tau_{4,7} l_{11}^2 + 3t(-s^2 + t^2 + u^2) \tau_{4,7} l_{11}^2 + 5u(-s^2 + t^2 + u^2) \tau_{4,7} l_{11}^2) - \\
& \frac{1}{2} u (s^2 - t^2 - u^2) (4 l_{11}^2 \tau_{1,10}^2 + 22 \tau_{3,10} l_6^2 \tau_{1,10} - 12 \tau_{3,14} l_6^2 \tau_{1,10} + 22 \tau_{4,13} l_6^2 \tau_{1,10} - 2 \tau_{1,12} l_{11}^2 \tau_{1,10} - \\
& \quad 5 \tau_{3,5} l_{11}^2 \tau_{1,10} - 2 \tau_{4,13}^2 \tau_{5,9} + 2 \tau_{4,13}^2 \tau_{5,13} + 6 \tau_{2,13} \tau_{4,13} \tau_{5,13} - 6 \tau_{3,5} \tau_{4,13} \tau_{5,13} - 4 \tau_{4,13}^2 \tau_{7,9} - \\
& \quad 6 \tau_{4,7} \tau_{4,13} \tau_{7,9} + 4 \tau_{4,13}^2 \tau_{7,13} + 6 \tau_{1,13} \tau_{4,13} \tau_{7,13} - 6 \tau_{3,7} \tau_{4,13} \tau_{7,13} + 2 \tau_{3,10}^2 l_6^2 + 10 \tau_{4,12}^2 l_6^2 + \\
& \quad 18 \tau_{4,13}^2 l_6^2 + 8 \tau_{1,5} \tau_{3,5} l_6^2 - 8 \tau_{1,5} \tau_{3,14} l_6^2 + 10 \tau_{3,10} \tau_{3,14} l_6^2 + 14 \tau_{1,12} \tau_{4,12} l_6^2 + 14 \tau_{3,5} \tau_{4,12} l_6^2 + \\
& \quad 24 \tau_{1,5} \tau_{4,13} l_6^2 + 20 \tau_{3,10} \tau_{4,13} l_6^2 - 14 \tau_{3,14} \tau_{4,13} l_6^2 - 4 \tau_{1,5} \tau_{4,15} l_6^2 - 12 \tau_{1,12} \tau_{4,15} l_6^2 - 12 \tau_{3,5} \tau_{4,15} l_6^2 + \\
& \quad 2 \tau_{4,12} \tau_{4,15} l_6^2 + 10 \tau_{3,10}^2 l_8^2 + 2 \tau_{4,12}^2 l_8^2 + 18 \tau_{4,13}^2 l_8^2 + 4 \tau_{2,7} \tau_{3,7} l_8^2 + 14 \tau_{2,10} \tau_{3,10} l_8^2 + 4 \tau_{2,7} \tau_{3,16} l_8^2 + \\
& \quad 12 \tau_{2,10} \tau_{3,16} l_8^2 - 2 \tau_{3,10} \tau_{3,16} l_8^2 + 8 \tau_{2,7} \tau_{4,7} l_8^2 + 14 \tau_{3,10} \tau_{4,7} l_8^2 + 12 \tau_{3,16} \tau_{4,7} l_8^2 + 22 \tau_{2,12} \tau_{4,12} l_8^2 + \\
& \quad 22 \tau_{3,7} \tau_{4,12} l_8^2 + 24 \tau_{2,7} \tau_{4,13} l_8^2 + 14 \tau_{2,10} \tau_{4,13} l_8^2 + 28 \tau_{3,10} \tau_{4,13} l_8^2 + 22 \tau_{3,16} \tau_{4,13} l_8^2 + 14 \tau_{4,7} \tau_{4,13} l_8^2 - \\
& \quad 8 \tau_{2,7} \tau_{4,17} l_8^2 - 12 \tau_{2,12} \tau_{4,17} l_8^2 - 12 \tau_{3,7} \tau_{4,17} l_8^2 + 10 \tau_{4,12} \tau_{4,17} l_8^2 + 2 \tau_{1,12}^2 l_{11}^2 + 4 \tau_{1,13}^2 l_{11}^2 + 4 \tau_{2,9}^2 l_{11}^2 + \\
& \quad 2 \tau_{2,10}^2 l_{11}^2 + 4 \tau_{2,12}^2 l_{11}^2 + 4 \tau_{2,13}^2 l_{11}^2 + 4 \tau_{3,5}^2 l_{11}^2 + 2 \tau_{3,6}^2 l_{11}^2 + 4 \tau_{3,7}^2 l_{11}^2 + 4 \tau_{3,8}^2 l_{11}^2 + 4 \tau_{4,5}^2 l_{11}^2 + \\
& \quad 4 \tau_{4,6}^2 l_{11}^2 + 4 \tau_{4,7}^2 l_{11}^2 + 2 \tau_{4,8}^2 l_{11}^2 + 3 \tau_{4,13}^2 l_{11}^2 - 2 \tau_{2,10} \tau_{2,12} l_{11}^2 + 3 \tau_{1,12} \tau_{3,5} l_{11}^2 + 3 \tau_{1,13} \tau_{3,6} l_{11}^2 - \\
& \quad 3 \tau_{2,13} \tau_{3,6} l_{11}^2 - 3 \tau_{2,10} \tau_{3,7} l_{11}^2 + 5 \tau_{2,12} \tau_{3,7} l_{11}^2 - 5 \tau_{1,13} \tau_{3,8} l_{11}^2 + 5 \tau_{2,13} \tau_{3,8} l_{11}^2 - 2 \tau_{3,6} \tau_{3,8} l_{11}^2 +
\end{aligned}$$

$$\begin{aligned}
& 3 \tau_{2,10} \tau_{4,7} l_{11}^2 - 5 \tau_{2,12} \tau_{4,7} l_{11}^2 - 2 \tau_{4,6} \tau_{4,8} l_{11}^2 + 5 \tau_{1,13} \tau_{4,13} l_{11}^2 + 3 \tau_{2,13} \tau_{4,13} l_{11}^2 - \tau_{3,6} \tau_{4,13} l_{11}^2 - \\
& 3 \tau_{3,8} \tau_{4,13} l_{11}^2 + \tau_{4,5} (2 (2 \tau_{1,5} + 11 \tau_{3,10} - 6 \tau_{3,14}) l_6^2 + \tau_{4,13} (22 l_6^2 - 6 \tau_{5,9}) + (5 \tau_{1,10} - 3 \tau_{1,12}) l_{11}^2) + \\
& \tau_{3,9} (-2 (3 \tau_{4,5} \tau_{5,9} + \tau_{4,13} (-\tau_{5,9} + \tau_{5,13} + \tau_{7,9} - \tau_{7,13})) + \\
& 2 (3 \tau_{2,13} \tau_{5,13} - 3 \tau_{4,7} \tau_{7,9} + 3 (\tau_{1,13} - \tau_{3,7}) \tau_{7,13} + (12 \tau_{1,5} + 7 \tau_{1,12} + 14 \tau_{4,12} - 11 \tau_{4,15}) l_6^2 + \\
& \tau_{3,5} (7 l_6^2 - 3 \tau_{5,13}) + (12 \tau_{2,7} + 11 \tau_{2,12}) l_8^2 + (11 \tau_{3,7} + 10 \tau_{4,12} - 7 \tau_{4,17}) l_8^2) - (3 \tau_{4,6} + \tau_{4,8}) l_{11}^2) + \\
& \tau_{2,9} (6 (\tau_{3,9} + \tau_{4,13}) \tau_{5,9} + 2 (7 \tau_{1,8} - 6 \tau_{1,16} + 4 \tau_{4,9}) l_{10}^2 + (5 \tau_{3,9} - 5 \tau_{4,6} + 3 \tau_{4,8}) l_{11}^2) + \\
& \tau_{3,9}^2 (4 \tau_{5,9} - 4 \tau_{5,13} + 2 \tau_{7,9} - 2 \tau_{7,13} + 3 (6 (l_6^2 + l_8^2) + l_{11}^2)) + \\
& 2 (5 \tau_{2,6}^2 - (\tau_{2,15} - 7 \tau_{3,6}) \tau_{2,6} + 4 \tau_{3,13}^2 + 6 \tau_{2,15} \tau_{3,6} + (11 \tau_{1,8} + 6 \tau_{1,17}) (\tau_{2,13} + \tau_{3,8}) + \\
& 2 (2 \tau_{1,17} + \tau_{2,13} + \tau_{2,15} + 2 \tau_{3,6} + \tau_{3,8}) \tau_{3,13} + \tau_{1,13} (7 \tau_{2,6} + 6 \tau_{2,15} + 4 \tau_{3,13})) l_{12}^2 + \\
& \tau_{2,5} (6 (\tau_{4,5} - \tau_{1,13}) \tau_{5,13} + 6 \tau_{3,7} \tau_{7,9} + 6 (\tau_{4,7} - \tau_{2,13}) \tau_{7,13} + 2 (14 \tau_{1,8} - 11 \tau_{1,16} + 7 \tau_{4,8} + 12 \tau_{4,9}) l_{10}^2 + \\
& 2 \tau_{2,9} (7 l_{10}^2 - 3 \tau_{7,9}) - (3 \tau_{1,10} + \tau_{1,12}) l_{11}^2 + 3 \tau_{4,5} l_{11}^2 + \tau_{3,5} (6 \tau_{5,9} + 5 l_{11}^2) + 2 (10 \tau_{1,8} + 7 \tau_{1,17}) l_{12}^2 + \\
& 2 (11 (\tau_{2,13} + \tau_{3,8}) + 12 \tau_{3,13}) l_{12}^2) + \tau_{2,5}^2 (4 \tau_{5,9} + 2 \tau_{5,13} - 4 \tau_{7,9} - 2 \tau_{7,13} + 3 (6 l_{10}^2 + l_{11}^2 + 6 l_{12}^2)) + \\
& 2 ((5 l_{10}^2 + l_{12}^2) \tau_{1,8}^2 + ((\tau_{1,16} + 7 \tau_{4,8}) l_{10}^2 - 5 \tau_{1,17} l_{12}^2) \tau_{1,8} + 2 \tau_{1,5} (2 \tau_{1,5} + \tau_{1,10} + 2 \tau_{1,12}) l_6^2 + \\
& 2 \tau_{2,7} (2 (\tau_{2,7} + \tau_{2,10}) + \tau_{2,12}) l_8^2 + (\tau_{2,6}^2 + (11 \tau_{4,6} - 5 \tau_{2,14}) \tau_{2,6} - \\
& 2 \tau_{1,16} (3 \tau_{4,8} + \tau_{4,9}) + \tau_{2,14} (6 \tau_{4,6} + 4 \tau_{4,9}) + 2 \tau_{4,9} (\tau_{4,6} + 2 (\tau_{4,8} + \tau_{4,9}))) l_{10}^2) + \\
& \tau_{1,7}^2 (s^2 \tau_{1,9}^2 - 2 s ((2 t - u) \tau_{2,5} + s \tau_{3,5}) \tau_{1,9} + s^2 \tau_{1,13}^2 + 4 (3 (t^2 + u^2) - 2 s^2) \tau_{2,5}^2 + 2 s \tau_{1,13} ((t - 2 u) \tau_{2,5} - s \tau_{4,5}) + \\
& 2 s \tau_{2,5} ((2 t - u) \tau_{2,9} - (t - 2 u) \tau_{2,13} + (2 t - u) \tau_{3,5} + (u - 2 t) \tau_{3,7} - (t - 2 u) (\tau_{4,5} - \tau_{4,7})) - \\
& s ((2 \tau_{5,9} - 2 \tau_{7,9} - 2 l_{10}^2 + l_{11}^2 - 2 l_{12}^2) t^2 + (\tau_{3,5}^2 + (\tau_{2,9} - \tau_{3,7})^2 + \tau_{4,5}^2 + (\tau_{2,13} - \tau_{4,7})^2) t + \\
& u (\tau_{3,5}^2 + (\tau_{2,9} - \tau_{3,7})^2 + \tau_{4,5}^2 + (\tau_{2,13} - \tau_{4,7})^2) + u^2 (2 \tau_{5,13} - 2 \tau_{7,13} - 2 l_{10}^2 + l_{11}^2 - 2 l_{12}^2) + \\
& (s^2 - t^2 - u^2) (\tau_{5,9} + \tau_{5,13} - \tau_{7,9} - \tau_{7,13} - 2 (4 l_{10}^2 + l_{11}^2 + 4 l_{12}^2))))))
\end{aligned}$$

■  $N_{47}^{(5)}$

$$\begin{aligned}
& \frac{1}{8} \left( - (4 \tau_{1,5} \tau_{9,15} l_6^2 + 4 \tau_{3,5} \tau_{9,15} l_6^2 + 2 \tau_{3,9} \tau_{9,15} l_6^2 - 6 \tau_{4,12} \tau_{9,15} l_6^2 + 4 \tau_{1,10} \tau_{13,14} l_6^2 + 2 \tau_{3,10} \tau_{13,14} l_6^2 + 4 \tau_{4,5} \tau_{13,14} l_6^2 + \right. \\
& 10 \tau_{4,13} \tau_{13,14} l_6^2 - 3 \tau_{1,9} l_8^2 l_6^2 + 3 \tau_{1,10} l_8^2 l_6^2 - 2 \tau_{1,13} l_8^2 l_6^2 - \tau_{1,14} l_8^2 l_6^2 - 5 \tau_{1,15} l_8^2 l_6^2 - 3 \tau_{1,16} l_8^2 l_6^2 + \\
& 7 \tau_{1,17} l_8^2 l_6^2 - 2 \tau_{2,9} l_8^2 l_6^2 + 7 \tau_{2,10} l_8^2 l_6^2 + 3 \tau_{2,12} l_8^2 l_6^2 - 3 \tau_{2,13} l_8^2 l_6^2 + 7 \tau_{2,14} l_8^2 l_6^2 + 3 \tau_{2,15} l_8^2 l_6^2 + 5 \tau_{2,16} l_8^2 l_6^2 - \\
& \tau_{2,17} l_8^2 l_6^2 - 2 \tau_{3,14} l_8^2 l_6^2 - 4 \tau_{3,15} l_8^2 l_6^2 - 3 \tau_{3,16} l_8^2 l_6^2 + 5 \tau_{3,17} l_8^2 l_6^2 + 5 \tau_{4,14} l_8^2 l_6^2 + 3 \tau_{4,15} l_8^2 l_6^2 + 4 \tau_{4,16} l_8^2 l_6^2 - \\
& 2 \tau_{4,17} l_8^2 l_6^2 + \tau_{1,12} (4 \tau_{9,15} + 7 l_8^2) l_6^2 + \tau_{1,7} l_{11}^2 l_6^2 + 2 \tau_{1,9} l_{11}^2 l_6^2 + \tau_{3,7} l_{11}^2 l_6^2 - \tau_{3,9} l_{11}^2 l_6^2 - \tau_{4,7} l_{11}^2 l_6^2 + \\
& 5 \tau_{4,13} l_{11}^2 l_6^2 + 4 (\tau_{2,12} + \tau_{3,7}) \tau_{9,17} l_8^2 + 10 \tau_{3,9} \tau_{9,17} l_8^2 + 2 \tau_{4,12} \tau_{9,17} l_8^2 - 4 \tau_{2,7} \tau_{13,16} l_8^2 - 4 \tau_{2,10} \tau_{13,16} l_8^2 + \\
& 6 \tau_{3,10} \tau_{13,16} l_8^2 - 4 \tau_{4,7} \tau_{13,16} l_8^2 - 2 \tau_{4,13} \tau_{13,16} l_8^2 + 2 (\tau_{2,5} - 3 \tau_{1,8}) \tau_{5,16} l_{10}^2 + 4 \tau_{2,9} \tau_{5,16} l_{10}^2 + 4 \tau_{4,8} \tau_{5,16} l_{10}^2 + \\
& 4 \tau_{4,9} \tau_{5,16} l_{10}^2 - 10 \tau_{1,7} \tau_{7,14} l_{10}^2 - 4 \tau_{1,9} \tau_{7,14} l_{10}^2 - 2 \tau_{2,6} \tau_{7,14} l_{10}^2 - 4 \tau_{4,6} \tau_{7,14} l_{10}^2 + \tau_{2,5} l_8^2 l_{11}^2 + 2 \tau_{2,13} l_8^2 l_{11}^2 - \\
& \tau_{3,5} l_8^2 l_{11}^2 + 5 \tau_{3,9} l_8^2 l_{11}^2 + \tau_{4,5} l_8^2 l_{11}^2 - \tau_{4,13} l_8^2 l_{11}^2 + 5 \tau_{1,7} l_{10}^2 l_{11}^2 - \tau_{1,13} l_{10}^2 l_{11}^2 - \tau_{2,5} l_{10}^2 l_{11}^2 + \tau_{2,13} l_{10}^2 l_{11}^2 +
\end{aligned}$$

$$\begin{aligned}
& 2 \tau_{4,5} l_{10}^2 l_{11}^2 + \tau_{4,13} l_{10}^2 l_{11}^2 - 2 \tau_{1,8} \tau_{5,17} l_{12}^2 - (4 (\tau_{2,13} + \tau_{3,8}) \tau_{5,17} + 2 (2 \tau_{1,13} - 3 \tau_{2,6} + 2 (\tau_{3,6} + \tau_{3,13})) \tau_{7,15} + \\
& (5 \tau_{1,14} - 4 \tau_{1,15} - 3 \tau_{1,16} - 2 \tau_{1,17} - 2 \tau_{2,14} + 3 \tau_{2,15} + 4 \tau_{2,16} + 5 \tau_{2,17} + 2 \tau_{3,5}) l_{10}^2 + (3 \tau_{3,7} - 7 \tau_{3,6}) l_{10}^2 - \\
& (3 \tau_{3,8} - 7 \tau_{3,14} + 5 \tau_{3,15} + 3 \tau_{3,16} + \tau_{3,17} - 3 \tau_{4,5} + 3 \tau_{4,6} - 2 \tau_{4,7} + 7 \tau_{4,8} + \tau_{4,14} - 3 \tau_{4,15} - 5 \tau_{4,16} - 7 \tau_{4,17}) \\
& l_{10}^2 + 5 \tau_{2,5} (2 \tau_{5,17} - l_{11}^2) - \tau_{1,9} l_{11}^2 + (\tau_{2,9} - 2 \tau_{3,7} - \tau_{3,9}) l_{11}^2 + \tau_{1,7} (2 \tau_{7,15} + l_{11}^2) l_{12}^2) t^3 + \\
& (2 l_6^2 \tau_{1,5}^3 + 4 (\tau_{1,12} + \tau_{3,5} - \tau_{3,9} - \tau_{4,12}) l_6^2 \tau_{1,5}^2 + (2 \tau_{1,10}^2 + 4 (\tau_{3,10} + \tau_{4,5} + \tau_{4,13}) \tau_{1,10} + 2 \tau_{1,12}^2 + \\
& 2 \tau_{3,5}^2 - \tau_{3,9}^2 + 3 \tau_{3,10}^2 + 2 \tau_{4,5}^2 + 3 \tau_{4,12}^2 - \tau_{4,13}^2 + 6 \tau_{3,9} \tau_{4,12} - 8 \tau_{3,5} (\tau_{3,9} + \tau_{4,12}) + \\
& 4 \tau_{1,12} (\tau_{3,5} - 2 (\tau_{3,9} + \tau_{4,12})) + 4 \tau_{4,5} \tau_{4,13} + \tau_{3,10} (4 \tau_{4,5} + 6 \tau_{4,13})) l_6^2 \tau_{1,5} - \\
& 4 \tau_{1,12}^2 (\tau_{3,9} + \tau_{4,12}) l_6^2 - 2 \tau_{1,12} (4 \tau_{3,5} + \tau_{3,9} - 3 \tau_{4,12}) (\tau_{3,9} + \tau_{4,12}) l_6^2 - \\
& 2 (\tau_{3,5} (2 \tau_{3,5} + \tau_{3,9} - 3 \tau_{4,12}) (\tau_{3,9} + \tau_{4,12}) + (\tau_{3,10} + \tau_{4,13}) (\tau_{1,10} + \tau_{3,10} + \tau_{4,5} + \tau_{4,13}) \\
& (2 \tau_{1,10} + \tau_{3,10} + 2 \tau_{4,5} + 5 \tau_{4,13})) l_6^2 + 2 \tau_{2,7} ((\tau_{2,7} + \tau_{2,10})^2 + (\tau_{2,12} + \tau_{3,7})^2) l_8^2 - \\
& (4 (\tau_{3,10} - \tau_{4,7} + \tau_{4,13}) \tau_{2,7}^2 + (-3 \tau_{3,10}^2 + (8 \tau_{4,7} - 6 \tau_{4,13}) \tau_{3,10} - 2 \tau_{4,7}^2 - 3 \tau_{4,12}^2 + \tau_{4,13}^2 + \tau_{3,9} \\
& (\tau_{3,9} - 4 (\tau_{2,12} + \tau_{3,7})) - 2 (2 (\tau_{2,12} + \tau_{3,7}) + 3 \tau_{3,9}) \tau_{4,12} + 8 \tau_{4,7} \tau_{4,13} + \tau_{2,10} (8 \tau_{3,10} - 4 \tau_{4,7} + 8 \tau_{4,13})) \\
& \tau_{2,7} + 2 ((\tau_{3,9} + \tau_{4,12}) (\tau_{2,12} + \tau_{3,7} + \tau_{3,9} + \tau_{4,12}) (2 \tau_{2,12} + 2 \tau_{3,7} + 5 \tau_{3,9} + \tau_{4,12}) + \\
& (\tau_{2,10} + \tau_{4,7}) (\tau_{3,10} + \tau_{4,13}) (2 \tau_{2,10} - 3 \tau_{3,10} + 2 \tau_{4,7} + \tau_{4,13}))) l_8^2 - \\
& 10 \tau_{1,7}^3 l_{10}^2 - 2 \tau_{2,6}^3 l_{10}^2 + 2 \tau_{4,9}^3 l_{10}^2 - 4 \tau_{1,8} \tau_{2,9}^2 l_{10}^2 - 4 \tau_{2,5} \tau_{2,9}^2 l_{10}^2 - 4 \tau_{2,6} \tau_{4,6}^2 l_{10}^2 - 4 \tau_{1,8} \tau_{4,8}^2 l_{10}^2 - \\
& 4 \tau_{2,5} \tau_{4,8}^2 l_{10}^2 - 4 \tau_{1,8} \tau_{4,9}^2 l_{10}^2 - 4 \tau_{2,5} \tau_{4,9}^2 l_{10}^2 + 4 \tau_{2,9} \tau_{4,9}^2 l_{10}^2 + 4 \tau_{4,8} \tau_{4,9}^2 l_{10}^2 + \\
& 6 \tau_{1,8}^2 \tau_{2,9} l_{10}^2 - 2 \tau_{2,5}^2 \tau_{2,9} l_{10}^2 + 4 \tau_{1,8} \tau_{2,5} \tau_{2,9} l_{10}^2 - 6 \tau_{2,6}^2 \tau_{4,6} l_{10}^2 + 6 \tau_{1,8}^2 \tau_{4,8} l_{10}^2 - \\
& 2 \tau_{2,5}^2 \tau_{4,8} l_{10}^2 + 4 \tau_{1,8} \tau_{2,5} \tau_{4,8} l_{10}^2 - 8 \tau_{1,8} \tau_{2,9} \tau_{4,8} l_{10}^2 - 8 \tau_{2,5} \tau_{2,9} \tau_{4,8} l_{10}^2 + \\
& 3 \tau_{1,8}^2 \tau_{4,9} l_{10}^2 - \tau_{2,5}^2 \tau_{4,9} l_{10}^2 + 3 \tau_{2,6}^2 \tau_{4,9} l_{10}^2 + 2 \tau_{2,9}^2 \tau_{4,9} l_{10}^2 + 2 \tau_{4,6}^2 \tau_{4,9} l_{10}^2 + \\
& 2 \tau_{4,8}^2 \tau_{4,9} l_{10}^2 + 6 \tau_{1,8} \tau_{2,5} \tau_{4,9} l_{10}^2 - 8 \tau_{1,8} \tau_{2,9} \tau_{4,9} l_{10}^2 - 8 \tau_{2,5} \tau_{2,9} \tau_{4,9} l_{10}^2 + \\
& 4 \tau_{2,6} \tau_{4,6} \tau_{4,9} l_{10}^2 - 8 \tau_{1,8} \tau_{4,8} \tau_{4,9} l_{10}^2 - 8 \tau_{2,5} \tau_{4,8} \tau_{4,9} l_{10}^2 + 4 \tau_{2,9} \tau_{4,8} \tau_{4,9} l_{10}^2 + \\
& 2 \tau_{1,9}^2 (\tau_{4,9} - 2 \tau_{2,6}) l_{10}^2 + 2 \tau_{1,9} (2 (\tau_{2,6} + \tau_{4,6}) \tau_{4,9} - \tau_{2,6} (3 \tau_{2,6} + 4 \tau_{4,6})) l_{10}^2 - \\
& (2 \tau_{1,8}^3 + (14 \tau_{2,5} + 6 (\tau_{2,13} + \tau_{3,8}) - 3 \tau_{3,13}) \tau_{1,8}^2 + (22 \tau_{2,5}^2 + (20 (\tau_{2,13} + \tau_{3,8}) - 6 \tau_{3,13}) \tau_{2,5} + \\
& 4 (\tau_{2,13} + \tau_{3,8}) (\tau_{2,13} + \tau_{3,8} - \tau_{3,13})) \tau_{1,8} + 10 \tau_{2,5}^3 + 2 \tau_{2,6} (\tau_{1,13} + \tau_{3,6}) (2 \tau_{1,13} - 3 \tau_{2,6} + 2 \tau_{3,6}) + \\
& 4 \tau_{2,5} (\tau_{2,13} + \tau_{3,8}) (\tau_{2,13} + \tau_{3,8} - \tau_{3,13}) + \tau_{2,5}^2 (14 (\tau_{2,13} + \tau_{3,8}) + \tau_{3,13}) - \tau_{3,13} \\
& (2 \tau_{1,13}^2 + 4 (-2 \tau_{2,6} + \tau_{3,6} + \tau_{3,13}) \tau_{1,13} + 3 \tau_{2,6}^2 - 4 \tau_{2,6} (2 \tau_{3,6} + \tau_{3,13}) + 2 ((\tau_{2,13} + \tau_{3,8})^2 + (\tau_{3,6} + \tau_{3,13})^2))) \\
& l_{12}^2 + \tau_{1,7}^2 (-14 \tau_{1,9} + 22 \tau_{2,6} + 14 \tau_{4,6} + \tau_{4,9}) l_{10}^2 - (2 (\tau_{1,13} + \tau_{3,6}) + \tau_{3,13}) l_{12}^2) - \\
& 2 \tau_{1,7} (2 l_{10}^2 \tau_{1,9}^2 + 2 (5 \tau_{2,6} + 2 \tau_{4,6} - \tau_{4,9}) l_{10}^2 \tau_{1,9} + 7 \tau_{2,6}^2 l_{10}^2 + 2 \tau_{4,6} (\tau_{4,6} - \tau_{4,9}) l_{10}^2 + \\
& 2 (\tau_{1,13} + \tau_{3,6} + \tau_{3,13})^2 l_{12}^2 + \tau_{2,6} ((10 \tau_{4,6} - 3 \tau_{4,9}) l_{10}^2 - (2 (\tau_{1,13} + \tau_{3,6}) + 3 \tau_{3,13}) l_{12}^2))) t^2 + \\
& \frac{1}{2} (s^2 - t^2 - u^2) (-12 \tau_{3,5} \tau_{9,15} l_6^2 - 14 \tau_{3,9} \tau_{9,15} l_6^2 + 10 \tau_{4,12} \tau_{9,15} l_6^2 - 12 \tau_{1,10} \tau_{13,14} l_6^2 + 2 \tau_{3,10} \tau_{13,14} l_6^2 - \\
& 12 \tau_{4,5} \tau_{13,14} l_6^2 - 22 \tau_{4,13} \tau_{13,14} l_6^2 - 4 \tau_{1,5} (2 \tau_{9,15} + \tau_{13,14}) l_6^2 + 24 \tau_{1,9} l_8^2 l_6^2 + 5 \tau_{1,10} l_8^2 l_6^2 + \\
& 31 \tau_{1,13} l_8^2 l_6^2 + \tau_{1,14} l_8^2 l_6^2 + 5 \tau_{1,15} l_8^2 l_6^2 - 7 \tau_{1,16} l_8^2 l_6^2 + 3 \tau_{1,17} l_8^2 l_6^2 + 31 \tau_{2,9} l_8^2 l_6^2 - \\
& 7 \tau_{2,10} l_8^2 l_6^2 + 5 \tau_{2,12} l_8^2 l_6^2 + 24 \tau_{2,13} l_8^2 l_6^2 + 3 \tau_{2,14} l_8^2 l_6^2 + 7 \tau_{2,15} l_8^2 l_6^2 - 5 \tau_{2,16} l_8^2 l_6^2 +
\end{aligned}$$

$$\begin{aligned}
& \tau_{2,17} l_8^2 l_6^2 + 7 \tau_{3,14} l_8^2 l_6^2 + 9 \tau_{3,15} l_8^2 l_6^2 - 2 \tau_{3,16} l_8^2 l_6^2 + 2 \tau_{4,15} l_8^2 l_6^2 - 9 \tau_{4,16} l_8^2 l_6^2 + \\
& 7 \tau_{4,17} l_8^2 l_6^2 - \tau_{1,12} (12 \tau_{9,15} + 7 l_8^2) l_6^2 + 15 \tau_{1,7} l_{11}^2 l_6^2 + 16 \tau_{1,9} l_{11}^2 l_6^2 + 14 \tau_{1,13} l_{11}^2 l_6^2 + \\
& \tau_{3,7} l_{11}^2 l_6^2 + 15 \tau_{3,9} l_{11}^2 l_6^2 - \tau_{4,7} l_{11}^2 l_6^2 - 11 \tau_{4,13} l_{11}^2 l_6^2 - 22 \tau_{3,9} \tau_{9,17} l_8^2 + 2 \tau_{4,12} \tau_{9,17} l_8^2 + \\
& 8 \tau_{2,7} \tau_{13,16} l_8^2 + 12 \tau_{2,10} \tau_{13,16} l_8^2 - 10 \tau_{3,10} \tau_{13,16} l_8^2 + 12 \tau_{4,7} \tau_{13,16} l_8^2 + 14 \tau_{4,13} \tau_{13,16} l_8^2 - \\
& 12 \tau_{2,9} \tau_{5,16} l_{10}^2 - 12 \tau_{4,8} \tau_{5,16} l_{10}^2 - 8 \tau_{4,9} \tau_{5,16} l_{10}^2 + 22 \tau_{1,7} \tau_{7,14} l_{10}^2 + 12 \tau_{1,9} \tau_{7,14} l_{10}^2 - \\
& 2 \tau_{2,6} \tau_{7,14} l_{10}^2 + 12 \tau_{4,6} \tau_{7,14} l_{10}^2 + 4 \tau_{4,9} \tau_{7,14} l_{10}^2 + 15 \tau_{2,5} l_8^2 l_{11}^2 + 14 \tau_{2,9} l_8^2 l_{11}^2 + \\
& 16 \tau_{2,13} l_8^2 l_{11}^2 - \tau_{3,5} l_8^2 l_{11}^2 - 11 \tau_{3,9} l_8^2 l_{11}^2 + \tau_{4,5} l_8^2 l_{11}^2 + 15 \tau_{4,13} l_8^2 l_{11}^2 - 11 \tau_{1,7} l_{10}^2 l_{11}^2 - \\
& \tau_{1,13} l_{10}^2 l_{11}^2 + 15 \tau_{2,5} l_{10}^2 l_{11}^2 + \tau_{2,13} l_{10}^2 l_{11}^2 + 16 \tau_{4,5} l_{10}^2 l_{11}^2 + 14 \tau_{4,7} l_{10}^2 l_{11}^2 + 15 \tau_{4,13} l_{10}^2 l_{11}^2 + \\
& (4 (3 (\tau_{2,13} + \tau_{3,8}) + \tau_{3,13}) \tau_{5,17} + 2 (6 \tau_{1,13} - 5 \tau_{2,6} + 6 \tau_{3,6}) \tau_{7,15} + 8 \tau_{3,13} \tau_{7,15} + \\
& (-9 \tau_{1,15} + 2 \tau_{1,16} - 7 \tau_{1,17} - 7 \tau_{2,14} - 2 \tau_{2,15} + 9 \tau_{2,16} + 31 \tau_{3,5}) l_{10}^2 + (24 \tau_{3,7} - 7 \tau_{3,6}) l_{10}^2 + \\
& (5 \tau_{3,8} - 3 \tau_{3,14} - 5 \tau_{3,15} + 7 \tau_{3,16} - \tau_{3,17} + 24 \tau_{4,5} + 5 \tau_{4,6} + 31 \tau_{4,7} - 7 \tau_{4,8} - \tau_{4,14} - 7 \tau_{4,15} + 5 \tau_{4,16} - 3 \tau_{4,17}) \\
& l_{10}^2 + 11 \tau_{2,5} (2 \tau_{5,17} - l_{11}^2) + \tau_{1,9} l_{11}^2 + (-\tau_{2,9} + 14 \tau_{3,5} + 16 \tau_{3,7} + 15 \tau_{3,9}) l_{11}^2 + \tau_{1,7} (14 \tau_{7,15} + 15 l_{11}^2) l_{12}^2 - \\
& 2 (2 (\tau_{2,7} + 3 (\tau_{2,12} + \tau_{3,7})) \tau_{9,17} l_8^2 + (7 \tau_{2,5} - 5 \tau_{1,8}) \tau_{5,16} l_{10}^2 + \tau_{1,8} \tau_{5,17} l_{12}^2) t - \\
& u^3 (4 \tau_{3,5} \tau_{9,15} l_6^2 + 10 \tau_{3,9} \tau_{9,15} l_6^2 + 2 \tau_{4,12} \tau_{9,15} l_6^2 + 4 \tau_{1,5} \tau_{13,14} l_6^2 + 4 \tau_{1,10} \tau_{13,14} l_6^2 - 6 \tau_{3,10} \tau_{13,14} l_6^2 + \\
& 4 \tau_{4,5} \tau_{13,14} l_6^2 + 2 \tau_{4,13} \tau_{13,14} l_6^2 - 2 \tau_{1,9} l_8^2 l_6^2 + 7 \tau_{1,10} l_8^2 l_6^2 - 3 \tau_{1,13} l_8^2 l_6^2 - 5 \tau_{1,14} l_8^2 l_6^2 - \\
& \tau_{1,15} l_8^2 l_6^2 - 7 \tau_{1,16} l_8^2 l_6^2 + 3 \tau_{1,17} l_8^2 l_6^2 - 3 \tau_{2,9} l_8^2 l_6^2 + 3 \tau_{2,10} l_8^2 l_6^2 + 7 \tau_{2,12} l_8^2 l_6^2 - 2 \tau_{2,13} l_8^2 l_6^2 + \\
& 3 \tau_{2,14} l_8^2 l_6^2 + 7 \tau_{2,15} l_8^2 l_6^2 + \tau_{2,16} l_8^2 l_6^2 - 5 \tau_{2,17} l_8^2 l_6^2 + 3 \tau_{3,14} l_8^2 l_6^2 + 5 \tau_{3,15} l_8^2 l_6^2 + 2 \tau_{3,16} l_8^2 l_6^2 - \\
& 4 \tau_{3,17} l_8^2 l_6^2 - 4 \tau_{4,14} l_8^2 l_6^2 - 2 \tau_{4,15} l_8^2 l_6^2 - 5 \tau_{4,16} l_8^2 l_6^2 + 3 \tau_{4,17} l_8^2 l_6^2 + \tau_{1,12} (4 \tau_{9,15} + 3 l_8^2) l_6^2 + \\
& \tau_{1,7} l_{11}^2 l_6^2 + 2 \tau_{1,13} l_{11}^2 l_6^2 - \tau_{3,7} l_{11}^2 l_6^2 + 5 \tau_{3,9} l_{11}^2 l_6^2 + \tau_{4,7} l_{11}^2 l_6^2 - \tau_{4,13} l_{11}^2 l_6^2 + 2 \tau_{3,9} \tau_{9,17} l_8^2 - \\
& 6 \tau_{4,12} \tau_{9,17} l_8^2 - 4 \tau_{2,10} \tau_{13,16} l_8^2 - 2 \tau_{3,10} \tau_{13,16} l_8^2 - 4 \tau_{4,7} \tau_{13,16} l_8^2 - 10 \tau_{4,13} \tau_{13,16} l_8^2 + \\
& 4 \tau_{2,9} \tau_{5,16} l_{10}^2 + 4 \tau_{4,8} \tau_{5,16} l_{10}^2 - 2 \tau_{1,7} \tau_{7,14} l_{10}^2 - 4 \tau_{1,9} \tau_{7,14} l_{10}^2 + 6 \tau_{2,6} \tau_{7,14} l_{10}^2 - \\
& 4 \tau_{4,6} \tau_{7,14} l_{10}^2 - 4 \tau_{4,9} \tau_{7,14} l_{10}^2 + \tau_{2,5} l_8^2 l_{11}^2 + 2 \tau_{2,9} l_8^2 l_{11}^2 + \tau_{3,5} l_8^2 l_{11}^2 - \tau_{3,9} l_8^2 l_{11}^2 - \\
& \tau_{4,5} l_8^2 l_{11}^2 + 5 \tau_{4,13} l_8^2 l_{11}^2 - \tau_{1,7} l_{10}^2 l_{11}^2 + \tau_{1,13} l_{10}^2 l_{11}^2 + 5 \tau_{2,5} l_{10}^2 l_{11}^2 - \tau_{2,13} l_{10}^2 l_{11}^2 + \\
& 2 \tau_{4,7} l_{10}^2 l_{11}^2 + \tau_{4,13} l_{10}^2 l_{11}^2 - (4 (\tau_{2,13} + \tau_{3,8} + \tau_{3,13}) \tau_{5,17} + 2 (2 \tau_{1,13} + \tau_{2,6} + 2 \tau_{3,6}) \tau_{7,15} + \\
& (-4 \tau_{1,14} + 5 \tau_{1,15} + 2 \tau_{1,16} + 3 \tau_{1,17} + 3 \tau_{2,14} - 2 \tau_{2,15} - 5 \tau_{2,16} - 4 \tau_{2,17} + 3 \tau_{3,5}) l_{10}^2 + (2 \tau_{3,7} - 3 \tau_{3,6}) l_{10}^2 + \\
& (-7 \tau_{3,8} + 3 \tau_{3,14} - \tau_{3,15} - 7 \tau_{3,16} - 5 \tau_{3,17} + 2 \tau_{4,5} - 7 \tau_{4,6} + 3 \tau_{4,7} - 3 \tau_{4,8} - 5 \tau_{4,14} + 7 \tau_{4,15} + \tau_{4,16} + 3 \tau_{4,17}) \\
& l_{10}^2 + 5 \tau_{1,7} (2 \tau_{7,15} - l_{11}^2) - (-\tau_{1,9} + \tau_{2,9} + 2 \tau_{3,5} + \tau_{3,9}) l_{11}^2 + \tau_{2,5} (2 \tau_{5,17} + l_{11}^2) l_{12}^2 + \\
& 2 (2 (\tau_{2,7} + \tau_{2,12} + \tau_{3,7}) \tau_{9,17} l_8^2 + (\tau_{1,8} + 5 \tau_{2,5}) \tau_{5,16} l_{10}^2 + 3 \tau_{1,8} \tau_{5,17} l_{12}^2) + \\
& \frac{1}{2} u (s^2 - t^2 - u^2) (-12 \tau_{3,5} \tau_{9,15} l_6^2 - 22 \tau_{3,9} \tau_{9,15} l_6^2 + 2 \tau_{4,12} \tau_{9,15} l_6^2 - 12 \tau_{1,10} \tau_{13,14} l_6^2 + 10 \tau_{3,10} \tau_{13,14} l_6^2 - \\
& 12 \tau_{4,5} \tau_{13,14} l_6^2 - 14 \tau_{4,13} \tau_{13,14} l_6^2 - 4 \tau_{1,5} (\tau_{9,15} + 2 \tau_{13,14}) l_6^2 + 31 \tau_{1,9} l_8^2 l_6^2 - 7 \tau_{1,10} l_8^2 l_6^2 + \\
& 24 \tau_{1,13} l_8^2 l_6^2 + 5 \tau_{1,14} l_8^2 l_6^2 + \tau_{1,15} l_8^2 l_6^2 - 3 \tau_{1,16} l_8^2 l_6^2 + 7 \tau_{1,17} l_8^2 l_6^2 + 24 \tau_{2,9} l_8^2 l_6^2 + 5 \tau_{2,10} l_8^2 l_6^2 - \\
& 7 \tau_{2,12} l_8^2 l_6^2 + 31 \tau_{2,13} l_8^2 l_6^2 + 7 \tau_{2,14} l_8^2 l_6^2 + 3 \tau_{2,15} l_8^2 l_6^2 - \tau_{2,16} l_8^2 l_6^2 + 5 \tau_{2,17} l_8^2 l_6^2 + 2 \tau_{3,14} l_8^2 l_6^2 -
\end{aligned}$$

$$\begin{aligned}
& 7 \tau_{3,16} l_8^2 l_6^2 + 9 \tau_{3,17} l_8^2 l_6^2 + 9 \tau_{4,14} l_8^2 l_6^2 + 7 \tau_{4,15} l_8^2 l_6^2 + 2 \tau_{4,17} l_8^2 l_6^2 + \tau_{1,12} (5 l_8^2 - 12 \tau_{9,15}) l_6^2 + \\
& 15 \tau_{1,7} l_{11}^2 l_6^2 + 14 \tau_{1,9} l_{11}^2 l_6^2 + 16 \tau_{1,13} l_{11}^2 l_6^2 - \tau_{3,7} l_{11}^2 l_6^2 - 11 \tau_{3,9} l_{11}^2 l_6^2 + \tau_{4,7} l_{11}^2 l_6^2 + 15 \tau_{4,13} l_{11}^2 l_6^2 - \\
& 14 \tau_{3,9} \tau_{9,17} l_8^2 + 10 \tau_{4,12} \tau_{9,17} l_8^2 + 4 \tau_{2,7} \tau_{13,16} l_8^2 + 12 \tau_{2,10} \tau_{13,16} l_8^2 - 2 \tau_{3,10} \tau_{13,16} l_8^2 + \\
& 12 \tau_{4,7} \tau_{13,16} l_8^2 + 22 \tau_{4,13} \tau_{13,16} l_8^2 - 12 \tau_{2,9} \tau_{5,16} l_{10}^2 - 12 \tau_{4,8} \tau_{5,16} l_{10}^2 - 4 \tau_{4,9} \tau_{5,16} l_{10}^2 + \\
& 14 \tau_{1,7} \tau_{7,14} l_{10}^2 + 12 \tau_{1,9} \tau_{7,14} l_{10}^2 - 10 \tau_{2,6} \tau_{7,14} l_{10}^2 + 12 \tau_{4,6} \tau_{7,14} l_{10}^2 + 8 \tau_{4,9} \tau_{7,14} l_{10}^2 + \\
& 15 \tau_{2,5} l_8^2 l_{11}^2 + 16 \tau_{2,9} l_8^2 l_{11}^2 + 14 \tau_{2,13} l_8^2 l_{11}^2 + \tau_{3,5} l_8^2 l_{11}^2 + 15 \tau_{3,9} l_8^2 l_{11}^2 - \tau_{4,5} l_8^2 l_{11}^2 - 11 \tau_{4,13} l_8^2 l_{11}^2 + \\
& 15 \tau_{1,7} l_{10}^2 l_{11}^2 + \tau_{1,13} l_{10}^2 l_{11}^2 - 11 \tau_{2,5} l_{10}^2 l_{11}^2 - \tau_{2,13} l_{10}^2 l_{11}^2 + 14 \tau_{4,5} l_{10}^2 l_{11}^2 + 16 \tau_{4,7} l_{10}^2 l_{11}^2 + \\
& 15 \tau_{4,13} l_{10}^2 l_{11}^2 + (4 (3 (\tau_{2,13} + \tau_{3,8}) + 2 \tau_{3,13}) \tau_{5,17} + 2 (6 \tau_{1,13} - \tau_{2,6} + 6 \tau_{3,6}) \tau_{7,15} + 4 \tau_{3,13} \tau_{7,15} - \\
& (9 \tau_{1,14} - 7 \tau_{1,16} + 2 \tau_{1,17} + 2 \tau_{2,14} + 7 \tau_{2,15} + 9 \tau_{2,17} - 24 \tau_{3,5}) l_{10}^2 + (5 \tau_{3,6} + 31 \tau_{3,7}) l_{10}^2 - \\
& (7 \tau_{3,8} + 7 \tau_{3,14} + \tau_{3,15} - 3 \tau_{3,16} + 5 \tau_{3,17} - 31 \tau_{4,5} + 7 \tau_{4,6} - 24 \tau_{4,7} - 5 \tau_{4,8} + 5 \tau_{4,14} + 3 \tau_{4,15} - \tau_{4,16} + 7 \tau_{4,17}) \\
& l_{10}^2 + 11 \tau_{1,7} (2 \tau_{7,15} - l_{11}^2) - \tau_{1,9} l_{11}^2 + (\tau_{2,9} + 16 \tau_{3,5} + 14 \tau_{3,7} + 15 \tau_{3,9}) l_{11}^2 + \tau_{2,5} (14 \tau_{5,17} + 15 l_{11}^2)) l_{12}^2 - \\
& 2 (2 (2 \tau_{2,7} + 3 (\tau_{2,12} + \tau_{3,7})) \tau_{9,17} l_8^2 - (\tau_{1,8} - 11 \tau_{2,5}) \tau_{5,16} l_{10}^2 + 5 \tau_{1,8} \tau_{5,17} l_{12}^2)) + \\
& (s^2 - t^2 - u^2) (- (l_{10}^2 + l_{12}^2) \tau_{1,7}^3 + ((-8 \tau_{1,9} + \tau_{2,6} - 8 \tau_{4,6} - 7 \tau_{4,9}) l_{10}^2 + (-8 \tau_{1,13} + \tau_{2,6} - 8 \tau_{3,6} - 7 \tau_{3,13}) l_{12}^2) \tau_{1,7}^2 - \\
& (4 l_{10}^2 \tau_{1,9}^2 + 2 (4 (\tau_{2,6} + \tau_{4,6}) + \tau_{4,9}) l_{10}^2 \tau_{1,9} + 2 (2 \tau_{4,6} - \tau_{4,9}) (\tau_{4,6} + \tau_{4,9}) l_{10}^2 + \\
& 2 (2 (\tau_{1,13} + \tau_{3,6}) - \tau_{3,13}) (\tau_{1,13} + \tau_{3,6} + \tau_{3,13}) l_{12}^2 - 5 \tau_{2,6}^2 (l_{10}^2 + l_{12}^2) + \\
& 2 \tau_{2,6} ((4 \tau_{4,6} + 3 \tau_{4,9}) l_{10}^2 + (4 (\tau_{1,13} + \tau_{3,6}) + 3 \tau_{3,13}) l_{12}^2)) \tau_{1,7} - 4 \tau_{1,12}^2 (\tau_{3,9} + \tau_{4,12}) l_6^2 - \\
& 8 \tau_{1,12} (\tau_{3,5} + \tau_{3,9}) (\tau_{3,9} + \tau_{4,12}) l_6^2 + 2 \tau_{1,5}^2 (\tau_{1,10} + \tau_{1,12} + \tau_{3,5} + \tau_{3,9} + \tau_{3,10} + \tau_{4,5} + \tau_{4,12} + \tau_{4,13}) l_6^2 + \\
& \tau_{1,5} (2 \tau_{1,10}^2 - 2 (\tau_{3,10} - 2 \tau_{4,5} + \tau_{4,13}) \tau_{1,10} + 2 \tau_{1,12}^2 + 2 \tau_{3,5}^2 - 7 \tau_{3,9}^2 - 3 \tau_{3,10}^2 + 2 \tau_{4,5}^2 - 3 \tau_{4,12}^2 - 7 \tau_{4,13}^2 - \\
& 6 \tau_{3,9} \tau_{4,12} - 2 \tau_{3,5} (\tau_{3,9} + \tau_{4,12}) + \tau_{1,12} (4 \tau_{3,5} - 2 (\tau_{3,9} + \tau_{4,12})) - 2 \tau_{4,5} \tau_{4,13} - 2 \tau_{3,10} (\tau_{4,5} + 3 \tau_{4,13})) l_6^2 - \\
& ((\tau_{3,9} + \tau_{4,12}) (4 \tau_{3,5}^2 + 8 \tau_{3,9} \tau_{3,5} + (\tau_{3,9} - 3 \tau_{4,12}) (\tau_{3,9} + \tau_{4,12})) + \\
& (\tau_{3,10} + \tau_{4,13}) (-3 \tau_{3,10}^2 + 4 (\tau_{1,10} + \tau_{4,5})^2 + \tau_{4,13}^2 + 2 (4 \tau_{1,10} - \tau_{3,10} + 4 \tau_{4,5}) \tau_{4,13})) l_6^2 + \\
& 2 \tau_{2,7} (\tau_{2,10}^2 + (\tau_{2,12} + \tau_{3,7})^2 + \tau_{2,7} (\tau_{2,10} + \tau_{2,12} + \tau_{3,7})) l_8^2 + \\
& (2 (\tau_{3,9} + \tau_{3,10} + \tau_{4,7} + \tau_{4,12} + \tau_{4,13}) \tau_{2,7}^2 - (3 \tau_{3,10}^2 + 2 (\tau_{4,7} + 3 \tau_{4,13}) \tau_{3,10} - 2 \tau_{4,7}^2 + 3 \tau_{4,12}^2 + 7 \tau_{4,13}^2 + \\
& \tau_{3,9} (2 (\tau_{2,12} + \tau_{3,7}) + 7 \tau_{3,9}) + 2 (\tau_{2,12} + \tau_{3,7} + 3 \tau_{3,9}) \tau_{4,12} + 2 \tau_{4,7} \tau_{4,13} + 2 \tau_{2,10} (\tau_{3,10} - 2 \tau_{4,7} + \tau_{4,13})) \\
& \tau_{2,7} - (\tau_{3,9} + \tau_{4,12}) (4 \tau_{2,12}^2 + 8 (\tau_{3,7} + \tau_{3,9}) \tau_{2,12} + 4 \tau_{3,7}^2 + 8 \tau_{3,7} \tau_{3,9} + (\tau_{3,9} - 3 \tau_{4,12}) (\tau_{3,9} + \tau_{4,12})) - \\
& (\tau_{3,10} + \tau_{4,13}) (-3 \tau_{3,10}^2 + 4 (\tau_{2,10} + \tau_{4,7})^2 + \tau_{4,13}^2 + 2 (4 \tau_{2,10} - \tau_{3,10} + 4 \tau_{4,7}) \tau_{4,13})) l_8^2 - \\
& \tau_{2,5}^3 l_{10}^2 + 3 \tau_{2,6}^3 l_{10}^2 - 4 \tau_{2,5} \tau_{2,9}^2 l_{10}^2 - 4 \tau_{2,6} \tau_{4,6}^2 l_{10}^2 - 4 \tau_{2,5} \tau_{4,8}^2 l_{10}^2 + 2 \tau_{2,5} \tau_{4,9}^2 l_{10}^2 + 2 \tau_{2,6} \tau_{4,9}^2 l_{10}^2 + \\
& 2 \tau_{2,9} \tau_{4,9}^2 l_{10}^2 + 2 \tau_{4,6} \tau_{4,9}^2 l_{10}^2 + 2 \tau_{4,8} \tau_{4,9}^2 l_{10}^2 - 8 \tau_{2,5}^2 \tau_{2,9} l_{10}^2 - 8 \tau_{2,5}^2 \tau_{4,8} l_{10}^2 - \\
& 7 \tau_{2,5}^2 \tau_{4,9} l_{10}^2 - 3 \tau_{2,6}^2 \tau_{4,9} l_{10}^2 + 2 \tau_{2,9}^2 \tau_{4,9} l_{10}^2 + 2 \tau_{4,6}^2 \tau_{4,9} l_{10}^2 + 2 \tau_{4,8}^2 \tau_{4,9} l_{10}^2 - \\
& 2 \tau_{2,6} \tau_{4,6} \tau_{4,9} l_{10}^2 - 2 \tau_{2,5} \tau_{4,8} \tau_{4,9} l_{10}^2 + 4 \tau_{2,9} \tau_{4,8} \tau_{4,9} l_{10}^2 + 2 \tau_{1,9}^2 (\tau_{4,9} - 2 \tau_{2,6}) l_{10}^2 - \\
& 2 \tau_{2,5} \tau_{2,9} (4 \tau_{4,8} + \tau_{4,9}) l_{10}^2 + 2 \tau_{1,9} (\tau_{4,9} (2 \tau_{4,6} + \tau_{4,9}) - \tau_{2,6} (4 \tau_{4,6} + \tau_{4,9})) l_{10}^2 - \\
& (\tau_{2,5}^3 + (8 (\tau_{2,13} + \tau_{3,8}) + 7 \tau_{3,13}) \tau_{2,5}^2 + 2 (2 (\tau_{2,13} + \tau_{3,8}) - \tau_{3,13}) (\tau_{2,13} + \tau_{3,8} + \tau_{3,13}) \tau_{2,5} - \\
& 2 (\tau_{1,13} + \tau_{2,6} + \tau_{2,13} + \tau_{3,6} + \tau_{3,8}) \tau_{3,13}^2 + \tau_{2,6} (4 (\tau_{1,13} + \tau_{3,6})^2 - 3 \tau_{2,6}^2) -
\end{aligned}$$

$$\begin{aligned}
& (2 \tau_{1,13}^2 - 2 (\tau_{2,6} - 2 \tau_{3,6}) \tau_{1,13} - 3 \tau_{2,6}^2 - 2 \tau_{2,6} \tau_{3,6} + 2 (\tau_{3,6}^2 + (\tau_{2,13} + \tau_{3,8})^2)) \tau_{3,13} l_{12}^2 + 3 \tau_{1,8}^3 (l_{10}^2 + l_{12}^2) + \\
& \tau_{1,8} ((\tau_{2,5}^2 - 2 (4 (\tau_{2,9} + \tau_{4,8}) + 3 \tau_{4,9}) \tau_{2,5} - 2 (2 (\tau_{2,9} + \tau_{4,8}) - \tau_{4,9}) (\tau_{2,9} + \tau_{4,8} + \tau_{4,9})) l_{10}^2 + \\
& (\tau_{2,5}^2 - 2 (4 (\tau_{2,13} + \tau_{3,8}) + 3 \tau_{3,13}) \tau_{2,5} - 2 (2 (\tau_{2,13} + \tau_{3,8}) - \tau_{3,13}) (\tau_{2,13} + \tau_{3,8} + \tau_{3,13})) l_{12}^2) + \\
& \tau_{1,8}^2 (5 \tau_{2,5} (l_{10}^2 + l_{12}^2) - 3 (\tau_{4,9} l_{10}^2 + \tau_{3,13} l_{12}^2)) + u^2 (2 l_6^2 \tau_{1,5}^3 + 4 (\tau_{1,10} - \tau_{3,10} + \tau_{4,5} - \tau_{4,13}) l_6^2 \tau_{1,5}^2 + \\
& (2 \tau_{1,10}^2 + 4 (-2 \tau_{3,10} + \tau_{4,5} - 2 \tau_{4,13}) \tau_{1,10} + 2 \tau_{1,12}^2 + 2 \tau_{3,5}^2 - \tau_{3,9}^2 + 3 \tau_{3,10}^2 + 2 \tau_{4,5}^2 + 3 \tau_{4,12}^2 - \tau_{4,13}^2 + \\
& 6 \tau_{3,9} \tau_{4,12} + 4 \tau_{3,5} (\tau_{3,9} + \tau_{4,12}) + 4 \tau_{1,12} (\tau_{3,5} + \tau_{3,9} + \tau_{4,12}) - 8 \tau_{4,5} \tau_{4,13} + \tau_{3,10} (6 \tau_{4,13} - 8 \tau_{4,5})) l_6^2 \tau_{1,5} - \\
& 4 \tau_{1,12}^2 (\tau_{3,9} + \tau_{4,12}) l_6^2 - 2 \tau_{1,12} (\tau_{3,9} + \tau_{4,12}) (4 \tau_{3,5} + 7 \tau_{3,9} + 3 \tau_{4,12}) l_6^2 - \\
& 2 ((\tau_{3,9} + \tau_{4,12}) (\tau_{3,5} + \tau_{3,9} + \tau_{4,12}) (2 \tau_{3,5} + 5 \tau_{3,9} + \tau_{4,12}) + \\
& (\tau_{1,10} + \tau_{4,5}) (\tau_{3,10} + \tau_{4,13}) (2 \tau_{1,10} - 3 \tau_{3,10} + 2 \tau_{4,5} + \tau_{4,13})) l_6^2 + 2 \tau_{2,7} (\tau_{2,10}^2 + (\tau_{2,7} + \tau_{2,12} + \tau_{3,7})^2) l_8^2 - \\
& (4 (\tau_{3,9} + \tau_{4,12}) \tau_{2,7}^2 + (-3 \tau_{3,10}^2 - 2 (2 \tau_{4,7} + 3 \tau_{4,13}) \tau_{3,10} - 2 \tau_{4,7}^2 - 3 \tau_{4,12}^2 + \tau_{4,13}^2 + \tau_{3,9} (8 (\tau_{2,12} + \tau_{3,7}) + \tau_{3,9}) + \\
& 2 (4 (\tau_{2,12} + \tau_{3,7}) - 3 \tau_{3,9}) \tau_{4,12} - 4 \tau_{4,7} \tau_{4,13} - 4 \tau_{2,10} (\tau_{3,10} + \tau_{4,7} + \tau_{4,13})) \tau_{2,7} + \\
& 2 ((\tau_{2,12} + \tau_{3,7}) (2 \tau_{2,12} + 2 \tau_{3,7} + \tau_{3,9} - 3 \tau_{4,12}) (\tau_{3,9} + \tau_{4,12}) + (\tau_{3,10} + \tau_{4,13}) (\tau_{2,10} + \tau_{3,10} + \tau_{4,7} + \tau_{4,13}) \\
& (2 \tau_{2,10} + \tau_{3,10} + 2 \tau_{4,7} + 5 \tau_{4,13})) l_8^2 - 2 \tau_{1,8}^3 l_{10}^2 - 10 \tau_{2,5}^3 l_{10}^2 + 2 \tau_{4,9}^3 l_{10}^2 - \\
& 4 \tau_{2,6} \tau_{4,6}^2 l_{10}^2 - 4 \tau_{2,6} \tau_{4,9}^2 l_{10}^2 + 4 \tau_{4,6} \tau_{4,9}^2 l_{10}^2 + 6 \tau_{2,6}^2 \tau_{4,6} l_{10}^2 + 3 \tau_{2,6}^2 \tau_{4,9} l_{10}^2 + 2 \tau_{2,9}^2 \tau_{4,9} l_{10}^2 + \\
& 2 \tau_{4,6}^2 \tau_{4,9} l_{10}^2 + 2 \tau_{4,8}^2 \tau_{4,9} l_{10}^2 - 8 \tau_{2,6} \tau_{4,6} \tau_{4,9} l_{10}^2 + 4 \tau_{2,9} \tau_{4,8} \tau_{4,9} l_{10}^2 + \\
& 2 \tau_{1,9}^2 (\tau_{4,9} - 2 \tau_{2,6}) l_{10}^2 + 2 \tau_{1,9} (3 \tau_{2,6}^2 - 4 (\tau_{4,6} + \tau_{4,9}) \tau_{2,6} + 2 \tau_{4,9} (\tau_{4,6} + \tau_{4,9})) l_{10}^2 - \\
& 10 \tau_{1,7}^3 l_{12}^2 - 2 \tau_{2,6}^3 l_{12}^2 + 2 \tau_{3,13}^3 l_{12}^2 - 6 \tau_{1,13} \tau_{2,6}^2 l_{12}^2 - 4 \tau_{2,6} \tau_{3,6}^2 l_{12}^2 + \\
& 4 \tau_{2,13} \tau_{3,13}^2 l_{12}^2 + 4 \tau_{3,8} \tau_{3,13}^2 l_{12}^2 - 4 \tau_{1,13}^2 \tau_{2,6} l_{12}^2 - 6 \tau_{2,6}^2 \tau_{3,6} l_{12}^2 - 8 \tau_{1,13} \tau_{2,6} \tau_{3,6} l_{12}^2 + \\
& 2 \tau_{1,13}^2 \tau_{3,13} l_{12}^2 + 3 \tau_{2,6}^2 \tau_{3,13} l_{12}^2 + 2 \tau_{2,13}^2 \tau_{3,13} l_{12}^2 + 2 \tau_{3,6}^2 \tau_{3,13} l_{12}^2 + 2 \tau_{3,8}^2 \tau_{3,13} l_{12}^2 + \\
& 4 \tau_{1,13} \tau_{2,6} \tau_{3,13} l_{12}^2 + 4 \tau_{1,13} \tau_{3,6} \tau_{3,13} l_{12}^2 + 4 \tau_{2,6} \tau_{3,6} \tau_{3,13} l_{12}^2 + 4 \tau_{2,13} \tau_{3,8} \tau_{3,13} l_{12}^2 + \\
& \tau_{1,7}^2 (-(2 (\tau_{1,9} + \tau_{4,6}) + \tau_{4,9}) l_{10}^2 - (14 \tau_{1,13} + 22 \tau_{2,6} + 14 \tau_{3,6} + \tau_{3,13}) l_{12}^2) + \\
& 4 \tau_{2,5} (-l_{12}^2 (\tau_{2,13} + \tau_{3,8} + \tau_{3,13})^2 - (\tau_{2,9} + \tau_{4,8}) (\tau_{2,9} + \tau_{4,8} - \tau_{4,9}) l_{10}^2) + \\
& \tau_{2,5}^2 (-(14 (\tau_{2,9} + \tau_{4,8}) + \tau_{4,9}) l_{10}^2 - (2 (\tau_{2,13} + \tau_{3,8}) + \tau_{3,13}) l_{12}^2) + \\
& \tau_{1,8}^2 (3 (2 (\tau_{2,13} + \tau_{3,8}) + \tau_{3,13}) l_{12}^2 - (14 \tau_{2,5} + 6 (\tau_{2,9} + \tau_{4,8}) - 3 \tau_{4,9}) l_{10}^2) - \\
& 2 \tau_{1,7} (2 l_{10}^2 \tau_{1,9}^2 - 2 (\tau_{2,6} - 2 (\tau_{4,6} + \tau_{4,9})) l_{10}^2 \tau_{1,9} + 2 (\tau_{4,6} + \tau_{4,9})^2 l_{10}^2 + 7 \tau_{2,6}^2 l_{12}^2 + \\
& 2 (\tau_{1,13} + \tau_{3,6}) (\tau_{1,13} + \tau_{3,6} - \tau_{3,13}) l_{12}^2 + \tau_{2,6} ((10 (\tau_{1,13} + \tau_{3,6}) - 3 \tau_{3,13}) l_{12}^2 - (2 \tau_{4,6} + 3 \tau_{4,9}) l_{10}^2)) - \\
& 2 \tau_{1,8} (11 l_{10}^2 \tau_{2,5}^2 + ((10 (\tau_{2,9} + \tau_{4,8}) - 3 \tau_{4,9}) l_{10}^2 - (2 (\tau_{2,13} + \tau_{3,8}) + 3 \tau_{3,13}) l_{12}^2) \tau_{2,5} + \\
& 2 (\tau_{2,9} + \tau_{4,8}) (\tau_{2,9} + \tau_{4,8} - \tau_{4,9}) l_{10}^2 + 2 (\tau_{2,13} + \tau_{3,8} + \tau_{3,13})^2 l_{12}^2)) \Big)
\end{aligned}$$

■  $N_{47}^{(6)}$

$$\begin{aligned}
& \frac{1}{8} \left( 2 \tau_{9,15} l_6^2 l_8^2 t^3 - 2 \tau_{9,17} l_6^2 l_8^2 t^3 - 2 \tau_{13,14} l_6^2 l_8^2 t^3 - 2 \tau_{13,16} l_6^2 l_8^2 t^3 - 4 l_6^2 l_8^2 l_{11}^2 t^3 - 9 \tau_{1,12}^2 l_6^2 l_8^2 t^2 - 9 \tau_{1,13}^2 l_6^2 l_8^2 t^2 - \right. \\
& 3 \tau_{1,14}^2 l_6^2 l_8^2 t^2 - 3 \tau_{1,15}^2 l_6^2 l_8^2 t^2 - 3 \tau_{1,16}^2 l_6^2 l_8^2 t^2 - 3 \tau_{1,17}^2 l_6^2 l_8^2 t^2 - 9 \tau_{2,9}^2 l_6^2 l_8^2 t^2 - 9 \tau_{2,10}^2 l_6^2 l_8^2 t^2 - 3 \tau_{2,12}^2 l_6^2 l_8^2 t^2 - \\
& 3 \tau_{2,13}^2 l_6^2 l_8^2 t^2 - 3 \tau_{2,14}^2 l_6^2 l_8^2 t^2 - 3 \tau_{2,15}^2 l_6^2 l_8^2 t^2 - 3 \tau_{2,16}^2 l_6^2 l_8^2 t^2 - 3 \tau_{2,17}^2 l_6^2 l_8^2 t^2 - 2 \tau_{3,14}^2 l_6^2 l_8^2 t^2 - 2 \tau_{3,15}^2 l_6^2 l_8^2 t^2 - \\
& 2 \tau_{3,16}^2 l_6^2 l_8^2 t^2 - 2 \tau_{3,17}^2 l_6^2 l_8^2 t^2 - 2 \tau_{4,14}^2 l_6^2 l_8^2 t^2 - 2 \tau_{4,15}^2 l_6^2 l_8^2 t^2 - 2 \tau_{4,16}^2 l_6^2 l_8^2 t^2 - 2 \tau_{4,17}^2 l_6^2 l_8^2 t^2 + 8 \tau_{1,12} \tau_{1,14} l_6^2 l_8^2 t^2 + \\
& 8 \tau_{1,12} \tau_{1,15} l_6^2 l_8^2 t^2 - 6 \tau_{1,14} \tau_{1,15} l_6^2 l_8^2 t^2 + 2 \tau_{1,12} \tau_{1,16} l_6^2 l_8^2 t^2 - \tau_{1,13} \tau_{1,16} l_6^2 l_8^2 t^2 - 2 \tau_{1,12} \tau_{1,17} l_6^2 l_8^2 t^2 + \tau_{1,13} \tau_{1,17} l_6^2 l_8^2 t^2 + \\
& 6 \tau_{1,16} \tau_{1,17} l_6^2 l_8^2 t^2 - 4 \tau_{1,12} \tau_{2,9} l_6^2 l_8^2 t^2 + 3 \tau_{1,14} \tau_{2,9} l_6^2 l_8^2 t^2 + 3 \tau_{1,15} \tau_{2,9} l_6^2 l_8^2 t^2 + 8 \tau_{1,16} \tau_{2,9} l_6^2 l_8^2 t^2 - 8 \tau_{1,17} \tau_{2,9} l_6^2 l_8^2 t^2 - \\
& 4 \tau_{1,13} \tau_{2,10} l_6^2 l_8^2 t^2 - 9 \tau_{1,12} \tau_{2,12} l_6^2 l_8^2 t^2 + 3 \tau_{1,14} \tau_{2,12} l_6^2 l_8^2 t^2 + 3 \tau_{1,15} \tau_{2,12} l_6^2 l_8^2 t^2 + 3 \tau_{1,16} \tau_{2,12} l_6^2 l_8^2 t^2 - \\
& 3 \tau_{1,17} \tau_{2,12} l_6^2 l_8^2 t^2 - 2 \tau_{2,9} \tau_{2,12} l_6^2 l_8^2 t^2 - 9 \tau_{1,13} \tau_{2,13} l_6^2 l_8^2 t^2 - \tau_{1,16} \tau_{2,13} l_6^2 l_8^2 t^2 + \tau_{1,17} \tau_{2,13} l_6^2 l_8^2 t^2 - 2 \tau_{2,10} \tau_{2,13} l_6^2 l_8^2 t^2 - \\
& 8 \tau_{1,13} \tau_{2,14} l_6^2 l_8^2 t^2 + \tau_{2,9} \tau_{2,14} l_6^2 l_8^2 t^2 - 2 \tau_{2,10} \tau_{2,14} l_6^2 l_8^2 t^2 + \tau_{2,12} \tau_{2,14} l_6^2 l_8^2 t^2 - 2 \tau_{2,13} \tau_{2,14} l_6^2 l_8^2 t^2 - 8 \tau_{1,13} \tau_{2,15} l_6^2 l_8^2 t^2 + \\
& \tau_{2,9} \tau_{2,15} l_6^2 l_8^2 t^2 - 2 \tau_{2,10} \tau_{2,15} l_6^2 l_8^2 t^2 + \tau_{2,12} \tau_{2,15} l_6^2 l_8^2 t^2 - 2 \tau_{2,13} \tau_{2,15} l_6^2 l_8^2 t^2 - 6 \tau_{2,14} \tau_{2,15} l_6^2 l_8^2 t^2 - 3 \tau_{1,13} \tau_{2,16} l_6^2 l_8^2 t^2 - \\
& 8 \tau_{2,10} \tau_{2,16} l_6^2 l_8^2 t^2 + \tau_{2,12} \tau_{2,16} l_6^2 l_8^2 t^2 - 3 \tau_{2,13} \tau_{2,16} l_6^2 l_8^2 t^2 + 3 \tau_{1,13} \tau_{2,17} l_6^2 l_8^2 t^2 + 8 \tau_{2,10} \tau_{2,17} l_6^2 l_8^2 t^2 - \tau_{2,12} \tau_{2,17} l_6^2 l_8^2 t^2 + \\
& 3 \tau_{2,13} \tau_{2,17} l_6^2 l_8^2 t^2 + 6 \tau_{2,16} \tau_{2,17} l_6^2 l_8^2 t^2 + 8 \tau_{1,12} \tau_{3,14} l_6^2 l_8^2 t^2 - 5 \tau_{1,14} \tau_{3,14} l_6^2 l_8^2 t^2 - 5 \tau_{1,15} \tau_{3,14} l_6^2 l_8^2 t^2 + 3 \tau_{2,9} \tau_{3,14} l_6^2 l_8^2 t^2 + \\
& 3 \tau_{2,12} \tau_{3,14} l_6^2 l_8^2 t^2 + \tau_{2,14} \tau_{3,14} l_6^2 l_8^2 t^2 + \tau_{2,15} \tau_{3,14} l_6^2 l_8^2 t^2 + 8 \tau_{1,12} \tau_{3,15} l_6^2 l_8^2 t^2 - 5 \tau_{1,14} \tau_{3,15} l_6^2 l_8^2 t^2 - 5 \tau_{1,15} \tau_{3,15} l_6^2 l_8^2 t^2 + \\
& 3 \tau_{2,9} \tau_{3,15} l_6^2 l_8^2 t^2 + 3 \tau_{2,12} \tau_{3,15} l_6^2 l_8^2 t^2 + \tau_{2,14} \tau_{3,15} l_6^2 l_8^2 t^2 + \tau_{2,15} \tau_{3,15} l_6^2 l_8^2 t^2 - 4 \tau_{3,14} \tau_{3,15} l_6^2 l_8^2 t^2 + 3 \tau_{1,12} \tau_{3,16} l_6^2 l_8^2 t^2 - \\
& 5 \tau_{1,16} \tau_{3,16} l_6^2 l_8^2 t^2 + 5 \tau_{1,17} \tau_{3,16} l_6^2 l_8^2 t^2 + 8 \tau_{2,9} \tau_{3,16} l_6^2 l_8^2 t^2 + 4 \tau_{2,12} \tau_{3,16} l_6^2 l_8^2 t^2 + \tau_{2,16} \tau_{3,16} l_6^2 l_8^2 t^2 - \tau_{2,17} \tau_{3,16} l_6^2 l_8^2 t^2 - \\
& 3 \tau_{1,12} \tau_{3,17} l_6^2 l_8^2 t^2 + 5 \tau_{1,16} \tau_{3,17} l_6^2 l_8^2 t^2 - 5 \tau_{1,17} \tau_{3,17} l_6^2 l_8^2 t^2 - 8 \tau_{2,9} \tau_{3,17} l_6^2 l_8^2 t^2 - 4 \tau_{2,12} \tau_{3,17} l_6^2 l_8^2 t^2 - \tau_{2,16} \tau_{3,17} l_6^2 l_8^2 t^2 + \\
& \tau_{2,17} \tau_{3,17} l_6^2 l_8^2 t^2 + 4 \tau_{3,16} \tau_{3,17} l_6^2 l_8^2 t^2 - 8 \tau_{1,13} \tau_{4,14} l_6^2 l_8^2 t^2 + \tau_{1,14} \tau_{4,14} l_6^2 l_8^2 t^2 + \tau_{1,15} \tau_{4,14} l_6^2 l_8^2 t^2 - 3 \tau_{2,10} \tau_{4,14} l_6^2 l_8^2 t^2 - \\
& 3 \tau_{2,13} \tau_{4,14} l_6^2 l_8^2 t^2 - 5 \tau_{2,14} \tau_{4,14} l_6^2 l_8^2 t^2 - 5 \tau_{2,15} \tau_{4,14} l_6^2 l_8^2 t^2 - 8 \tau_{1,13} \tau_{4,15} l_6^2 l_8^2 t^2 + \tau_{1,14} \tau_{4,15} l_6^2 l_8^2 t^2 + \tau_{1,15} \tau_{4,15} l_6^2 l_8^2 t^2 - \\
& 3 \tau_{2,10} \tau_{4,15} l_6^2 l_8^2 t^2 - 3 \tau_{2,13} \tau_{4,15} l_6^2 l_8^2 t^2 - 5 \tau_{2,14} \tau_{4,15} l_6^2 l_8^2 t^2 - 5 \tau_{2,15} \tau_{4,15} l_6^2 l_8^2 t^2 - 4 \tau_{4,14} \tau_{4,15} l_6^2 l_8^2 t^2 - \\
& 3 \tau_{1,13} \tau_{4,16} l_6^2 l_8^2 t^2 + \tau_{1,16} \tau_{4,16} l_6^2 l_8^2 t^2 - \tau_{1,17} \tau_{4,16} l_6^2 l_8^2 t^2 - 8 \tau_{2,10} \tau_{4,16} l_6^2 l_8^2 t^2 - 4 \tau_{2,13} \tau_{4,16} l_6^2 l_8^2 t^2 - 5 \tau_{2,16} \tau_{4,16} l_6^2 l_8^2 t^2 + \\
& 5 \tau_{2,17} \tau_{4,16} l_6^2 l_8^2 t^2 + 3 \tau_{1,13} \tau_{4,17} l_6^2 l_8^2 t^2 - \tau_{1,16} \tau_{4,17} l_6^2 l_8^2 t^2 + \tau_{1,17} \tau_{4,17} l_6^2 l_8^2 t^2 + 8 \tau_{2,10} \tau_{4,17} l_6^2 l_8^2 t^2 + 4 \tau_{2,13} \tau_{4,17} l_6^2 l_8^2 t^2 + \\
& 5 \tau_{2,16} \tau_{4,17} l_6^2 l_8^2 t^2 - 5 \tau_{2,17} \tau_{4,17} l_6^2 l_8^2 t^2 + 4 \tau_{4,16} \tau_{4,17} l_6^2 l_8^2 t^2 - (-s^2 + t^2 + u^2) \tau_{9,15} l_6^2 l_8^2 t + (-s^2 + t^2 + u^2) \tau_{9,17} l_6^2 l_8^2 t + \\
& (-s^2 + t^2 + u^2) \tau_{13,14} l_6^2 l_8^2 t + (-s^2 + t^2 + u^2) \tau_{13,16} l_6^2 l_8^2 t + 34 (-s^2 + t^2 + u^2) l_6^2 l_8^2 l_{11}^2 t + (2s^2 - 5t^2 - 11u^2) \tau_{1,9}^2 l_6^2 l_8^2 + \\
& (2s^2 - 5t^2 - 11u^2) \tau_{1,10}^2 l_6^2 l_8^2 - 3u^2 \tau_{1,12}^2 l_6^2 l_8^2 + 2(s^2 - t^2 - u^2) \tau_{1,12}^2 l_6^2 l_8^2 - 3u^2 \tau_{1,13}^2 l_6^2 l_8^2 + 2(s^2 - t^2 - u^2) \tau_{1,13}^2 l_6^2 l_8^2 - \\
& 3u^2 \tau_{1,14}^2 l_6^2 l_8^2 + (s^2 - t^2 - u^2) \tau_{1,14}^2 l_6^2 l_8^2 - 3u^2 \tau_{1,15}^2 l_6^2 l_8^2 + (s^2 - t^2 - u^2) \tau_{1,15}^2 l_6^2 l_8^2 - 3u^2 \tau_{1,16}^2 l_6^2 l_8^2 + \\
& (s^2 - t^2 - u^2) \tau_{1,16}^2 l_6^2 l_8^2 - 3u^2 \tau_{1,17}^2 l_6^2 l_8^2 + (s^2 - t^2 - u^2) \tau_{1,17}^2 l_6^2 l_8^2 - 3u^2 \tau_{2,9}^2 l_6^2 l_8^2 + 2(s^2 - t^2 - u^2) \tau_{2,9}^2 l_6^2 l_8^2 - \\
& 3u^2 \tau_{2,10}^2 l_6^2 l_8^2 + 2(s^2 - t^2 - u^2) \tau_{2,10}^2 l_6^2 l_8^2 - 9u^2 \tau_{2,12}^2 l_6^2 l_8^2 + 2(s^2 - t^2 - u^2) \tau_{2,12}^2 l_6^2 l_8^2 - 9u^2 \tau_{2,13}^2 l_6^2 l_8^2 + \\
& 2(s^2 - t^2 - u^2) \tau_{2,13}^2 l_6^2 l_8^2 - 3u^2 \tau_{2,14}^2 l_6^2 l_8^2 + (s^2 - t^2 - u^2) \tau_{2,14}^2 l_6^2 l_8^2 - 3u^2 \tau_{2,15}^2 l_6^2 l_8^2 + (s^2 - t^2 - u^2) \tau_{2,15}^2 l_6^2 l_8^2 - \\
& 3u^2 \tau_{2,16}^2 l_6^2 l_8^2 + (s^2 - t^2 - u^2) \tau_{2,16}^2 l_6^2 l_8^2 - 3u^2 \tau_{2,17}^2 l_6^2 l_8^2 + (s^2 - t^2 - u^2) \tau_{2,17}^2 l_6^2 l_8^2 - 2u^2 \tau_{3,14}^2 l_6^2 l_8^2 + \\
& 2(-s^2 + t^2 + u^2) \tau_{3,14}^2 l_6^2 l_8^2 - 2u^2 \tau_{3,15}^2 l_6^2 l_8^2 + 2(-s^2 + t^2 + u^2) \tau_{3,15}^2 l_6^2 l_8^2 - 2u^2 \tau_{3,16}^2 l_6^2 l_8^2 + 2(-s^2 + t^2 + u^2) \tau_{3,16}^2 l_6^2 l_8^2 - \\
& 2u^2 \tau_{3,17}^2 l_6^2 l_8^2 + 2(-s^2 + t^2 + u^2) \tau_{3,17}^2 l_6^2 l_8^2 - 2u^2 \tau_{4,14}^2 l_6^2 l_8^2 + 2(-s^2 + t^2 + u^2) \tau_{4,14}^2 l_6^2 l_8^2 - 2u^2 \tau_{4,15}^2 l_6^2 l_8^2 + \\
& 2(-s^2 + t^2 + u^2) \tau_{4,15}^2 l_6^2 l_8^2 - 2u^2 \tau_{4,16}^2 l_6^2 l_8^2 + 2(-s^2 + t^2 + u^2) \tau_{4,16}^2 l_6^2 l_8^2 - 2u^2 \tau_{4,17}^2 l_6^2 l_8^2 + 2(-s^2 + t^2 + u^2) \tau_{4,17}^2 l_6^2 l_8^2 -
\end{aligned}$$

$$\begin{aligned}
& u^2 \tau_{1,12} \tau_{1,14} l_6^2 l_8^2 - \frac{5}{2} (s^2 - t^2 - u^2) \tau_{1,12} \tau_{1,14} l_6^2 l_8^2 + 3 u^2 \tau_{1,13} \tau_{1,14} l_6^2 l_8^2 - \frac{9}{2} (s^2 - t^2 - u^2) \tau_{1,13} \tau_{1,14} l_6^2 l_8^2 - \\
& u^2 \tau_{1,12} \tau_{1,15} l_6^2 l_8^2 - \frac{5}{2} (s^2 - t^2 - u^2) \tau_{1,12} \tau_{1,15} l_6^2 l_8^2 + 3 u^2 \tau_{1,13} \tau_{1,15} l_6^2 l_8^2 - \frac{9}{2} (s^2 - t^2 - u^2) \tau_{1,13} \tau_{1,15} l_6^2 l_8^2 - \\
& 6 u^2 \tau_{1,14} \tau_{1,15} l_6^2 l_8^2 + 2 (s^2 - t^2 - u^2) \tau_{1,14} \tau_{1,15} l_6^2 l_8^2 - u^2 \tau_{1,12} \tau_{1,16} l_6^2 l_8^2 - \frac{3}{2} (s^2 - t^2 - u^2) \tau_{1,12} \tau_{1,16} l_6^2 l_8^2 + \\
& 2 u^2 \tau_{1,13} \tau_{1,16} l_6^2 l_8^2 - \frac{3}{2} (s^2 - t^2 - u^2) \tau_{1,13} \tau_{1,16} l_6^2 l_8^2 + u^2 \tau_{1,12} \tau_{1,17} l_6^2 l_8^2 + \frac{3}{2} (s^2 - t^2 - u^2) \tau_{1,12} \tau_{1,17} l_6^2 l_8^2 - \\
& 2 u^2 \tau_{1,13} \tau_{1,17} l_6^2 l_8^2 + \frac{3}{2} (s^2 - t^2 - u^2) \tau_{1,13} \tau_{1,17} l_6^2 l_8^2 + 6 u^2 \tau_{1,16} \tau_{1,17} l_6^2 l_8^2 + 2 (-s^2 + t^2 + u^2) \tau_{1,16} \tau_{1,17} l_6^2 l_8^2 + \\
& 2 u^2 \tau_{1,12} \tau_{2,9} l_6^2 l_8^2 + 11 (s^2 - t^2 - u^2) \tau_{1,12} \tau_{2,9} l_6^2 l_8^2 - \frac{3}{2} (s^2 - t^2 - u^2) \tau_{1,14} \tau_{2,9} l_6^2 l_8^2 - \frac{3}{2} (s^2 - t^2 - u^2) \tau_{1,15} \tau_{2,9} l_6^2 l_8^2 - \\
& u^2 \tau_{1,16} \tau_{2,9} l_6^2 l_8^2 - \frac{5}{2} (s^2 - t^2 - u^2) \tau_{1,16} \tau_{2,9} l_6^2 l_8^2 + u^2 \tau_{1,17} \tau_{2,9} l_6^2 l_8^2 + \frac{5}{2} (s^2 - t^2 - u^2) \tau_{1,17} \tau_{2,9} l_6^2 l_8^2 + 2 u^2 \tau_{1,13} \tau_{2,10} l_6^2 l_8^2 + \\
& 11 (s^2 - t^2 - u^2) \tau_{1,13} \tau_{2,10} l_6^2 l_8^2 + 3 u^2 \tau_{1,14} \tau_{2,10} l_6^2 l_8^2 - \frac{3}{2} (s^2 - t^2 - u^2) \tau_{1,14} \tau_{2,10} l_6^2 l_8^2 + 3 u^2 \tau_{1,15} \tau_{2,10} l_6^2 l_8^2 - \\
& \frac{3}{2} (s^2 - t^2 - u^2) \tau_{1,15} \tau_{2,10} l_6^2 l_8^2 + 3 u^2 \tau_{1,16} \tau_{2,10} l_6^2 l_8^2 - \frac{9}{2} (s^2 - t^2 - u^2) \tau_{1,16} \tau_{2,10} l_6^2 l_8^2 - 3 u^2 \tau_{1,17} \tau_{2,10} l_6^2 l_8^2 + \\
& \frac{9}{2} (s^2 - t^2 - u^2) \tau_{1,17} \tau_{2,10} l_6^2 l_8^2 - 9 u^2 \tau_{1,12} \tau_{2,12} l_6^2 l_8^2 + 3 (s^2 - t^2 - u^2) \tau_{1,12} \tau_{2,12} l_6^2 l_8^2 - \frac{3}{2} (s^2 - t^2 - u^2) \tau_{1,14} \tau_{2,12} l_6^2 l_8^2 - \\
& \frac{3}{2} (s^2 - t^2 - u^2) \tau_{1,15} \tau_{2,12} l_6^2 l_8^2 - \frac{9}{2} (s^2 - t^2 - u^2) \tau_{1,16} \tau_{2,12} l_6^2 l_8^2 + \frac{9}{2} (s^2 - t^2 - u^2) \tau_{1,17} \tau_{2,12} l_6^2 l_8^2 - 2 u^2 \tau_{2,9} \tau_{2,12} l_6^2 l_8^2 + \\
& 14 (s^2 - t^2 - u^2) \tau_{2,9} \tau_{2,12} l_6^2 l_8^2 - 9 u^2 \tau_{1,13} \tau_{2,13} l_6^2 l_8^2 + 3 (s^2 - t^2 - u^2) \tau_{1,13} \tau_{2,13} l_6^2 l_8^2 + 3 u^2 \tau_{1,14} \tau_{2,13} l_6^2 l_8^2 - \\
& \frac{3}{2} (s^2 - t^2 - u^2) \tau_{1,14} \tau_{2,13} l_6^2 l_8^2 + 3 u^2 \tau_{1,15} \tau_{2,13} l_6^2 l_8^2 - \frac{3}{2} (s^2 - t^2 - u^2) \tau_{1,15} \tau_{2,13} l_6^2 l_8^2 + 8 u^2 \tau_{1,16} \tau_{2,13} l_6^2 l_8^2 - \\
& \frac{5}{2} (s^2 - t^2 - u^2) \tau_{1,16} \tau_{2,13} l_6^2 l_8^2 - 8 u^2 \tau_{1,17} \tau_{2,13} l_6^2 l_8^2 + \frac{5}{2} (s^2 - t^2 - u^2) \tau_{1,17} \tau_{2,13} l_6^2 l_8^2 - 2 u^2 \tau_{2,10} \tau_{2,13} l_6^2 l_8^2 + \\
& 14 (s^2 - t^2 - u^2) \tau_{2,10} \tau_{2,13} l_6^2 l_8^2 - 3 u^2 \tau_{1,12} \tau_{2,14} l_6^2 l_8^2 + \frac{9}{2} (s^2 - t^2 - u^2) \tau_{1,12} \tau_{2,14} l_6^2 l_8^2 + u^2 \tau_{1,13} \tau_{2,14} l_6^2 l_8^2 + \\
& \frac{5}{2} (s^2 - t^2 - u^2) \tau_{1,13} \tau_{2,14} l_6^2 l_8^2 + 6 (-s^2 + t^2 + u^2) \tau_{1,14} \tau_{2,14} l_6^2 l_8^2 + 6 (-s^2 + t^2 + u^2) \tau_{1,15} \tau_{2,14} l_6^2 l_8^2 - 2 u^2 \tau_{2,9} \tau_{2,14} l_6^2 l_8^2 + \\
& \frac{3}{2} (s^2 - t^2 - u^2) \tau_{2,9} \tau_{2,14} l_6^2 l_8^2 + u^2 \tau_{2,10} \tau_{2,14} l_6^2 l_8^2 + \frac{3}{2} (s^2 - t^2 - u^2) \tau_{2,10} \tau_{2,14} l_6^2 l_8^2 - 2 u^2 \tau_{2,12} \tau_{2,14} l_6^2 l_8^2 +
\end{aligned}$$

$$\begin{aligned}
& \frac{3}{2} (s^2 - t^2 - u^2) \tau_{2,12} \tau_{2,14} l_6^2 l_8^2 + u^2 \tau_{2,13} \tau_{2,14} l_6^2 l_8^2 + \frac{3}{2} (s^2 - t^2 - u^2) \tau_{2,13} \tau_{2,14} l_6^2 l_8^2 - 3 u^2 \tau_{1,12} \tau_{2,15} l_6^2 l_8^2 + \\
& \frac{9}{2} (s^2 - t^2 - u^2) \tau_{1,12} \tau_{2,15} l_6^2 l_8^2 + u^2 \tau_{1,13} \tau_{2,15} l_6^2 l_8^2 + \frac{5}{2} (s^2 - t^2 - u^2) \tau_{1,13} \tau_{2,15} l_6^2 l_8^2 + 6 (-s^2 + t^2 + u^2) \tau_{1,14} \tau_{2,15} l_6^2 l_8^2 + \\
& 6 (-s^2 + t^2 + u^2) \tau_{1,15} \tau_{2,15} l_6^2 l_8^2 - 2 u^2 \tau_{2,9} \tau_{2,15} l_6^2 l_8^2 + \frac{3}{2} (s^2 - t^2 - u^2) \tau_{2,9} \tau_{2,15} l_6^2 l_8^2 + u^2 \tau_{2,10} \tau_{2,15} l_6^2 l_8^2 + \\
& \frac{3}{2} (s^2 - t^2 - u^2) \tau_{2,10} \tau_{2,15} l_6^2 l_8^2 - 2 u^2 \tau_{2,12} \tau_{2,15} l_6^2 l_8^2 + \frac{3}{2} (s^2 - t^2 - u^2) \tau_{2,12} \tau_{2,15} l_6^2 l_8^2 + u^2 \tau_{2,13} \tau_{2,15} l_6^2 l_8^2 + \\
& \frac{3}{2} (s^2 - t^2 - u^2) \tau_{2,13} \tau_{2,15} l_6^2 l_8^2 - 6 u^2 \tau_{2,14} \tau_{2,15} l_6^2 l_8^2 + 2 (s^2 - t^2 - u^2) \tau_{2,14} \tau_{2,15} l_6^2 l_8^2 - 3 u^2 \tau_{1,12} \tau_{2,16} l_6^2 l_8^2 + \\
& \frac{3}{2} (s^2 - t^2 - u^2) \tau_{1,12} \tau_{2,16} l_6^2 l_8^2 + \frac{3}{2} (s^2 - t^2 - u^2) \tau_{1,13} \tau_{2,16} l_6^2 l_8^2 + 6 (-s^2 + t^2 + u^2) \tau_{1,16} \tau_{2,16} l_6^2 l_8^2 + \\
& 6 (s^2 - t^2 - u^2) \tau_{1,17} \tau_{2,16} l_6^2 l_8^2 - 3 u^2 \tau_{2,9} \tau_{2,16} l_6^2 l_8^2 + \frac{9}{2} (s^2 - t^2 - u^2) \tau_{2,9} \tau_{2,16} l_6^2 l_8^2 + u^2 \tau_{2,10} \tau_{2,16} l_6^2 l_8^2 + \\
& \frac{5}{2} (s^2 - t^2 - u^2) \tau_{2,10} \tau_{2,16} l_6^2 l_8^2 - 8 u^2 \tau_{2,12} \tau_{2,16} l_6^2 l_8^2 + \frac{5}{2} (s^2 - t^2 - u^2) \tau_{2,12} \tau_{2,16} l_6^2 l_8^2 + \frac{9}{2} (s^2 - t^2 - u^2) \tau_{2,13} \tau_{2,16} l_6^2 l_8^2 + \\
& 3 u^2 \tau_{1,12} \tau_{2,17} l_6^2 l_8^2 - \frac{3}{2} (s^2 - t^2 - u^2) \tau_{1,12} \tau_{2,17} l_6^2 l_8^2 - \frac{3}{2} (s^2 - t^2 - u^2) \tau_{1,13} \tau_{2,17} l_6^2 l_8^2 + 6 (s^2 - t^2 - u^2) \tau_{1,16} \tau_{2,17} l_6^2 l_8^2 + \\
& 6 (-s^2 + t^2 + u^2) \tau_{1,17} \tau_{2,17} l_6^2 l_8^2 + 3 u^2 \tau_{2,9} \tau_{2,17} l_6^2 l_8^2 - \frac{9}{2} (s^2 - t^2 - u^2) \tau_{2,9} \tau_{2,17} l_6^2 l_8^2 - u^2 \tau_{2,10} \tau_{2,17} l_6^2 l_8^2 - \\
& \frac{5}{2} (s^2 - t^2 - u^2) \tau_{2,10} \tau_{2,17} l_6^2 l_8^2 + 8 u^2 \tau_{2,12} \tau_{2,17} l_6^2 l_8^2 - \frac{5}{2} (s^2 - t^2 - u^2) \tau_{2,12} \tau_{2,17} l_6^2 l_8^2 - \frac{9}{2} (s^2 - t^2 - u^2) \tau_{2,13} \tau_{2,17} l_6^2 l_8^2 + \\
& 6 u^2 \tau_{2,16} \tau_{2,17} l_6^2 l_8^2 + 2 (-s^2 + t^2 + u^2) \tau_{2,16} \tau_{2,17} l_6^2 l_8^2 - 4 u^2 \tau_{1,12} \tau_{3,14} l_6^2 l_8^2 + 2 (s^2 - t^2 - u^2) \tau_{1,12} \tau_{3,14} l_6^2 l_8^2 + \\
& u^2 \tau_{1,14} \tau_{3,14} l_6^2 l_8^2 + 2 (-s^2 + t^2 + u^2) \tau_{1,14} \tau_{3,14} l_6^2 l_8^2 + u^2 \tau_{1,15} \tau_{3,14} l_6^2 l_8^2 + 2 (-s^2 + t^2 + u^2) \tau_{1,15} \tau_{3,14} l_6^2 l_8^2 - \\
& 3 u^2 \tau_{2,9} \tau_{3,14} l_6^2 l_8^2 - 3 u^2 \tau_{2,12} \tau_{3,14} l_6^2 l_8^2 - 5 u^2 \tau_{2,14} \tau_{3,14} l_6^2 l_8^2 + 2 (-s^2 + t^2 + u^2) \tau_{2,14} \tau_{3,14} l_6^2 l_8^2 - 5 u^2 \tau_{2,15} \tau_{3,14} l_6^2 l_8^2 + \\
& 2 (-s^2 + t^2 + u^2) \tau_{2,15} \tau_{3,14} l_6^2 l_8^2 - 4 u^2 \tau_{1,12} \tau_{3,15} l_6^2 l_8^2 + 2 (s^2 - t^2 - u^2) \tau_{1,12} \tau_{3,15} l_6^2 l_8^2 + u^2 \tau_{1,14} \tau_{3,15} l_6^2 l_8^2 + \\
& 2 (-s^2 + t^2 + u^2) \tau_{1,14} \tau_{3,15} l_6^2 l_8^2 + u^2 \tau_{1,15} \tau_{3,15} l_6^2 l_8^2 + 2 (-s^2 + t^2 + u^2) \tau_{1,15} \tau_{3,15} l_6^2 l_8^2 - 3 u^2 \tau_{2,9} \tau_{3,15} l_6^2 l_8^2 - \\
& 3 u^2 \tau_{2,12} \tau_{3,15} l_6^2 l_8^2 - 5 u^2 \tau_{2,14} \tau_{3,15} l_6^2 l_8^2 + 2 (-s^2 + t^2 + u^2) \tau_{2,14} \tau_{3,15} l_6^2 l_8^2 - 5 u^2 \tau_{2,15} \tau_{3,15} l_6^2 l_8^2 + \\
& 2 (-s^2 + t^2 + u^2) \tau_{2,15} \tau_{3,15} l_6^2 l_8^2 - 4 u^2 \tau_{3,14} \tau_{3,15} l_6^2 l_8^2 + 4 (-s^2 + t^2 + u^2) \tau_{3,14} \tau_{3,15} l_6^2 l_8^2 - 3 u^2 \tau_{1,12} \tau_{3,16} l_6^2 l_8^2 + \\
& u^2 \tau_{1,16} \tau_{3,16} l_6^2 l_8^2 + 2 (-s^2 + t^2 + u^2) \tau_{1,16} \tau_{3,16} l_6^2 l_8^2 - u^2 \tau_{1,17} \tau_{3,16} l_6^2 l_8^2 + 2 (s^2 - t^2 - u^2) \tau_{1,17} \tau_{3,16} l_6^2 l_8^2 - \\
& 4 u^2 \tau_{2,9} \tau_{3,16} l_6^2 l_8^2 + 2 (s^2 - t^2 - u^2) \tau_{2,9} \tau_{3,16} l_6^2 l_8^2 - 8 u^2 \tau_{2,12} \tau_{3,16} l_6^2 l_8^2 + 2 (-s^2 + t^2 + u^2) \tau_{2,12} \tau_{3,16} l_6^2 l_8^2 - \\
& 5 u^2 \tau_{2,16} \tau_{3,16} l_6^2 l_8^2 + 2 (-s^2 + t^2 + u^2) \tau_{2,16} \tau_{3,16} l_6^2 l_8^2 + 5 u^2 \tau_{2,17} \tau_{3,16} l_6^2 l_8^2 + 2 (s^2 - t^2 - u^2) \tau_{2,17} \tau_{3,16} l_6^2 l_8^2 -
\end{aligned}$$

$$\begin{aligned}
& \tau_{1,9} \left( -(3\tau_{1,15} + 2\tau_{1,16} - 2\tau_{1,17} - 9\tau_{2,9} + 2\tau_{2,12} + \tau_{2,14} + \tau_{2,15} + 4\tau_{3,14} + 4\tau_{3,15} + 3\tau_{3,16} - 3\tau_{3,17})t^2 - \right. \\
& \quad 3(t - 3u)\tau_{1,14}t + 2(8(t^2 + u^2) - 7s^2)\tau_{1,12} + \\
& \quad \frac{1}{2}(s^2 - t^2 - u^2)(9\tau_{1,15} + 3\tau_{1,16} - 3\tau_{1,17} - 6\tau_{2,9} - 22\tau_{2,12} - 5\tau_{2,14} - 5\tau_{2,15} - 3\tau_{2,16} + 3\tau_{2,17} + 4(\tau_{3,14} + \tau_{3,15})) + \\
& \quad \left. u^2(\tau_{1,16} - \tau_{1,17} + 9\tau_{2,9} + 4\tau_{2,12} + 8\tau_{2,14} + 8\tau_{2,15} + 3\tau_{2,16} - 3\tau_{2,17} + 8\tau_{3,14} + 8\tau_{3,15} + 3\tau_{3,16} - 3\tau_{3,17}) \right) l_6^2 l_8^2 + \\
& 3u^2\tau_{1,12}\tau_{3,17}l_6^2 l_8^2 - u^2\tau_{1,16}\tau_{3,17}l_6^2 l_8^2 + 2(s^2 - t^2 - u^2)\tau_{1,16}\tau_{3,17}l_6^2 l_8^2 + u^2\tau_{1,17}\tau_{3,17}l_6^2 l_8^2 + \\
& 2(-s^2 + t^2 + u^2)\tau_{1,17}\tau_{3,17}l_6^2 l_8^2 + 4u^2\tau_{2,9}\tau_{3,17}l_6^2 l_8^2 + 2(-s^2 + t^2 + u^2)\tau_{2,9}\tau_{3,17}l_6^2 l_8^2 + 8u^2\tau_{2,12}\tau_{3,17}l_6^2 l_8^2 + \\
& 2(s^2 - t^2 - u^2)\tau_{2,12}\tau_{3,17}l_6^2 l_8^2 + 5u^2\tau_{2,16}\tau_{3,17}l_6^2 l_8^2 + 2(s^2 - t^2 - u^2)\tau_{2,16}\tau_{3,17}l_6^2 l_8^2 - 5u^2\tau_{2,17}\tau_{3,17}l_6^2 l_8^2 + \\
& 2(-s^2 + t^2 + u^2)\tau_{2,17}\tau_{3,17}l_6^2 l_8^2 + 4u^2\tau_{3,16}\tau_{3,17}l_6^2 l_8^2 + 4(s^2 - t^2 - u^2)\tau_{3,16}\tau_{3,17}l_6^2 l_8^2 + 4u^2\tau_{1,13}\tau_{4,14}l_6^2 l_8^2 + \\
& 2(-s^2 + t^2 + u^2)\tau_{1,13}\tau_{4,14}l_6^2 l_8^2 - 5u^2\tau_{1,14}\tau_{4,14}l_6^2 l_8^2 + 2(-s^2 + t^2 + u^2)\tau_{1,14}\tau_{4,14}l_6^2 l_8^2 - \\
& 5u^2\tau_{1,15}\tau_{4,14}l_6^2 l_8^2 + 2(-s^2 + t^2 + u^2)\tau_{1,15}\tau_{4,14}l_6^2 l_8^2 + 3u^2\tau_{2,10}\tau_{4,14}l_6^2 l_8^2 + 3u^2\tau_{2,13}\tau_{4,14}l_6^2 l_8^2 + \\
& u^2\tau_{2,14}\tau_{4,14}l_6^2 l_8^2 + 2(-s^2 + t^2 + u^2)\tau_{2,14}\tau_{4,14}l_6^2 l_8^2 + u^2\tau_{2,15}\tau_{4,14}l_6^2 l_8^2 + 2(-s^2 + t^2 + u^2)\tau_{2,15}\tau_{4,14}l_6^2 l_8^2 + \\
& 4u^2\tau_{1,13}\tau_{4,15}l_6^2 l_8^2 + 2(-s^2 + t^2 + u^2)\tau_{1,13}\tau_{4,15}l_6^2 l_8^2 - 5u^2\tau_{1,14}\tau_{4,15}l_6^2 l_8^2 + 2(-s^2 + t^2 + u^2)\tau_{1,14}\tau_{4,15}l_6^2 l_8^2 - \\
& 5u^2\tau_{1,15}\tau_{4,15}l_6^2 l_8^2 + 2(-s^2 + t^2 + u^2)\tau_{1,15}\tau_{4,15}l_6^2 l_8^2 + 3u^2\tau_{2,10}\tau_{4,15}l_6^2 l_8^2 + 3u^2\tau_{2,13}\tau_{4,15}l_6^2 l_8^2 + \\
& u^2\tau_{2,14}\tau_{4,15}l_6^2 l_8^2 + 2(-s^2 + t^2 + u^2)\tau_{2,14}\tau_{4,15}l_6^2 l_8^2 + u^2\tau_{2,15}\tau_{4,15}l_6^2 l_8^2 + 2(-s^2 + t^2 + u^2)\tau_{2,15}\tau_{4,15}l_6^2 l_8^2 - \\
& 4u^2\tau_{4,14}\tau_{4,15}l_6^2 l_8^2 + 4(-s^2 + t^2 + u^2)\tau_{4,14}\tau_{4,15}l_6^2 l_8^2 + 3u^2\tau_{1,13}\tau_{4,16}l_6^2 l_8^2 - 5u^2\tau_{1,16}\tau_{4,16}l_6^2 l_8^2 + \\
& 2(-s^2 + t^2 + u^2)\tau_{1,16}\tau_{4,16}l_6^2 l_8^2 + 5u^2\tau_{1,17}\tau_{4,16}l_6^2 l_8^2 + 2(s^2 - t^2 - u^2)\tau_{1,17}\tau_{4,16}l_6^2 l_8^2 + \\
& 4u^2\tau_{2,10}\tau_{4,16}l_6^2 l_8^2 + 2(-s^2 + t^2 + u^2)\tau_{2,10}\tau_{4,16}l_6^2 l_8^2 + 8u^2\tau_{2,13}\tau_{4,16}l_6^2 l_8^2 + 2(s^2 - t^2 - u^2)\tau_{2,13}\tau_{4,16}l_6^2 l_8^2 + \\
& u^2\tau_{2,16}\tau_{4,16}l_6^2 l_8^2 + 2(-s^2 + t^2 + u^2)\tau_{2,16}\tau_{4,16}l_6^2 l_8^2 - u^2\tau_{2,17}\tau_{4,16}l_6^2 l_8^2 + 2(s^2 - t^2 - u^2)\tau_{2,17}\tau_{4,16}l_6^2 l_8^2 - \\
& 3u^2\tau_{1,13}\tau_{4,17}l_6^2 l_8^2 + 5u^2\tau_{1,16}\tau_{4,17}l_6^2 l_8^2 + 2(s^2 - t^2 - u^2)\tau_{1,16}\tau_{4,17}l_6^2 l_8^2 - 5u^2\tau_{1,17}\tau_{4,17}l_6^2 l_8^2 + \\
& 2(-s^2 + t^2 + u^2)\tau_{1,17}\tau_{4,17}l_6^2 l_8^2 - 4u^2\tau_{2,10}\tau_{4,17}l_6^2 l_8^2 + 2(s^2 - t^2 - u^2)\tau_{2,10}\tau_{4,17}l_6^2 l_8^2 - \\
& 8u^2\tau_{2,13}\tau_{4,17}l_6^2 l_8^2 + 2(-s^2 + t^2 + u^2)\tau_{2,13}\tau_{4,17}l_6^2 l_8^2 - u^2\tau_{2,16}\tau_{4,17}l_6^2 l_8^2 + 2(s^2 - t^2 - u^2)\tau_{2,16}\tau_{4,17}l_6^2 l_8^2 + \\
& u^2\tau_{2,17}\tau_{4,17}l_6^2 l_8^2 + 2(-s^2 + t^2 + u^2)\tau_{2,17}\tau_{4,17}l_6^2 l_8^2 + 4u^2\tau_{4,16}\tau_{4,17}l_6^2 l_8^2 + 4(s^2 - t^2 - u^2)\tau_{4,16}\tau_{4,17}l_6^2 l_8^2 - \\
& \tau_{1,10} \left( (\tau_{1,15} + \tau_{1,16} - \tau_{1,17} + 9\tau_{2,10} - 2\tau_{2,13} + 3\tau_{2,14} + 3\tau_{2,15} + 3\tau_{2,16} - 3\tau_{2,17} + 4\tau_{4,14} + 4\tau_{4,15} + 3\tau_{4,16} - 3\tau_{4,17})t^2 + \right. \\
& \quad 2(8(t^2 + u^2) - 7s^2)\tau_{1,13} + \frac{1}{2}(5s^2 - 3(t^2 + 7u^2))\tau_{1,14} + \\
& \quad \frac{1}{2}(s^2 - t^2 - u^2)(5\tau_{1,15} + 3\tau_{1,16} - 3\tau_{1,17} - 6\tau_{2,10} - 22\tau_{2,13} - 9\tau_{2,14} - 9\tau_{2,15} - 3\tau_{2,16} + 3\tau_{2,17} - 4\tau_{4,14} - 4\tau_{4,15}) + \\
& \quad \left. u^2(-8\tau_{1,15} - 2\tau_{1,16} + 2\tau_{1,17} + 9\tau_{2,10} + 4\tau_{2,13} - 8\tau_{4,14} - 8\tau_{4,15} - 3\tau_{4,16} + 3\tau_{4,17}) \right) l_6^2 l_8^2 -
\end{aligned}$$

$$\begin{aligned}
& 2u^3 \tau_{9,15} l_6^2 l_8^2 + u(-s^2 + t^2 + u^2) \tau_{9,15} l_6^2 l_8^2 + 2u^3 \tau_{9,17} l_6^2 l_8^2 - u(-s^2 + t^2 + u^2) \tau_{9,17} l_6^2 l_8^2 + 2u^3 \tau_{13,14} l_6^2 l_8^2 - \\
& u(-s^2 + t^2 + u^2) \tau_{13,14} l_6^2 l_8^2 + 2u^3 \tau_{13,16} l_6^2 l_8^2 - u(-s^2 + t^2 + u^2) \tau_{13,16} l_6^2 l_8^2 - 4u^3 l_6^2 l_8^2 l_{11}^2 + \\
& 34u(-s^2 + t^2 + u^2) l_6^2 l_8^2 l_{11}^2 - l_{10}^2 \left( -2(\tau_{5,16} + \tau_{5,17} + \tau_{7,14} - \tau_{7,15} - 2l_{11}^2) t^3 + \right. \\
& (2\tau_{1,15}^2 + (4\tau_{1,17} + 8\tau_{3,6} + 4\tau_{3,7} + 5\tau_{3,15} + 5\tau_{3,17} + 3\tau_{4,6} + 3\tau_{4,7} - \tau_{4,15} - \tau_{4,17}) \tau_{1,15} + 2\tau_{1,16}^2 + 2\tau_{1,17}^2 + \\
& 2\tau_{2,14}^2 + 2\tau_{2,16}^2 + 2(\tau_{2,15} + \tau_{2,17})^2 + 9\tau_{3,6}^2 + 3\tau_{3,7}^2 + 3\tau_{3,8}^2 + 3\tau_{3,14}^2 + 3\tau_{3,15}^2 + 3\tau_{3,16}^2 + 3\tau_{3,17}^2 + \\
& 3\tau_{4,5}^2 + 3\tau_{4,6}^2 + 9\tau_{4,7}^2 + 9\tau_{4,8}^2 + 3\tau_{4,14}^2 + 3\tau_{4,15}^2 + 3\tau_{4,16}^2 + 3\tau_{4,17}^2 + \tau_{3,5}(9\tau_{3,5} - 8(\tau_{2,15} + \tau_{2,17})) + \\
& 2(\tau_{3,5} - 2(\tau_{2,15} + \tau_{2,17})) \tau_{3,8} - 3\tau_{2,16}(\tau_{3,5} + \tau_{3,8}) + \tau_{2,14}(3(\tau_{3,5} + \tau_{3,8}) - 4\tau_{2,16}) + \tau_{3,8} \tau_{3,14} - \\
& \tau_{3,8} \tau_{3,15} + (\tau_{2,16} + \tau_{3,5})(\tau_{3,14} - \tau_{3,16}) - \tau_{3,8} \tau_{3,16} - 6\tau_{3,14} \tau_{3,16} - \tau_{3,8} \tau_{3,17} + 6\tau_{3,15} \tau_{3,17} - \\
& 4\tau_{2,16} \tau_{4,5} + 9\tau_{3,5} \tau_{4,5} - 2\tau_{3,8} \tau_{4,5} + \tau_{3,14} \tau_{4,5} - \tau_{3,16} \tau_{4,5} - 3\tau_{3,14} \tau_{4,6} + 3\tau_{3,15} \tau_{4,6} + \\
& 3\tau_{3,16} \tau_{4,6} + 3\tau_{3,17} \tau_{4,6} - 8\tau_{3,14} \tau_{4,7} + 3\tau_{3,15} \tau_{4,7} + 8\tau_{3,16} \tau_{4,7} + 3\tau_{3,17} \tau_{4,7} + 2\tau_{4,6} \tau_{4,7} + \\
& \tau_{3,6}(2\tau_{3,7} - 2\tau_{3,14} + 8\tau_{3,15} + 2\tau_{3,16} + 8\tau_{3,17} + 9\tau_{4,6} + 4\tau_{4,7}) - 8\tau_{2,16} \tau_{4,8} + 4\tau_{3,5} \tau_{4,8} + 9\tau_{3,8} \tau_{4,8} + 2\tau_{4,5} \\
& \tau_{4,8} - 5\tau_{2,16} \tau_{4,14} + 3\tau_{3,5} \tau_{4,14} + 3\tau_{3,8} \tau_{4,14} + 3\tau_{4,5} \tau_{4,14} - \tau_{4,6} \tau_{4,14} + 8\tau_{4,8} \tau_{4,14} - 8\tau_{3,5} \tau_{4,15} - 3\tau_{3,8} \tau_{4,15} - \\
& 2\tau_{4,5} \tau_{4,15} + \tau_{4,6} \tau_{4,15} + \tau_{4,7} \tau_{4,15} - 2\tau_{4,8} \tau_{4,15} + \tau_{2,14}(-\tau_{3,14} + \tau_{3,16} + 4\tau_{4,5} + 8\tau_{4,8} + 5\tau_{4,14} - 5\tau_{4,16}) + \\
& \tau_{1,16}(3\tau_{3,6} + 3\tau_{3,7} - 5\tau_{3,14} + 5\tau_{3,16} + 4\tau_{4,6} + 8\tau_{4,7} + \tau_{4,14} - \tau_{4,16}) + 5\tau_{2,16} \tau_{4,16} - 3\tau_{3,5} \tau_{4,16} - 3\tau_{3,8} \tau_{4,16} - \\
& 3\tau_{4,5} \tau_{4,16} + \tau_{4,6} \tau_{4,16} - 8\tau_{4,8} \tau_{4,16} - 6\tau_{4,14} \tau_{4,16} + \tau_{1,17}(8\tau_{3,6} + 4\tau_{3,7} + 5\tau_{3,15} + 5\tau_{3,17} + 3\tau_{4,6} + \\
& 3\tau_{4,7} - \tau_{4,15} - \tau_{4,17}) - 8\tau_{3,5} \tau_{4,17} - 3\tau_{3,8} \tau_{4,17} - 2\tau_{4,5} \tau_{4,17} + \tau_{4,6} \tau_{4,17} + \tau_{4,7} \tau_{4,17} - 2\tau_{4,8} \tau_{4,17} + \\
& 6\tau_{4,15} \tau_{4,17} + \tau_{3,7}(-2\tau_{3,14} + 3\tau_{3,15} + 2\tau_{3,16} + 3\tau_{3,17} - 2\tau_{4,6} + 9\tau_{4,7} + \tau_{4,15} + \tau_{4,17}) - \tau_{2,15} \\
& (\tau_{3,15} + \tau_{3,17} + 3\tau_{4,5} + 3\tau_{4,8} - 5(\tau_{4,15} + \tau_{4,17})) - \tau_{2,17}(\tau_{3,15} + \tau_{3,17} + 3\tau_{4,5} + 3\tau_{4,8} - 5(\tau_{4,15} + \tau_{4,17})) \Big) t^2 + \\
& (-s^2 + t^2 + u^2) (\tau_{5,16} + \tau_{5,17} + \tau_{7,14} - \tau_{7,15} - 34l_{11}^2) t + 2s^2 \tau_{1,14}^2 + s \tau_{1,14} (-4s \tau_{1,16} + 3(t - u) \tau_{3,6} + 3(t - u) \tau_{3,7} + \\
& (u - 5t) \tau_{3,14} + (5t - u) \tau_{3,16} + 4t \tau_{4,6} - 8u \tau_{4,6} + 8t \tau_{4,7} - 4u \tau_{4,7} + t \tau_{4,14} - 5u \tau_{4,14} - t \tau_{4,16} + 5u \tau_{4,16}) + \\
& \frac{1}{2} (s^2 - t^2 - u^2) (4\tau_{1,15}^2 + 4(2\tau_{1,17} + \tau_{3,6} - \tau_{3,7} + \tau_{3,15} + \tau_{3,17} + \tau_{4,15} + \tau_{4,17}) \tau_{1,15} + 4\tau_{1,16}^2 + 4\tau_{1,17}^2 - \\
& 4\tau_{3,6}^2 - 4\tau_{3,7}^2 - 2\tau_{3,14}^2 - 2\tau_{3,15}^2 - 2\tau_{3,16}^2 - 2\tau_{3,17}^2 - 4\tau_{4,5}^2 - 4\tau_{4,6}^2 - 4\tau_{4,7}^2 - 4\tau_{4,8}^2 - 2\tau_{4,14}^2 - \\
& 2\tau_{4,15}^2 - 2\tau_{4,16}^2 - 2\tau_{4,17}^2 + 4(\tau_{2,15}^2 + (2\tau_{2,17} - \tau_{3,5} + \tau_{3,8}) \tau_{2,15} + (\tau_{2,14} - \tau_{2,16})^2 + \tau_{2,17}^2 - \tau_{3,5}^2 - \tau_{3,8}^2 - \\
& 7\tau_{3,5} \tau_{3,8} + \tau_{2,17}(\tau_{3,8} - \tau_{3,5})) + 3\tau_{3,5} \tau_{3,14} + 3\tau_{3,8} \tau_{3,14} - 5\tau_{3,8} \tau_{3,15} - 3\tau_{3,8} \tau_{3,16} + 4\tau_{3,14} \tau_{3,16} - \\
& 5\tau_{3,8} \tau_{3,17} - 4\tau_{3,15} \tau_{3,17} - 22\tau_{3,8} \tau_{4,5} + 5\tau_{3,14} \tau_{4,5} - 3\tau_{3,15} \tau_{4,5} - 5\tau_{3,16} \tau_{4,5} - 3\tau_{3,17} \tau_{4,5} + 9\tau_{3,14} \tau_{4,6} - \\
& 3\tau_{3,15} \tau_{4,6} - 9\tau_{3,16} \tau_{4,6} - 3\tau_{3,17} \tau_{4,6} + 5\tau_{3,14} \tau_{4,7} - 3\tau_{3,15} \tau_{4,7} - 5\tau_{3,16} \tau_{4,7} - 3\tau_{3,17} \tau_{4,7} - 28\tau_{4,6} \tau_{4,7} - \\
& 6\tau_{3,8} \tau_{4,8} + 9\tau_{3,14} \tau_{4,8} - 3\tau_{3,15} \tau_{4,8} - 9\tau_{3,16} \tau_{4,8} - 3\tau_{3,17} \tau_{4,8} - 28\tau_{4,5} \tau_{4,8} - 3\tau_{3,8} \tau_{4,14} + 12\tau_{3,14} \tau_{4,14} - \\
& 12\tau_{3,16} \tau_{4,14} - 9\tau_{4,5} \tau_{4,14} - 5\tau_{4,6} \tau_{4,14} - 9\tau_{4,7} \tau_{4,14} - 5\tau_{4,8} \tau_{4,14} + 9\tau_{3,8} \tau_{4,15} + 12\tau_{3,15} \tau_{4,15} + 12\tau_{3,17} \tau_{4,15} + \\
& 3\tau_{4,5} \tau_{4,15} + 3\tau_{4,6} \tau_{4,15} + 3\tau_{4,7} \tau_{4,15} + 3\tau_{4,8} \tau_{4,15} + 4\tau_{2,14}(\tau_{3,14} - \tau_{3,16} - \tau_{4,5} + \tau_{4,8} + \tau_{4,14} - \tau_{4,16}) + \\
& 3\tau_{3,8} \tau_{4,16} - 12\tau_{3,14} \tau_{4,16} + 12\tau_{3,16} \tau_{4,16} + 9\tau_{4,5} \tau_{4,16} + 5\tau_{4,6} \tau_{4,16} + 9\tau_{4,7} \tau_{4,16} + 5\tau_{4,8} \tau_{4,16} + 4\tau_{4,14} \tau_{4,16} + \\
& 4\tau_{1,16}(-\tau_{3,14} + \tau_{3,16} - \tau_{4,6} + \tau_{4,7} - \tau_{4,14} + \tau_{4,16}) + 4\tau_{2,16}(-\tau_{3,14} + \tau_{3,16} + \tau_{4,5} - \tau_{4,8} - \tau_{4,14} + \tau_{4,16}) - \\
& \tau_{3,6}(28\tau_{3,7} - 3\tau_{3,14} + 5\tau_{3,15} + 3\tau_{3,16} + 5\tau_{3,17} + 6\tau_{4,6} + 22\tau_{4,7} + 3\tau_{4,14} - 9\tau_{4,15} - 3\tau_{4,16} - 9\tau_{4,17}) - \\
& \tau_{3,5}(9\tau_{3,15} + 3\tau_{3,16} + 9\tau_{3,17} + 6\tau_{4,5} + 22\tau_{4,8} + 3\tau_{4,14} - 5\tau_{4,15} - 3\tau_{4,16} - 5\tau_{4,17}) + 9\tau_{3,8} \tau_{4,17} + \\
& 12\tau_{3,15} \tau_{4,17} + 12\tau_{3,17} \tau_{4,17} + 3\tau_{4,5} \tau_{4,17} + 3\tau_{4,6} \tau_{4,17} + 3\tau_{4,7} \tau_{4,17} + 3\tau_{4,8} \tau_{4,17} - 4\tau_{4,15} \tau_{4,17} + 4\tau_{2,15}
\end{aligned}$$

$$\begin{aligned}
& (\tau_{3,15} + \tau_{3,17} + \tau_{4,15} + \tau_{4,17}) + 4\tau_{2,17}(\tau_{3,15} + \tau_{3,17} + \tau_{4,15} + \tau_{4,17}) + 4\tau_{1,17}(\tau_{3,6} - \tau_{3,7} + \tau_{3,15} + \tau_{3,17} + \tau_{4,15} + \\
& \tau_{4,17}) + \tau_{3,7}(3\tau_{3,14} - 9\tau_{3,15} - 3\tau_{3,16} - 9\tau_{3,17} - 22\tau_{4,6} - 6\tau_{4,7} - 3\tau_{4,14} + 5\tau_{4,15} + 3\tau_{4,16} + 5\tau_{4,17})) + \\
& u^2 \left( 2\tau_{1,15}^2 + (4\tau_{1,17} - 4\tau_{3,6} - 8\tau_{3,7} - \tau_{3,15} - \tau_{3,17} - 3\tau_{4,6} - 3\tau_{4,7} + 5\tau_{4,15} + 5\tau_{4,17})\tau_{1,15} + 2\tau_{1,16}^2 + 2\tau_{1,17}^2 + \right. \\
& 2\tau_{2,14}^2 + 2\tau_{2,16}^2 + 2(\tau_{2,15} + \tau_{2,17})^2 + 3\tau_{3,6}^2 + 9\tau_{3,7}^2 + 9\tau_{3,8}^2 + 3\tau_{3,14}^2 + 3\tau_{3,15}^2 + 3\tau_{3,16}^2 + 3\tau_{3,17}^2 + \\
& 9\tau_{4,5}^2 + 9\tau_{4,6}^2 + 3\tau_{4,7}^2 + 3\tau_{4,8}^2 + 3\tau_{4,14}^2 + 3\tau_{4,15}^2 + 3\tau_{4,16}^2 + 3\tau_{4,17}^2 + \tau_{3,5}(4(\tau_{2,15} + \tau_{2,17}) + 3\tau_{3,5}) + \\
& 2(4(\tau_{2,15} + \tau_{2,17}) + \tau_{3,5})\tau_{3,8} + 3\tau_{2,16}(\tau_{3,5} + \tau_{3,8}) - \tau_{2,14}(4\tau_{2,16} + 3(\tau_{3,5} + \tau_{3,8})) - 2\tau_{3,5}\tau_{3,14} - 2\tau_{3,8}\tau_{3,14} + \\
& 3\tau_{3,5}\tau_{3,15} + 8\tau_{3,8}\tau_{3,15} + 2\tau_{3,5}\tau_{3,16} + 2\tau_{3,8}\tau_{3,16} - 6\tau_{3,14}\tau_{3,16} + 5\tau_{2,16}(\tau_{3,16} - \tau_{3,14}) + 3\tau_{3,5}\tau_{3,17} + \\
& 8\tau_{3,8}\tau_{3,17} + 6\tau_{3,15}\tau_{3,17} + 8\tau_{2,16}\tau_{4,5} + 9\tau_{3,5}\tau_{4,5} + 4\tau_{3,8}\tau_{4,5} - 8\tau_{3,14}\tau_{4,5} + 3\tau_{3,15}\tau_{4,5} + 8\tau_{3,16}\tau_{4,5} + \\
& 3\tau_{3,17}\tau_{4,5} + \tau_{3,14}\tau_{4,7} - \tau_{3,16}\tau_{4,7} + 2\tau_{4,6}\tau_{4,7} + 4\tau_{2,16}\tau_{4,8} - 2\tau_{3,5}\tau_{4,8} + 9\tau_{3,8}\tau_{4,8} - 3\tau_{3,14}\tau_{4,8} + 3\tau_{3,15}\tau_{4,8} + \\
& 3\tau_{3,16}\tau_{4,8} + 3\tau_{3,17}\tau_{4,8} + 2\tau_{4,5}\tau_{4,8} + \tau_{2,16}\tau_{4,14} + 8\tau_{4,6}\tau_{4,14} + 3\tau_{4,7}\tau_{4,14} - \tau_{4,8}\tau_{4,14} + \tau_{3,5}\tau_{4,15} + \tau_{4,5}\tau_{4,15} - \\
& 2\tau_{4,6}\tau_{4,15} - 2\tau_{4,7}\tau_{4,15} + \tau_{4,8}\tau_{4,15} - \tau_{1,16}(3\tau_{3,6} + 3\tau_{3,7} - \tau_{3,14} + \tau_{3,16} + 8\tau_{4,6} + 4\tau_{4,7} + 5\tau_{4,14} - 5\tau_{4,16}) - \\
& \tau_{2,16}\tau_{4,16} - 8\tau_{4,6}\tau_{4,16} - 3\tau_{4,7}\tau_{4,16} + \tau_{4,8}\tau_{4,16} - 6\tau_{4,14}\tau_{4,16} + \tau_{2,14}(5\tau_{3,14} - 5\tau_{3,16} - 8\tau_{4,5} - \\
& 4\tau_{4,8} - \tau_{4,14} + \tau_{4,16}) + \tau_{3,7}(\tau_{3,14} - \tau_{3,16} + 4\tau_{4,6} + 9\tau_{4,7} + 3\tau_{4,14} - 8\tau_{4,15} - 3\tau_{4,16} - 8\tau_{4,17}) + \\
& \tau_{3,6}(2\tau_{3,7} + \tau_{3,14} - \tau_{3,15} - \tau_{3,16} - \tau_{3,17} + 9\tau_{4,6} - 2\tau_{4,7} + 3\tau_{4,14} - 3\tau_{4,15} - 3\tau_{4,16} - 3\tau_{4,17}) + \\
& \tau_{2,15}(5\tau_{3,15} + 5\tau_{3,17} + 3\tau_{4,5} + 3\tau_{4,8} - \tau_{4,15} - \tau_{4,17}) + \tau_{2,17}(5\tau_{3,15} + 5\tau_{3,17} + 3\tau_{4,5} + 3\tau_{4,8} - \tau_{4,15} - \tau_{4,17}) + \\
& \tau_{3,5}\tau_{4,17} + \tau_{4,5}\tau_{4,17} - 2\tau_{4,6}\tau_{4,17} - 2\tau_{4,7}\tau_{4,17} + \tau_{4,8}\tau_{4,17} + 6\tau_{4,15}\tau_{4,17} - \\
& \left. \tau_{1,17}(4\tau_{3,6} + 8\tau_{3,7} + \tau_{3,15} + \tau_{3,17} + 3\tau_{4,6} + 3\tau_{4,7} - 5(\tau_{4,15} + \tau_{4,17})) \right) + \\
& 2u^3 \left( \tau_{5,16} + \tau_{5,17} + \tau_{7,14} - \tau_{7,15} + 2l_{11}^2 \right) - u \left( -s^2 + l^2 + u^2 \right) \left( \tau_{5,16} + \tau_{5,17} + \tau_{7,14} - \tau_{7,15} + 34l_{11}^2 \right) \left( l_{12}^2 \right)
\end{aligned}$$

■  $N_{47}^{(7)}$

0

■  $N_{47}^{(8)}$

0
