# Supplementary material for: The Ultraviolet Behavior of N=8 Supergravity at Four Loops
Source: arXiv:0905.2326 ancillary file (2012-01-08)
Supplement: Supplementary file 47 [file SUGRA50.pdf]

## Integral 50: $\mathcal{I}_{50}$

$\mathcal{N} = 8$  four-point four-loop amplitude.

### ■ 2D plot of graph associated with $\mathcal{I}_{50}$

This fixes the labelling associated with the numerator expressions given below.

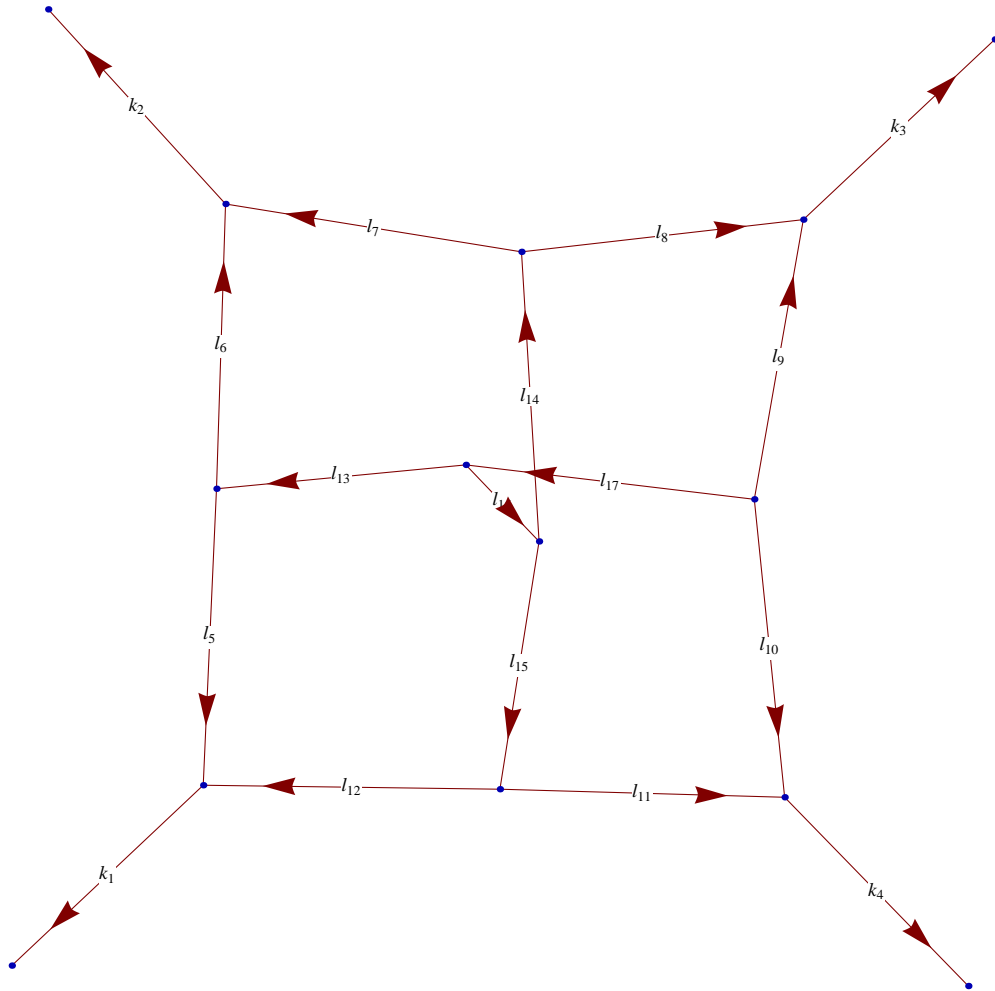

When using MathPlayer, by clicking three times (holding the click on the third click) directly on a vertex, one is able to move that vertex around, and its associated edges follow elastically. This functionality is absent when viewing as a pdf.

*Note: propagators for certain graphs were relabeled in the manuscript due to size constraints. The labels given in aux/rawData/Neq8FourLoops.m should be used for verification purposes.*

### ■ 3D plot of graph associated with $\mathcal{I}_{50}$

3D PLOT UNAVAILABLE FOR PDF. Please see .nb version for the 3D figure.

When using MathPlayer, by clicking anywhere in the image and dragging one should be able to rotate this 3D image. By holding (ALT) or (COMMAND) while clicking and moving the mouse up/down one should be able to zoom in/out. This functionality is absent when viewing as a pdf.

### ■ "Vertex Form" of graph associated with $\mathcal{I}_{50}$

This function returns the graph associated with the integral object in a vertex representation. This can be used as a way of specifying the topology of a graph using trivalent (cubic) vertices,  $\text{gVertex}[p_a, p_b, p_c]$ , where  $\{p_a, p_b, p_c\}$  are momenta labeling the propagators (edges) of the graph, and is understood that the edge labelled by  $p_a$  flows into the edge labelled by  $-p_a$ . Additionally, each vertex represents the manifest conservation of ( $D$  - dimensional) momenta :

$$\text{gVertex}[\{p_1, p_2, p_3\}] \iff (p_1 + p_2 + p_3 = 0)$$

$$\{\text{gVertex}(\{k_1, -l_{12}, -l_5\}), \text{gVertex}(\{k_2, -l_7, -l_6\}), \text{gVertex}(\{k_3, -l_9, -l_8\}), \text{gVertex}(\{k_4, -l_{10}, -l_{11}\}), \text{gVertex}(\{l_5, -l_{13}, l_6\}), \\ \text{gVertex}(\{l_7, l_8, -l_{14}\}), \text{gVertex}(\{l_9, l_{17}, l_{10}\}), \text{gVertex}(\{l_{11}, l_{12}, -l_{15}\}), \text{gVertex}(\{l_{13}, l_{16}, -l_{17}\}), \text{gVertex}(\{l_{14}, -l_{16}, l_{15}\})\}$$

### ■ Numerator expression for integral 50:

The following notation is used:  $\tau_{i,j} \equiv \begin{cases} 2 k_i \cdot l_j & \text{if } i \leq 4, j > 4 \\ 2 l_i \cdot l_j & \text{if } i, j > 4 \end{cases}$ .

$$s \equiv 2 k_1 \cdot k_2 = 2 k_3 \cdot k_4$$

We use  $s, t, u$  to represent the traditional Mandelstam variables for massless external four-point momenta:  $t \equiv 2 k_1 \cdot k_4 = 2 k_2 \cdot k_3$ .

$$u \equiv 2 k_1 \cdot k_3 = 2 k_2 \cdot k_4$$

Furthermore we use the shorthand  $(l_i)^2$  to represent the lorentz square:  $(l_i)^2 = l_i \cdot l_i$ .

The total numerator  $\mathcal{N}_{50}$  is given by summing over the following terms, distinguished here by explicit dependence on loop momenta:  $\mathcal{N}_{50} = \sum_{i=0}^8 \mathcal{N}_{50}^{(i)}$ :

#### ■ $\mathcal{N}_{50}^{(0)}$

$$\frac{1}{2} s^2 t^2 (s^2 + t^2)$$

#### ■ $\mathcal{N}_{50}^{(1)}$

$$\frac{1}{2} s^2 t^2 (-s \tau_{1,7} - t (\tau_{1,10} + \tau_{2,9} - \tau_{2,12} + \tau_{3,6} - \tau_{3,11} + \tau_{4,5} - \tau_{4,8}) + u (\tau_{2,12} + \tau_{3,11} + \tau_{4,8}))$$

■  $N_{50}^{(2)}$

$$\begin{aligned}
& -\frac{1}{8} s t \left( 4 (l_{13}^2 - l_{14}^2 - l_{15}^2 + l_{17}^2) t^3 + \right. \\
& 2 (\tau_{1,10}^2 + 4 \tau_{3,6} \tau_{1,10} + \tau_{2,9}^2 + \tau_{2,12}^2 + \tau_{3,6}^2 + \tau_{3,11}^2 + \tau_{4,5}^2 + \tau_{4,8}^2 + \tau_{1,9} \tau_{2,5} + \tau_{2,5} \tau_{2,9} + \tau_{2,8} \tau_{2,12} + \tau_{2,11} \tau_{3,7} + \tau_{3,6} \tau_{3,10} + \\
& \quad \tau_{3,7} \tau_{3,11} + \tau_{2,8} \tau_{3,12} + 4 \tau_{2,9} \tau_{4,5} + \tau_{3,10} \tau_{4,6} + \tau_{1,11} \tau_{4,7} + 4 \tau_{2,12} \tau_{4,8} + \tau_{3,5} \tau_{4,9} + \tau_{4,5} \tau_{4,9} + \tau_{1,8} \tau_{4,12} + \tau_{4,8} \tau_{4,12}) t^2 - \\
& 2 s \tau_{1,7}^2 t + (-s^2 + t^2 + u^2) (\tau_{5,8} + \tau_{6,11} + \tau_{7,10} + \tau_{9,12} - 2 l_{13}^2 + 4 l_{14}^2 + 4 l_{15}^2 - 2 l_{17}^2) t + \\
& 2 \tau_{1,6} \left( (\tau_{1,10} + \tau_{2,10}) t^2 + u^2 \tau_{1,11} - \frac{1}{2} (s^2 - t^2 - u^2) \tau_{2,11} \right) + 2 s \tau_{1,7} (s \tau_{1,11} - 4 t \tau_{3,11}) + \\
& (s^2 - t^2 - u^2) (\tau_{1,10}^2 + 4 \tau_{3,6} \tau_{1,10} + \tau_{2,9}^2 + \tau_{2,12}^2 + \tau_{3,6}^2 + \tau_{3,11}^2 + \tau_{4,5}^2 + \tau_{4,8}^2 + 2 \tau_{2,8} \tau_{2,12} + \\
& \quad \tau_{2,8} \tau_{3,5} + \tau_{2,10} \tau_{3,7} + 2 \tau_{2,11} \tau_{3,7} + 2 \tau_{3,7} \tau_{3,11} + 2 \tau_{2,8} \tau_{3,12} + 4 \tau_{2,9} \tau_{4,5} + \tau_{1,11} \tau_{4,6} + \\
& \quad 2 \tau_{1,11} \tau_{4,7} - \tau_{3,10} \tau_{4,7} + 4 \tau_{2,12} \tau_{4,8} - \tau_{3,12} \tau_{4,9} - \tau_{1,8} (\tau_{2,5} - 2 \tau_{4,12}) + \tau_{1,9} \tau_{4,12} + 2 \tau_{4,8} \tau_{4,12}) + \\
& 2 u^2 (\tau_{2,5} \tau_{2,8} + (\tau_{2,12} + \tau_{3,5} + \tau_{3,12}) \tau_{2,8} + \tau_{2,10} \tau_{3,7} + \tau_{2,11} \tau_{3,7} + \tau_{3,7} \tau_{3,10} + \tau_{3,7} \tau_{3,11} + \tau_{1,11} \tau_{4,6} + \tau_{1,11} \tau_{4,7} + \\
& \quad \tau_{1,8} \tau_{4,12} + \tau_{1,9} \tau_{4,12} + \tau_{4,8} \tau_{4,12} + \tau_{4,9} \tau_{4,12}) + u (-s^2 + t^2 + u^2) (\tau_{5,8} + \tau_{6,11} + \tau_{7,10} + \tau_{9,12} + 2 l_{14}^2 + 2 l_{15}^2) \Big)
\end{aligned}$$

■  $N_{50}^{(3)}$

$$-\frac{1}{8} s t$$

$$\left( -(2 \tau_{3,11} \tau_{5,8} + 2 \tau_{2,9} \tau_{6,11} + 2 \tau_{2,12} \tau_{6,11} + 2 \tau_{4,5} \tau_{6,11} + 2 \tau_{4,8} \tau_{6,11} + 2 \tau_{2,9} \tau_{7,10} + 2 \tau_{2,12} \tau_{7,10} + 2 \tau_{4,5} \tau_{7,10} + 2 \tau_{4,8} \tau_{7,10} + 2 \right.$$

$$\begin{aligned} & \tau_{3,11} \tau_{9,12} + 2 \tau_{1,10} (\tau_{5,8} + \tau_{9,12}) + 2 \tau_{3,6} (\tau_{5,8} + \tau_{9,12}) - 2 \tau_{1,9} l_{13}^2 - 2 \tau_{1,15} l_{13}^2 + 2 \tau_{1,16} l_{13}^2 - 2 \tau_{2,10} l_{13}^2 - 2 \tau_{2,14} l_{13}^2 + \\ & 2 \tau_{2,16} l_{13}^2 - 2 \tau_{3,7} l_{13}^2 + 4 \tau_{3,12} l_{13}^2 - 4 \tau_{3,15} l_{13}^2 + 4 \tau_{4,7} l_{13}^2 - 2 \tau_{4,12} l_{13}^2 - 4 \tau_{4,14} l_{13}^2 + 4 \tau_{1,9} l_{14}^2 + 4 \tau_{1,17} l_{14}^2 - \\ & 2 \tau_{2,11} l_{14}^2 - 2 \tau_{2,13} l_{14}^2 - 2 \tau_{2,16} l_{14}^2 - 2 \tau_{3,12} l_{14}^2 - 2 \tau_{3,16} l_{14}^2 + 2 \tau_{3,17} l_{14}^2 + 4 \tau_{4,6} l_{14}^2 - 2 \tau_{4,9} l_{14}^2 - 4 \tau_{4,13} l_{14}^2 - \\ & 2 \tau_{1,8} l_{15}^2 - 2 \tau_{1,13} l_{15}^2 - 2 \tau_{1,16} l_{15}^2 - 2 \tau_{2,5} l_{15}^2 + 4 \tau_{2,10} l_{15}^2 + 4 \tau_{2,17} l_{15}^2 + 4 \tau_{3,5} l_{15}^2 - 2 \tau_{3,10} l_{15}^2 - 4 \tau_{3,13} l_{15}^2 - \\ & 2 \tau_{4,7} l_{15}^2 - 2 \tau_{4,16} l_{15}^2 + 2 \tau_{4,17} l_{15}^2 + \tau_{1,11} l_{16}^2 + \tau_{1,13} l_{16}^2 + \tau_{1,15} l_{16}^2 + \tau_{2,5} l_{16}^2 + \tau_{2,8} l_{16}^2 + \tau_{2,13} l_{16}^2 + \tau_{2,14} l_{16}^2 + \tau_{3,7} l_{16}^2 + \\ & \tau_{3,10} l_{16}^2 + \tau_{3,14} l_{16}^2 - \tau_{3,17} l_{16}^2 + \tau_{4,9} l_{16}^2 + \tau_{4,12} l_{16}^2 + \tau_{4,15} l_{16}^2 - \tau_{4,17} l_{16}^2 + 4 \tau_{1,8} l_{17}^2 - 2 \tau_{1,11} l_{17}^2 - 4 \tau_{1,14} l_{17}^2 - \\ & 2 \tau_{2,8} l_{17}^2 + 4 \tau_{2,11} l_{17}^2 - 4 \tau_{2,15} l_{17}^2 - 2 \tau_{3,5} l_{17}^2 - 2 \tau_{3,14} l_{17}^2 + 2 \tau_{3,16} l_{17}^2 - 2 \tau_{4,6} l_{17}^2 - 2 \tau_{4,15} l_{17}^2 + 2 \tau_{4,16} l_{17}^2) t^2 - \\ & 2 (2 \tau_{3,6} \tau_{1,10}^2 + 2 \tau_{3,6}^2 \tau_{1,10} - \tau_{2,8} \tau_{3,5} \tau_{1,10} + \tau_{3,6} \tau_{3,10} \tau_{1,10} + \tau_{3,10} \tau_{4,6} \tau_{1,10} + \tau_{3,12} \tau_{4,9} \tau_{1,10} + \tau_{2,5} \tau_{2,9}^2 - \\ & \tau_{2,8} \tau_{2,12}^2 - \tau_{3,7} \tau_{3,11}^2 + 2 \tau_{2,9} \tau_{4,5}^2 - 2 \tau_{2,12} \tau_{4,8}^2 - \tau_{2,8} \tau_{3,5} \tau_{3,6} - \tau_{2,9} \tau_{2,10} \tau_{3,7} - \tau_{2,10} \tau_{2,12} \tau_{3,7} + \\ & \tau_{3,6}^2 \tau_{3,10} - \tau_{2,8} \tau_{3,5} \tau_{3,11} - \tau_{2,11} \tau_{3,7} \tau_{3,11} - \tau_{2,8} \tau_{2,12} \tau_{3,12} + 2 \tau_{2,9}^2 \tau_{4,5} + \tau_{2,5} \tau_{2,9} \tau_{4,5} - \tau_{2,10} \tau_{3,7} \tau_{4,5} - \\ & \tau_{1,11} \tau_{2,9} \tau_{4,6} - \tau_{1,11} \tau_{2,12} \tau_{4,6} + \tau_{3,6} \tau_{3,10} \tau_{4,6} - \tau_{1,11} \tau_{4,5} \tau_{4,6} + \tau_{2,9} \tau_{3,10} \tau_{4,7} + \tau_{2,12} \tau_{3,10} \tau_{4,7} - \\ & \tau_{1,11} \tau_{3,11} \tau_{4,7} + \tau_{3,10} \tau_{4,5} \tau_{4,7} - 2 \tau_{2,12}^2 \tau_{4,8} - \tau_{2,8} \tau_{2,12} \tau_{4,8} - \tau_{2,10} \tau_{3,7} \tau_{4,8} - \tau_{2,8} \tau_{3,12} \tau_{4,8} - \\ & \tau_{1,11} \tau_{4,6} \tau_{4,8} + \tau_{3,10} \tau_{4,7} \tau_{4,8} + \tau_{4,5}^2 \tau_{4,9} + \tau_{2,9} \tau_{3,5} \tau_{4,9} + \tau_{3,6} \tau_{3,12} \tau_{4,9} + \tau_{3,11} \tau_{3,12} \tau_{4,9} + \tau_{2,9} \tau_{4,5} \tau_{4,9} + \\ & \tau_{3,5} \tau_{4,5} \tau_{4,9} - \tau_{4,8}^2 \tau_{4,12} - \tau_{2,12} \tau_{4,8} \tau_{4,12} + \tau_{1,9} (\tau_{2,5} (\tau_{2,9} + \tau_{4,5}) - (\tau_{1,10} + \tau_{3,6} + \tau_{3,11}) \tau_{4,12}) + \\ & \tau_{1,8} (\tau_{1,10} \tau_{2,5} + (\tau_{3,6} + \tau_{3,11}) \tau_{2,5} - (\tau_{2,12} + \tau_{4,8}) \tau_{4,12})) t - 2 \tau_{1,7}^2 (s \tau_{1,11} - 2 t \tau_{3,11}) + \\ & 2 u (-2 \tau_{3,6} \tau_{1,10}^2 + (-2 \tau_{3,6}^2 + \tau_{2,5} \tau_{2,8} + \tau_{2,8} \tau_{3,5} + \tau_{1,9} \tau_{4,12} + \tau_{4,9} \tau_{4,12}) \tau_{1,10} + \tau_{3,7} \tau_{3,11}^2 - 2 \tau_{2,9} \tau_{4,5}^2 + \\ & \tau_{2,9} \tau_{2,10} \tau_{3,7} + \tau_{2,10} \tau_{2,12} \tau_{3,7} + \tau_{2,9} \tau_{3,7} \tau_{3,10} + \tau_{2,12} \tau_{3,7} \tau_{3,10} + \tau_{2,11} \tau_{3,7} \tau_{3,11} - 2 \tau_{2,9}^2 \tau_{4,5} + \tau_{2,10} \tau_{3,7} \tau_{4,5} + \\ & \tau_{3,7} \tau_{3,10} \tau_{4,5} + \tau_{1,11} \tau_{2,9} \tau_{4,6} + \tau_{1,11} \tau_{2,12} \tau_{4,6} + \tau_{1,11} \tau_{4,5} \tau_{4,6} + \tau_{1,11} \tau_{3,11} \tau_{4,7} + \tau_{2,10} \tau_{3,7} \tau_{4,8} + \tau_{3,7} \tau_{3,10} \tau_{4,8} + \\ & \tau_{1,11} \tau_{4,6} \tau_{4,8} + \tau_{2,8} (\tau_{2,12}^2 + (\tau_{3,12} + \tau_{4,8}) \tau_{2,12} + \tau_{3,5} \tau_{3,6} + \tau_{3,5} \tau_{3,11} + \tau_{2,5} (\tau_{3,6} + \tau_{3,11}) + \tau_{3,12} \tau_{4,8}) + \tau_{4,8}^2 \tau_{4,12} + \\ & \tau_{1,8} \tau_{2,12} \tau_{4,12} + \tau_{1,9} \tau_{3,6} \tau_{4,12} + \tau_{1,9} \tau_{3,11} \tau_{4,12} + \tau_{1,8} \tau_{4,8} \tau_{4,12} + \tau_{2,12} \tau_{4,8} \tau_{4,12} + \tau_{3,6} \tau_{4,9} \tau_{4,12} + \tau_{3,11} \tau_{4,9} \tau_{4,12}) - 2 \tau_{1,7} \\ & \left( (\tau_{5,8} + \tau_{9,12}) t^2 + \tau_{1,8} \tau_{2,5} t - (2 \tau_{3,11}^2 + \tau_{1,11} \tau_{3,11} + \tau_{3,7} \tau_{3,11} + \tau_{2,8} \tau_{3,5} + \tau_{2,11} \tau_{3,7} + \tau_{1,11} \tau_{4,7} - \tau_{3,12} \tau_{4,9} + \tau_{1,9} \tau_{4,12}) t - \right. \\ & u (\tau_{2,5} \tau_{2,8} + \tau_{3,5} \tau_{2,8} + \tau_{2,11} \tau_{3,7} + \tau_{1,11} \tau_{3,11} + \tau_{3,7} \tau_{3,11} + \tau_{1,11} \tau_{4,7} + \tau_{1,9} \tau_{4,12} + \tau_{4,9} \tau_{4,12}) + \\ & \left. \frac{1}{2} (s^2 - t^2 - u^2) (\tau_{5,8} + \tau_{9,12}) \right) - \\ & 4 u^2 (\tau_{1,9} l_{14}^2 + \tau_{1,17} l_{14}^2 + \tau_{4,6} l_{14}^2 - \tau_{4,13} l_{14}^2 + \tau_{2,10} l_{15}^2 + \tau_{2,17} l_{15}^2 + \tau_{3,5} l_{15}^2 - \tau_{3,13} l_{15}^2) + \\ & \tau_{1,6} \left( (2 l_{14}^2 - l_{16}^2) t^2 - 2 (\tau_{1,10}^2 + (\tau_{2,10} + \tau_{3,6}) \tau_{1,10} + \tau_{2,9} \tau_{2,11} + \tau_{2,11} \tau_{2,12} + \tau_{2,10} \tau_{3,6} + \tau_{2,11} \tau_{4,5} + \tau_{2,11} \tau_{4,8}) t + \right. \end{aligned}$$

$$\begin{aligned}
& 2u\tau_{1,11}(\tau_{2,9} + \tau_{2,12} + \tau_{4,5} + \tau_{4,8}) + \frac{1}{2}(s^2 - t^2 - u^2)(2l_{14}^2 - l_{16}^2) \Big) - \\
& \frac{1}{2}(s^2 - t^2 - u^2) \Big( 2\tau_{3,11}\tau_{5,8} + 2\tau_{2,9}\tau_{6,11} + 2\tau_{2,12}\tau_{6,11} + 2\tau_{4,5}\tau_{6,11} + 2\tau_{4,8}\tau_{6,11} + 2\tau_{2,9}\tau_{7,10} + 2\tau_{2,12}\tau_{7,10} + 2\tau_{4,5}\tau_{7,10} + \\
& 2\tau_{4,8}\tau_{7,10} + 2\tau_{3,11}\tau_{9,12} + 2\tau_{1,10}(\tau_{5,8} + \tau_{9,12}) + 2\tau_{3,6}(\tau_{5,8} + \tau_{9,12}) - 2\tau_{1,9}l_{13}^2 - 2\tau_{1,15}l_{13}^2 + 2\tau_{1,16}l_{13}^2 - 2\tau_{2,10}l_{13}^2 - \\
& 2\tau_{2,14}l_{13}^2 + 2\tau_{2,16}l_{13}^2 - 2\tau_{3,7}l_{13}^2 - 2\tau_{4,12}l_{13}^2 + 8\tau_{1,9}l_{14}^2 + 8\tau_{1,17}l_{14}^2 - 2\tau_{2,11}l_{14}^2 - 2\tau_{2,13}l_{14}^2 - 2\tau_{2,16}l_{14}^2 - \\
& 2\tau_{3,12}l_{14}^2 - 2\tau_{3,16}l_{14}^2 + 2\tau_{3,17}l_{14}^2 + 8\tau_{4,6}l_{14}^2 - 2\tau_{4,9}l_{14}^2 - 8\tau_{4,13}l_{14}^2 - 2\tau_{1,8}l_{15}^2 - 2\tau_{1,13}l_{15}^2 - 2\tau_{1,16}l_{15}^2 - 2\tau_{2,5}l_{15}^2 + \\
& 8\tau_{2,10}l_{15}^2 + 8\tau_{2,17}l_{15}^2 + 8\tau_{3,5}l_{15}^2 - 2\tau_{3,10}l_{15}^2 - 8\tau_{3,13}l_{15}^2 - 2\tau_{4,7}l_{15}^2 - 2\tau_{4,16}l_{15}^2 + 2\tau_{4,17}l_{15}^2 + \tau_{1,11}l_{16}^2 + \tau_{1,13}l_{16}^2 + \\
& \tau_{1,15}l_{16}^2 + \tau_{2,5}l_{16}^2 + \tau_{2,8}l_{16}^2 + \tau_{2,13}l_{16}^2 + \tau_{2,14}l_{16}^2 + \tau_{3,7}l_{16}^2 + \tau_{3,10}l_{16}^2 + \tau_{3,14}l_{16}^2 - \tau_{3,17}l_{16}^2 + \tau_{4,9}l_{16}^2 + \tau_{4,12}l_{16}^2 + \\
& \tau_{4,15}l_{16}^2 - \tau_{4,17}l_{16}^2 - 2\tau_{1,11}l_{17}^2 - 2\tau_{2,8}l_{17}^2 - 2\tau_{3,5}l_{17}^2 - 2\tau_{3,14}l_{17}^2 + 2\tau_{3,16}l_{17}^2 - 2\tau_{4,6}l_{17}^2 - 2\tau_{4,15}l_{17}^2 + 2\tau_{4,16}l_{17}^2 \Big)
\end{aligned}$$

■  $N_{50}^{(4)}$

$$\frac{1}{8}$$

$$\begin{aligned}
& \Big( (2\tau_{5,8}^2 + (-2l_{15}^2 + l_{16}^2 - 2l_{17}^2)\tau_{5,8} + 2\tau_{6,11}^2 + 2\tau_{7,10}^2 + 2\tau_{9,12}^2 - 2\tau_{7,10}l_{13}^2 - 2\tau_{7,16}l_{13}^2 - 2\tau_{9,12}l_{13}^2 - 2\tau_{12,16}l_{13}^2 + 2\tau_{6,16}l_{14}^2 - \\
& 2\tau_{9,12}l_{14}^2 + 2\tau_{9,16}l_{14}^2 + 2\tau_{5,16}l_{15}^2 - 2\tau_{7,10}l_{15}^2 + 2\tau_{10,16}l_{15}^2 + \tau_{7,10}l_{16}^2 + \tau_{9,12}l_{16}^2 + \tau_{13,14}l_{16}^2 + \\
& \tau_{13,15}l_{16}^2 - \tau_{14,17}l_{16}^2 - \tau_{15,17}l_{16}^2 + \tau_{6,11}(-2l_{14}^2 + l_{16}^2 - 2l_{17}^2) - 2\tau_{8,16}l_{17}^2 - 2\tau_{11,16}l_{17}^2)t^4 + \\
& (-4l_{15}^2\tau_{1,13}^2 - 4\tau_{1,16}l_{15}^2\tau_{1,13} - 4\tau_{2,5}l_{15}^2\tau_{1,13} + 4\tau_{2,8}l_{15}^2\tau_{1,13} - 4\tau_{2,16}l_{15}^2\tau_{1,13} + 4\tau_{3,5}l_{15}^2\tau_{1,13} - 4\tau_{3,13}l_{15}^2\tau_{1,13} + \\
& \tau_{2,5}l_{16}^2\tau_{1,13} + \tau_{2,15}l_{16}^2\tau_{1,13} + \tau_{3,12}l_{16}^2\tau_{1,13} - \tau_{3,15}l_{16}^2\tau_{1,13} - 4\tau_{2,8}\tau_{3,5}\tau_{5,8} + 2\tau_{1,10}\tau_{3,6}\tau_{5,8} - 2\tau_{2,11}\tau_{3,7}\tau_{5,8} - \\
& 2\tau_{1,7}\tau_{3,11}\tau_{5,8} - 2\tau_{3,7}\tau_{3,11}\tau_{5,8} + 2\tau_{1,9}\tau_{2,5}\tau_{6,11} + 2\tau_{2,5}\tau_{2,9}\tau_{6,11} + 2\tau_{2,9}\tau_{4,5}\tau_{6,11} - 4\tau_{1,11}\tau_{4,6}\tau_{6,11} - \\
& 2\tau_{2,12}\tau_{4,8}\tau_{6,11} - 2\tau_{4,8}\tau_{4,12}\tau_{6,11} - 2\tau_{2,8}\tau_{2,12}\tau_{7,10} - 4\tau_{2,10}\tau_{3,7}\tau_{7,10} - 2\tau_{2,8}\tau_{3,12}\tau_{7,10} + 2\tau_{2,9}\tau_{4,5}\tau_{7,10} + \\
& 4\tau_{3,10}\tau_{4,7}\tau_{7,10} - 2\tau_{2,12}\tau_{4,8}\tau_{7,10} + 2\tau_{3,5}\tau_{4,9}\tau_{7,10} + 2\tau_{4,5}\tau_{4,9}\tau_{7,10} - 2\tau_{1,7}\tau_{1,11}\tau_{9,12} + 2\tau_{1,10}\tau_{3,6}\tau_{9,12} + \\
& 2\tau_{3,6}\tau_{3,10}\tau_{9,12} - 2\tau_{1,7}\tau_{3,11}\tau_{9,12} + 2\tau_{3,10}\tau_{4,6}\tau_{9,12} - 2\tau_{1,11}\tau_{4,7}\tau_{9,12} + 4\tau_{3,12}\tau_{4,9}\tau_{9,12} - 4\tau_{1,9}\tau_{4,12}\tau_{9,12} + \\
& 4\tau_{1,15}^2l_{13}^2 + 4\tau_{2,14}^2l_{13}^2 + 4\tau_{1,9}\tau_{1,15}l_{13}^2 - 4\tau_{1,15}\tau_{1,16}l_{13}^2 + 4\tau_{2,10}\tau_{2,14}l_{13}^2 - 4\tau_{2,14}\tau_{2,16}l_{13}^2 + 4\tau_{2,10}\tau_{3,7}l_{13}^2 + \\
& 4\tau_{2,14}\tau_{3,7}l_{13}^2 - 4\tau_{2,14}\tau_{3,10}l_{13}^2 - 4\tau_{1,9}\tau_{3,12}l_{13}^2 - 4\tau_{1,15}\tau_{3,12}l_{13}^2 + 4\tau_{1,16}\tau_{3,12}l_{13}^2 + 4\tau_{1,9}\tau_{3,15}l_{13}^2 + 4\tau_{1,15}\tau_{3,15}l_{13}^2 - \\
& 4\tau_{1,16}\tau_{3,15}l_{13}^2 - 4\tau_{2,14}\tau_{3,16}l_{13}^2 - 4\tau_{2,10}\tau_{4,7}l_{13}^2 - 4\tau_{2,14}\tau_{4,7}l_{13}^2 + 4\tau_{2,16}\tau_{4,7}l_{13}^2 - 4\tau_{3,10}\tau_{4,7}l_{13}^2 - 4\tau_{1,15}\tau_{4,9}l_{13}^2 - \\
& 4\tau_{3,12}\tau_{4,9}l_{13}^2 + 4\tau_{1,9}\tau_{4,12}l_{13}^2 + 4\tau_{1,15}\tau_{4,12}l_{13}^2 + 4\tau_{2,10}\tau_{4,14}l_{13}^2 + 4\tau_{2,14}\tau_{4,14}l_{13}^2 - 4\tau_{2,16}\tau_{4,14}l_{13}^2 - \\
& 4\tau_{1,15}\tau_{4,16}l_{13}^2 - 4\tau_{2,13}^2l_{14}^2 - 4\tau_{3,17}^2l_{14}^2 + 4\tau_{1,11}\tau_{2,13}l_{14}^2 - 4\tau_{1,16}\tau_{2,13}l_{14}^2 - 4\tau_{2,11}\tau_{2,13}l_{14}^2 - 4\tau_{2,13}\tau_{2,16}l_{14}^2 + \\
& 4\tau_{1,9}\tau_{3,12}l_{14}^2 + 4\tau_{1,17}\tau_{3,12}l_{14}^2 + 4\tau_{1,9}\tau_{3,16}l_{14}^2 + 4\tau_{1,17}\tau_{3,16}l_{14}^2 - 4\tau_{1,9}\tau_{3,17}l_{14}^2 - 4\tau_{1,17}\tau_{3,17}l_{14}^2 + 4\tau_{3,12}\tau_{3,17}l_{14}^2 + \\
& 4\tau_{3,16}\tau_{3,17}l_{14}^2 + 4\tau_{1,11}\tau_{4,6}l_{14}^2 + 4\tau_{2,11}\tau_{4,6}l_{14}^2 + 4\tau_{2,13}\tau_{4,6}l_{14}^2 + 4\tau_{2,16}\tau_{4,6}l_{14}^2 - 4\tau_{3,12}\tau_{4,9}l_{14}^2 + 4\tau_{3,17}\tau_{4,9}l_{14}^2 + \\
& 4\tau_{1,9}\tau_{4,12}l_{14}^2 - 4\tau_{3,17}\tau_{4,12}l_{14}^2 - 4\tau_{2,11}\tau_{4,13}l_{14}^2 - 4\tau_{2,13}\tau_{4,13}l_{14}^2 - 4\tau_{2,16}\tau_{4,13}l_{14}^2 + 4\tau_{3,17}\tau_{4,16}l_{14}^2 - \\
& 4\tau_{4,17}^2l_{15}^2 + 4\tau_{1,16}\tau_{3,5}l_{15}^2 + 4\tau_{2,8}\tau_{3,5}l_{15}^2 + 4\tau_{2,10}\tau_{3,7}l_{15}^2 - 4\tau_{1,16}\tau_{3,13}l_{15}^2 + 4\tau_{2,10}\tau_{4,7}l_{15}^2 + 4\tau_{2,17}\tau_{4,7}l_{15}^2 -
\end{aligned}$$

$$\begin{aligned}
& 4 \tau_{3,10} \tau_{4,7} l_{15}^2 + 4 \tau_{2,10} \tau_{4,16} l_{15}^2 + 4 \tau_{2,17} \tau_{4,16} l_{15}^2 - 4 \tau_{2,10} \tau_{4,17} l_{15}^2 - 4 \tau_{2,17} \tau_{4,17} l_{15}^2 - 4 \tau_{3,7} \tau_{4,17} l_{15}^2 + \\
& 4 \tau_{3,10} \tau_{4,17} l_{15}^2 + 4 \tau_{3,16} \tau_{4,17} l_{15}^2 + 4 \tau_{4,7} \tau_{4,17} l_{15}^2 + 4 \tau_{4,16} \tau_{4,17} l_{15}^2 + \tau_{1,14} \tau_{2,13} l_{16}^2 - \tau_{1,15} \tau_{3,5} l_{16}^2 - 2 \tau_{2,8} \tau_{3,5} l_{16}^2 - \\
& 2 \tau_{2,10} \tau_{3,7} l_{16}^2 - \tau_{2,14} \tau_{3,7} l_{16}^2 + \tau_{1,15} \tau_{3,13} l_{16}^2 - \tau_{2,14} \tau_{3,13} l_{16}^2 - \tau_{1,9} \tau_{3,14} l_{16}^2 - \tau_{1,17} \tau_{3,14} l_{16}^2 - \tau_{2,8} \tau_{3,14} l_{16}^2 + \\
& \tau_{2,17} \tau_{3,14} l_{16}^2 + \tau_{1,14} \tau_{3,17} l_{16}^2 - 2 \tau_{1,11} \tau_{4,6} l_{16}^2 - \tau_{2,14} \tau_{4,6} l_{16}^2 + \tau_{2,13} \tau_{4,7} l_{16}^2 + 2 \tau_{3,10} \tau_{4,7} l_{16}^2 + 2 \tau_{3,12} \tau_{4,9} l_{16}^2 - \\
& \tau_{3,17} \tau_{4,9} l_{16}^2 - 2 \tau_{1,9} \tau_{4,12} l_{16}^2 - \tau_{1,15} \tau_{4,12} l_{16}^2 - \tau_{1,15} \tau_{4,13} l_{16}^2 + \tau_{2,14} \tau_{4,13} l_{16}^2 - \tau_{2,13} \tau_{4,14} l_{16}^2 - \tau_{3,17} \tau_{4,14} l_{16}^2 - \\
& \tau_{1,11} \tau_{4,15} l_{16}^2 + \tau_{1,17} \tau_{4,15} l_{16}^2 - \tau_{2,10} \tau_{4,15} l_{16}^2 - \tau_{2,17} \tau_{4,15} l_{16}^2 - \tau_{2,11} \tau_{4,17} l_{16}^2 + \tau_{2,15} \tau_{4,17} l_{16}^2 - \tau_{3,10} \tau_{4,17} l_{16}^2 - \\
& \tau_{3,15} \tau_{4,17} l_{16}^2 + 4 \tau_{3,14}^2 l_{17}^2 + 4 \tau_{4,15}^2 l_{17}^2 + 4 \tau_{1,14} \tau_{3,5} l_{17}^2 + 4 \tau_{2,8} \tau_{3,5} l_{17}^2 + 4 \tau_{1,14} \tau_{3,14} l_{17}^2 - 4 \tau_{2,5} \tau_{3,14} l_{17}^2 + \\
& 4 \tau_{2,8} \tau_{3,14} l_{17}^2 - 4 \tau_{2,16} \tau_{3,14} l_{17}^2 + 4 \tau_{3,5} \tau_{3,14} l_{17}^2 - 4 \tau_{1,14} \tau_{3,16} l_{17}^2 - 4 \tau_{3,14} \tau_{3,16} l_{17}^2 + 4 \tau_{1,11} \tau_{4,6} l_{17}^2 - \\
& 4 \tau_{2,11} \tau_{4,6} l_{17}^2 + 4 \tau_{2,15} \tau_{4,6} l_{17}^2 + 4 \tau_{1,11} \tau_{4,15} l_{17}^2 - 4 \tau_{1,16} \tau_{4,15} l_{17}^2 - 4 \tau_{2,11} \tau_{4,15} l_{17}^2 + 4 \tau_{2,15} \tau_{4,15} l_{17}^2 + \\
& 4 \tau_{4,6} \tau_{4,15} l_{17}^2 + 4 \tau_{2,11} \tau_{4,16} l_{17}^2 - 4 \tau_{2,15} \tau_{4,16} l_{17}^2 - 4 \tau_{4,15} \tau_{4,16} l_{17}^2 + \tau_{1,8} (-2 \tau_{4,12} \tau_{6,11} - 4 \tau_{1,13} l_{15}^2 + 4 \tau_{3,5} l_{15}^2 - \\
& 4 \tau_{3,13} l_{15}^2 - \tau_{3,17} l_{16}^2 + 2 \tau_{2,5} (2 \tau_{5,8} - 2 l_{15}^2 + l_{16}^2 - 2 l_{17}^2) - 4 \tau_{3,5} l_{17}^2 - 4 \tau_{3,14} l_{17}^2 + 4 \tau_{3,16} l_{17}^2) + \\
& \tau_{1,6} (2 \tau_{1,10} \tau_{5,8} + 2 \tau_{2,10} \tau_{5,8} + 4 \tau_{2,11} \tau_{6,11} - 4 \tau_{2,11} l_{14}^2 - 4 \tau_{2,13} l_{14}^2 + 2 \tau_{2,11} l_{16}^2 + \tau_{2,13} l_{16}^2 - 4 \tau_{2,11} l_{17}^2 - 4 \tau_{4,15} l_{17}^2)) \\
& t^3 + ((\tau_{1,10}^2 + 2 \tau_{2,10} \tau_{1,10} + \tau_{2,10}^2 + 2 \tau_{2,11}^2) \tau_{1,6}^2 + \\
& 2 (\tau_{3,6} \tau_{1,10}^2 - \tau_{2,8} \tau_{3,5} \tau_{1,10} + \tau_{2,10} \tau_{3,6} \tau_{1,10} + \tau_{1,9} \tau_{2,5} \tau_{2,11} + \tau_{2,5} \tau_{2,9} \tau_{2,11} - \tau_{2,8} \tau_{2,10} \tau_{3,5} + \tau_{2,9} \tau_{2,11} \tau_{4,5} - \\
& 2 \tau_{1,11} \tau_{2,11} \tau_{4,6} - \tau_{2,11} \tau_{2,12} \tau_{4,8} - \tau_{2,11} \tau_{4,8} \tau_{4,12} + \tau_{1,8} (\tau_{1,10} \tau_{2,5} + \tau_{2,10} \tau_{2,5} - \tau_{2,11} \tau_{4,12})) \tau_{1,6} + \\
& 2 \tau_{1,8}^2 \tau_{2,5}^2 + \tau_{1,9}^2 \tau_{2,5}^2 + \tau_{2,5}^2 \tau_{2,9}^2 + \tau_{2,8}^2 \tau_{2,12}^2 + 2 \tau_{2,8}^2 \tau_{3,5}^2 + 2 \tau_{1,10}^2 \tau_{3,6}^2 + 2 \tau_{2,10}^2 \tau_{3,7}^2 + \\
& \tau_{2,11}^2 \tau_{3,7}^2 + \tau_{3,6}^2 \tau_{3,10}^2 + \tau_{3,7}^2 \tau_{3,11}^2 + \tau_{2,8}^2 \tau_{3,12}^2 + 2 \tau_{2,9}^2 \tau_{4,5}^2 + 2 \tau_{1,11}^2 \tau_{4,6}^2 + \tau_{3,10}^2 \tau_{4,6}^2 + \tau_{1,11}^2 \tau_{4,7}^2 + \\
& 2 \tau_{3,10}^2 \tau_{4,7}^2 + 2 \tau_{2,12}^2 \tau_{4,8}^2 + \tau_{3,5}^2 \tau_{4,9}^2 + 2 \tau_{3,12}^2 \tau_{4,9}^2 + \tau_{4,5}^2 \tau_{4,9}^2 + 2 \tau_{3,5} \tau_{4,5} \tau_{4,9}^2 + \tau_{1,8}^2 \tau_{4,12}^2 + \\
& 2 \tau_{1,9}^2 \tau_{4,12}^2 + \tau_{4,8}^2 \tau_{4,12}^2 + 2 \tau_{1,8} \tau_{4,8} \tau_{4,12}^2 + 2 \tau_{1,9} \tau_{2,5}^2 \tau_{2,9} - 4 \tau_{1,8} \tau_{2,5} \tau_{2,8} \tau_{3,5} + 2 \tau_{1,8} \tau_{1,10} \tau_{2,5} \tau_{3,6} - \\
& 2 \tau_{1,10} \tau_{2,8} \tau_{3,5} \tau_{3,6} - 2 \tau_{1,8} \tau_{2,5} \tau_{2,11} \tau_{3,7} + 2 \tau_{2,8} \tau_{2,10} \tau_{2,12} \tau_{3,7} + 2 \tau_{2,8} \tau_{2,11} \tau_{3,5} \tau_{3,7} + 2 \tau_{1,10} \tau_{3,6}^2 \tau_{3,10} + \\
& 2 \tau_{2,11} \tau_{3,7}^2 \tau_{3,11} - 2 \tau_{1,8} \tau_{2,5} \tau_{3,7} \tau_{3,11} + 2 \tau_{2,8} \tau_{3,5} \tau_{3,7} \tau_{3,11} + \tau_{1,7}^2 (\tau_{1,11}^2 + 2 \tau_{3,11} \tau_{1,11} + 2 \tau_{3,11}^2) + \\
& 2 \tau_{2,8}^2 \tau_{2,12} \tau_{3,12} + 2 \tau_{2,8} \tau_{2,10} \tau_{3,7} \tau_{3,12} + 2 \tau_{2,5} \tau_{2,9}^2 \tau_{4,5} + 2 \tau_{1,9} \tau_{2,5} \tau_{2,9} \tau_{4,5} - 2 \tau_{2,9} \tau_{2,10} \tau_{3,7} \tau_{4,5} + 2 \tau_{3,6} \tau_{3,10}^2 \tau_{4,6} - \\
& 2 \tau_{1,9} \tau_{1,11} \tau_{2,5} \tau_{4,6} - 2 \tau_{1,11} \tau_{2,5} \tau_{2,9} \tau_{4,6} + 2 \tau_{1,10} \tau_{3,6} \tau_{3,10} \tau_{4,6} - 2 \tau_{1,11} \tau_{2,9} \tau_{4,5} \tau_{4,6} - 2 \tau_{2,8} \tau_{2,12} \tau_{3,10} \tau_{4,7} - \\
& 4 \tau_{2,10} \tau_{3,7} \tau_{3,10} \tau_{4,7} - 2 \tau_{2,8} \tau_{3,10} \tau_{3,12} \tau_{4,7} + 2 \tau_{2,9} \tau_{3,10} \tau_{4,5} \tau_{4,7} + 2 \tau_{2,8} \tau_{2,12}^2 \tau_{4,8} + 2 \tau_{2,10} \tau_{2,12} \tau_{3,7} \tau_{4,8} + \\
& 2 \tau_{2,8} \tau_{2,12} \tau_{3,12} \tau_{4,8} + 2 \tau_{1,11} \tau_{2,12} \tau_{4,6} \tau_{4,8} - 2 \tau_{2,12} \tau_{3,10} \tau_{4,7} \tau_{4,8} + 2 \tau_{2,9} \tau_{4,5}^2 \tau_{4,9} - 2 \tau_{2,10} \tau_{3,5} \tau_{3,7} \tau_{4,9} + \\
& 2 \tau_{1,10} \tau_{3,6} \tau_{3,12} \tau_{4,9} + 2 \tau_{3,6} \tau_{3,10} \tau_{3,12} \tau_{4,9} + 2 \tau_{2,9} \tau_{3,5} \tau_{4,5} \tau_{4,9} - 2 \tau_{2,10} \tau_{3,7} \tau_{4,5} \tau_{4,9} + 2 \tau_{3,10} \tau_{3,12} \tau_{4,6} \tau_{4,9} + \\
& 2 \tau_{3,5} \tau_{3,10} \tau_{4,7} \tau_{4,9} - 2 \tau_{1,11} \tau_{3,12} \tau_{4,7} \tau_{4,9} + 2 \tau_{3,10} \tau_{4,5} \tau_{4,7} \tau_{4,9} + 2 \tau_{2,12} \tau_{4,8}^2 \tau_{4,12} - 2 \tau_{1,9} \tau_{1,10} \tau_{3,6} \tau_{4,12} - \\
& 2 \tau_{1,9} \tau_{3,6} \tau_{3,10} \tau_{4,12} + 2 \tau_{1,8} \tau_{1,11} \tau_{4,6} \tau_{4,12} - 2 \tau_{1,9} \tau_{3,10} \tau_{4,6} \tau_{4,12} + 2 \tau_{1,9} \tau_{1,11} \tau_{4,7} \tau_{4,12} + 2 \tau_{1,8} \tau_{2,12} \tau_{4,8} \tau_{4,12} + \\
& 2 \tau_{1,11} \tau_{4,6} \tau_{4,8} \tau_{4,12} - 4 \tau_{1,9} \tau_{3,12} \tau_{4,9} \tau_{4,12} + 2 \tau_{1,7} (\tau_{4,7} \tau_{1,11}^2 + \tau_{3,11} \tau_{4,7} \tau_{1,11} - \tau_{3,12} \tau_{4,9} \tau_{1,11} + \tau_{1,9} \tau_{4,12} \tau_{1,11} + \\
& \tau_{3,7} \tau_{3,11}^2 - \tau_{1,8} \tau_{2,5} \tau_{3,11} + \tau_{2,8} \tau_{3,5} \tau_{3,11} + \tau_{2,11} \tau_{3,7} \tau_{3,11} - \tau_{3,11} \tau_{3,12} \tau_{4,9} + \tau_{1,9} \tau_{3,11} \tau_{4,12})) t^2 + \\
& (s^2 - t^2 - u^2) (2 \tau_{5,8}^2 + (-2 l_{15}^2 + l_{16}^2 - 2 l_{17}^2) \tau_{5,8} + 2 \tau_{6,11}^2 + 2 \tau_{7,10}^2 + 2 \tau_{9,12}^2 - 2 \tau_{7,10} l_{13}^2 - 2 \tau_{7,16} l_{13}^2 - \\
& 2 \tau_{9,12} l_{13}^2 - 2 \tau_{12,16} l_{13}^2 + 2 \tau_{6,16} l_{14}^2 - 2 \tau_{9,12} l_{14}^2 + 2 \tau_{9,16} l_{14}^2 + 2 \tau_{5,16} l_{15}^2 - 2 \tau_{7,10} l_{15}^2 + 2 \tau_{10,16} l_{15}^2 + \tau_{7,10} l_{16}^2 + \\
& \tau_{9,12} l_{16}^2 + \tau_{13,14} l_{16}^2 + \tau_{13,15} l_{16}^2 - \tau_{14,17} l_{16}^2 - \tau_{15,17} l_{16}^2 + \tau_{6,11} (-2 l_{14}^2 + l_{16}^2 - 2 l_{17}^2) - 2 \tau_{8,16} l_{17}^2 - 2 \tau_{11,16} l_{17}^2) t^2 -
\end{aligned}$$

$$\begin{aligned}
& \frac{1}{2} u (-s^2 + t^2 + u^2) (2 \tau_{5,8}^2 + (-2 l_{15}^2 + l_{16}^2 - 2 l_{17}^2) \tau_{5,8} + 2 \tau_{6,11}^2 + 2 \tau_{7,10}^2 + 2 \tau_{9,12}^2 - 2 \tau_{7,10} l_{13}^2 - 2 \tau_{7,16} l_{13}^2 - \\
& \quad 2 \tau_{9,12} l_{13}^2 - 2 \tau_{12,16} l_{13}^2 + 2 \tau_{6,16} l_{14}^2 - 2 \tau_{9,12} l_{14}^2 + 2 \tau_{9,16} l_{14}^2 + 2 \tau_{5,16} l_{15}^2 - 2 \tau_{7,10} l_{15}^2 + 2 \tau_{10,16} l_{15}^2 + \tau_{7,10} l_{16}^2 + \\
& \quad \tau_{9,12} l_{16}^2 + \tau_{13,14} l_{16}^2 + \tau_{13,15} l_{16}^2 - \tau_{14,17} l_{16}^2 - \tau_{15,17} l_{16}^2 + \tau_{6,11} (-2 l_{14}^2 + l_{16}^2 - 2 l_{17}^2) - 2 \tau_{8,16} l_{17}^2 - 2 \tau_{11,16} l_{17}^2) t + \\
& \frac{1}{2} (-s^2 + t^2 + u^2) (4 l_{15}^2 \tau_{1,13}^2 + 4 \tau_{1,16} l_{15}^2 \tau_{1,13} + 4 \tau_{2,5} l_{15}^2 \tau_{1,13} - 12 \tau_{2,8} l_{15}^2 \tau_{1,13} + 4 \tau_{2,16} l_{15}^2 \tau_{1,13} - 8 \tau_{3,5} l_{15}^2 \tau_{1,13} + \\
& \quad 8 \tau_{3,13} l_{15}^2 \tau_{1,13} + \tau_{1,15} l_{16}^2 \tau_{1,13} - \tau_{2,5} l_{16}^2 \tau_{1,13} - \tau_{2,15} l_{16}^2 \tau_{1,13} - \tau_{3,12} l_{16}^2 \tau_{1,13} + \tau_{3,15} l_{16}^2 \tau_{1,13} + 4 \tau_{2,5} \tau_{2,8} \tau_{5,8} + \\
& \quad 8 \tau_{2,8} \tau_{3,5} \tau_{5,8} - 4 \tau_{1,10} \tau_{3,6} \tau_{5,8} + 4 \tau_{2,11} \tau_{3,7} \tau_{5,8} + 2 \tau_{1,7} \tau_{3,11} \tau_{5,8} + 4 \tau_{3,7} \tau_{3,11} \tau_{5,8} - 2 \tau_{1,9} \tau_{2,5} \tau_{6,11} - \\
& \quad 2 \tau_{2,5} \tau_{2,9} \tau_{6,11} - 4 \tau_{2,9} \tau_{4,5} \tau_{6,11} + 8 \tau_{1,11} \tau_{4,6} \tau_{6,11} + 2 \tau_{2,12} \tau_{4,8} \tau_{6,11} + 4 \tau_{4,8} \tau_{4,12} \tau_{6,11} + 4 \tau_{2,8} \tau_{2,12} \tau_{7,10} + \\
& \quad 8 \tau_{2,10} \tau_{3,7} \tau_{7,10} + 4 \tau_{3,7} \tau_{3,10} \tau_{7,10} + 4 \tau_{2,8} \tau_{3,12} \tau_{7,10} - 4 \tau_{2,9} \tau_{4,5} \tau_{7,10} - 4 \tau_{3,10} \tau_{4,7} \tau_{7,10} + 2 \tau_{2,12} \tau_{4,8} \tau_{7,10} - \\
& \quad 2 \tau_{3,5} \tau_{4,9} \tau_{7,10} - 2 \tau_{4,5} \tau_{4,9} \tau_{7,10} + 4 \tau_{1,7} \tau_{1,11} \tau_{9,12} - 4 \tau_{1,10} \tau_{3,6} \tau_{9,12} - 2 \tau_{3,6} \tau_{3,10} \tau_{9,12} + 2 \tau_{1,7} \tau_{3,11} \tau_{9,12} - \\
& \quad 2 \tau_{3,10} \tau_{4,6} \tau_{9,12} + 4 \tau_{1,11} \tau_{4,7} \tau_{9,12} - 4 \tau_{3,12} \tau_{4,9} \tau_{9,12} + 8 \tau_{1,9} \tau_{4,12} \tau_{9,12} + 4 \tau_{4,9} \tau_{4,12} \tau_{9,12} - 8 \tau_{1,15}^2 l_{13}^2 - \\
& \quad 8 \tau_{2,14}^2 l_{13}^2 - 8 \tau_{1,9} \tau_{1,15} l_{13}^2 + 8 \tau_{1,15} \tau_{1,16} l_{13}^2 - 8 \tau_{2,10} \tau_{2,14} l_{13}^2 + 8 \tau_{2,14} \tau_{2,16} l_{13}^2 - 8 \tau_{2,10} \tau_{3,7} l_{13}^2 - 8 \tau_{2,14} \tau_{3,7} l_{13}^2 - \\
& \quad 4 \tau_{3,7} \tau_{3,10} l_{13}^2 + 4 \tau_{1,9} \tau_{3,12} l_{13}^2 + 4 \tau_{1,15} \tau_{3,12} l_{13}^2 - 4 \tau_{1,16} \tau_{3,12} l_{13}^2 - 4 \tau_{1,9} \tau_{3,15} l_{13}^2 - 4 \tau_{1,15} \tau_{3,15} l_{13}^2 + 4 \tau_{1,16} \tau_{3,15} l_{13}^2 + \\
& \quad 8 \tau_{2,14} \tau_{3,16} l_{13}^2 + 4 \tau_{2,10} \tau_{4,7} l_{13}^2 + 4 \tau_{2,14} \tau_{4,7} l_{13}^2 - 4 \tau_{2,16} \tau_{4,7} l_{13}^2 + 4 \tau_{3,10} \tau_{4,7} l_{13}^2 + 4 \tau_{3,12} \tau_{4,9} l_{13}^2 - 8 \tau_{1,9} \tau_{4,12} l_{13}^2 - \\
& \quad 8 \tau_{1,15} \tau_{4,12} l_{13}^2 - 4 \tau_{4,9} \tau_{4,12} l_{13}^2 - 4 \tau_{2,10} \tau_{4,14} l_{13}^2 - 4 \tau_{2,14} \tau_{4,14} l_{13}^2 + 4 \tau_{2,16} \tau_{4,14} l_{13}^2 + 8 \tau_{1,15} \tau_{4,16} l_{13}^2 + 4 \tau_{2,13}^2 l_{14}^2 + \\
& \quad 4 \tau_{3,17}^2 l_{14}^2 - 12 \tau_{1,11} \tau_{2,13} l_{14}^2 + 4 \tau_{1,16} \tau_{2,13} l_{14}^2 + 4 \tau_{2,11} \tau_{2,13} l_{14}^2 + 4 \tau_{2,13} \tau_{2,16} l_{14}^2 - 8 \tau_{1,9} \tau_{3,12} l_{14}^2 - 8 \tau_{1,17} \tau_{3,12} l_{14}^2 - \\
& \quad 8 \tau_{1,9} \tau_{3,16} l_{14}^2 - 8 \tau_{1,17} \tau_{3,16} l_{14}^2 + 8 \tau_{1,9} \tau_{3,17} l_{14}^2 + 8 \tau_{1,17} \tau_{3,17} l_{14}^2 - 4 \tau_{3,12} \tau_{3,17} l_{14}^2 - 4 \tau_{3,16} \tau_{3,17} l_{14}^2 - 8 \tau_{1,11} \tau_{4,6} l_{14}^2 - \\
& \quad 8 \tau_{2,11} \tau_{4,6} l_{14}^2 - 8 \tau_{2,13} \tau_{4,6} l_{14}^2 - 8 \tau_{2,16} \tau_{4,6} l_{14}^2 + 4 \tau_{3,12} \tau_{4,9} l_{14}^2 - 4 \tau_{3,17} \tau_{4,9} l_{14}^2 - 8 \tau_{1,9} \tau_{4,12} l_{14}^2 + 12 \tau_{3,17} \tau_{4,12} l_{14}^2 - \\
& \quad 4 \tau_{4,9} \tau_{4,12} l_{14}^2 + 8 \tau_{2,11} \tau_{4,13} l_{14}^2 + 8 \tau_{2,13} \tau_{4,13} l_{14}^2 + 8 \tau_{2,16} \tau_{4,13} l_{14}^2 - 4 \tau_{3,17} \tau_{4,16} l_{14}^2 + 4 \tau_{4,17}^2 l_{15}^2 - 4 \tau_{2,5} \tau_{2,8} l_{15}^2 - \\
& \quad 8 \tau_{1,16} \tau_{3,5} l_{15}^2 - 8 \tau_{2,8} \tau_{3,5} l_{15}^2 - 8 \tau_{2,10} \tau_{3,7} l_{15}^2 - 4 \tau_{3,7} \tau_{3,10} l_{15}^2 + 8 \tau_{1,16} \tau_{3,13} l_{15}^2 - 8 \tau_{2,10} \tau_{4,7} l_{15}^2 - 8 \tau_{2,17} \tau_{4,7} l_{15}^2 + \\
& \quad 4 \tau_{3,10} \tau_{4,7} l_{15}^2 - 8 \tau_{2,10} \tau_{4,16} l_{15}^2 - 8 \tau_{2,17} \tau_{4,16} l_{15}^2 + 8 \tau_{2,10} \tau_{4,17} l_{15}^2 + 8 \tau_{2,17} \tau_{4,17} l_{15}^2 + 12 \tau_{3,7} \tau_{4,17} l_{15}^2 - \\
& \quad 4 \tau_{3,10} \tau_{4,17} l_{15}^2 - 4 \tau_{3,16} \tau_{4,17} l_{15}^2 - 4 \tau_{4,7} \tau_{4,17} l_{15}^2 - 4 \tau_{4,16} \tau_{4,17} l_{15}^2 + 2 \tau_{2,5} \tau_{2,8} l_{16}^2 - \tau_{1,14} \tau_{2,13} l_{16}^2 + \tau_{2,13} \tau_{2,14} l_{16}^2 + \\
& \quad 2 \tau_{1,15} \tau_{3,5} l_{16}^2 + 4 \tau_{2,8} \tau_{3,5} l_{16}^2 + 4 \tau_{2,10} \tau_{3,7} l_{16}^2 + 2 \tau_{2,14} \tau_{3,7} l_{16}^2 + 2 \tau_{3,7} \tau_{3,10} l_{16}^2 - 2 \tau_{1,15} \tau_{3,13} l_{16}^2 + 2 \tau_{2,14} \tau_{3,13} l_{16}^2 + \\
& \quad 2 \tau_{1,9} \tau_{3,14} l_{16}^2 + 2 \tau_{1,17} \tau_{3,14} l_{16}^2 + 2 \tau_{2,8} \tau_{3,14} l_{16}^2 - 2 \tau_{2,17} \tau_{3,14} l_{16}^2 - \tau_{1,14} \tau_{3,17} l_{16}^2 - \tau_{3,14} \tau_{3,17} l_{16}^2 + 4 \tau_{1,11} \tau_{4,6} l_{16}^2 + \\
& \quad 2 \tau_{2,14} \tau_{4,6} l_{16}^2 - \tau_{2,13} \tau_{4,7} l_{16}^2 - 2 \tau_{3,10} \tau_{4,7} l_{16}^2 - 2 \tau_{3,12} \tau_{4,9} l_{16}^2 + \tau_{3,17} \tau_{4,9} l_{16}^2 + 4 \tau_{1,9} \tau_{4,12} l_{16}^2 + 2 \tau_{1,15} \tau_{4,12} l_{16}^2 + \\
& \quad 2 \tau_{4,9} \tau_{4,12} l_{16}^2 + 2 \tau_{1,15} \tau_{4,13} l_{16}^2 - 2 \tau_{2,14} \tau_{4,13} l_{16}^2 + \tau_{2,13} \tau_{4,14} l_{16}^2 + \tau_{3,17} \tau_{4,14} l_{16}^2 + 2 \tau_{1,11} \tau_{4,15} l_{16}^2 - 2 \tau_{1,17} \tau_{4,15} l_{16}^2 + \\
& \quad 2 \tau_{2,10} \tau_{4,15} l_{16}^2 + 2 \tau_{2,17} \tau_{4,15} l_{16}^2 + \tau_{2,11} \tau_{4,17} l_{16}^2 - \tau_{2,15} \tau_{4,17} l_{16}^2 + \tau_{3,10} \tau_{4,17} l_{16}^2 + \tau_{3,15} \tau_{4,17} l_{16}^2 - \tau_{4,15} \tau_{4,17} l_{16}^2 - \\
& \quad 8 \tau_{3,14}^2 l_{17}^2 - 8 \tau_{4,15}^2 l_{17}^2 - 4 \tau_{2,5} \tau_{2,8} l_{17}^2 - 4 \tau_{1,14} \tau_{3,5} l_{17}^2 - 8 \tau_{2,8} \tau_{3,5} l_{17}^2 - 4 \tau_{1,14} \tau_{3,14} l_{17}^2 - 8 \tau_{2,8} \tau_{3,14} l_{17}^2 + \\
& \quad 8 \tau_{2,16} \tau_{3,14} l_{17}^2 - 8 \tau_{3,5} \tau_{3,14} l_{17}^2 + 4 \tau_{1,14} \tau_{3,16} l_{17}^2 + 8 \tau_{3,14} \tau_{3,16} l_{17}^2 - 8 \tau_{1,11} \tau_{4,6} l_{17}^2 + 4 \tau_{2,11} \tau_{4,6} l_{17}^2 - 4 \tau_{2,15} \tau_{4,6} l_{17}^2 - \\
& \quad 8 \tau_{1,11} \tau_{4,15} l_{17}^2 + 8 \tau_{1,16} \tau_{4,15} l_{17}^2 + 4 \tau_{2,11} \tau_{4,15} l_{17}^2 - 4 \tau_{2,15} \tau_{4,15} l_{17}^2 - 8 \tau_{4,6} \tau_{4,15} l_{17}^2 - 4 \tau_{2,11} \tau_{4,16} l_{17}^2 + 4 \tau_{2,15} \tau_{4,16} l_{17}^2 + \\
& \quad 8 \tau_{4,15} \tau_{4,16} l_{17}^2 - \tau_{1,6} (2 \tau_{1,10} \tau_{5,8} + 2 \tau_{2,10} \tau_{5,8} - 4 \tau_{1,11} \tau_{6,11} + 4 \tau_{2,11} \tau_{6,11} + 4 \tau_{1,11} l_{14}^2 - 4 \tau_{2,11} l_{14}^2 - 4 \tau_{2,13} l_{14}^2 - \\
& \quad 2 \tau_{1,11} l_{16}^2 + 2 \tau_{2,11} l_{16}^2 + \tau_{2,13} l_{16}^2 + 4 \tau_{1,11} l_{17}^2 - 4 \tau_{2,11} l_{17}^2) + \tau_{1,8} (4 \tau_{4,12} \tau_{6,11} + 4 \tau_{1,13} l_{15}^2 - 8 \tau_{3,5} l_{15}^2 + \\
& \quad 8 \tau_{3,13} l_{15}^2 + \tau_{3,17} l_{16}^2 - 2 \tau_{2,5} (2 \tau_{5,8} - 2 l_{15}^2 + l_{16}^2 - 2 l_{17}^2) + 4 \tau_{3,5} l_{17}^2 + 4 \tau_{3,14} l_{17}^2 - 4 \tau_{3,16} l_{17}^2)) t +
\end{aligned}$$

$$\begin{aligned}
& (s^2 - t^2 - u^2) \left( -2 \tau_{1,11} \tau_{2,11} \tau_{1,6}^2 - (-\tau_{3,6} \tau_{1,10}^2 + (\tau_{2,5} \tau_{2,8} + \tau_{3,5} \tau_{2,8} - \tau_{2,10} \tau_{3,6}) \tau_{1,10} + \tau_{1,9} \tau_{1,11} \tau_{2,5} + \right. \\
& \quad \tau_{1,11} \tau_{2,5} \tau_{2,9} + \tau_{2,5} \tau_{2,8} \tau_{2,10} + \tau_{2,8} \tau_{2,10} \tau_{3,5} + \tau_{1,11} \tau_{2,9} \tau_{4,5} - \tau_{2,9} \tau_{2,11} \tau_{4,5} - 2 \tau_{1,11}^2 \tau_{4,6} + \\
& \quad 2 \tau_{1,11} \tau_{2,11} \tau_{4,6} - \tau_{1,11} \tau_{2,12} \tau_{4,8} - \tau_{1,8} \tau_{1,11} \tau_{4,12} + \tau_{1,8} \tau_{2,11} \tau_{4,12} - \tau_{1,11} \tau_{4,8} \tau_{4,12} + \tau_{2,11} \tau_{4,8} \tau_{4,12}) \tau_{1,6} + \\
& \quad \tau_{2,8}^2 \tau_{2,12}^2 + 2 \tau_{2,8}^2 \tau_{3,5}^2 + 2 \tau_{1,10}^2 \tau_{3,6}^2 + 2 \tau_{2,10}^2 \tau_{3,7}^2 + \tau_{2,11}^2 \tau_{3,7}^2 + \tau_{3,7}^2 \tau_{3,11}^2 + \tau_{2,8}^2 \tau_{3,12}^2 + \\
& \quad 2 \tau_{2,9}^2 \tau_{4,5}^2 + 2 \tau_{1,11}^2 \tau_{4,6}^2 + \tau_{1,11}^2 \tau_{4,7}^2 + \tau_{1,8}^2 \tau_{4,12}^2 + 2 \tau_{1,9}^2 \tau_{4,12}^2 + \tau_{4,8}^2 \tau_{4,12}^2 + 2 \tau_{1,8} \tau_{4,8} \tau_{4,12}^2 + \\
& \quad 2 \tau_{1,9} \tau_{4,9} \tau_{4,12}^2 - 2 \tau_{1,8} \tau_{2,5}^2 \tau_{2,8} + 2 \tau_{2,5} \tau_{2,8}^2 \tau_{3,5} - 2 \tau_{1,8} \tau_{2,5} \tau_{2,8} \tau_{3,5} + \tau_{1,8} \tau_{1,10} \tau_{2,5} \tau_{3,6} - \tau_{1,10} \tau_{2,5} \tau_{2,8} \tau_{3,6} - \\
& \quad 2 \tau_{1,10} \tau_{2,8} \tau_{3,5} \tau_{3,6} - \tau_{1,8} \tau_{2,5} \tau_{2,11} \tau_{3,7} + \tau_{2,5} \tau_{2,8} \tau_{2,11} \tau_{3,7} + 2 \tau_{2,8} \tau_{2,10} \tau_{2,12} \tau_{3,7} + 2 \tau_{2,8} \tau_{2,11} \tau_{3,5} \tau_{3,7} + \\
& \quad \tau_{1,10} \tau_{3,6}^2 \tau_{3,10} + 2 \tau_{2,10} \tau_{3,7}^2 \tau_{3,10} + \tau_{2,8} \tau_{2,12} \tau_{3,7} \tau_{3,10} + 2 \tau_{2,11} \tau_{3,7}^2 \tau_{3,11} - \tau_{1,8} \tau_{2,5} \tau_{3,7} \tau_{3,11} + \tau_{2,5} \tau_{2,8} \tau_{3,7} \tau_{3,11} + \\
& \quad 2 \tau_{2,8} \tau_{3,5} \tau_{3,7} \tau_{3,11} + \tau_{1,7}^2 \tau_{1,11} (\tau_{1,11} + \tau_{3,11}) + 2 \tau_{2,8}^2 \tau_{2,12} \tau_{3,12} + 2 \tau_{2,8} \tau_{2,10} \tau_{3,7} \tau_{3,12} + \tau_{2,8} \tau_{3,7} \tau_{3,10} \tau_{3,12} + \\
& \quad \tau_{2,5} \tau_{2,9}^2 \tau_{4,5} + \tau_{1,9} \tau_{2,5} \tau_{2,9} \tau_{4,5} - 2 \tau_{2,9} \tau_{2,10} \tau_{3,7} \tau_{4,5} - \tau_{2,9} \tau_{3,7} \tau_{3,10} \tau_{4,5} - \tau_{1,9} \tau_{1,11} \tau_{2,5} \tau_{4,6} - \tau_{1,11} \tau_{2,5} \tau_{2,9} \tau_{4,6} + \\
& \quad \tau_{1,10} \tau_{3,6} \tau_{3,10} \tau_{4,6} - 2 \tau_{1,11} \tau_{2,9} \tau_{4,5} \tau_{4,6} - 2 \tau_{3,7} \tau_{3,10}^2 \tau_{4,7} - \tau_{2,8} \tau_{2,12} \tau_{3,10} \tau_{4,7} - 2 \tau_{2,10} \tau_{3,7} \tau_{3,10} \tau_{4,7} - \\
& \quad \tau_{2,8} \tau_{3,10} \tau_{3,12} \tau_{4,7} + \tau_{2,9} \tau_{3,10} \tau_{4,5} \tau_{4,7} + \tau_{2,8} \tau_{2,12}^2 \tau_{4,8} + \tau_{2,10} \tau_{2,12} \tau_{3,7} \tau_{4,8} + \tau_{2,12} \tau_{3,7} \tau_{3,10} \tau_{4,8} + \tau_{2,8} \tau_{2,12} \tau_{3,12} \tau_{4,8} + \\
& \quad \tau_{1,11} \tau_{2,12} \tau_{4,6} \tau_{4,8} + \tau_{2,9} \tau_{4,5}^2 \tau_{4,9} - \tau_{2,10} \tau_{3,5} \tau_{3,7} \tau_{4,9} - \tau_{3,5} \tau_{3,7} \tau_{3,10} \tau_{4,9} + \tau_{1,10} \tau_{3,6} \tau_{3,12} \tau_{4,9} + \tau_{2,9} \tau_{3,5} \tau_{4,5} \tau_{4,9} - \\
& \quad \tau_{2,10} \tau_{3,7} \tau_{4,5} \tau_{4,9} - \tau_{3,7} \tau_{3,10} \tau_{4,5} \tau_{4,9} - \tau_{1,11} \tau_{3,12} \tau_{4,7} \tau_{4,9} + \tau_{2,12} \tau_{4,8}^2 \tau_{4,12} - 2 \tau_{3,12} \tau_{4,9}^2 \tau_{4,12} - 2 \tau_{1,9} \tau_{1,10} \tau_{3,6} \tau_{4,12} - \\
& \quad \tau_{1,9} \tau_{3,6} \tau_{3,10} \tau_{4,12} + 2 \tau_{1,8} \tau_{1,11} \tau_{4,6} \tau_{4,12} - \tau_{1,9} \tau_{3,10} \tau_{4,6} \tau_{4,12} + 2 \tau_{1,9} \tau_{1,11} \tau_{4,7} \tau_{4,12} + \tau_{1,8} \tau_{2,12} \tau_{4,8} \tau_{4,12} + \\
& \quad 2 \tau_{1,11} \tau_{4,6} \tau_{4,8} \tau_{4,12} - \tau_{1,10} \tau_{3,6} \tau_{4,9} \tau_{4,12} - \tau_{3,6} \tau_{3,10} \tau_{4,9} \tau_{4,12} - 2 \tau_{1,9} \tau_{3,12} \tau_{4,9} \tau_{4,12} - \tau_{3,10} \tau_{4,6} \tau_{4,9} \tau_{4,12} + \\
& \quad \tau_{1,11} \tau_{4,7} \tau_{4,9} \tau_{4,12} + \tau_{1,7} (2 \tau_{4,7} \tau_{1,11}^2 + \tau_{3,11} \tau_{4,7} \tau_{1,11} - \tau_{3,12} \tau_{4,9} \tau_{1,11} + 2 \tau_{1,9} \tau_{4,12} \tau_{1,11} + \tau_{4,9} \tau_{4,12} \tau_{1,11} + \\
& \quad \tau_{3,7} \tau_{3,11}^2 + \tau_{2,5} \tau_{2,8} \tau_{3,11} + \tau_{2,8} \tau_{3,5} \tau_{3,11} + \tau_{2,11} \tau_{3,7} \tau_{3,11} + \tau_{1,9} \tau_{3,11} \tau_{4,12} + \tau_{3,11} \tau_{4,9} \tau_{4,12})) + \\
& u^2 (2 \tau_{1,6}^2 \tau_{1,11}^2 + \tau_{1,7}^2 \tau_{1,11}^2 + 2 \tau_{4,6}^2 \tau_{1,11}^2 + \tau_{4,7}^2 \tau_{1,11}^2 - 2 \tau_{2,9} \tau_{4,5} \tau_{4,6} \tau_{1,11} + 2 \tau_{1,8} \tau_{4,6} \tau_{4,12} \tau_{1,11} + \\
& \quad 2 \tau_{1,9} \tau_{4,7} \tau_{4,12} \tau_{1,11} + 2 \tau_{4,6} \tau_{4,8} \tau_{4,12} \tau_{1,11} + 2 \tau_{4,7} \tau_{4,9} \tau_{4,12} \tau_{1,11} + \\
& \quad 2 \tau_{1,6} (-\tau_{2,9} \tau_{4,5} + 2 \tau_{1,11} \tau_{4,6} + (\tau_{1,8} + \tau_{4,8}) \tau_{4,12}) \tau_{1,11} + 2 \tau_{1,7} (\tau_{1,11} \tau_{4,7} + (\tau_{1,9} + \tau_{4,9}) \tau_{4,12}) \tau_{1,11} + \\
& \quad 2 \tau_{2,5}^2 \tau_{2,8}^2 + \tau_{2,8}^2 \tau_{2,12}^2 + 2 \tau_{2,8}^2 \tau_{3,5}^2 + 2 \tau_{1,10}^2 \tau_{3,6}^2 + 2 \tau_{2,10}^2 \tau_{3,7}^2 + \tau_{2,11}^2 \tau_{3,7}^2 + 2 \tau_{3,7}^2 \tau_{3,10}^2 + \\
& \quad \tau_{3,7}^2 \tau_{3,11}^2 + \tau_{2,8}^2 \tau_{3,12}^2 + 2 \tau_{2,9}^2 \tau_{4,5}^2 + \tau_{1,8}^2 \tau_{4,12}^2 + 2 \tau_{1,9}^2 \tau_{4,12}^2 + \tau_{4,8}^2 \tau_{4,12}^2 + 2 \tau_{4,9}^2 \tau_{4,12}^2 + \\
& \quad 2 \tau_{1,8} \tau_{4,8} \tau_{4,12}^2 + 4 \tau_{1,9} \tau_{4,9} \tau_{4,12}^2 + 4 \tau_{2,5} \tau_{2,8}^2 \tau_{3,5} - 2 \tau_{1,10} \tau_{2,5} \tau_{2,8} \tau_{3,6} - 2 \tau_{1,10} \tau_{2,8} \tau_{3,5} \tau_{3,6} + \\
& \quad 2 \tau_{2,5} \tau_{2,8} \tau_{2,11} \tau_{3,7} + 2 \tau_{2,8} \tau_{2,10} \tau_{2,12} \tau_{3,7} + 2 \tau_{2,8} \tau_{2,11} \tau_{3,5} \tau_{3,7} + 4 \tau_{2,10} \tau_{3,7}^2 \tau_{3,10} + 2 \tau_{2,8} \tau_{2,12} \tau_{3,7} \tau_{3,10} + \\
& \quad 2 \tau_{2,11} \tau_{3,7}^2 \tau_{3,11} + 2 \tau_{2,5} \tau_{2,8} \tau_{3,7} \tau_{3,11} + 2 \tau_{2,8} \tau_{3,5} \tau_{3,7} \tau_{3,11} + 2 \tau_{2,8}^2 \tau_{2,12} \tau_{3,12} + 2 \tau_{2,8} \tau_{2,10} \tau_{3,7} \tau_{3,12} + \\
& \quad 2 \tau_{2,8} \tau_{3,7} \tau_{3,10} \tau_{3,12} - 2 \tau_{2,9} \tau_{2,10} \tau_{3,7} \tau_{4,5} - 2 \tau_{2,9} \tau_{3,7} \tau_{3,10} \tau_{4,5} - 2 \tau_{1,9} \tau_{1,10} \tau_{3,6} \tau_{4,12} - 2 \tau_{1,10} \tau_{3,6} \tau_{4,9} \tau_{4,12}) + \\
& \frac{1}{2} u (-s^2 + t^2 + u^2) (-4 l_{13}^2 \tau_{1,15}^2 - 4 \tau_{1,9} l_{13}^2 \tau_{1,15} + 4 \tau_{1,16} l_{13}^2 \tau_{1,15} - 4 \tau_{4,9} l_{13}^2 \tau_{1,15} - 4 \tau_{4,12} l_{13}^2 \tau_{1,15} + \\
& \quad 4 \tau_{4,16} l_{13}^2 \tau_{1,15} + \tau_{1,13} l_{16}^2 \tau_{1,15} + \tau_{3,5} l_{16}^2 \tau_{1,15} - \tau_{3,13} l_{16}^2 \tau_{1,15} + \tau_{4,12} l_{16}^2 \tau_{1,15} + \tau_{4,13} l_{16}^2 \tau_{1,15} - 2 \tau_{1,10} \tau_{3,6} \tau_{5,8} + \\
& \quad 2 \tau_{2,11} \tau_{3,7} \tau_{5,8} + 2 \tau_{3,7} \tau_{3,11} \tau_{5,8} + 4 \tau_{1,6} \tau_{1,11} \tau_{6,11} - 2 \tau_{2,9} \tau_{4,5} \tau_{6,11} + 4 \tau_{1,11} \tau_{4,6} \tau_{6,11} + 2 \tau_{1,8} \tau_{4,12} \tau_{6,11} + \\
& \quad 2 \tau_{4,8} \tau_{4,12} \tau_{6,11} + 4 \tau_{2,10} \tau_{3,7} \tau_{7,10} + 4 \tau_{3,7} \tau_{3,10} \tau_{7,10} - 2 \tau_{2,9} \tau_{4,5} \tau_{7,10} + 2 \tau_{1,7} \tau_{1,11} \tau_{9,12} - 2 \tau_{1,10} \tau_{3,6} \tau_{9,12} + \\
& \quad 2 \tau_{1,11} \tau_{4,7} \tau_{9,12} + 4 \tau_{1,9} \tau_{4,12} \tau_{9,12} + 4 \tau_{4,9} \tau_{4,12} \tau_{9,12} - 4 \tau_{2,14}^2 l_{13}^2 - 4 \tau_{2,10} \tau_{2,14} l_{13}^2 + 4 \tau_{2,14} \tau_{2,16} l_{13}^2 - \\
& \quad 4 \tau_{2,10} \tau_{3,7} l_{13}^2 - 4 \tau_{2,14} \tau_{3,7} l_{13}^2 - 4 \tau_{2,14} \tau_{3,10} l_{13}^2 - 4 \tau_{3,7} \tau_{3,10} l_{13}^2 + 4 \tau_{2,14} \tau_{3,16} l_{13}^2 - 4 \tau_{1,9} \tau_{4,12} l_{13}^2 - \\
& \quad 4 \tau_{4,9} \tau_{4,12} l_{13}^2 - 4 \tau_{1,6} \tau_{1,11} l_{14}^2 - 8 \tau_{1,11} \tau_{2,13} l_{14}^2 - 4 \tau_{1,9} \tau_{3,12} l_{14}^2 - 4 \tau_{1,17} \tau_{3,12} l_{14}^2 - 4 \tau_{1,9} \tau_{3,16} l_{14}^2 -
\end{aligned}$$



$$\begin{aligned}
& 4 \tau_{1,17} \tau_{3,16} l_{14}^2 + 4 \tau_{1,9} \tau_{3,17} l_{14}^2 + 4 \tau_{1,17} \tau_{3,17} l_{14}^2 - 4 \tau_{1,11} \tau_{4,6} l_{14}^2 - 4 \tau_{2,11} \tau_{4,6} l_{14}^2 - 4 \tau_{2,13} \tau_{4,6} l_{14}^2 - 4 \tau_{2,16} \tau_{4,6} l_{14}^2 - \\
& 4 \tau_{1,9} \tau_{4,12} l_{14}^2 + 8 \tau_{3,17} \tau_{4,12} l_{14}^2 - 4 \tau_{4,9} \tau_{4,12} l_{14}^2 + 4 \tau_{2,11} \tau_{4,13} l_{14}^2 + 4 \tau_{2,13} \tau_{4,13} l_{14}^2 + 4 \tau_{2,16} \tau_{4,13} l_{14}^2 - \\
& 4 \tau_{1,8} \tau_{3,5} l_{15}^2 - 4 \tau_{1,13} \tau_{3,5} l_{15}^2 - 4 \tau_{1,16} \tau_{3,5} l_{15}^2 - 4 \tau_{2,10} \tau_{3,7} l_{15}^2 - 4 \tau_{3,7} \tau_{3,10} l_{15}^2 + 4 \tau_{1,8} \tau_{3,13} l_{15}^2 + 4 \tau_{1,13} \tau_{3,13} l_{15}^2 + \\
& 4 \tau_{1,16} \tau_{3,13} l_{15}^2 - 4 \tau_{2,10} \tau_{4,7} l_{15}^2 - 4 \tau_{2,17} \tau_{4,7} l_{15}^2 - 4 \tau_{2,10} \tau_{4,16} l_{15}^2 - 4 \tau_{2,17} \tau_{4,16} l_{15}^2 + 4 \tau_{2,10} \tau_{4,17} l_{15}^2 + \\
& 4 \tau_{2,17} \tau_{4,17} l_{15}^2 + 8 \tau_{3,7} \tau_{4,17} l_{15}^2 + 2 \tau_{1,6} \tau_{1,11} l_{16}^2 + \tau_{2,13} \tau_{2,14} l_{16}^2 + 2 \tau_{2,10} \tau_{3,7} l_{16}^2 + \tau_{2,14} \tau_{3,7} l_{16}^2 + 2 \tau_{3,7} \tau_{3,10} l_{16}^2 + \\
& \tau_{2,14} \tau_{3,13} l_{16}^2 + \tau_{1,9} \tau_{3,14} l_{16}^2 + \tau_{1,17} \tau_{3,14} l_{16}^2 - \tau_{2,17} \tau_{3,14} l_{16}^2 - \tau_{3,14} \tau_{3,17} l_{16}^2 + 2 \tau_{1,11} \tau_{4,6} l_{16}^2 + \tau_{2,14} \tau_{4,6} l_{16}^2 + \\
& 2 \tau_{1,9} \tau_{4,12} l_{16}^2 + 2 \tau_{4,9} \tau_{4,12} l_{16}^2 - \tau_{2,14} \tau_{4,13} l_{16}^2 + \tau_{1,11} \tau_{4,15} l_{16}^2 - \tau_{1,17} \tau_{4,15} l_{16}^2 + \tau_{2,10} \tau_{4,15} l_{16}^2 + \tau_{2,17} \tau_{4,15} l_{16}^2 - \\
& \tau_{4,15} \tau_{4,17} l_{16}^2 - 4 \tau_{3,14}^2 l_{17}^2 - 4 \tau_{4,15}^2 l_{17}^2 - 4 \tau_{1,6} \tau_{1,11} l_{17}^2 + 4 \tau_{2,16} \tau_{3,14} l_{17}^2 - 4 \tau_{3,5} \tau_{3,14} l_{17}^2 + 4 \tau_{3,14} \tau_{3,16} l_{17}^2 - \\
& 4 \tau_{1,11} \tau_{4,6} l_{17}^2 - 4 \tau_{1,6} \tau_{4,15} l_{17}^2 - 4 \tau_{1,11} \tau_{4,15} l_{17}^2 + 4 \tau_{1,16} \tau_{4,15} l_{17}^2 - 4 \tau_{4,6} \tau_{4,15} l_{17}^2 + 4 \tau_{4,15} \tau_{4,16} l_{17}^2 + \\
& \tau_{2,8} (2 \tau_{2,12} \tau_{7,10} + 2 \tau_{3,12} \tau_{7,10} - 8 \tau_{1,13} l_{15}^2 + \tau_{3,14} l_{16}^2 + 2 \tau_{3,5} (2 \tau_{5,8} - 2 l_{15}^2 + l_{16}^2 - 2 l_{17}^2) - 4 \tau_{3,14} l_{17}^2) + \\
& 2 \tau_{2,5} (\tau_{2,8} (2 \tau_{5,8} - 2 l_{15}^2 + l_{16}^2 - 2 l_{17}^2) - 2 \tau_{3,14} l_{17}^2)) \Big)
\end{aligned}$$

■  $N_{50}^{(5)}$

0

■  $N_{50}^{(6)}$

0

■  $N_{50}^{(7)}$

0

■  $N_{50}^{(8)}$

0
